# Supplementary material for: An Assessment of Different Electronic Structure Approaches for Modeling Time-Resolved X-ray Absorption Spectroscopy
Source: arXiv:2101.06643 source file (2021-01-17)
Supplement: Supplementary file 1 [file mom_ccsd_SI.pdf]

# **An Assessment of Different Electronic Structure Approaches for Modeling Time-Resolved X-ray Absorption Spectroscopy: Supporting Information**

Shota Tsuru,<sup>\*,†,¶</sup> Marta L. Vidal,<sup>†</sup> Mátyás Pápai,<sup>†,§</sup> Anna I. Krylov,<sup>‡</sup> Klaus B.  
Møller,<sup>†</sup> and Sonia Coriani<sup>\*,†</sup>

<sup>†</sup>*DTU Chemistry, Technical University of Denmark, Kemitorvet Bldg 207, DK-2800, Kgs.  
Lyngby, Denmark*

<sup>‡</sup>*Department of Chemistry, University of Southern California, Los Angeles, California  
90089, United States*

<sup>¶</sup>*Current address: Arbeitsgruppe Quantenchemie, Ruhr-Universität Bochum, D-44780,  
Bochum, Germany*

<sup>§</sup>*Current address: Wigner Research Centre for Physics, Hungarian Academy of Sciences,  
P.O. Box 49, H-1525 Budapest, Hungary*

E-mail: Shota.Tsuru@ruhr-uni-bochum.de; soco@kemi.dtu.dk

# S1 Natural transition orbitals of core excitations from the ground state

Table S1: Uracil. CVS-EOM-CCSD/6-311++G\*\* energies, strengths and NTOs of the  $O_{1s}$  core excitations from the ground state at the FC geometry (NTO isosurface is 0.04 for the Rydberg transition and 0.05 for the others).

| Final state | Ex. energy (eV) | Osc. strength | Hole                                                                                 | $\sigma_K^2$ | Particle                                                                             |
|-------------|-----------------|---------------|--------------------------------------------------------------------------------------|--------------|--------------------------------------------------------------------------------------|
| 1A''        | 533.17          | 0.0367        | 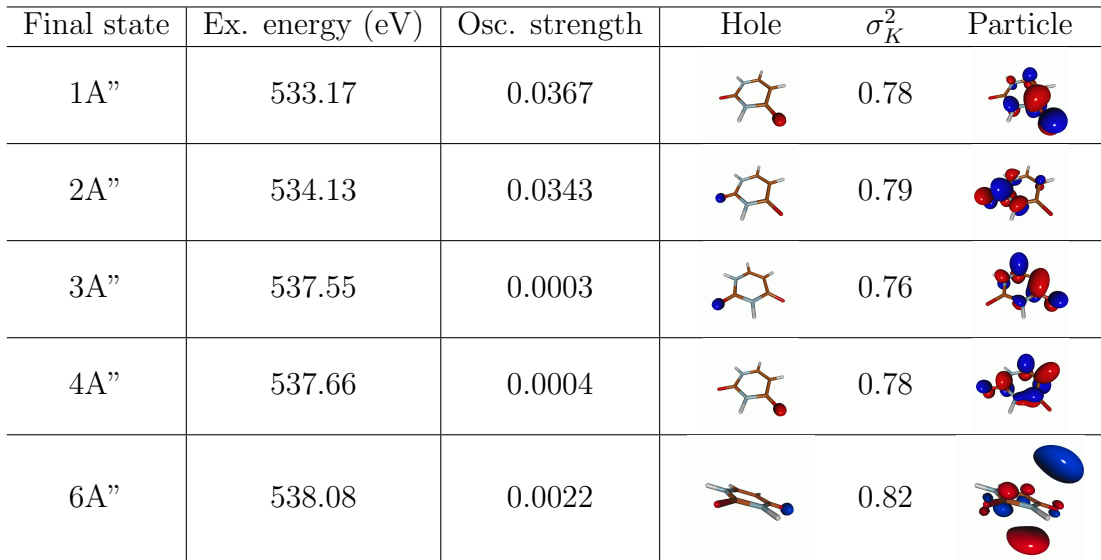   | 0.78         | 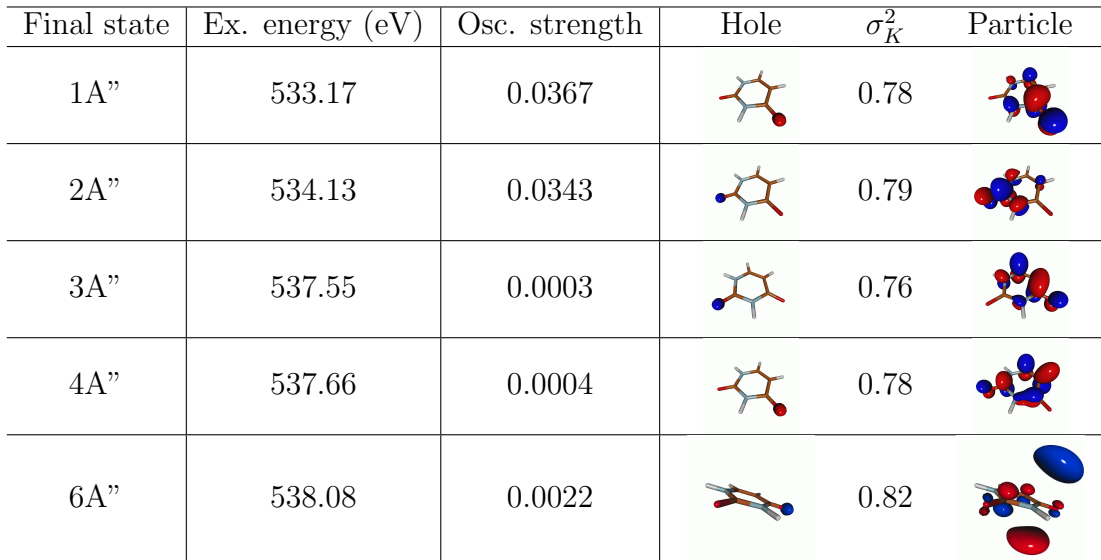  |
| 2A''        | 534.13          | 0.0343        | 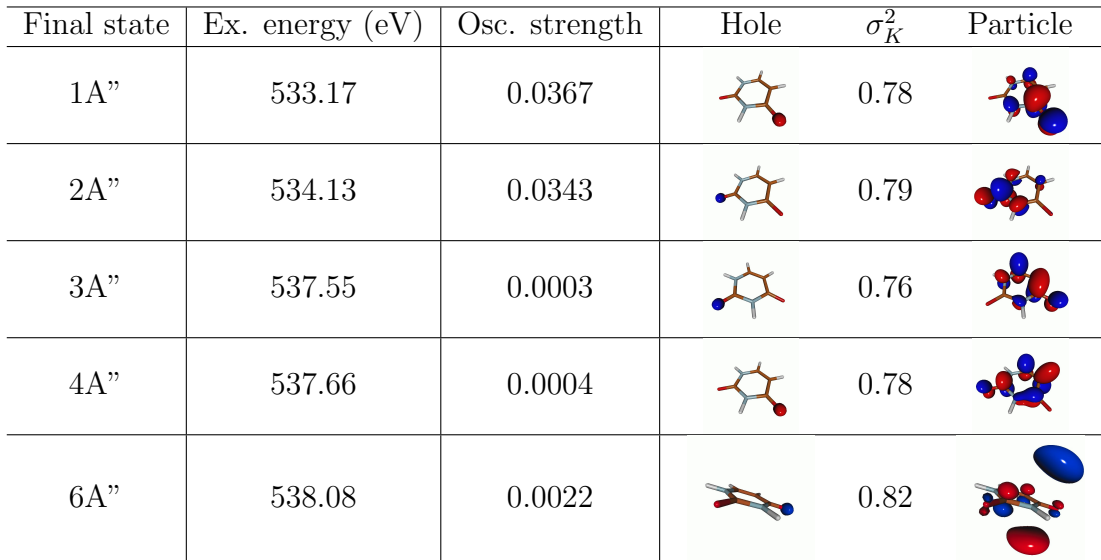   | 0.79         | 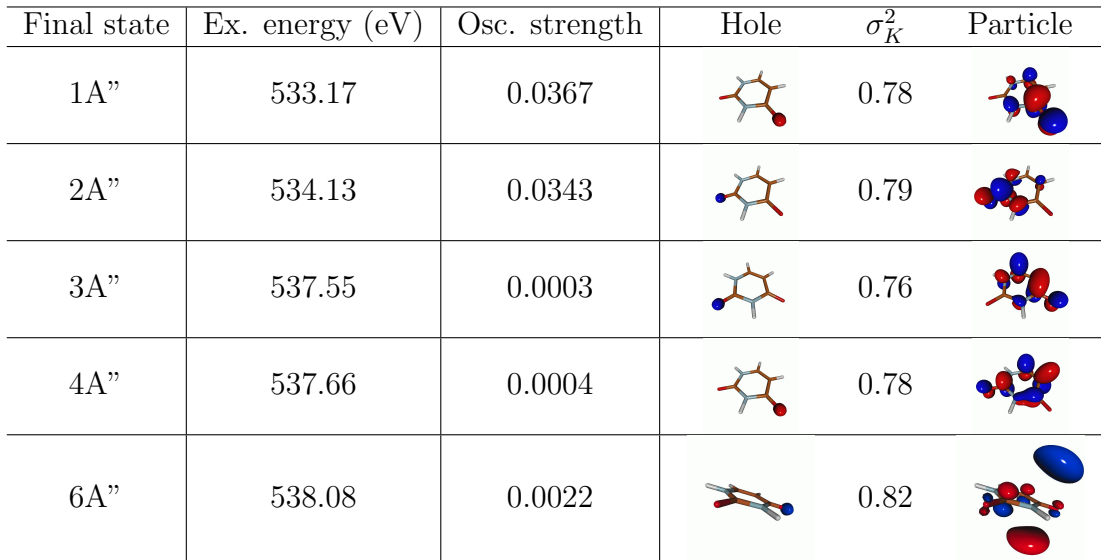  |
| 3A''        | 537.55          | 0.0003        | 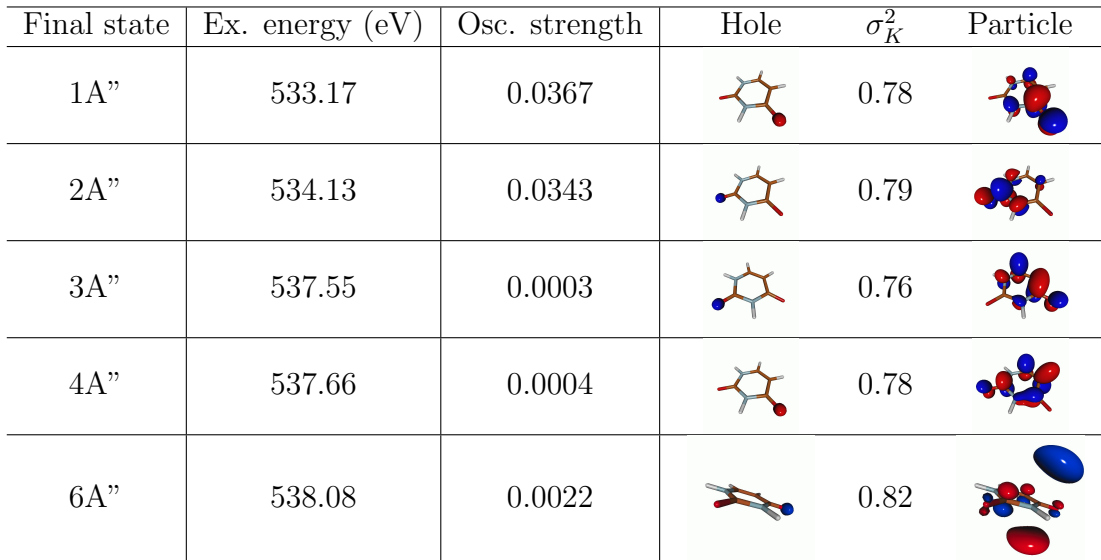   | 0.76         | 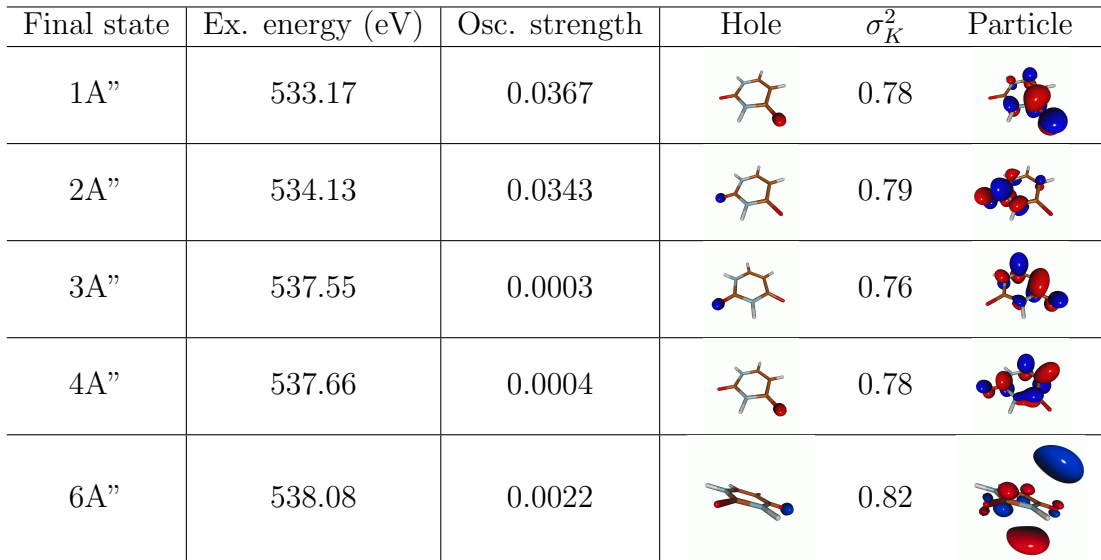  |
| 4A''        | 537.66          | 0.0004        | 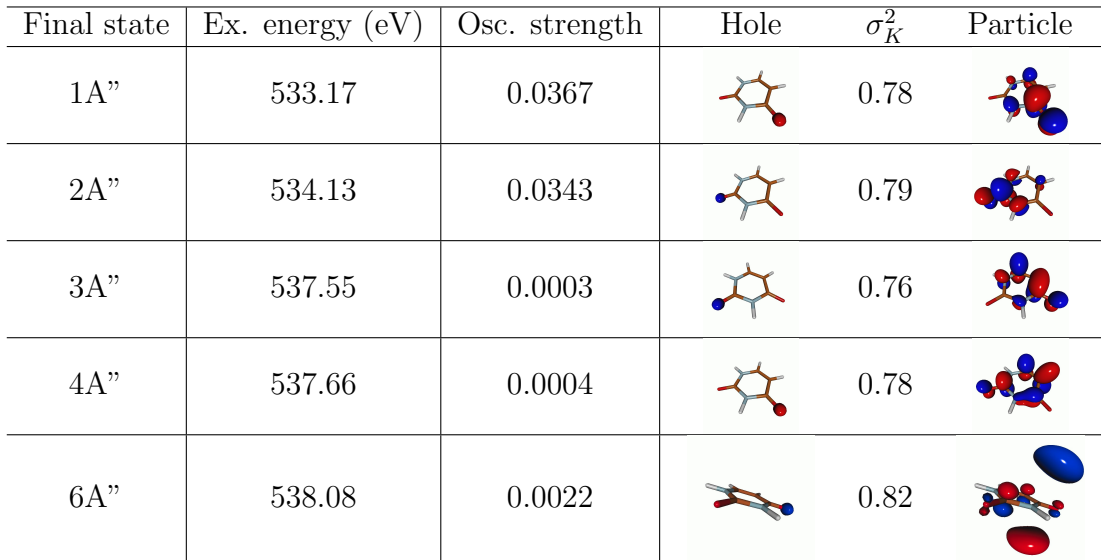   | 0.78         | 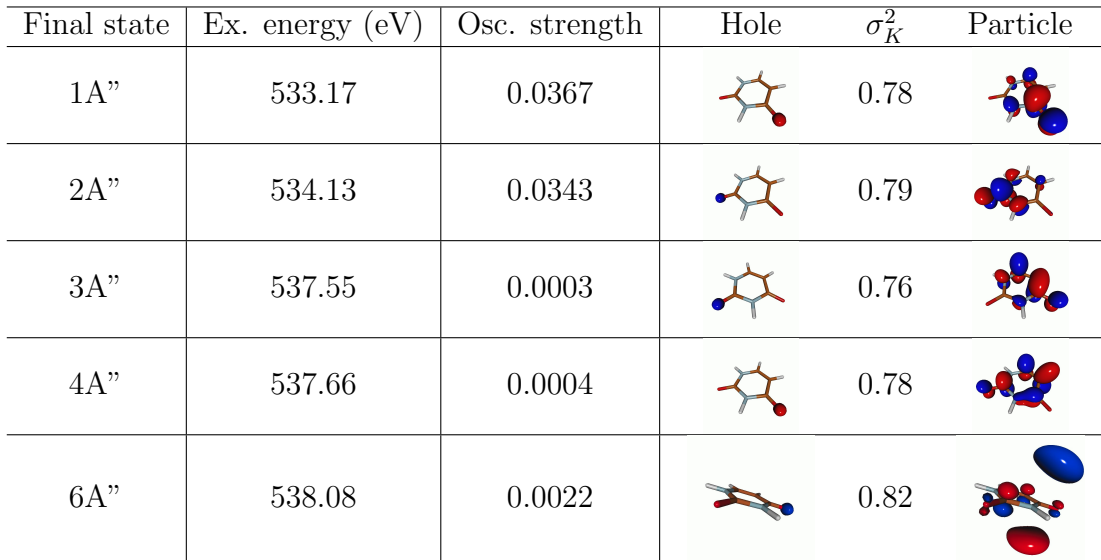  |
| 6A''        | 538.08          | 0.0022        | 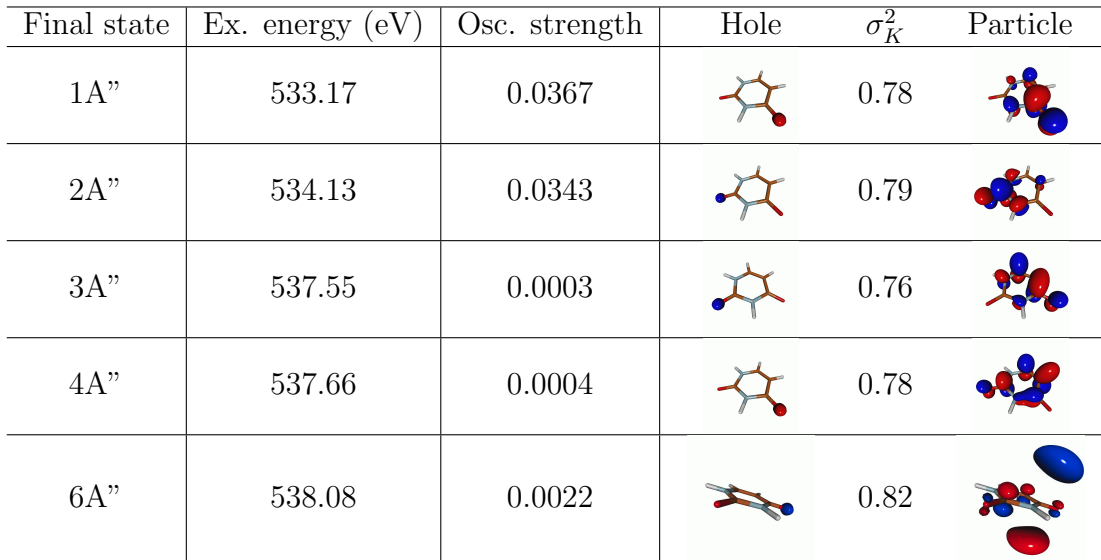 | 0.82         | 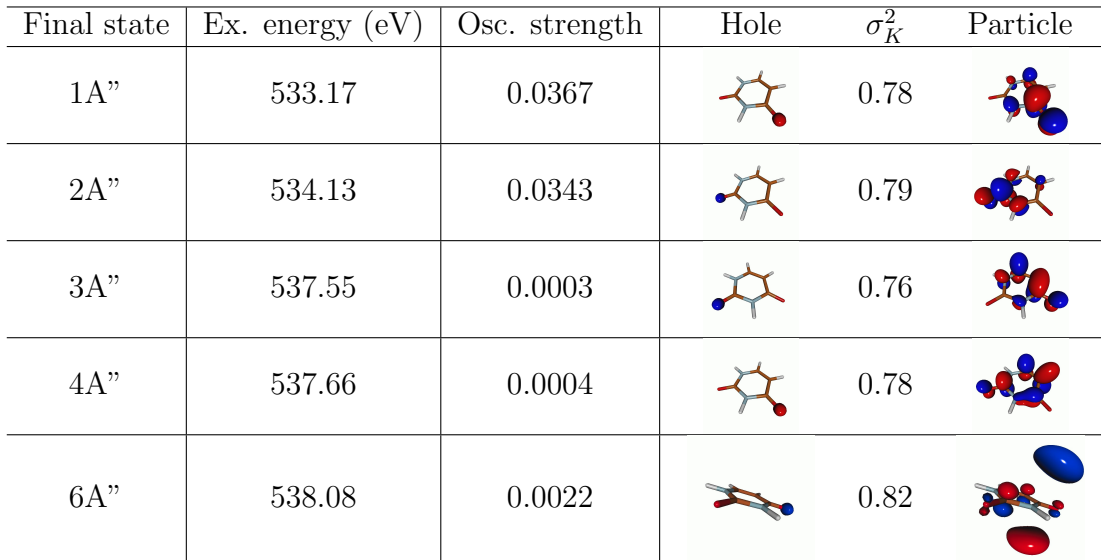 |

Table S2: Uracil. CVS-ADC(2)/6-311++G\*\* energies, strengths and NTOs of the  $O_{1s}$  core excitations from the ground state at the FC geometry (NTO isosurface is 0.04 for the Rydberg transition and 0.05 for the others).

| Final state | Ex. energy (eV) | Osc. strength | Hole                                                                                | $\sigma_K^2$ | Particle                                                                             |
|-------------|-----------------|---------------|-------------------------------------------------------------------------------------|--------------|--------------------------------------------------------------------------------------|
| 1A''        | 533.22          | 0.0243        | 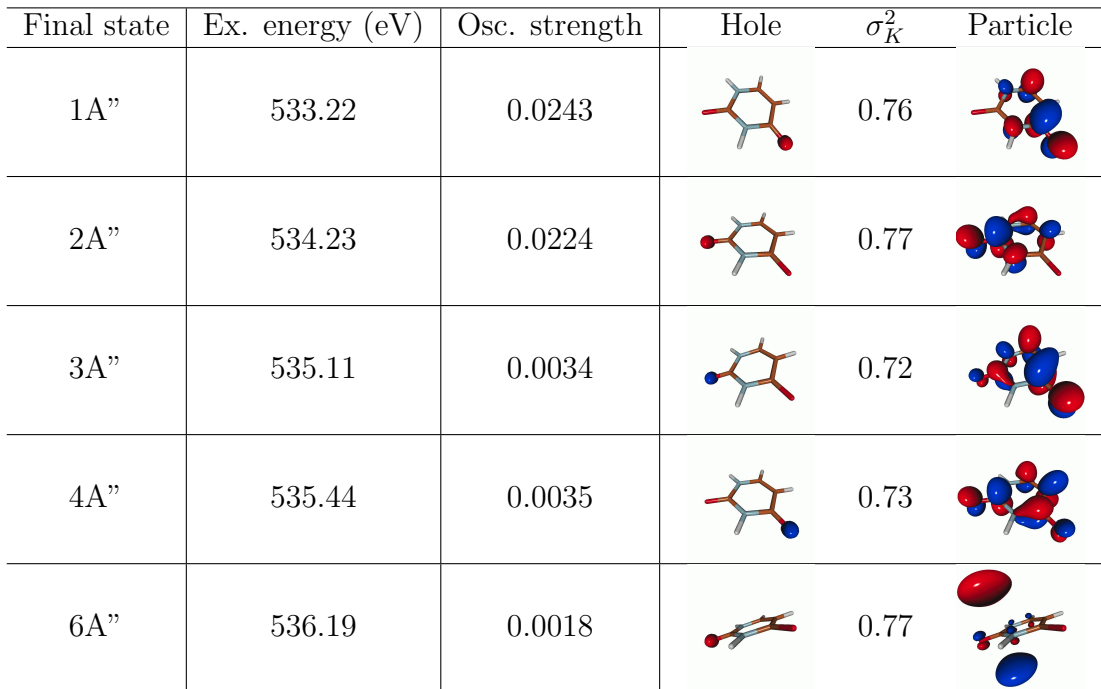  | 0.76         | 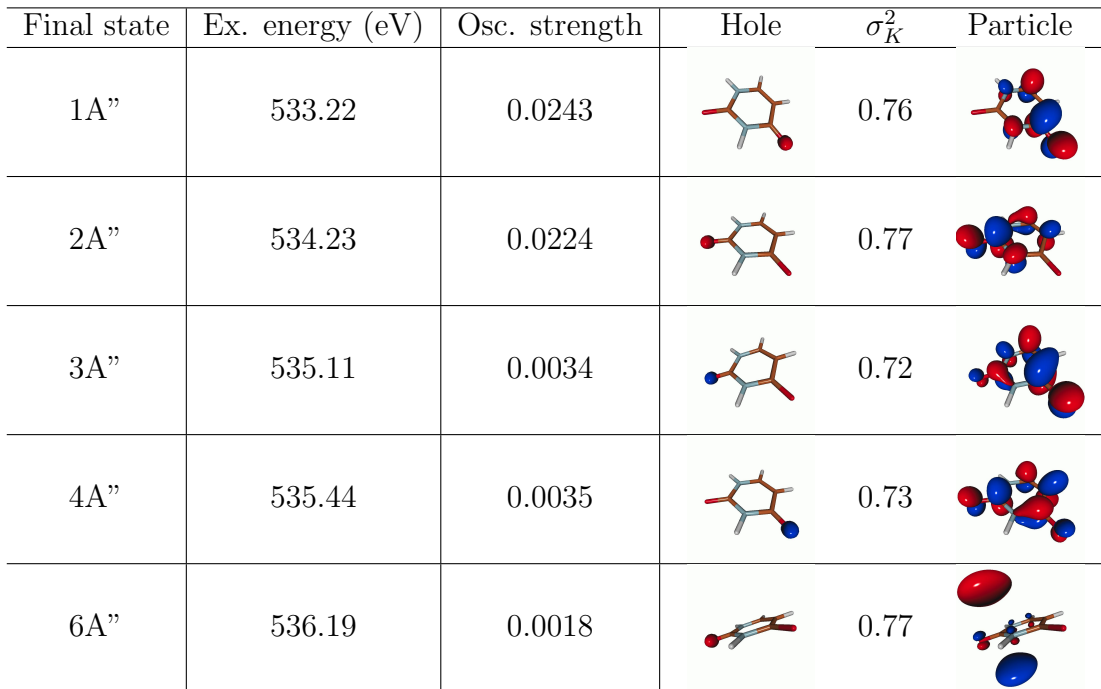  |
| 2A''        | 534.23          | 0.0224        | 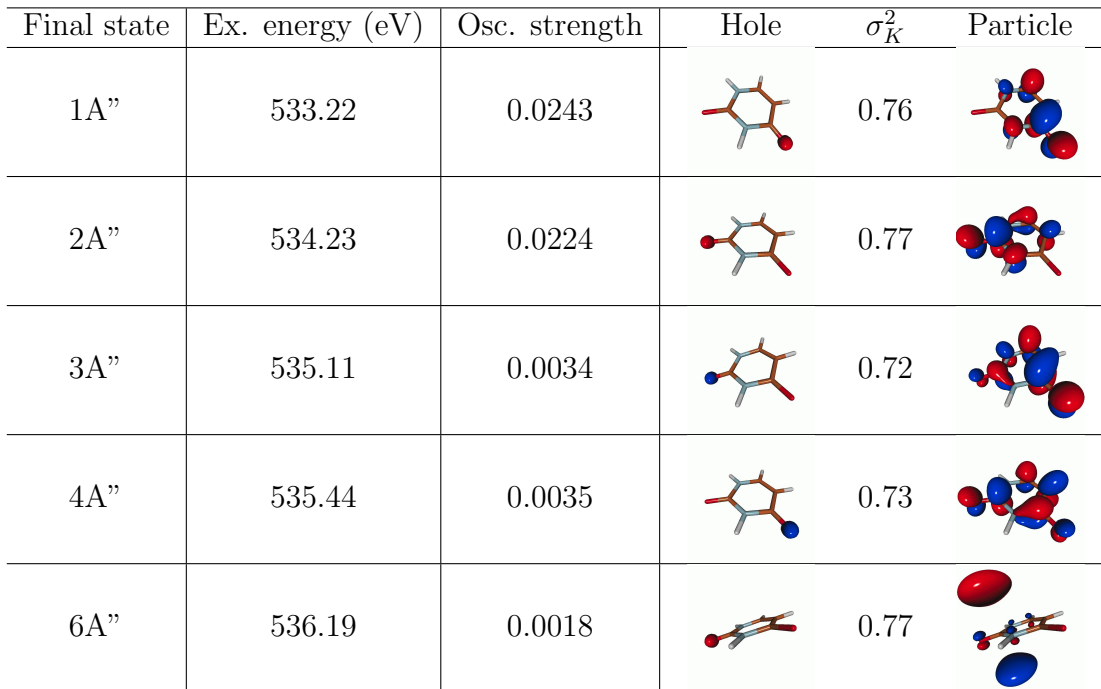  | 0.77         | 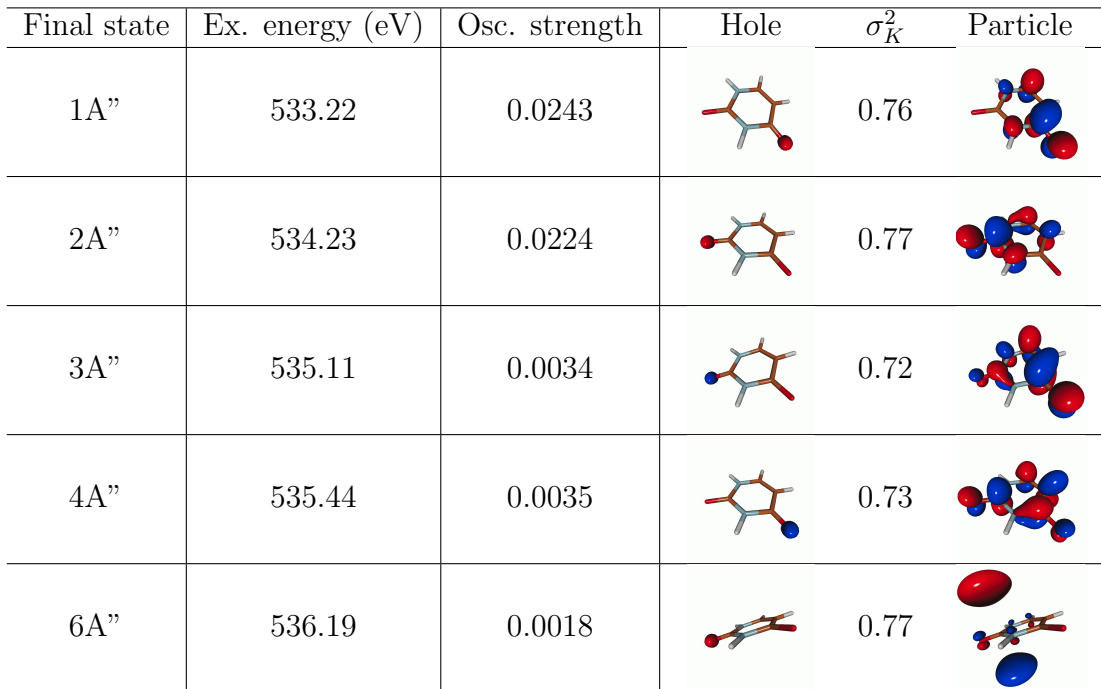  |
| 3A''        | 535.11          | 0.0034        | 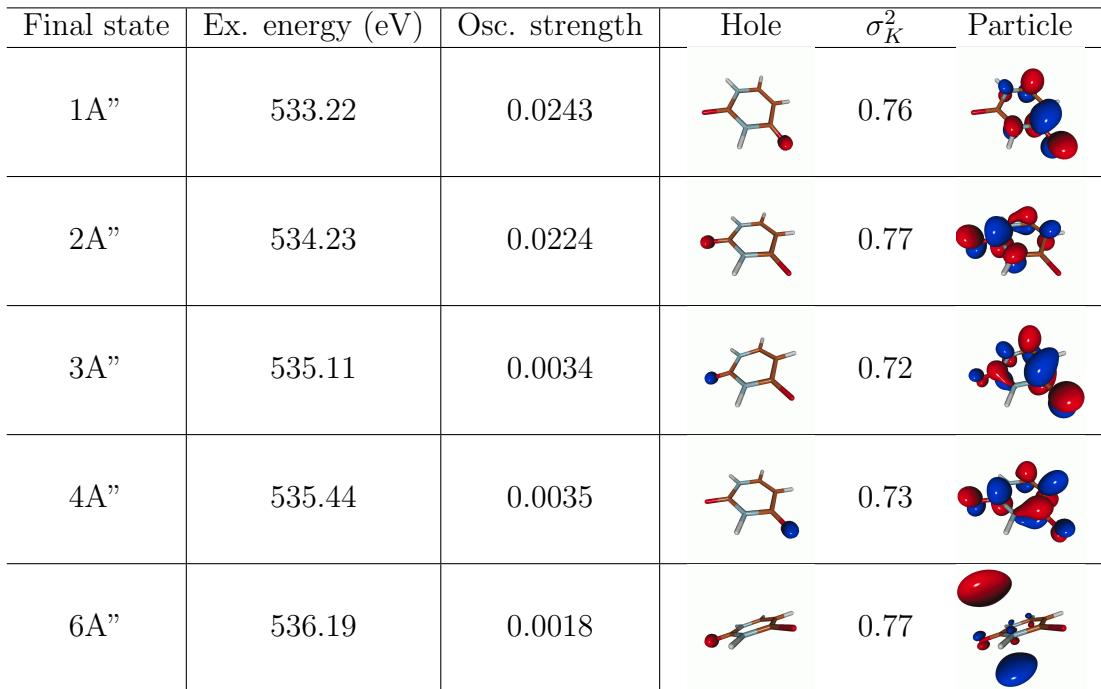  | 0.72         | 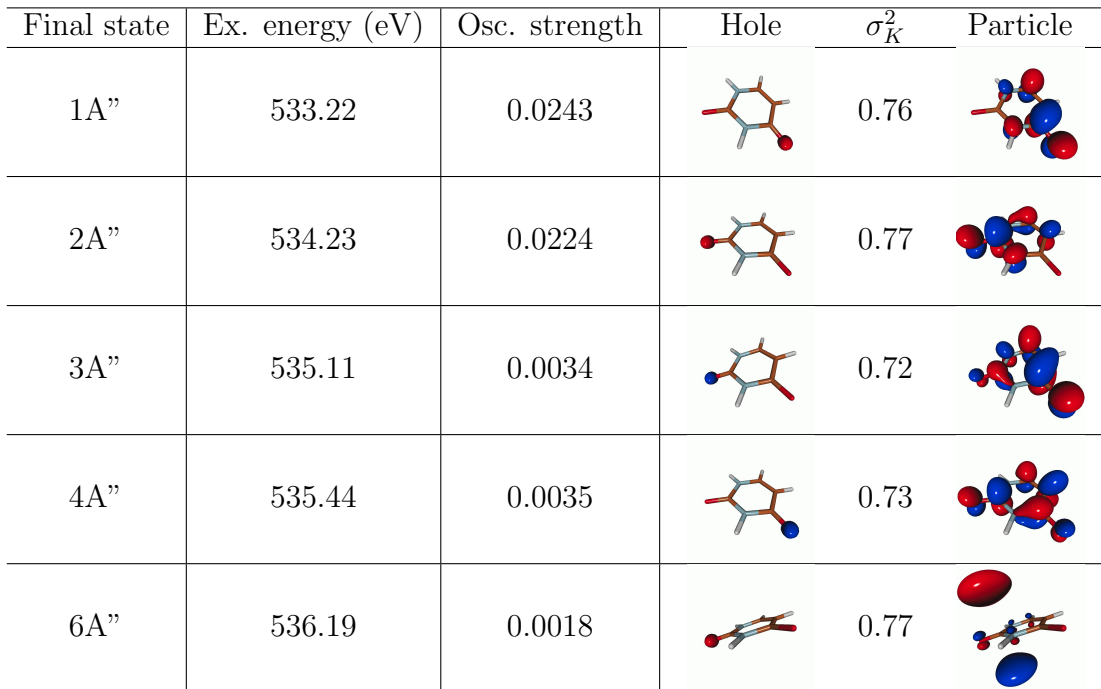  |
| 4A''        | 535.44          | 0.0035        | 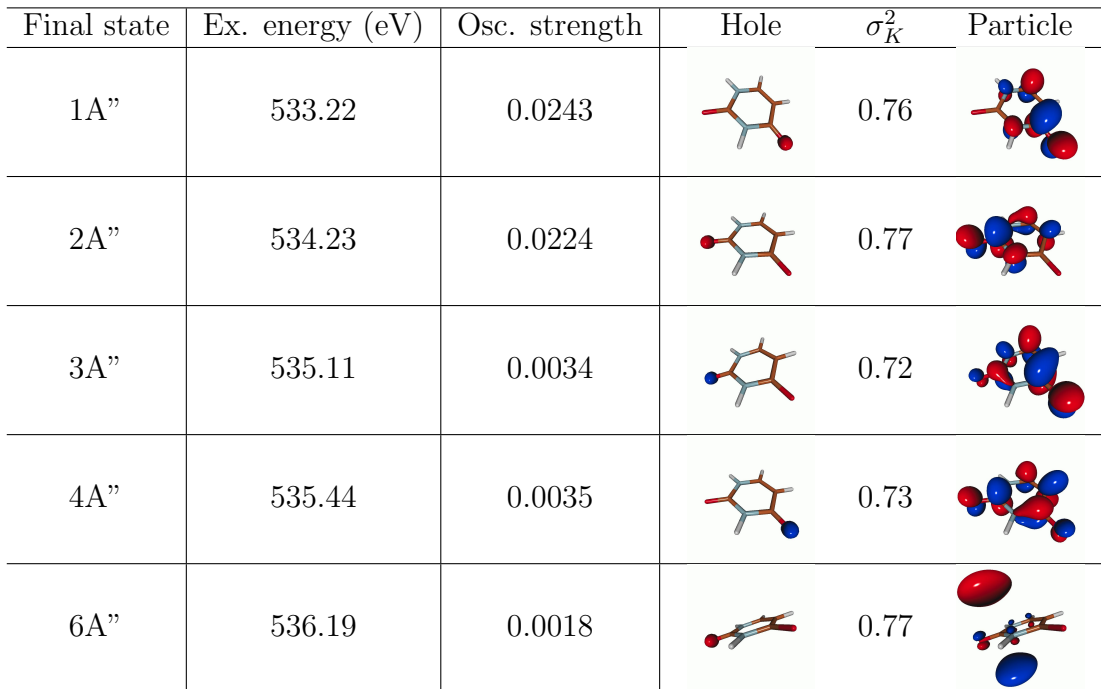  | 0.73         | 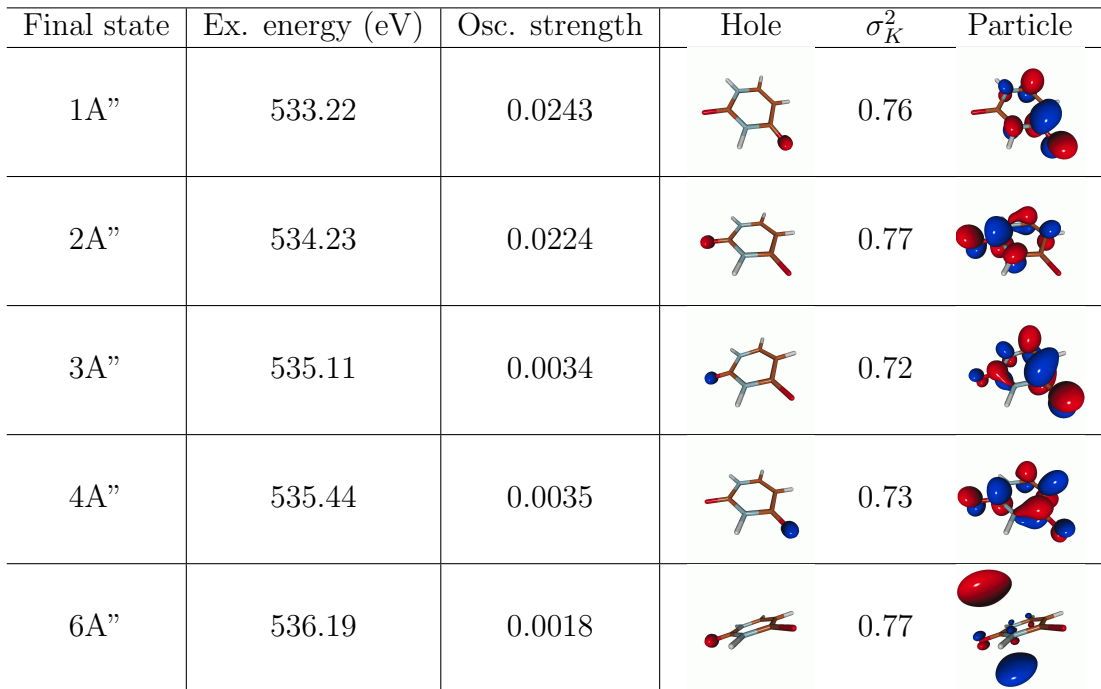  |
| 6A''        | 536.19          | 0.0018        | 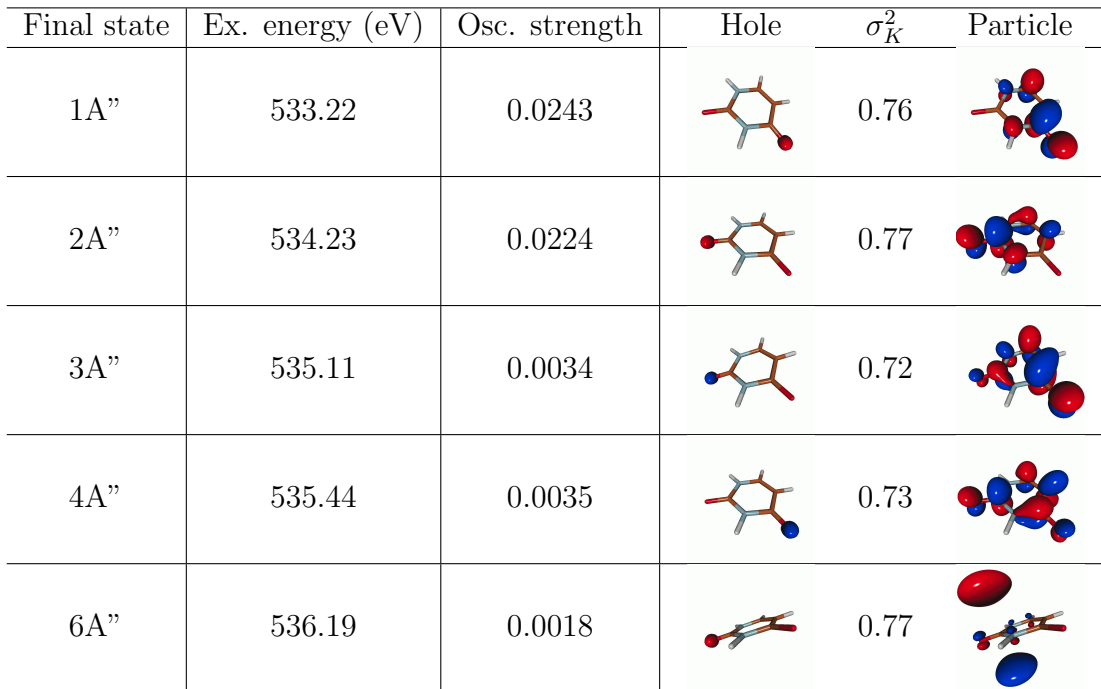 | 0.77         | 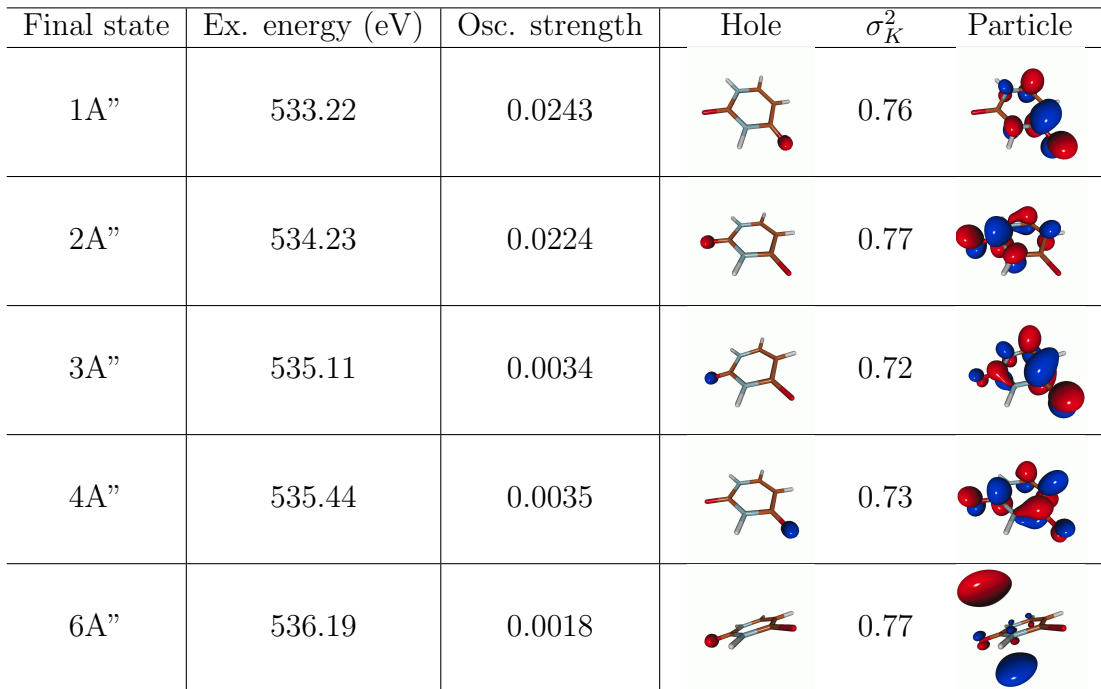 |

Table S3: Uracil. TDDFT/B3LYP/6-311++G\*\* energies, strengths and NTOs of the  $O_{1s}$  core excitations from the ground state at the FC geometry (NTO isosurface is 0.05).

| Final state | Ex. energy (eV) | Osc. strength | Hole                                                                                 | $\sigma_K^2$ | Particle                                                                              |
|-------------|-----------------|---------------|--------------------------------------------------------------------------------------|--------------|---------------------------------------------------------------------------------------|
| 1A''        | 516.58          | 0.0240        | 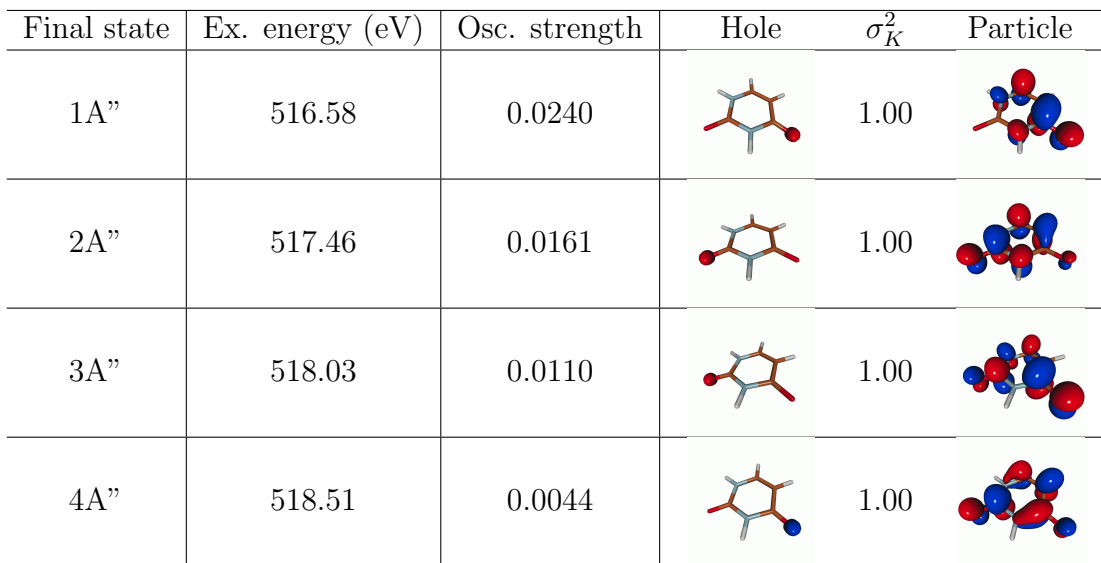 | 1.00         | 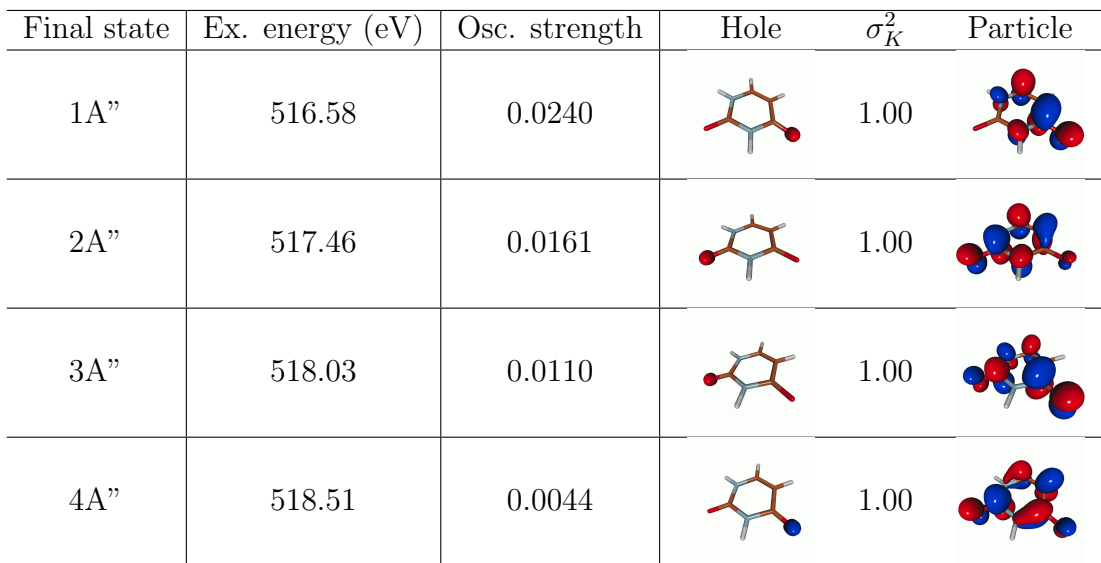 |
| 2A''        | 517.46          | 0.0161        | 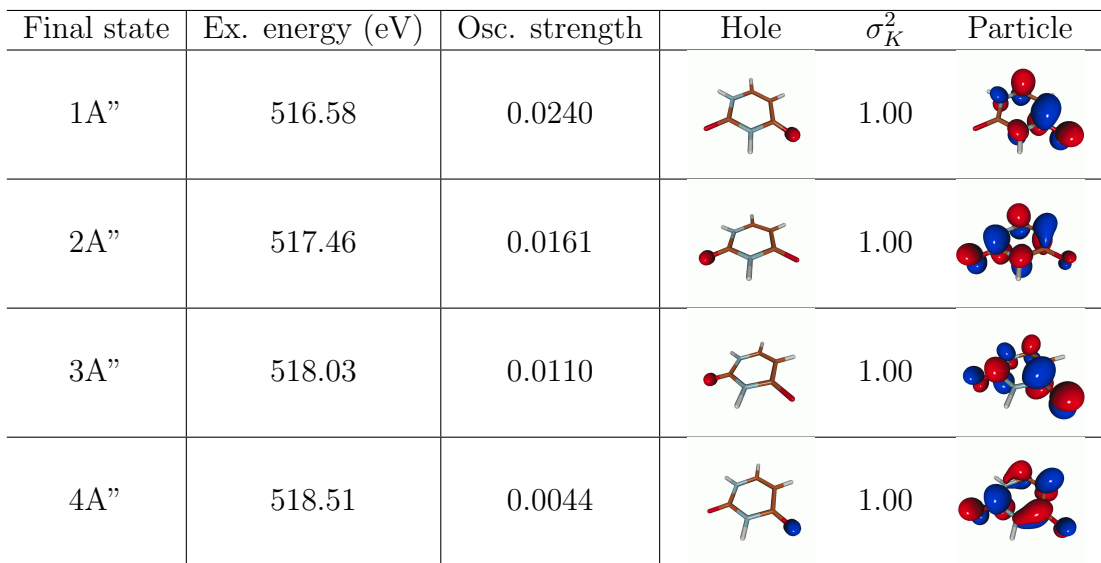 | 1.00         | 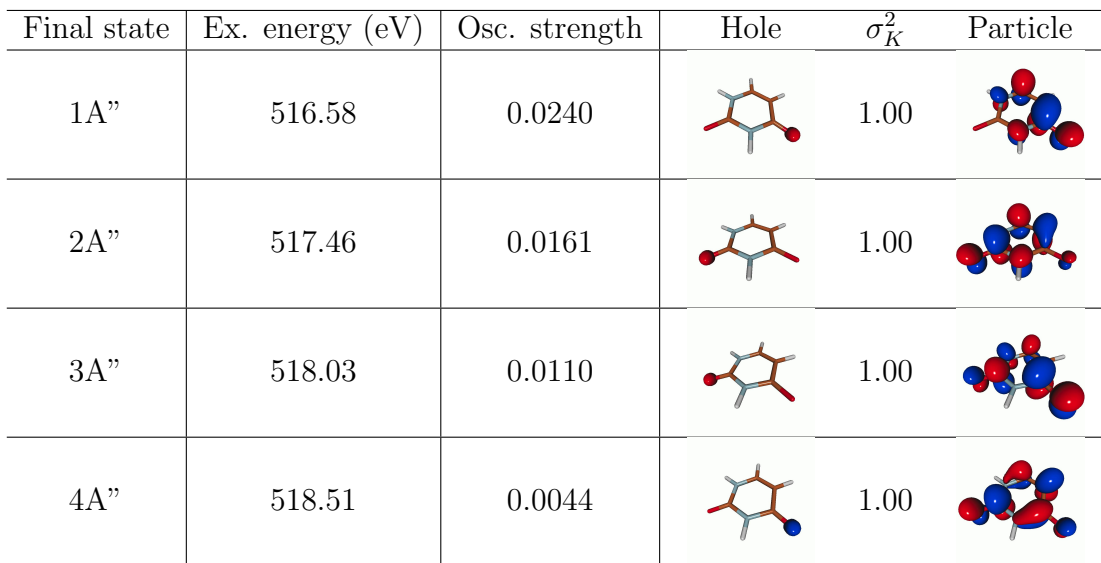 |
| 3A''        | 518.03          | 0.0110        | 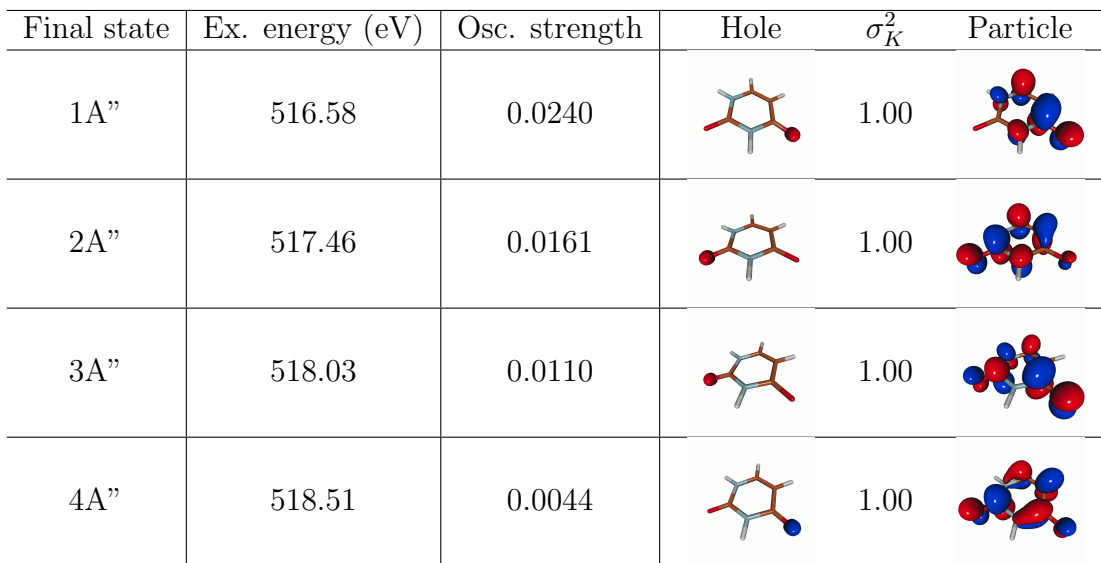 | 1.00         | 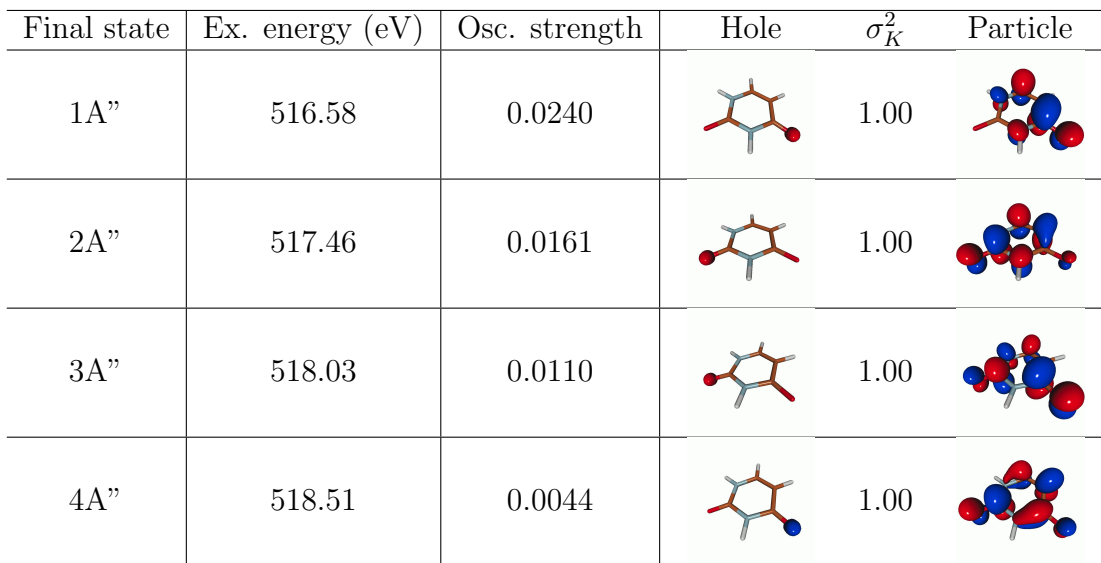 |
| 4A''        | 518.51          | 0.0044        | 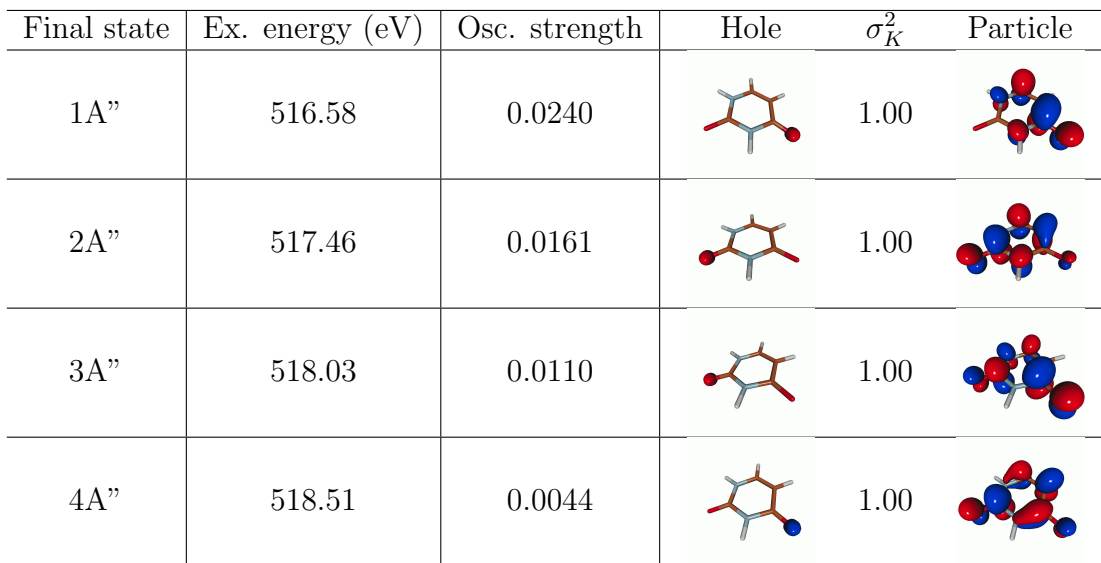 | 1.00         | 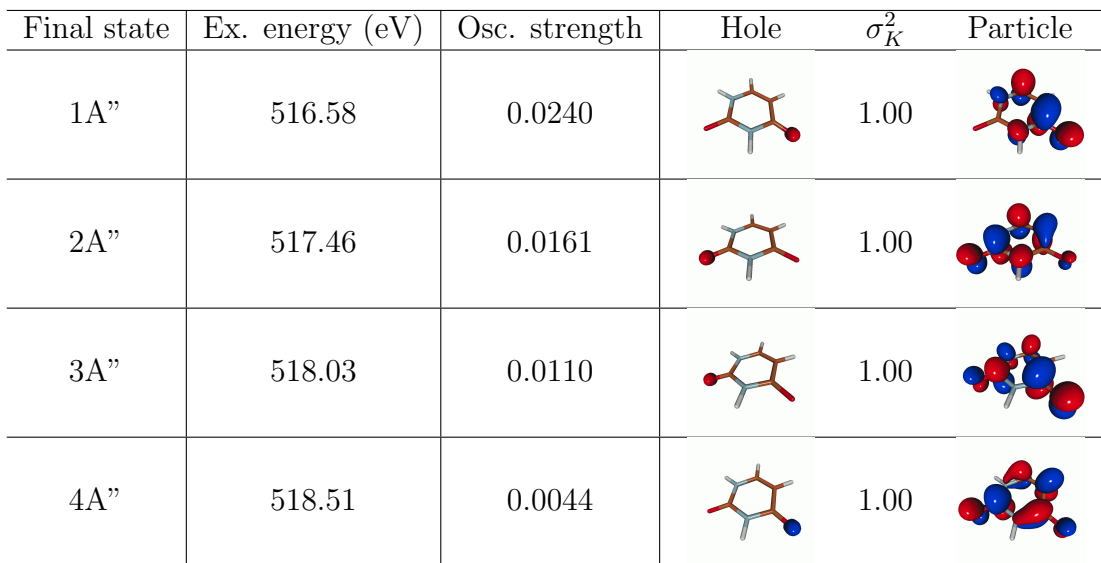 |

Table S4: Thymine. NTOs of the  $O_{1s}$  core excitations from the ground state at the FC geometry (NTO isosurface is 0.03 for the Rydberg transition and 0.05 for the others) at the CVS-EOM-CCSD/6-311++G\*\* level.

| Final state | Ex. energy (eV) | Osc. strength | Hole                                                                                | $\sigma_K^2$ | Particle                                                                             |
|-------------|-----------------|---------------|-------------------------------------------------------------------------------------|--------------|--------------------------------------------------------------------------------------|
| 1A          | 533.12          | 0.0368        | 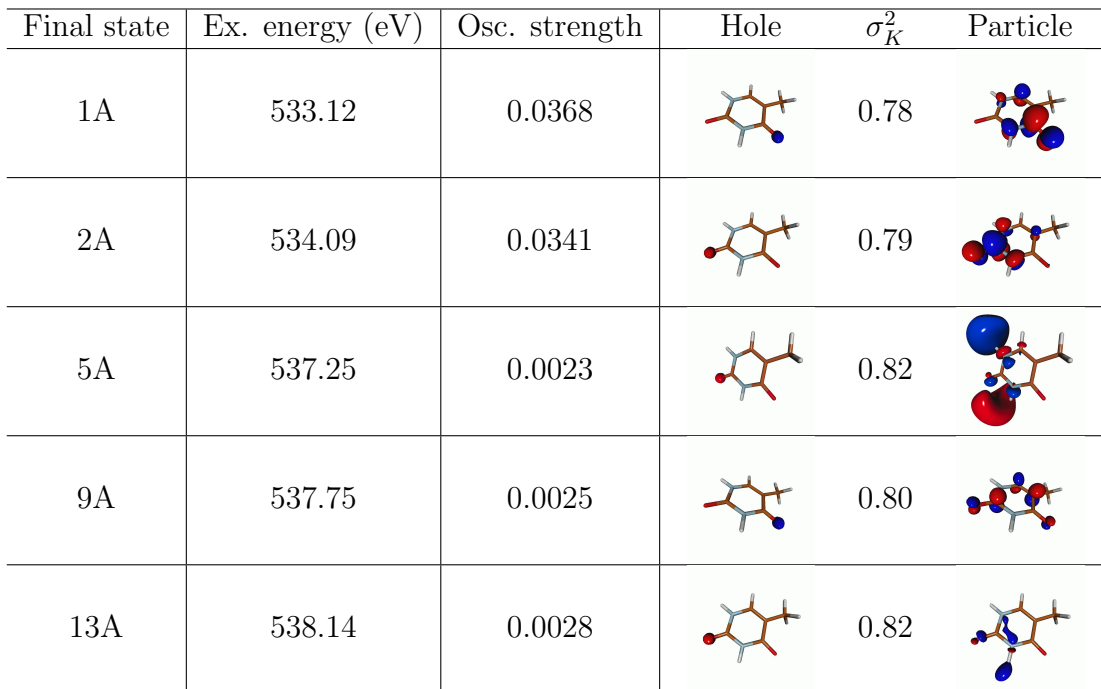  | 0.78         | 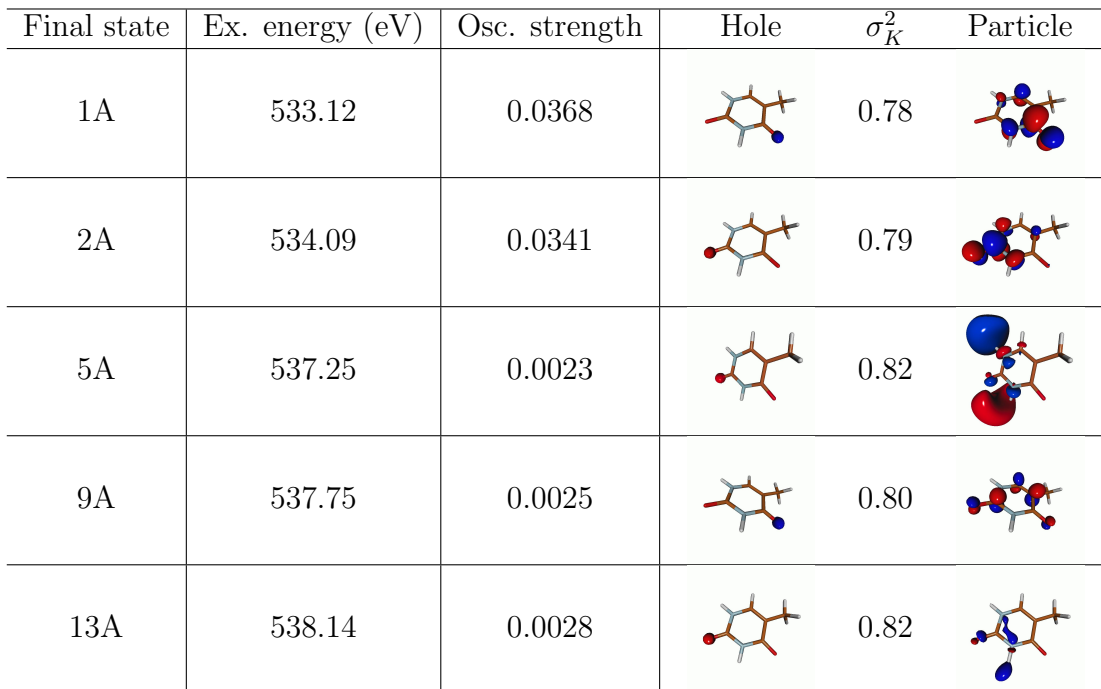  |
| 2A          | 534.09          | 0.0341        | 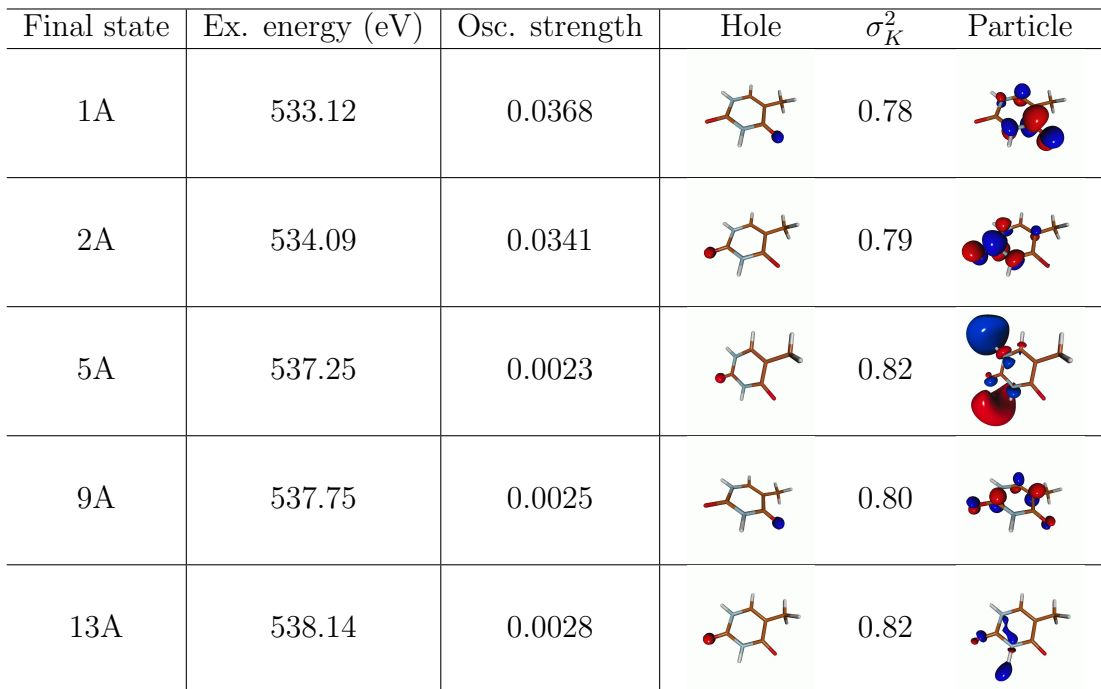  | 0.79         | 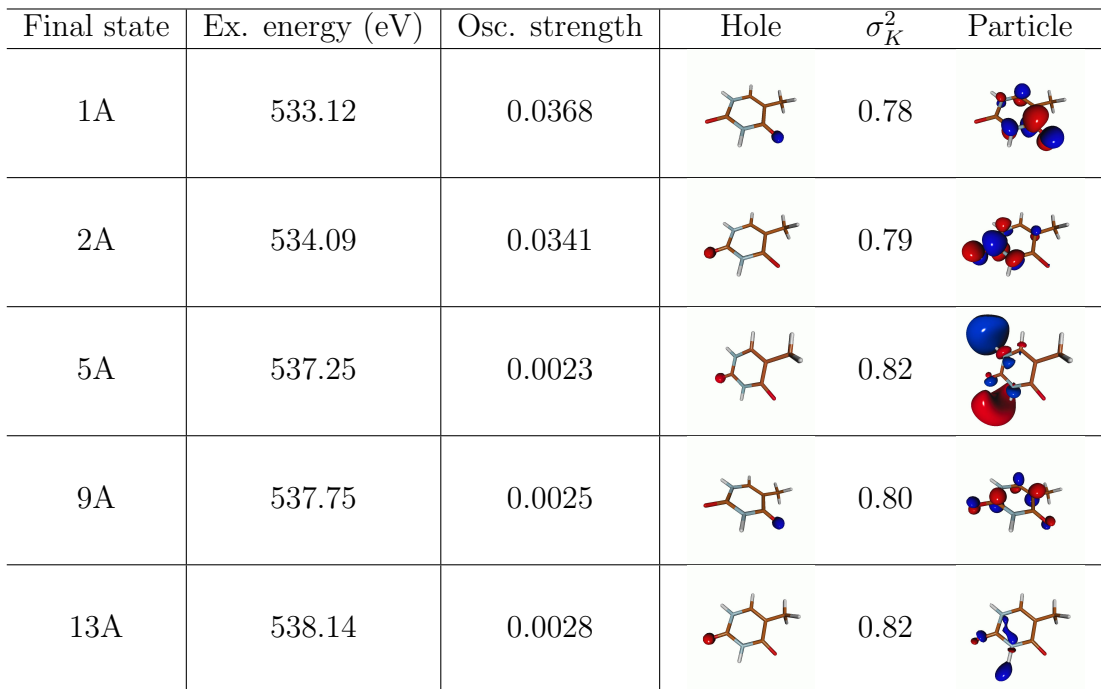  |
| 5A          | 537.25          | 0.0023        | 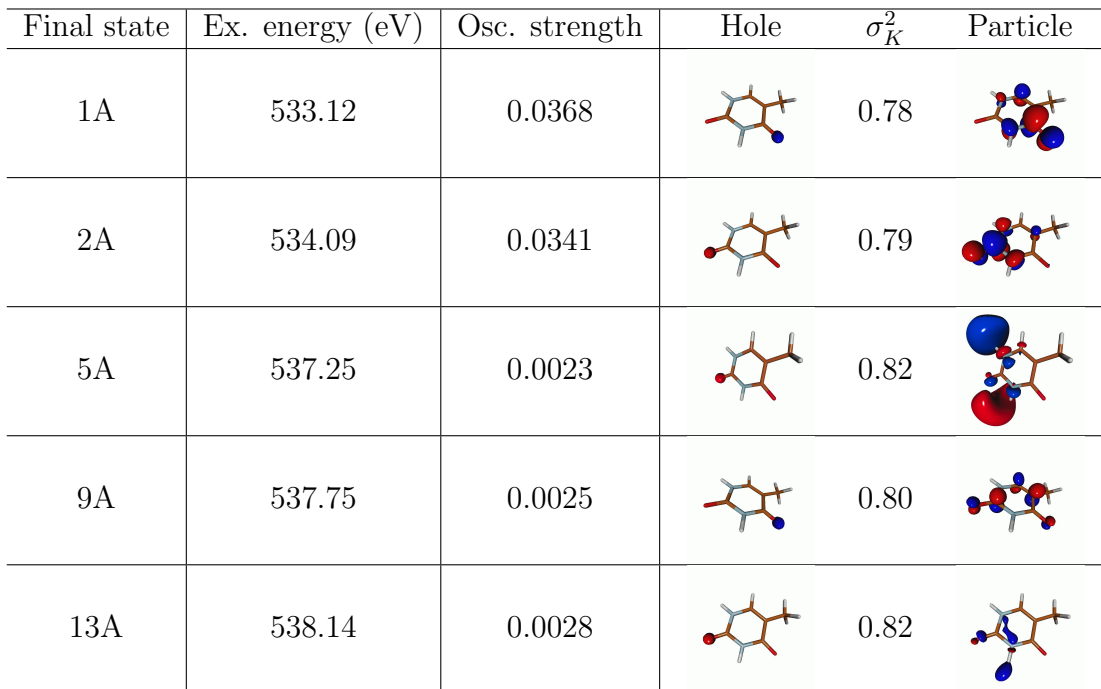  | 0.82         | 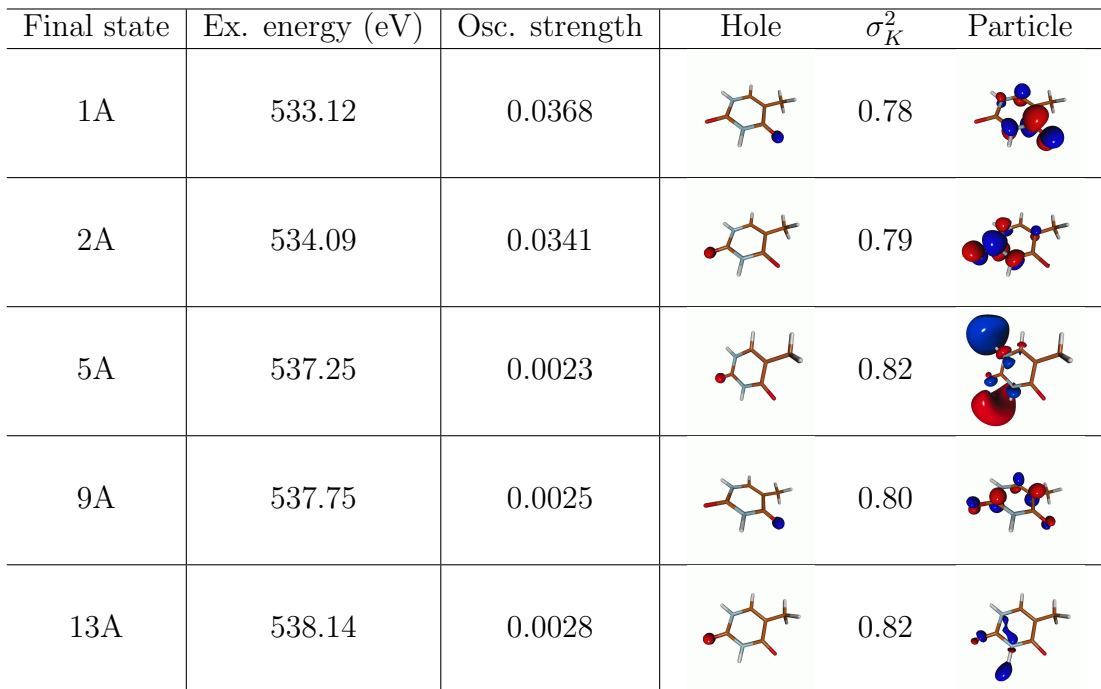  |
| 9A          | 537.75          | 0.0025        | 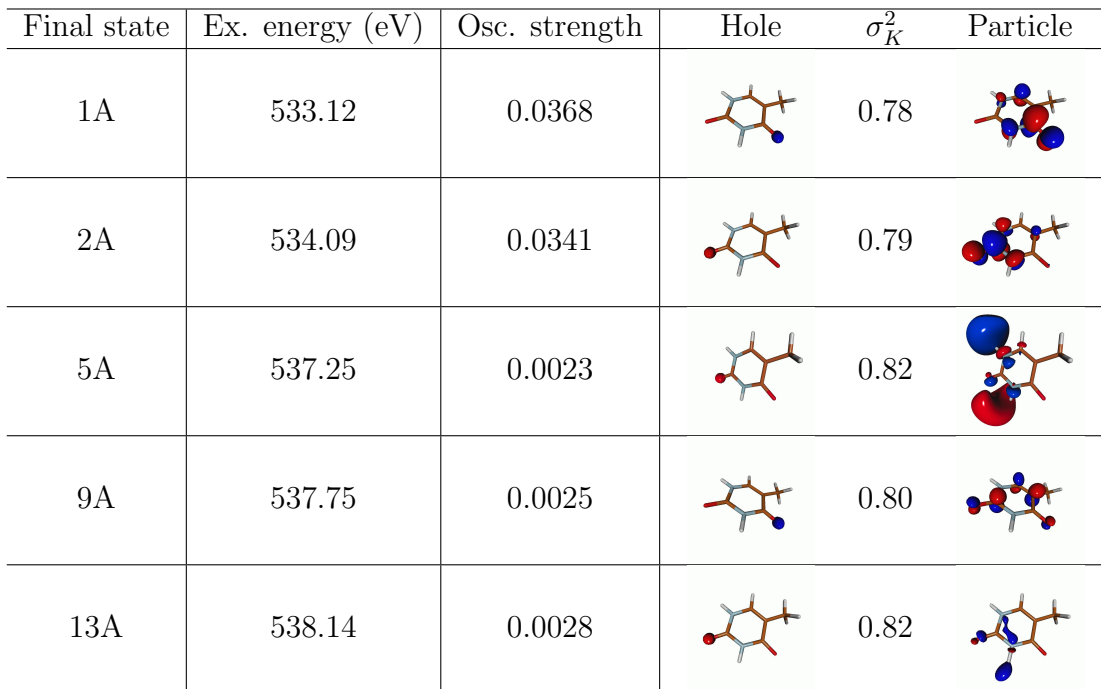  | 0.80         | 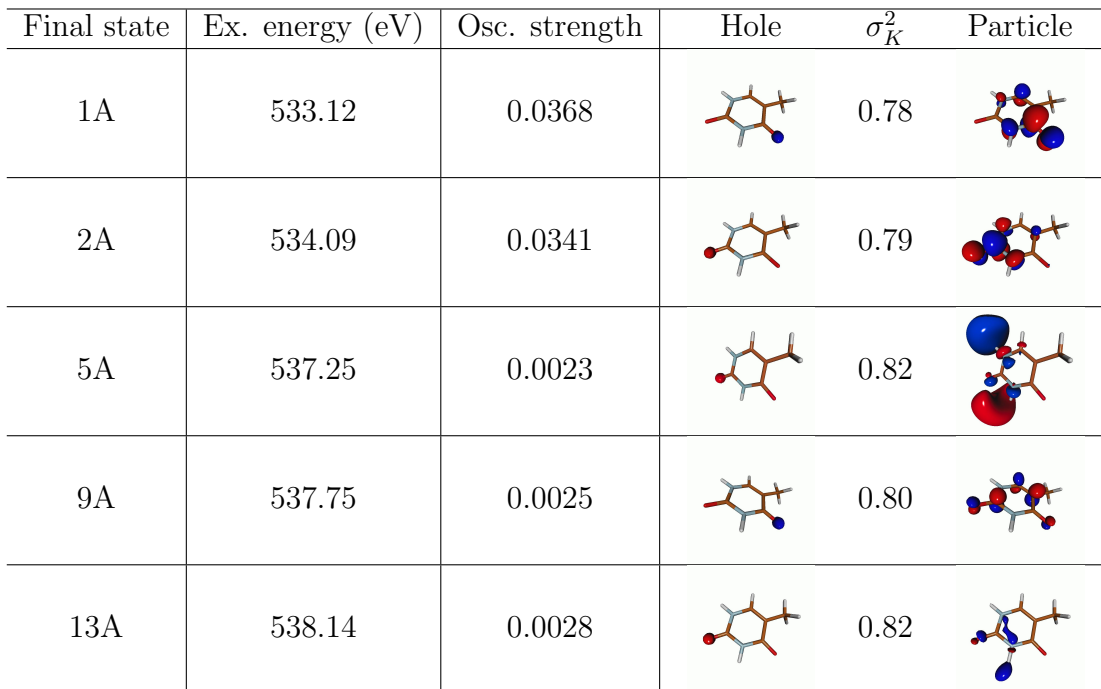  |
| 13A         | 538.14          | 0.0028        | 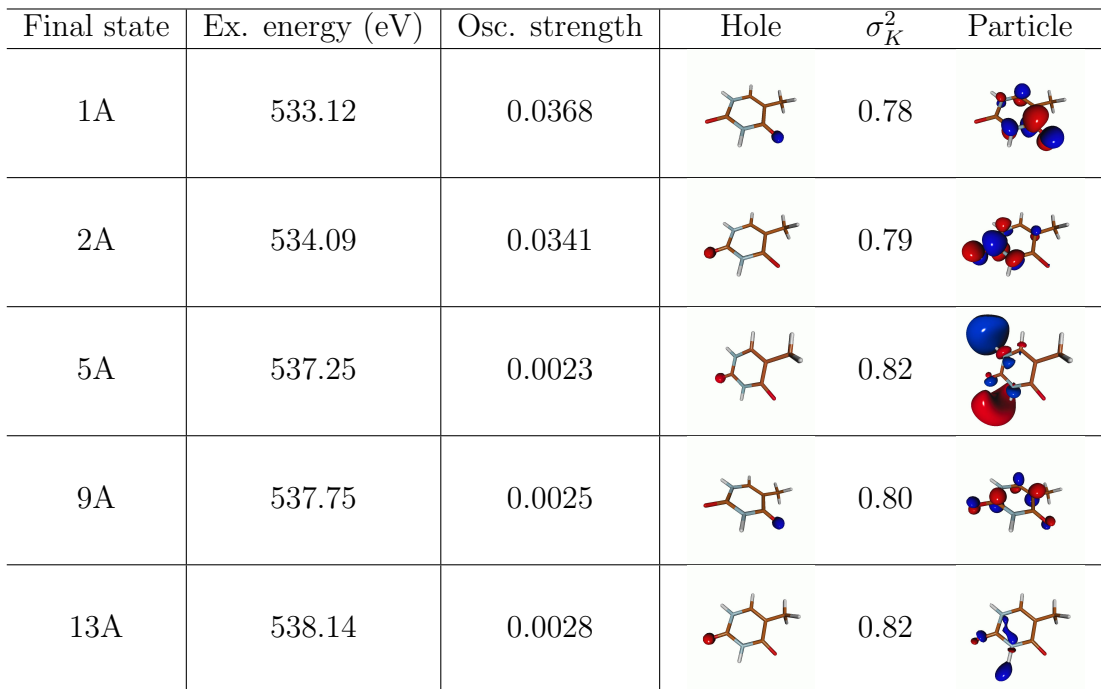 | 0.82         | 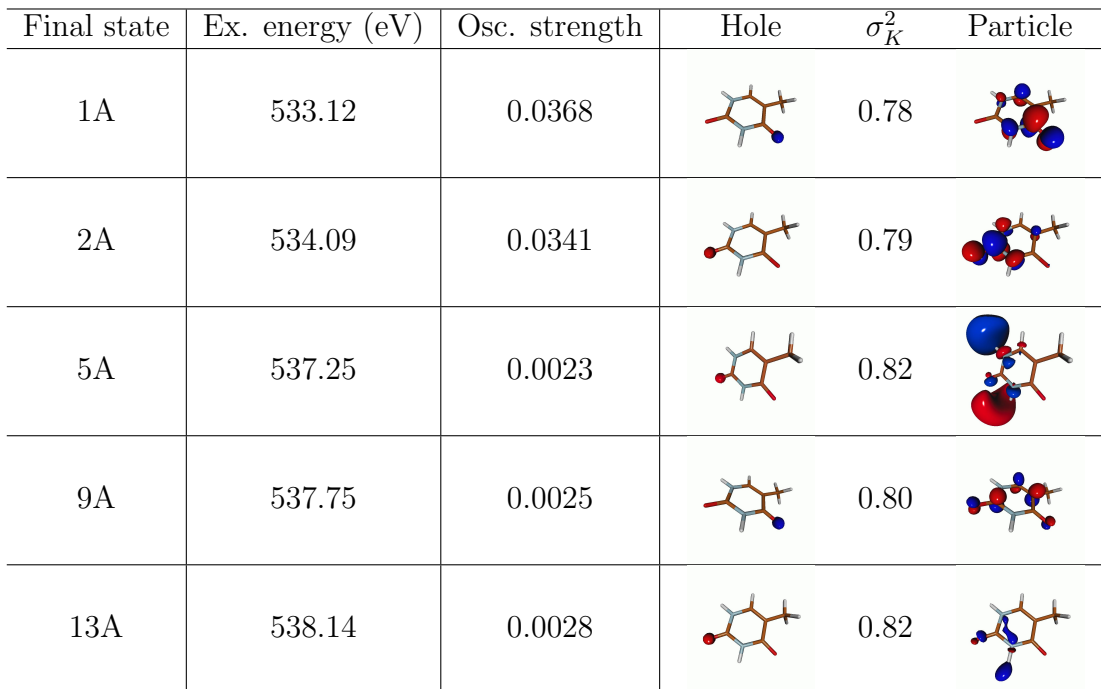 |

Table S5: Thymine. NTOs of the  $O_{1s}$  core excitations from the ground state at the FC geometry (NTO isosurface is 0.03 for the Rydberg transition and 0.05 for the others) at the CVS-ADC(2)/6-311++G\*\* level.

| Final state | Ex. energy (eV) | Osc. strength | Hole                                                                                 | $\sigma_K^2$ | Particle                                                                              |
|-------------|-----------------|---------------|--------------------------------------------------------------------------------------|--------------|---------------------------------------------------------------------------------------|
| 1A          | 533.15          | 0.0244        | 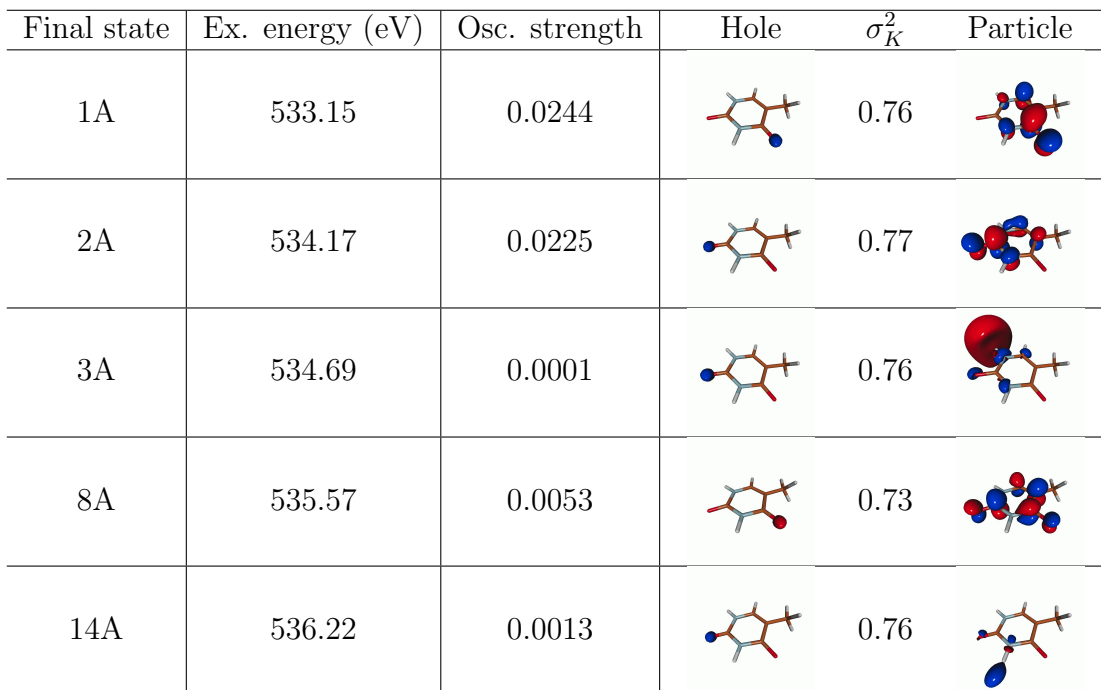 | 0.76         | 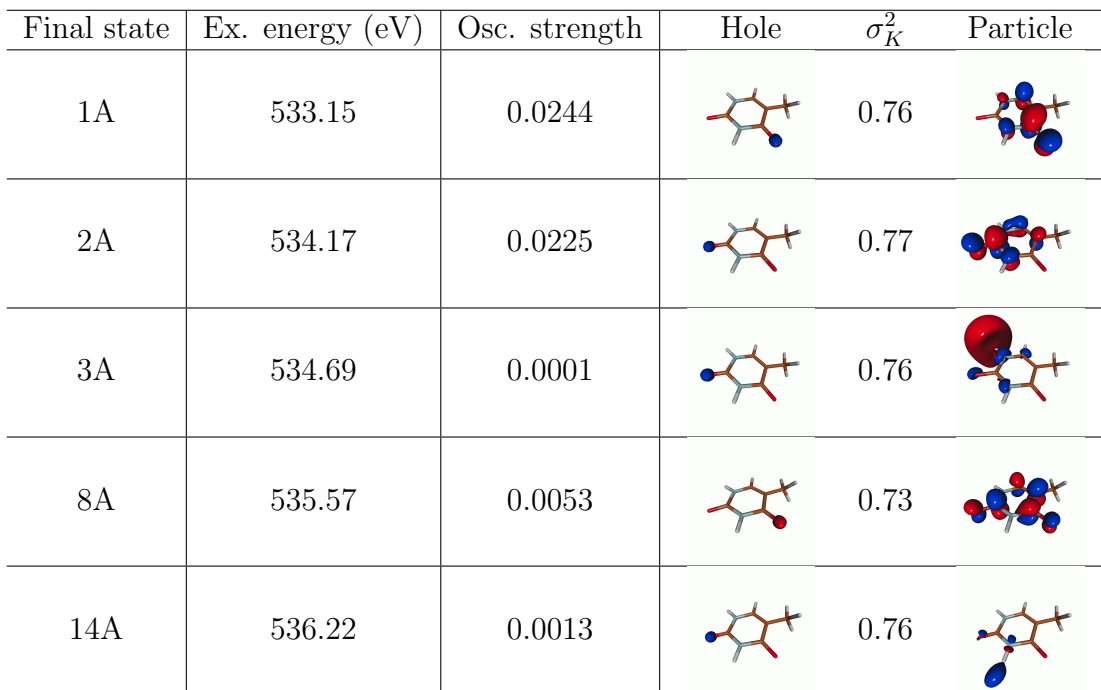 |
| 2A          | 534.17          | 0.0225        | 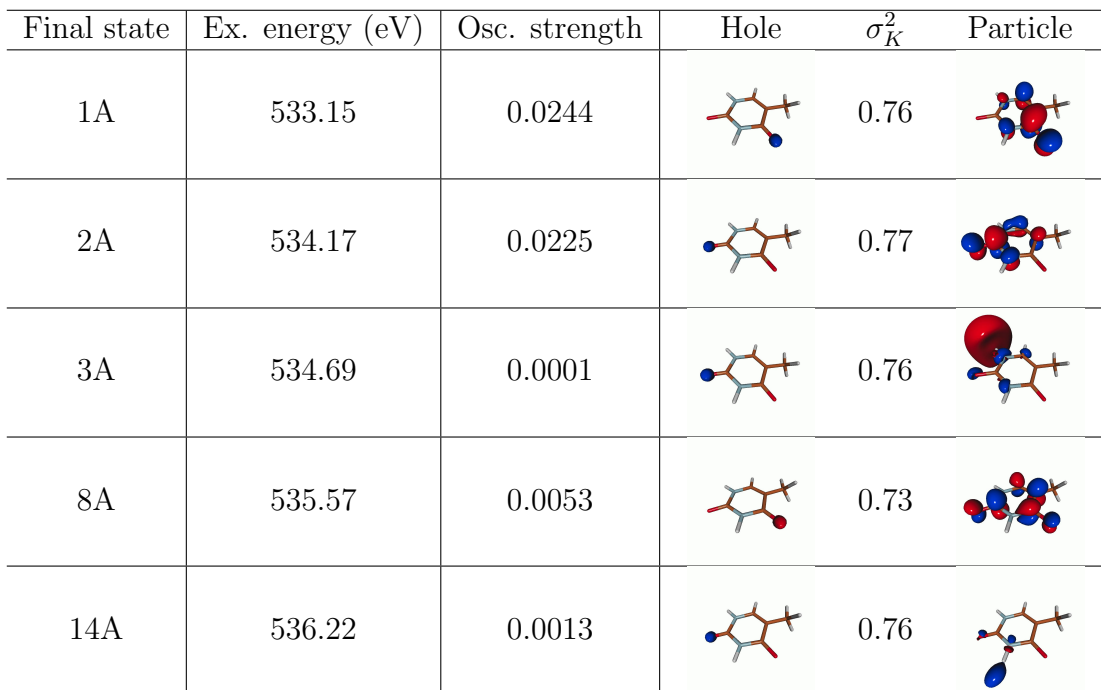 | 0.77         | 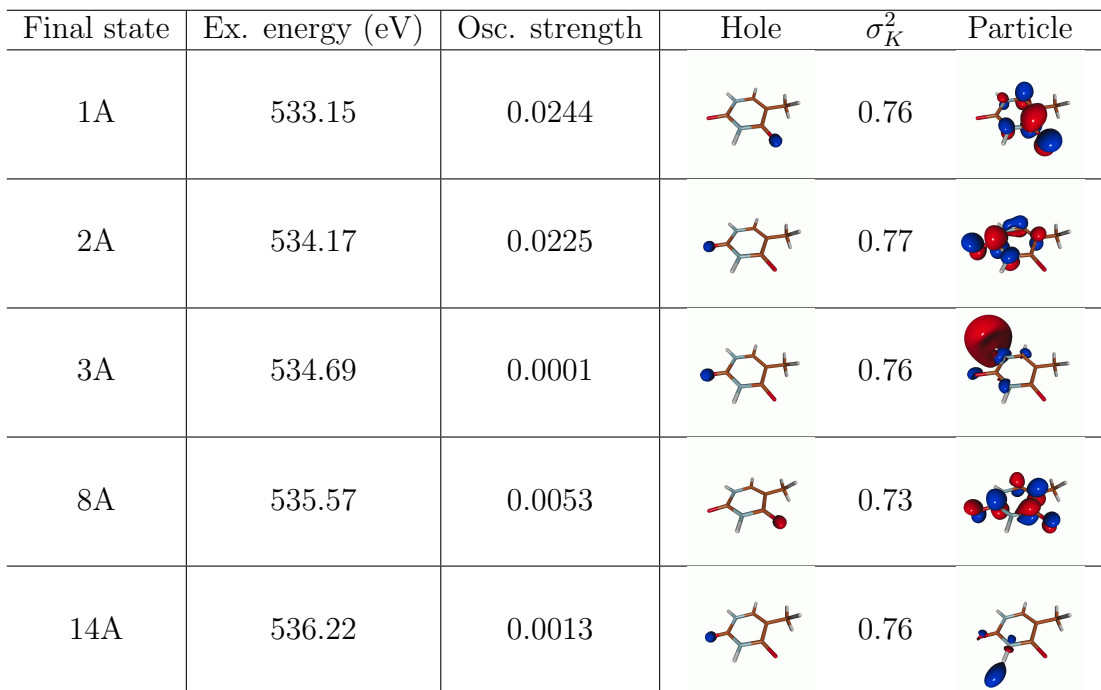 |
| 3A          | 534.69          | 0.0001        | 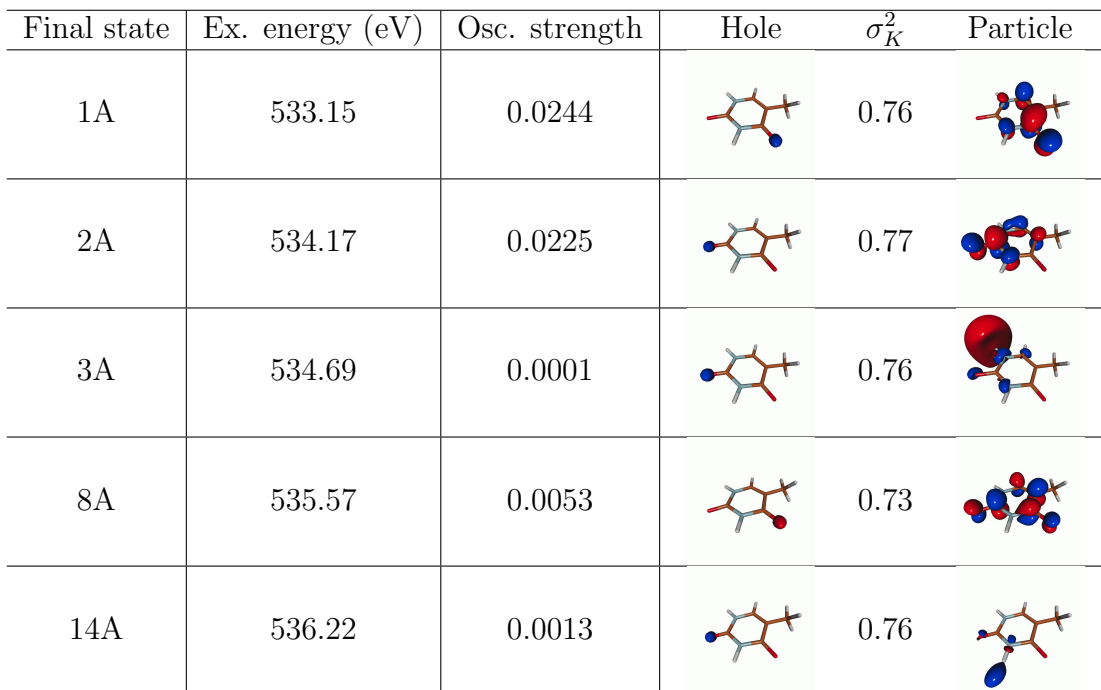 | 0.76         | 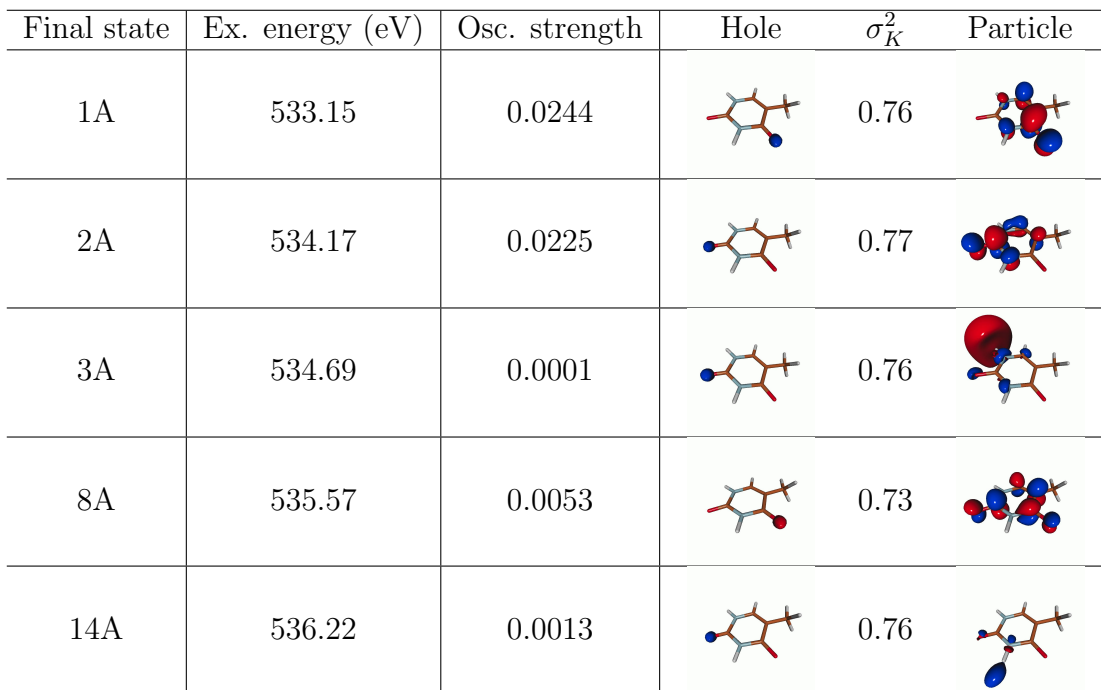 |
| 8A          | 535.57          | 0.0053        | 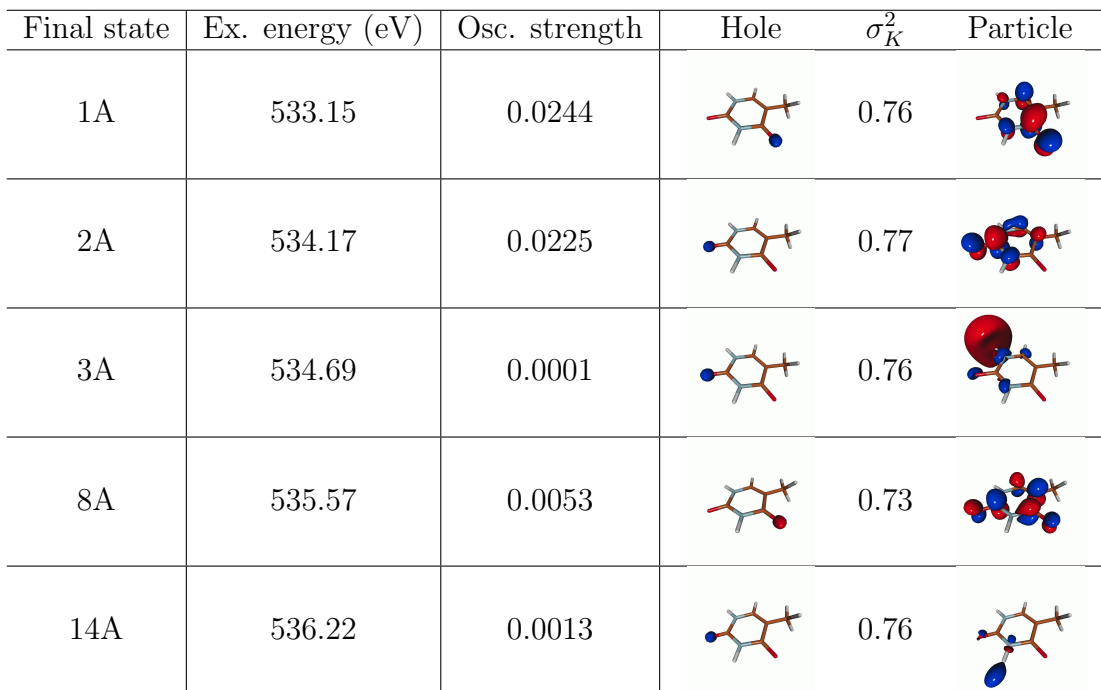 | 0.73         | 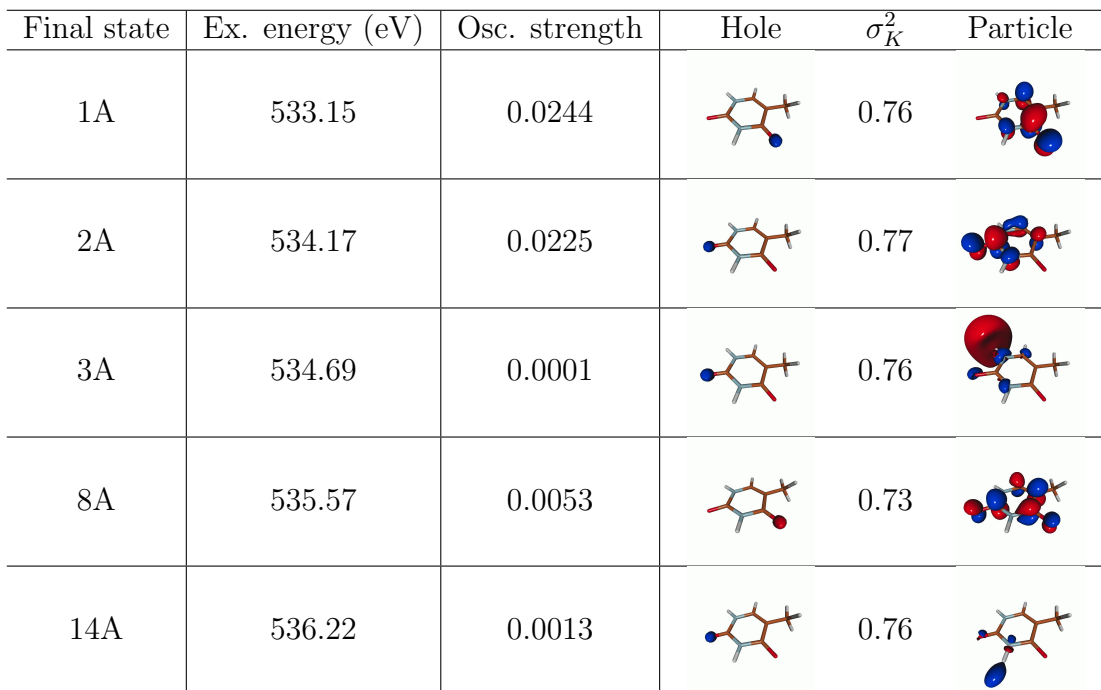 |
| 14A         | 536.22          | 0.0013        | 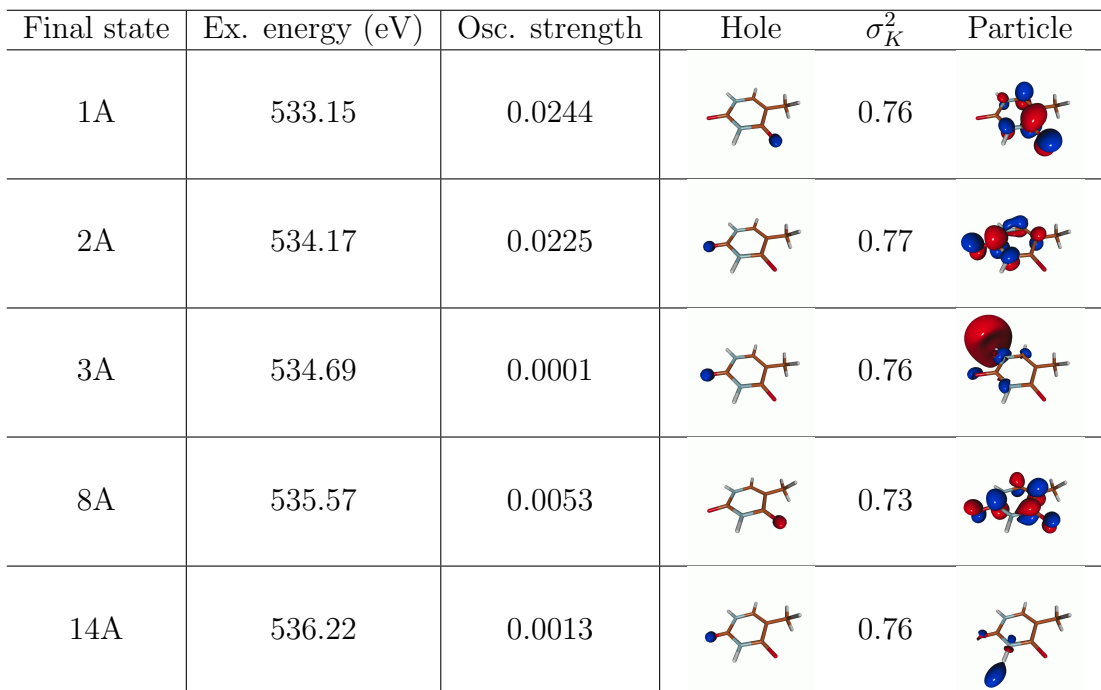 | 0.76         | 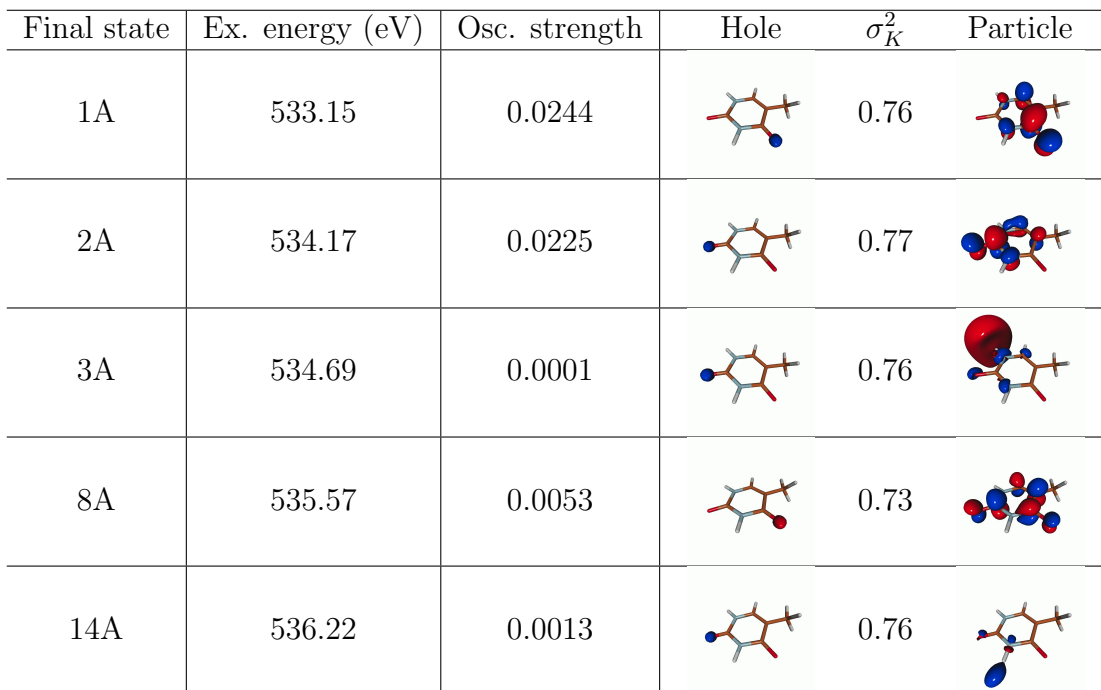 |



Table S6: Thymine. NTOs of the  $O_{1s}$  core excitations from the ground state at the FC geometry (NTO isosurface is 0.05) at the TDDFT/B3LYP/6-311++G\*\* level.

| Final state | Ex. energy (eV) | Osc. strength | Hole                                                                               | $\sigma_K^2$ | Particle                                                                            |
|-------------|-----------------|---------------|------------------------------------------------------------------------------------|--------------|-------------------------------------------------------------------------------------|
| 1A          | 516.60          | 0.0245        | 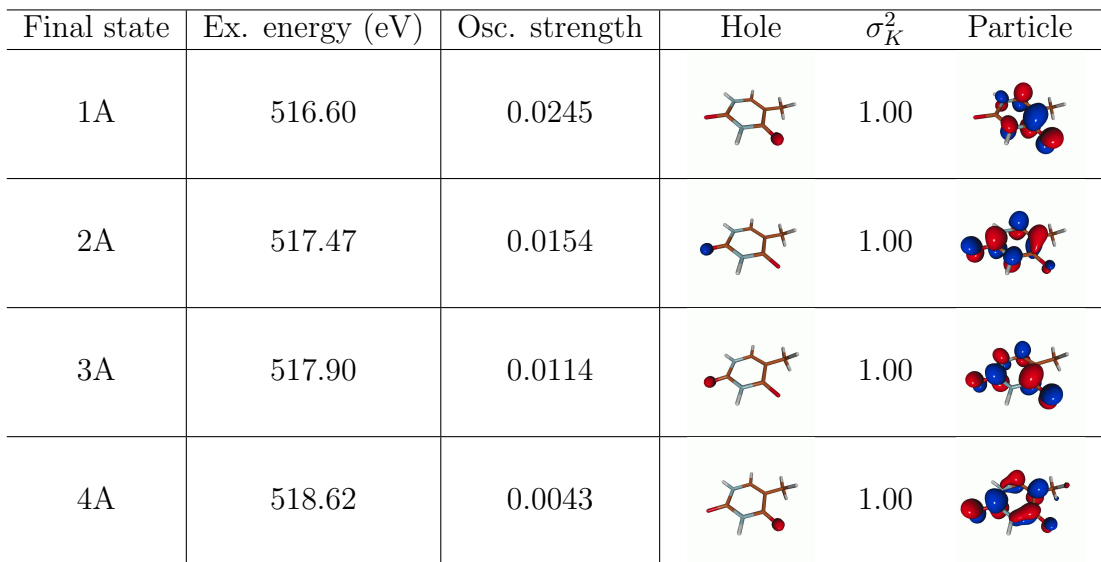 | 1.00         | 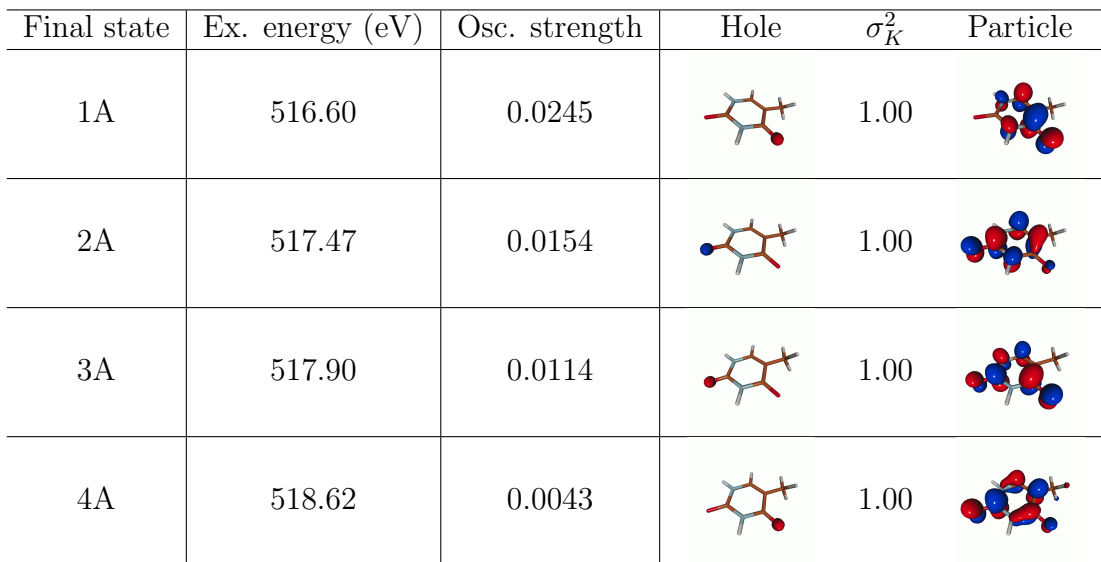 |
| 2A          | 517.47          | 0.0154        | 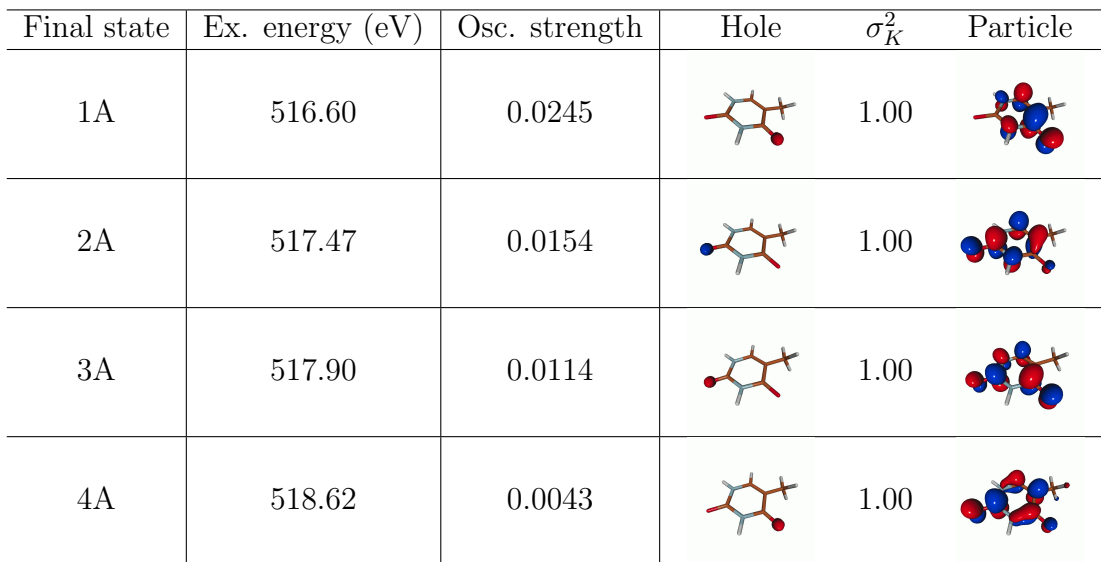 | 1.00         | 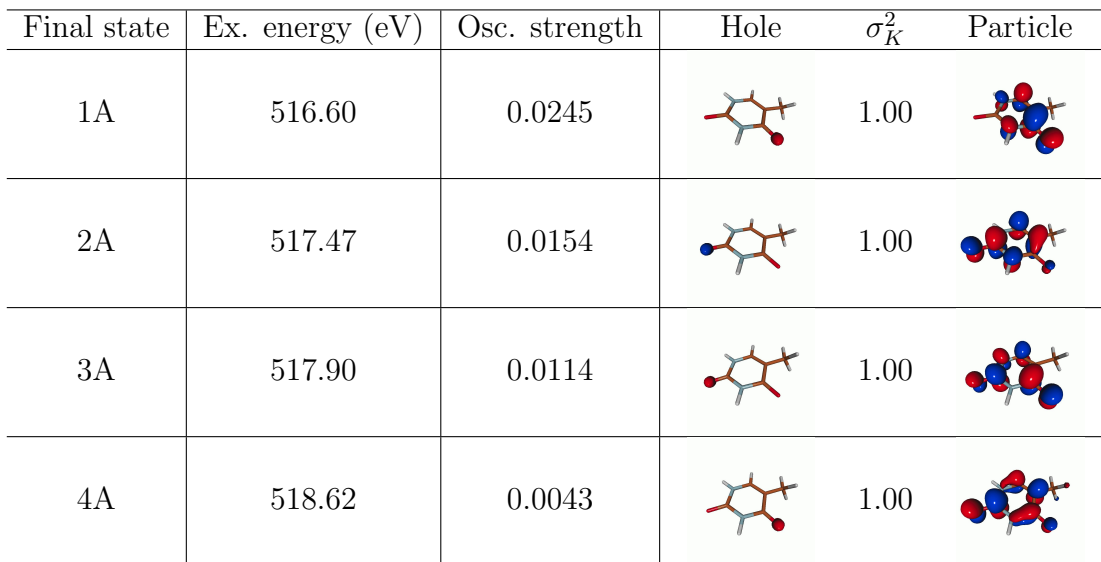 |
| 3A          | 517.90          | 0.0114        | 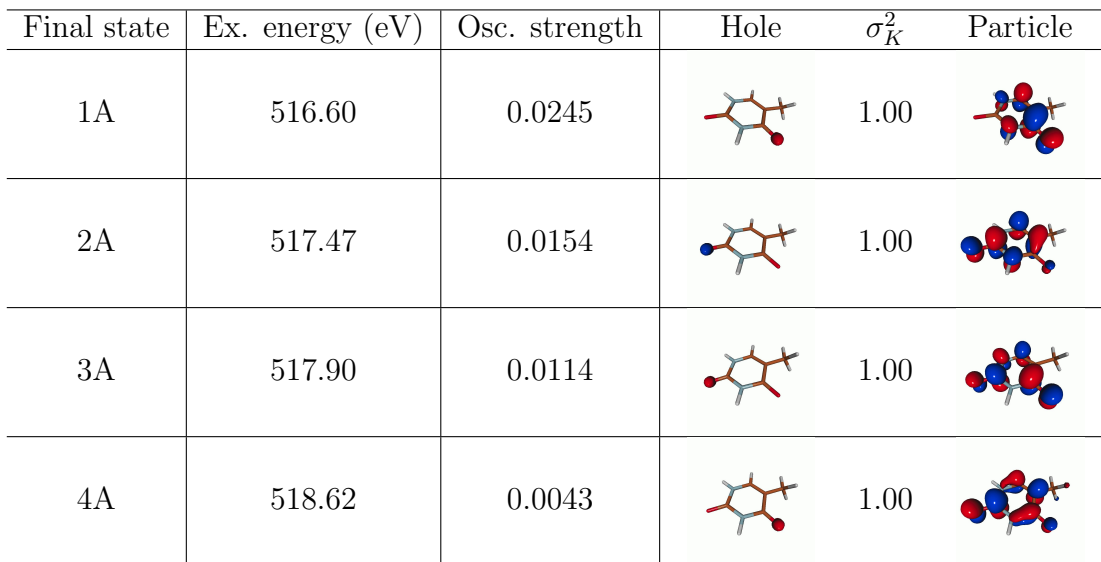 | 1.00         | 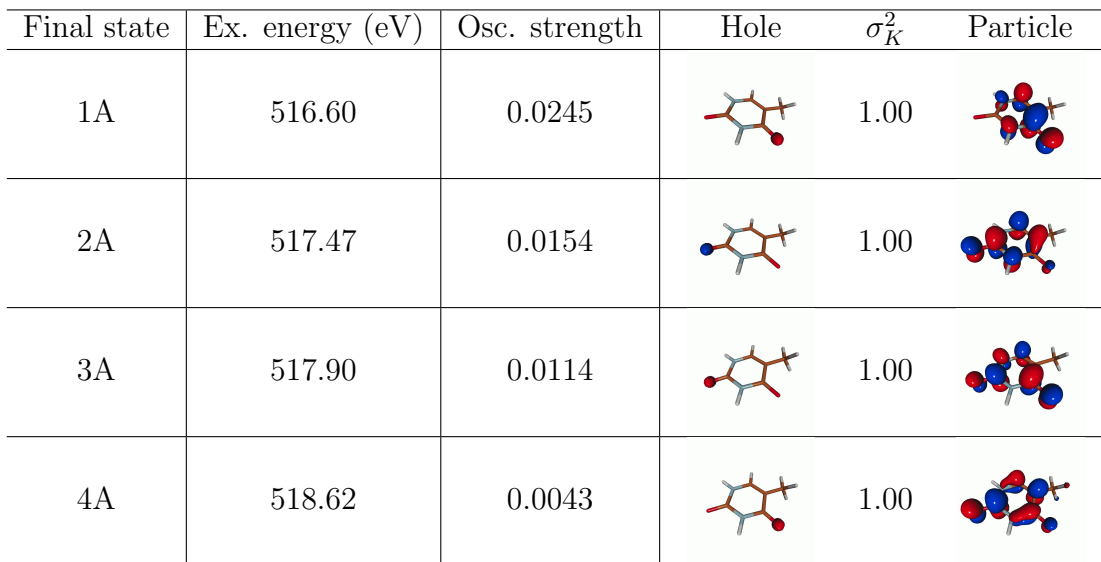 |
| 4A          | 518.62          | 0.0043        | 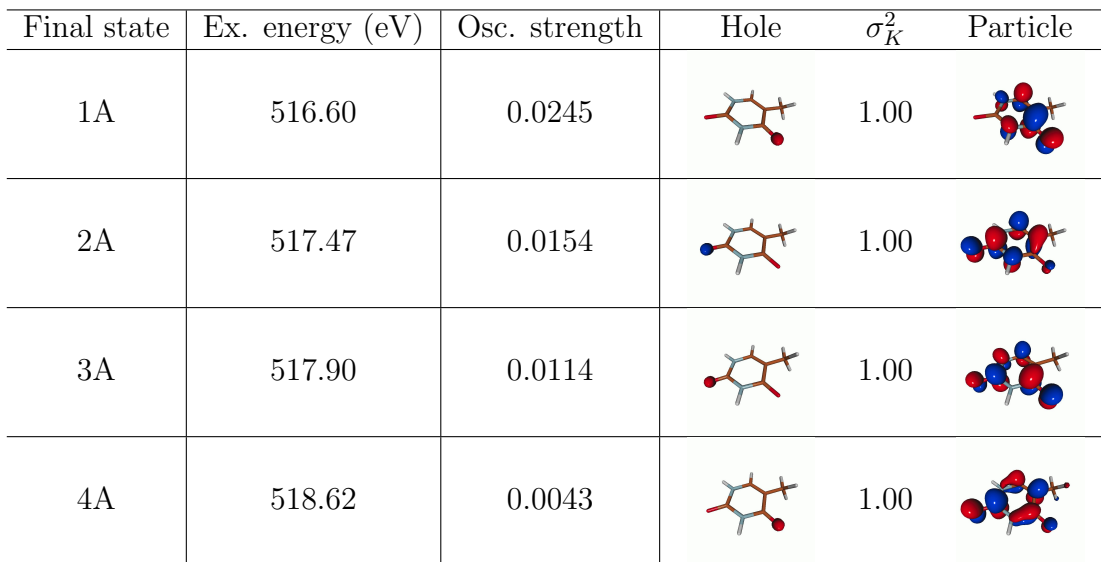 | 1.00         | 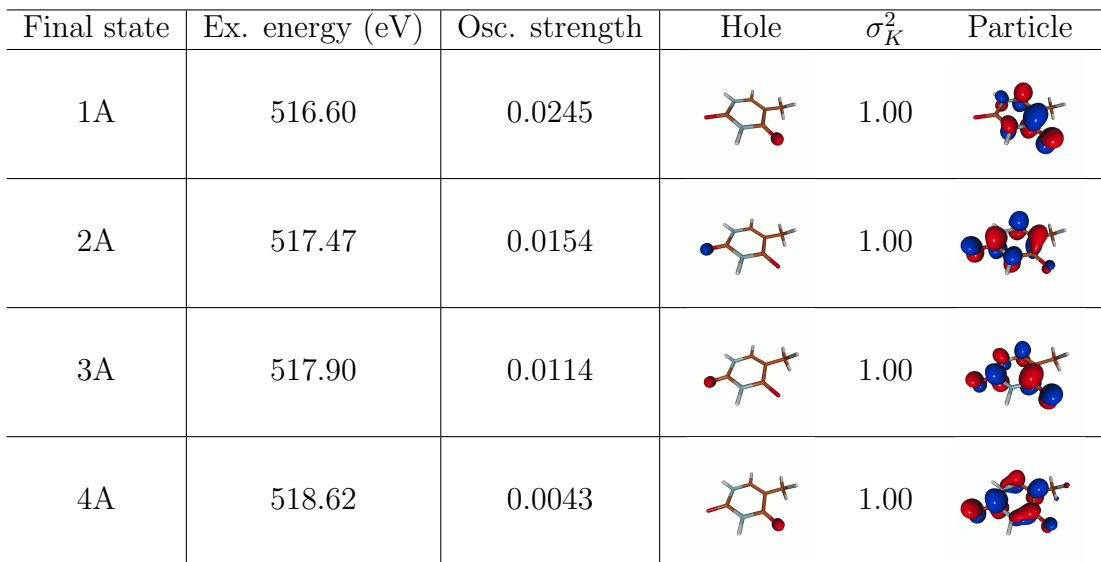 |

Table S7: Acetylacetone. CVS-EOM-CCSD/6-311++G\*\* NTOs of the  $C_{1s}$  core excitations from the ground state at the FC geometry (NTO isosurface is 0.03 for the Rydberg transition and 0.05 for the others).

| Final state | Ex. energy (eV) | Osc. strength | Hole                                                                                 | $\sigma_K^2$ | Particle                                                                              |
|-------------|-----------------|---------------|--------------------------------------------------------------------------------------|--------------|---------------------------------------------------------------------------------------|
| 1A          | 285.88          | 0.0133        | 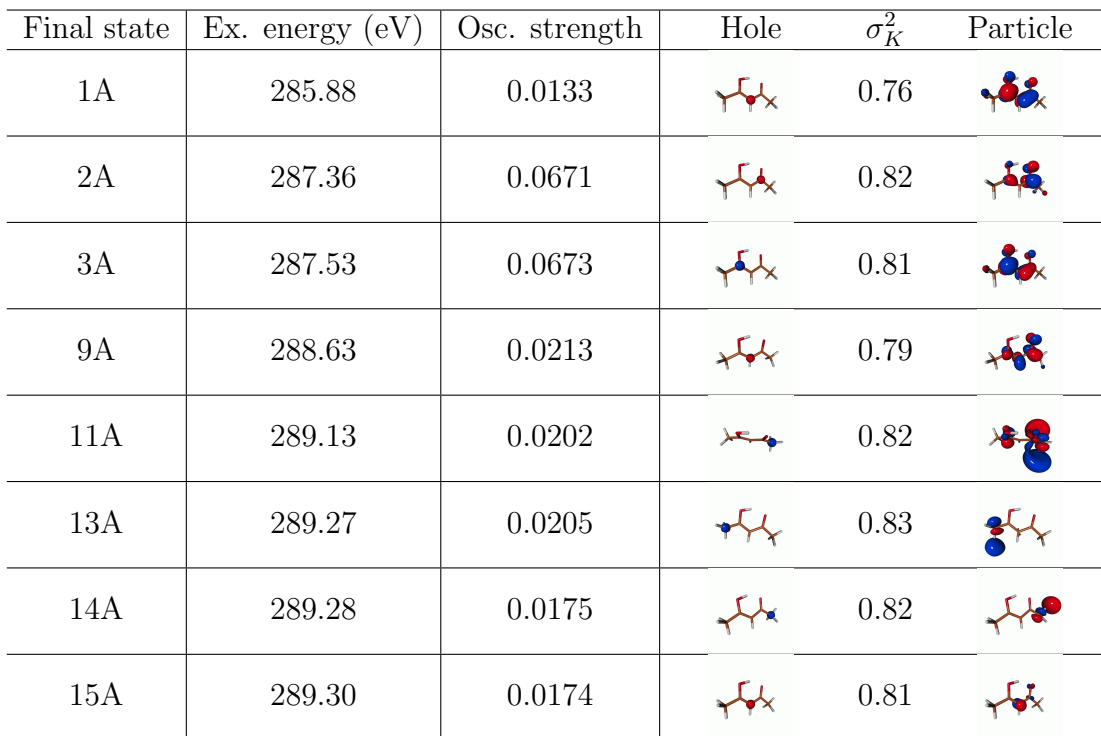 | 0.76         | 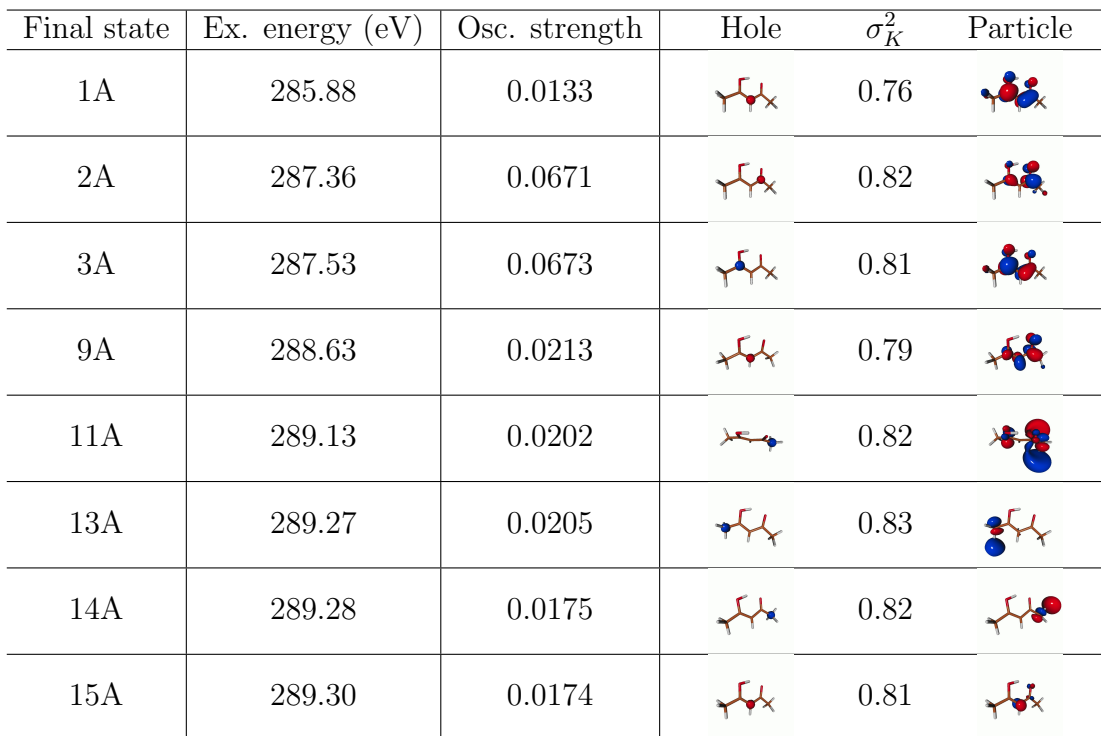 |
| 2A          | 287.36          | 0.0671        | 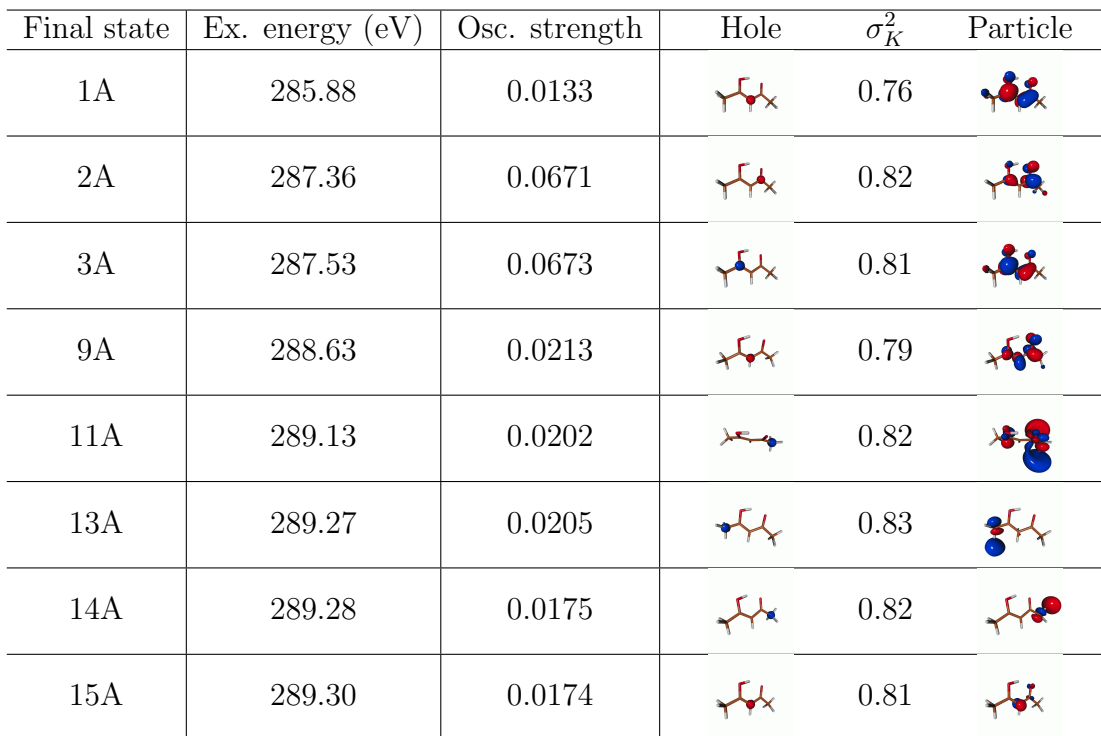 | 0.82         | 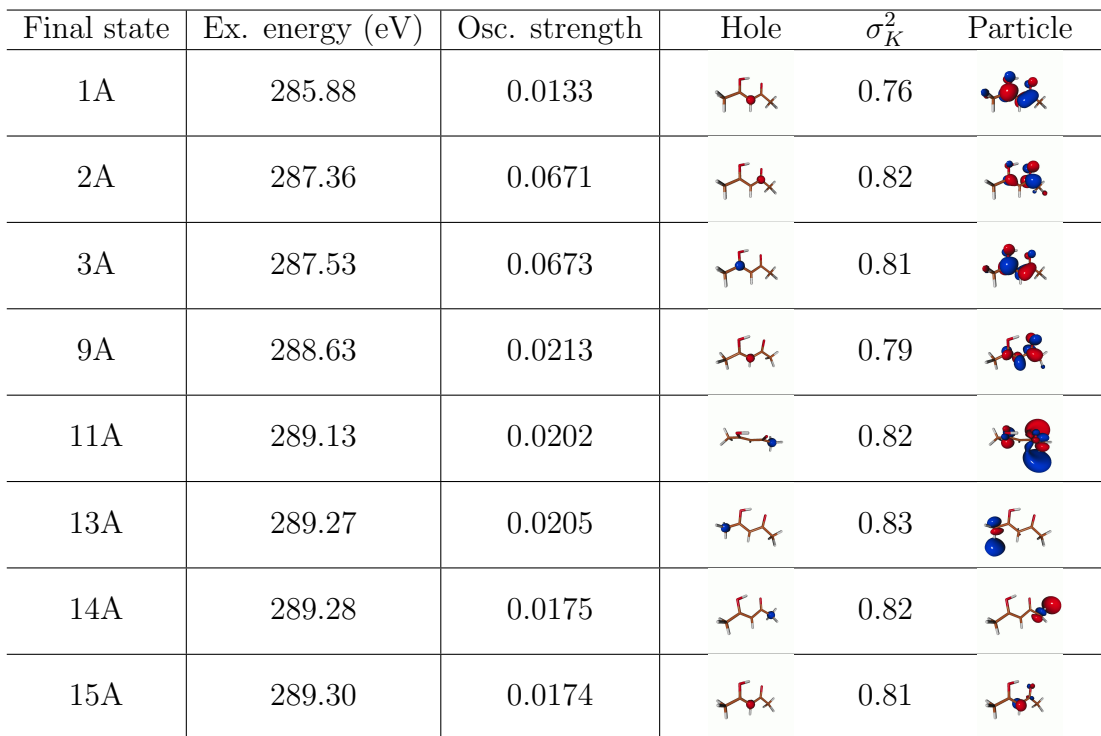 |
| 3A          | 287.53          | 0.0673        | 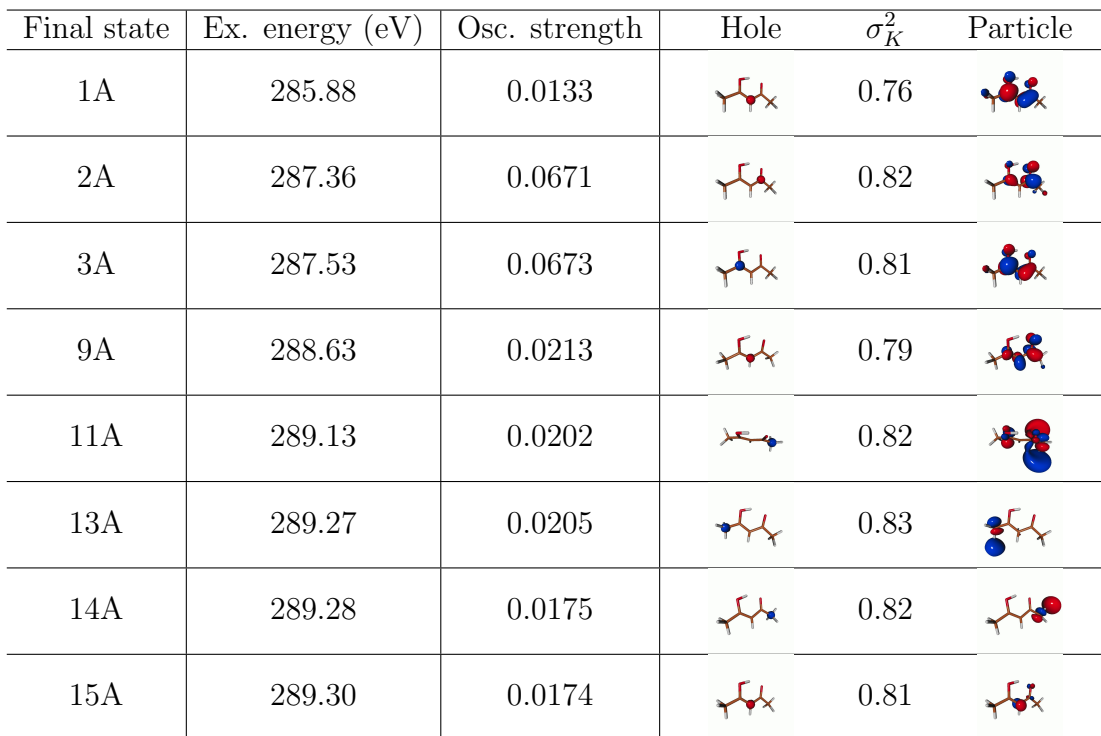 | 0.81         | 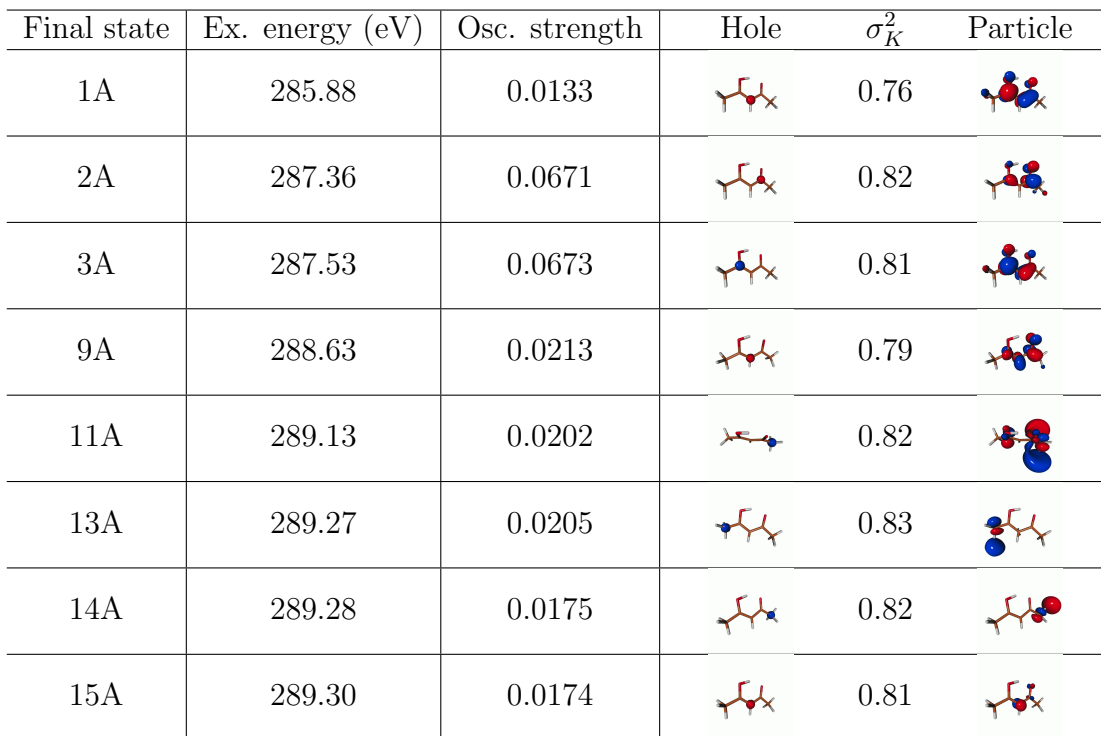 |
| 9A          | 288.63          | 0.0213        | 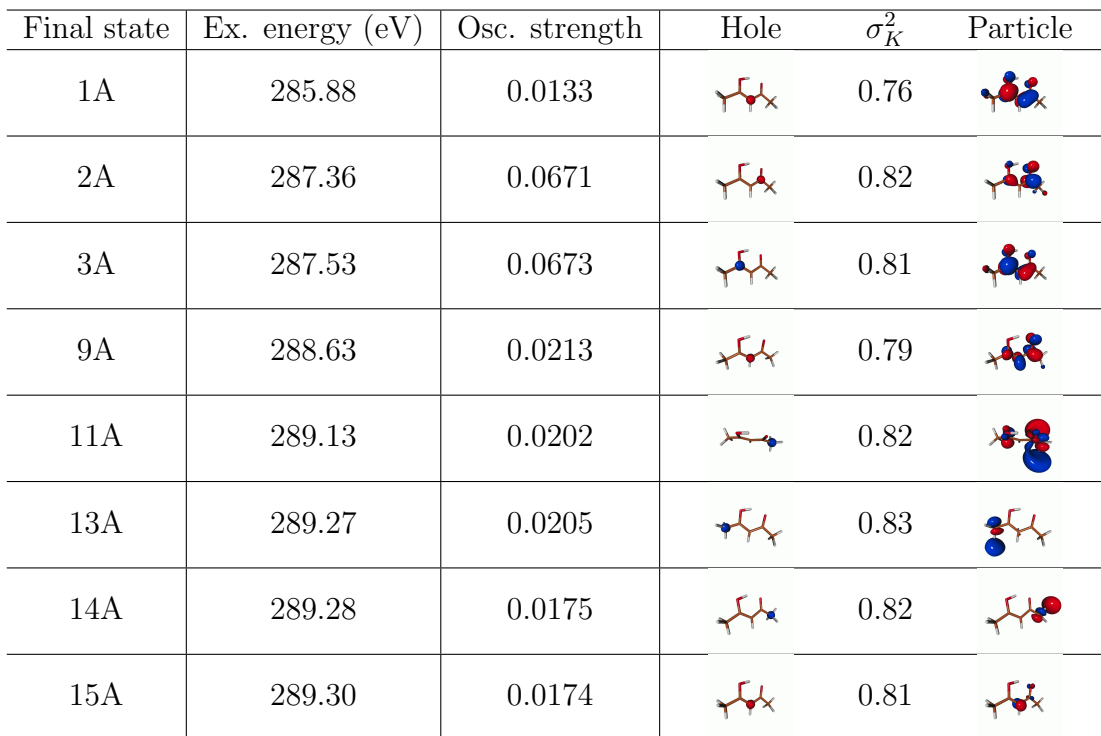 | 0.79         | 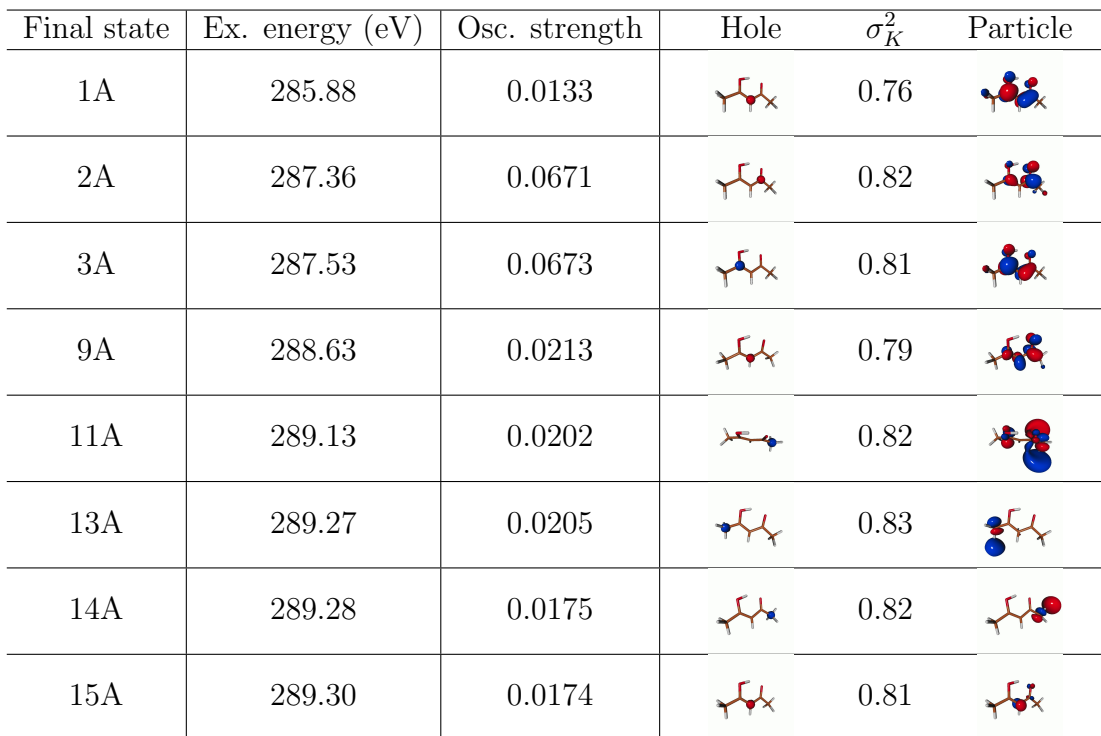 |
| 11A         | 289.13          | 0.0202        | 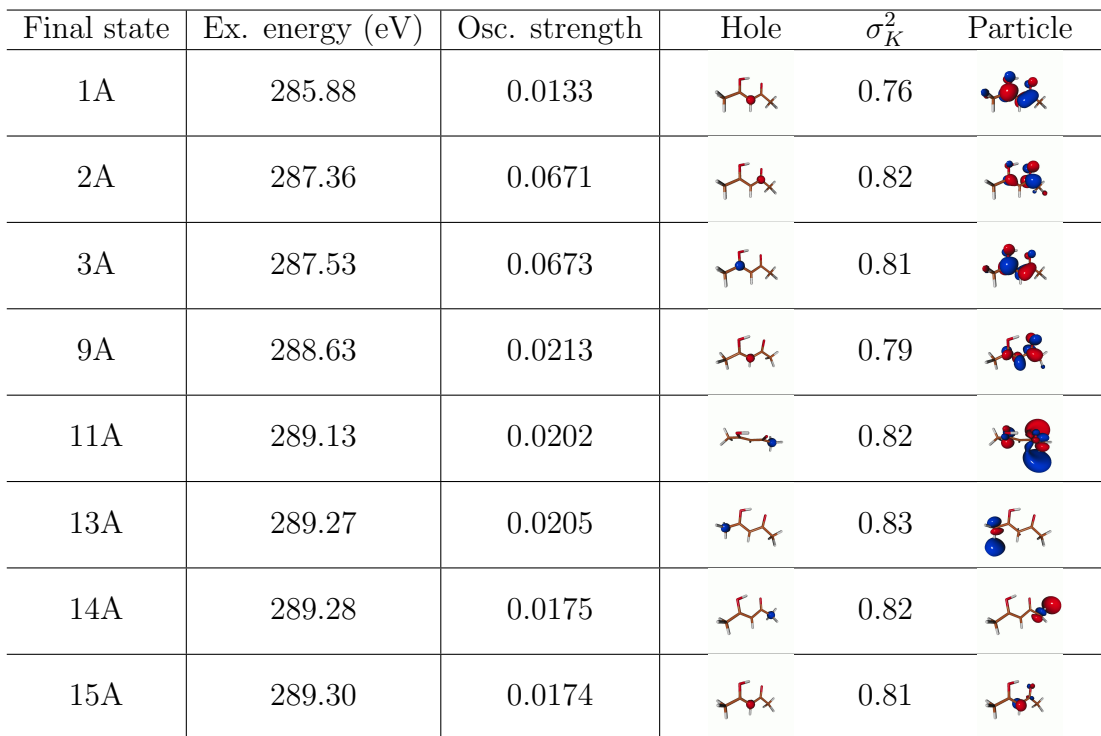 | 0.82         | 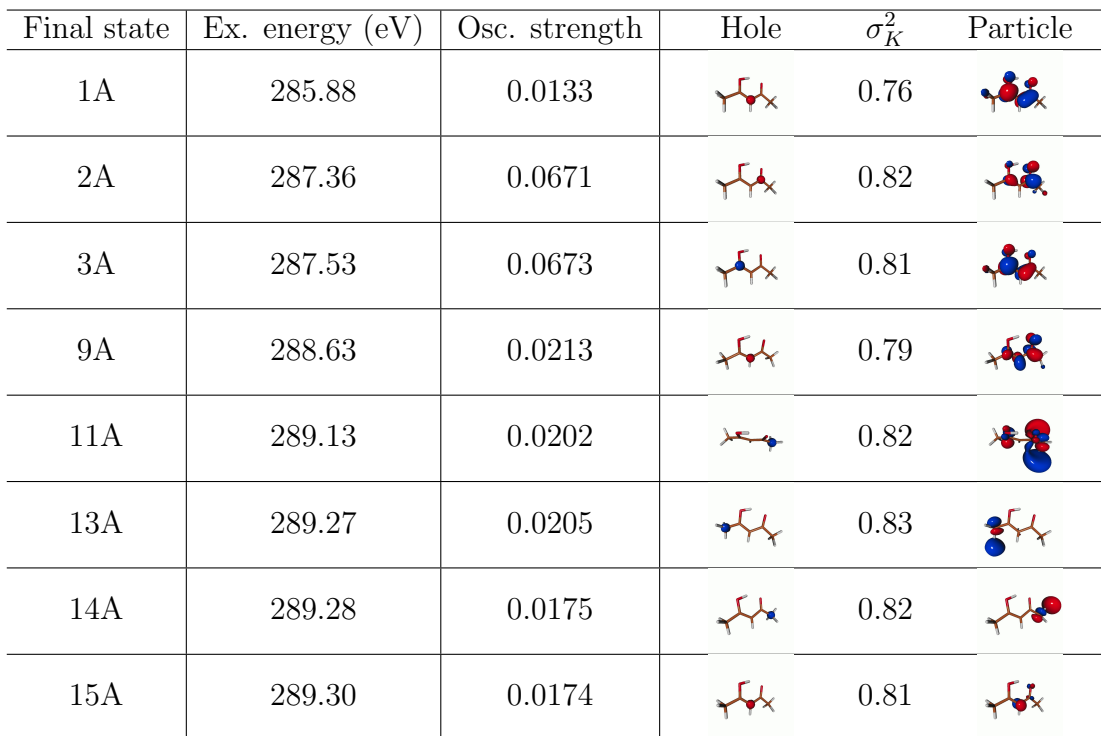 |
| 13A         | 289.27          | 0.0205        | 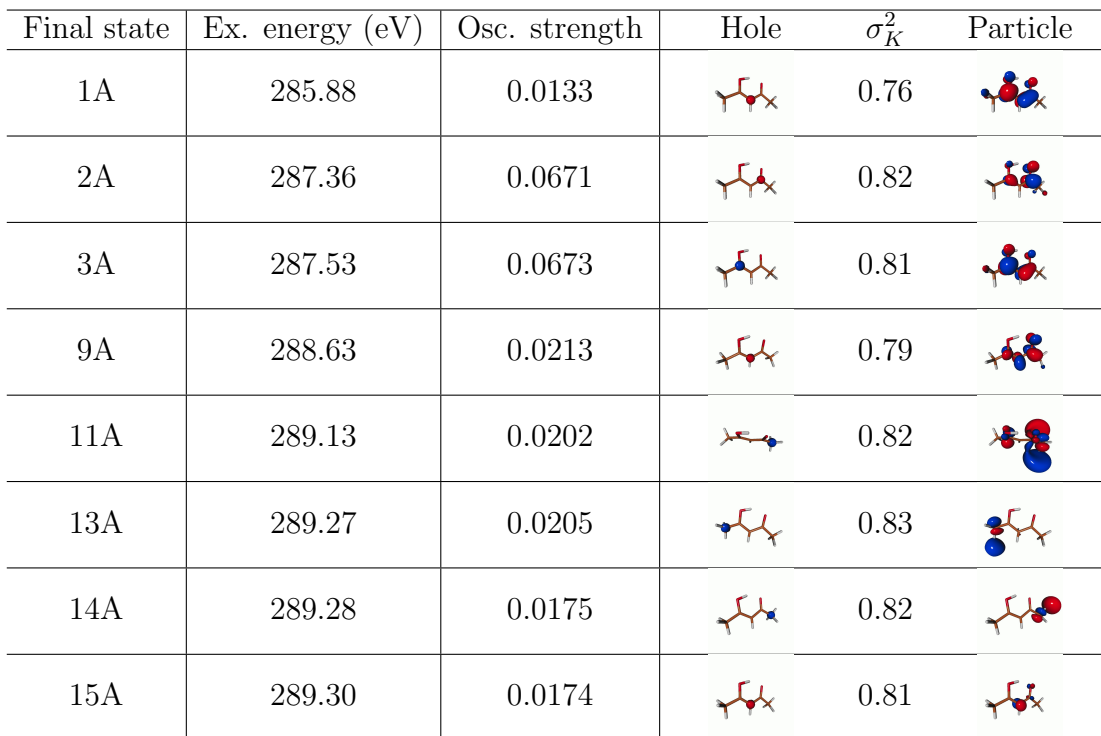 | 0.83         | 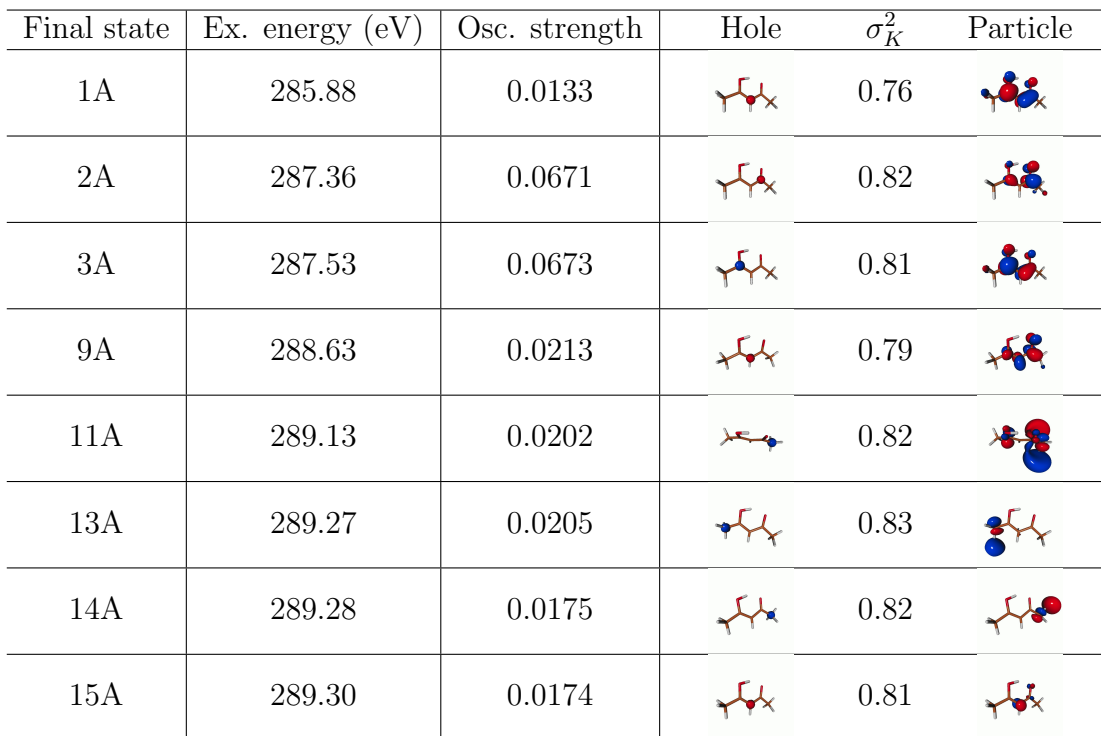 |
| 14A         | 289.28          | 0.0175        | 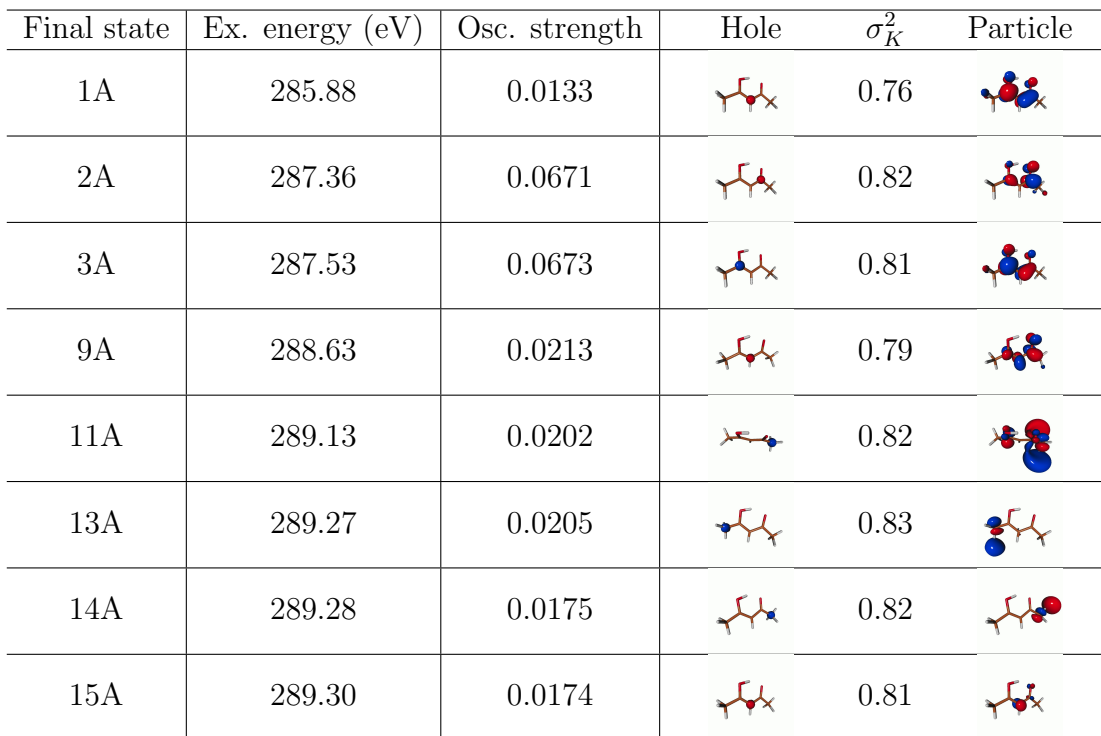 | 0.82         | 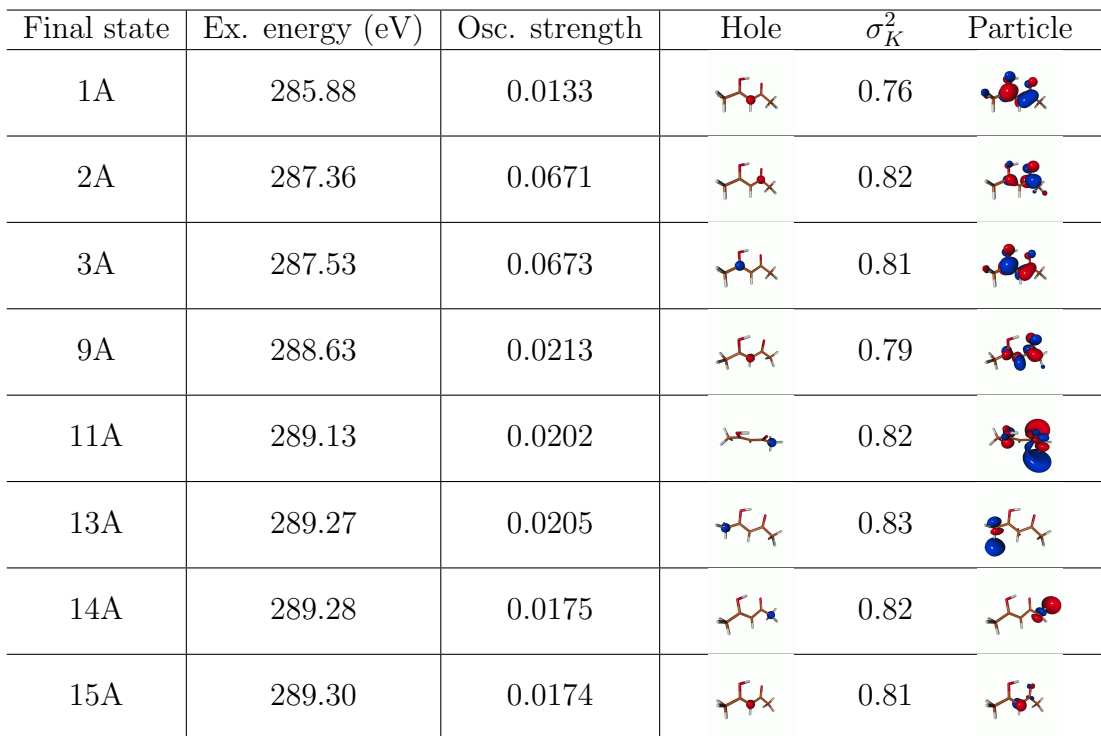 |
| 15A         | 289.30          | 0.0174        | 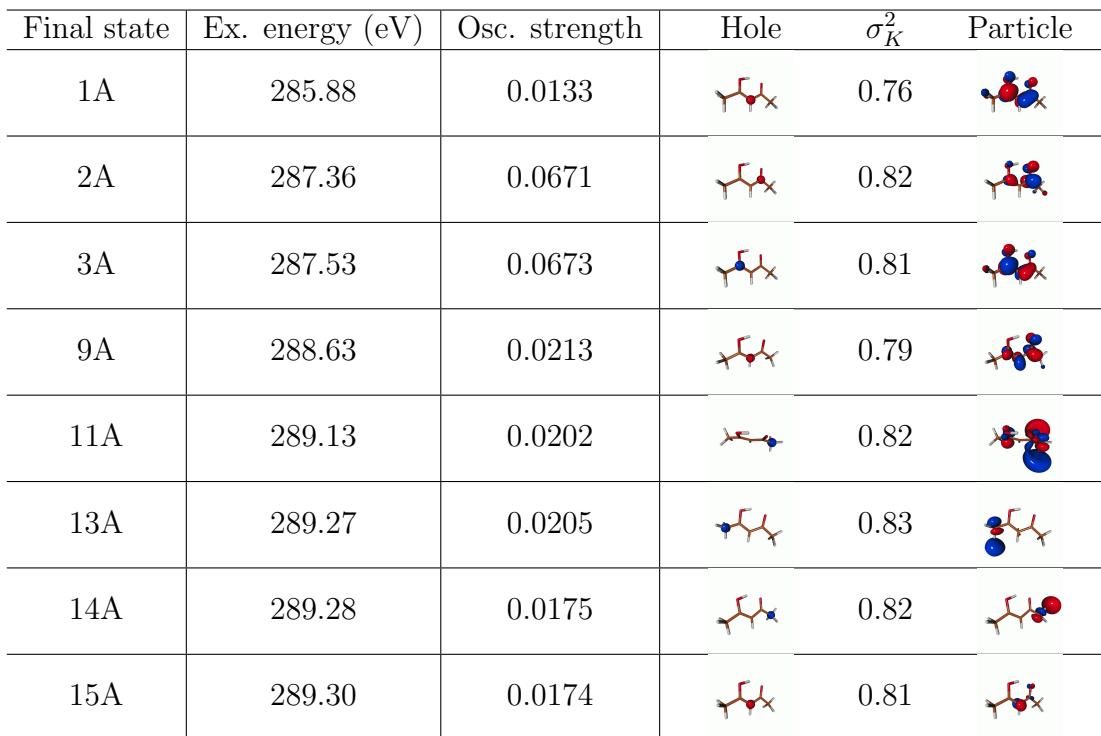 | 0.81         | 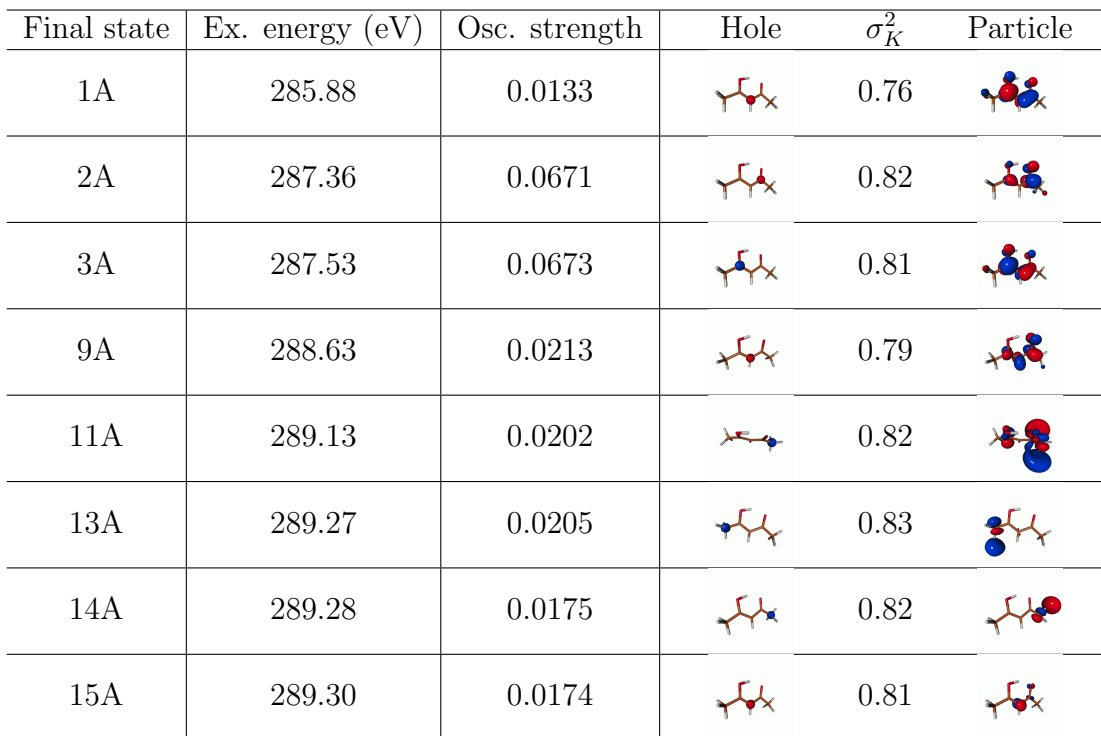 |

Table S8: Acetylacetone. CVS-ADC(2)/6-311++G\*\* NTOs of the  $C_{1s}$  core excitations from the ground state at the FC geometry (NTO isosurface is 0.05).

| Final state | Ex. energy (eV) | Osc. strength | Hole                                                                               | $\sigma_K^2$ | Particle                                                                            |
|-------------|-----------------|---------------|------------------------------------------------------------------------------------|--------------|-------------------------------------------------------------------------------------|
| 1A          | 288.23          | 0.0101        | 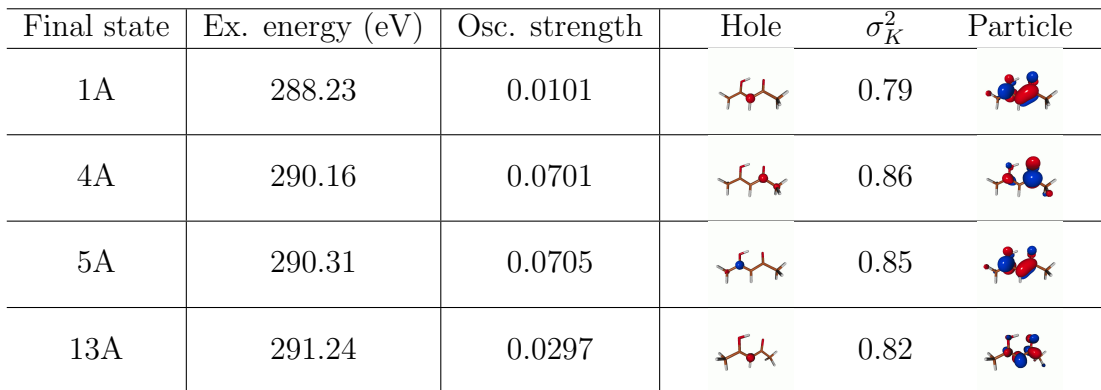 | 0.79         | 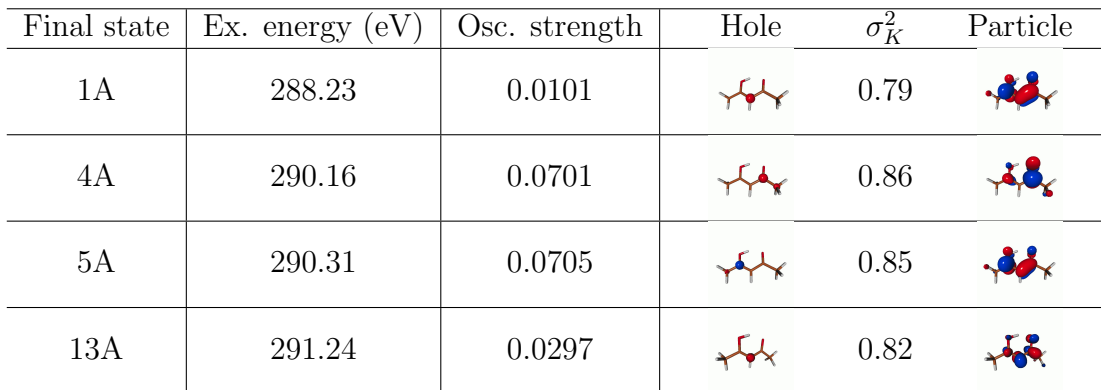 |
| 4A          | 290.16          | 0.0701        | 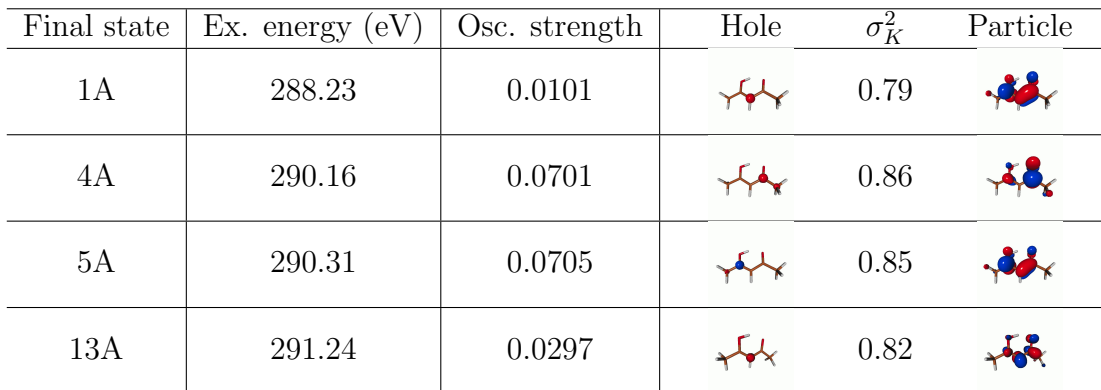 | 0.86         | 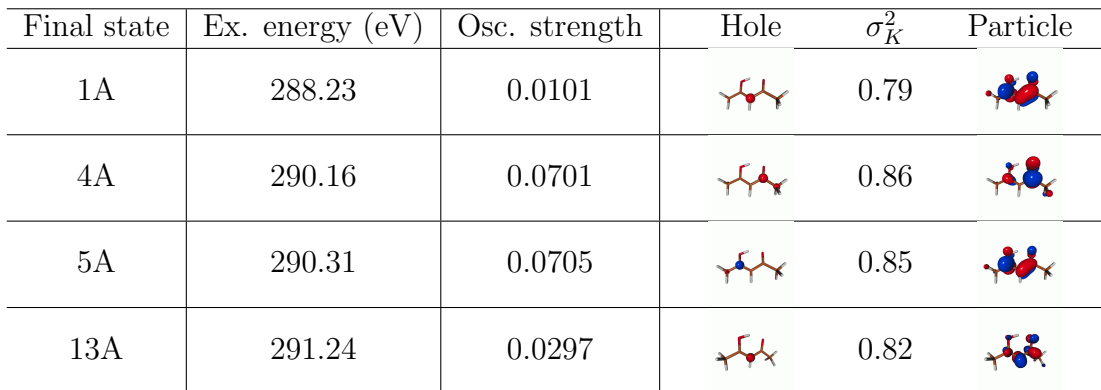 |
| 5A          | 290.31          | 0.0705        | 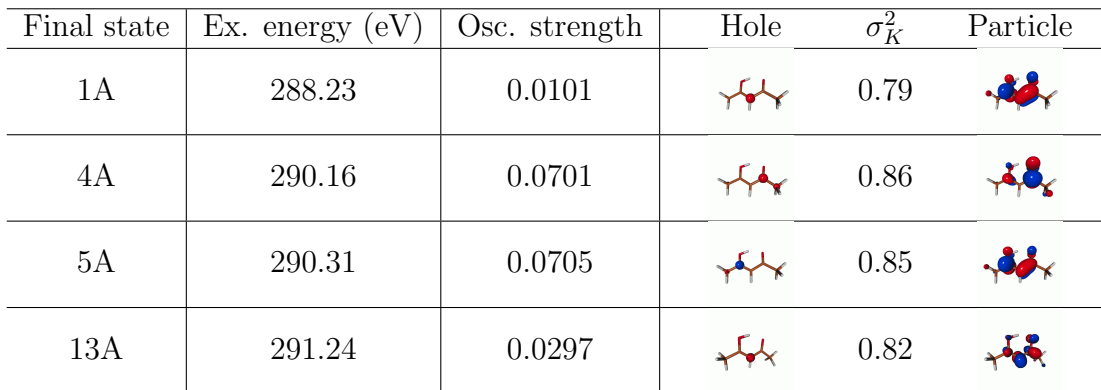 | 0.85         | 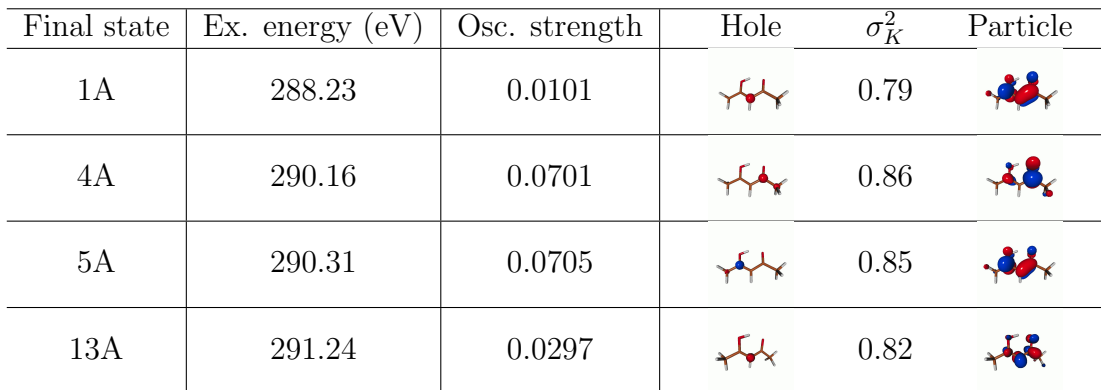 |
| 13A         | 291.24          | 0.0297        | 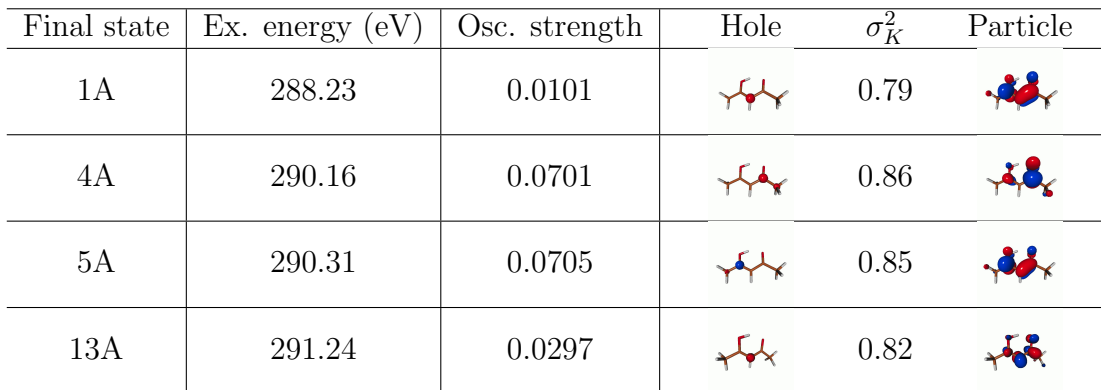 | 0.82         | 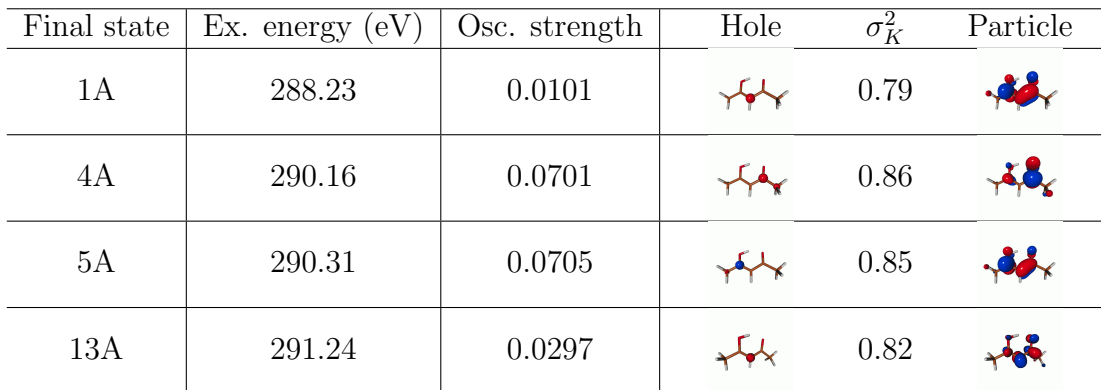 |

Table S9: Acetylacetone. TDDFT/B3LYP/6-311++G\*\* NTOs of the  $C_{1s}$  core excitations from the ground state at the FC geometry (NTO isosurface is 0.03 for the Rydberg transition and 0.05 for the others).

| Final state | Ex. energy (eV) | Osc. strength | Hole                                                                                 | $\sigma_K^2$ | Particle                                                                              |
|-------------|-----------------|---------------|--------------------------------------------------------------------------------------|--------------|---------------------------------------------------------------------------------------|
| 1A          | 273.63          | 0.0037        | 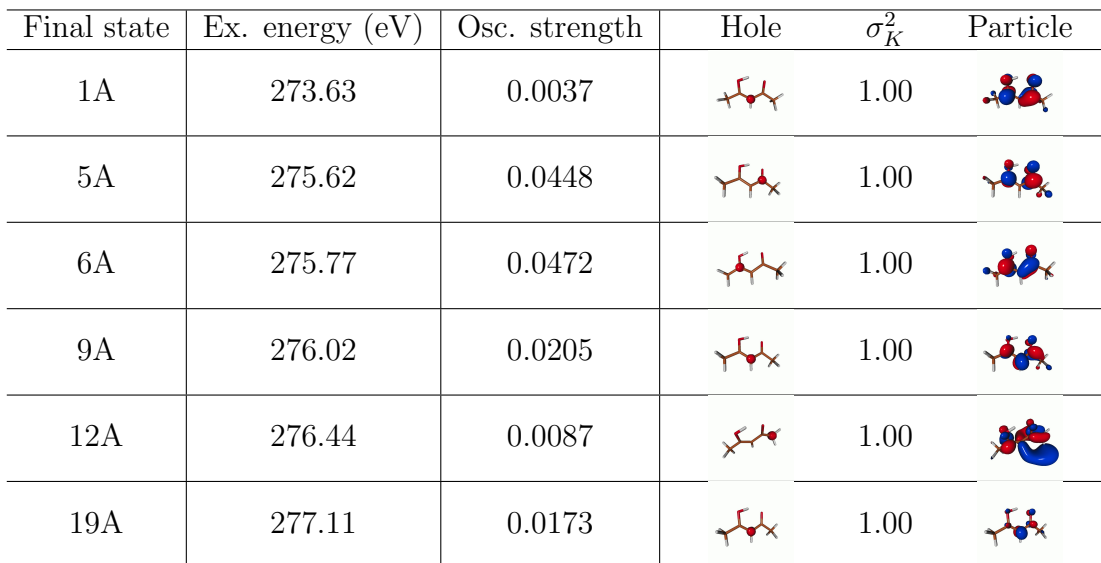 | 1.00         | 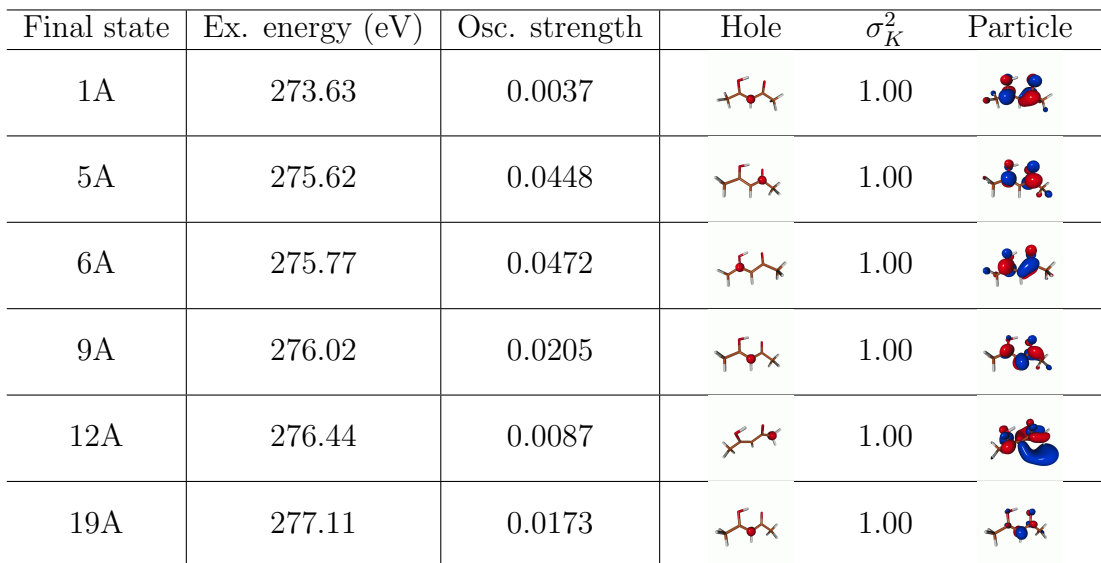 |
| 5A          | 275.62          | 0.0448        | 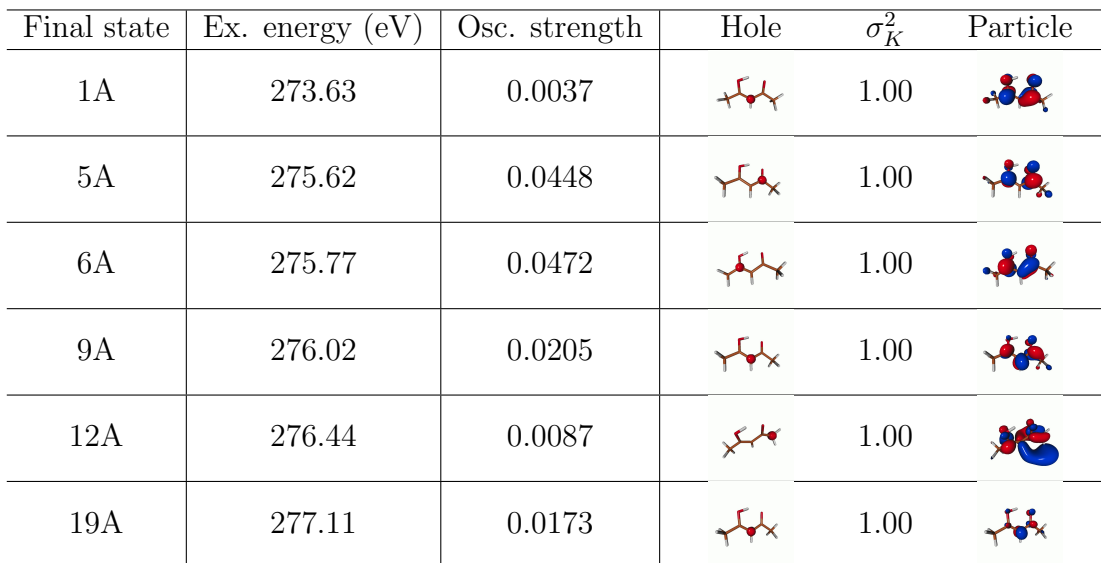 | 1.00         | 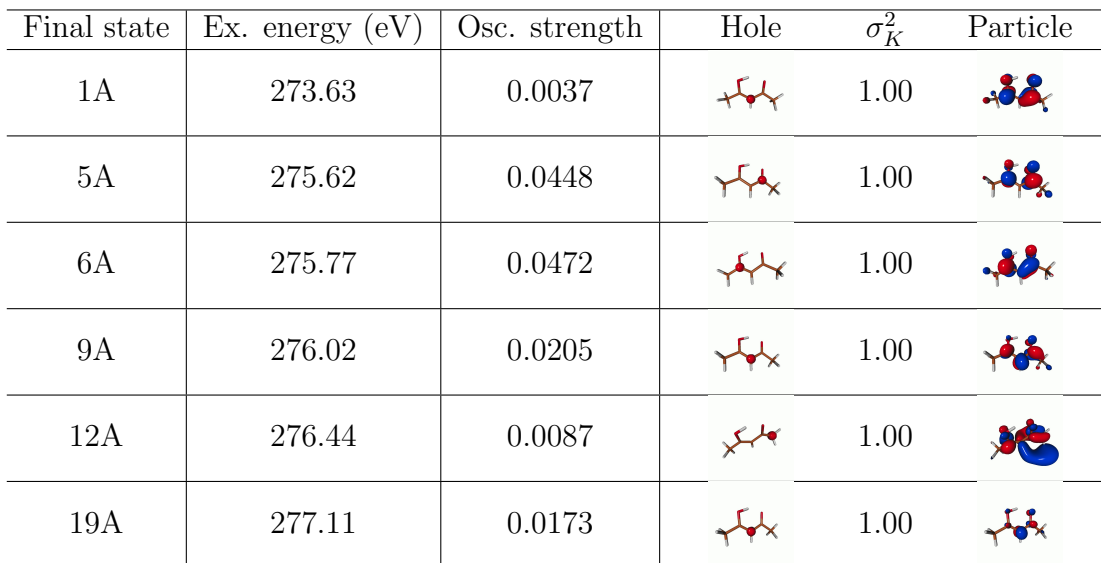 |
| 6A          | 275.77          | 0.0472        | 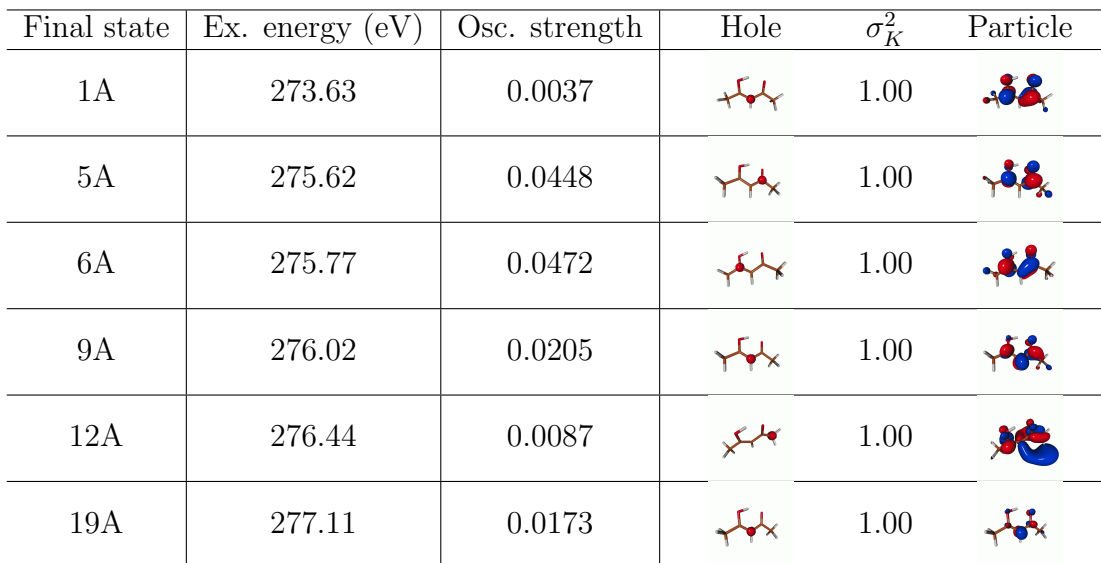 | 1.00         | 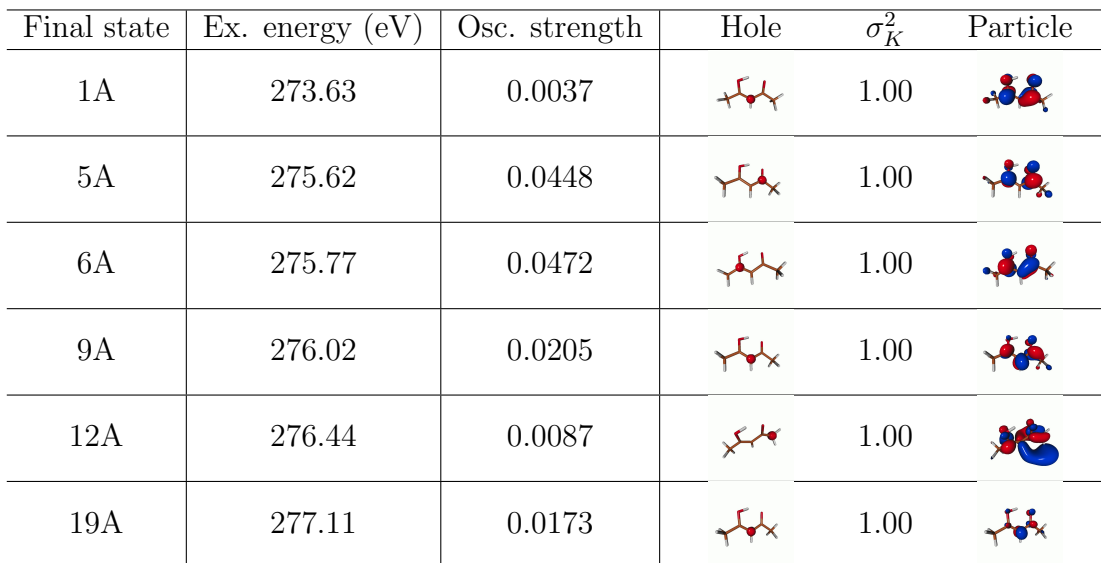 |
| 9A          | 276.02          | 0.0205        | 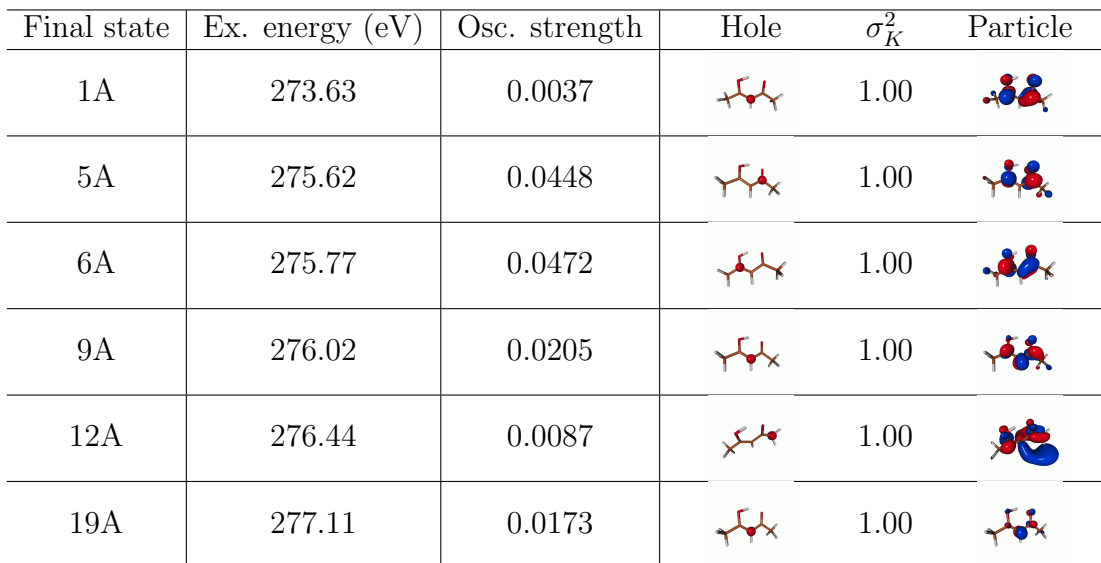 | 1.00         | 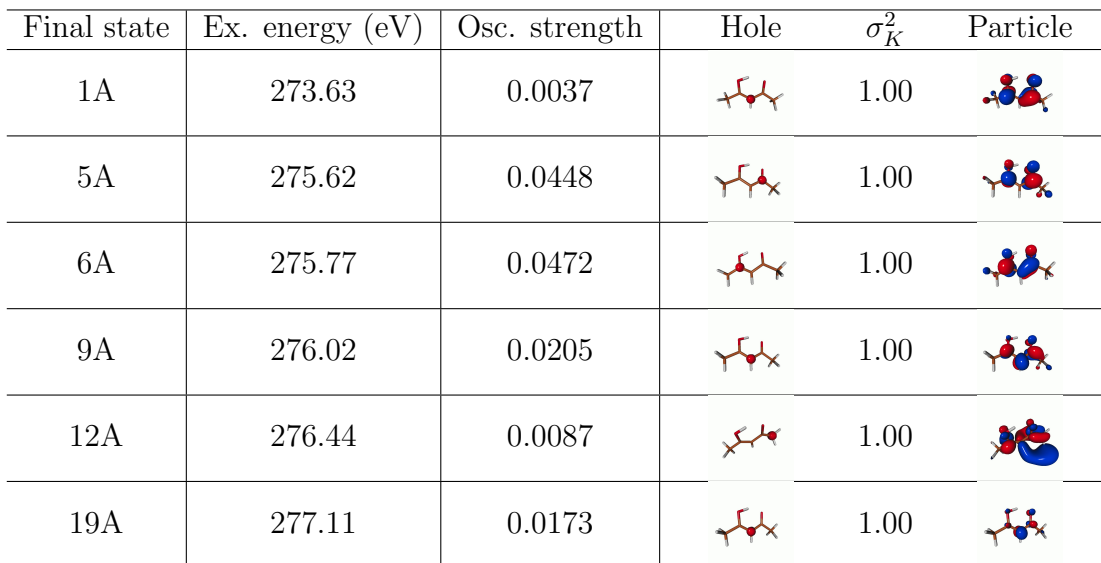 |
| 12A         | 276.44          | 0.0087        | 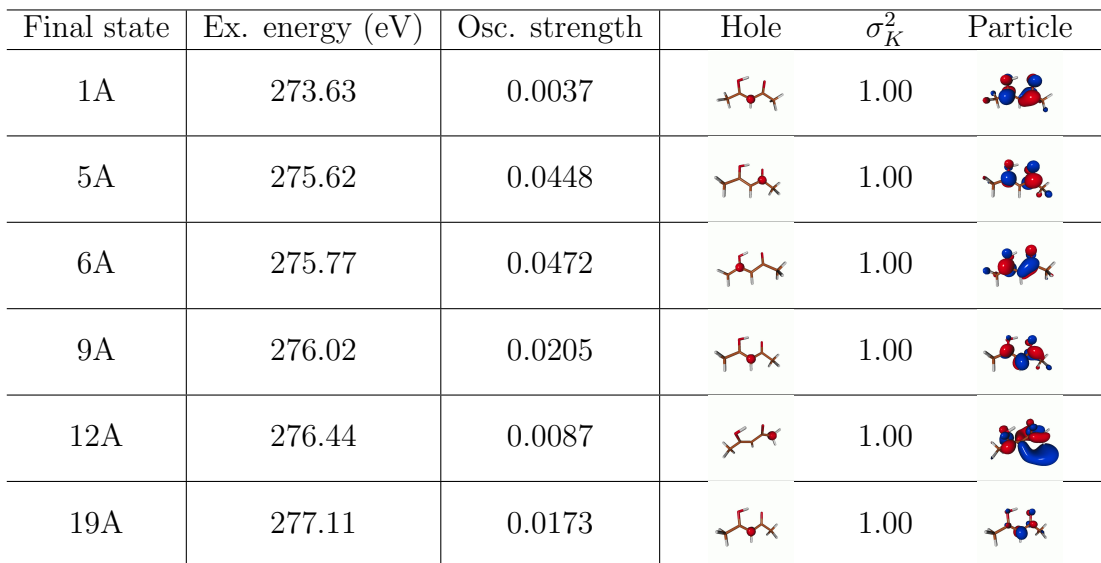 | 1.00         | 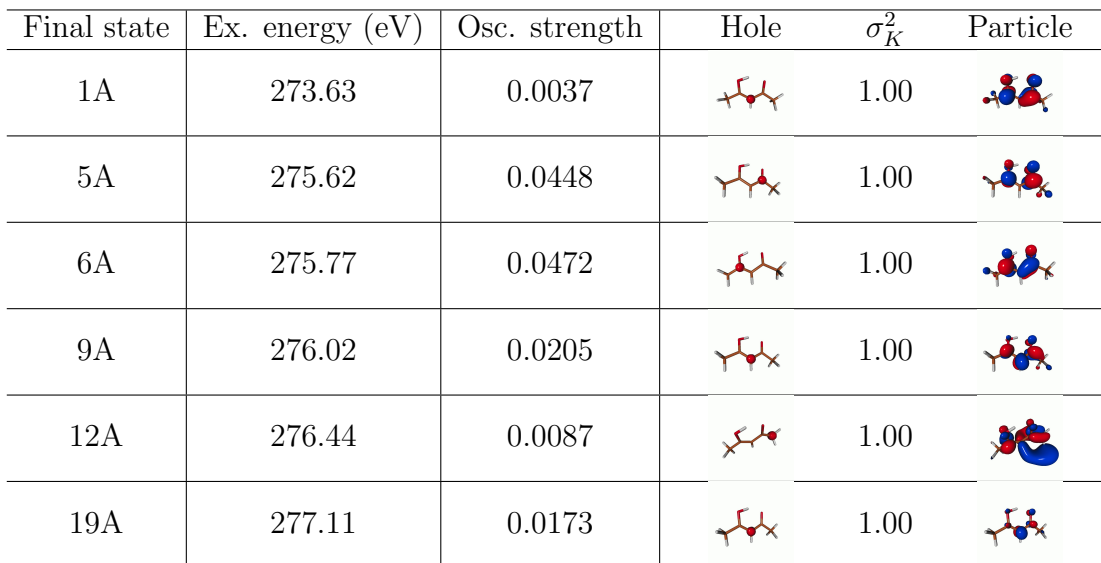 |
| 19A         | 277.11          | 0.0173        | 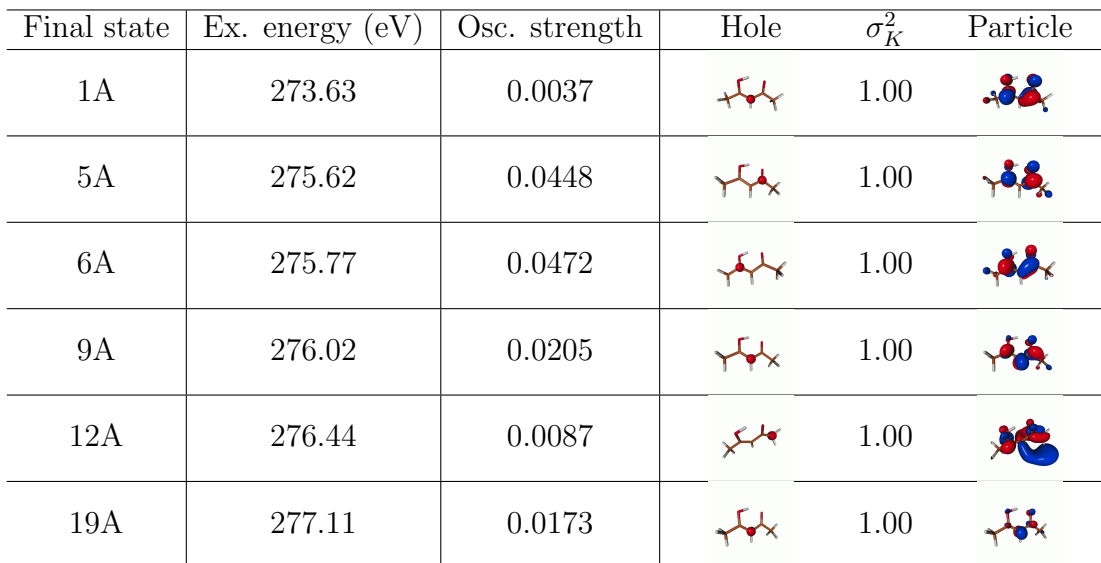 | 1.00         | 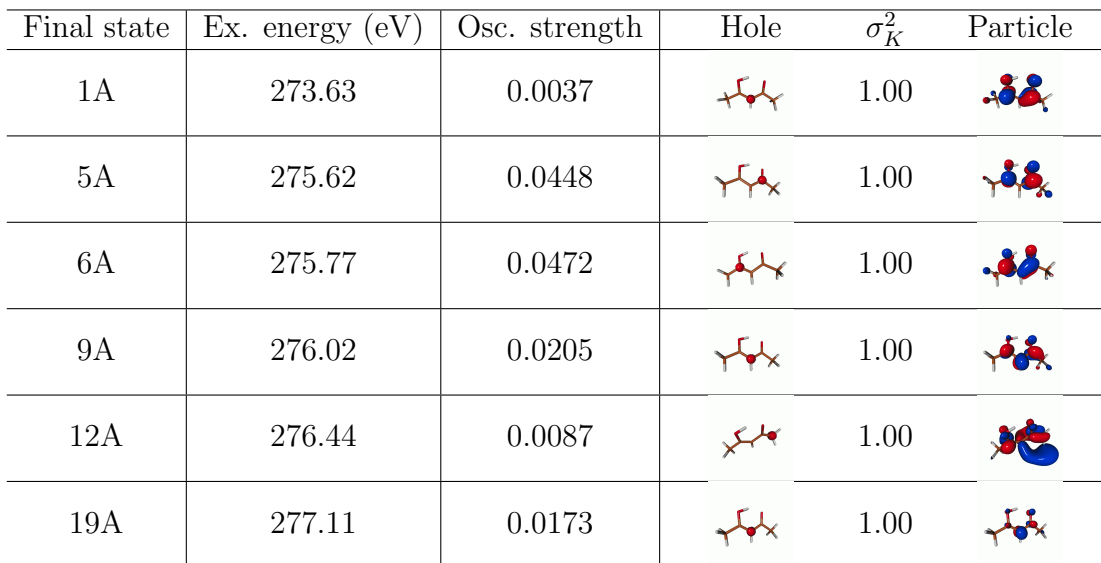 |

## S2 Natural transition orbitals of valence excitations

Table S10: Uracil. EOM-EE-CCSD/6-311++G\*\* NTOs of the excitations from the ground state to the lowest-lying valence-excited states at the FC geometry (NTO isosurface is 0.05).

| Final state         | Ex. energy (eV) | Osc. strength | Hole                                                                                 | $\sigma_K^2$ | Particle                                                                              |
|---------------------|-----------------|---------------|--------------------------------------------------------------------------------------|--------------|---------------------------------------------------------------------------------------|
| $T_1(A', \pi\pi^*)$ | 3.84            | -             | 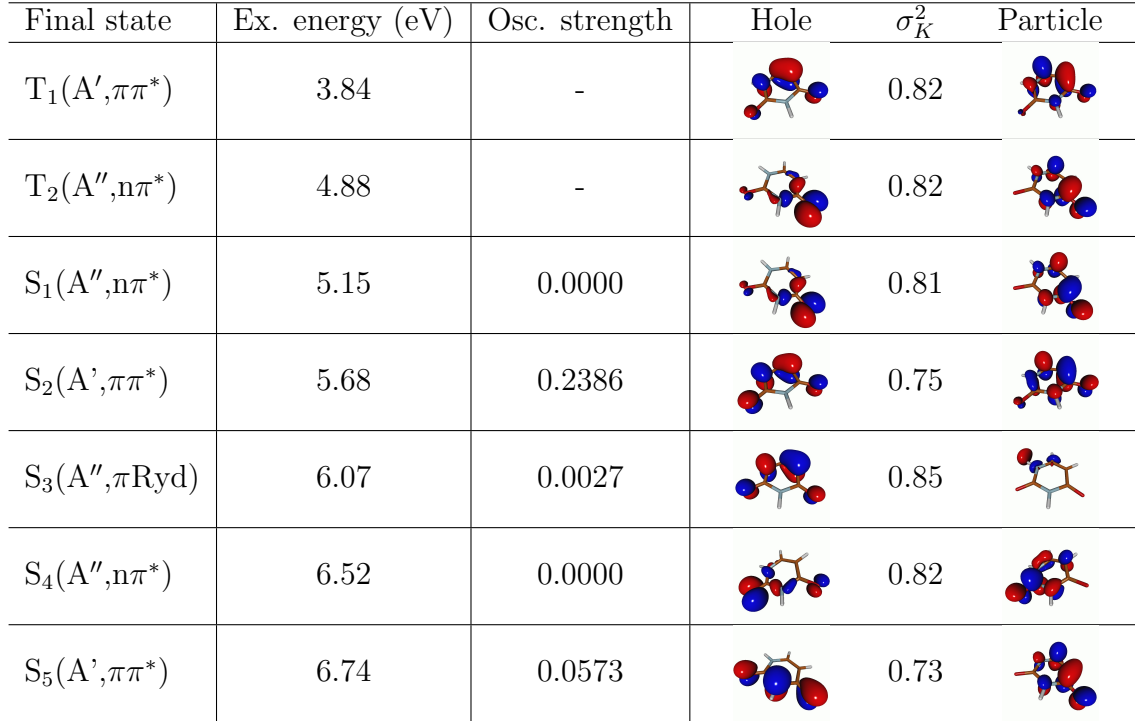   | 0.82         | 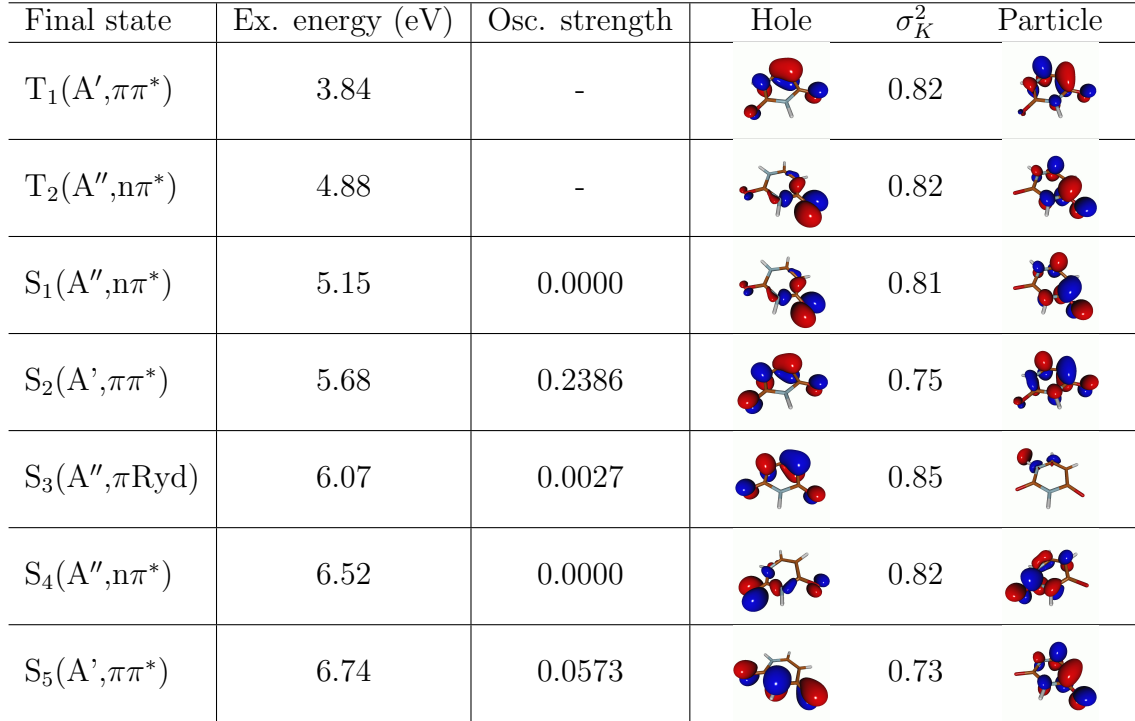   |
| $T_2(A'', n\pi^*)$  | 4.88            | -             | 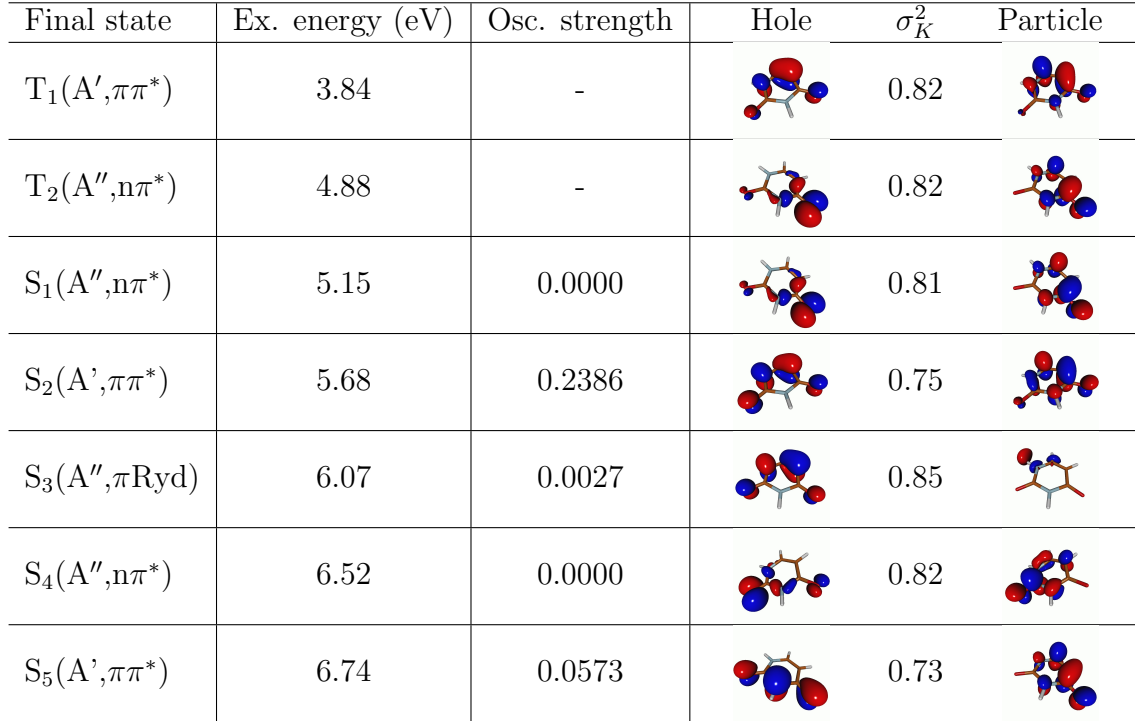   | 0.82         | 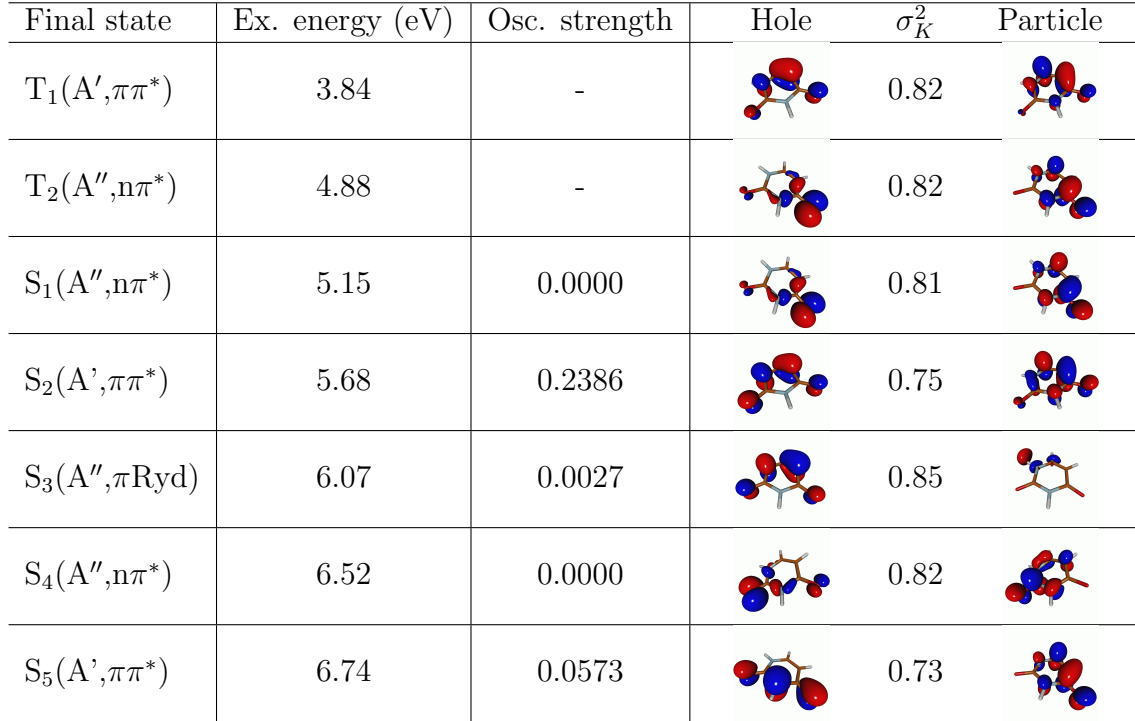   |
| $S_1(A'', n\pi^*)$  | 5.15            | 0.0000        | 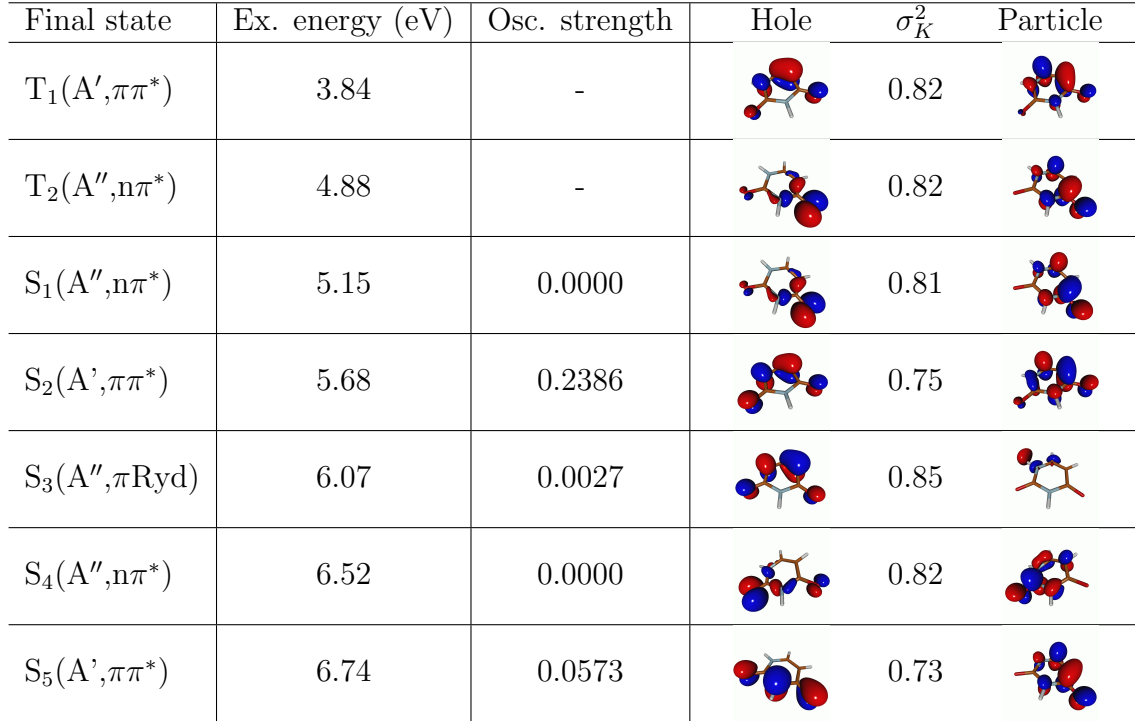   | 0.81         | 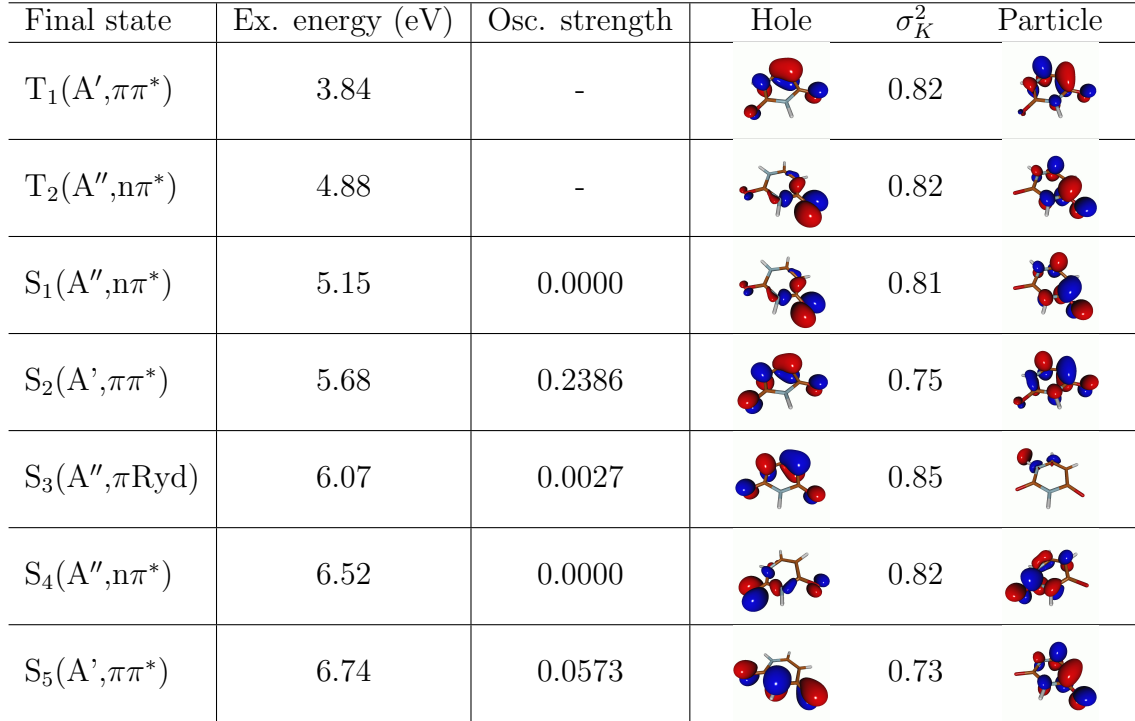   |
| $S_2(A', \pi\pi^*)$ | 5.68            | 0.2386        | 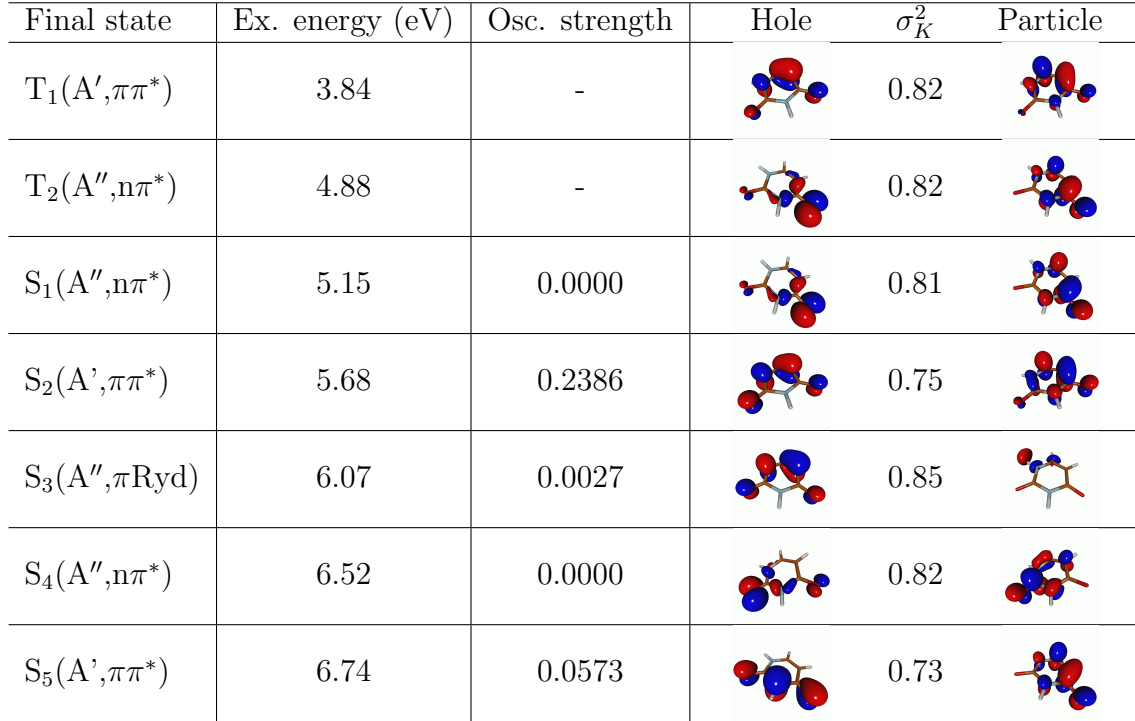   | 0.75         | 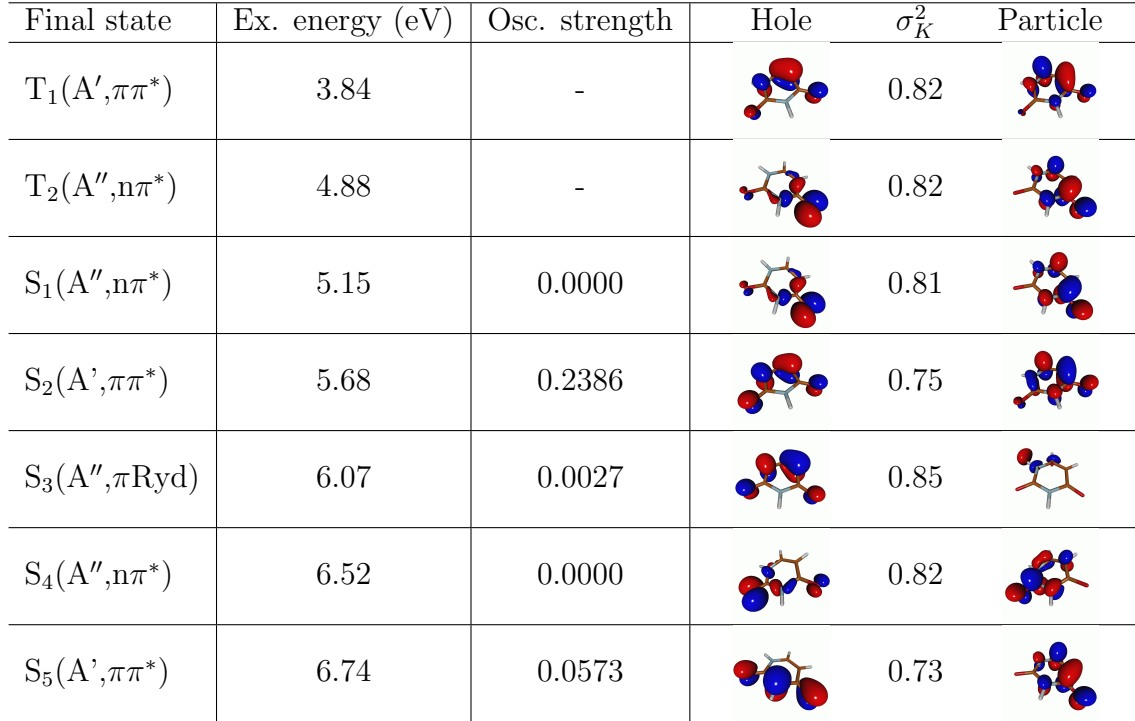   |
| $S_3(A'', \pi Ryd)$ | 6.07            | 0.0027        | 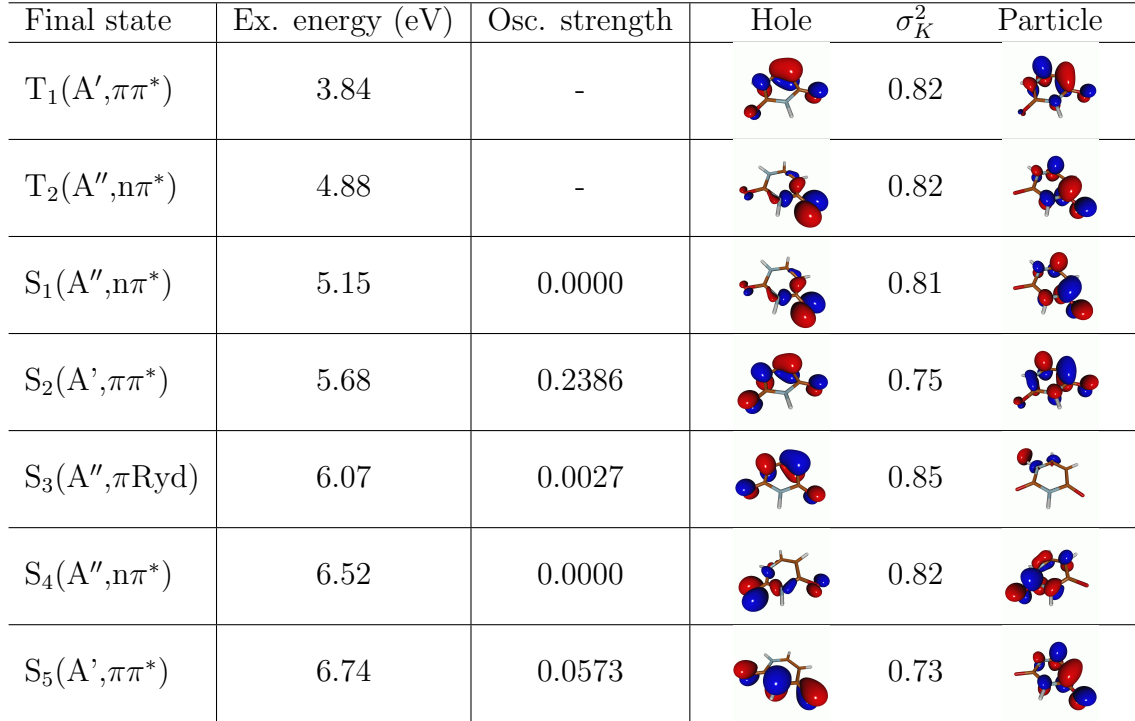   | 0.85         | 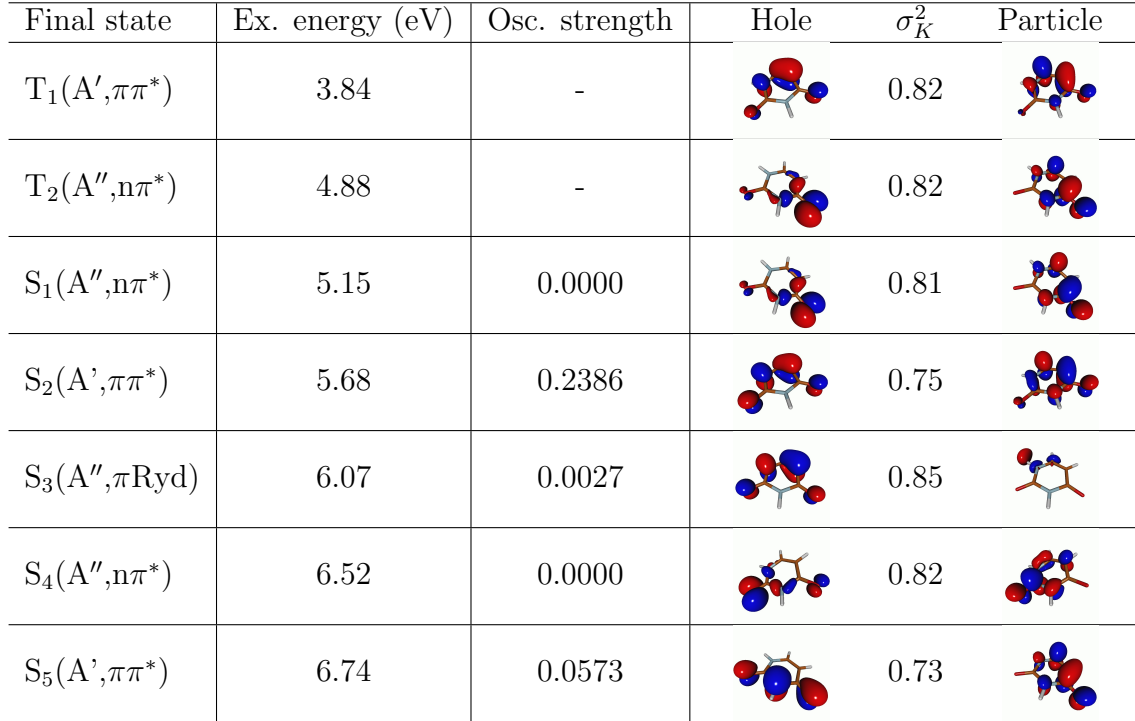   |
| $S_4(A'', n\pi^*)$  | 6.52            | 0.0000        | 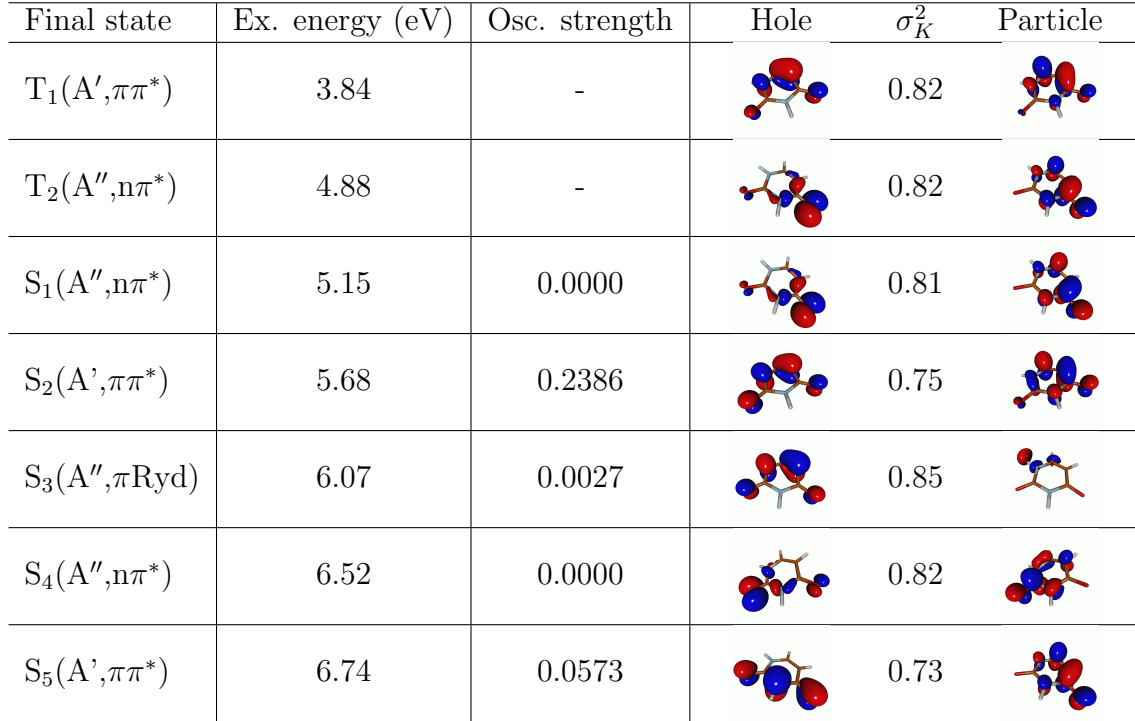  | 0.82         | 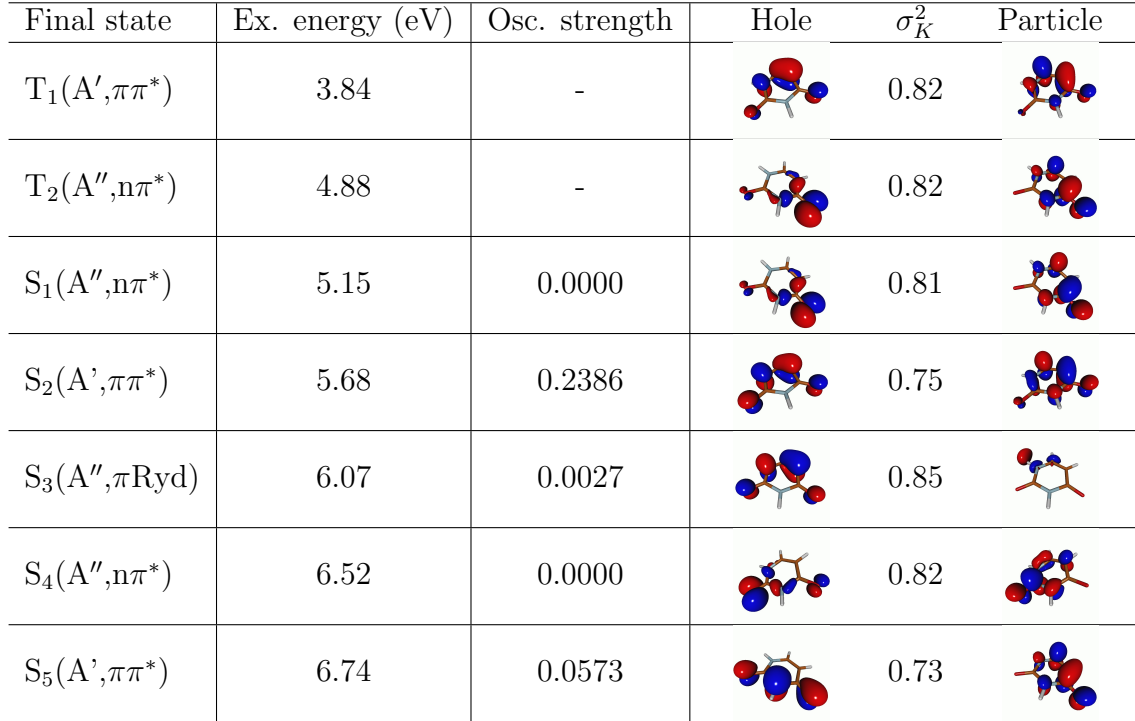  |
| $S_5(A', \pi\pi^*)$ | 6.74            | 0.0573        | 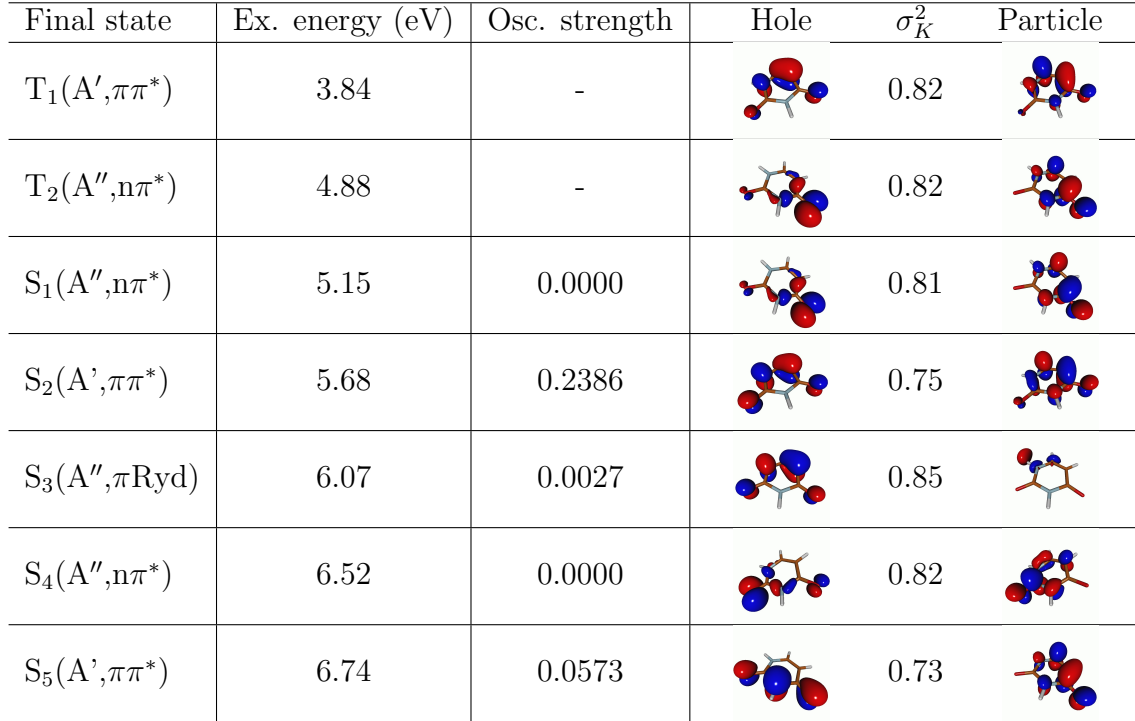 | 0.73         | 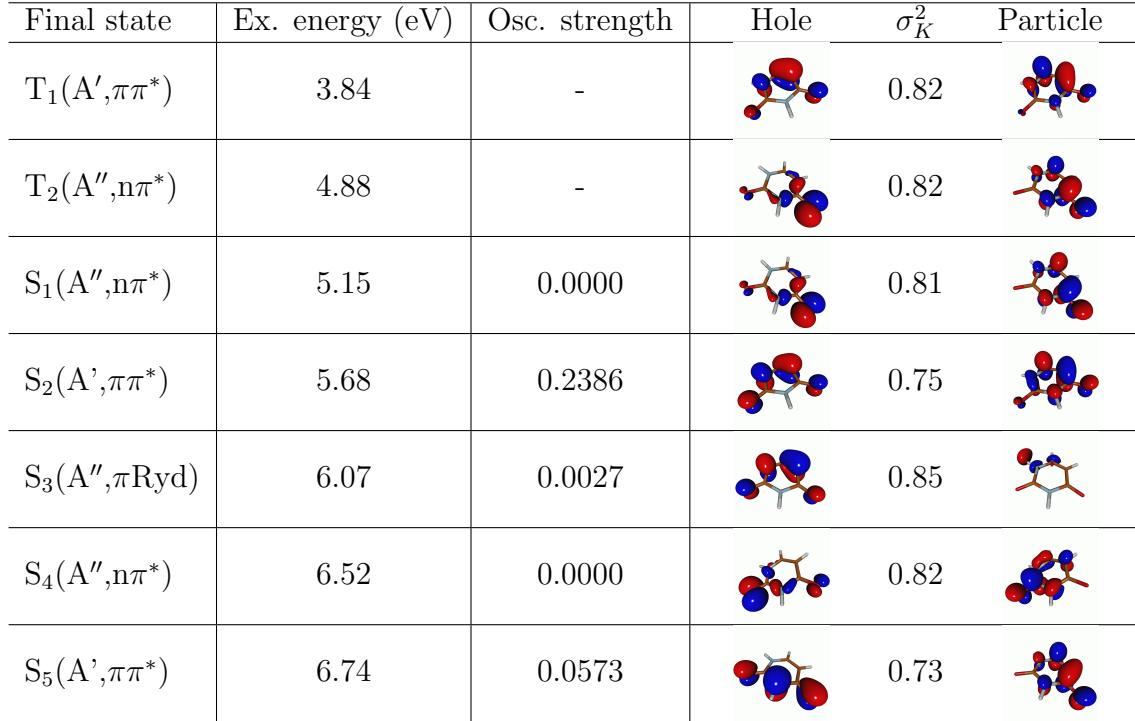 |

Table S11: Uracil. ADC(2)/6-311++G\*\* NTOs of the excitations from the ground state to the lowest-lying valence-excited states at the FC geometry (NTO isosurface is 0.05).

| Final state         | Ex. energy (eV) | Osc. strength | Hole                                                                                 | $\sigma_K^2$ | Particle                                                                              |
|---------------------|-----------------|---------------|--------------------------------------------------------------------------------------|--------------|---------------------------------------------------------------------------------------|
| $T_1(A', \pi\pi^*)$ | 3.91            | -             | 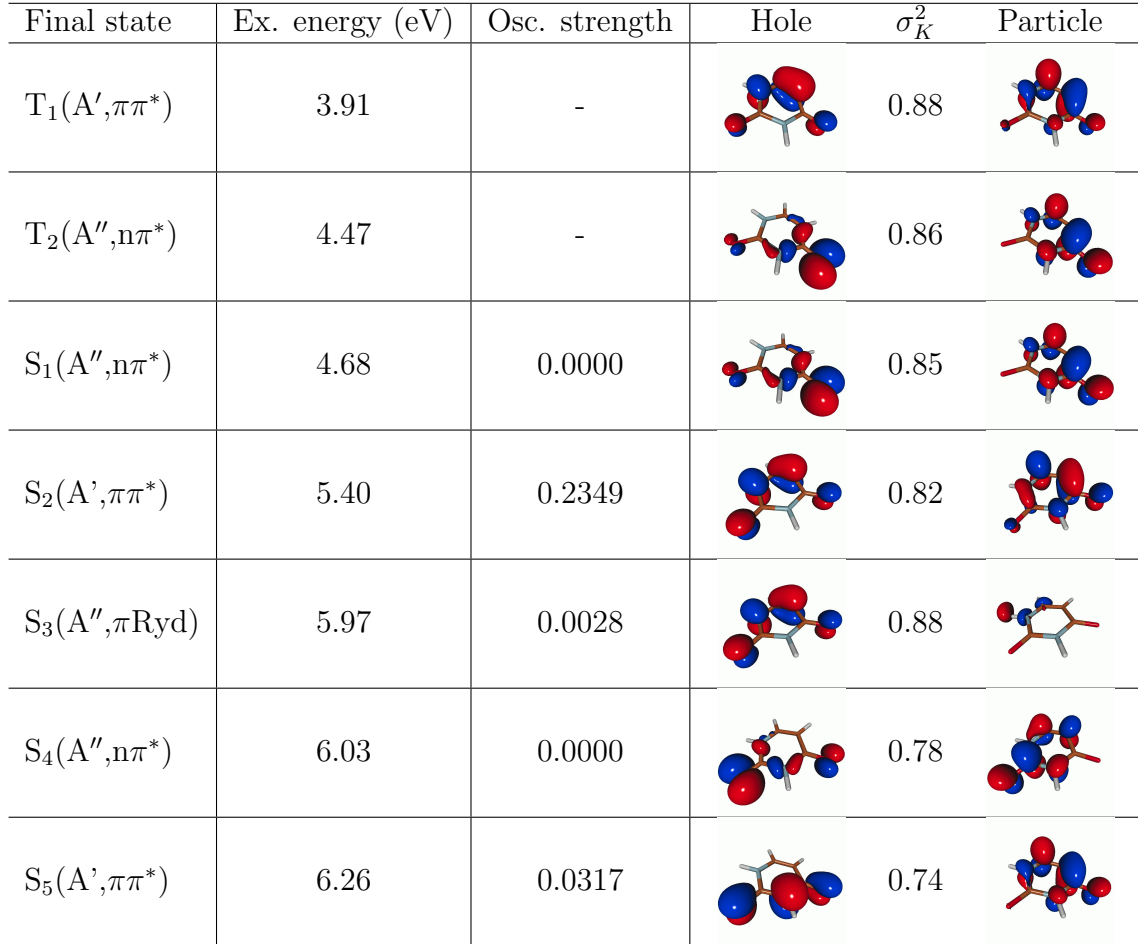   | 0.88         | 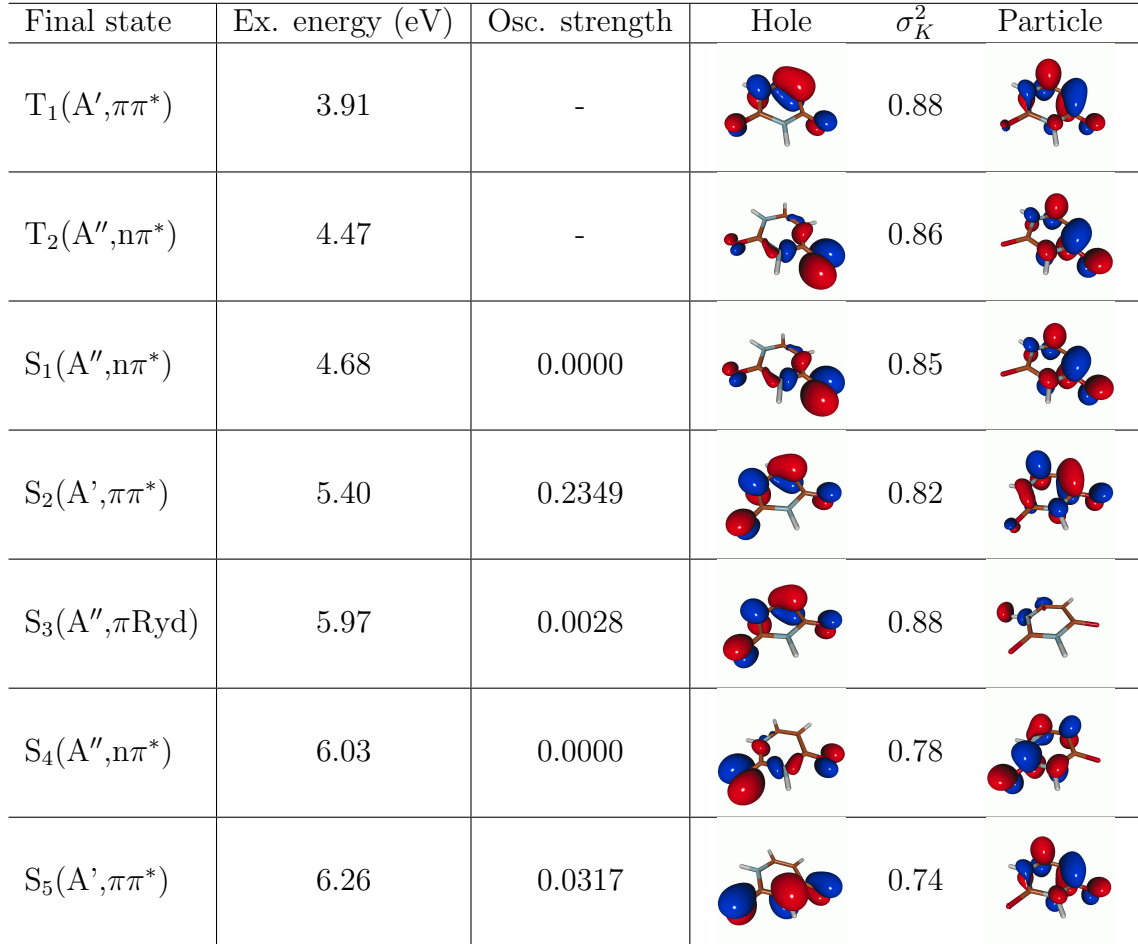   |
| $T_2(A'', n\pi^*)$  | 4.47            | -             | 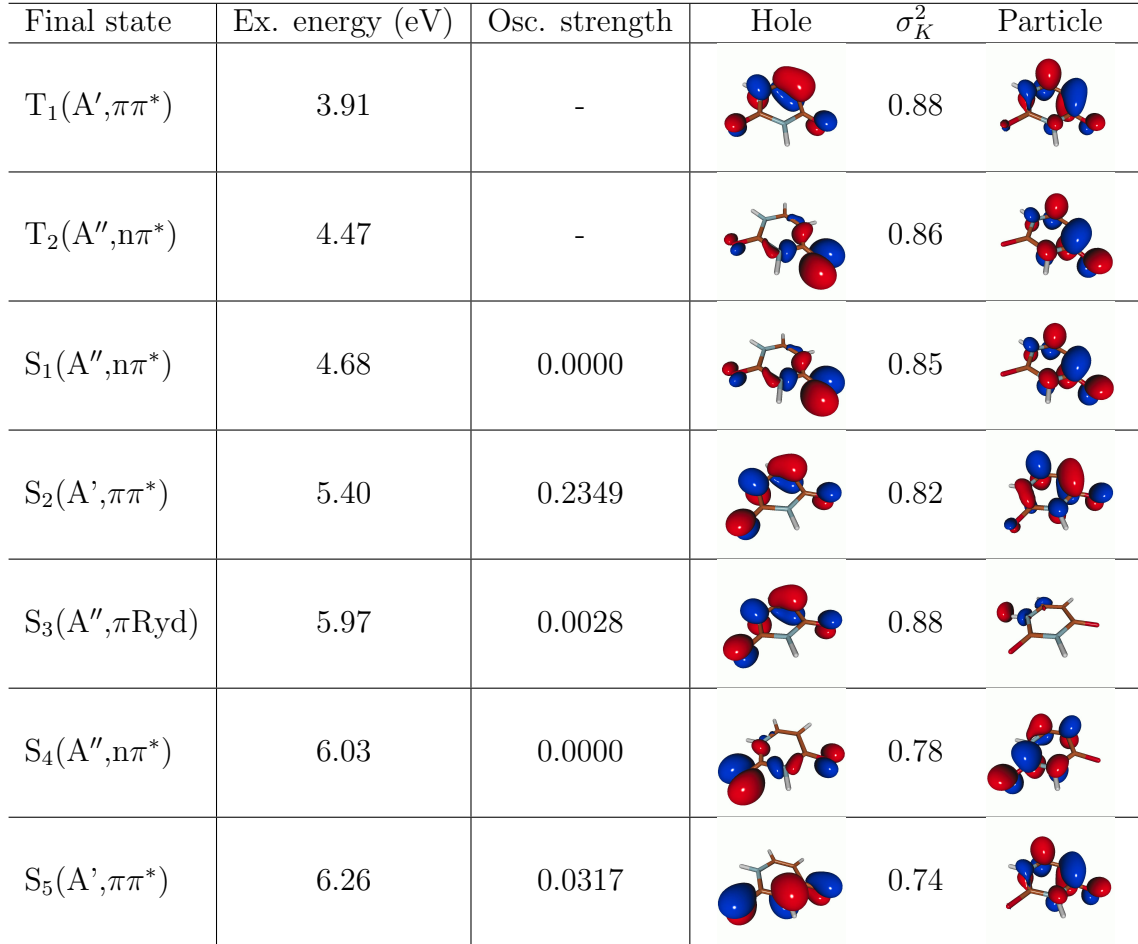   | 0.86         | 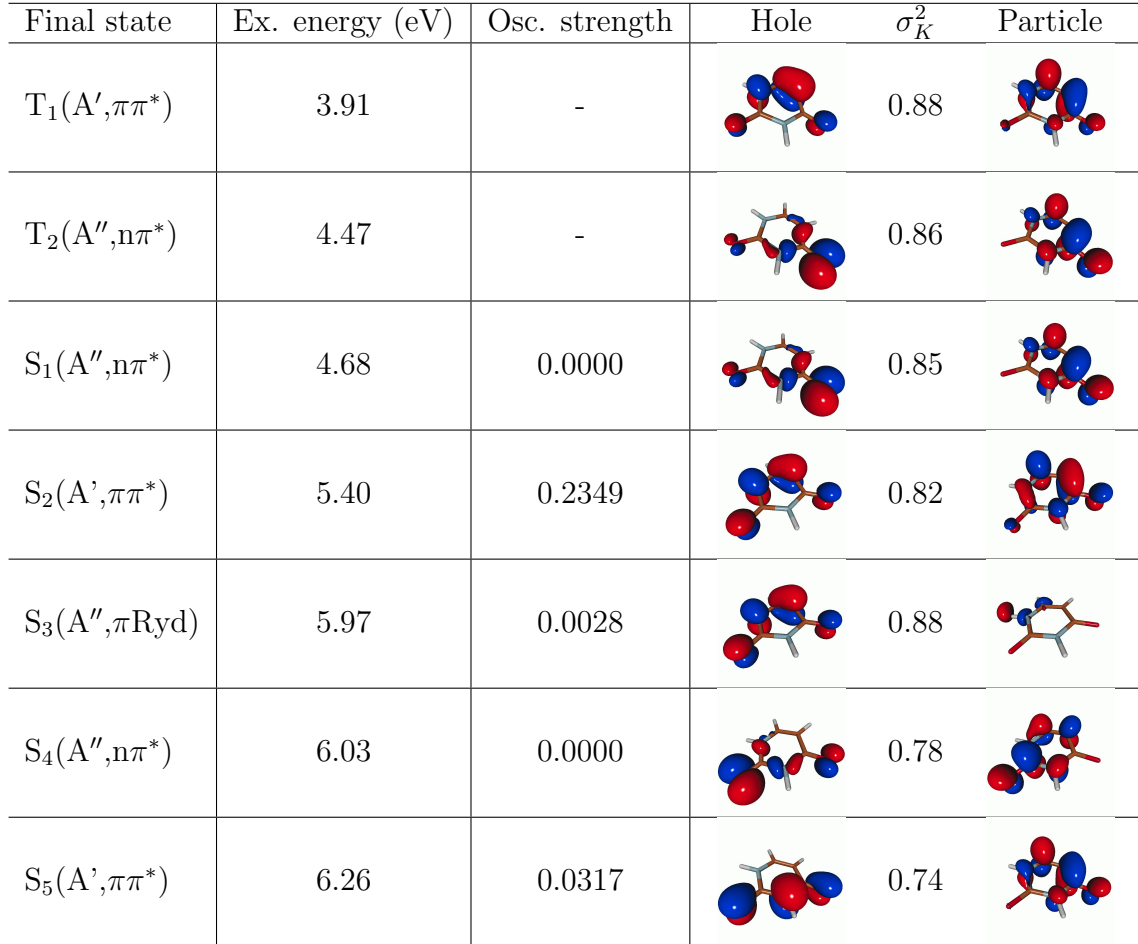   |
| $S_1(A'', n\pi^*)$  | 4.68            | 0.0000        | 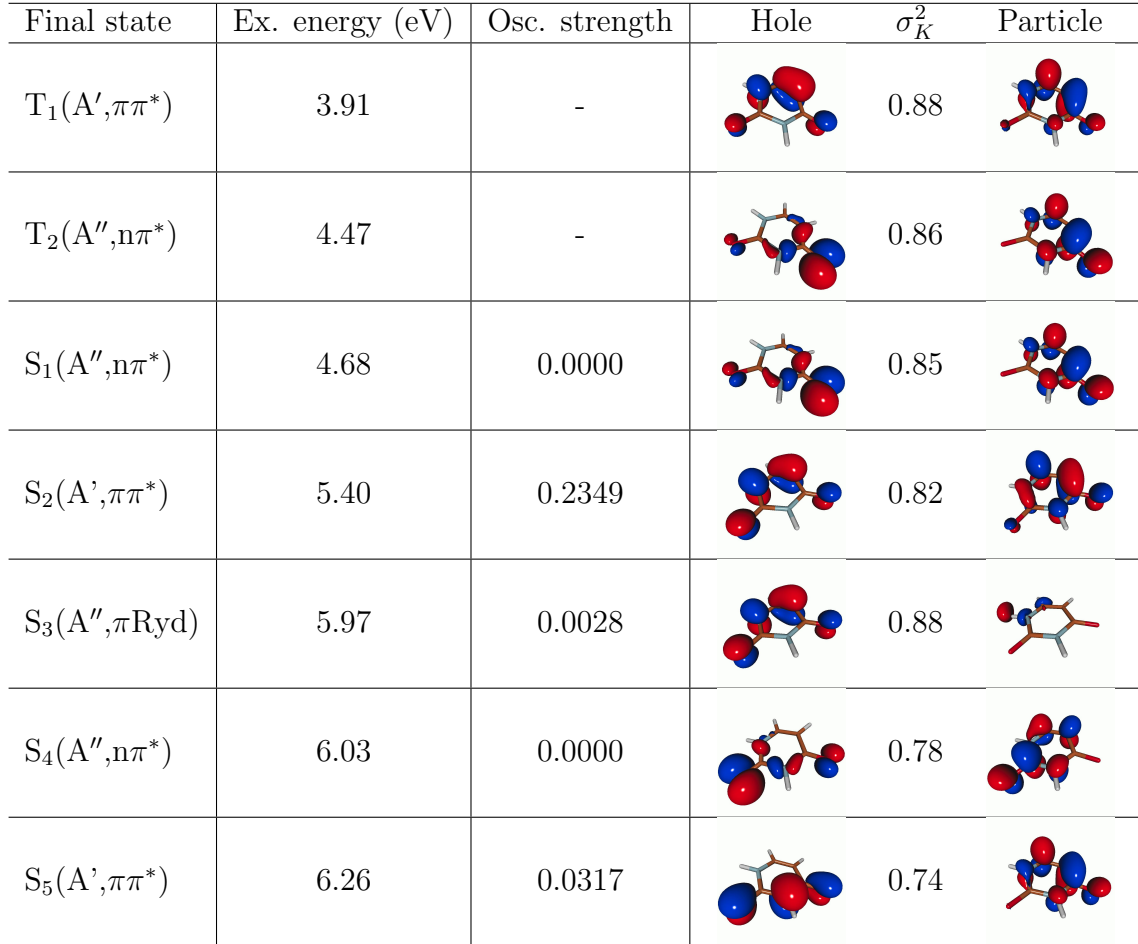  | 0.85         | 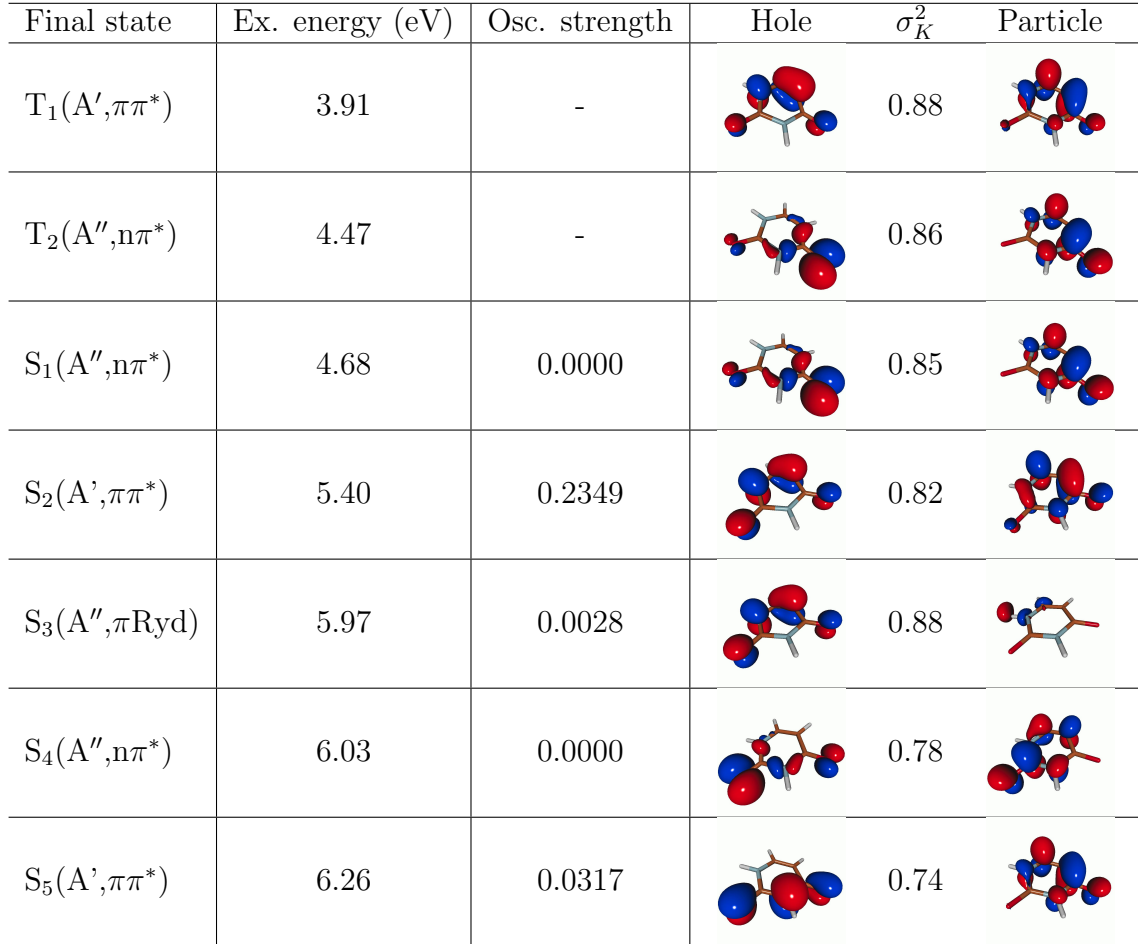  |
| $S_2(A', \pi\pi^*)$ | 5.40            | 0.2349        | 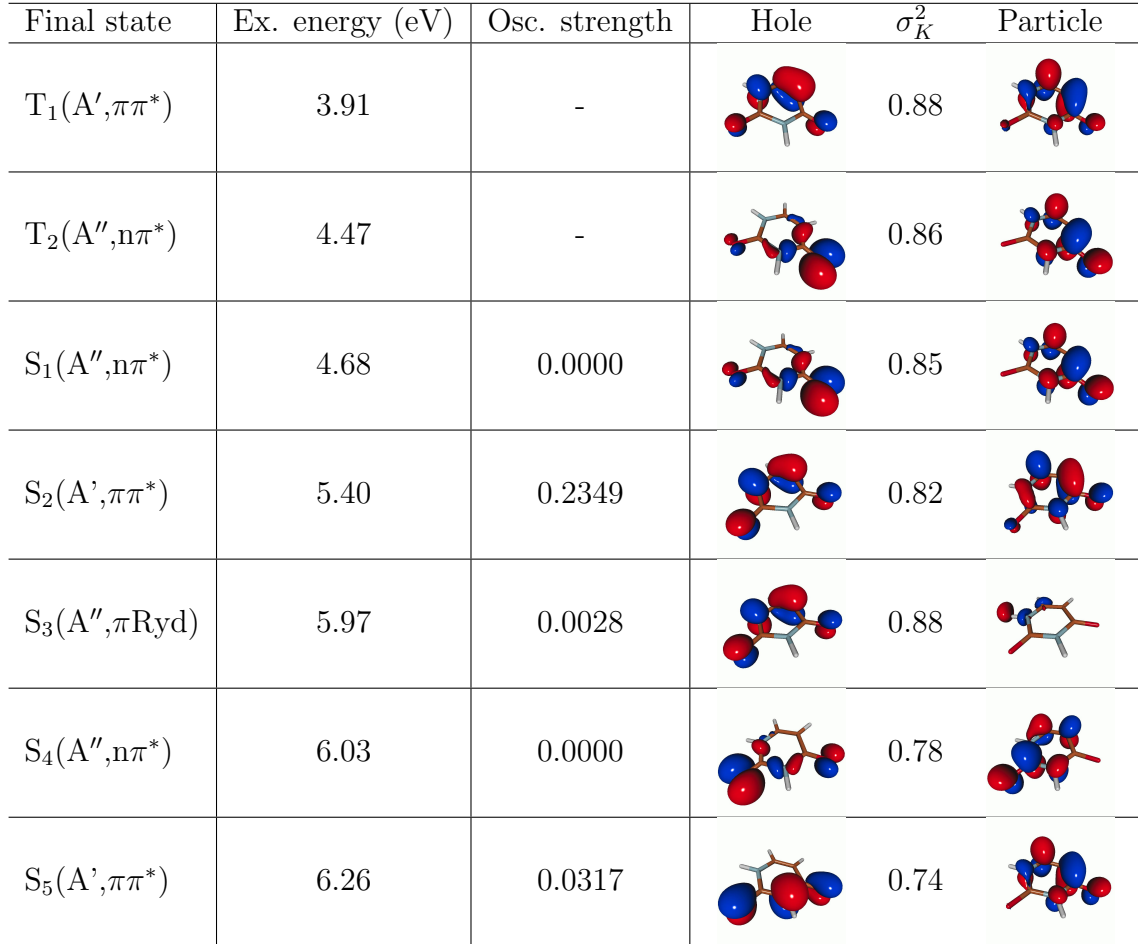 | 0.82         | 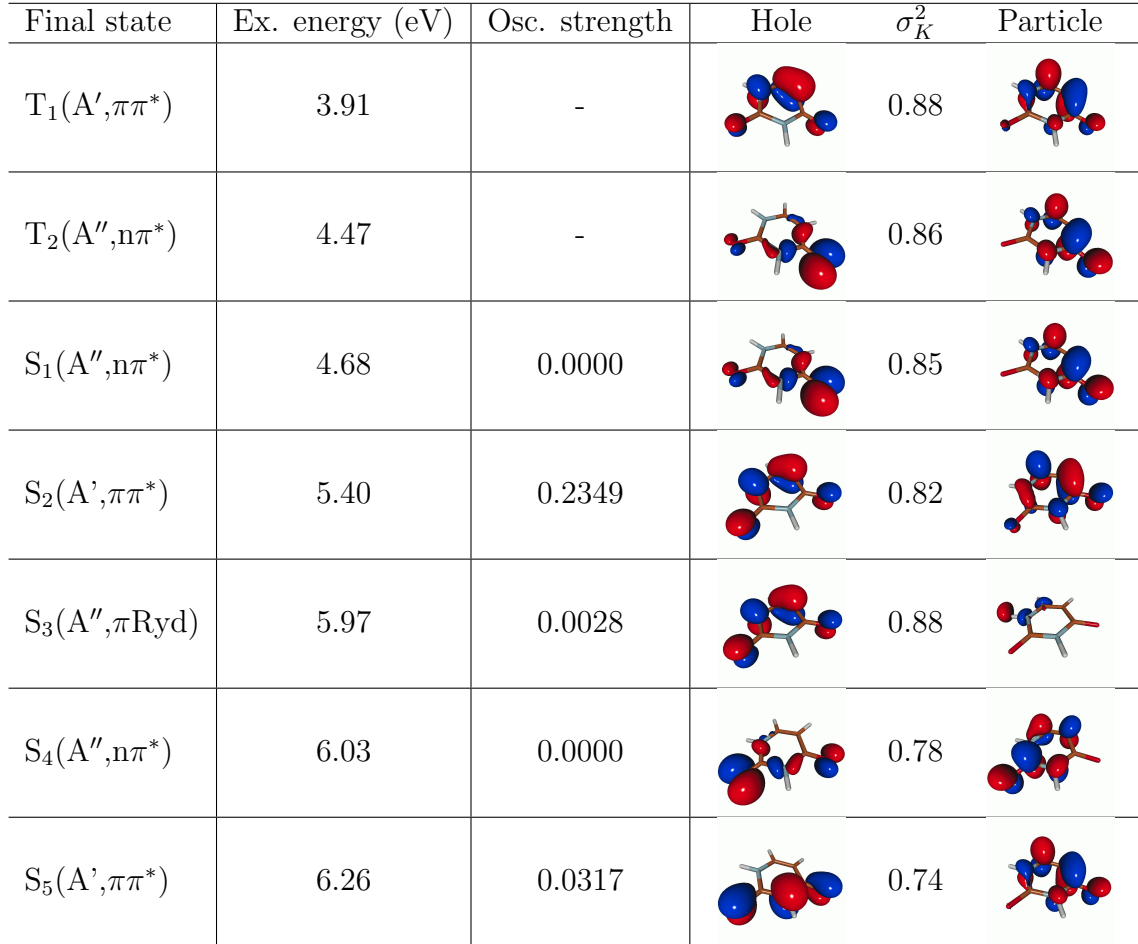 |
| $S_3(A'', \pi Ryd)$ | 5.97            | 0.0028        | 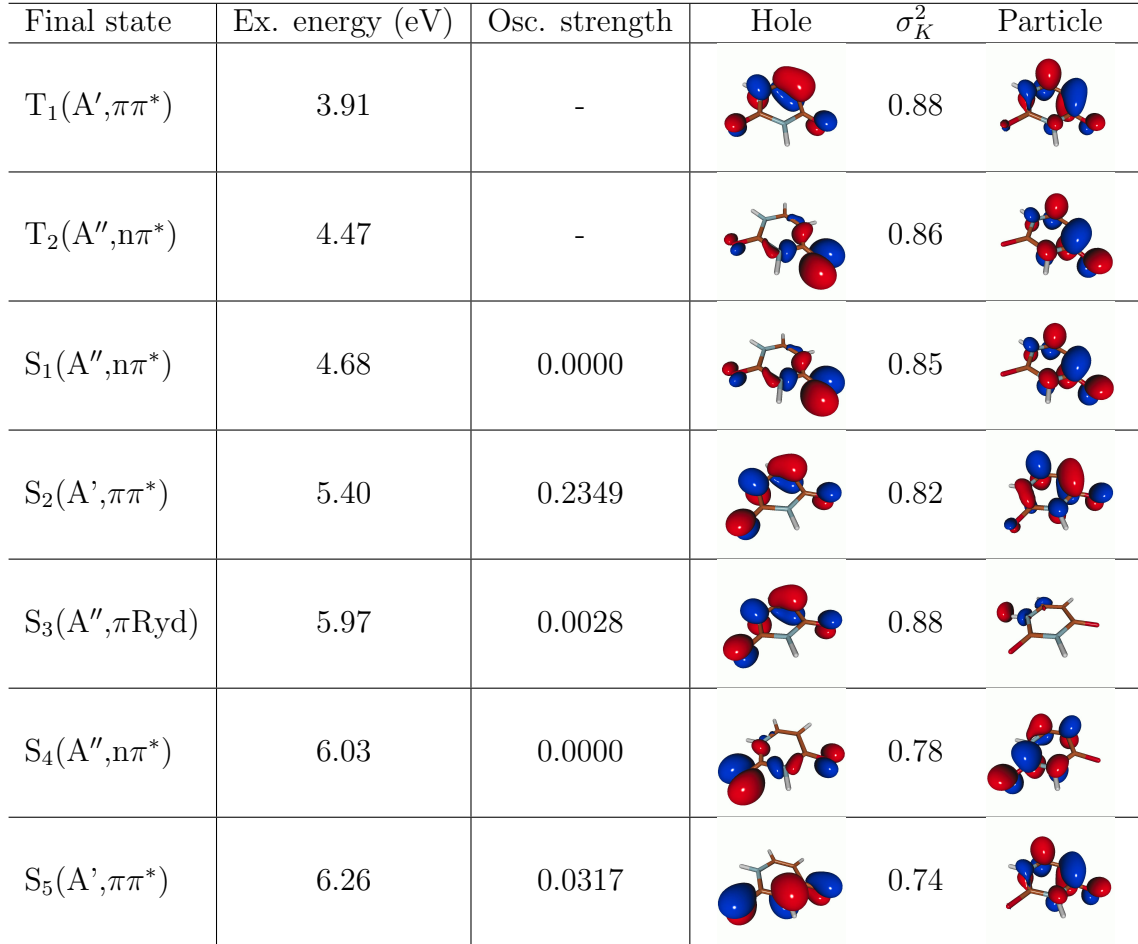 | 0.88         | 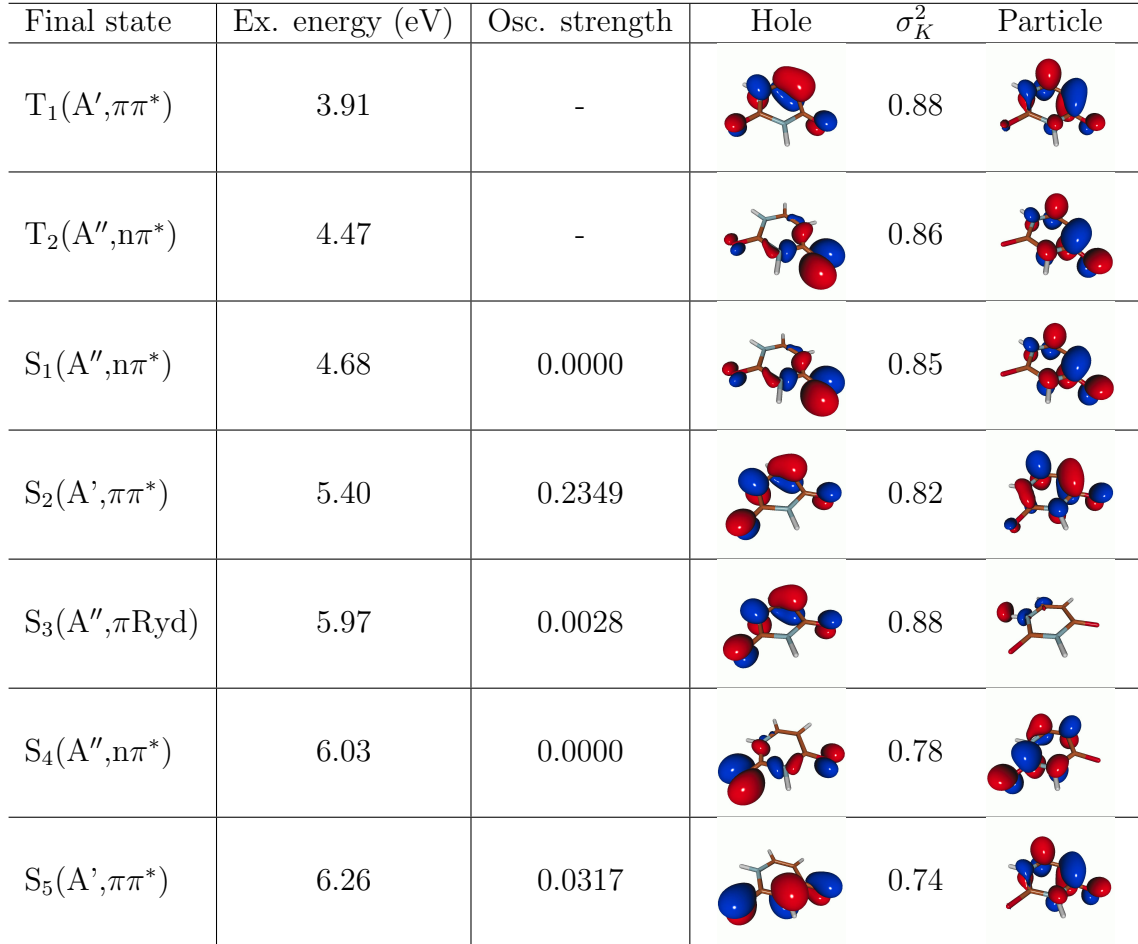 |
| $S_4(A'', n\pi^*)$  | 6.03            | 0.0000        | 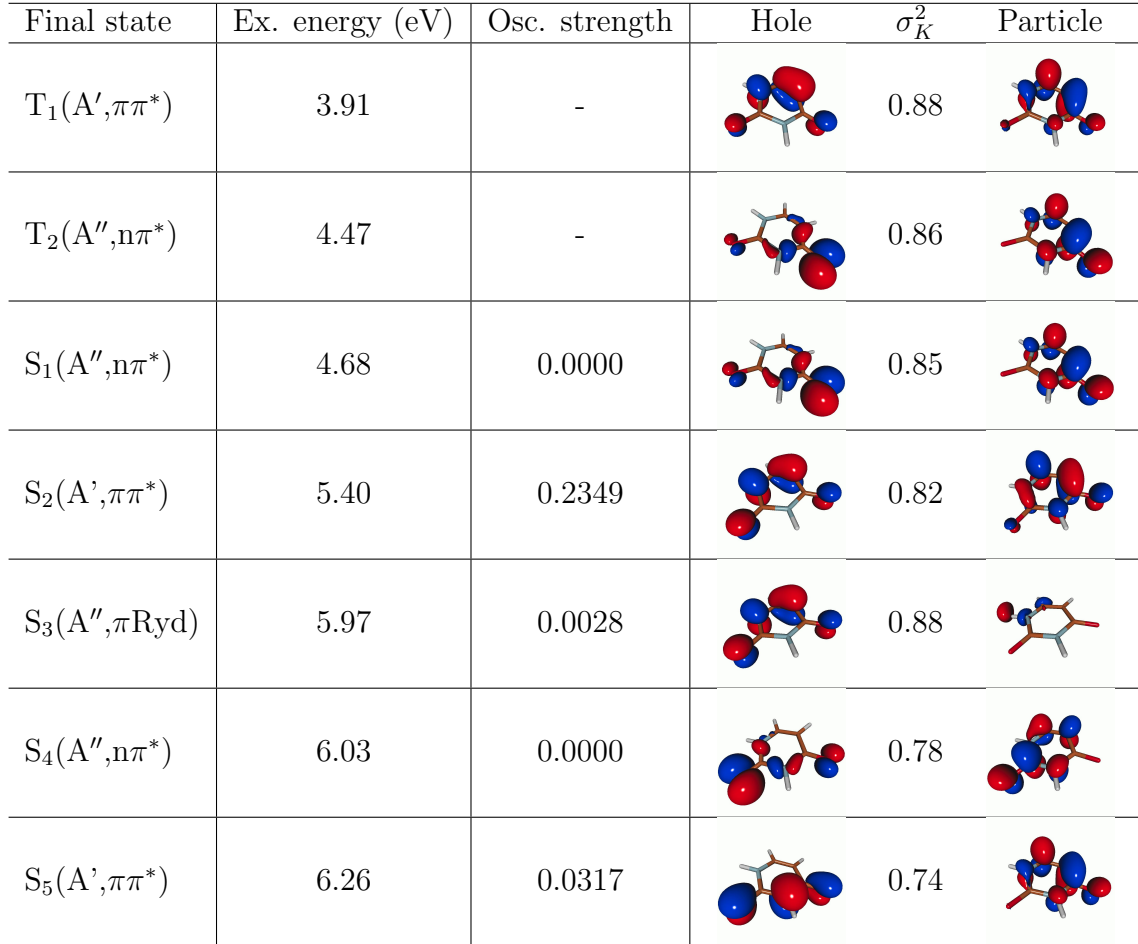 | 0.78         | 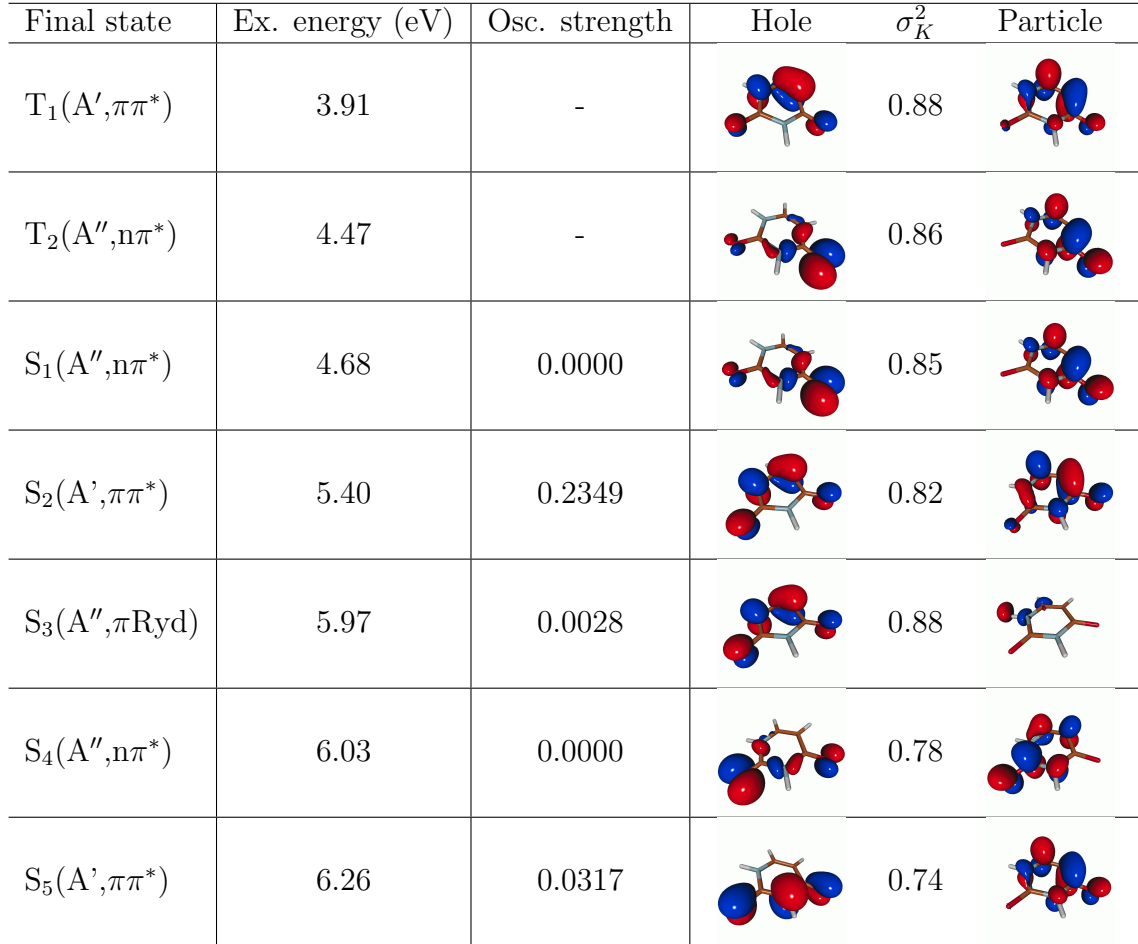 |
| $S_5(A', \pi\pi^*)$ | 6.26            | 0.0317        | 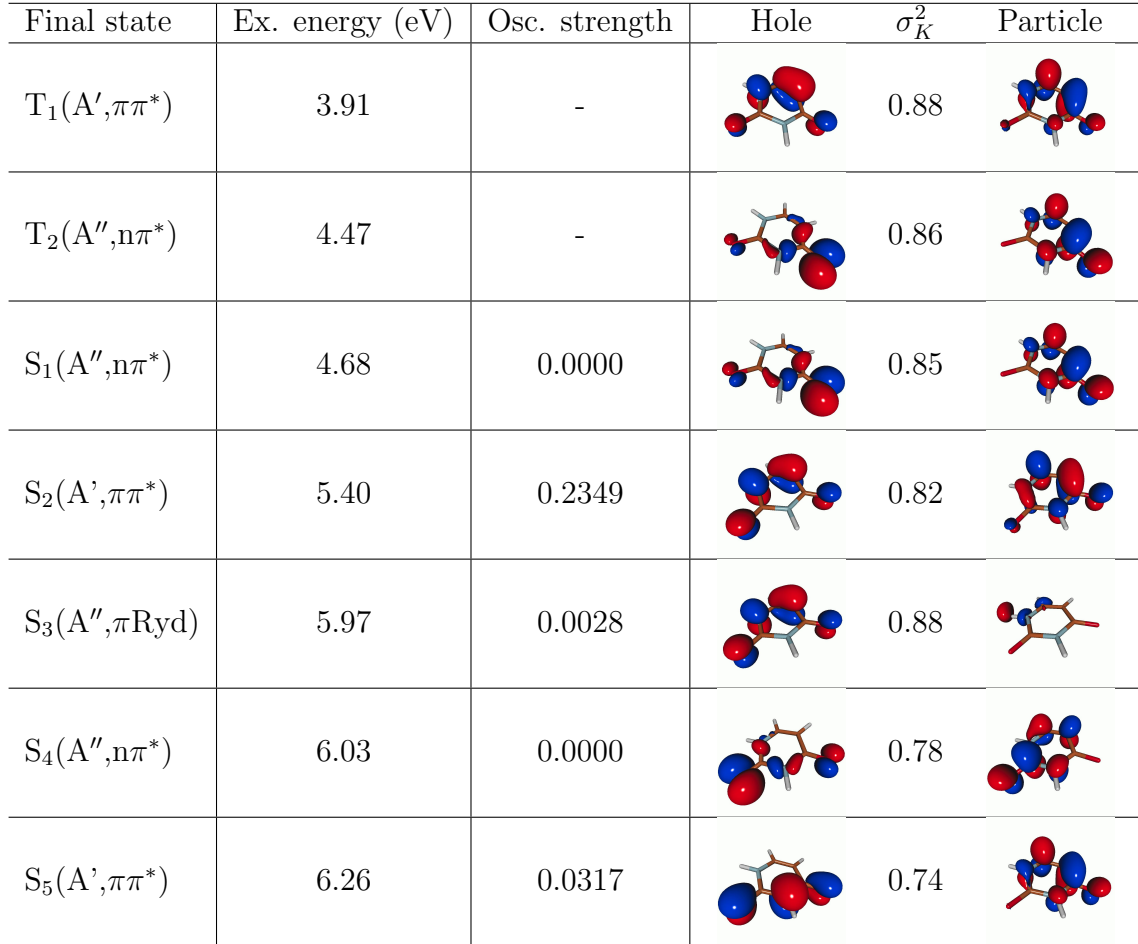 | 0.74         | 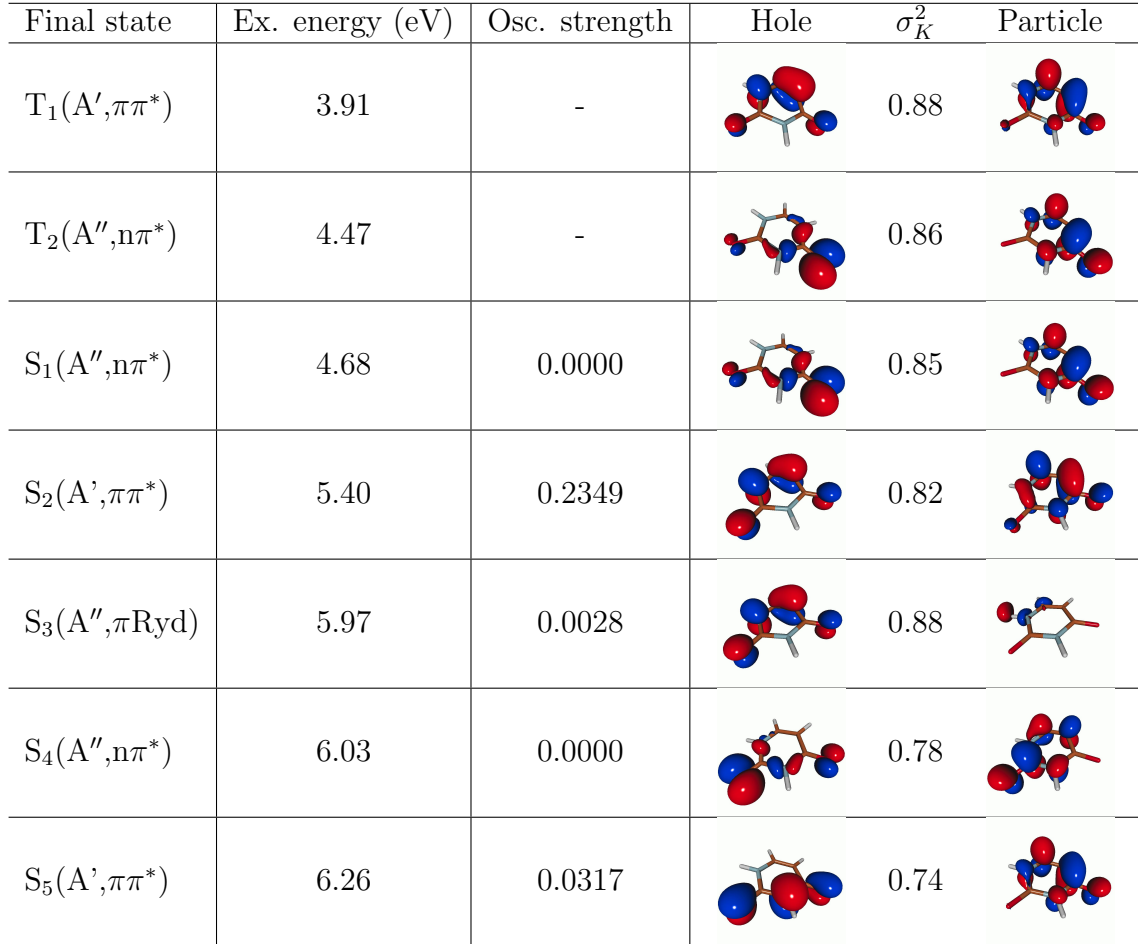 |

Table S12: Uracil. TDDFT/B3LYP/6-311++G\*\* NTOs of the excitations from the ground state to the lowest-lying valence-excited states at the FC geometry (NTO isosurface is 0.05).

| Final state         | Ex. energy (eV) | Osc. strength | Hole                                                                                 | $\sigma_K^2$ | Particle                                                                              |
|---------------------|-----------------|---------------|--------------------------------------------------------------------------------------|--------------|---------------------------------------------------------------------------------------|
| $T_1(A', \pi\pi^*)$ | 3.43            | -             | 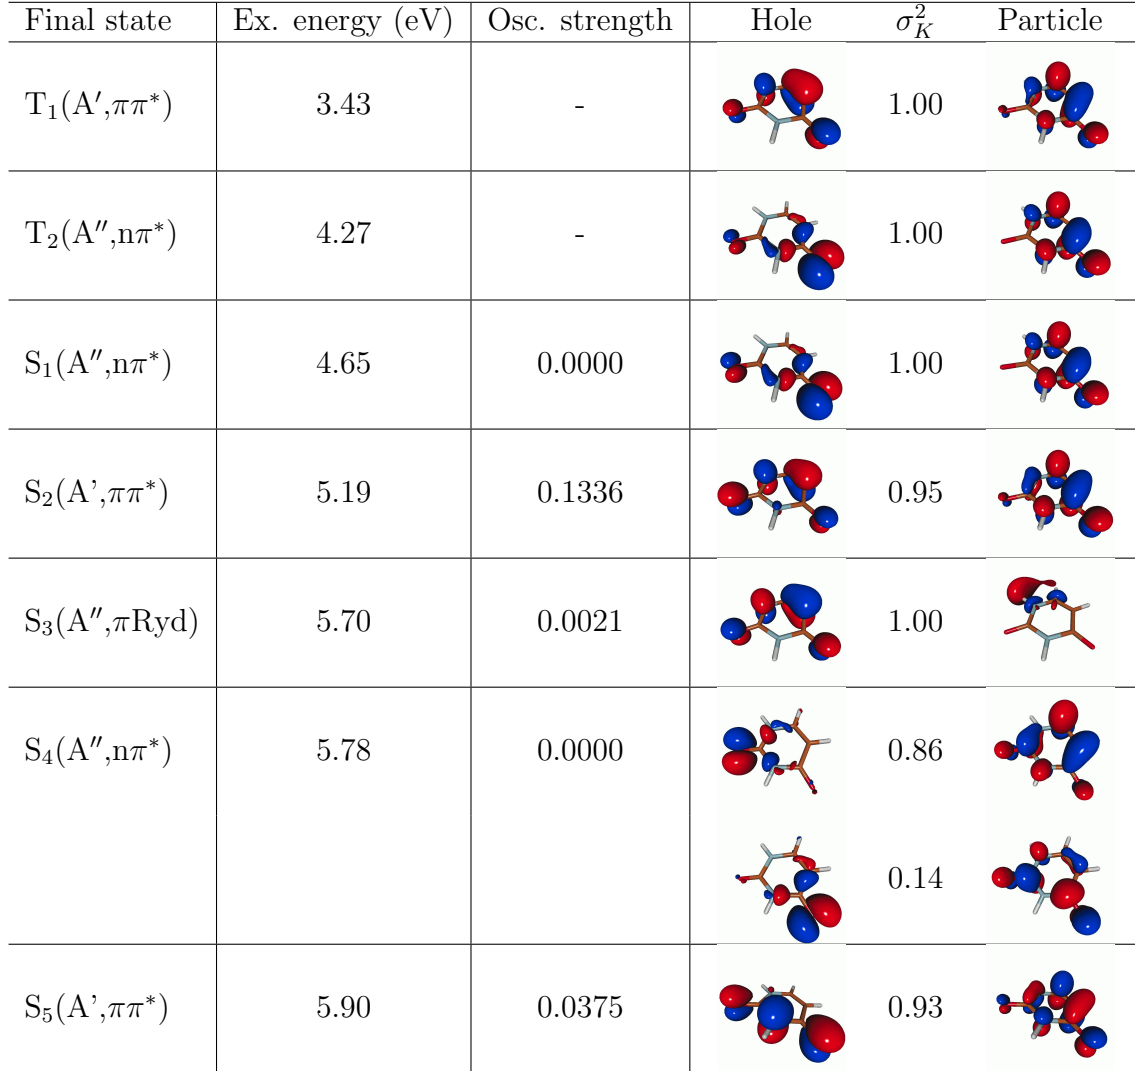   | 1.00         | 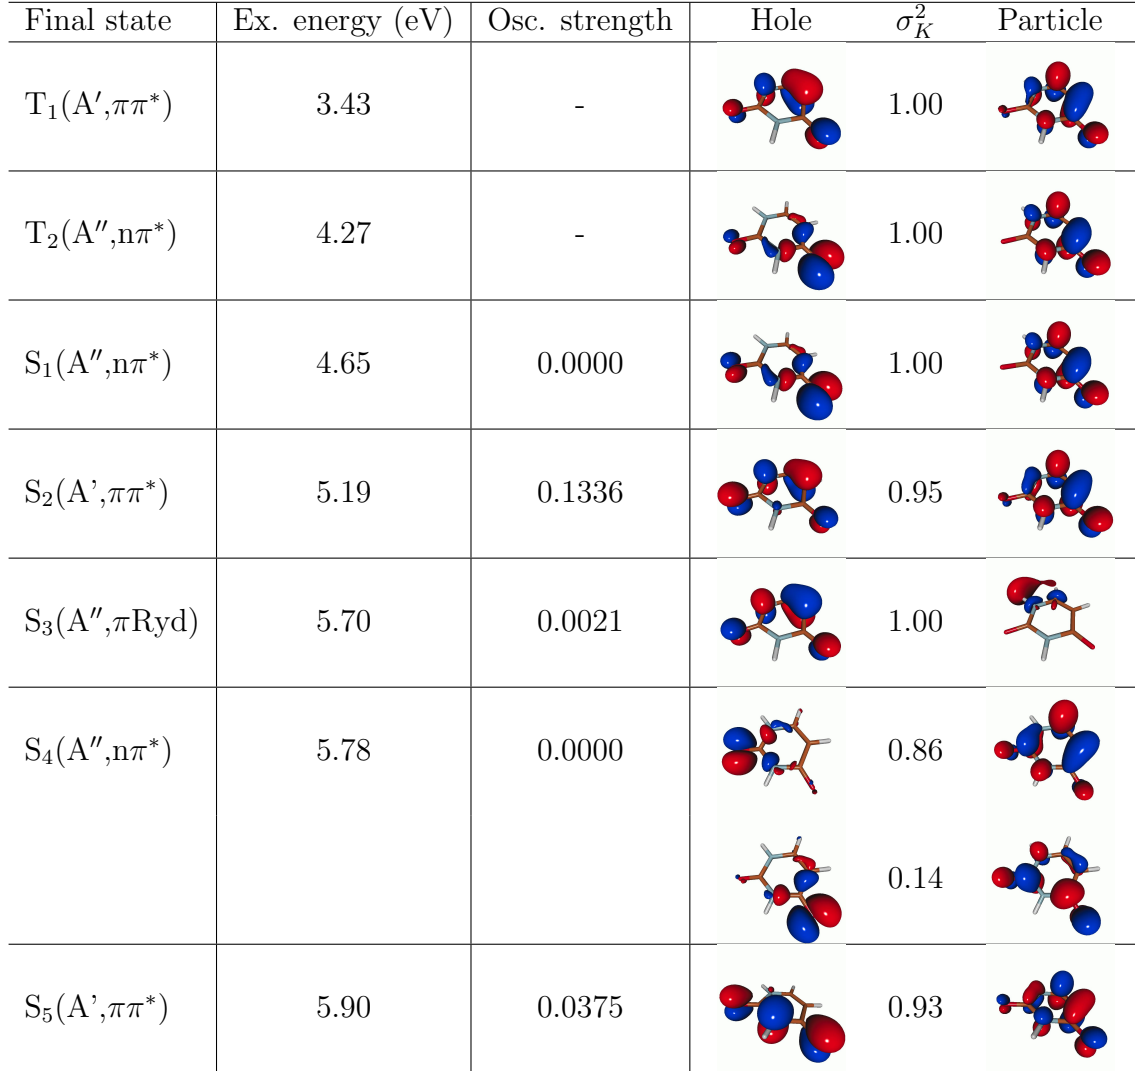   |
| $T_2(A'', n\pi^*)$  | 4.27            | -             | 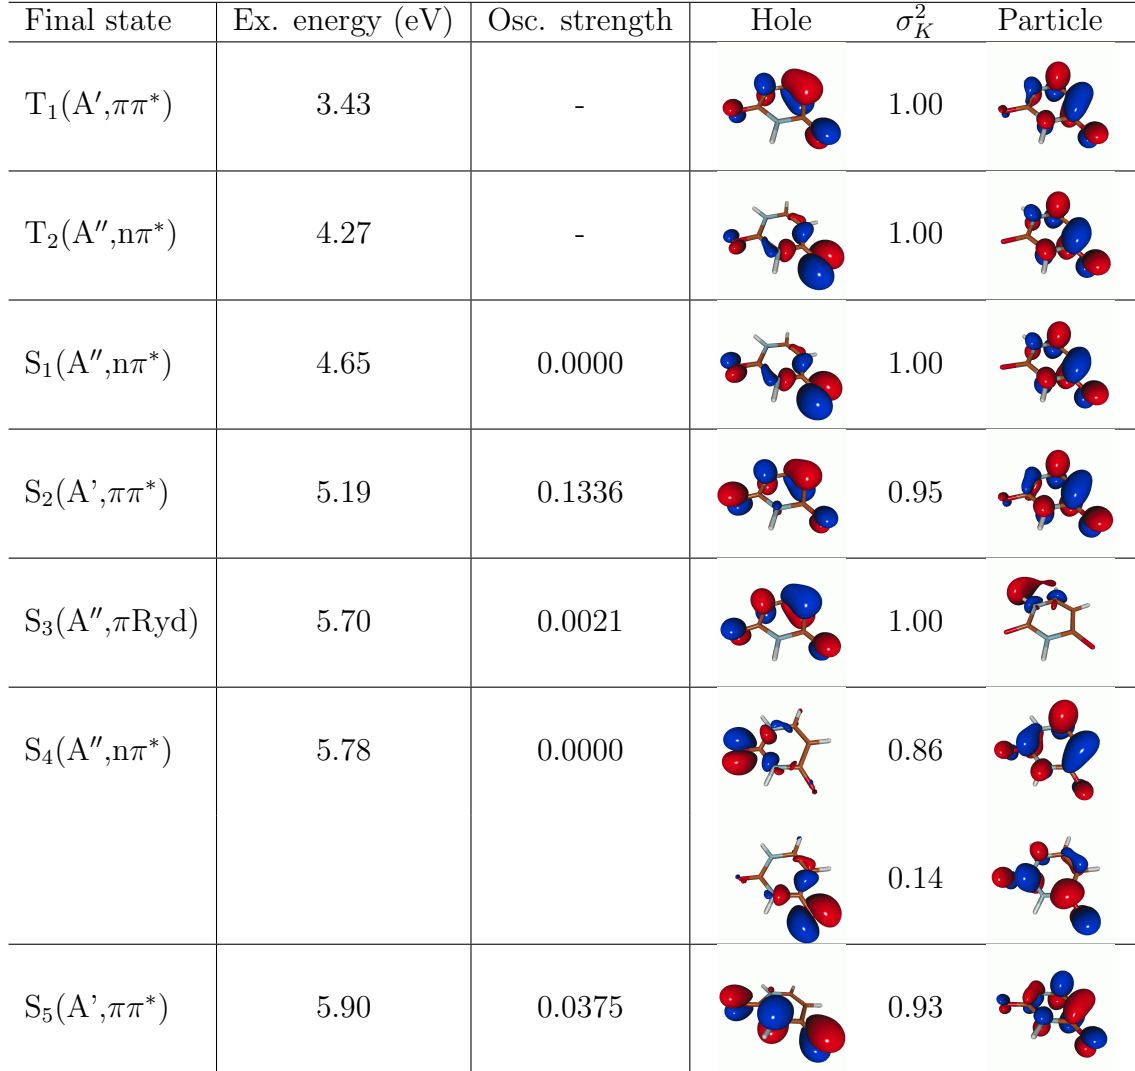   | 1.00         | 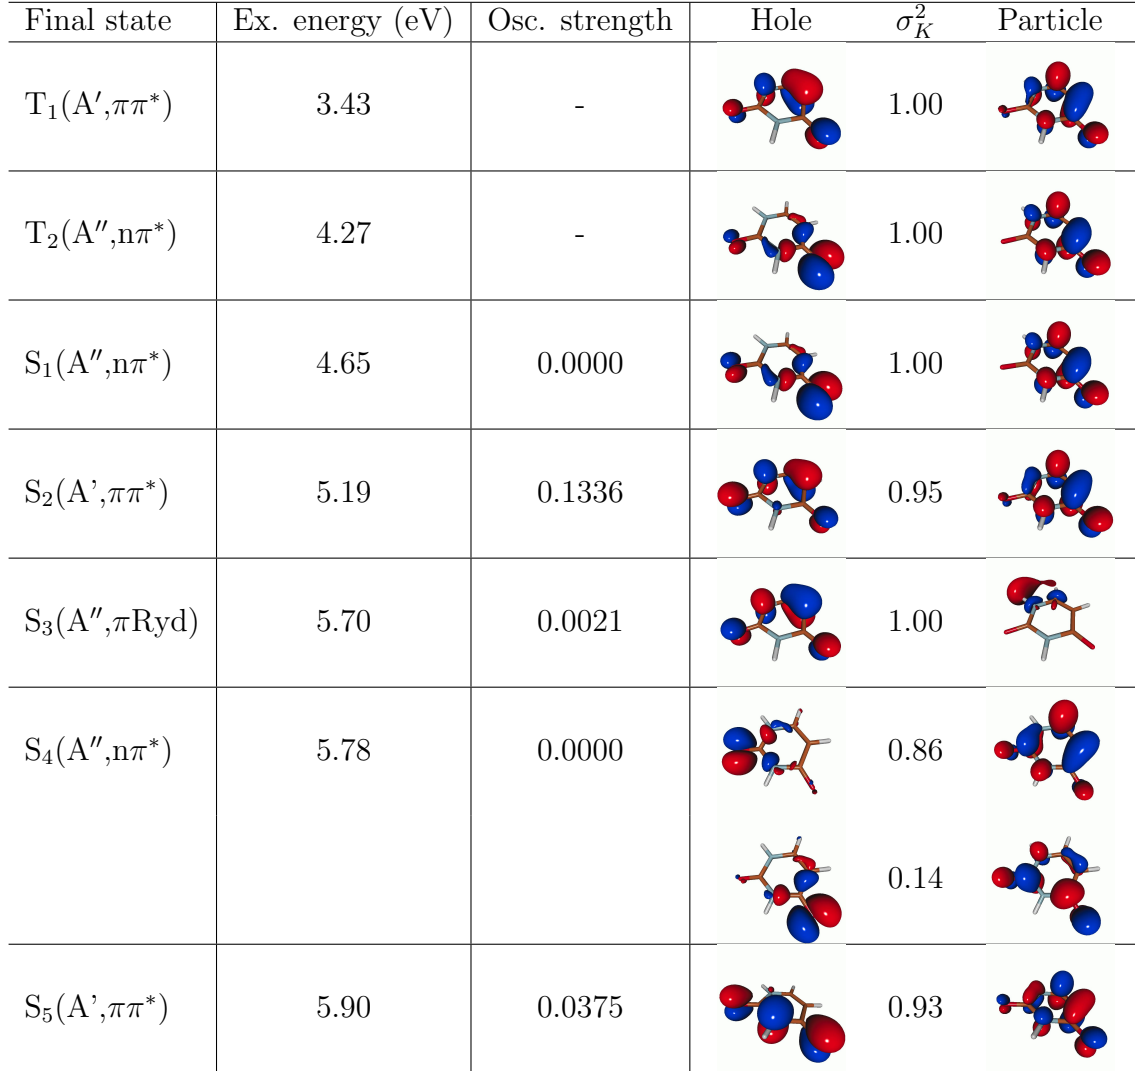   |
| $S_1(A'', n\pi^*)$  | 4.65            | 0.0000        | 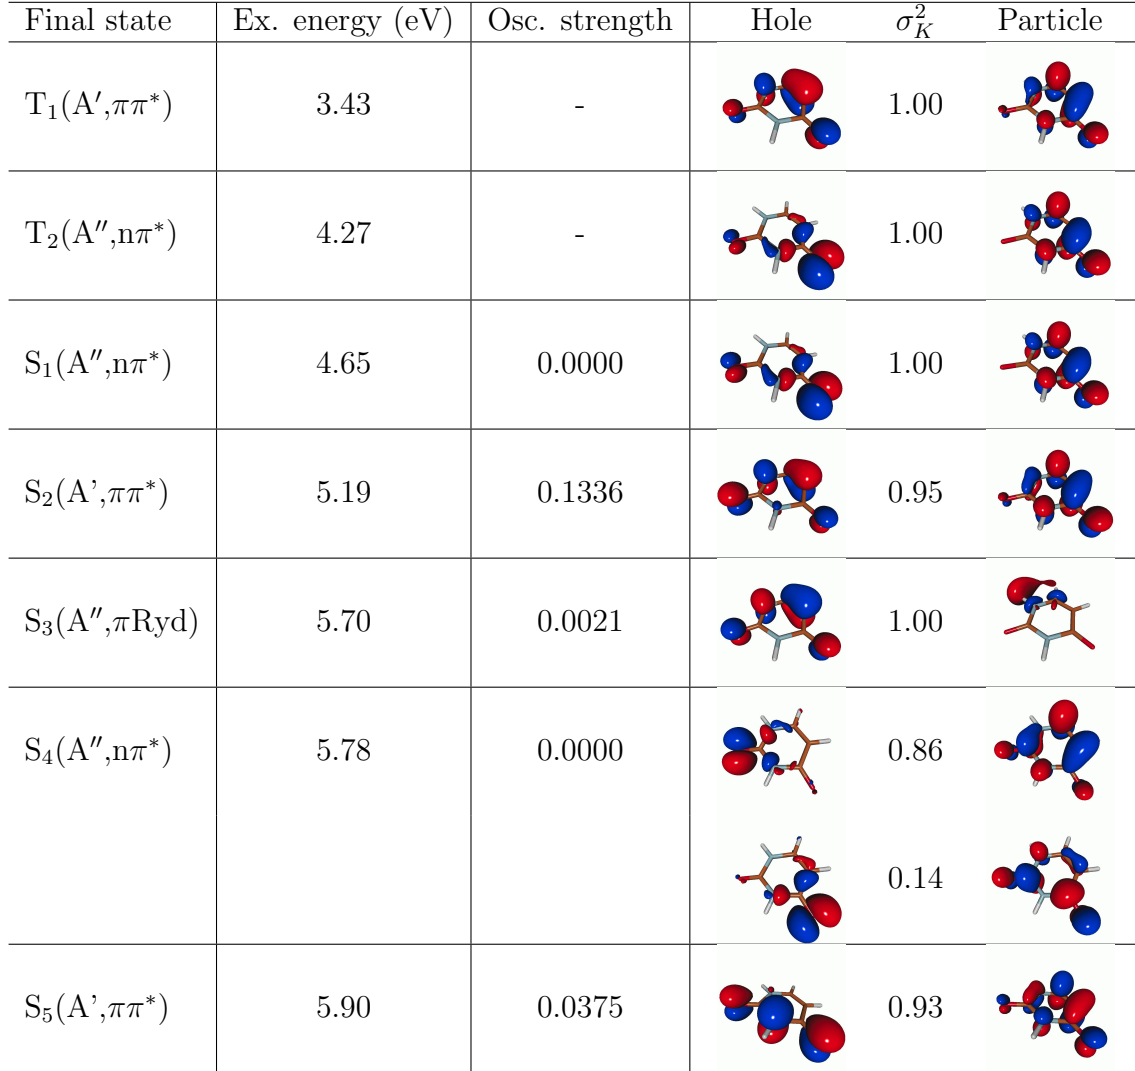   | 1.00         | 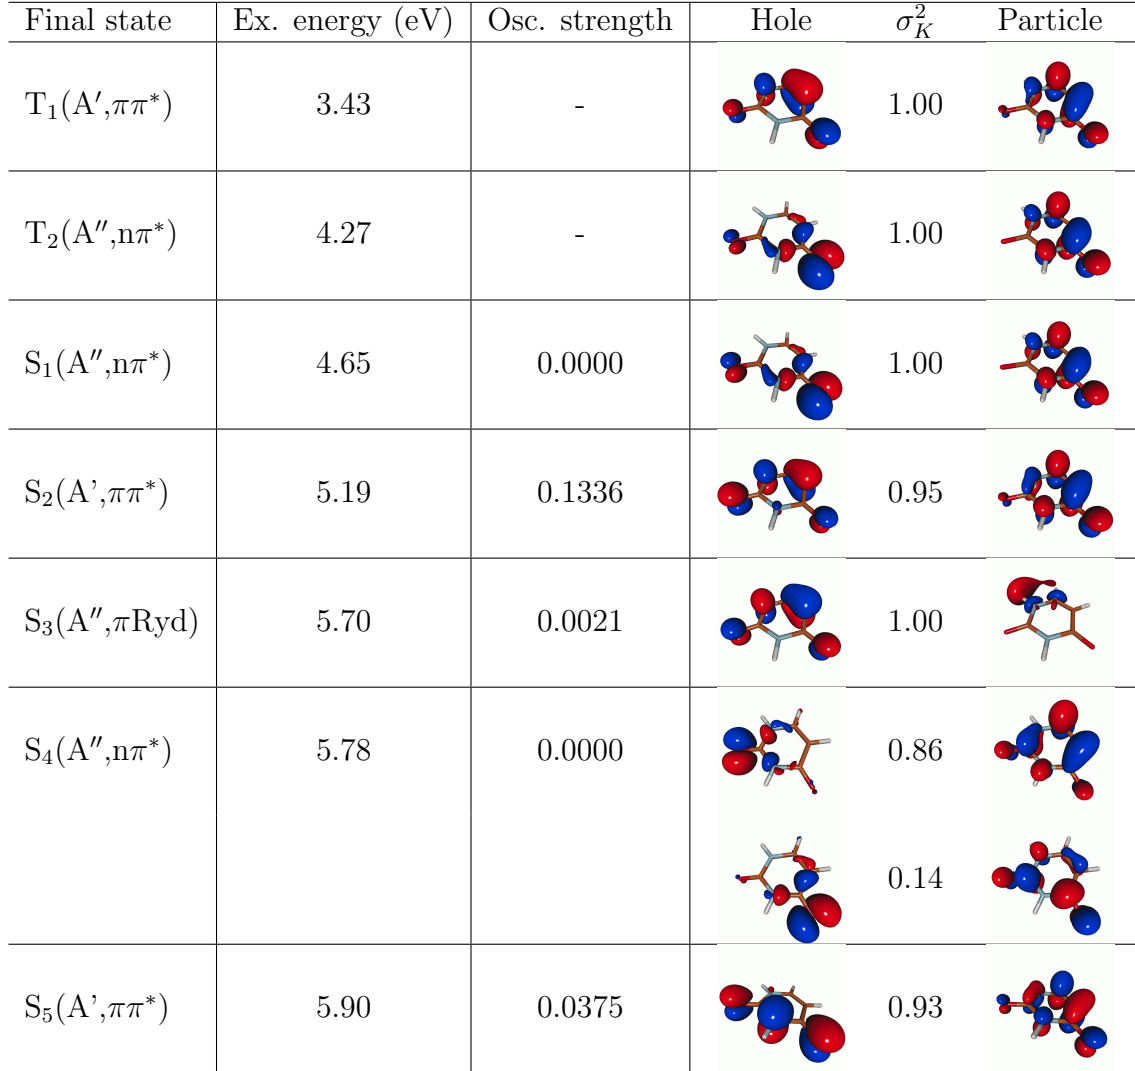   |
| $S_2(A', \pi\pi^*)$ | 5.19            | 0.1336        | 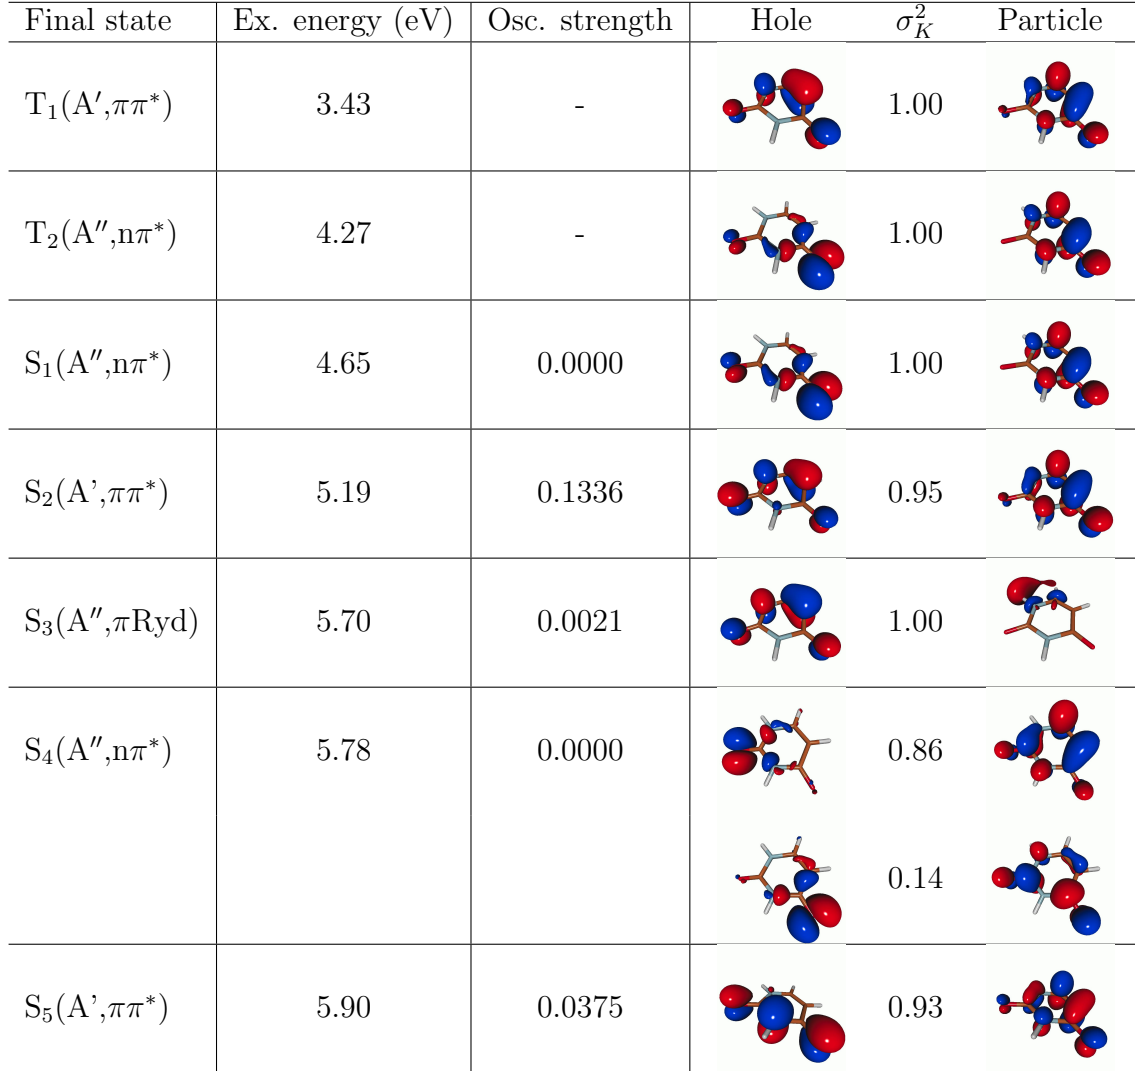 | 0.95         | 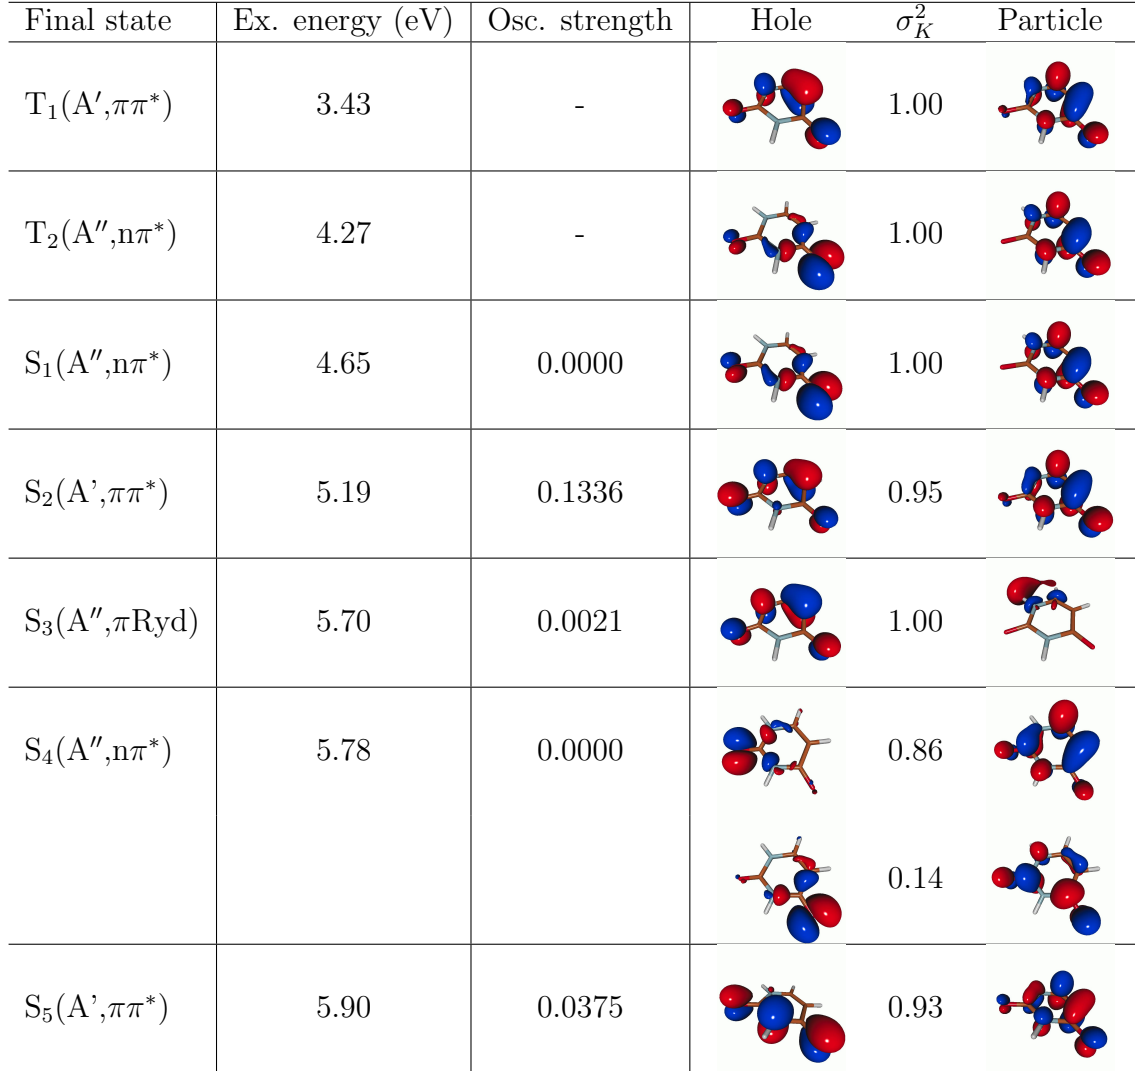 |
| $S_3(A'', \pi Ryd)$ | 5.70            | 0.0021        | 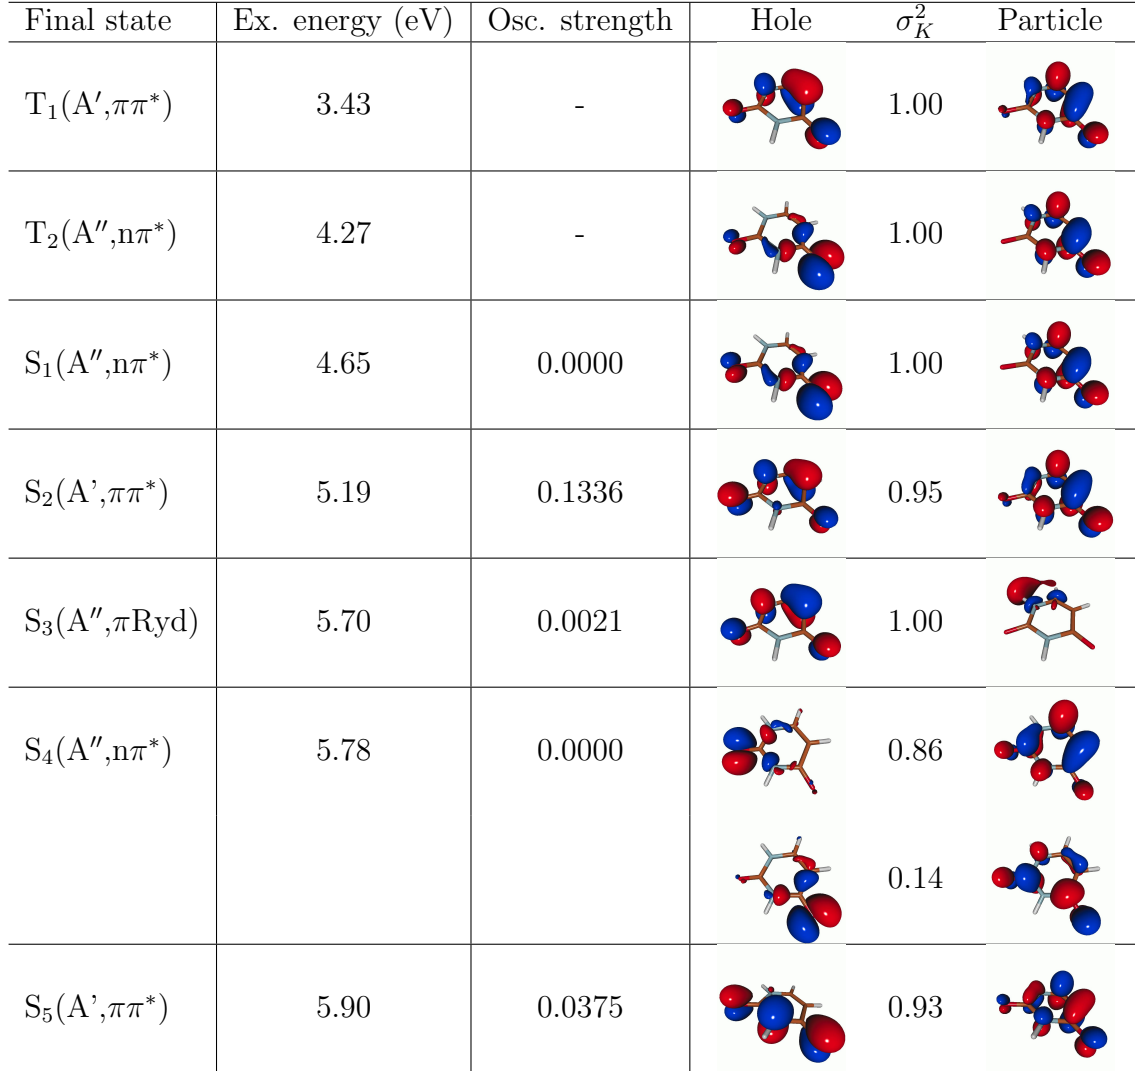 | 1.00         | 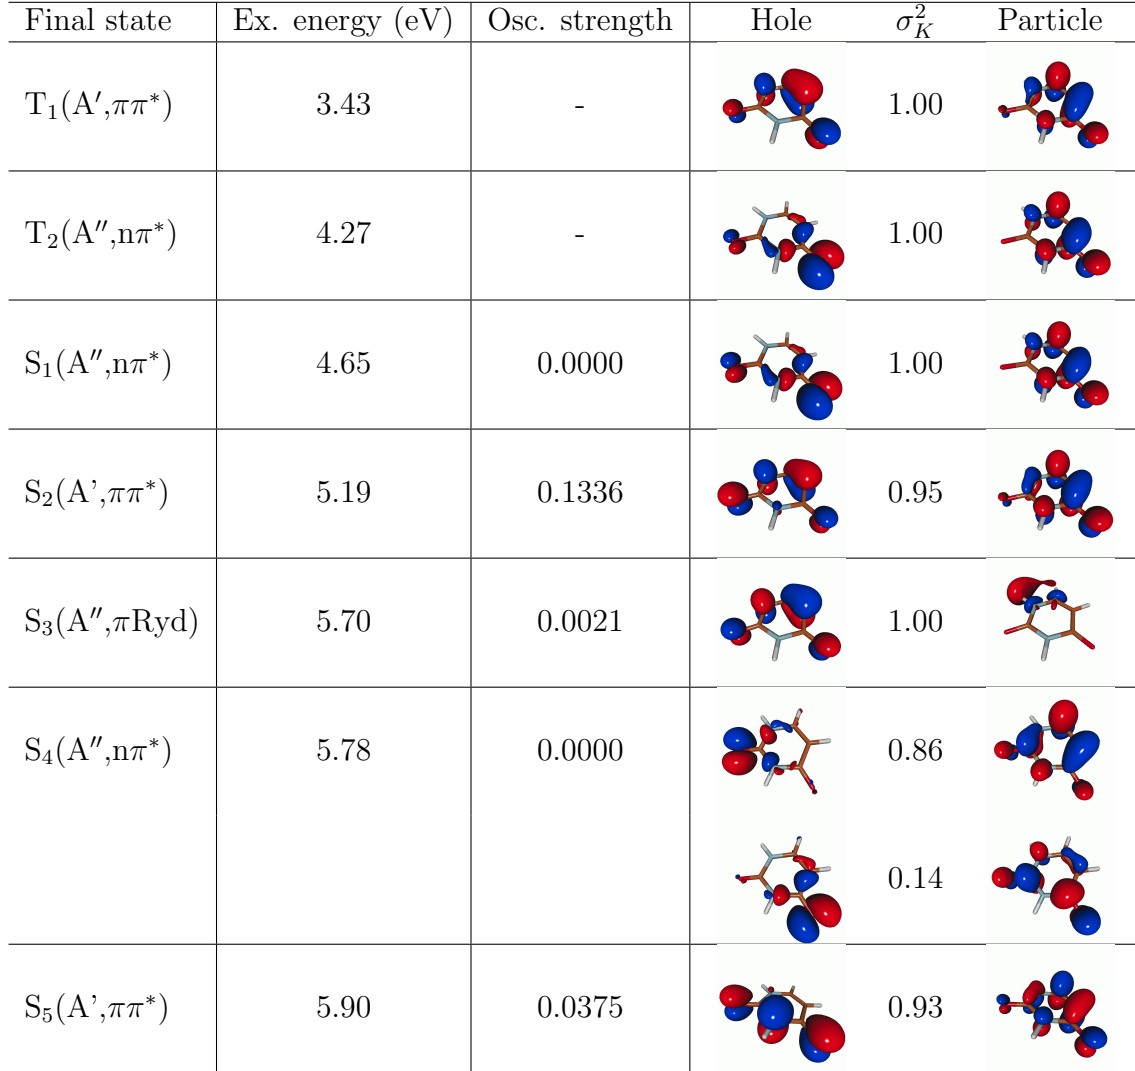 |
| $S_4(A'', n\pi^*)$  | 5.78            | 0.0000        | 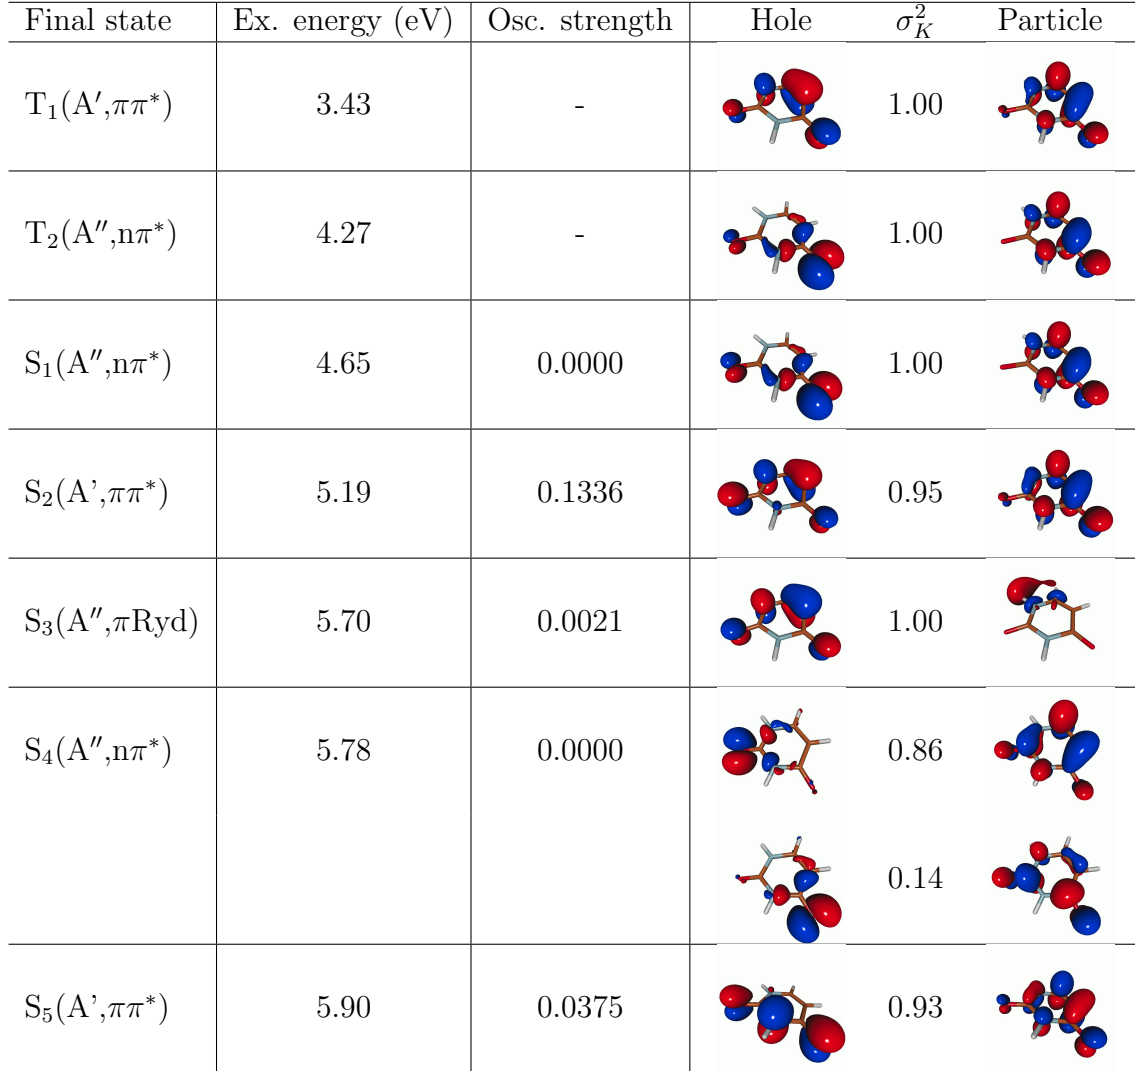 | 0.86         | 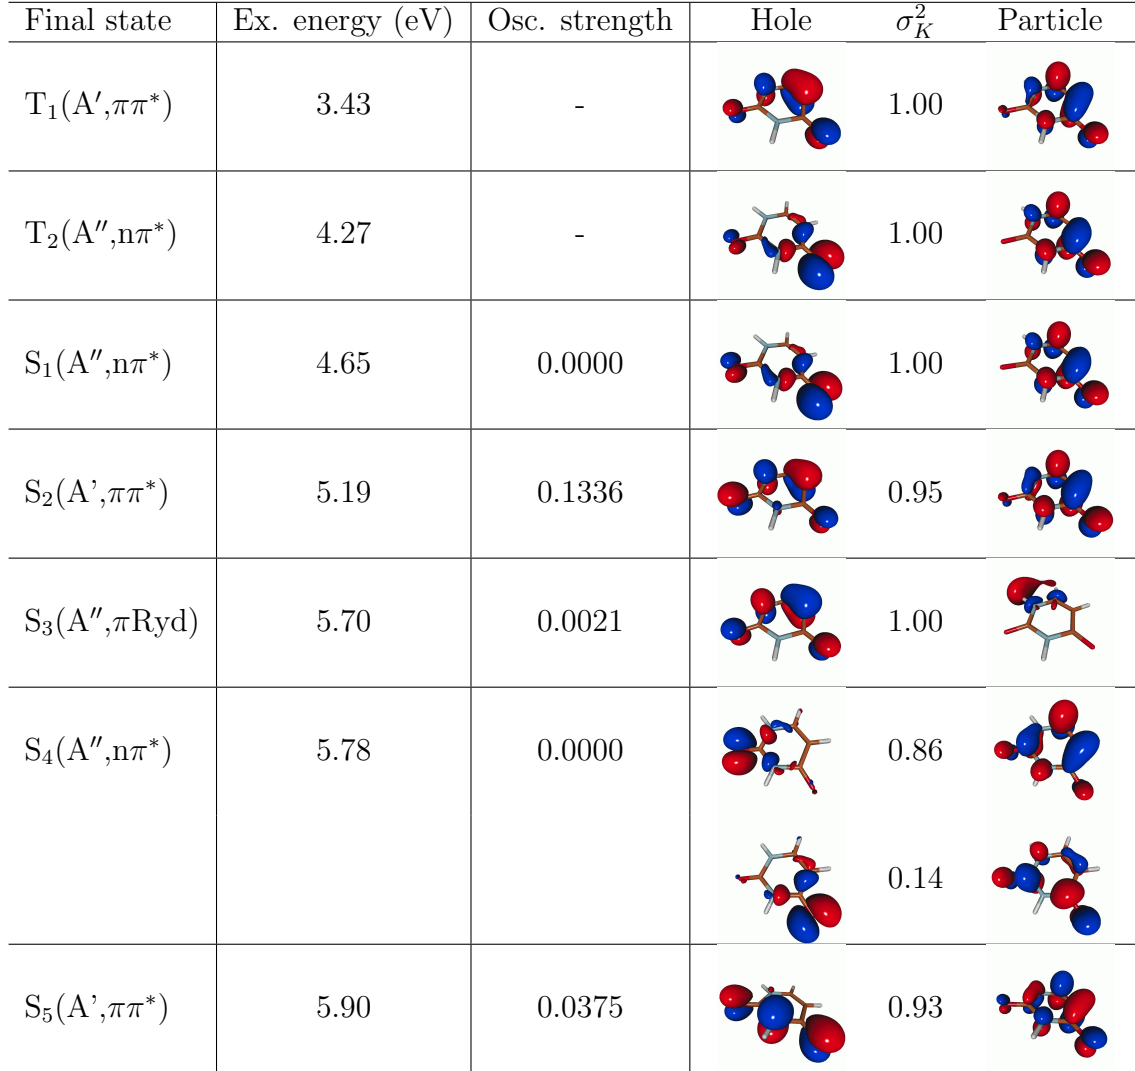 |
|                     |                 |               | 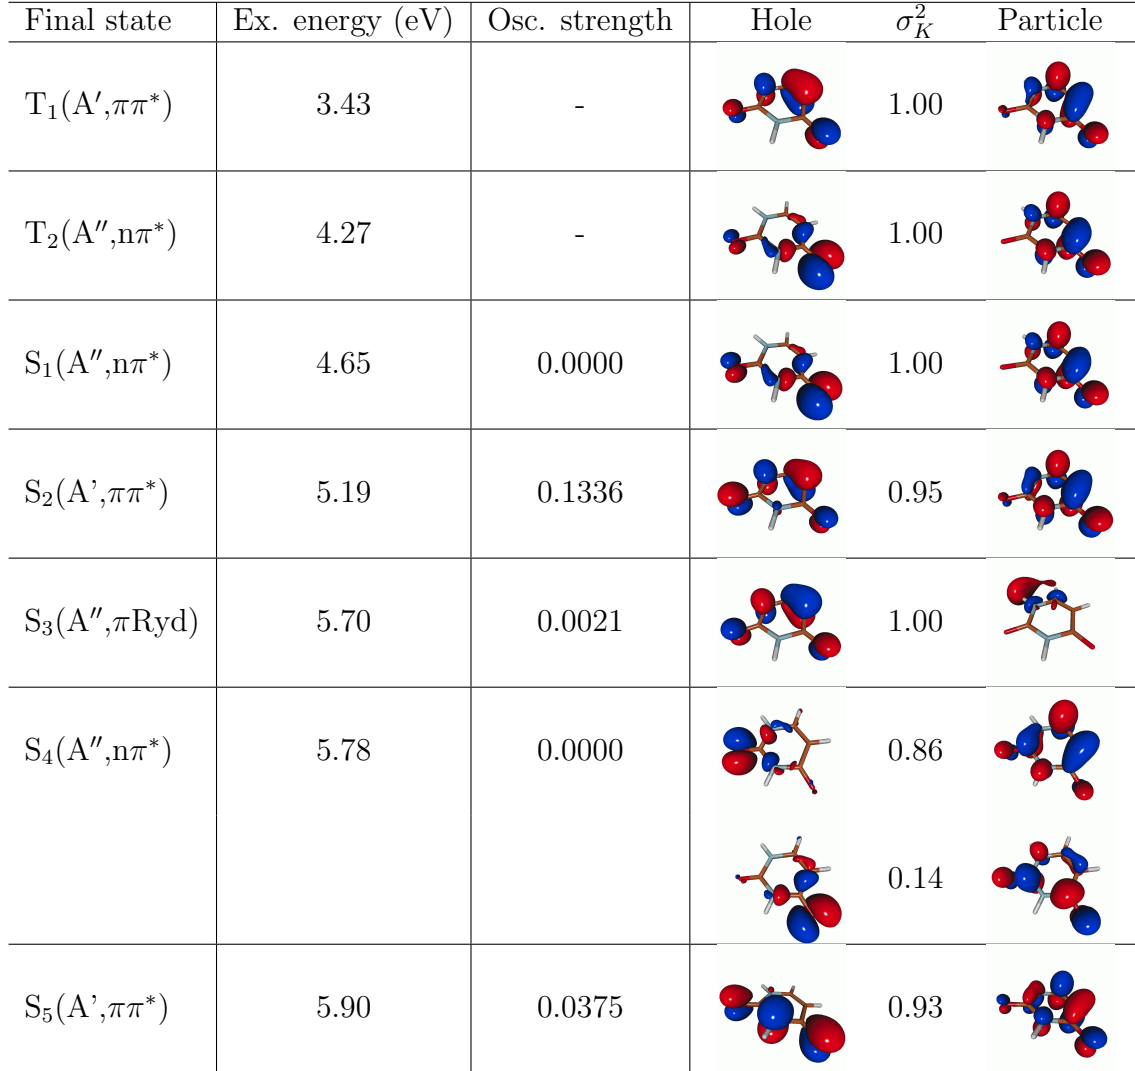 | 0.14         | 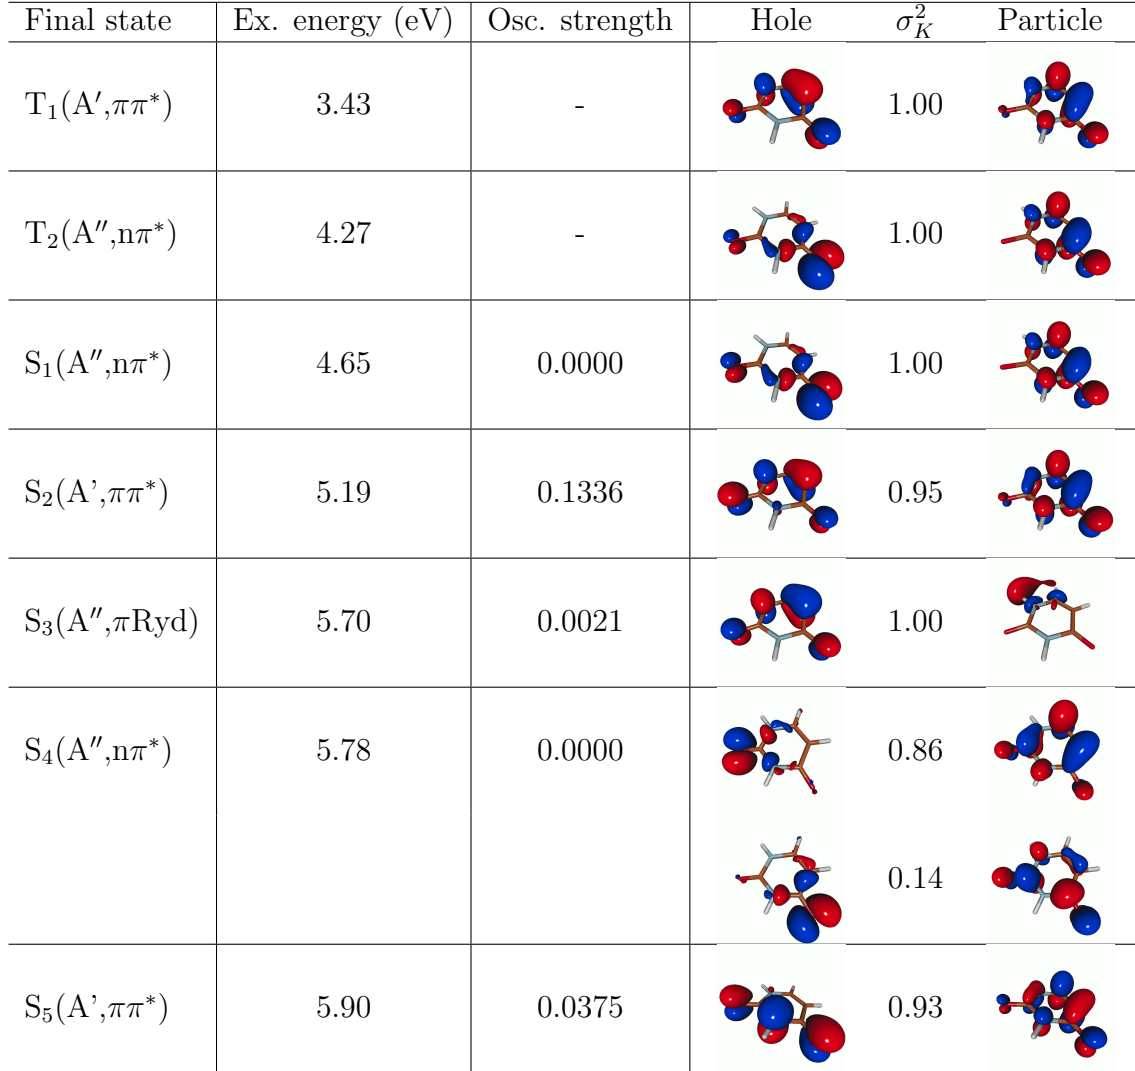 |
| $S_5(A', \pi\pi^*)$ | 5.90            | 0.0375        | 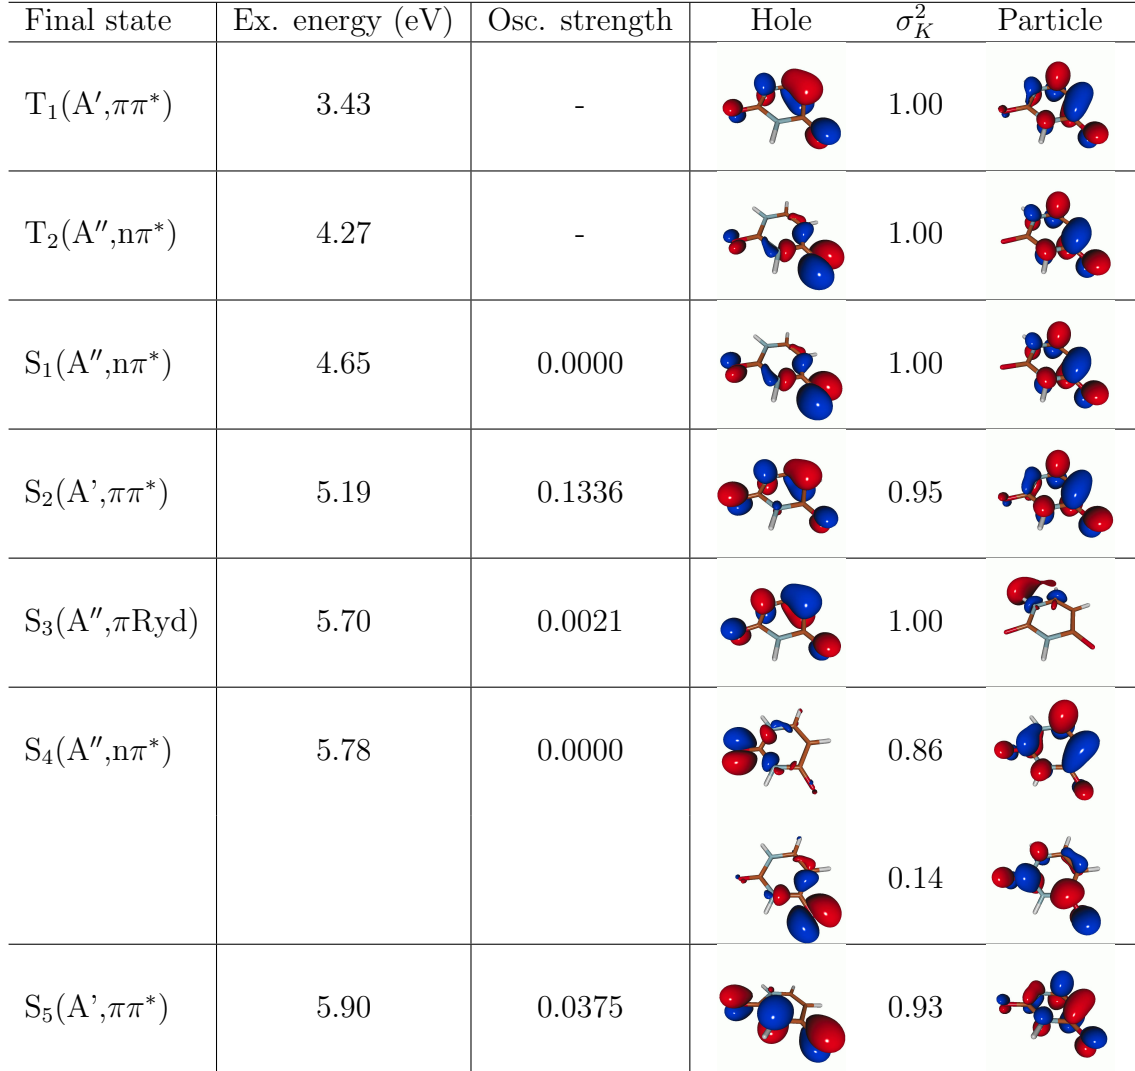 | 0.93         | 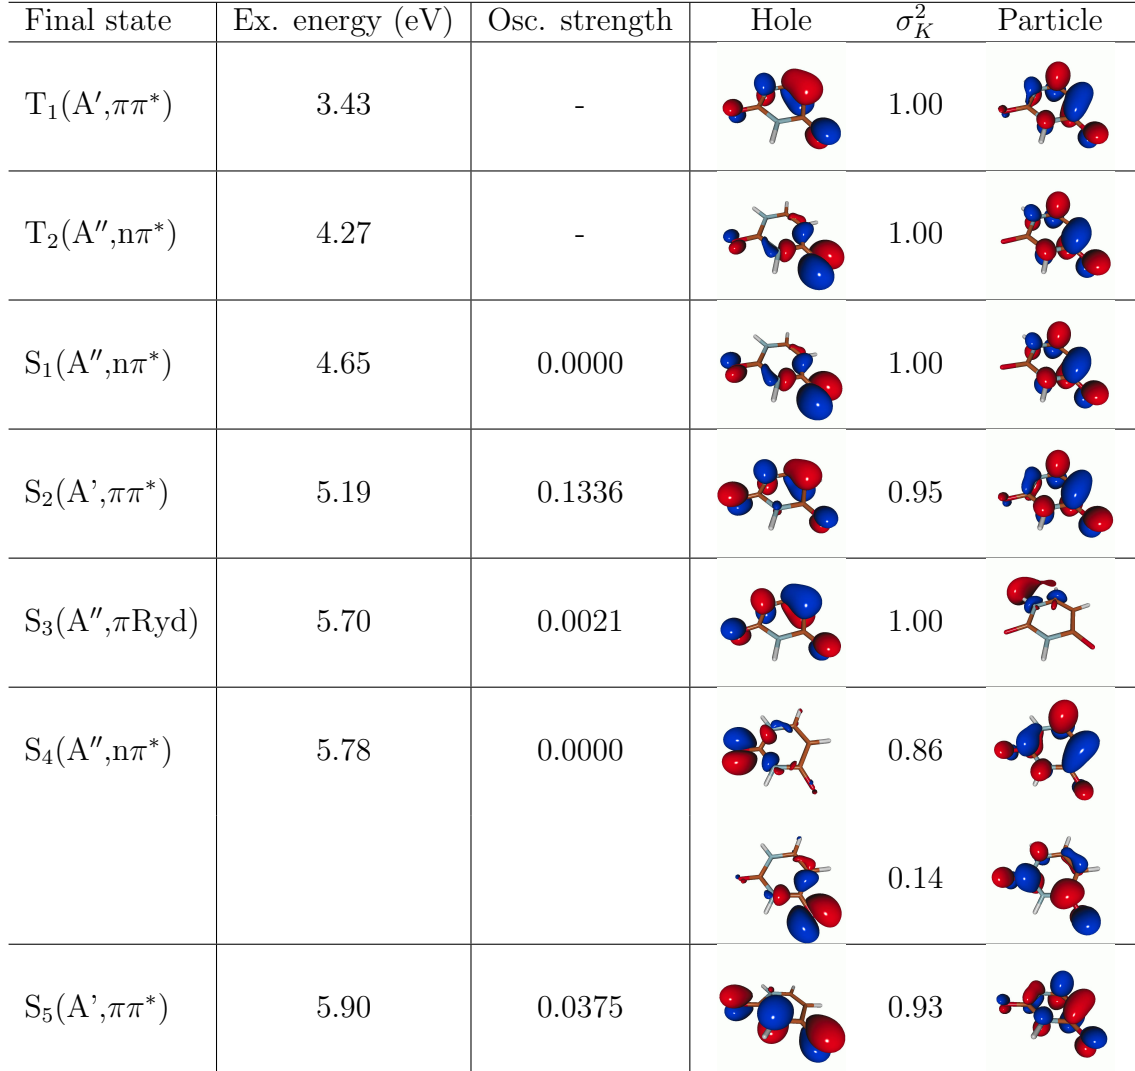 |

Table S13: Thymine. EOM-EE-CCSD/6-311++G\*\* NTOs of the excitations from the ground state to the lowest-lying valence-excited states at the FC geometry (NTO isosurface is 0.05).

| Final state     | Ex. energy (eV) | Osc. strength | Hole                                                                                 | $\sigma_K^2$ | Particle                                                                              |
|-----------------|-----------------|---------------|--------------------------------------------------------------------------------------|--------------|---------------------------------------------------------------------------------------|
| $T_1(\pi\pi^*)$ | 3.63            | -             | 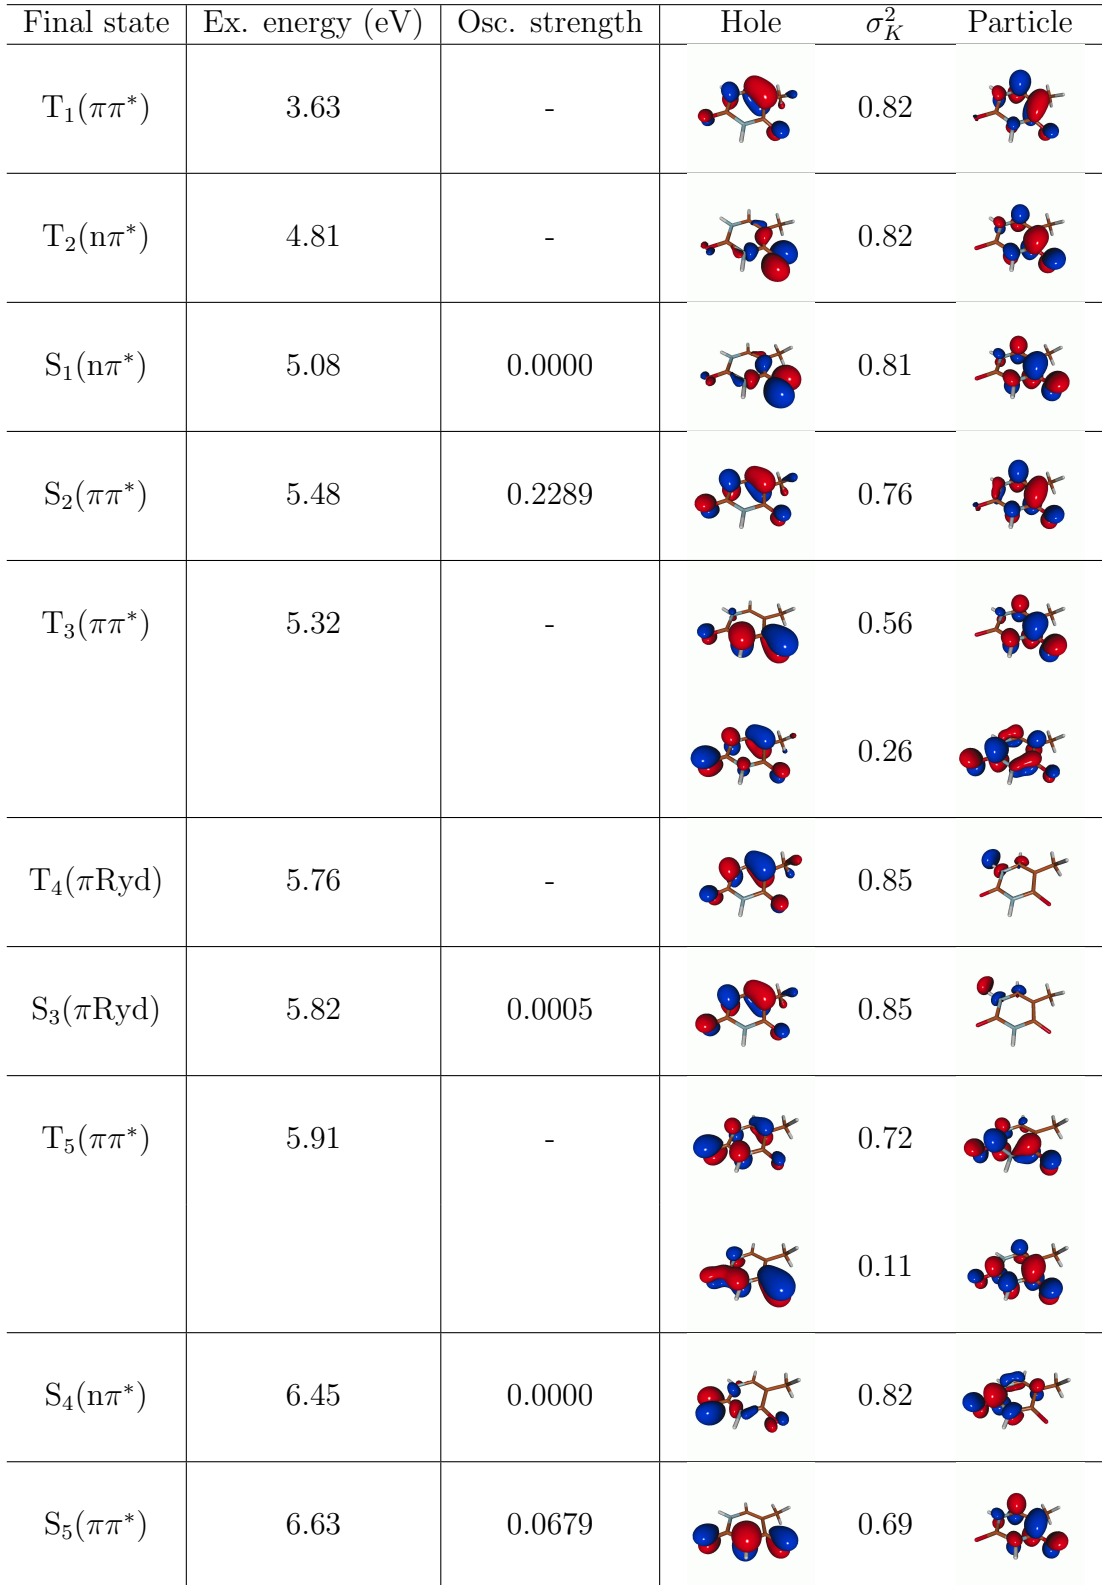   | 0.82         | 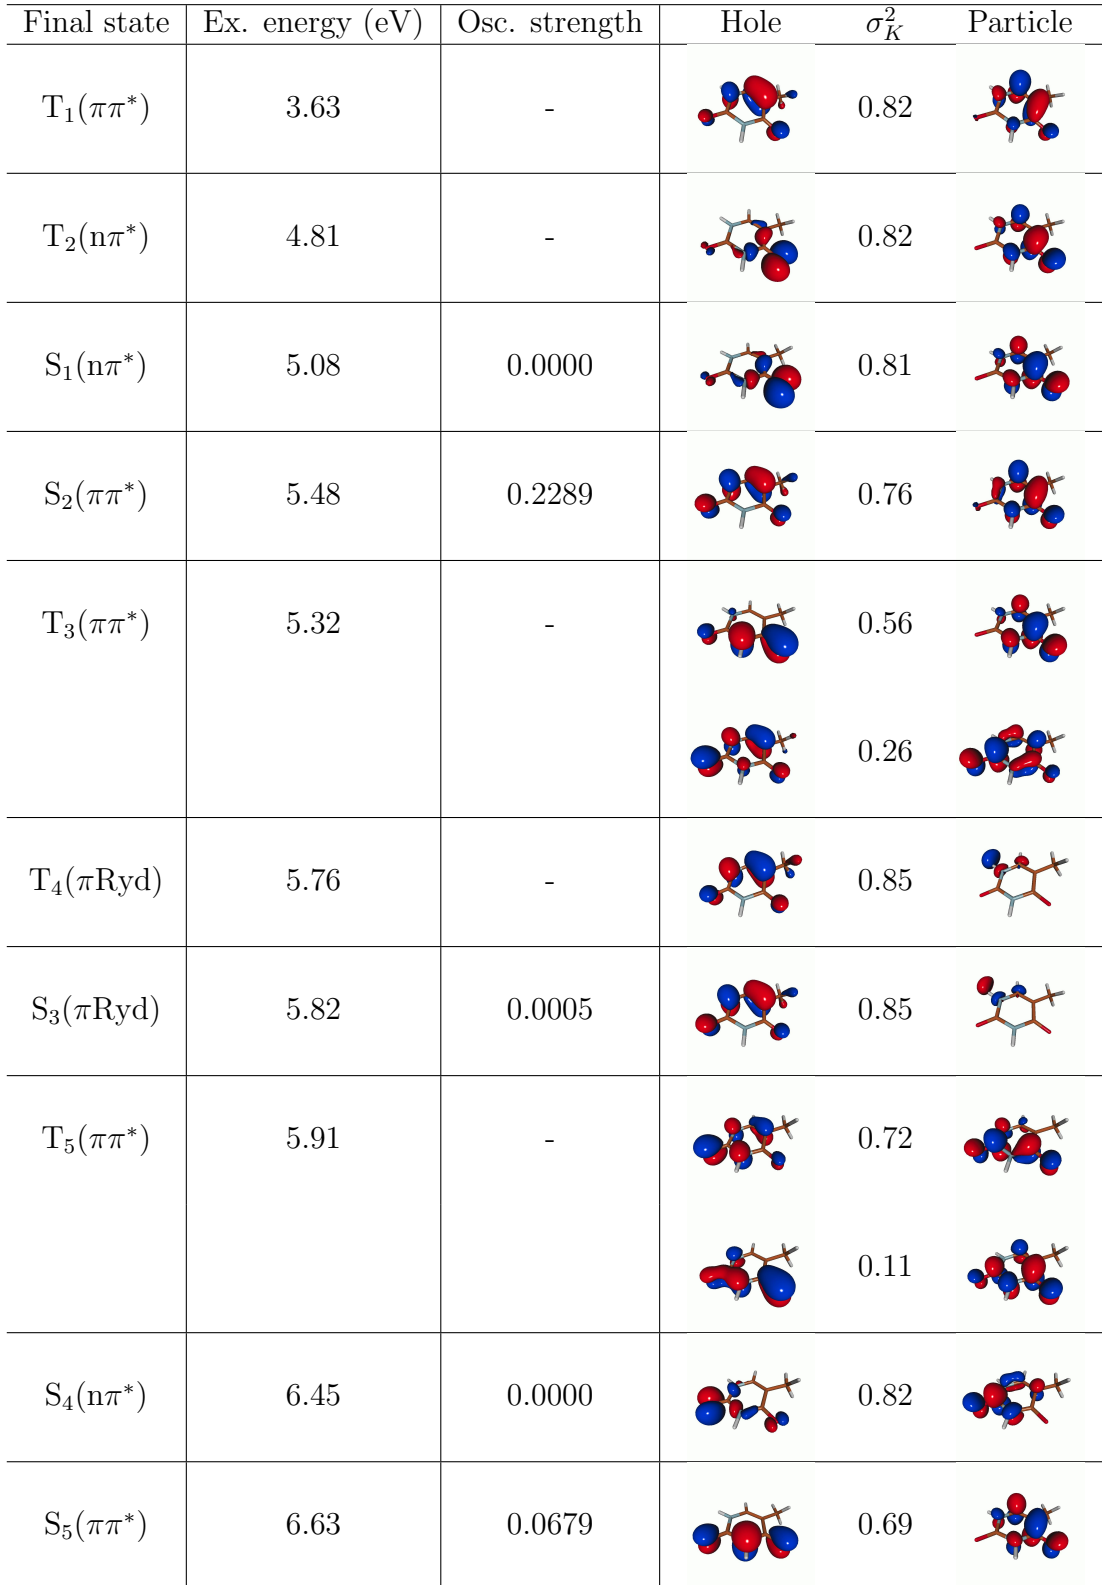   |
| $T_2(n\pi^*)$   | 4.81            | -             | 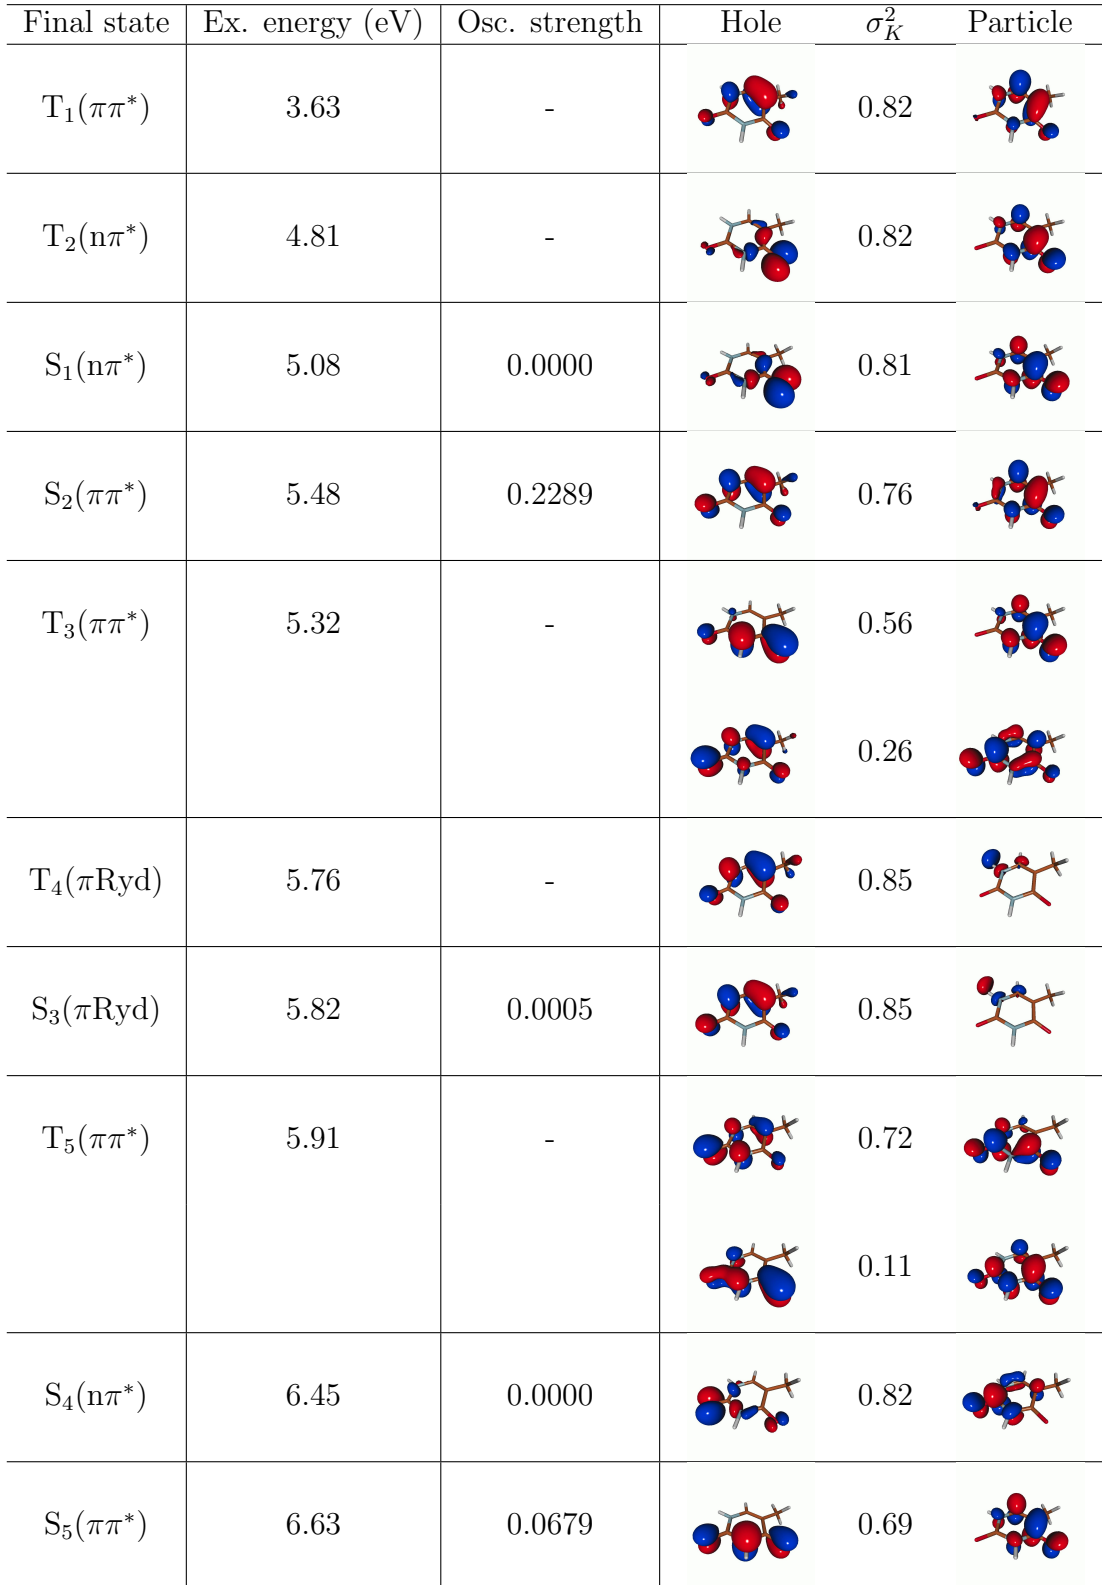   | 0.82         | 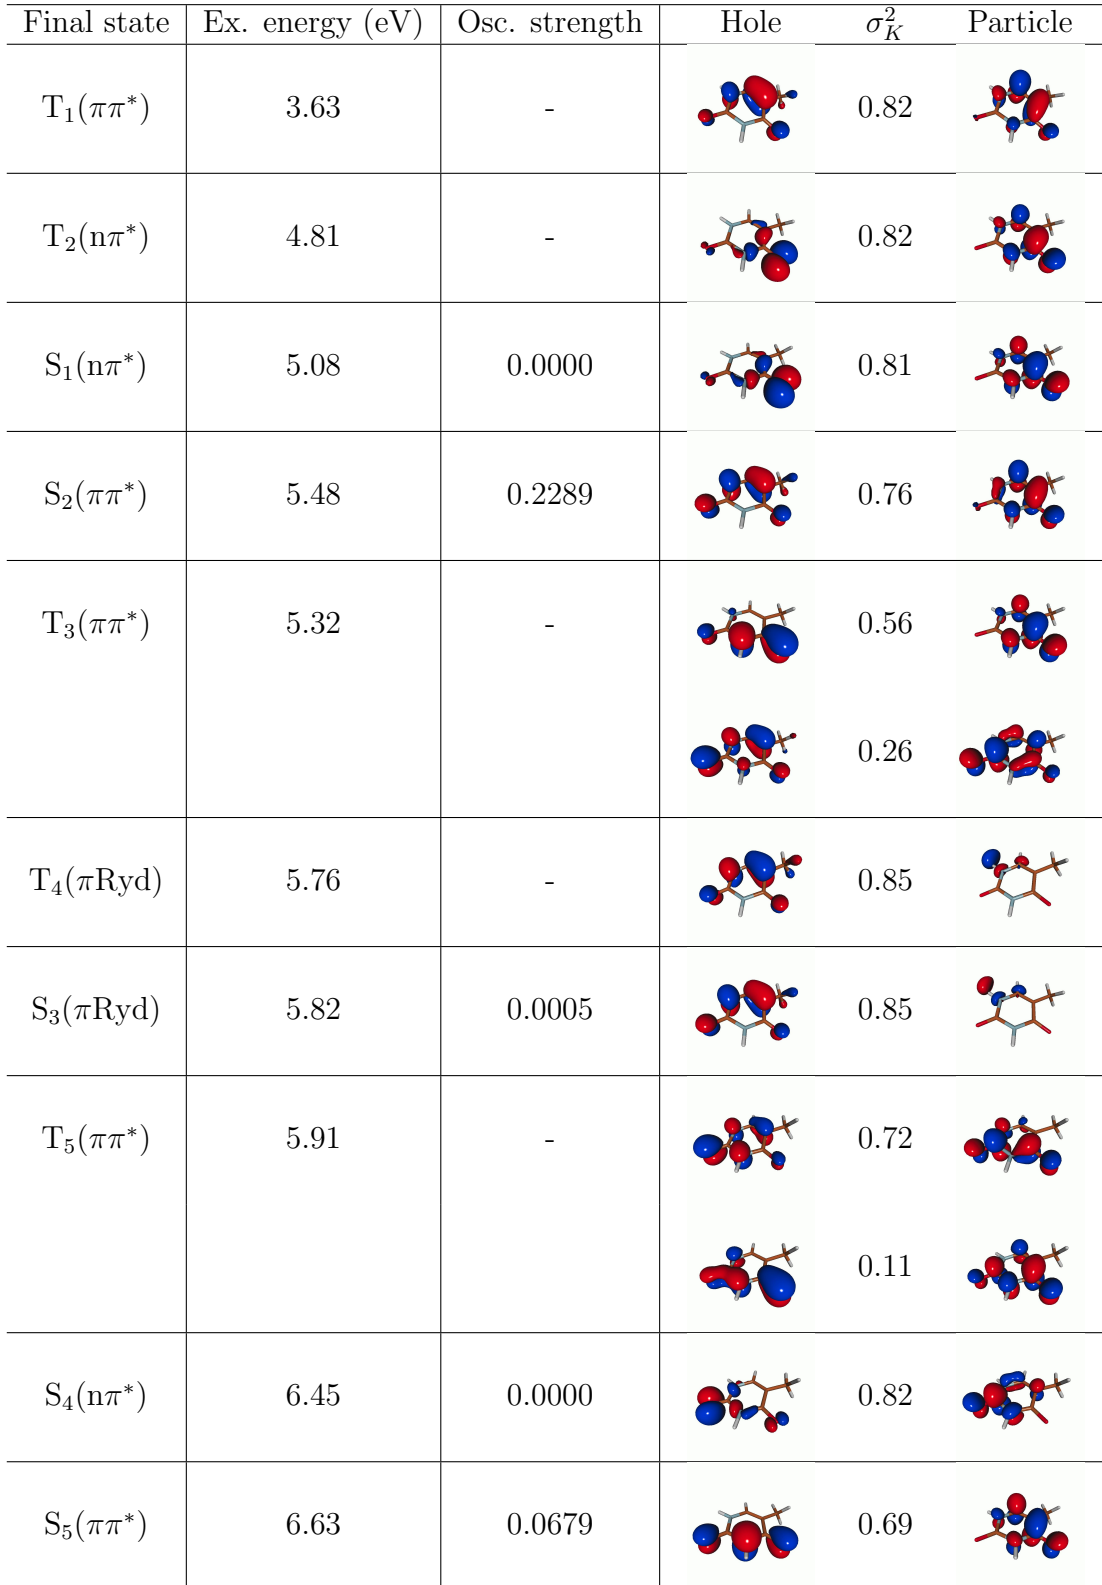   |
| $S_1(n\pi^*)$   | 5.08            | 0.0000        | 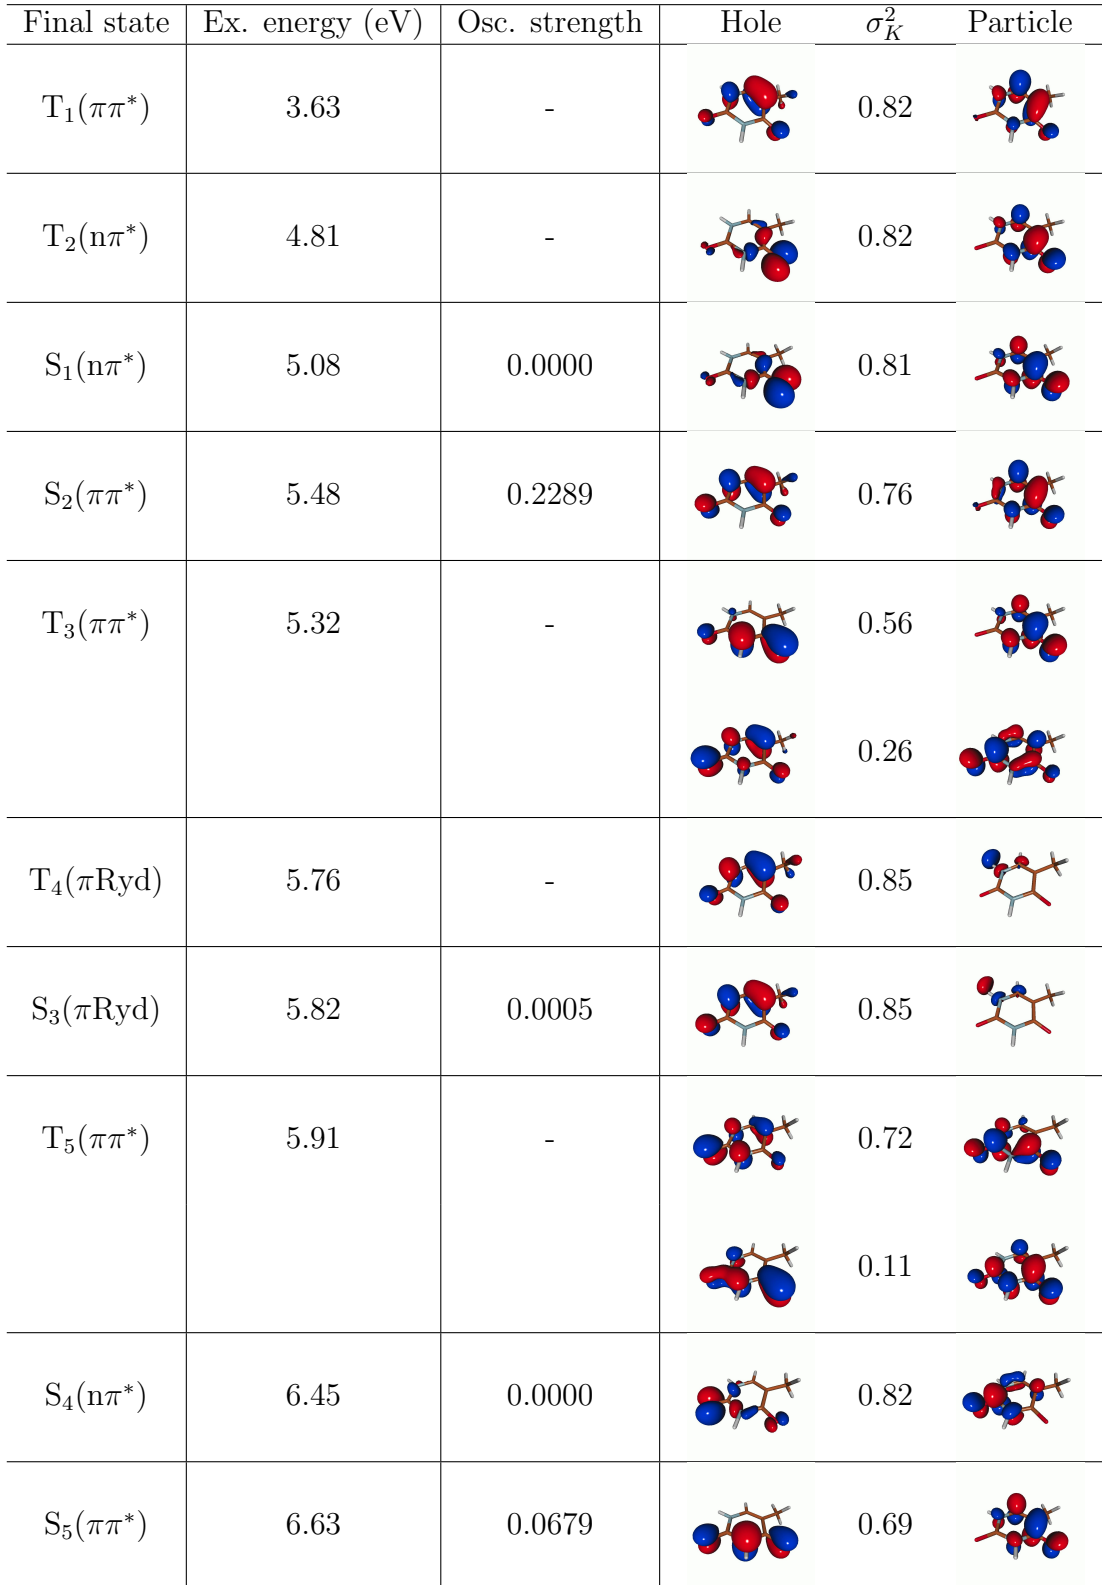   | 0.81         | 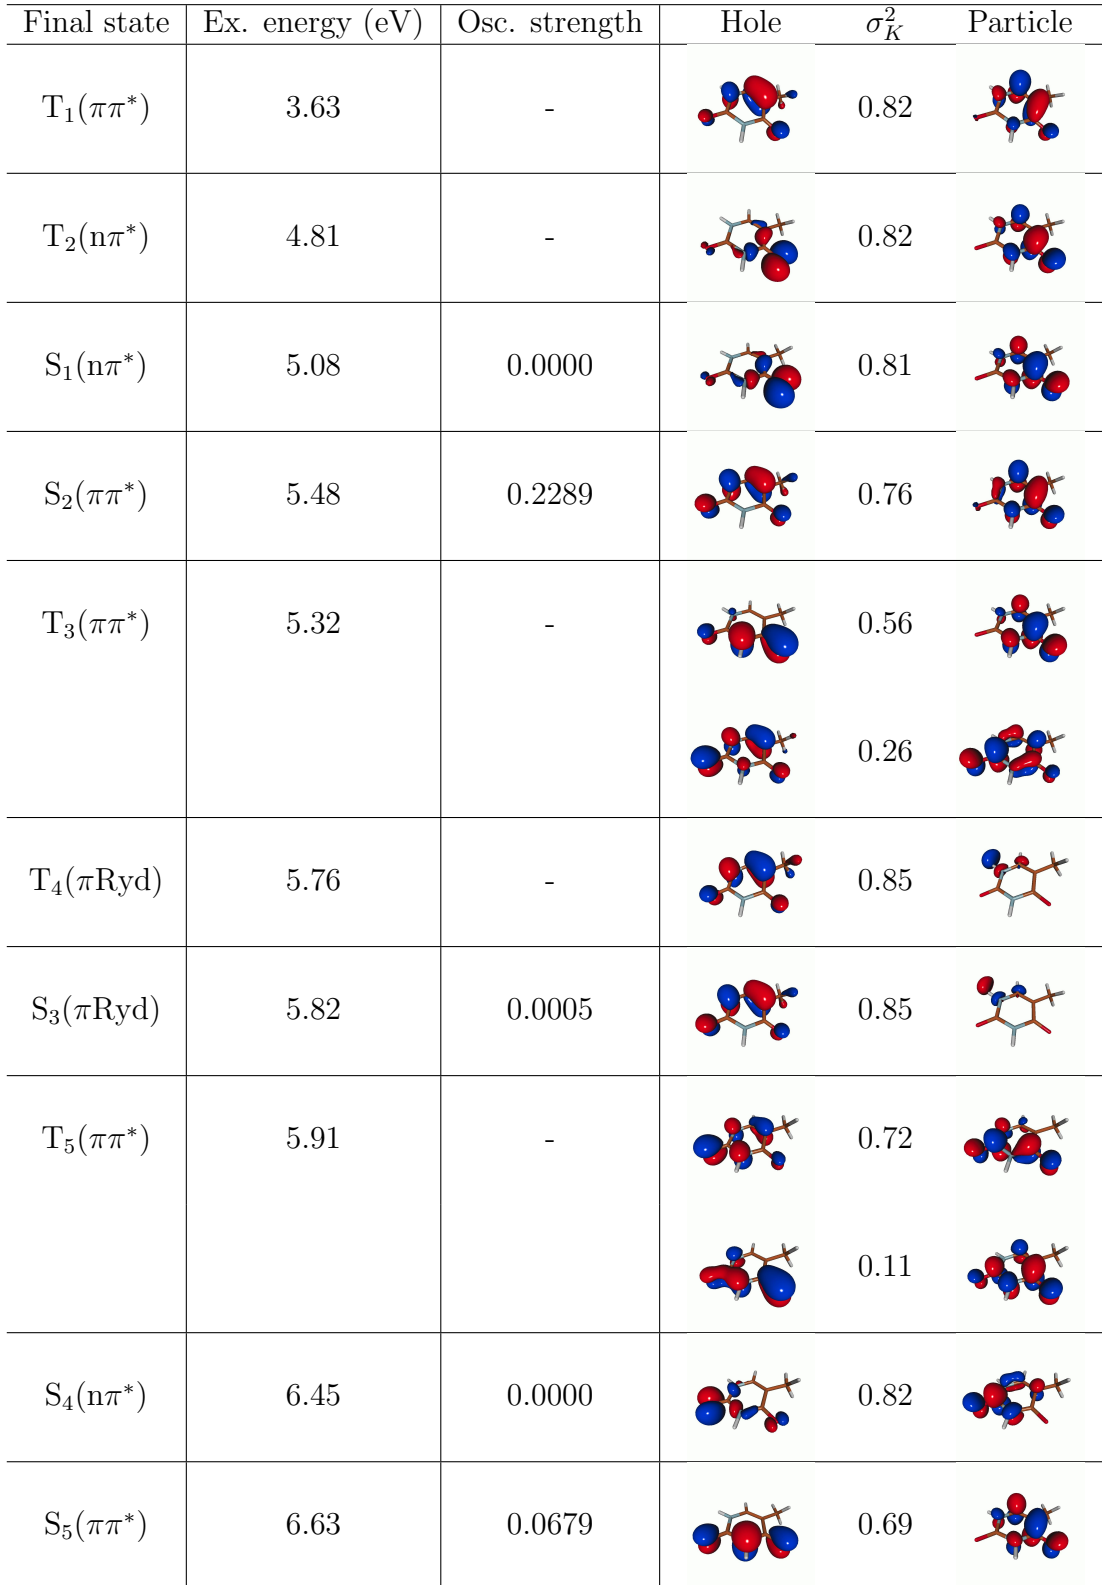   |
| $S_2(\pi\pi^*)$ | 5.48            | 0.2289        | 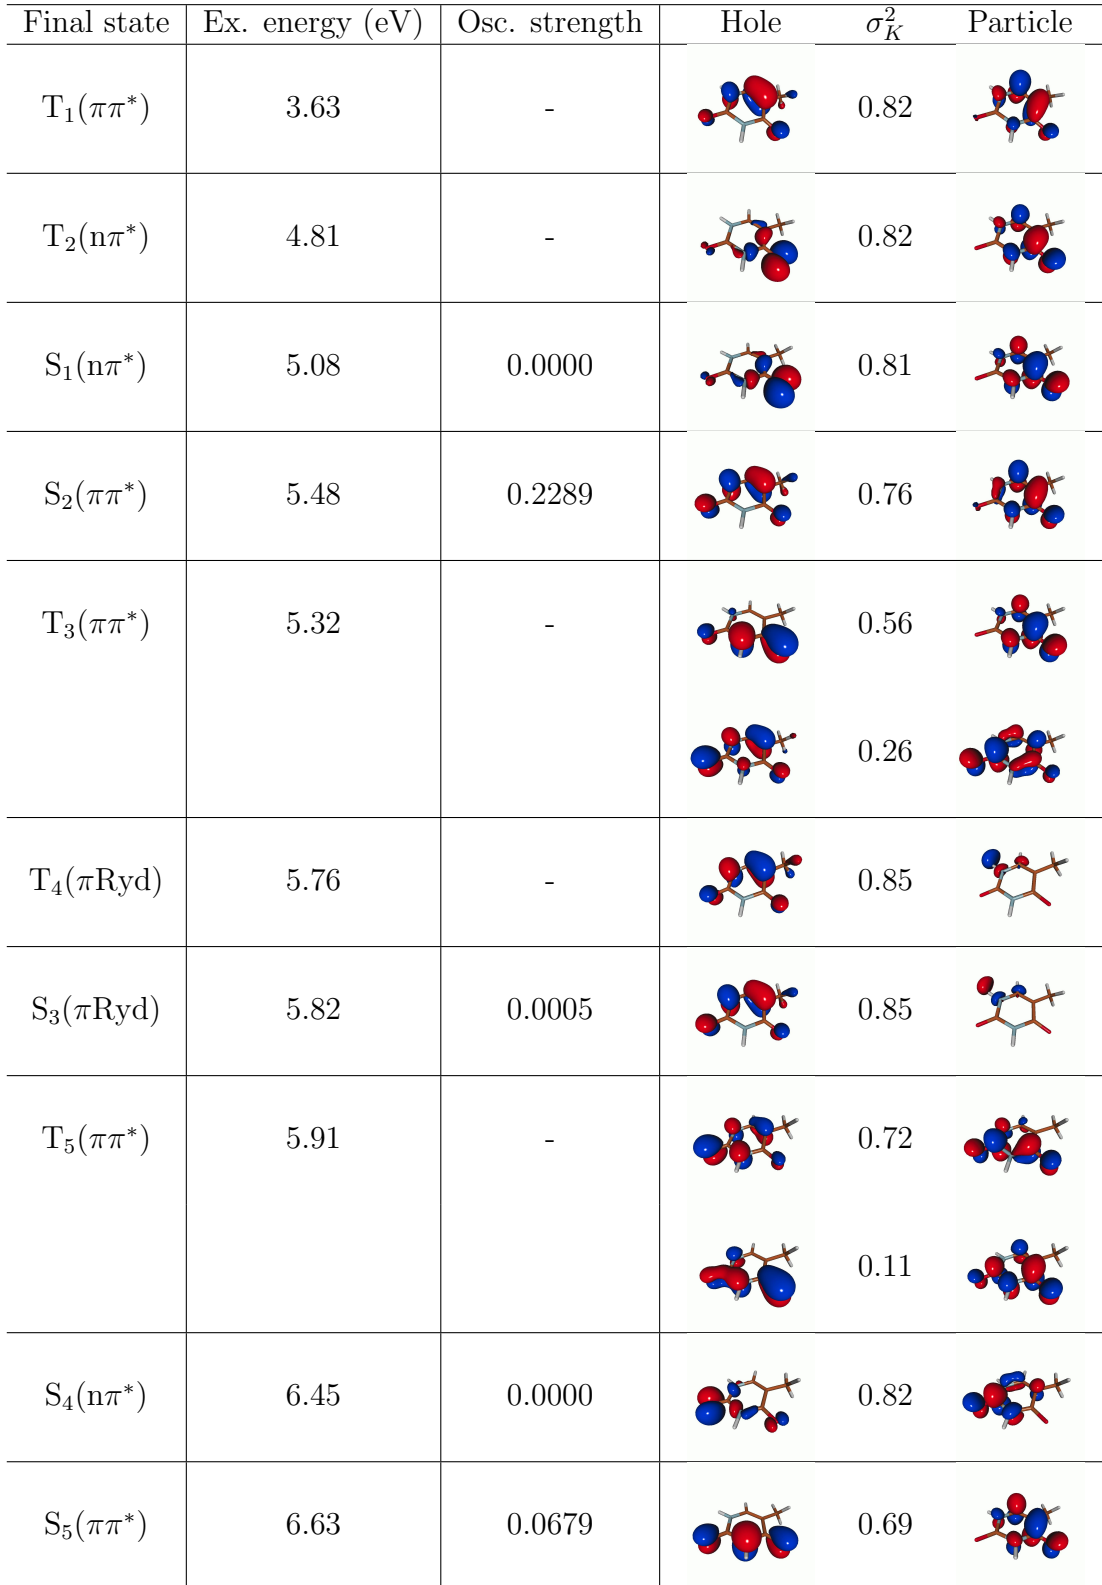   | 0.76         | 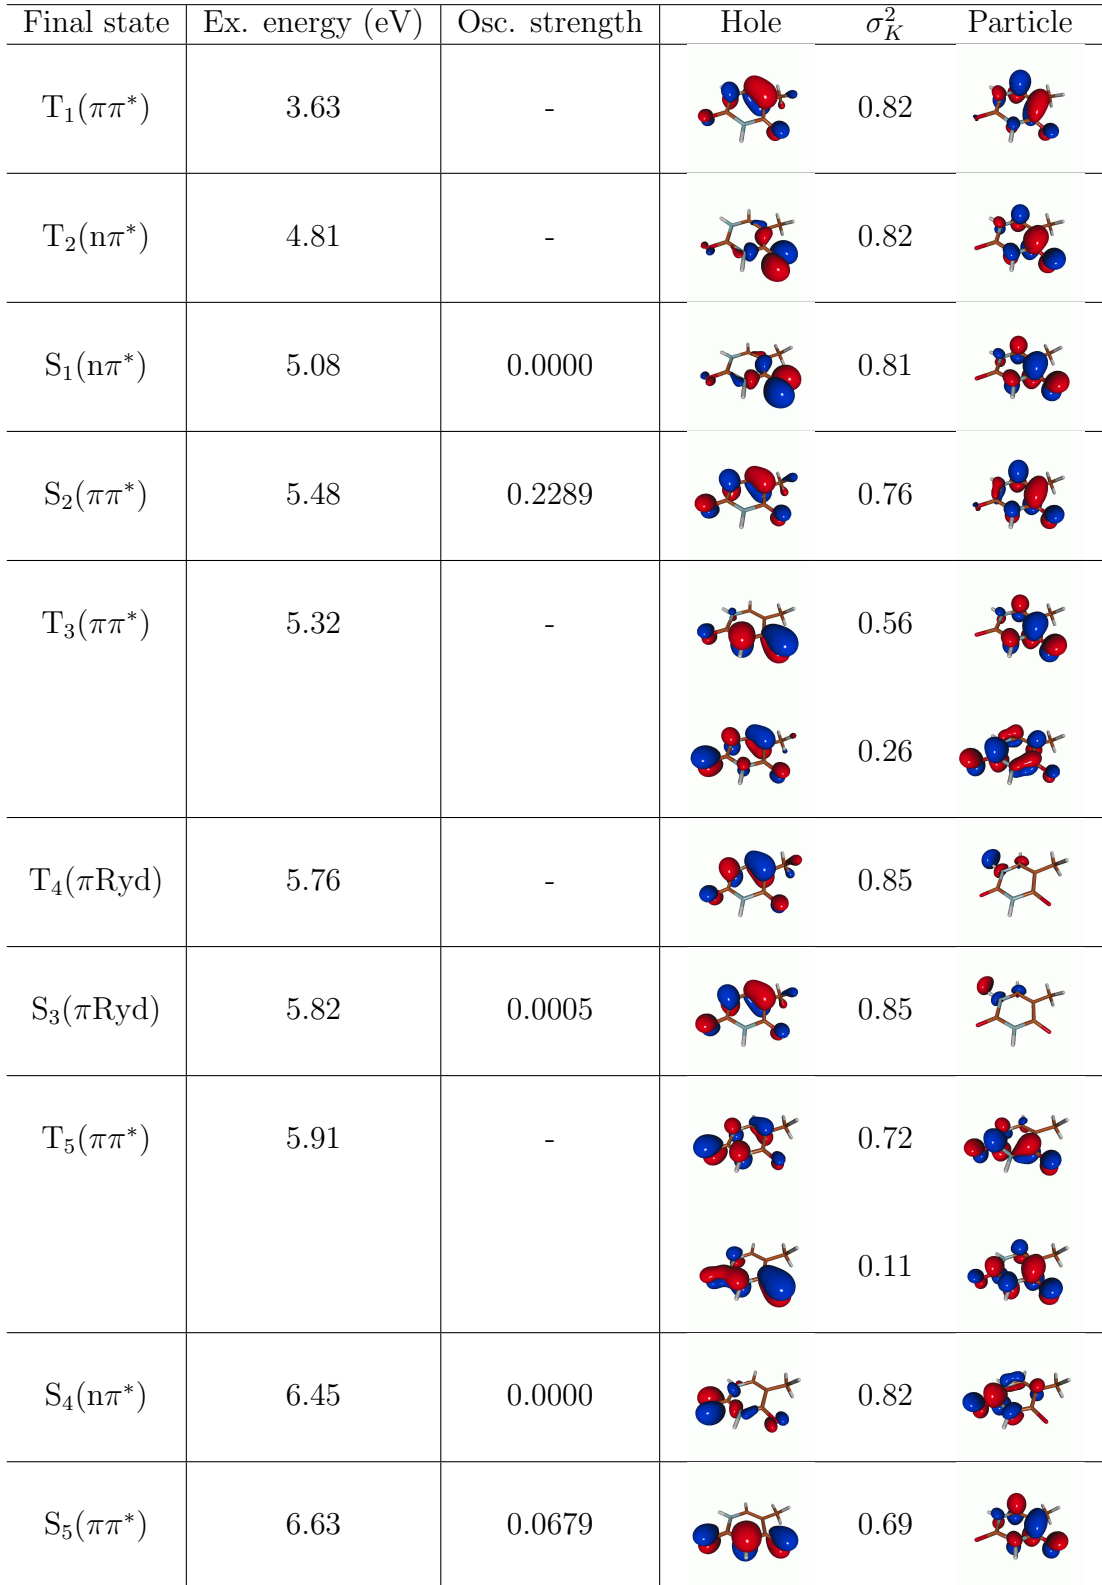   |
| $T_3(\pi\pi^*)$ | 5.32            | -             | 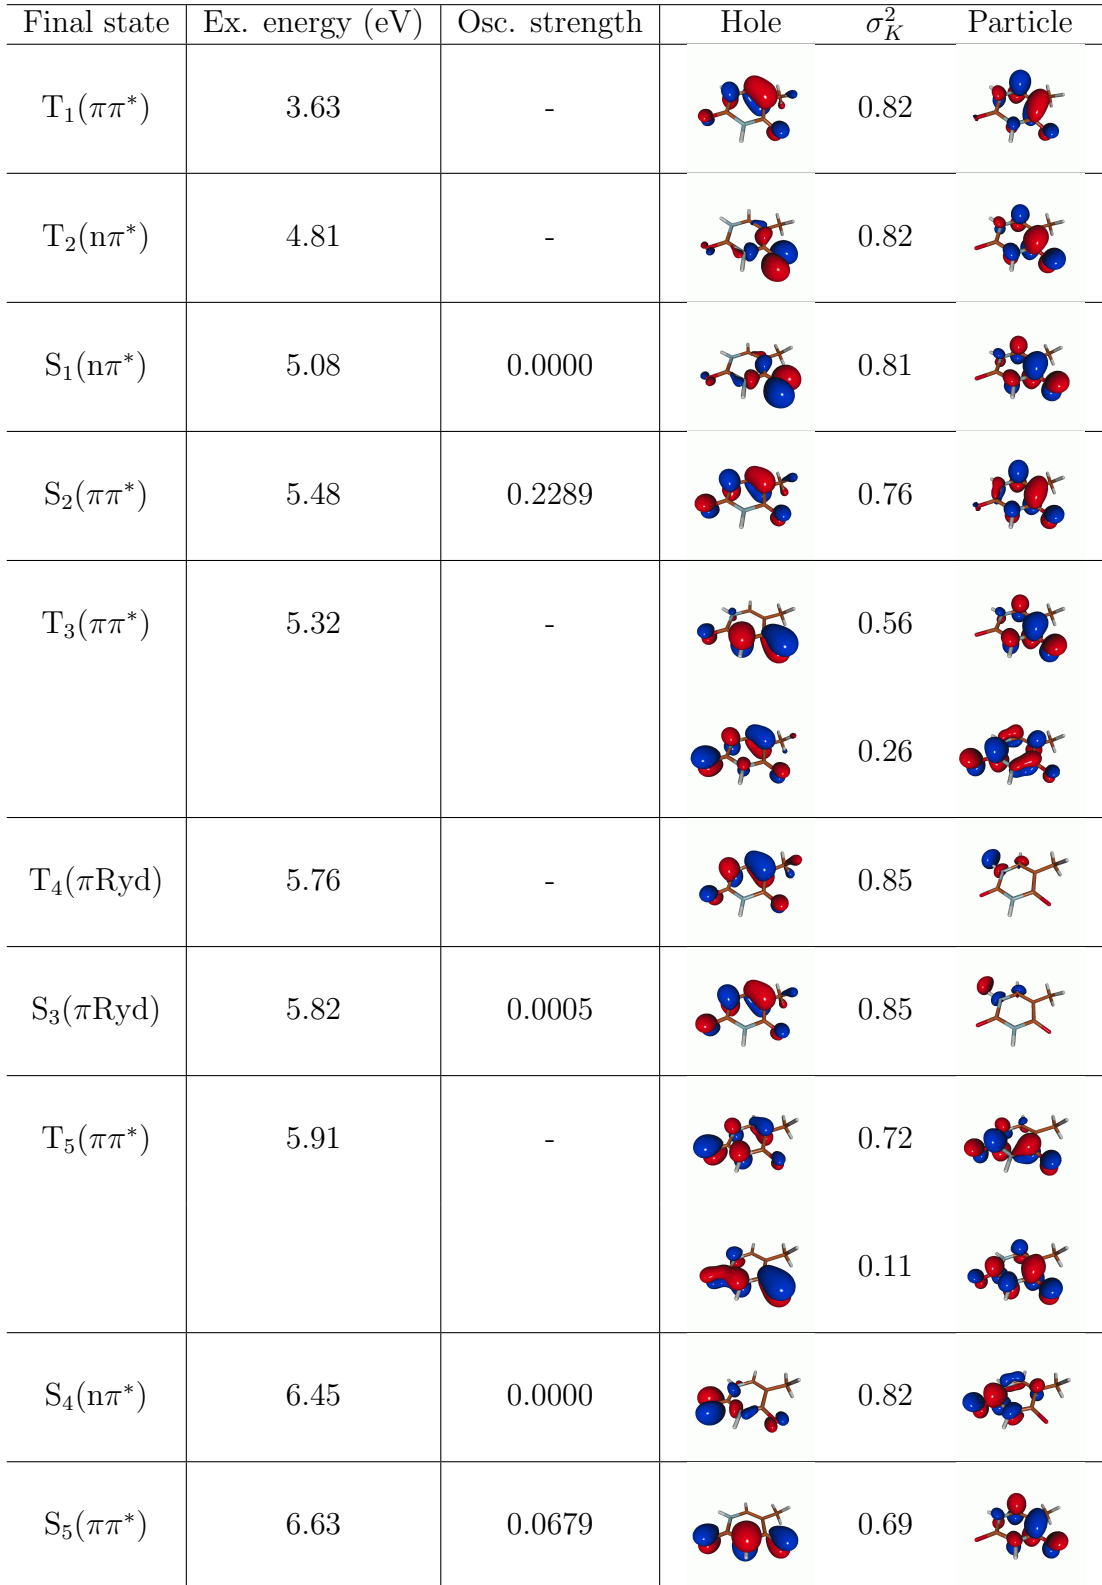  | 0.56         | 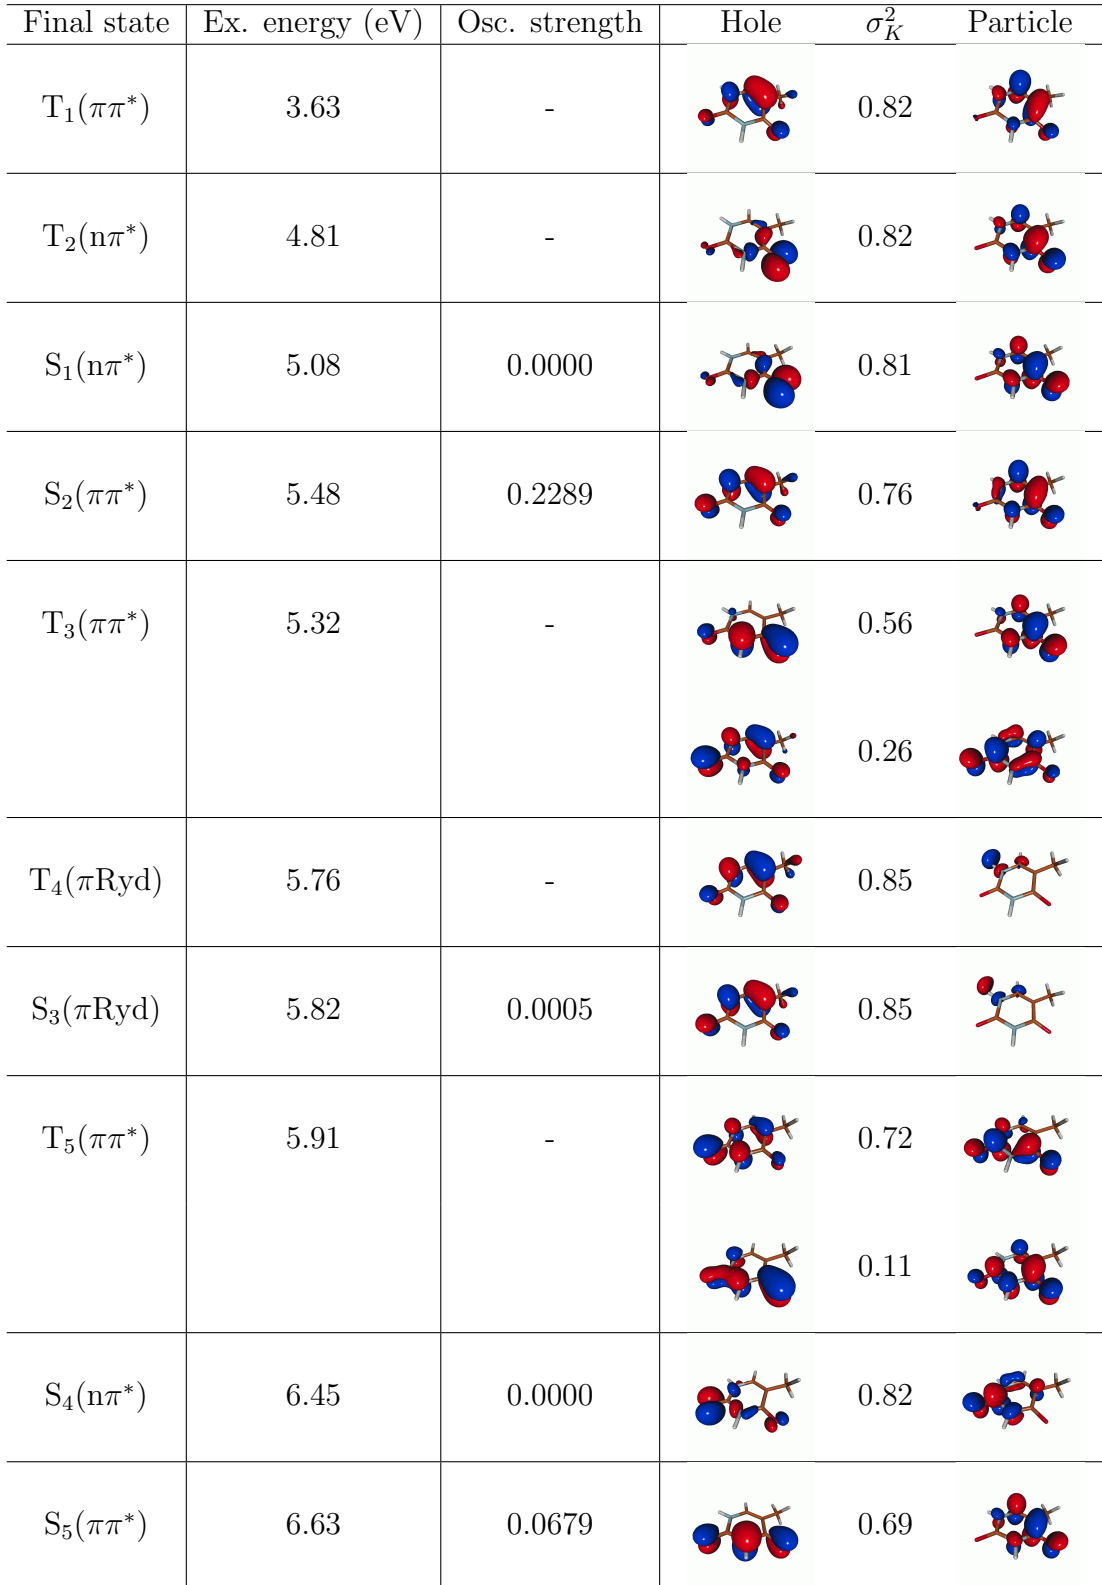  |
|                 |                 |               | 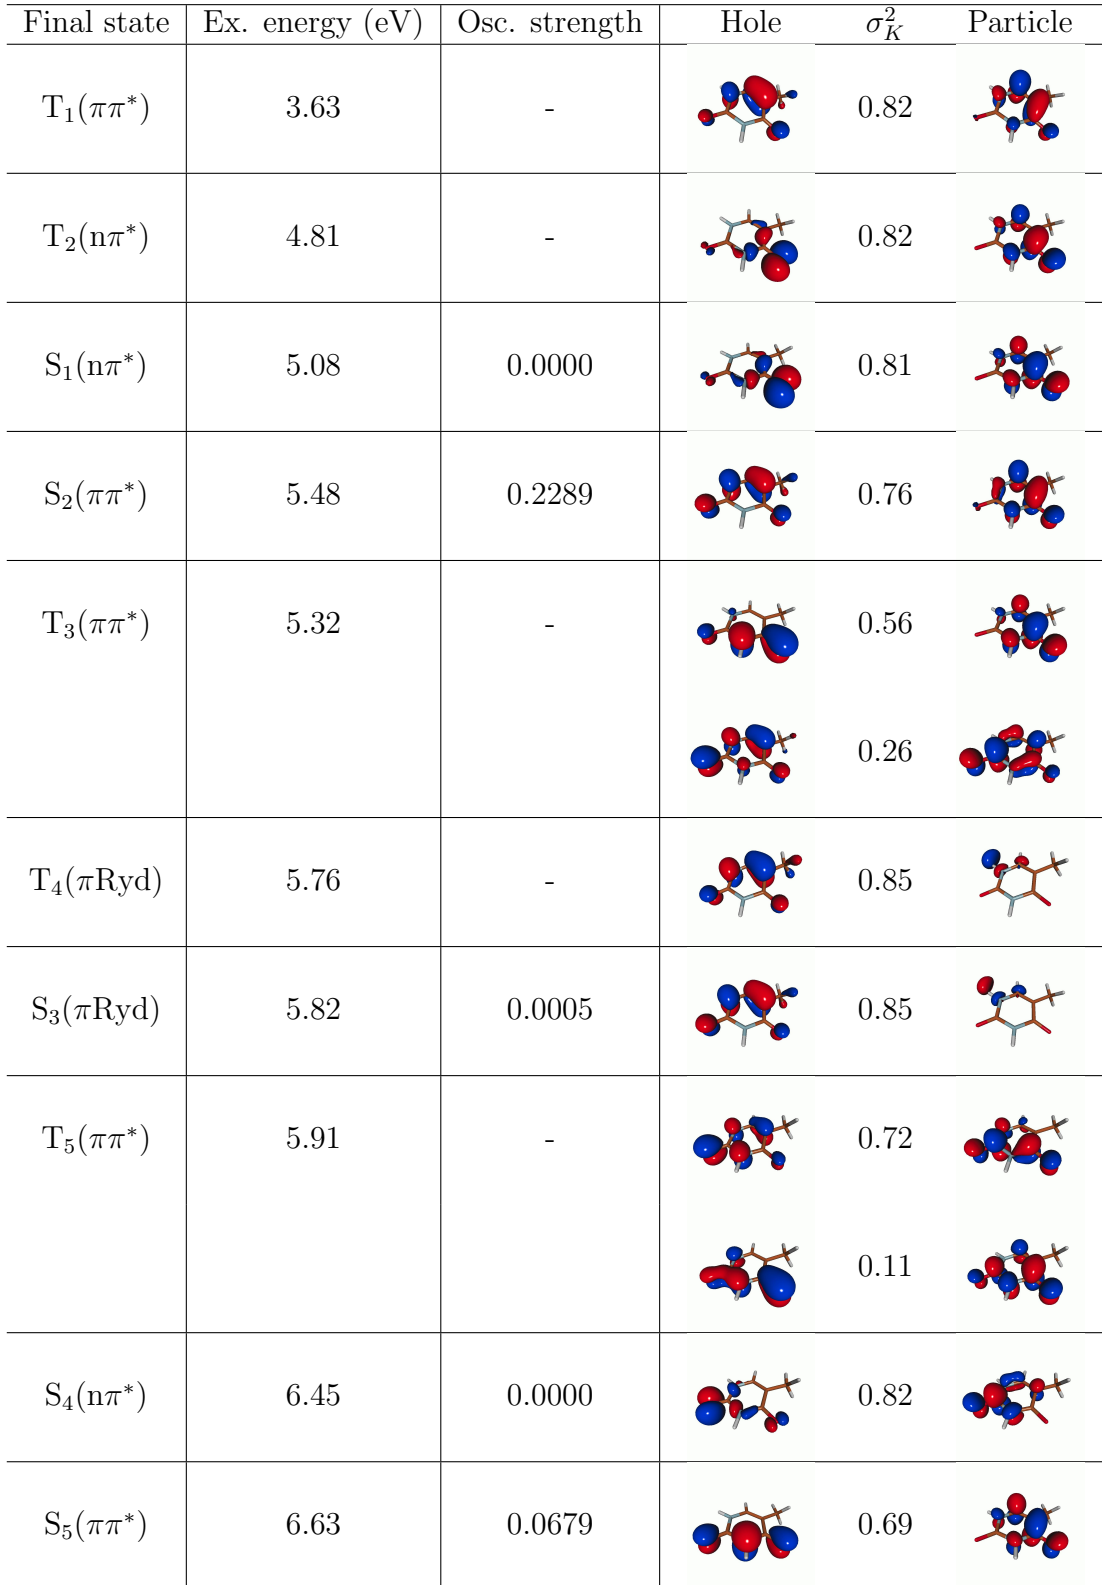 | 0.26         | 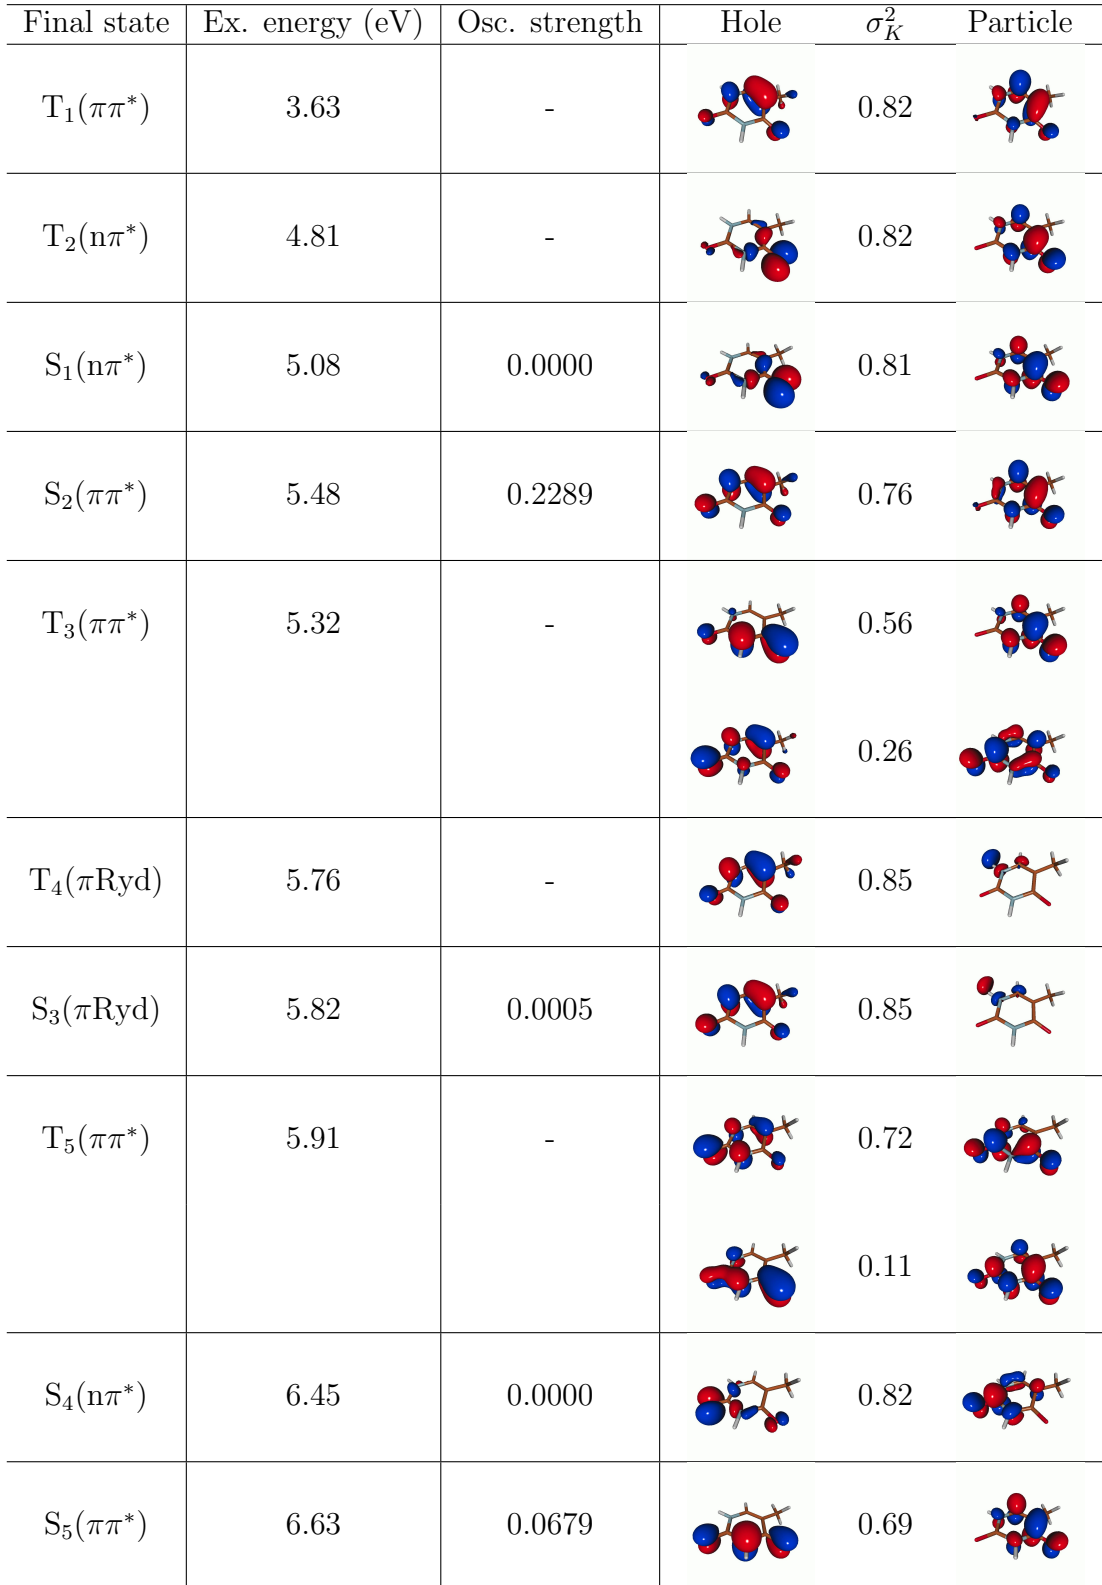 |
| $T_4(\pi Ryd)$  | 5.76            | -             | 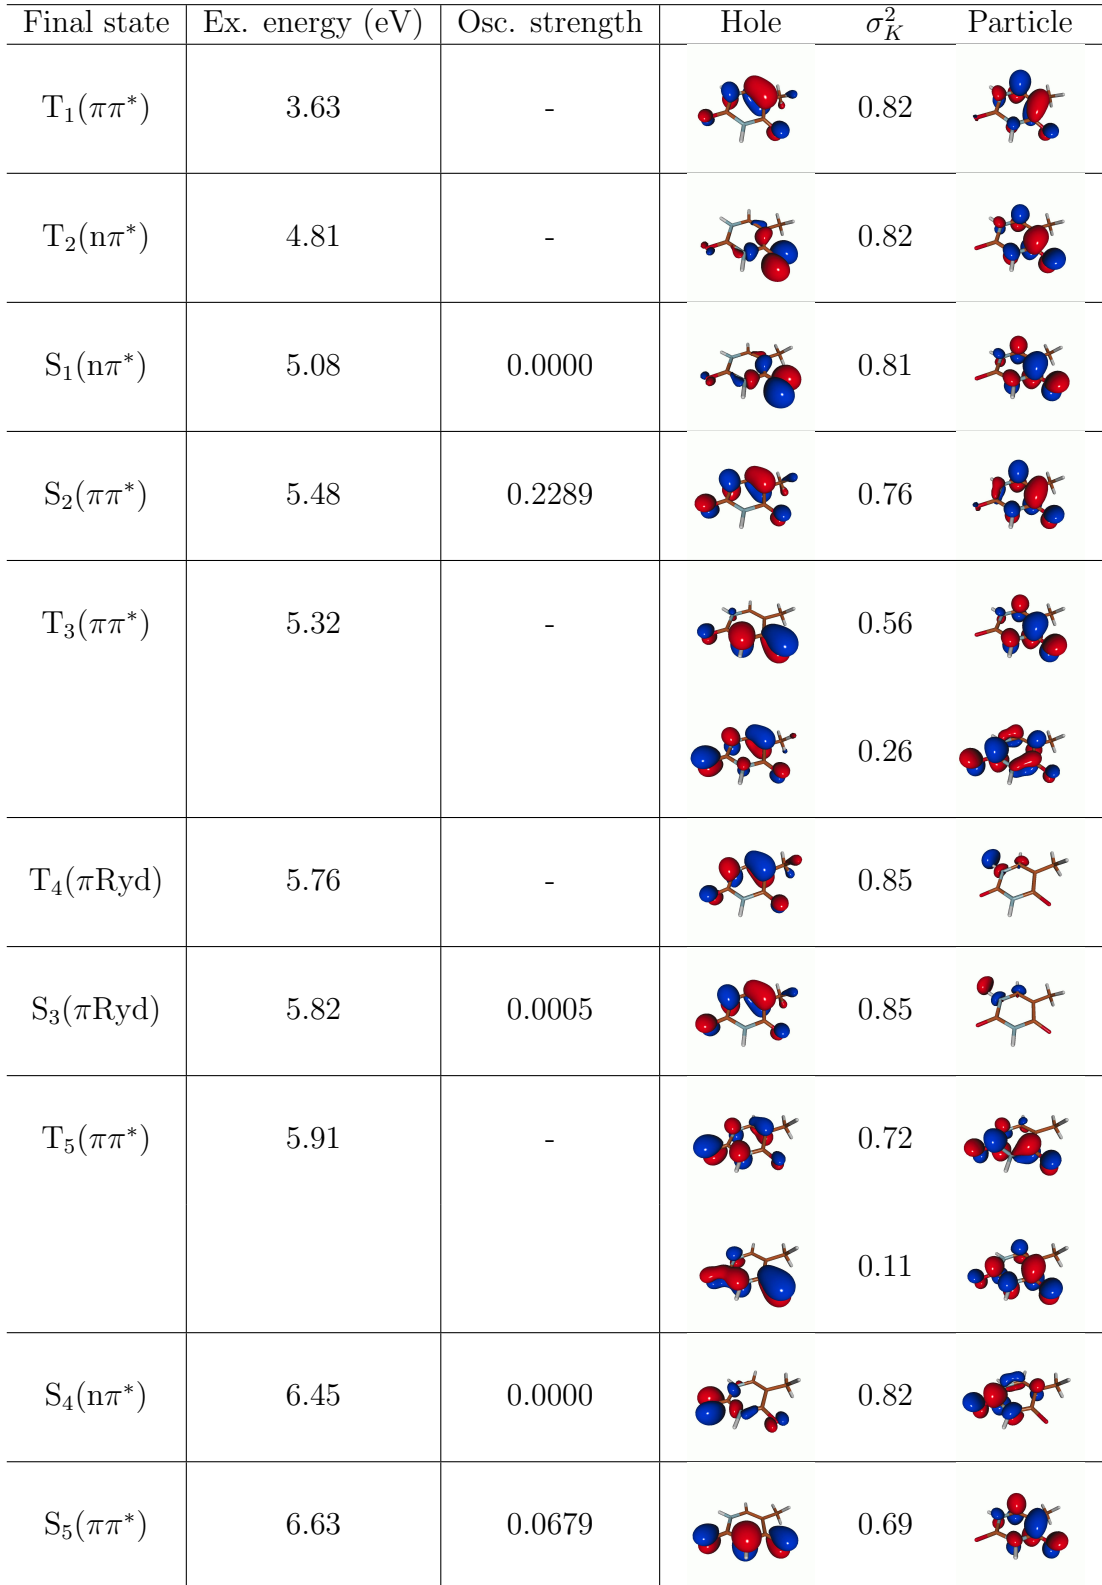 | 0.85         | 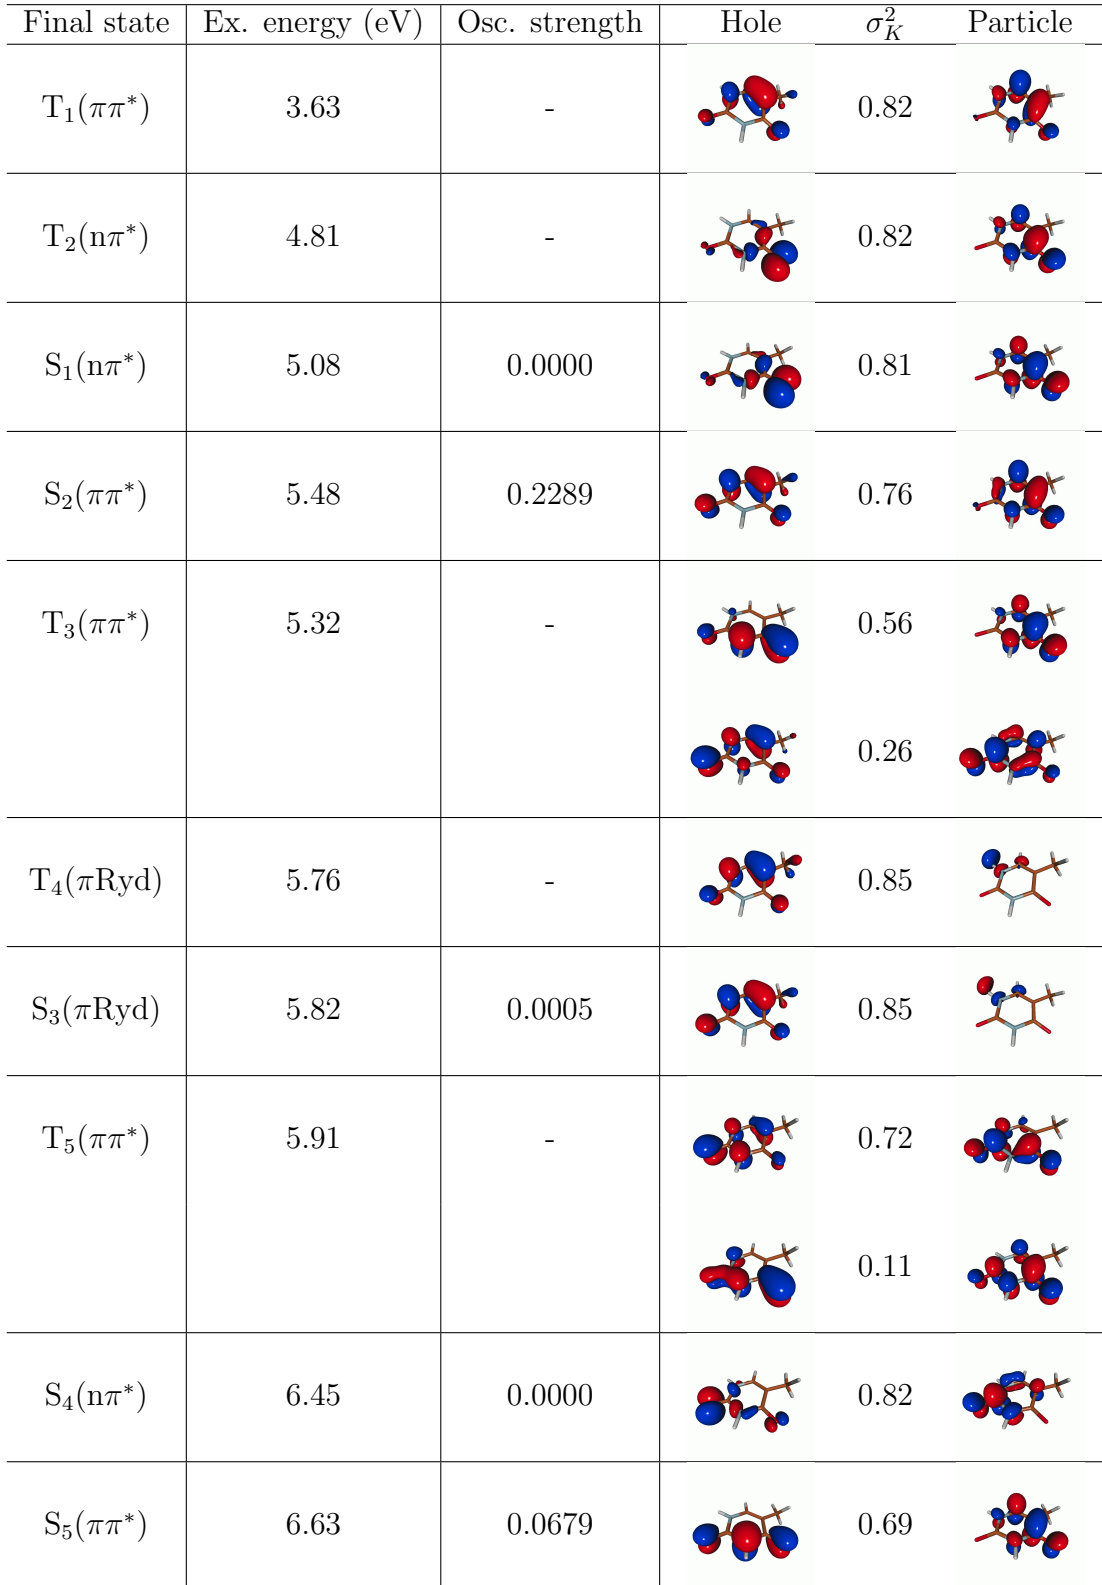 |
| $S_3(\pi Ryd)$  | 5.82            | 0.0005        | 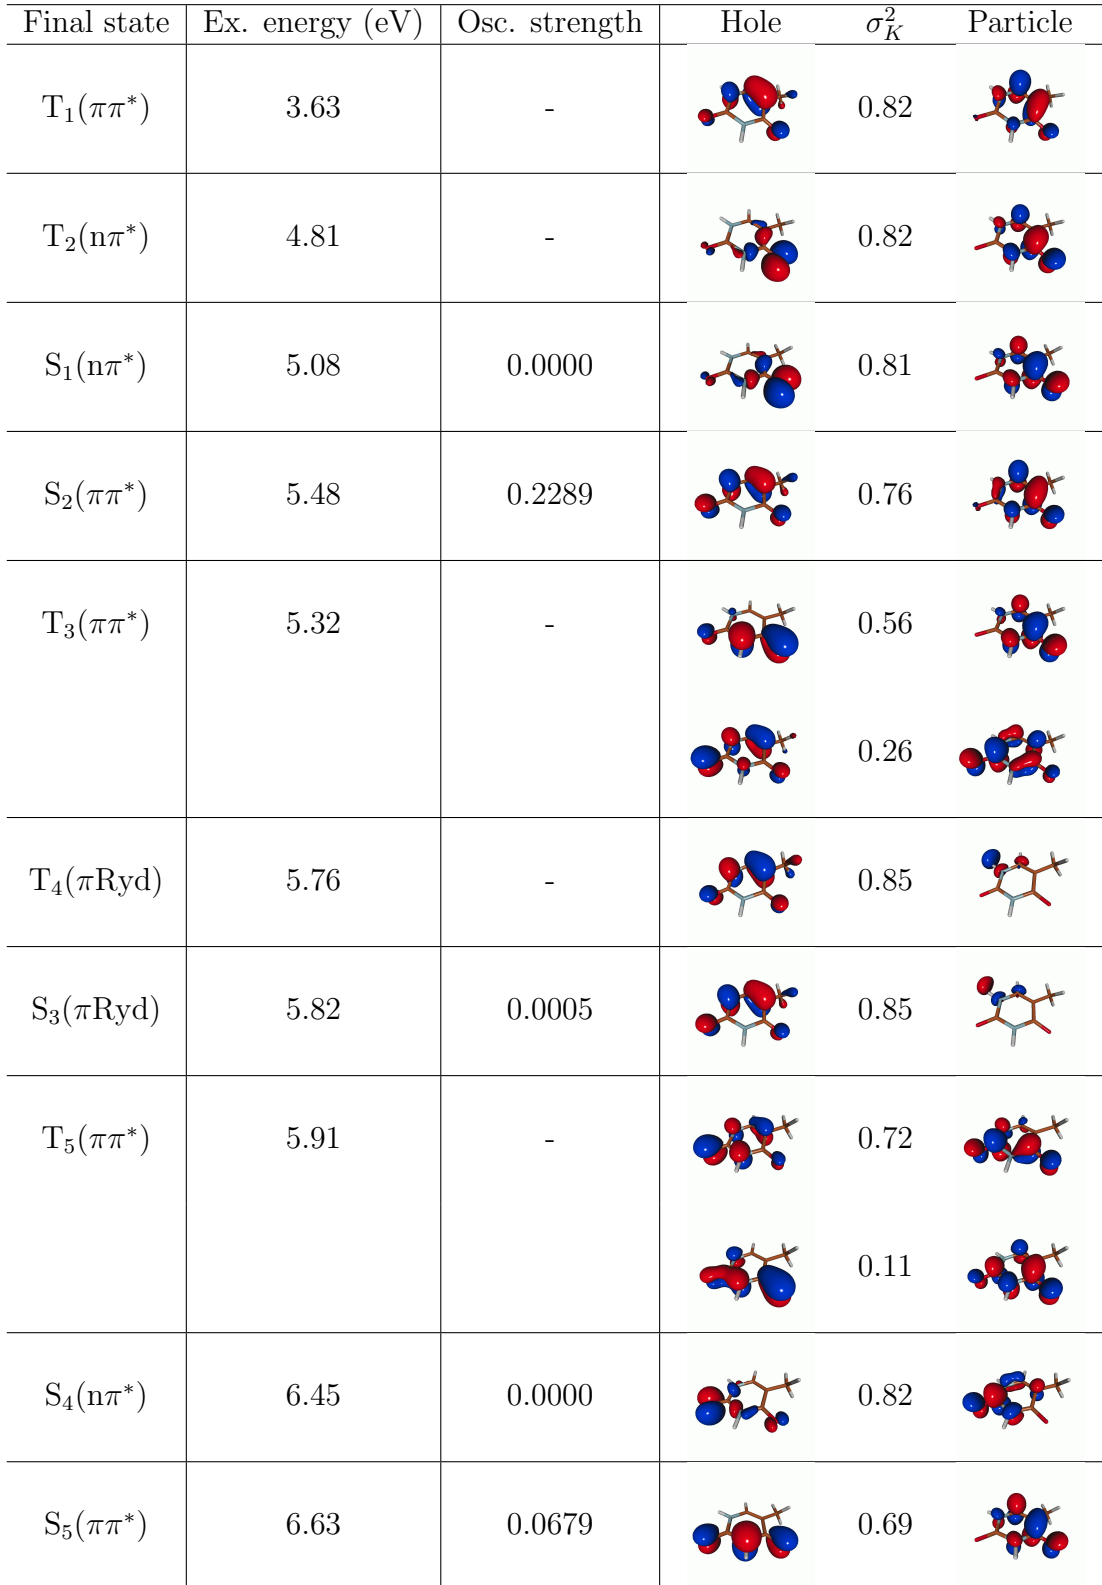 | 0.85         | 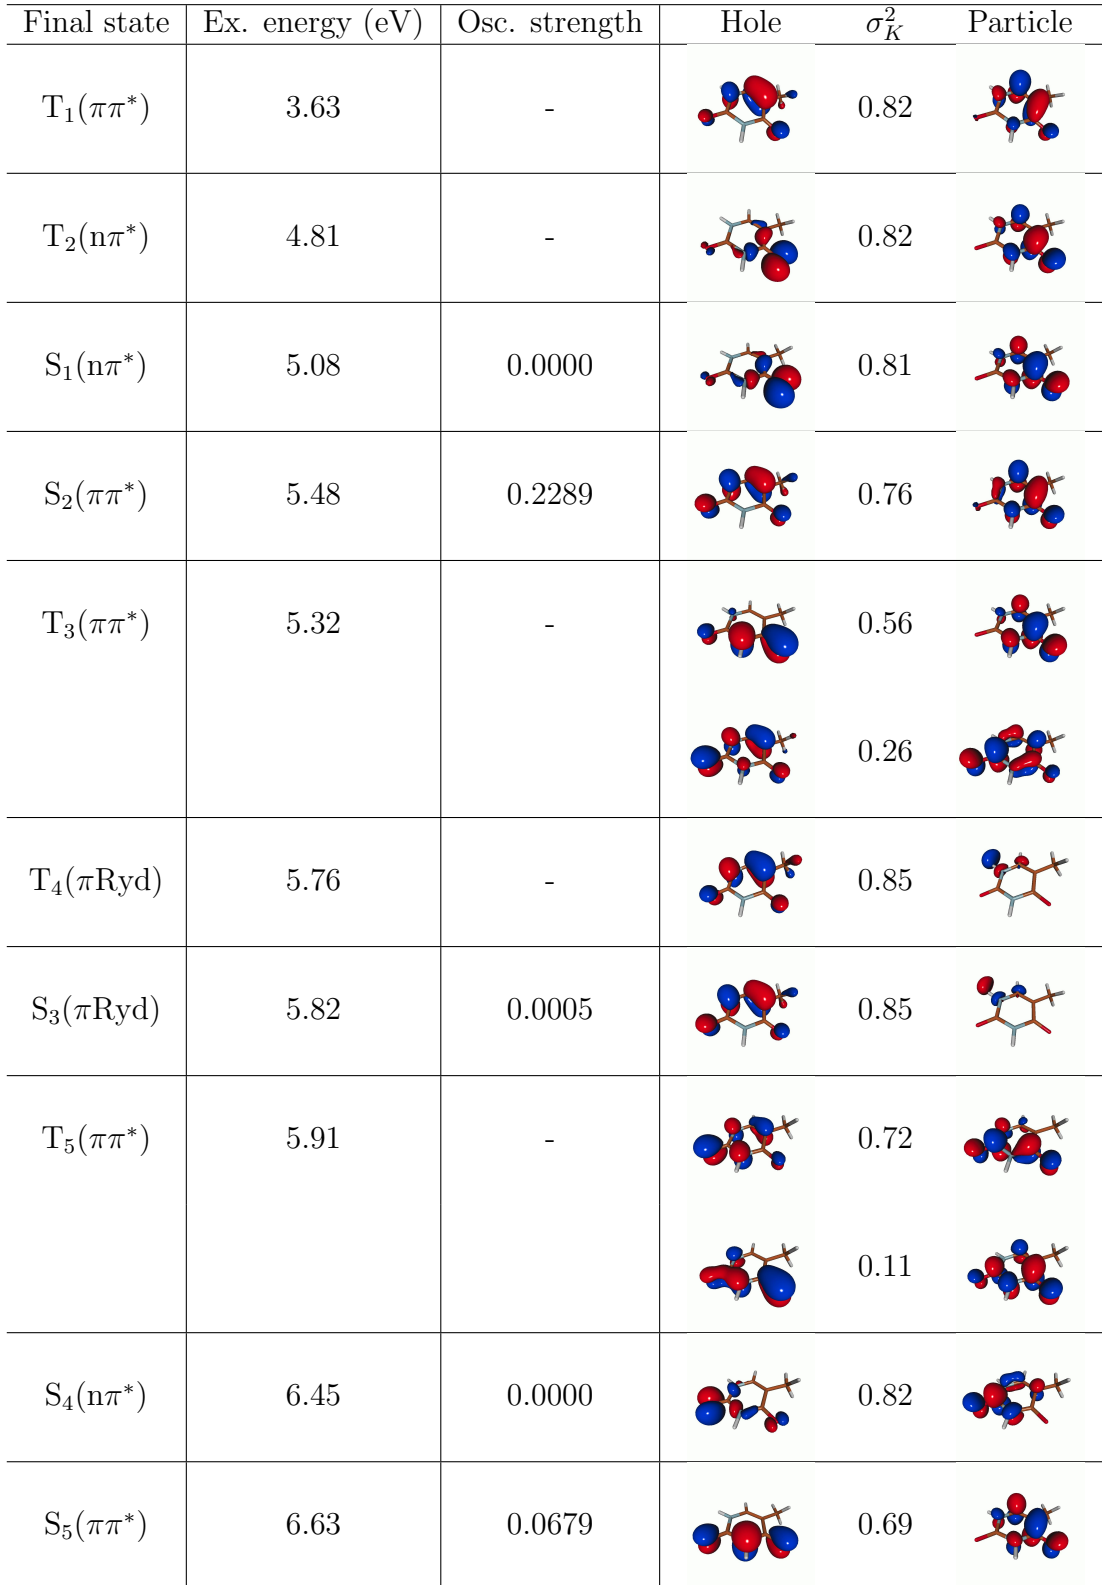 |
| $T_5(\pi\pi^*)$ | 5.91            | -             | 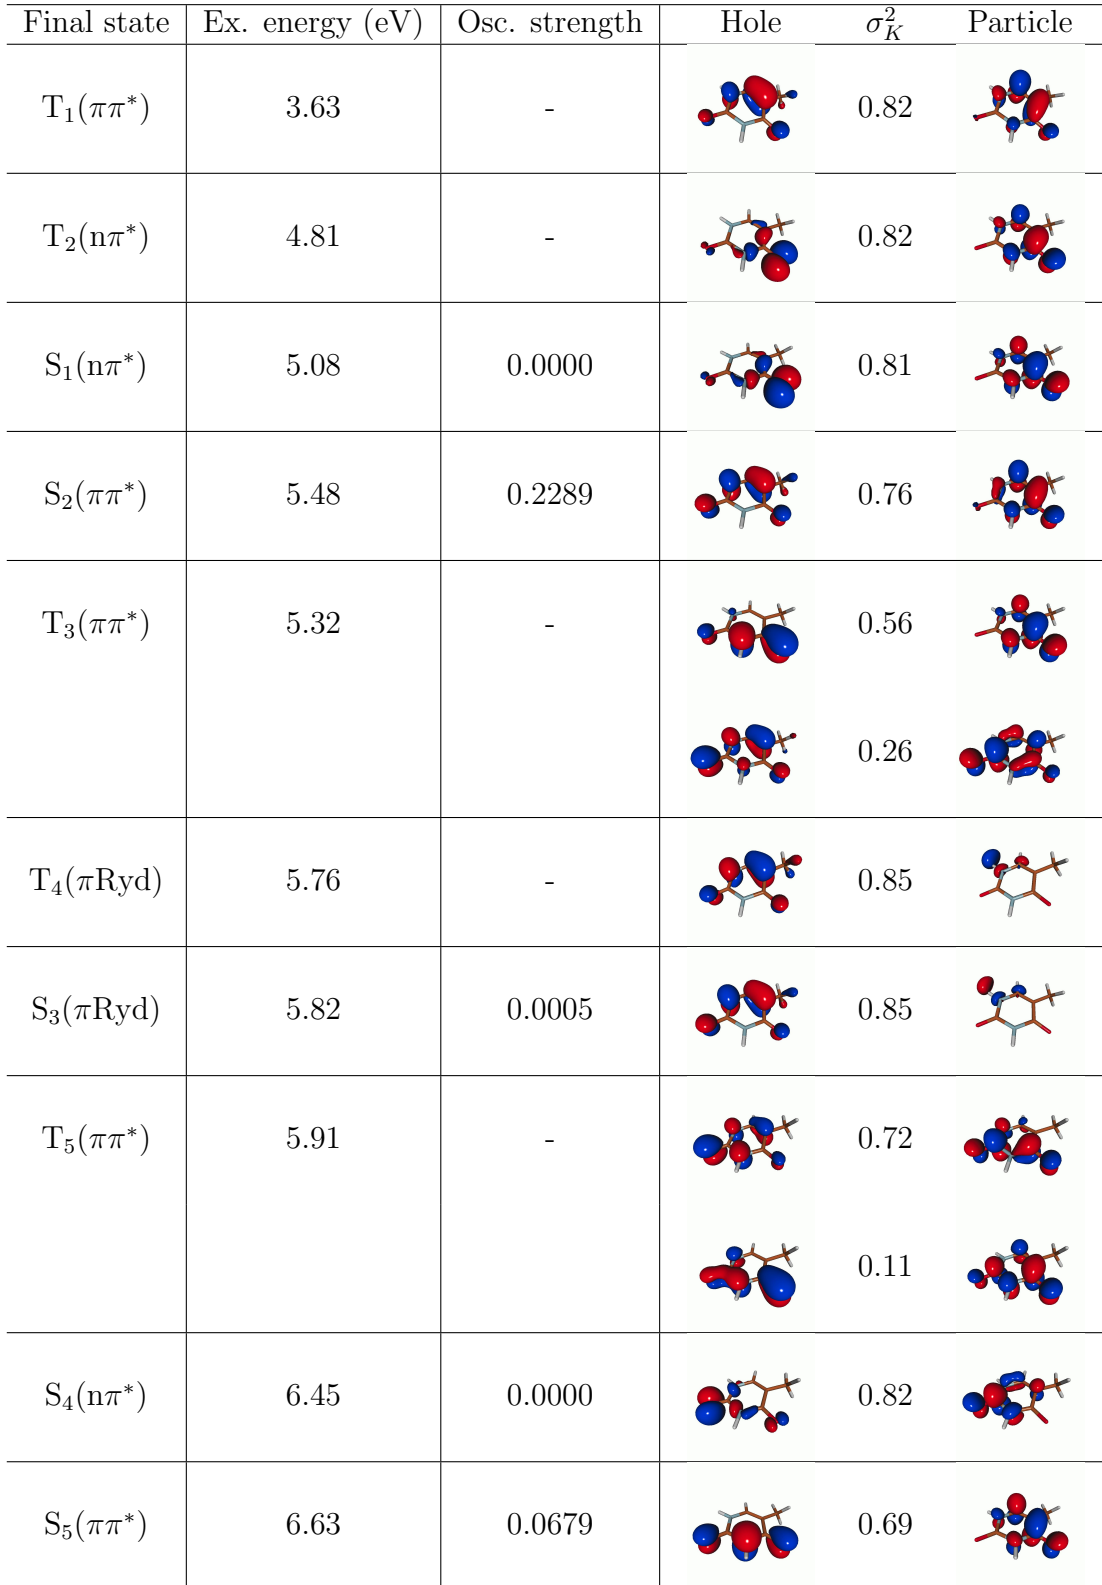 | 0.72         | 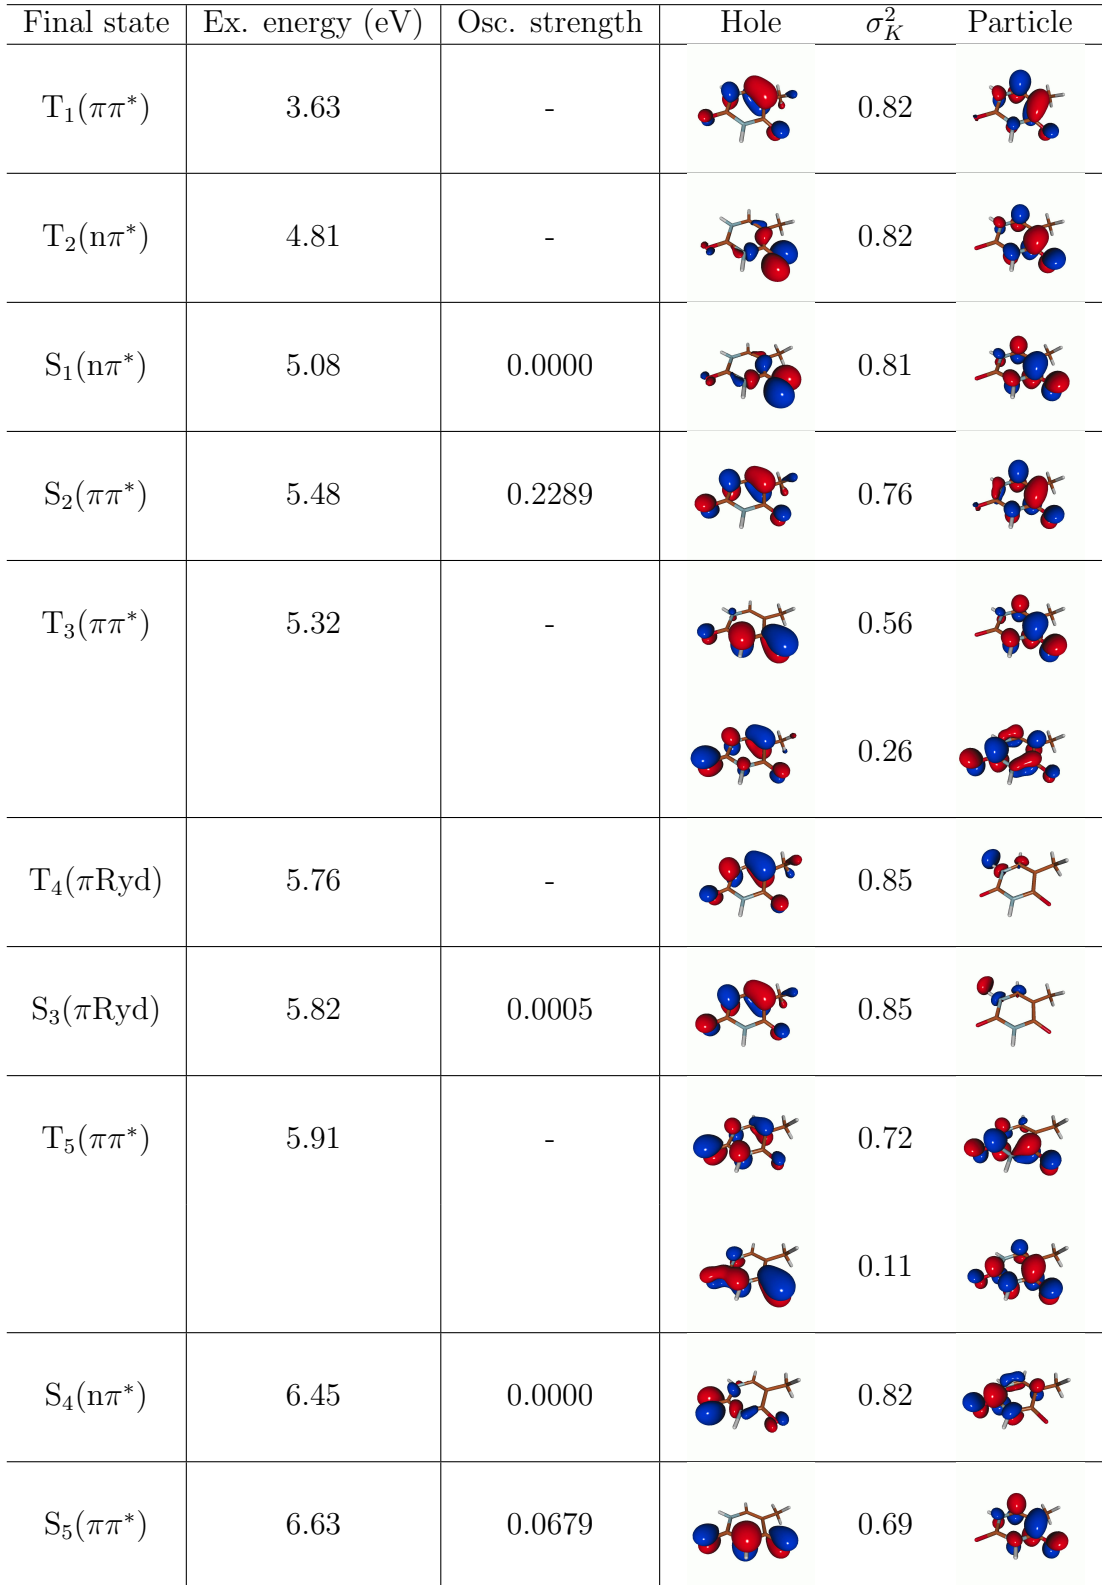 |
|                 |                 |               | 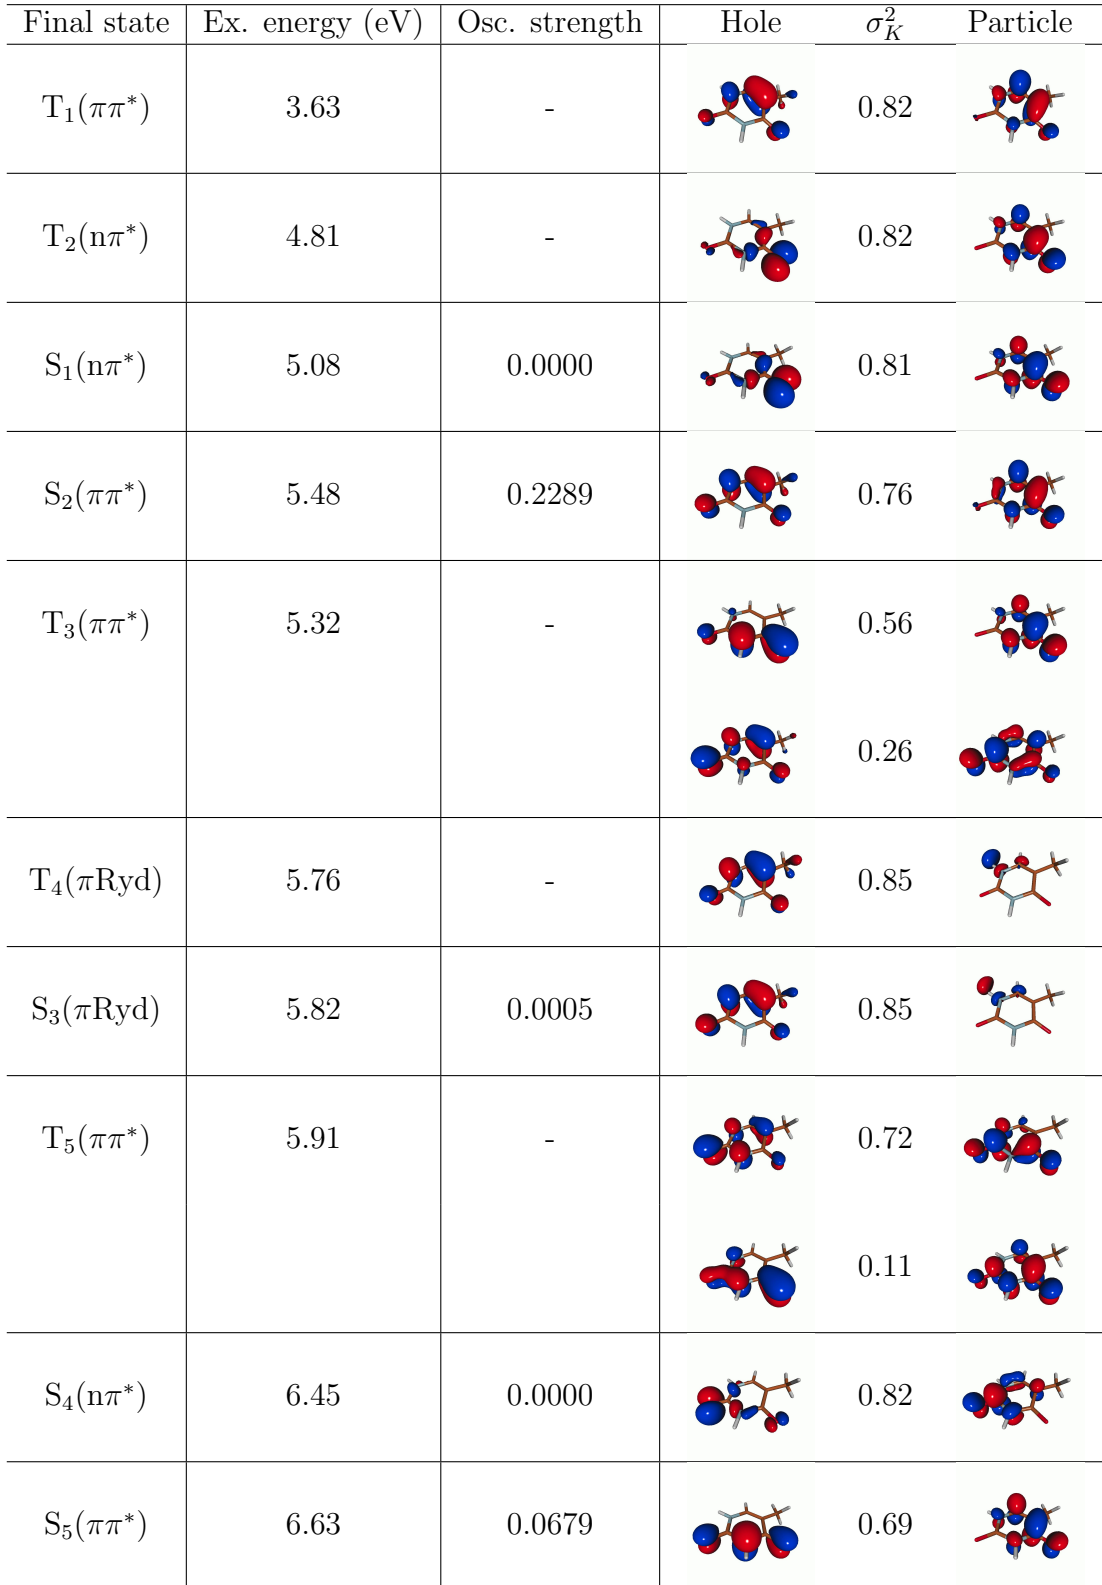 | 0.11         | 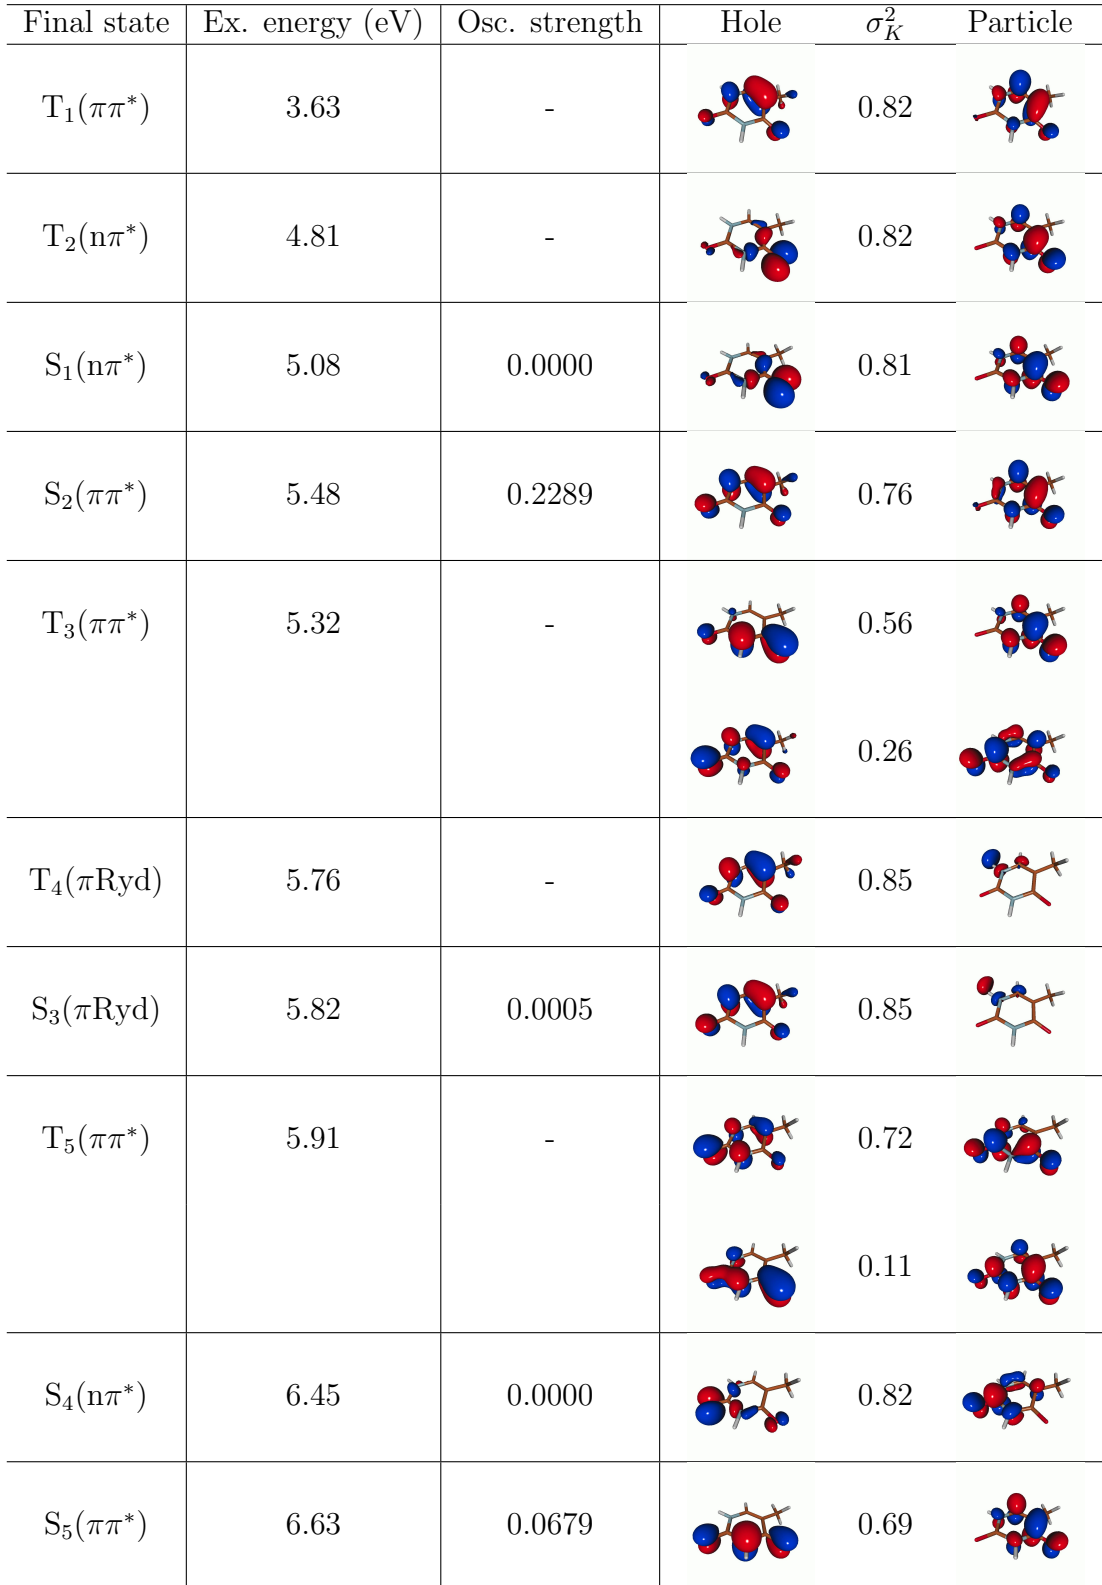 |
| $S_4(n\pi^*)$   | 6.45            | 0.0000        | 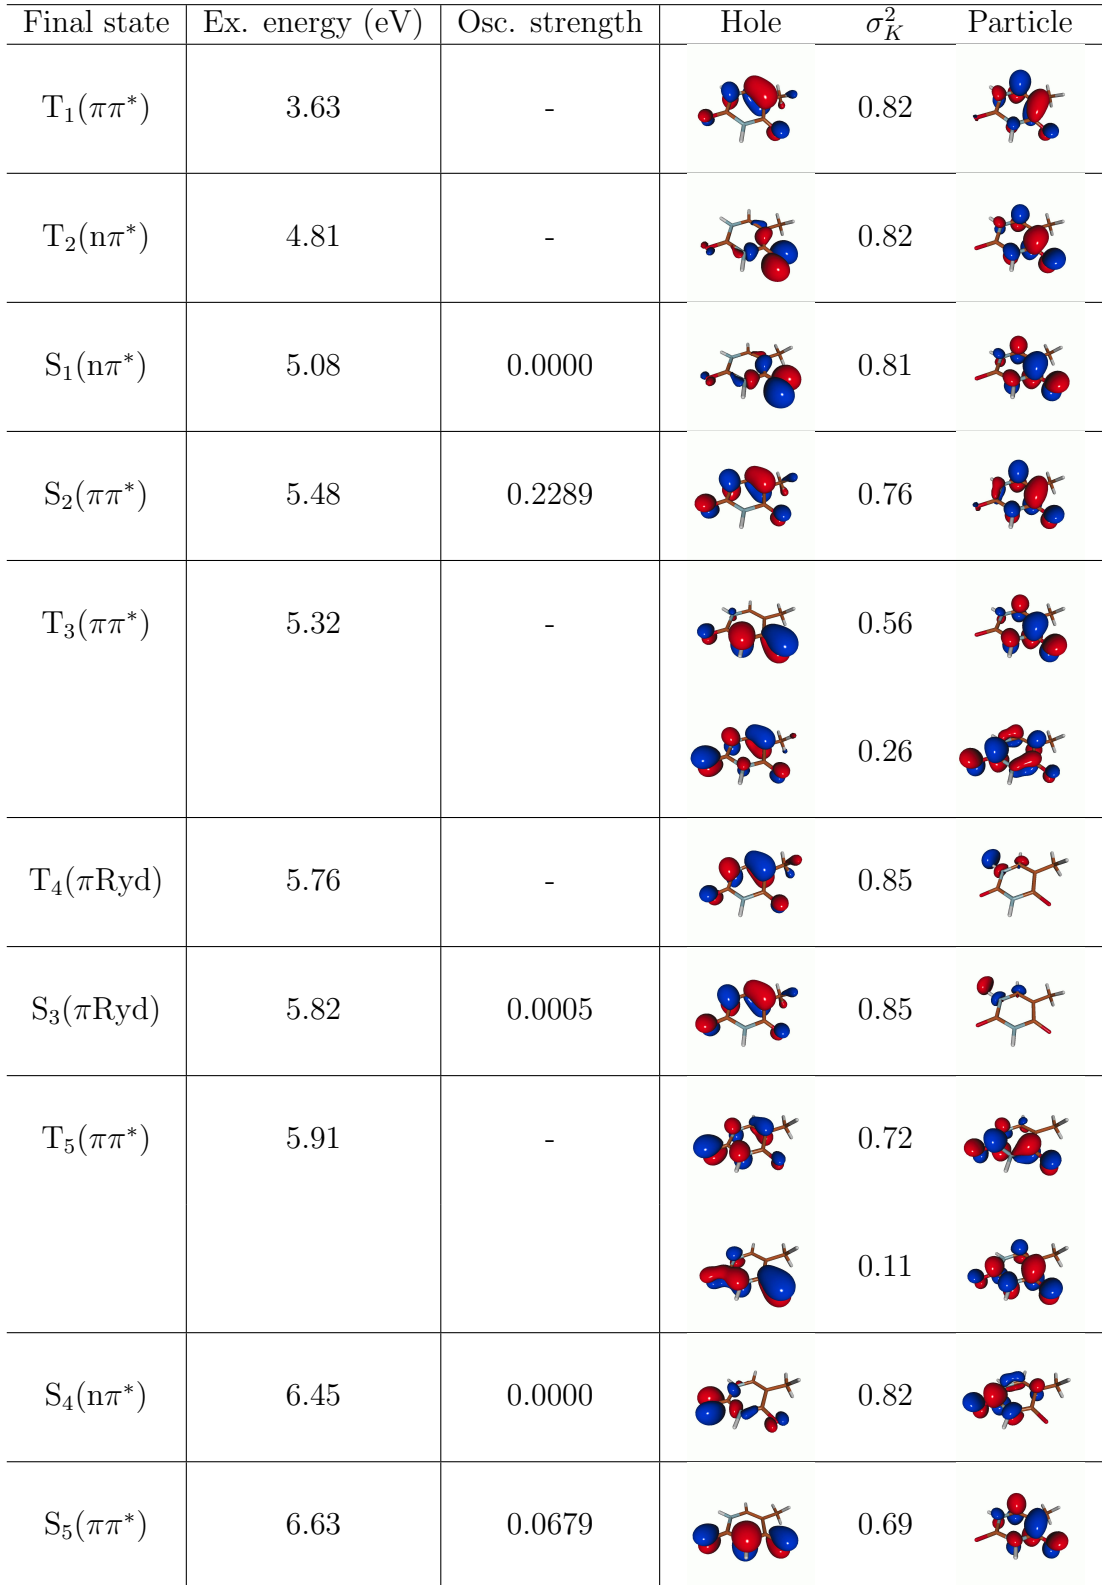 | 0.82         | 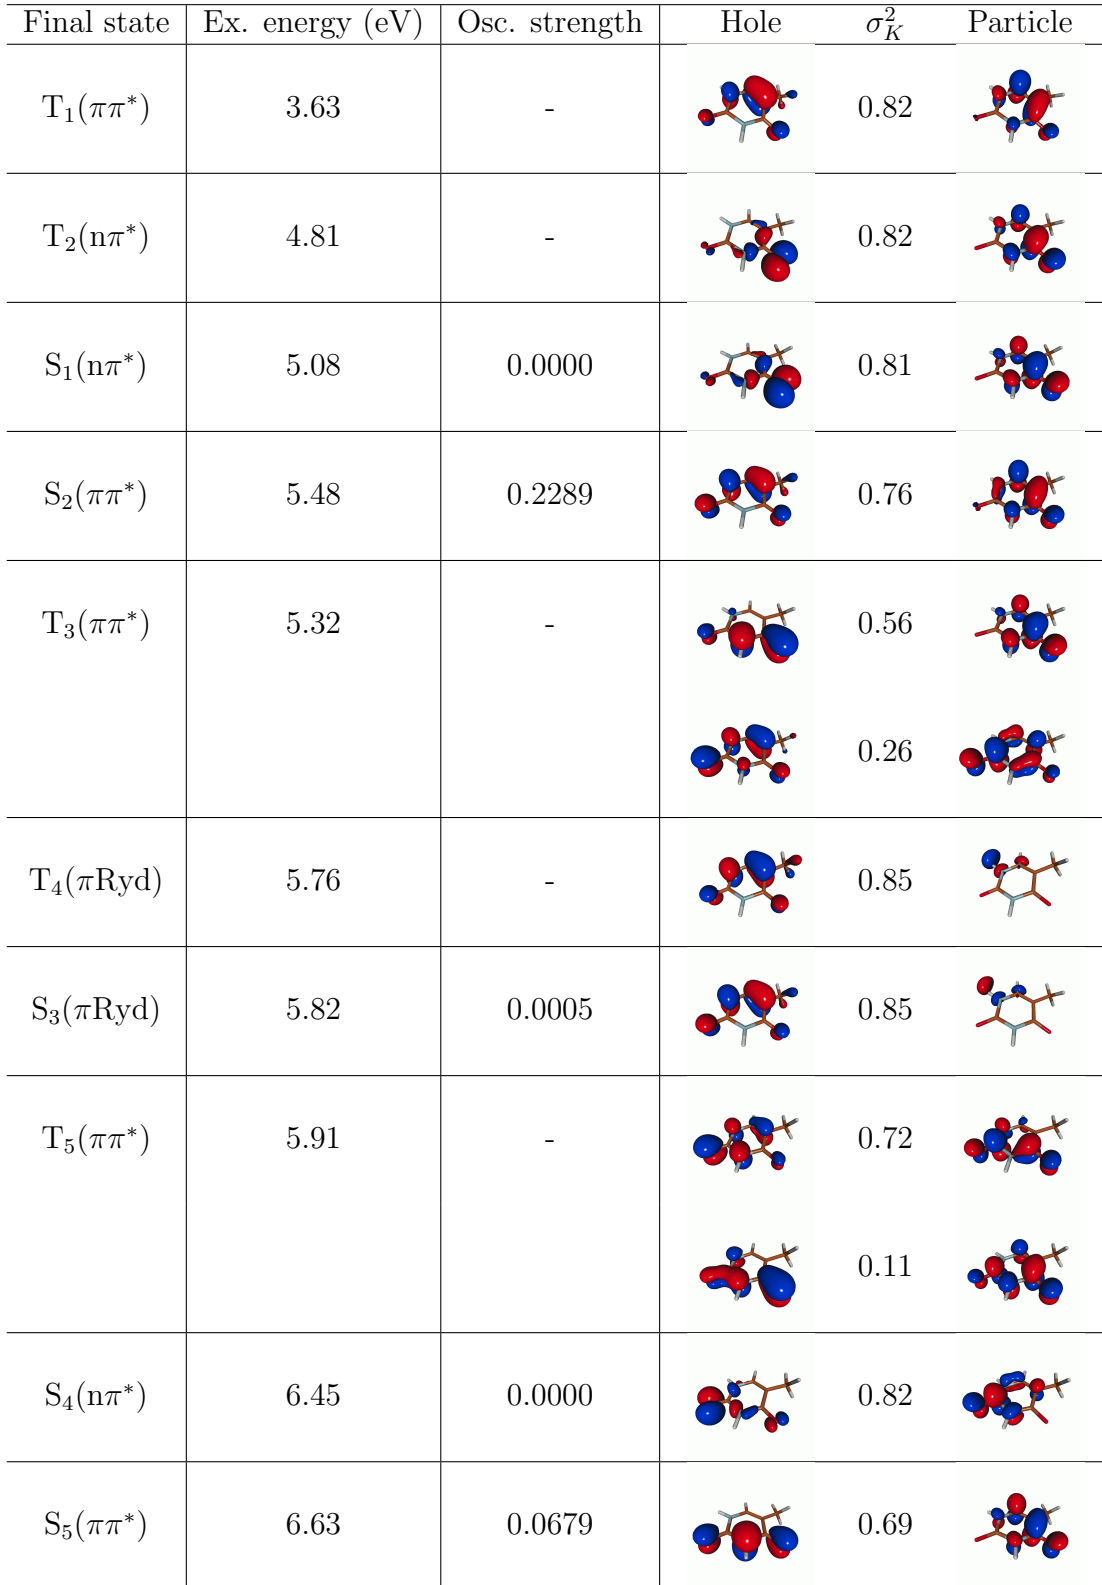 |
| $S_5(\pi\pi^*)$ | 6.63            | 0.0679        | 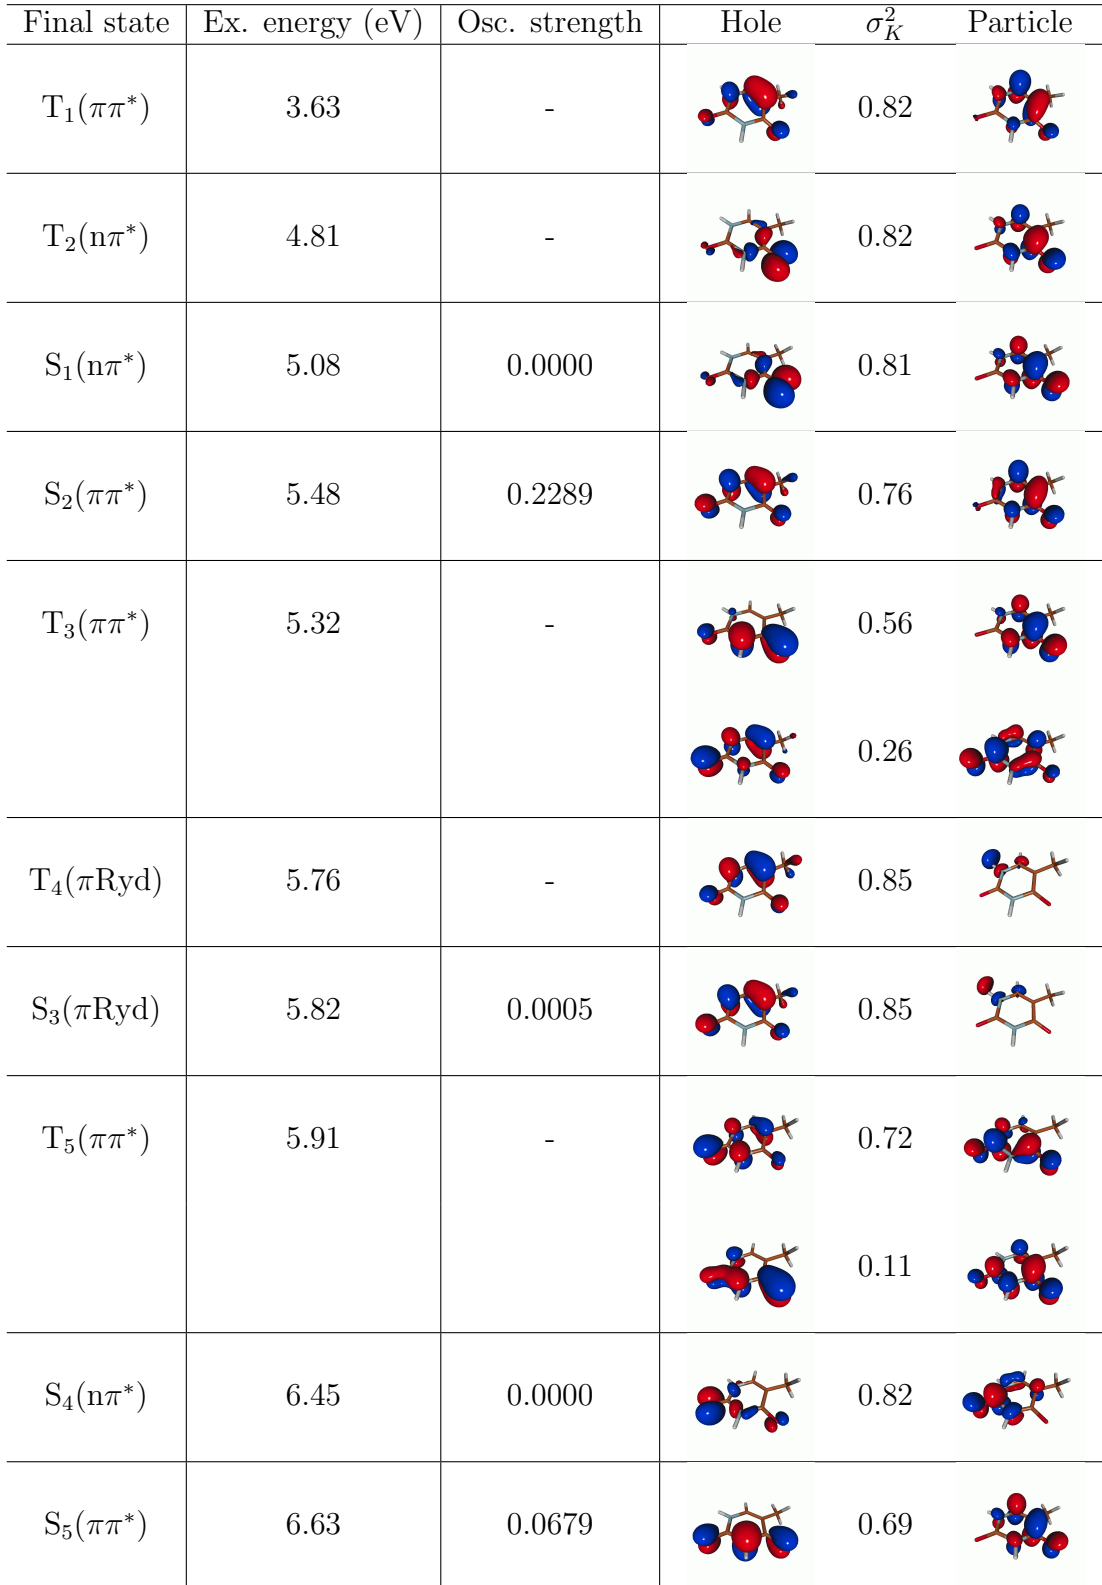 | 0.69         | 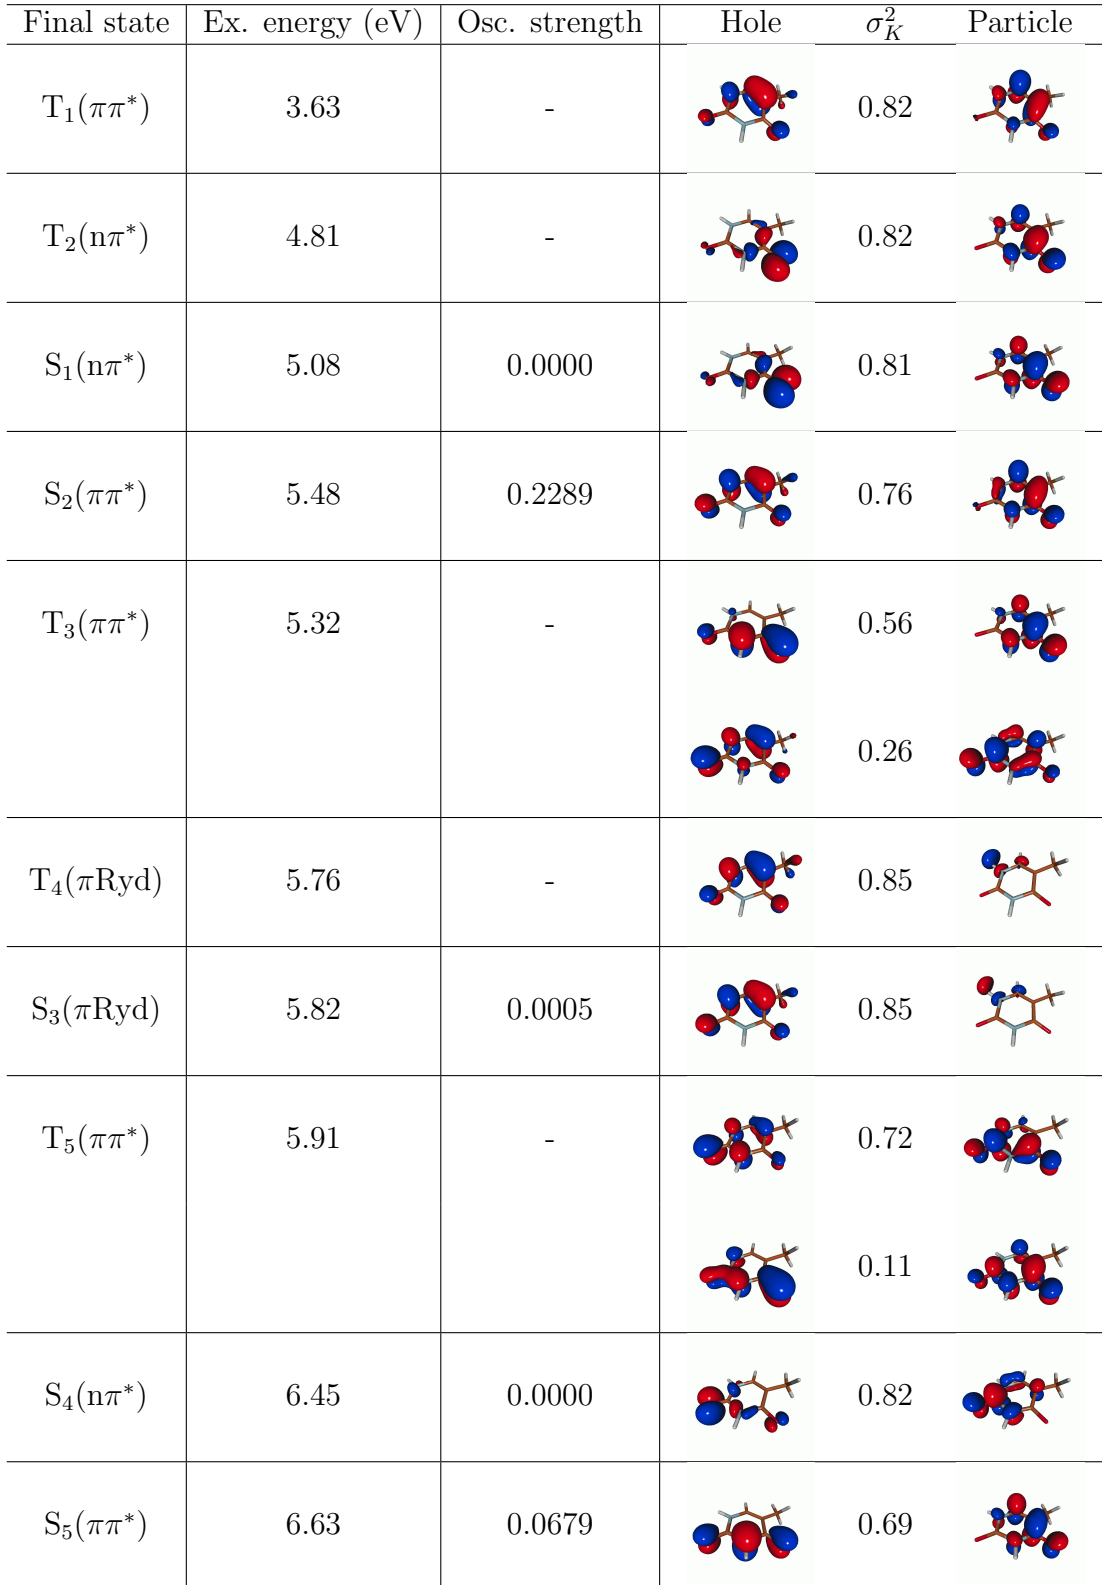 |

Table S14: Thymine. ADC(2)/6-311++G\*\* NTOs of the excitations from the ground state to the lowest-lying valence-excited states at the FC geometry (NTO isosurface is 0.05).

| Final state     | Ex. energy (eV) | Osc. strength | Hole                                                                                 | $\sigma_K^2$ | Particle                                                                              |
|-----------------|-----------------|---------------|--------------------------------------------------------------------------------------|--------------|---------------------------------------------------------------------------------------|
| $T_1(\pi\pi^*)$ | 3.70            | -             | 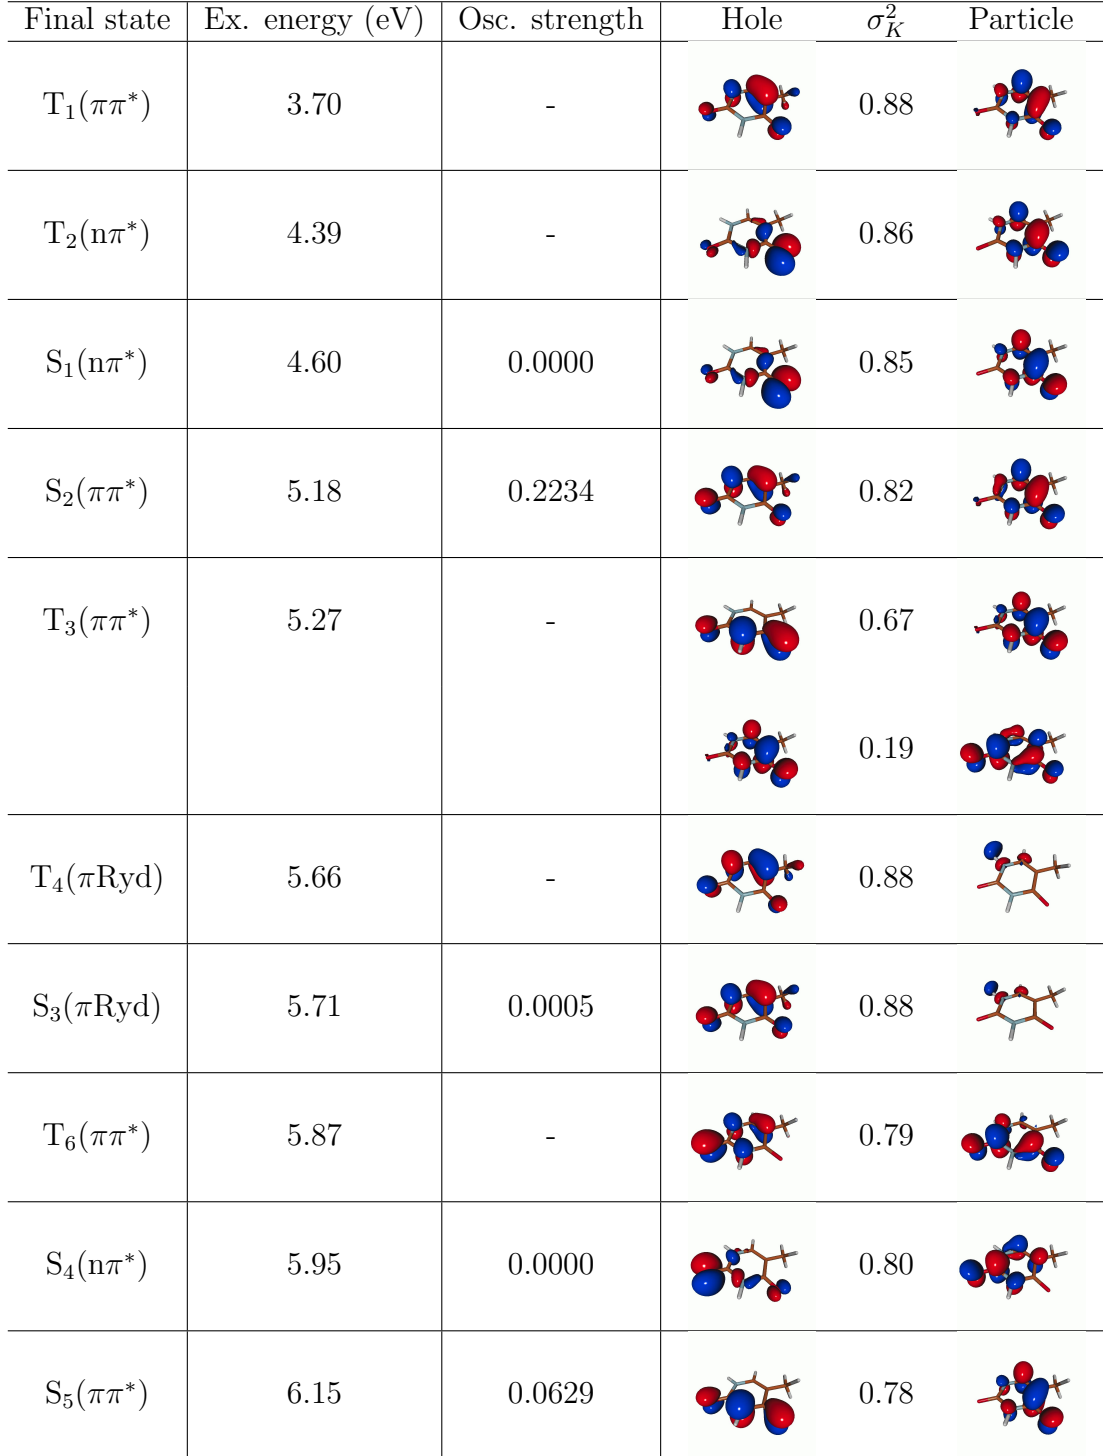   | 0.88         | 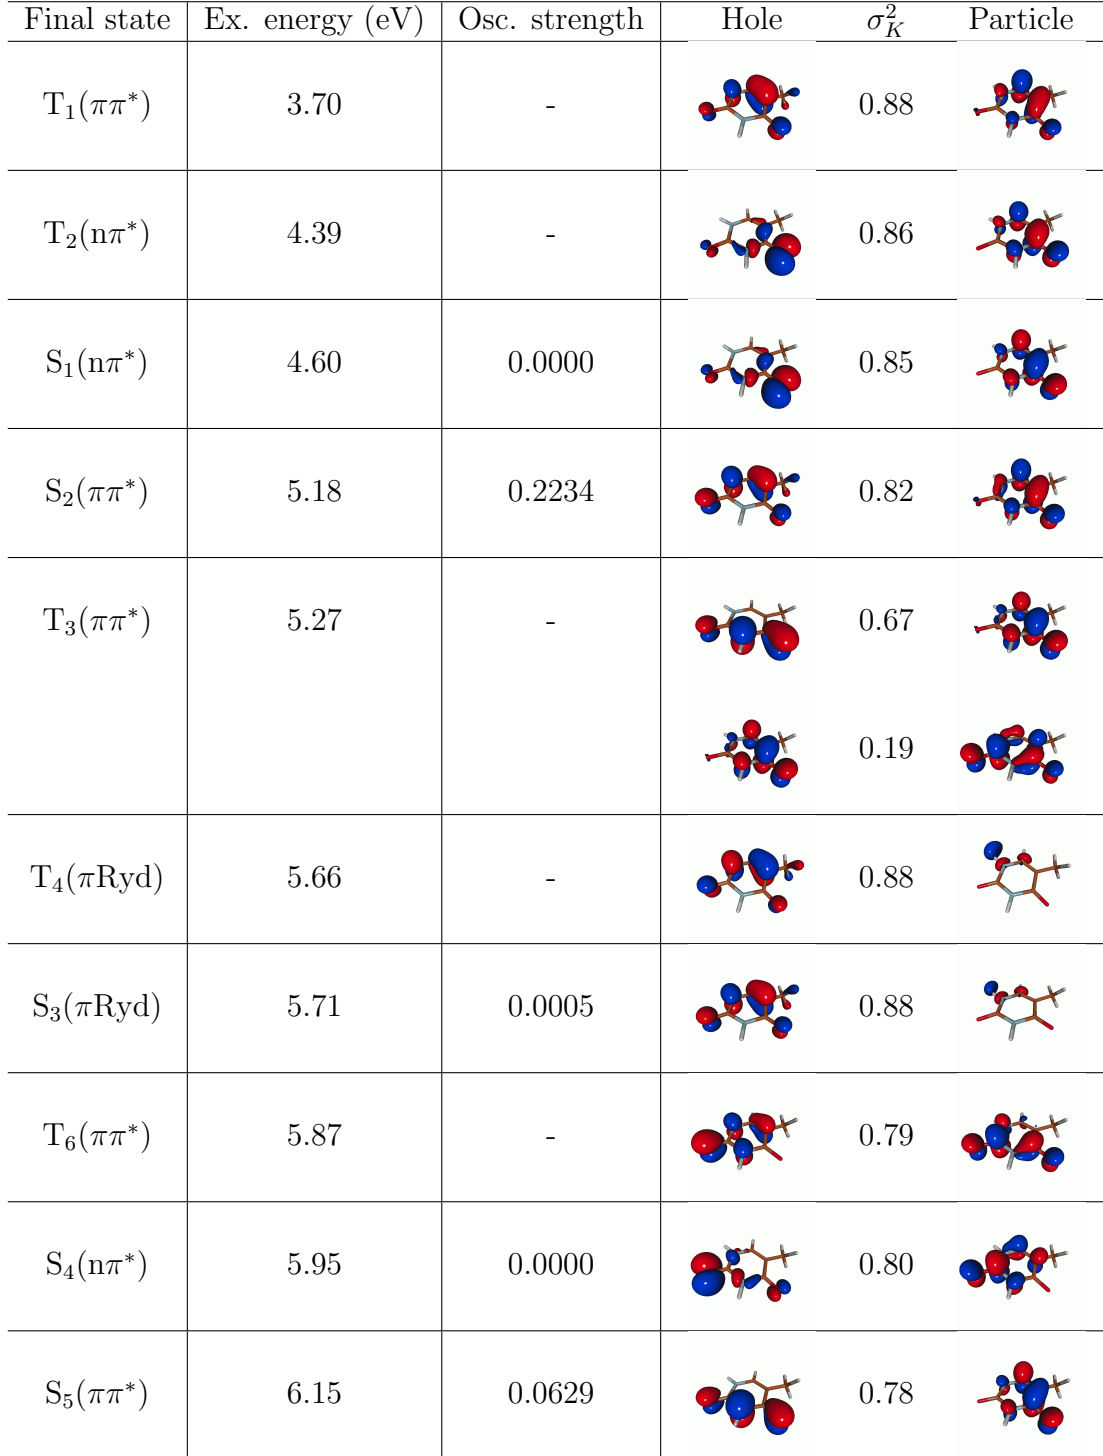   |
| $T_2(n\pi^*)$   | 4.39            | -             | 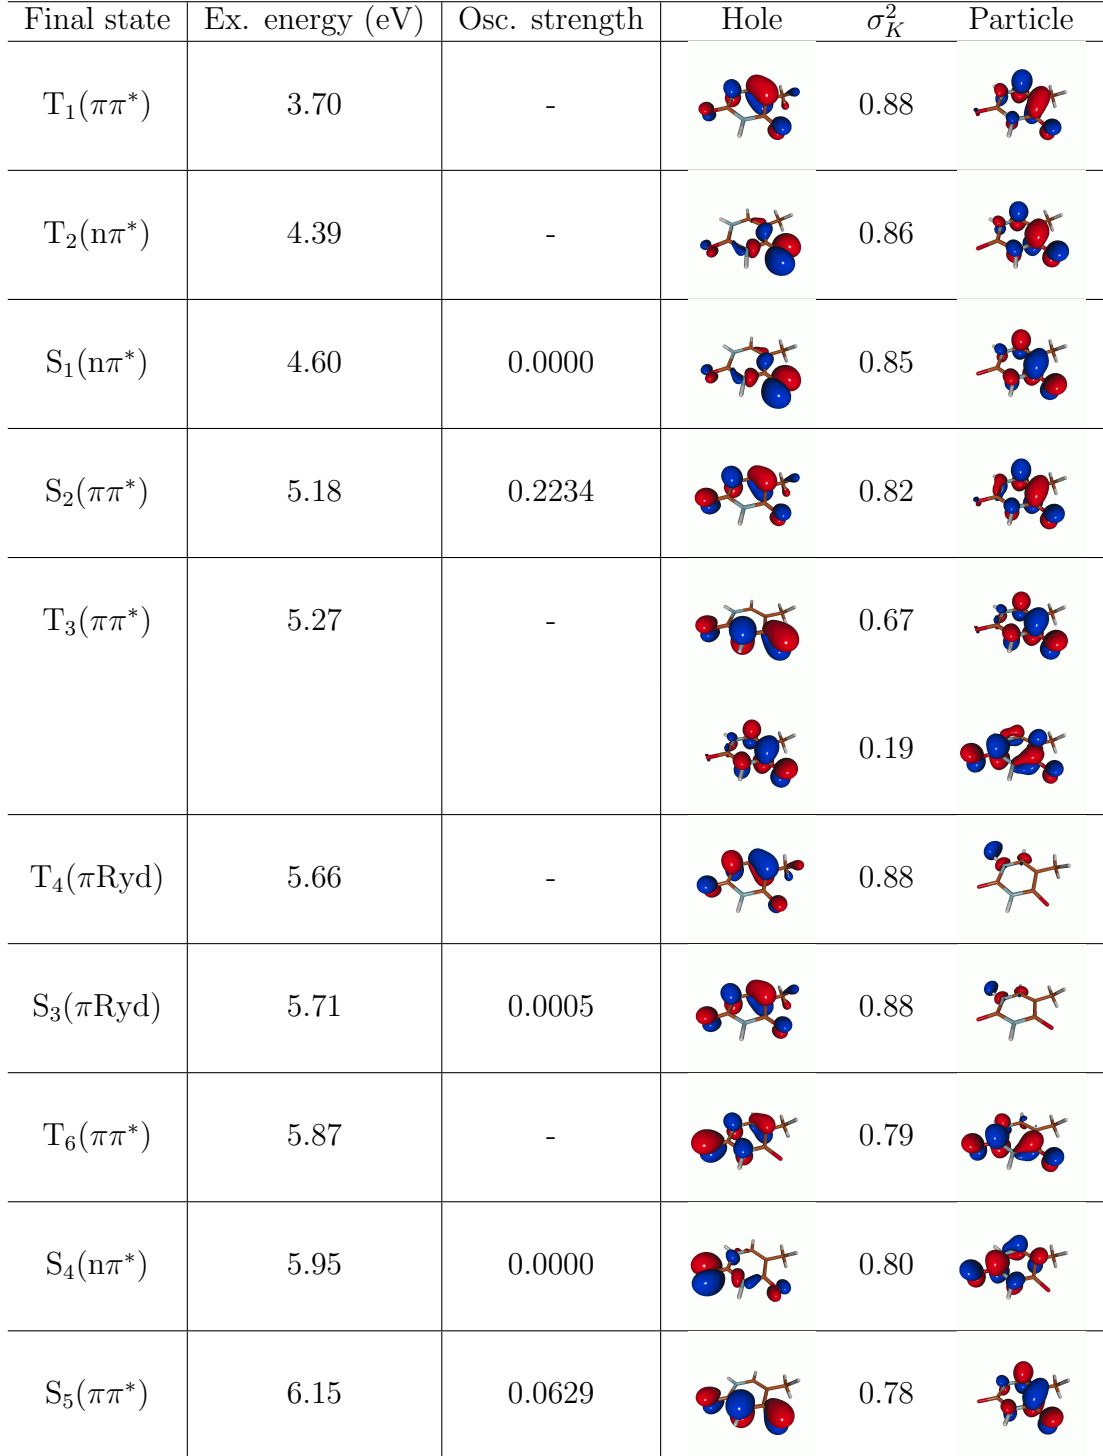   | 0.86         | 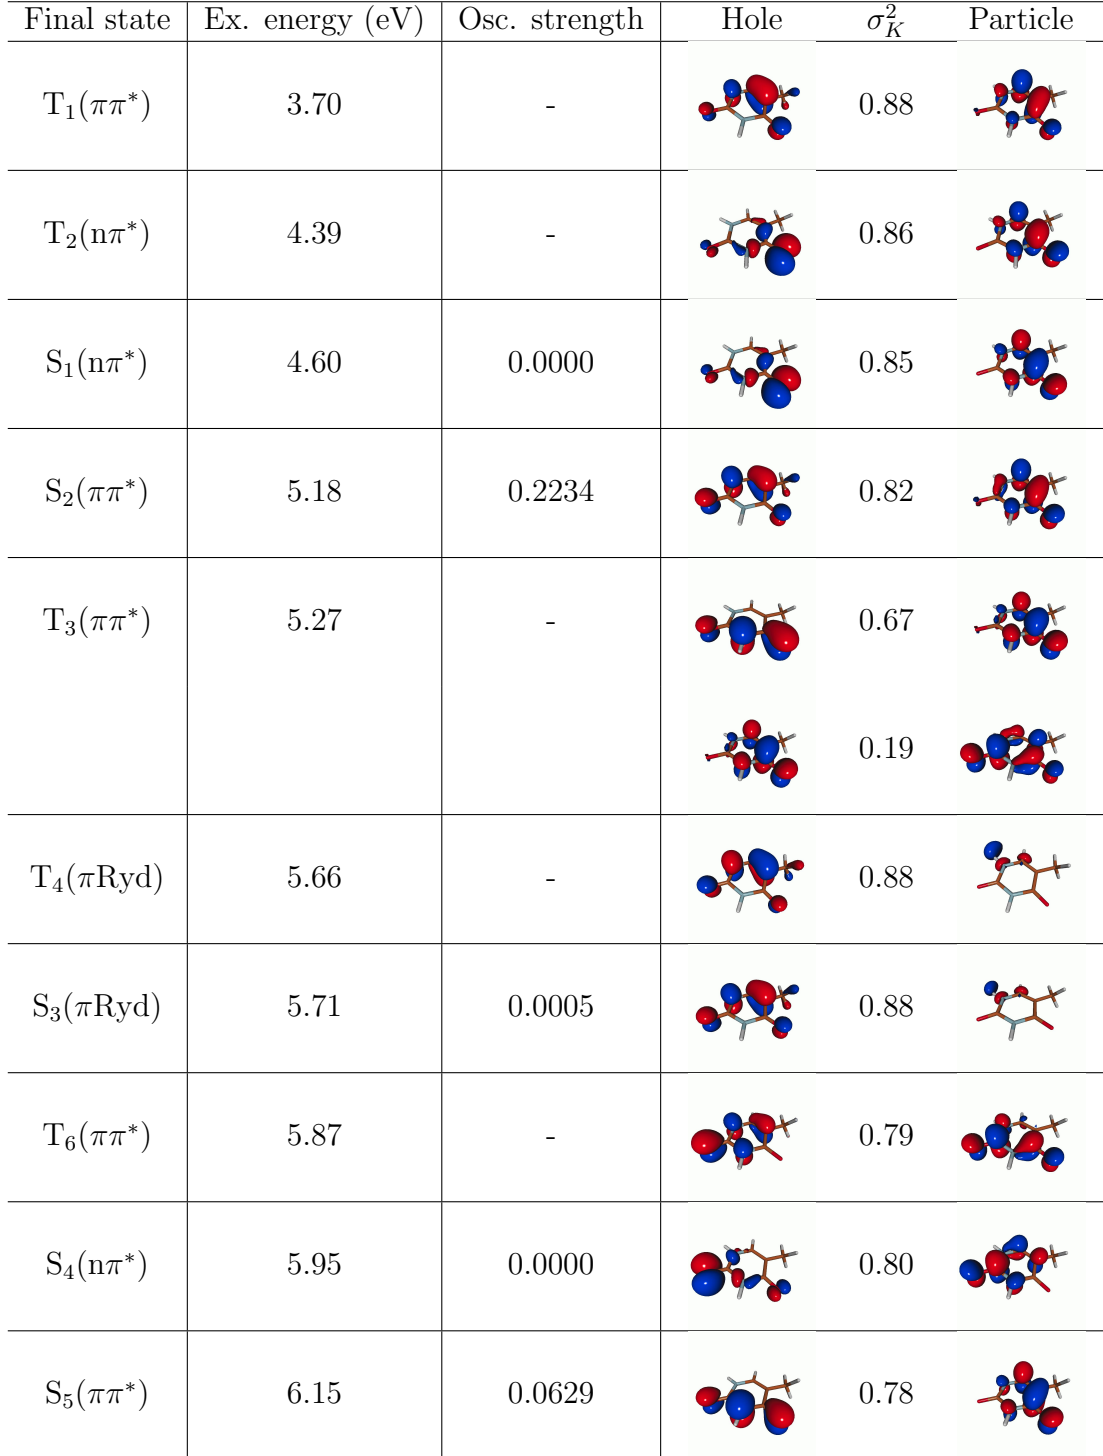   |
| $S_1(n\pi^*)$   | 4.60            | 0.0000        | 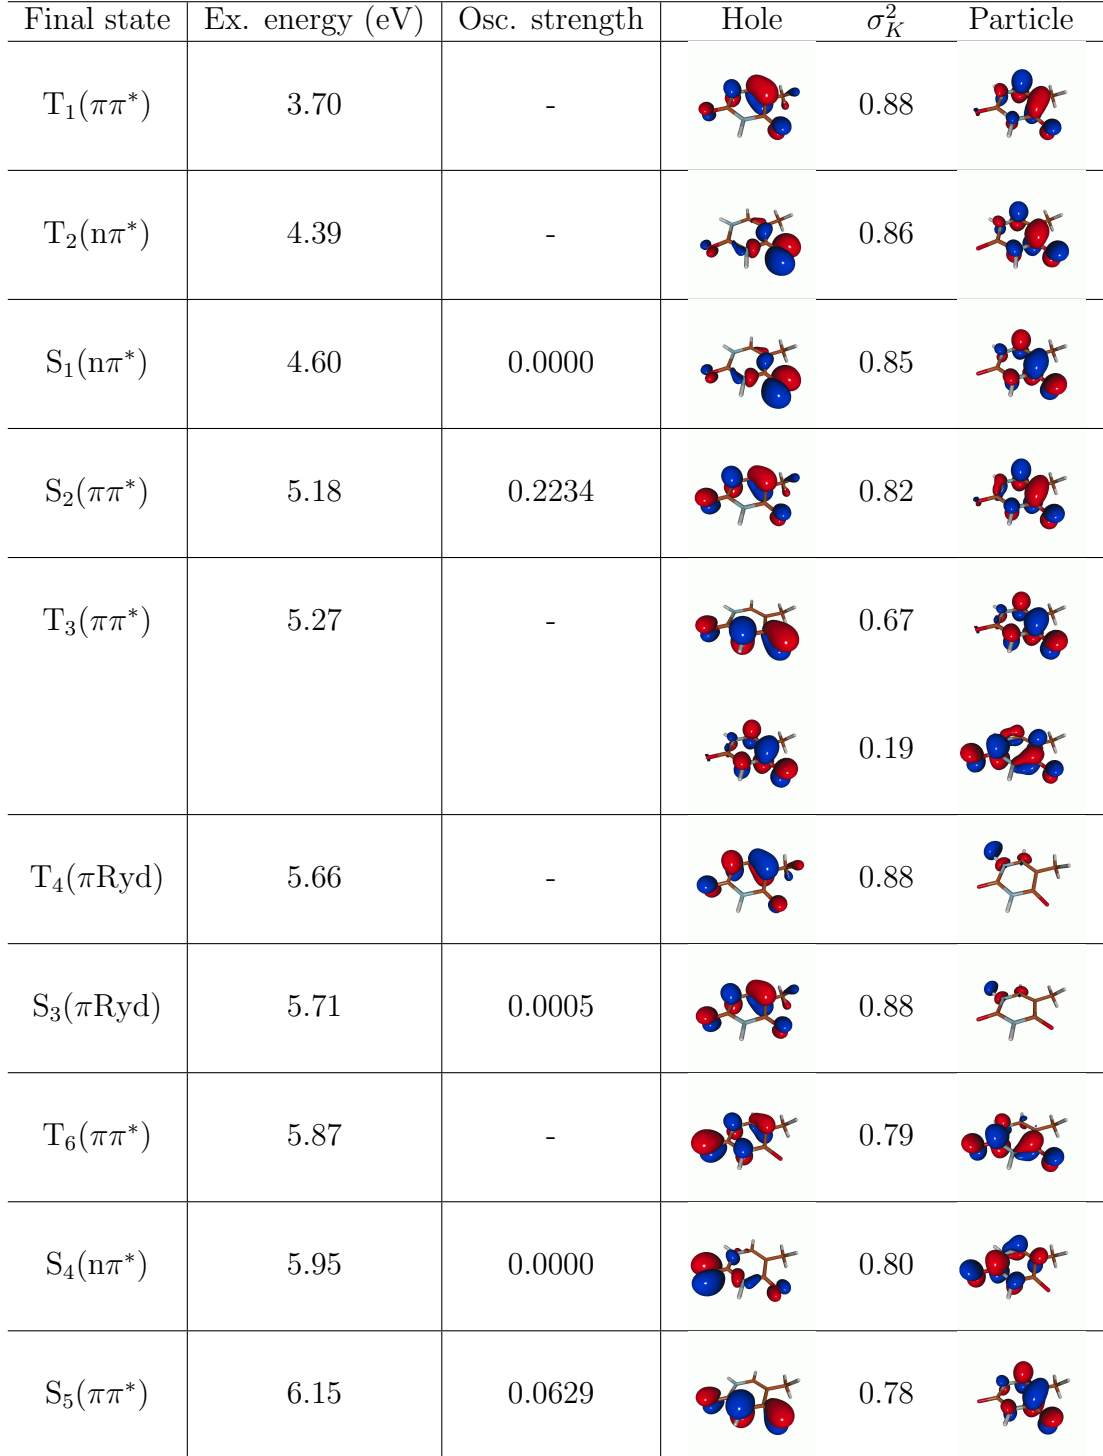   | 0.85         | 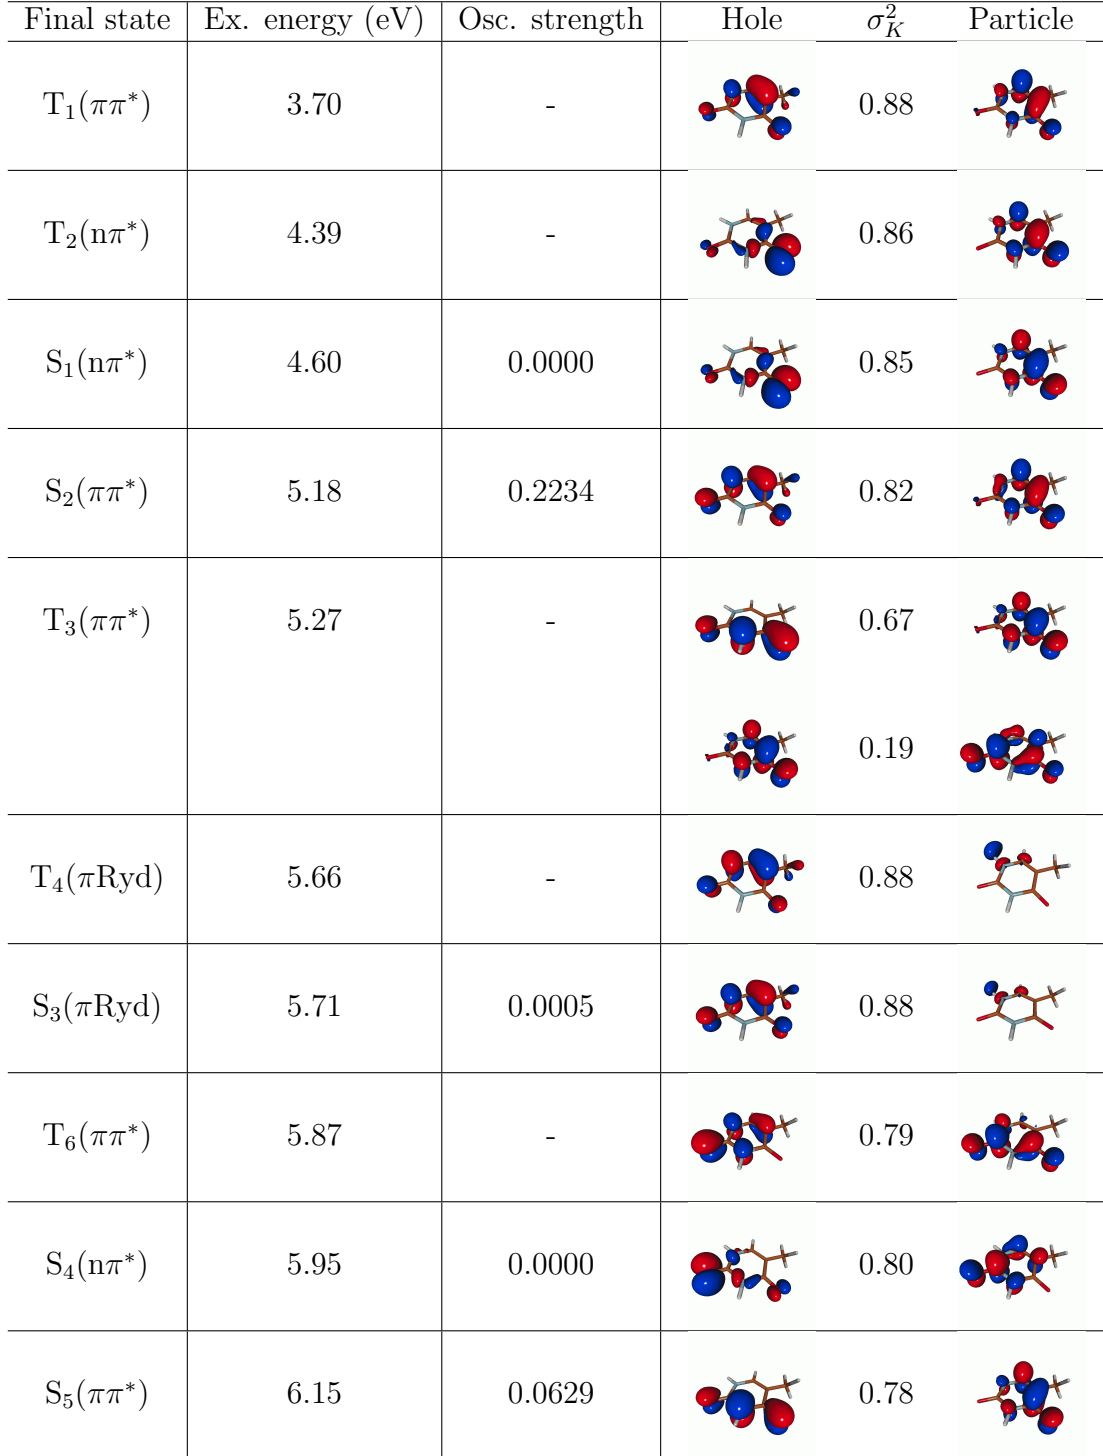   |
| $S_2(\pi\pi^*)$ | 5.18            | 0.2234        | 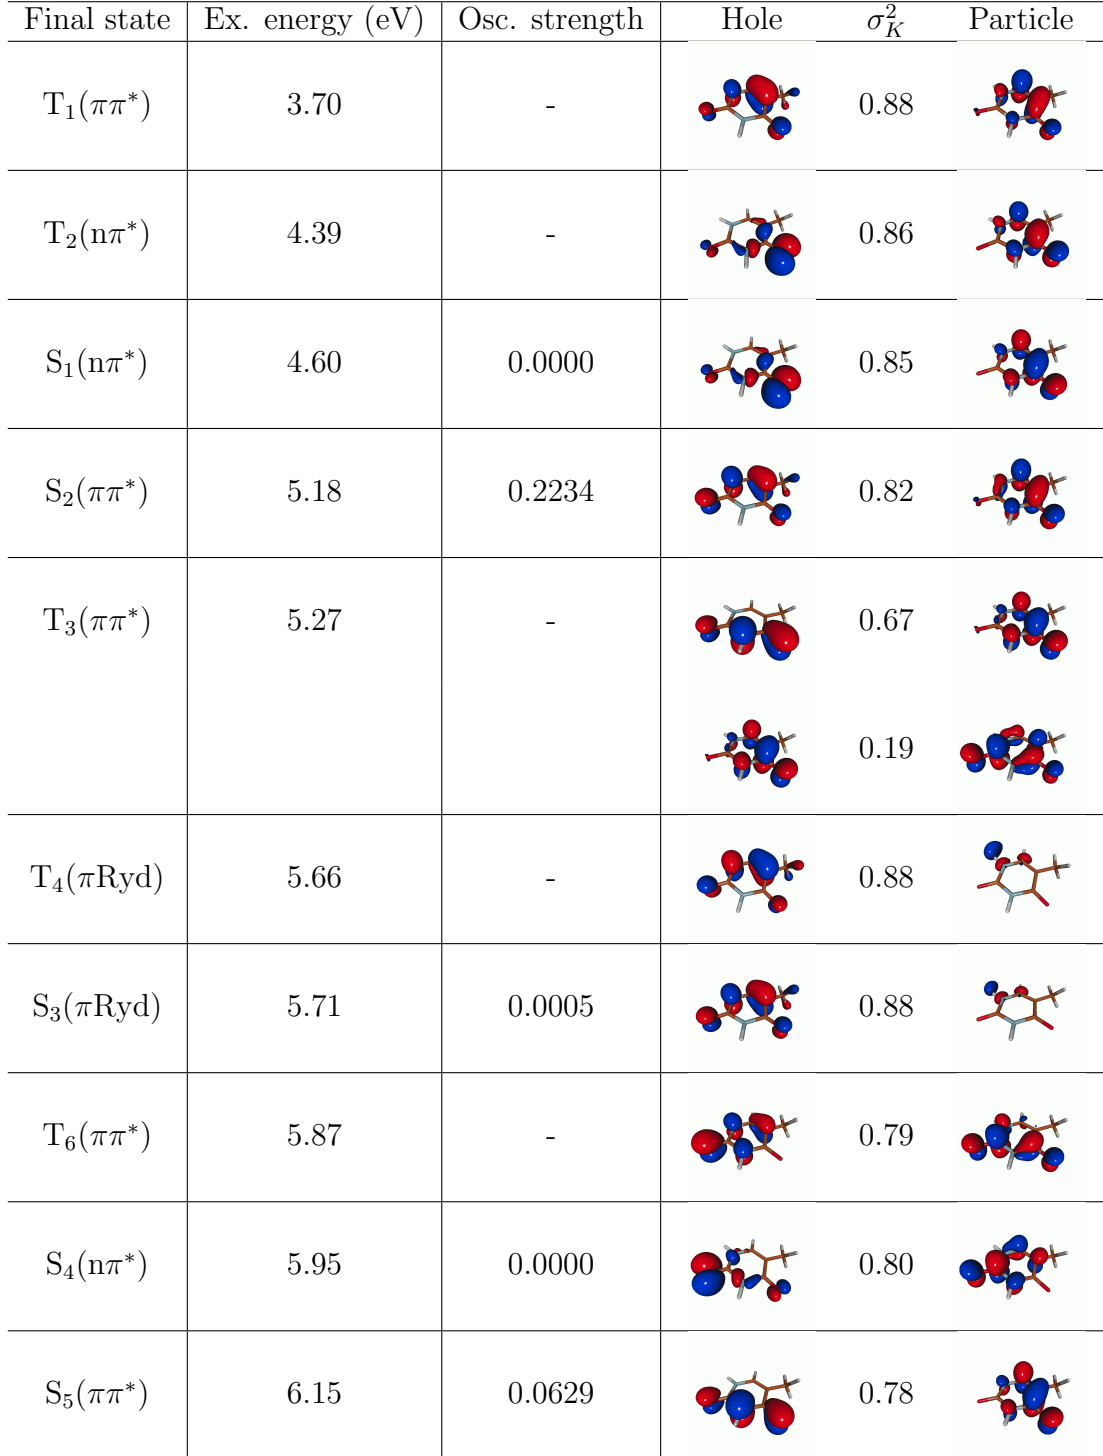   | 0.82         | 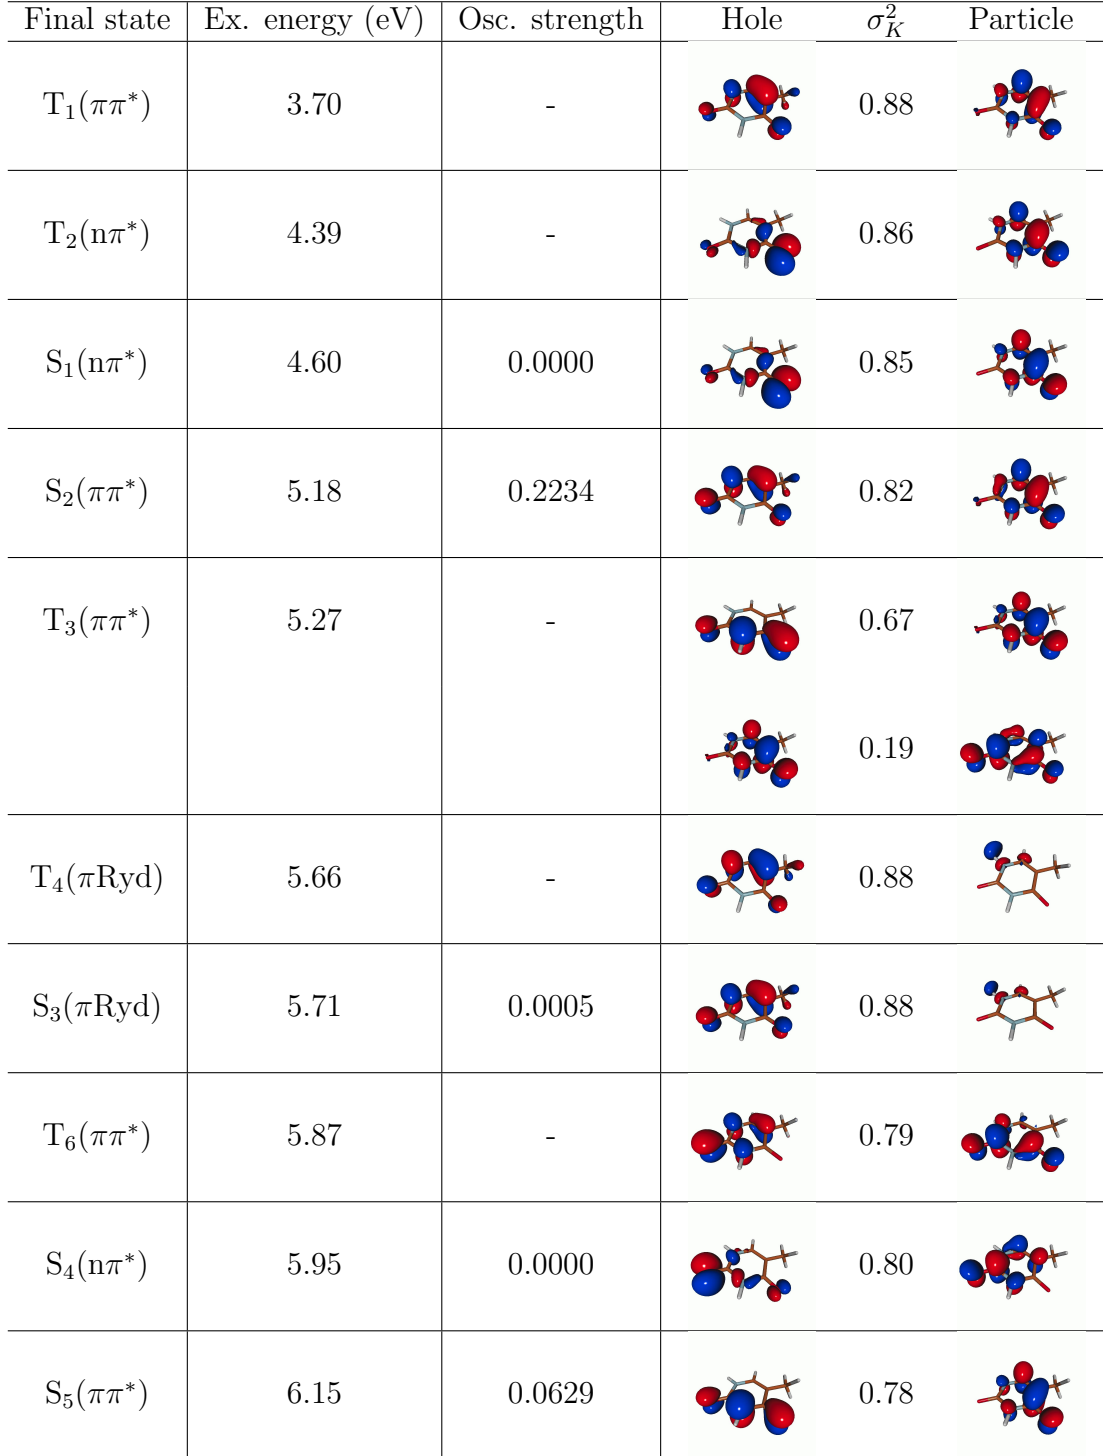   |
| $T_3(\pi\pi^*)$ | 5.27            | -             | 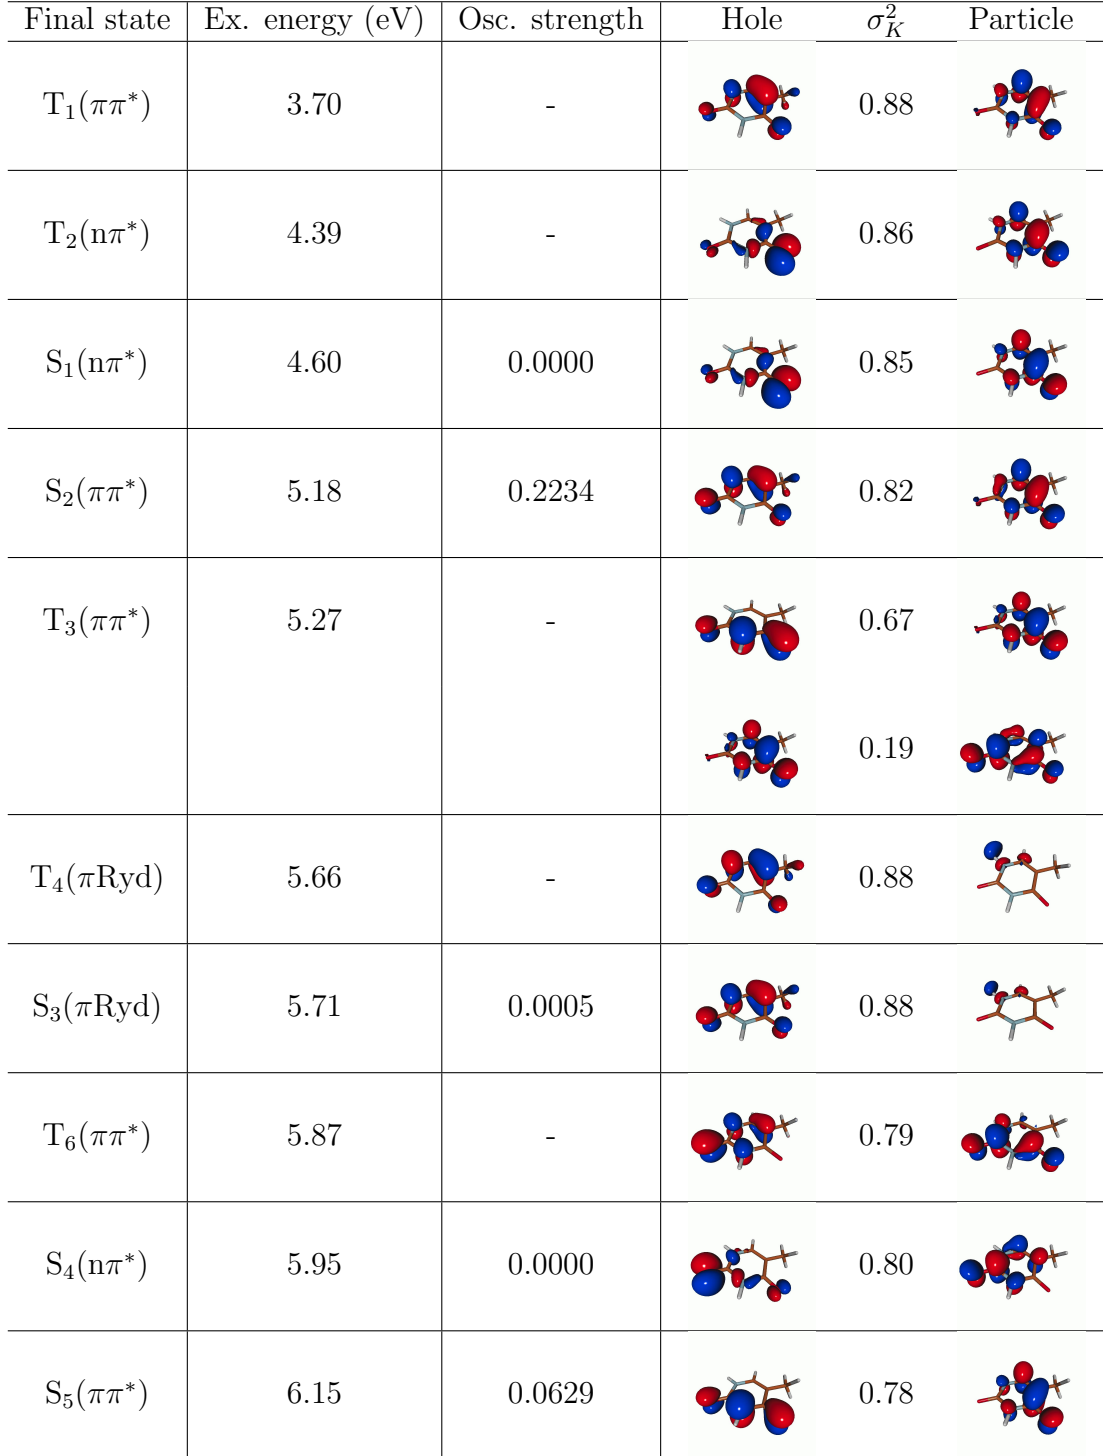  | 0.67         | 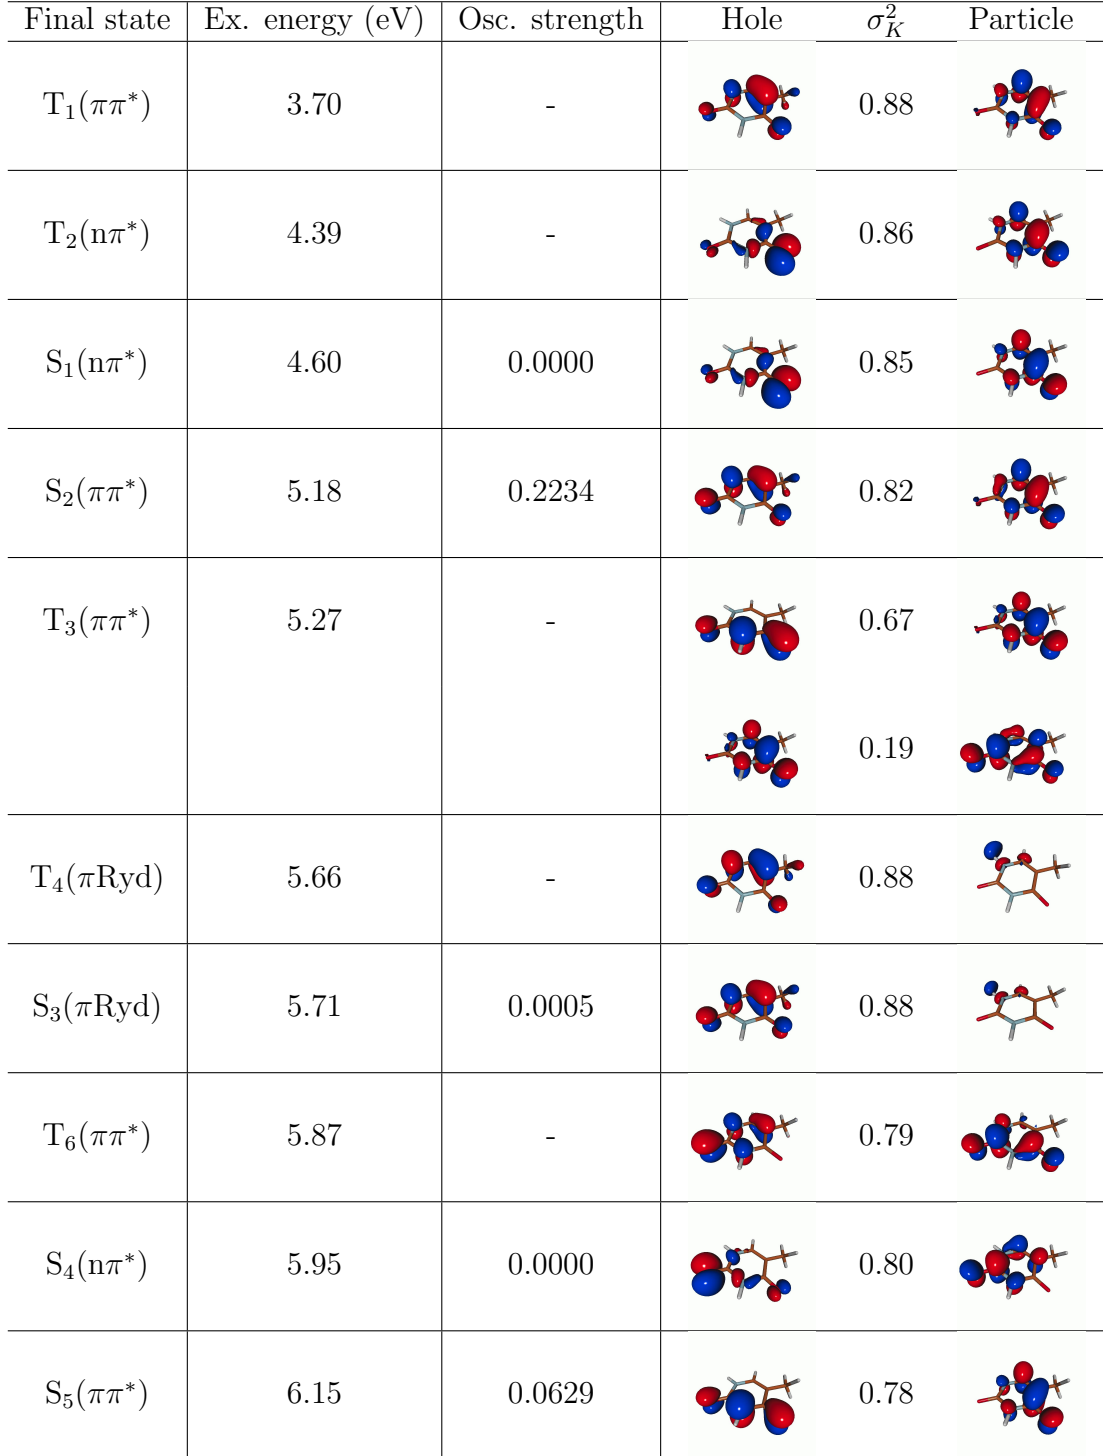  |
|                 |                 |               | 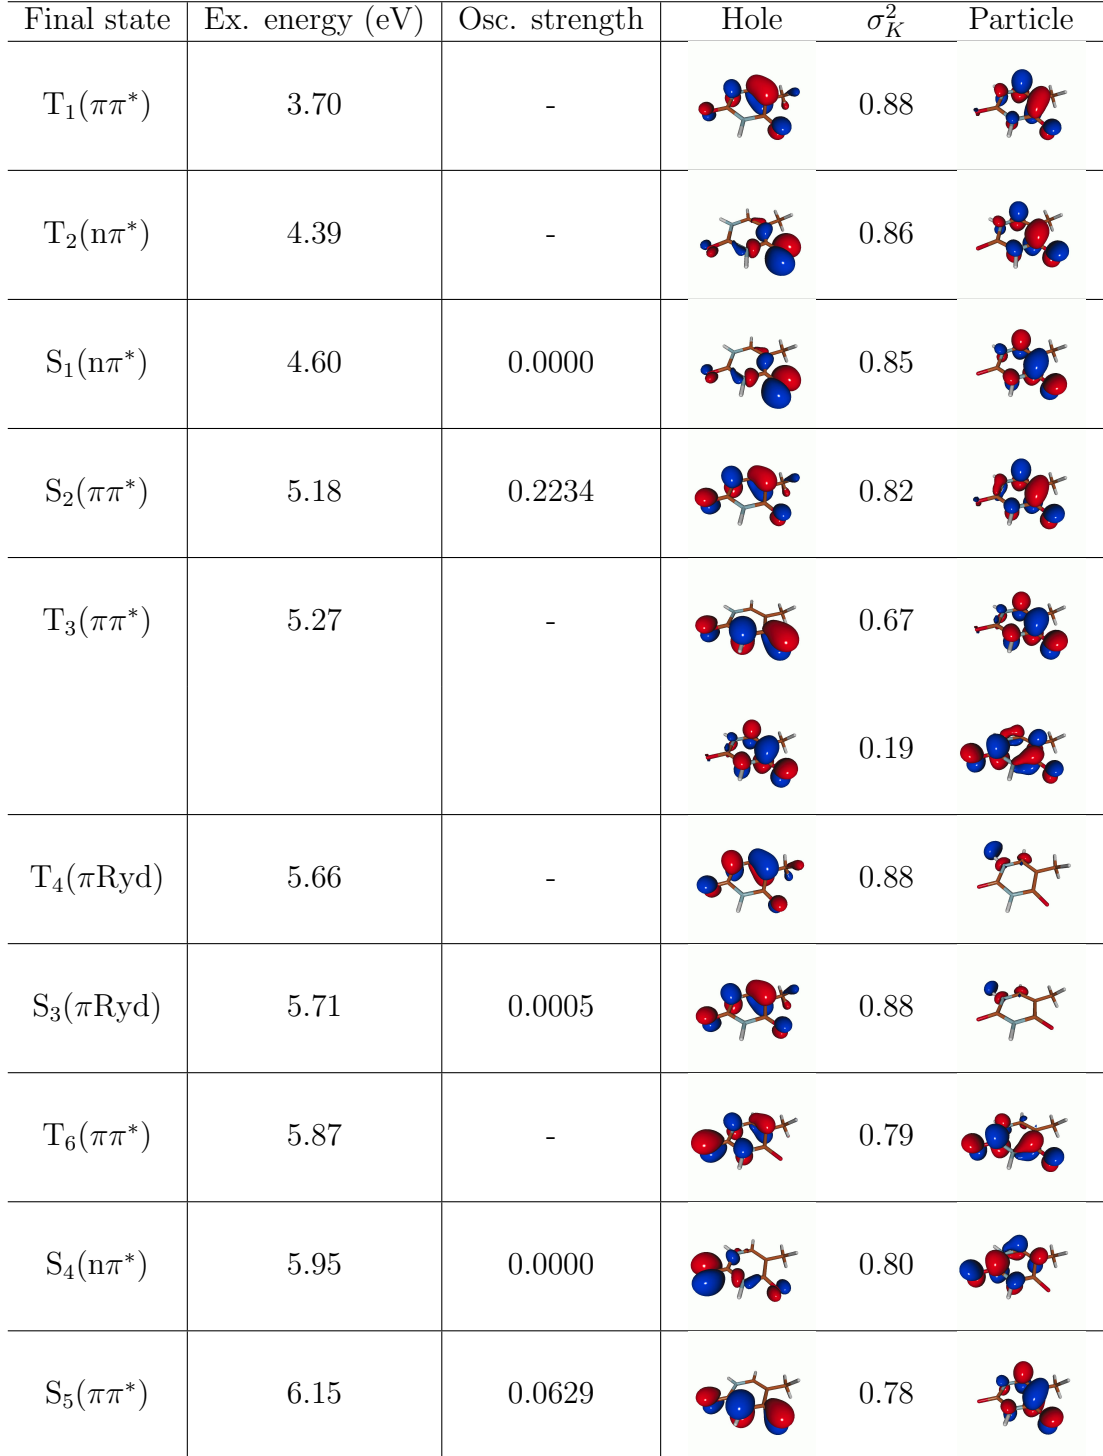 | 0.19         | 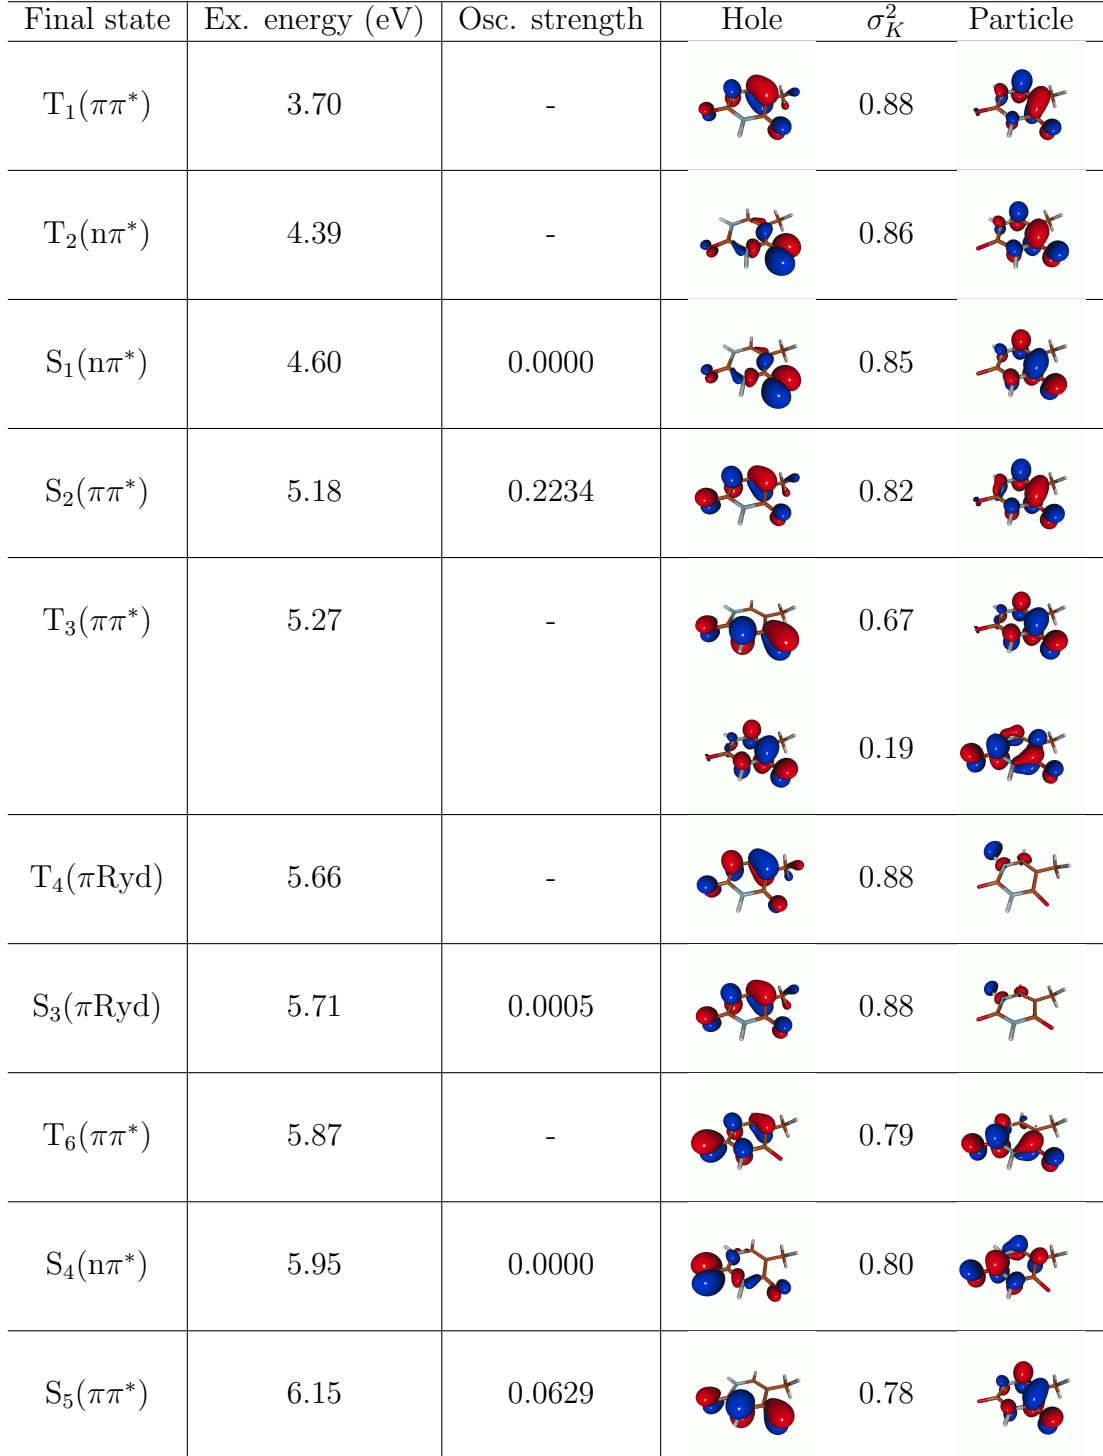 |
| $T_4(\pi Ryd)$  | 5.66            | -             | 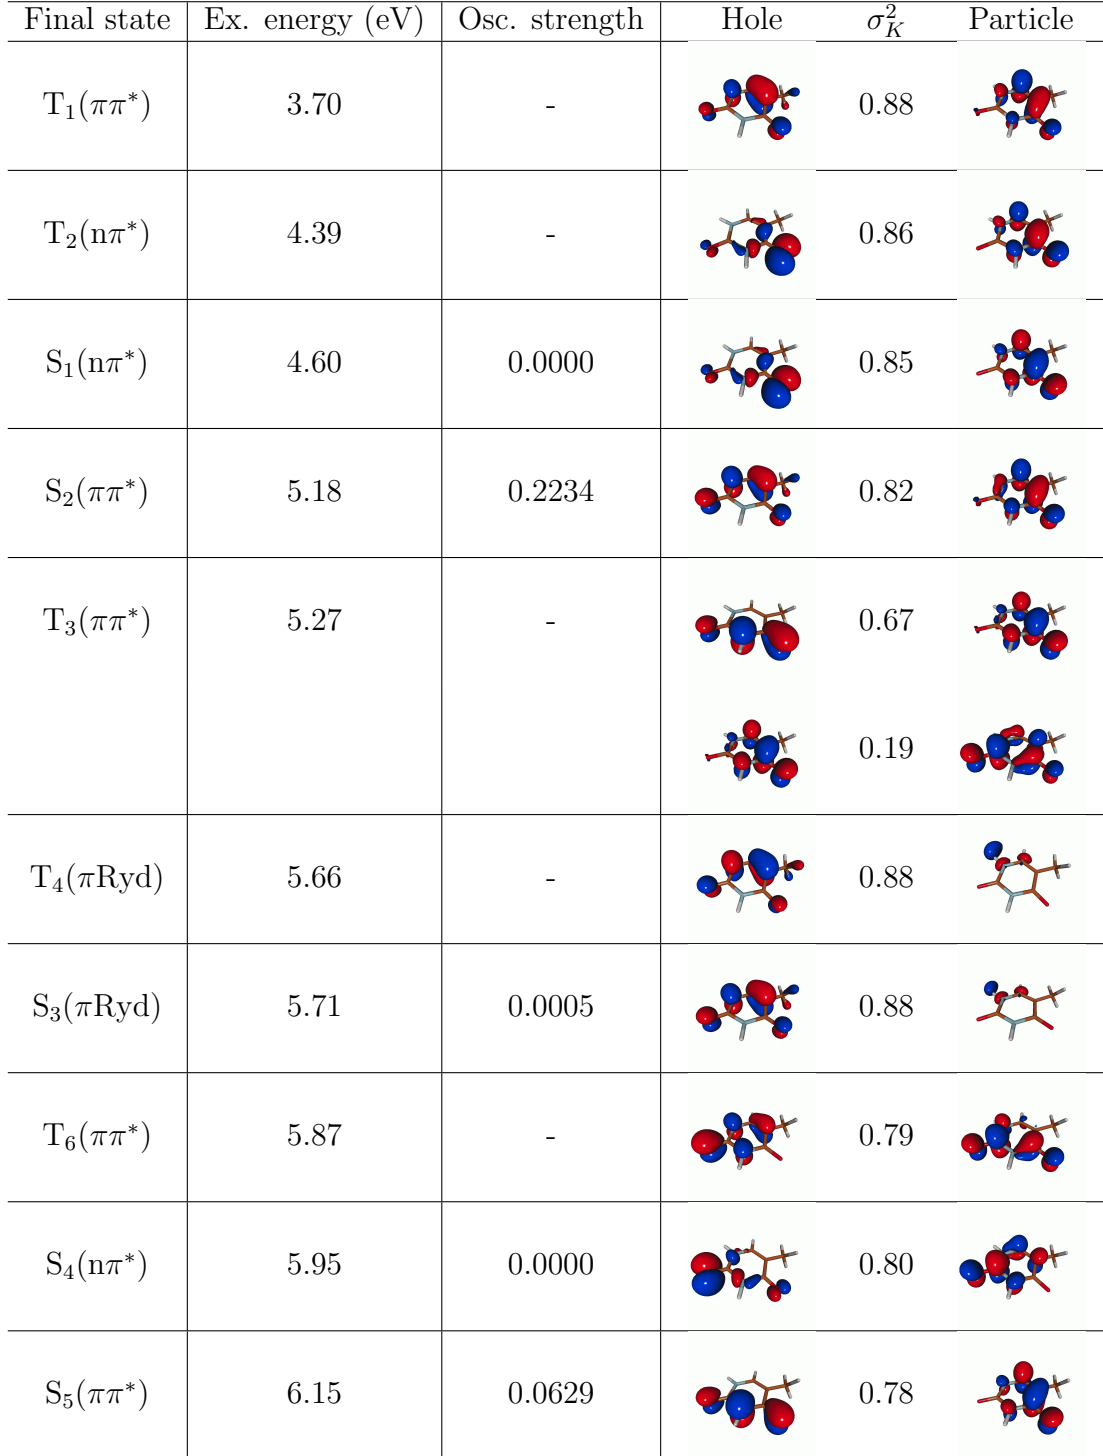 | 0.88         | 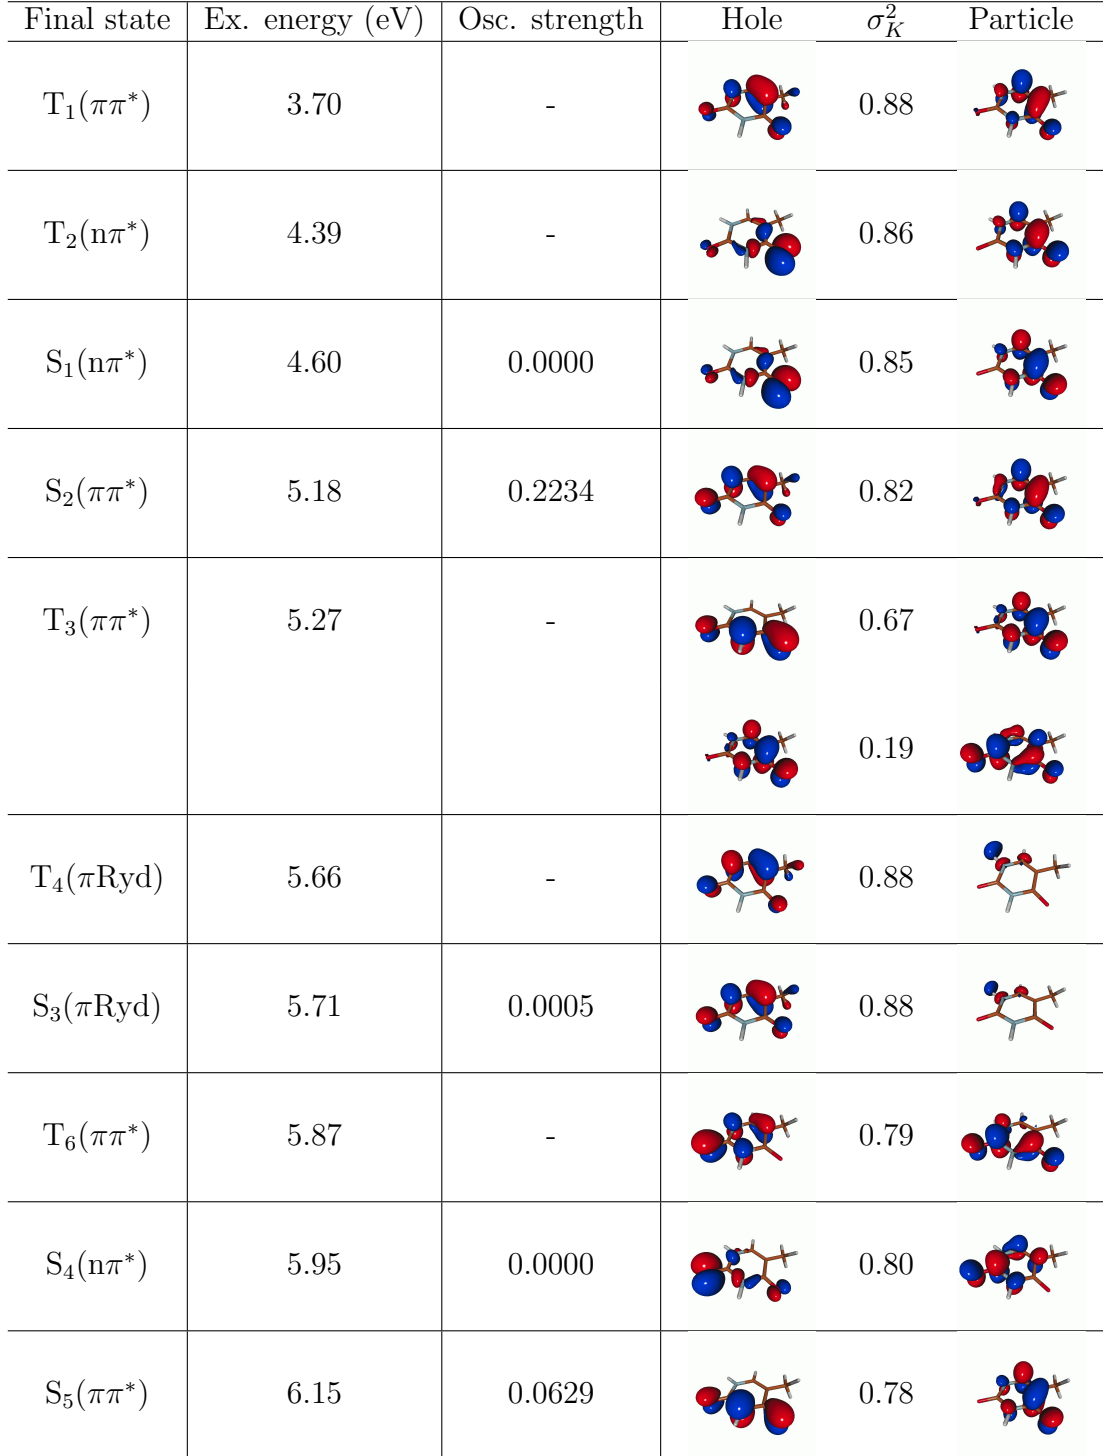 |
| $S_3(\pi Ryd)$  | 5.71            | 0.0005        | 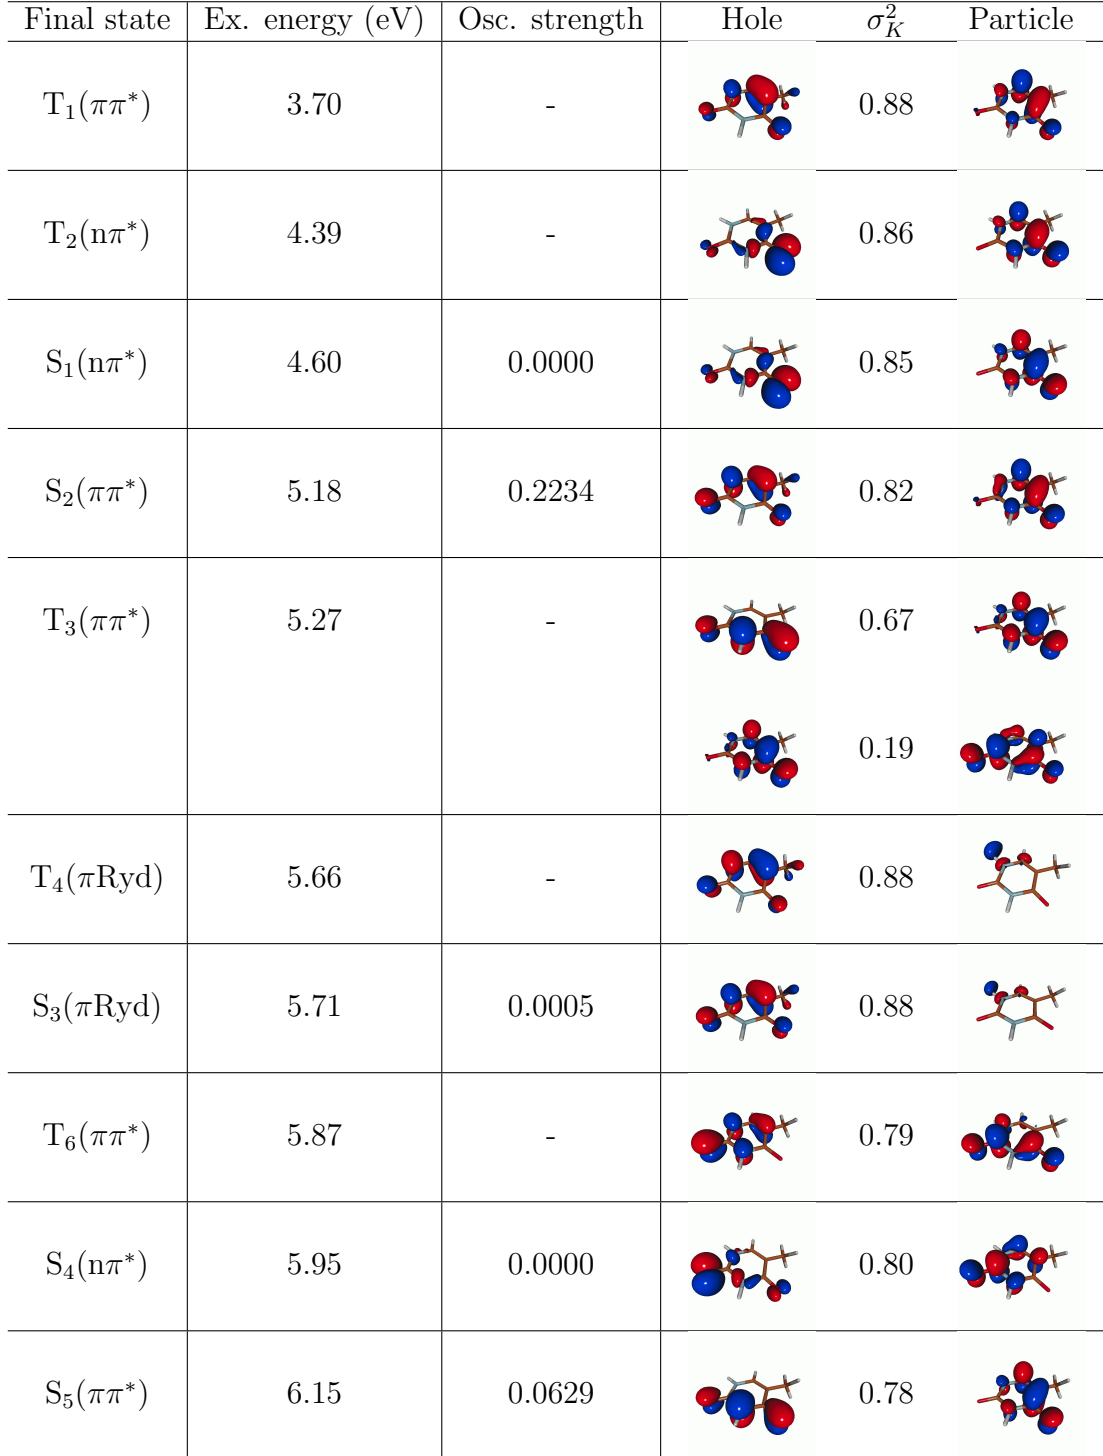 | 0.88         | 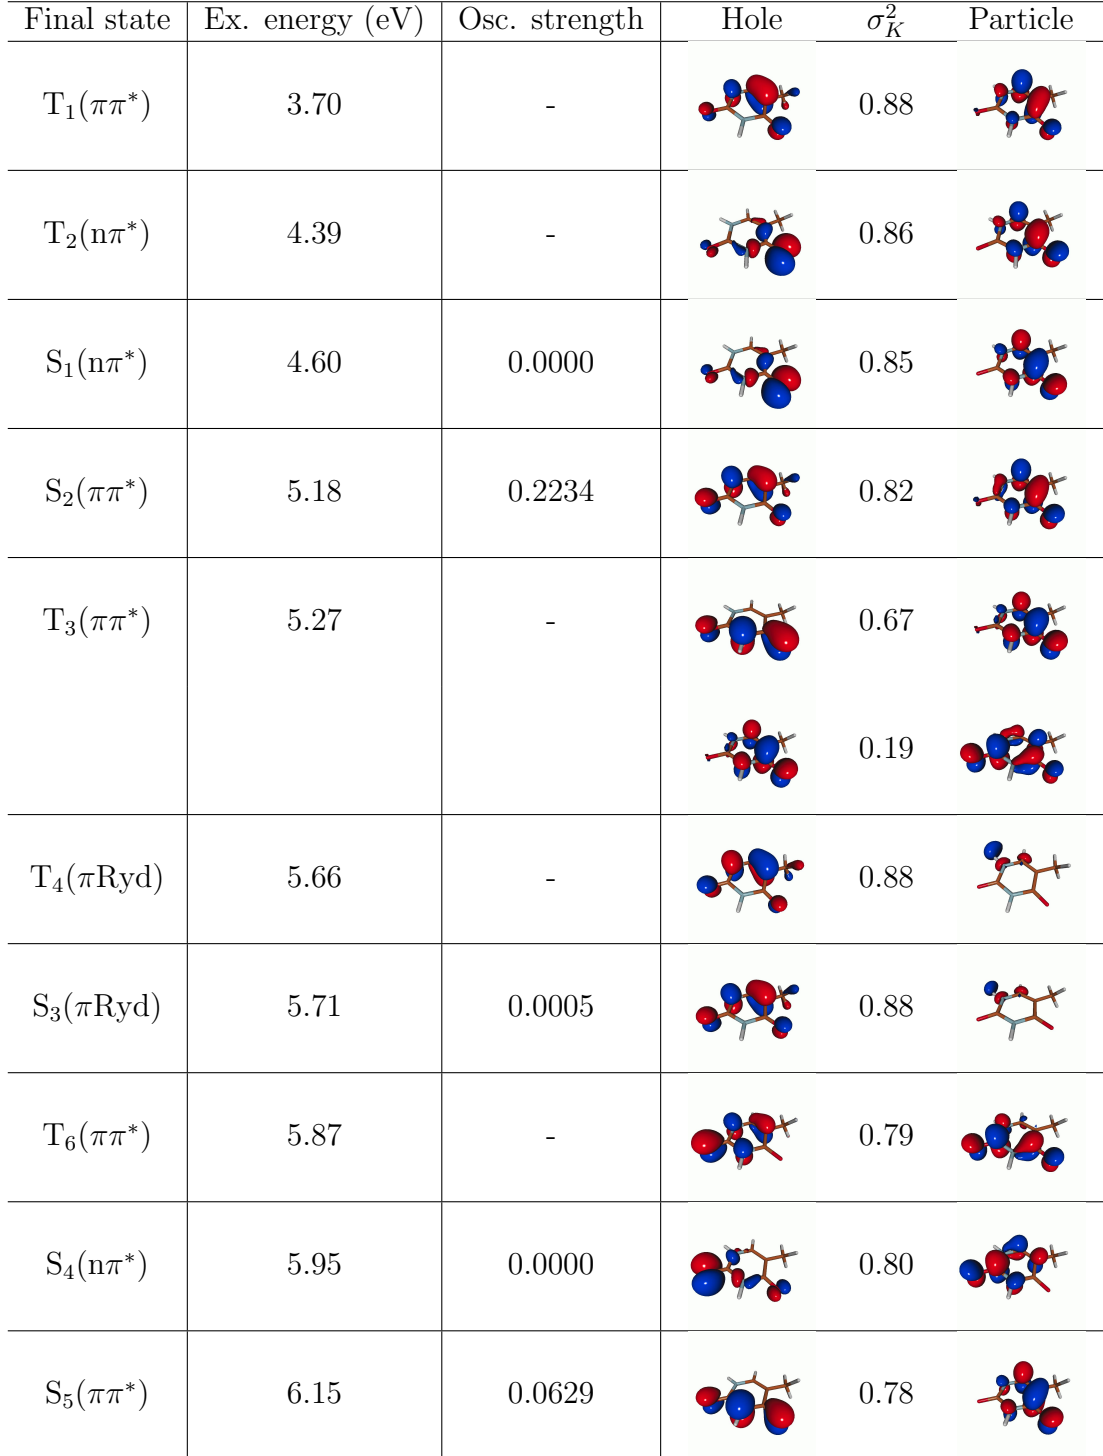 |
| $T_6(\pi\pi^*)$ | 5.87            | -             | 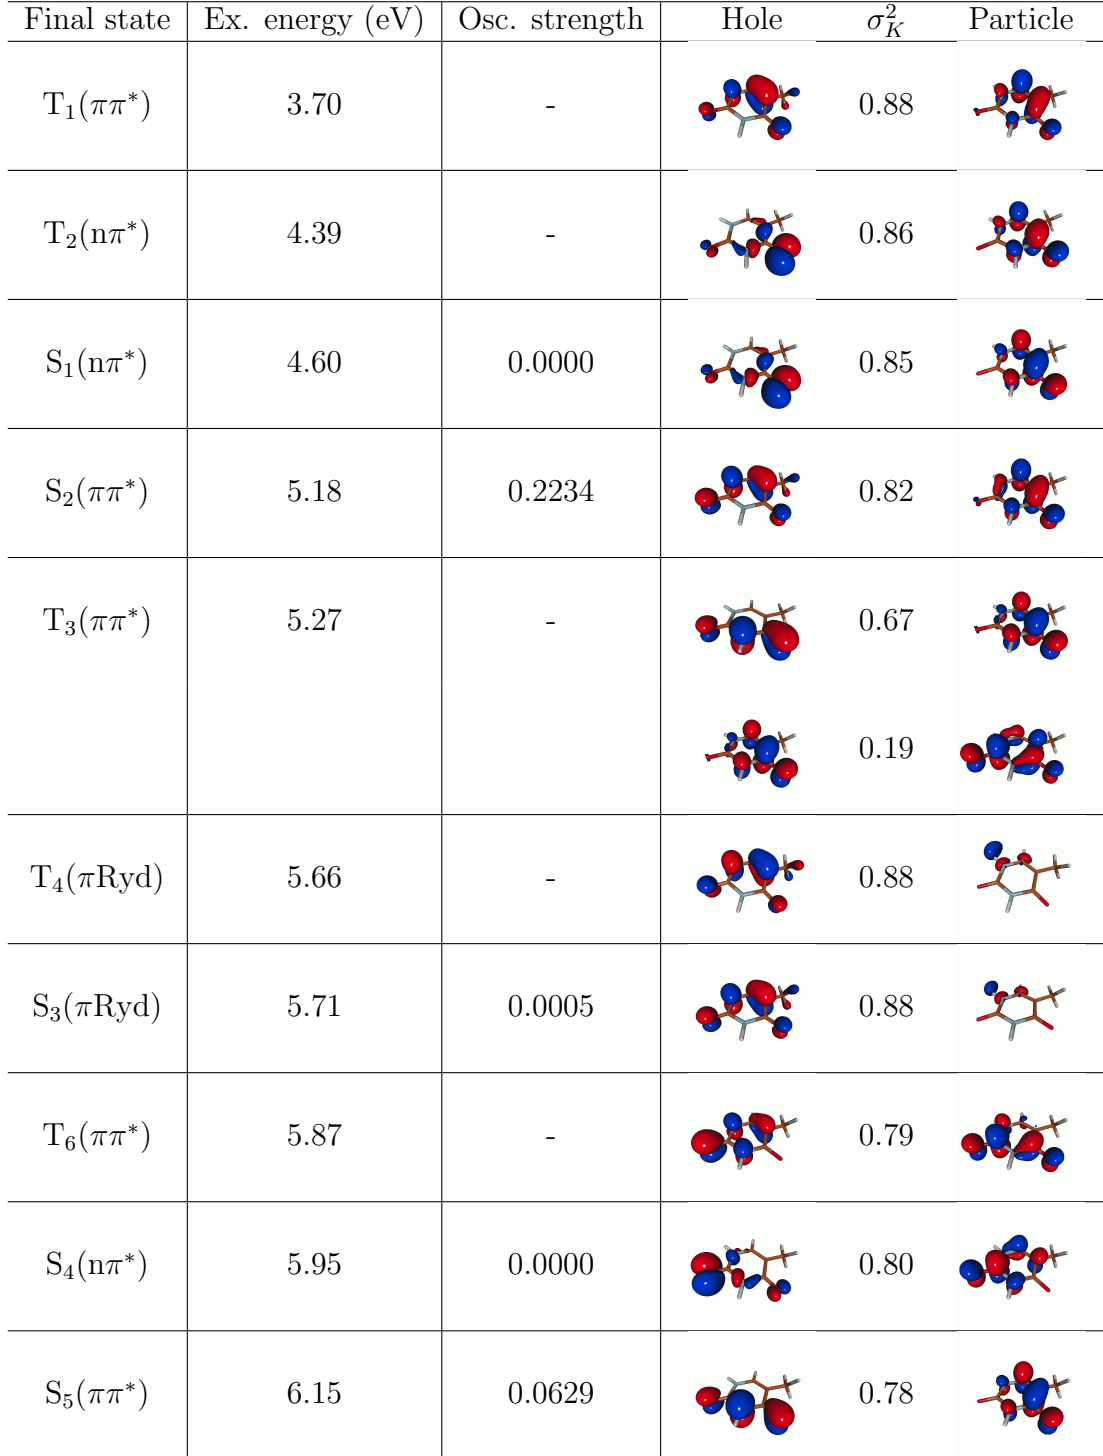 | 0.79         | 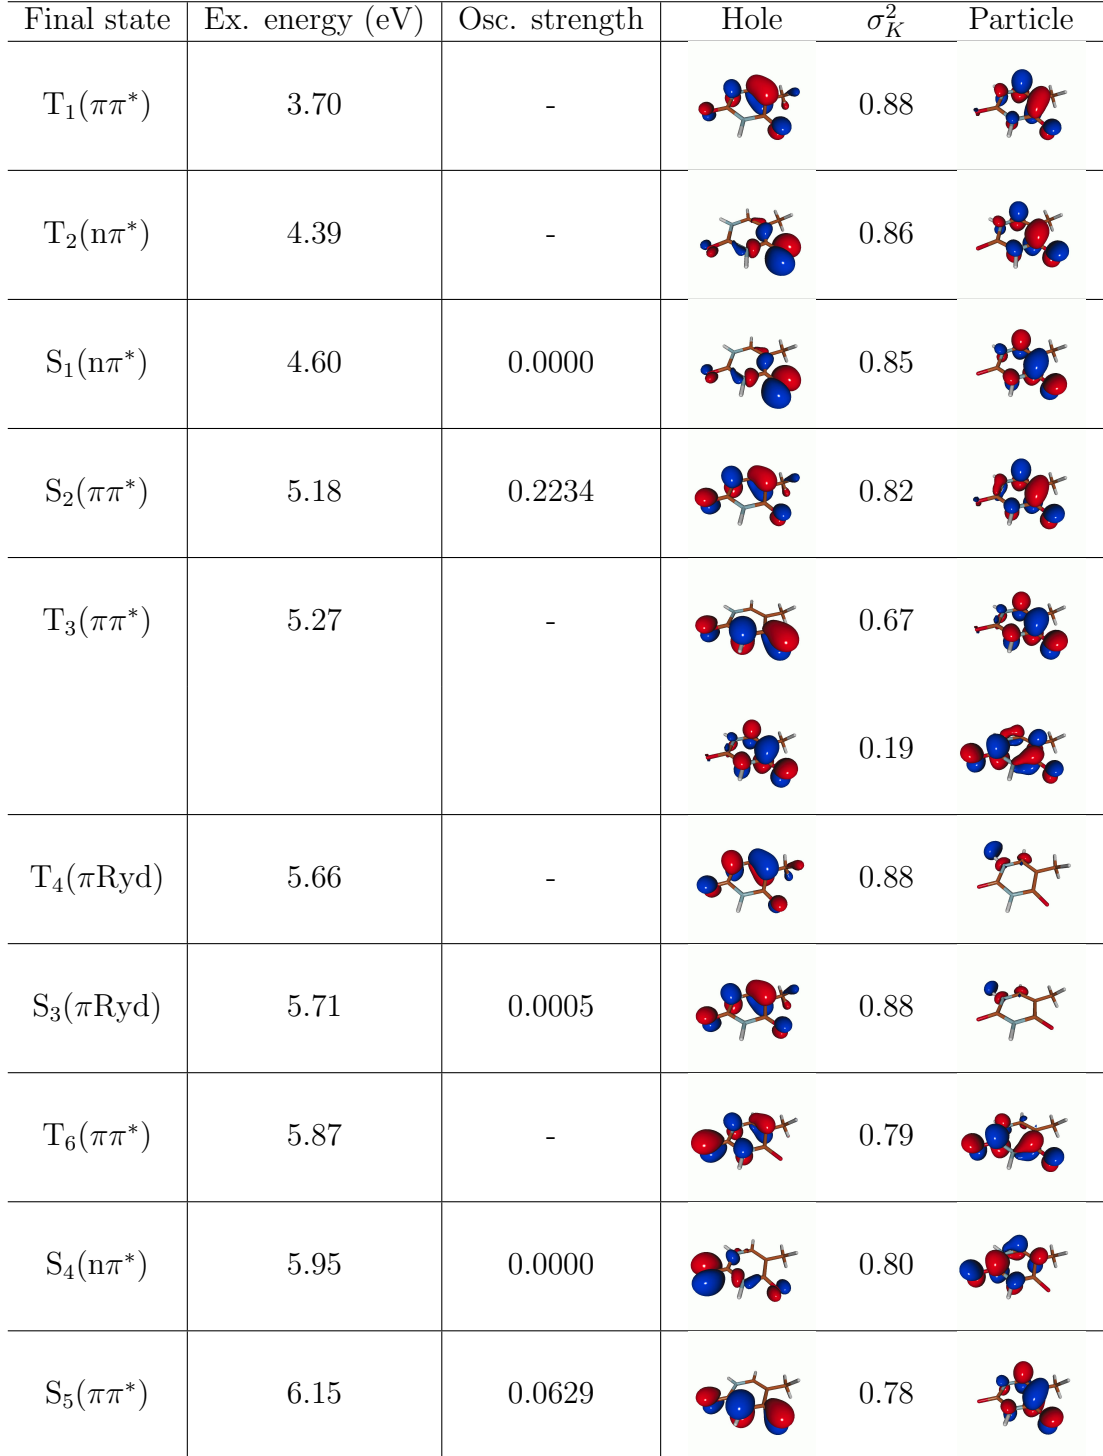 |
| $S_4(n\pi^*)$   | 5.95            | 0.0000        | 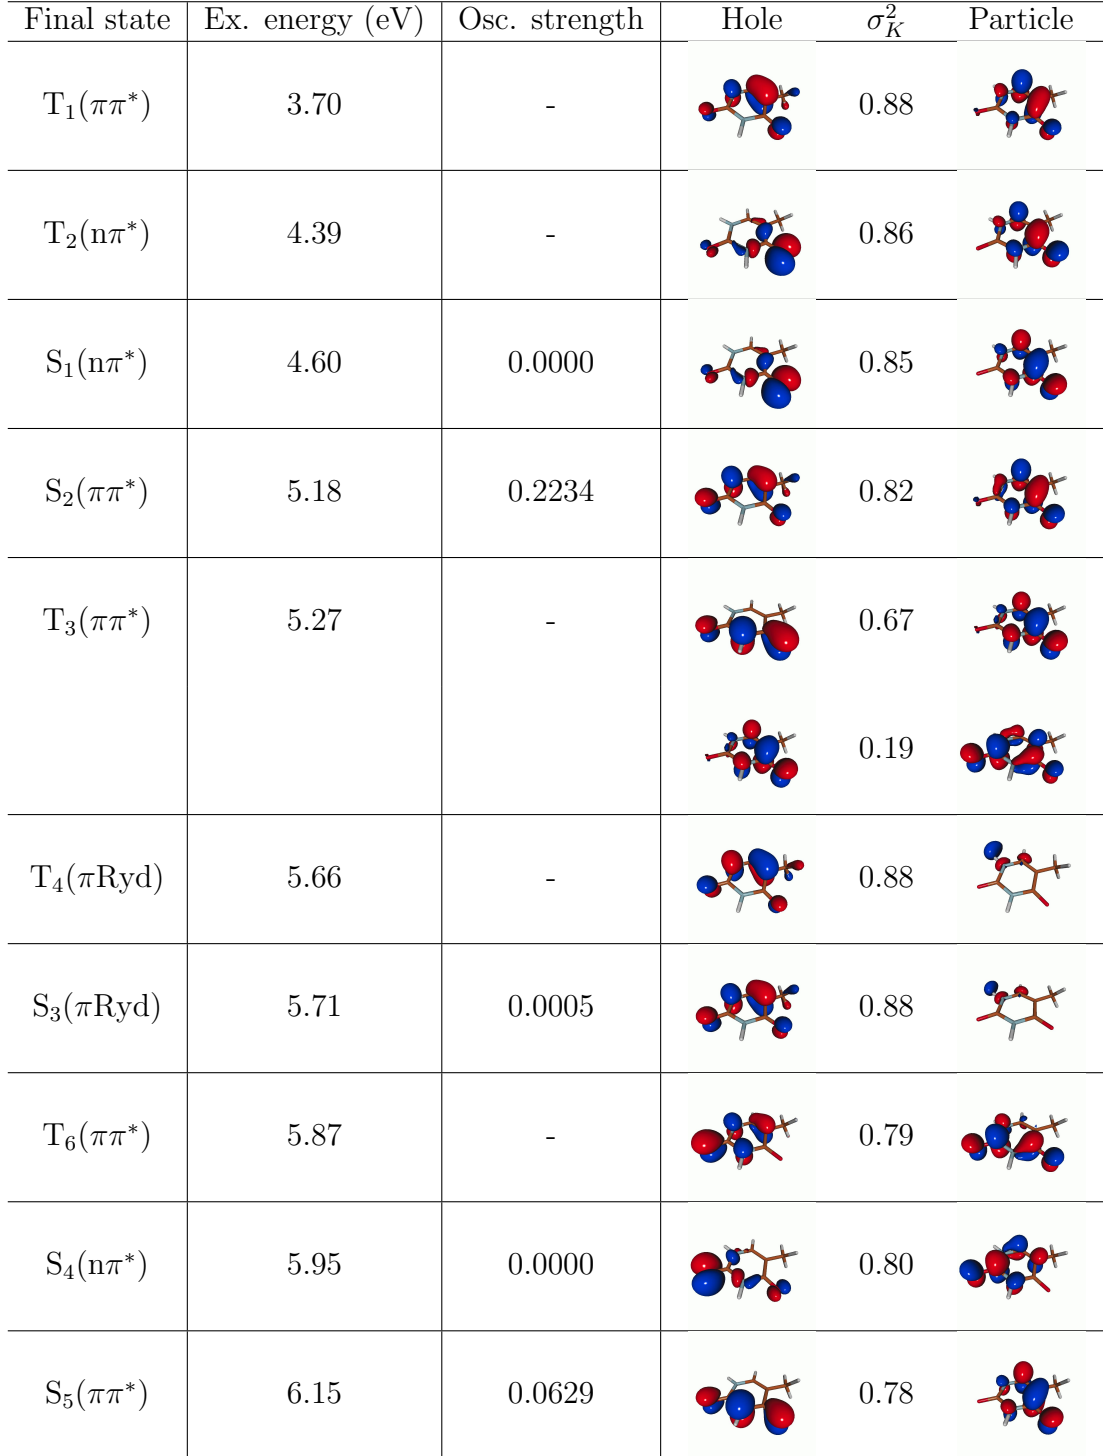 | 0.80         | 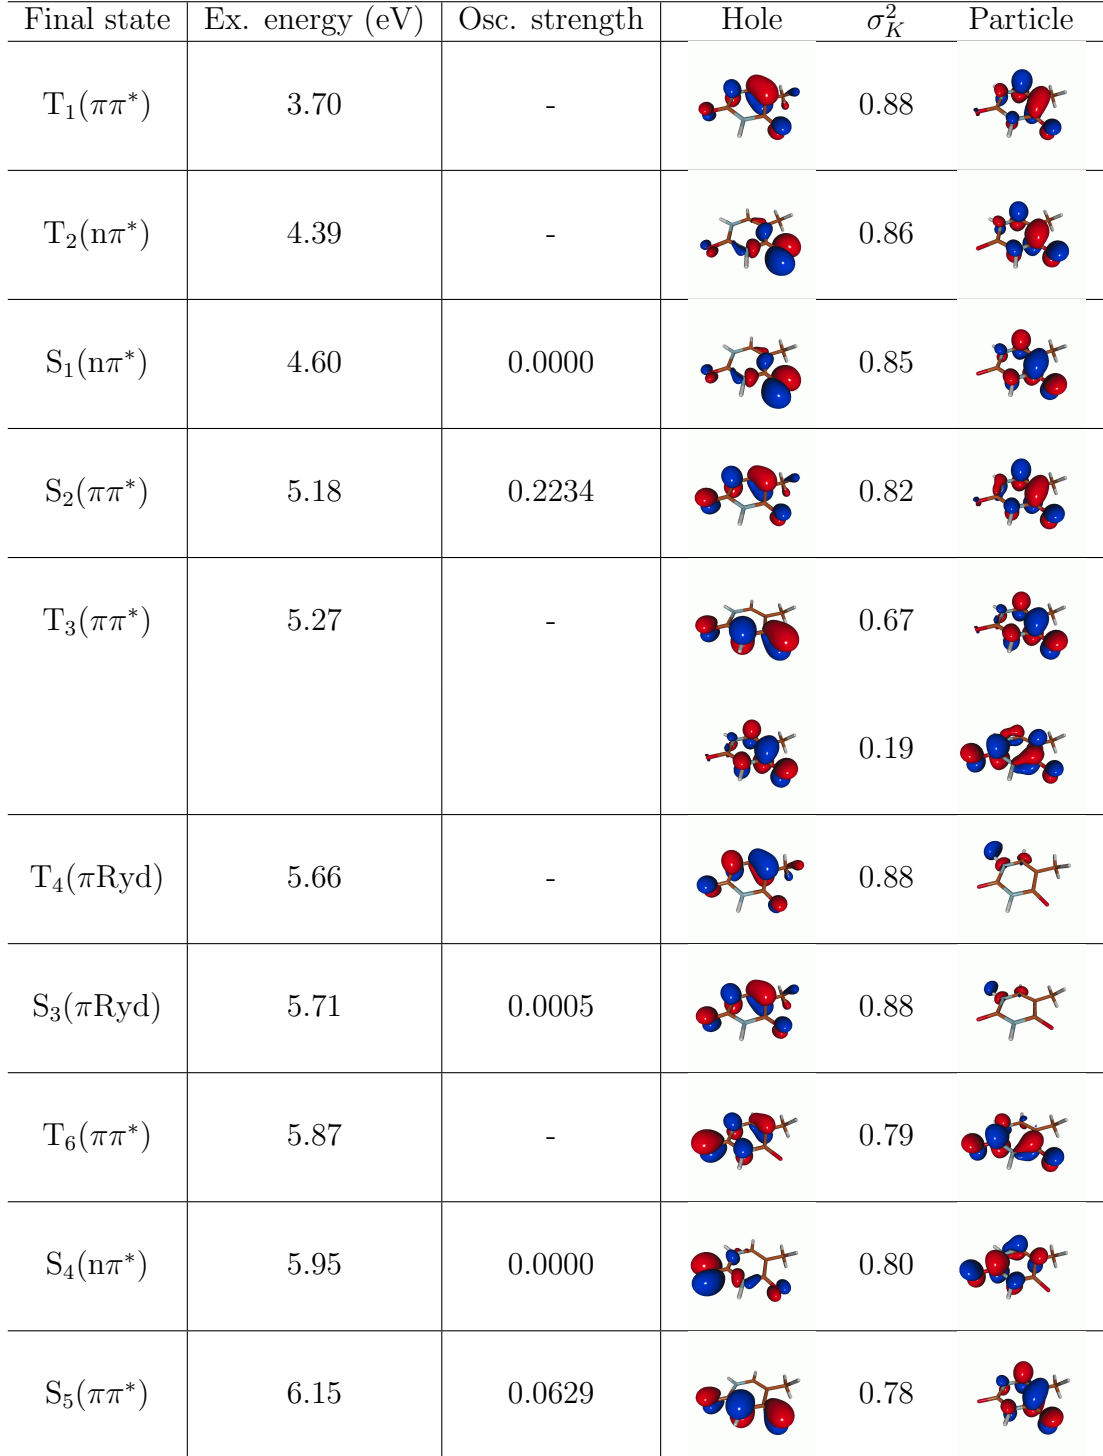 |
| $S_5(\pi\pi^*)$ | 6.15            | 0.0629        | 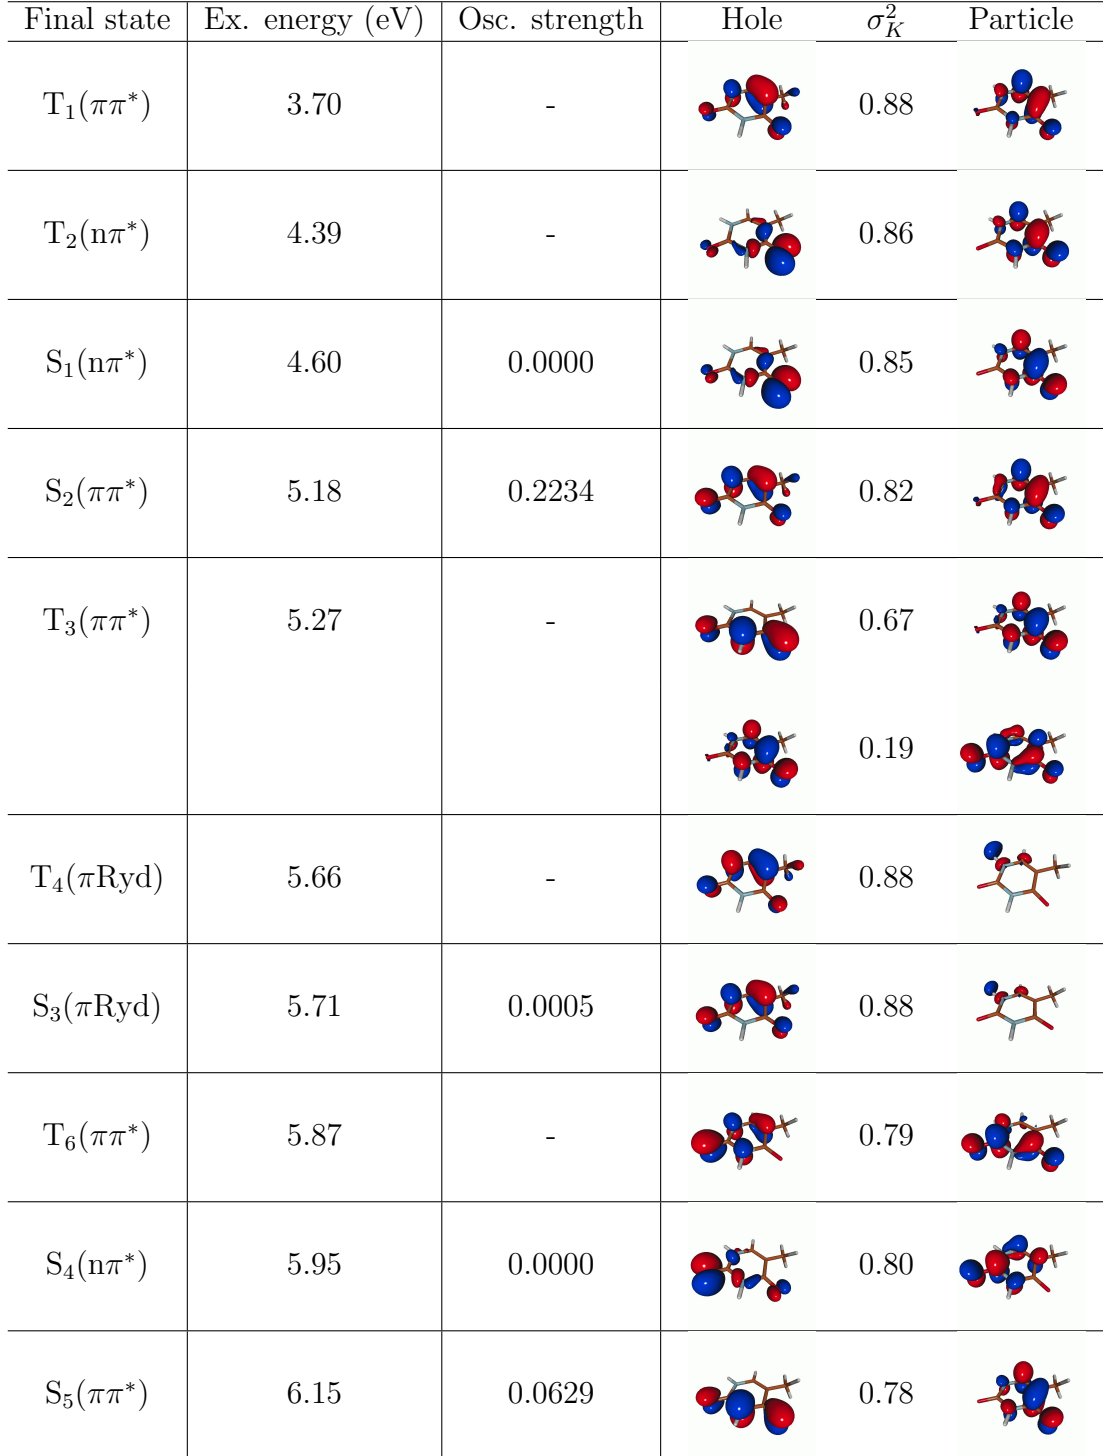 | 0.78         | 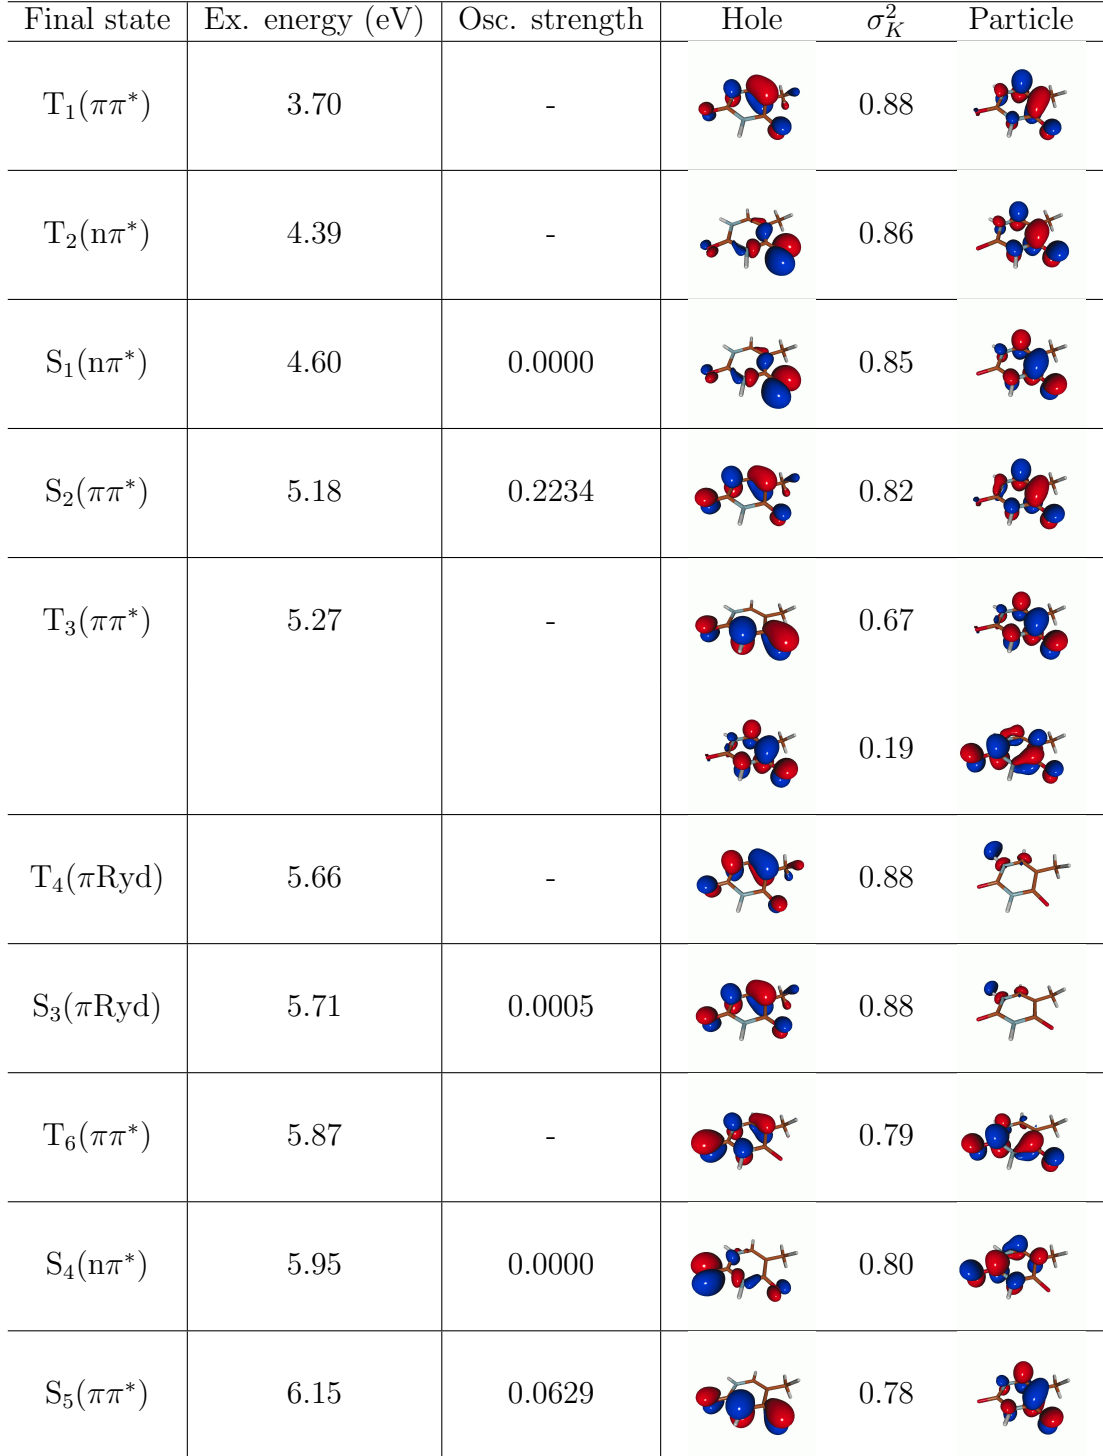 |

Table S15: Thymine. TDDFT/B3LYP/6-311++G\*\* NTOs of the excitations from the ground state to the lowest-lying valence-excited states at the FC geometry (NTO isosurface is 0.05).

| Final state     | Ex. energy (eV) | Osc. strength | Hole                                                                                 | $\sigma_K^2$ | Particle                                                                              |
|-----------------|-----------------|---------------|--------------------------------------------------------------------------------------|--------------|---------------------------------------------------------------------------------------|
| $T_1(\pi\pi^*)$ | 3.19            | -             | 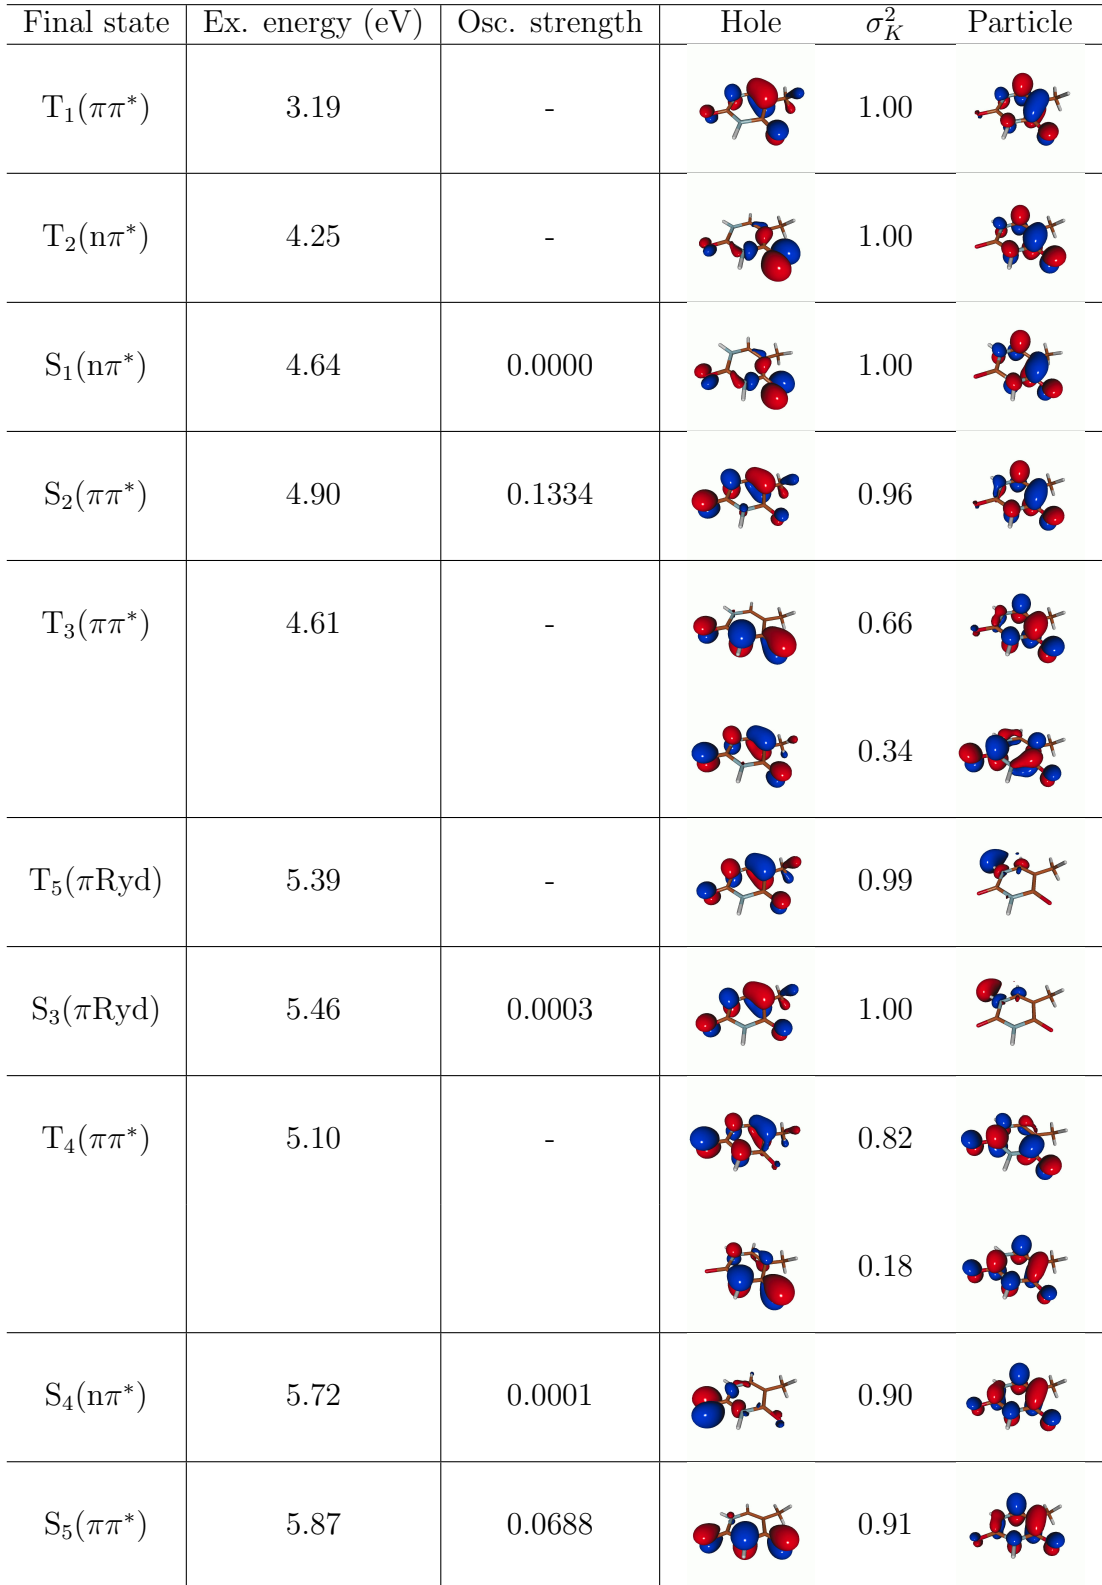   | 1.00         | 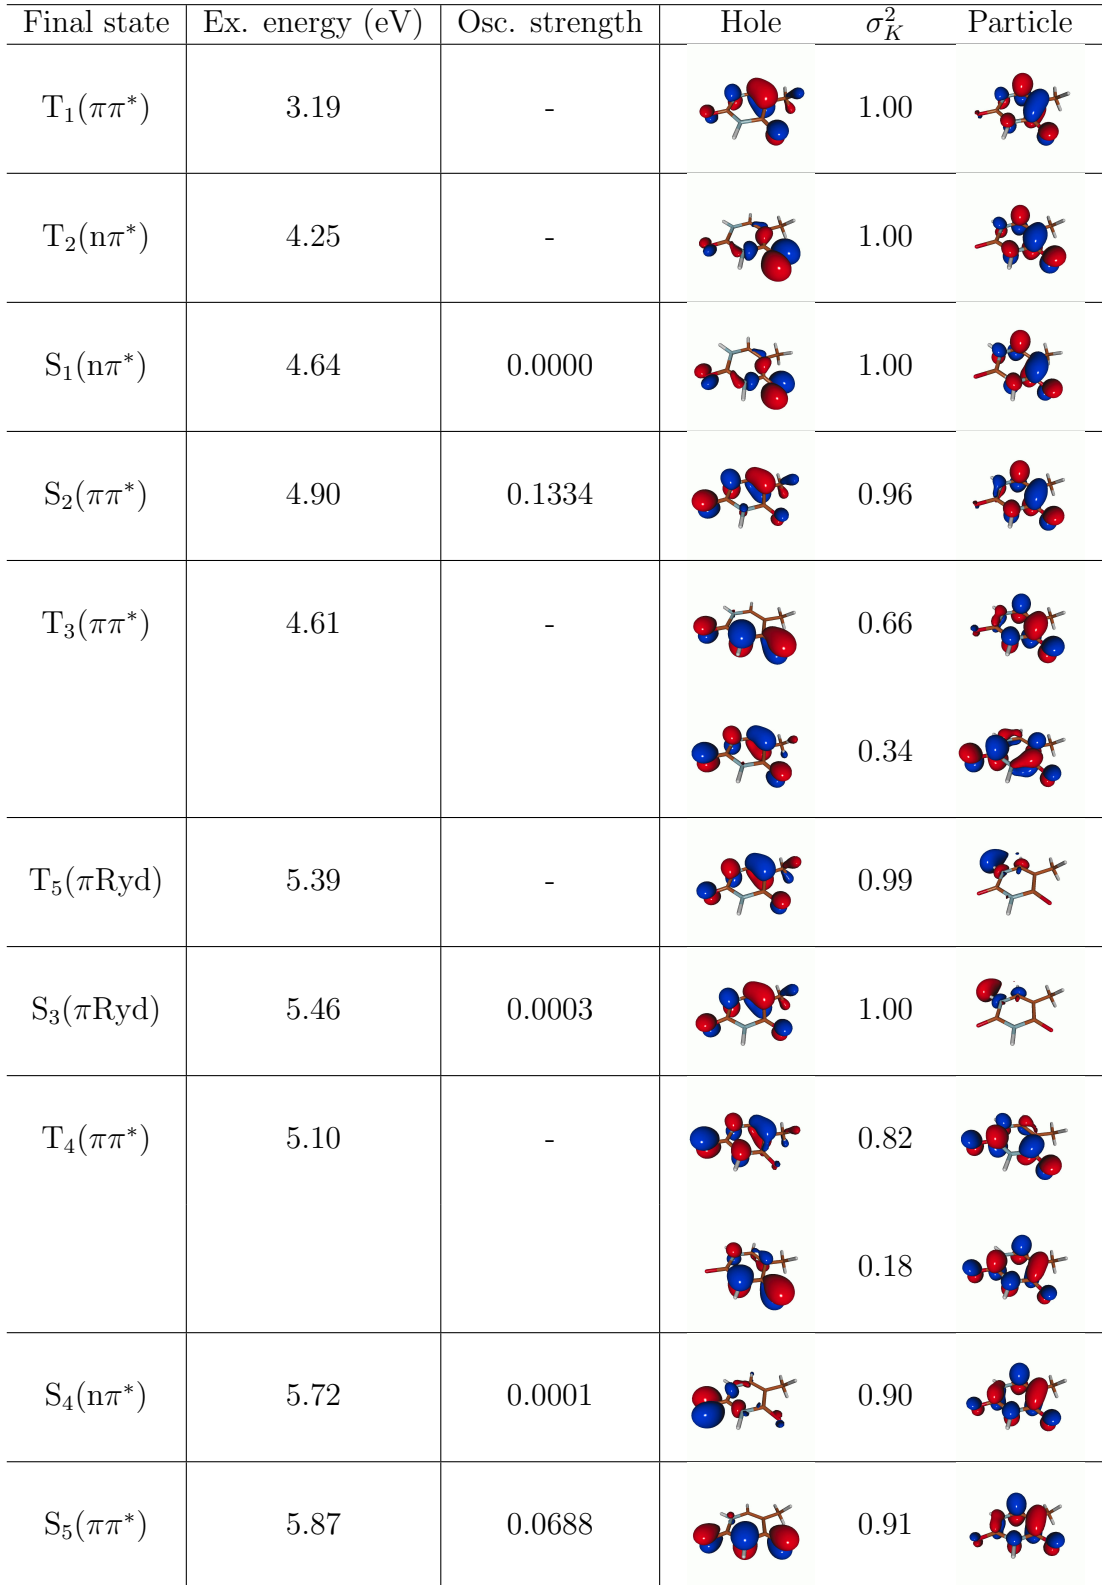   |
| $T_2(n\pi^*)$   | 4.25            | -             | 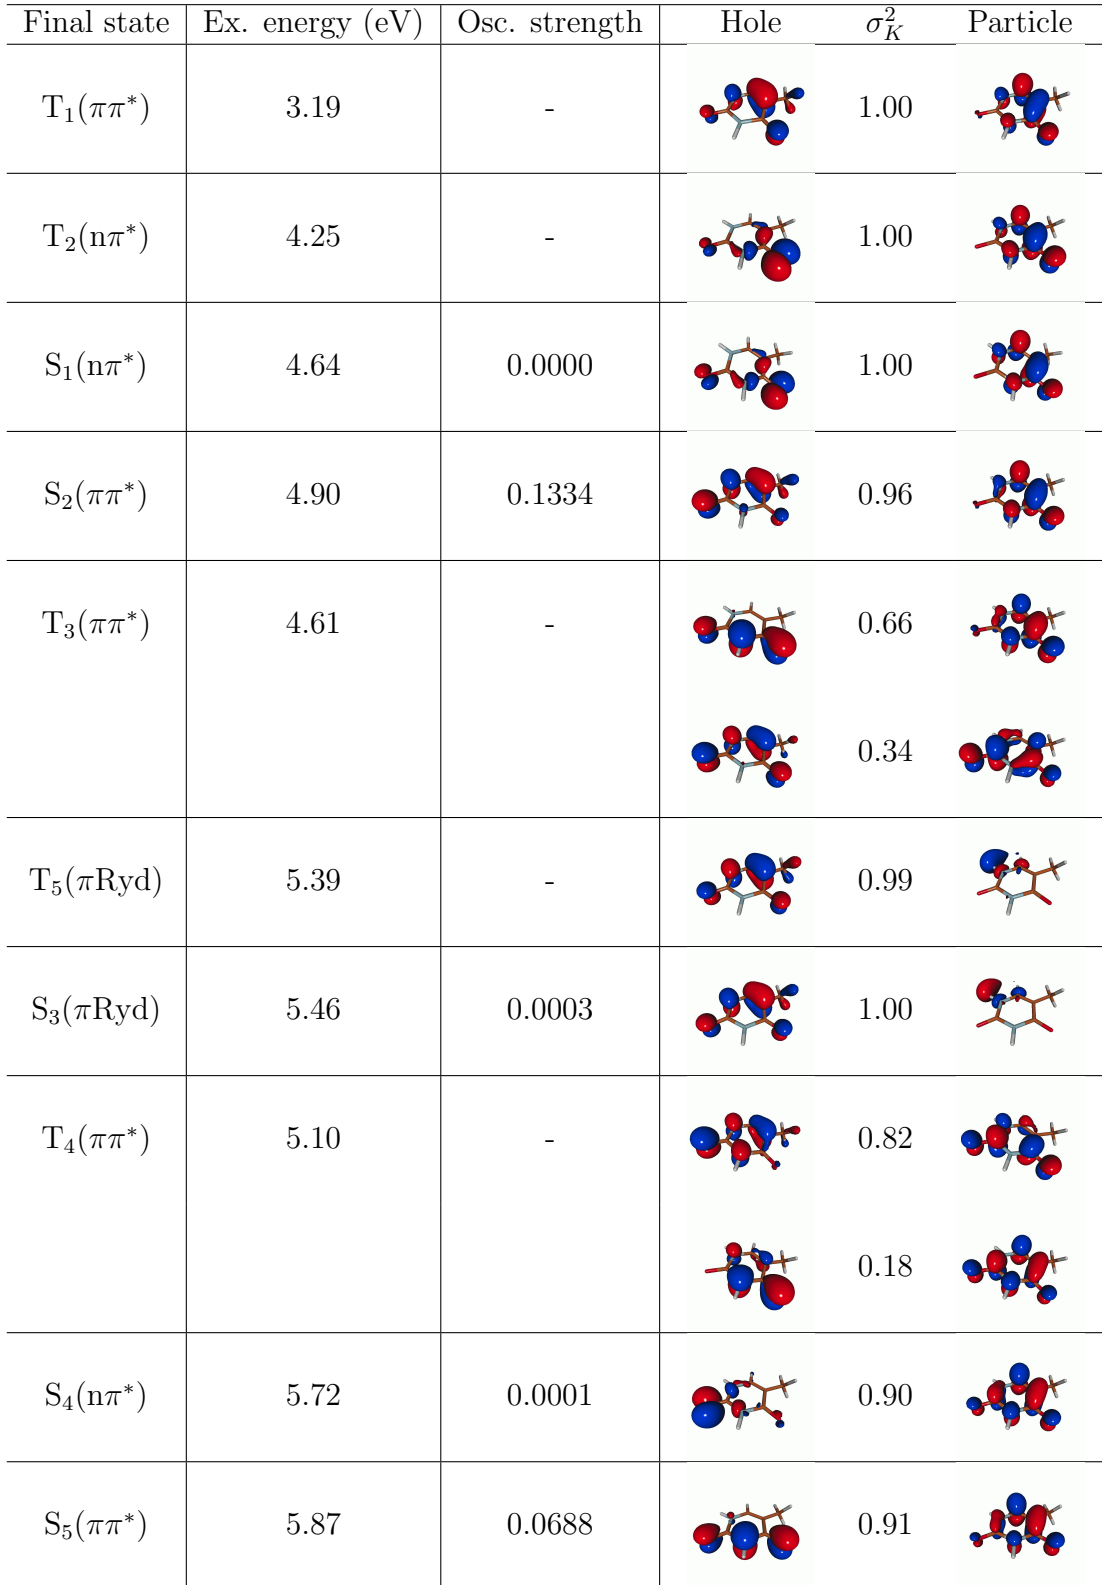   | 1.00         | 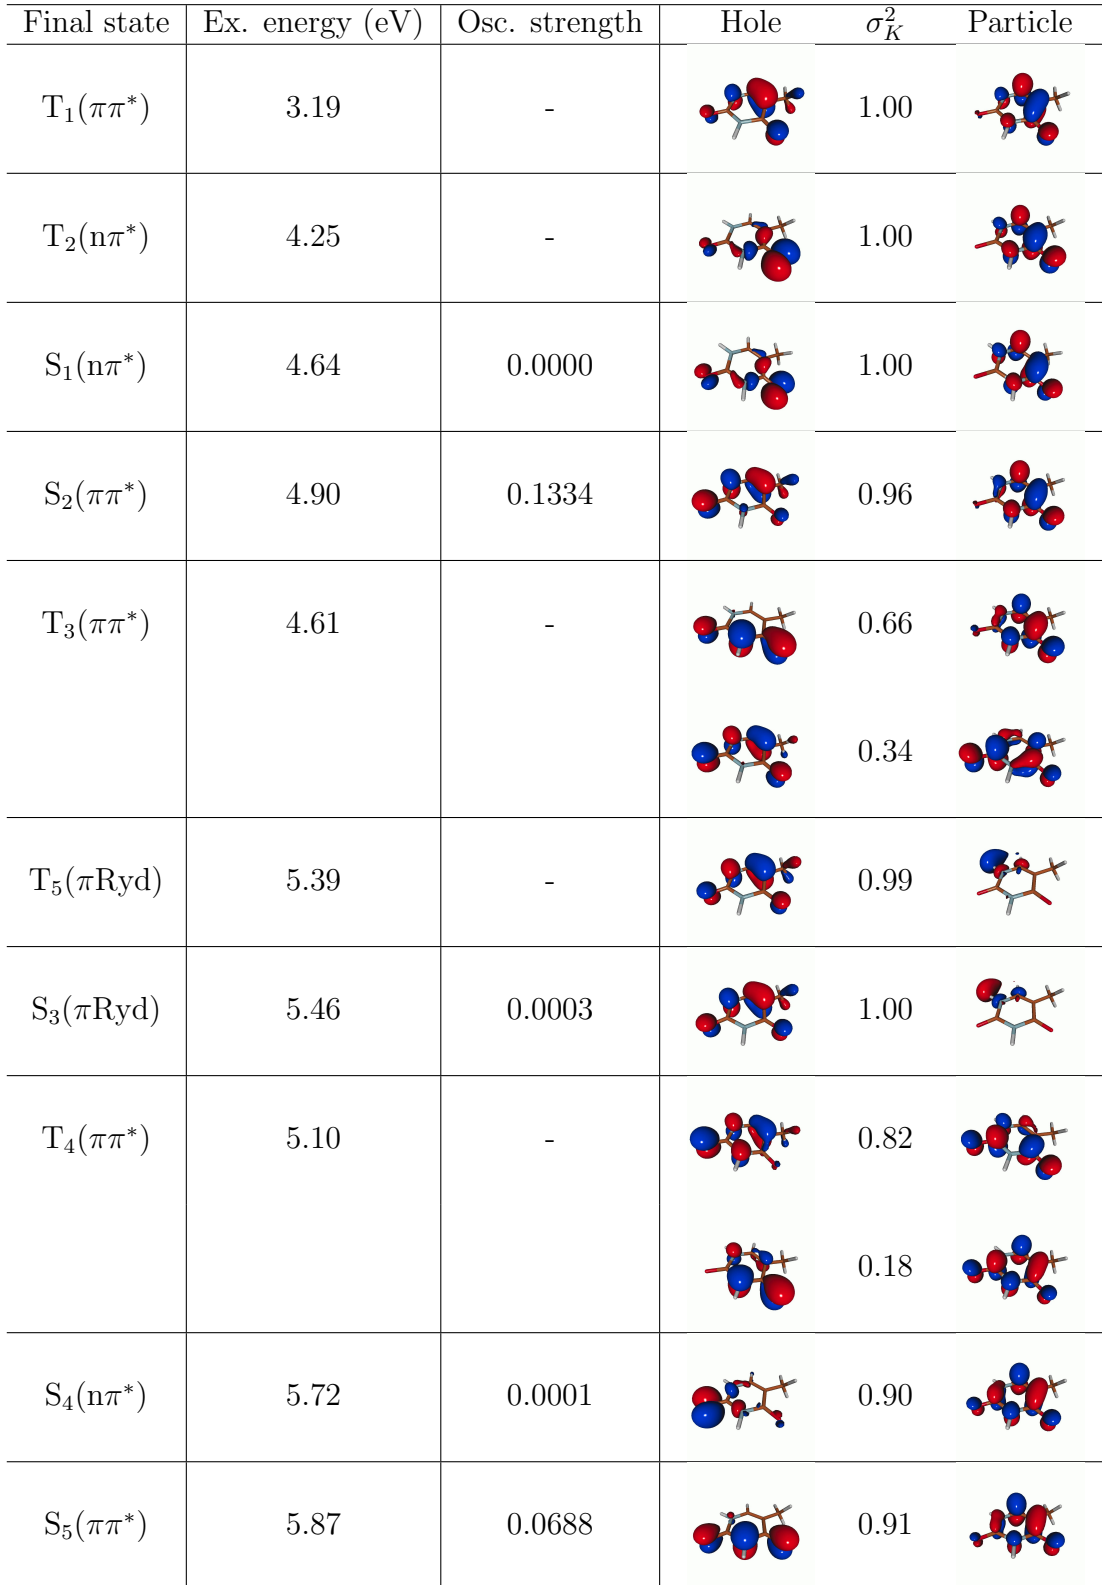   |
| $S_1(n\pi^*)$   | 4.64            | 0.0000        | 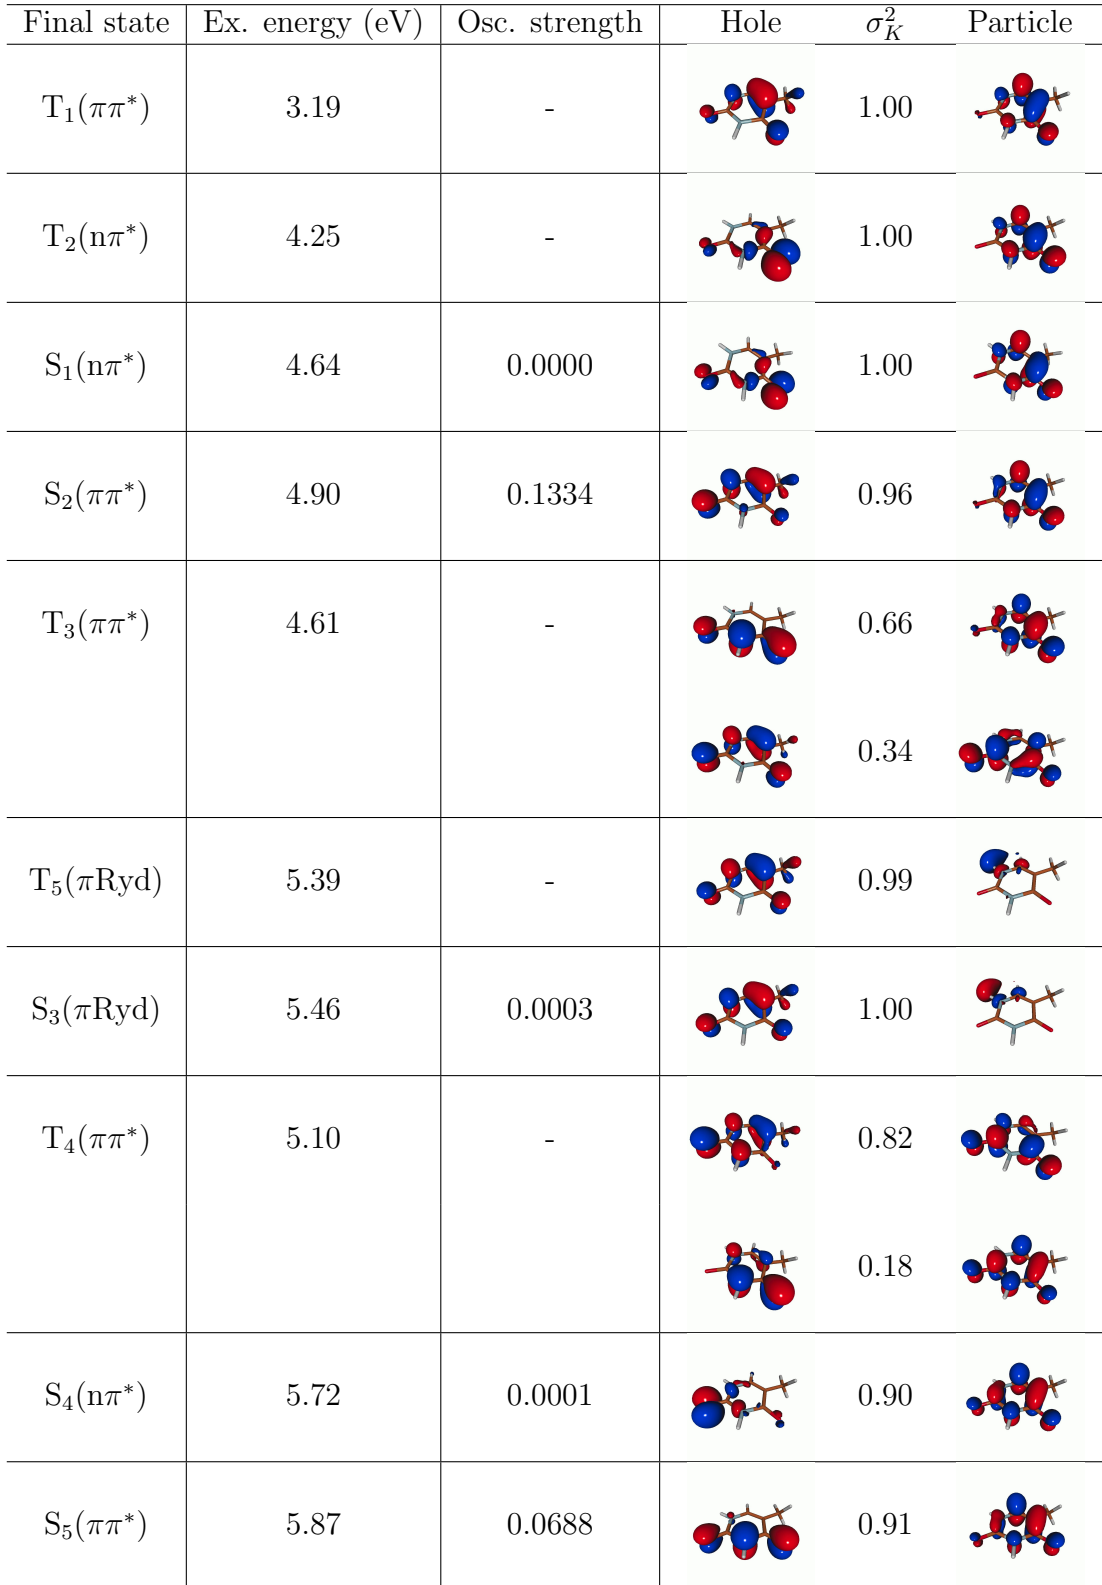   | 1.00         | 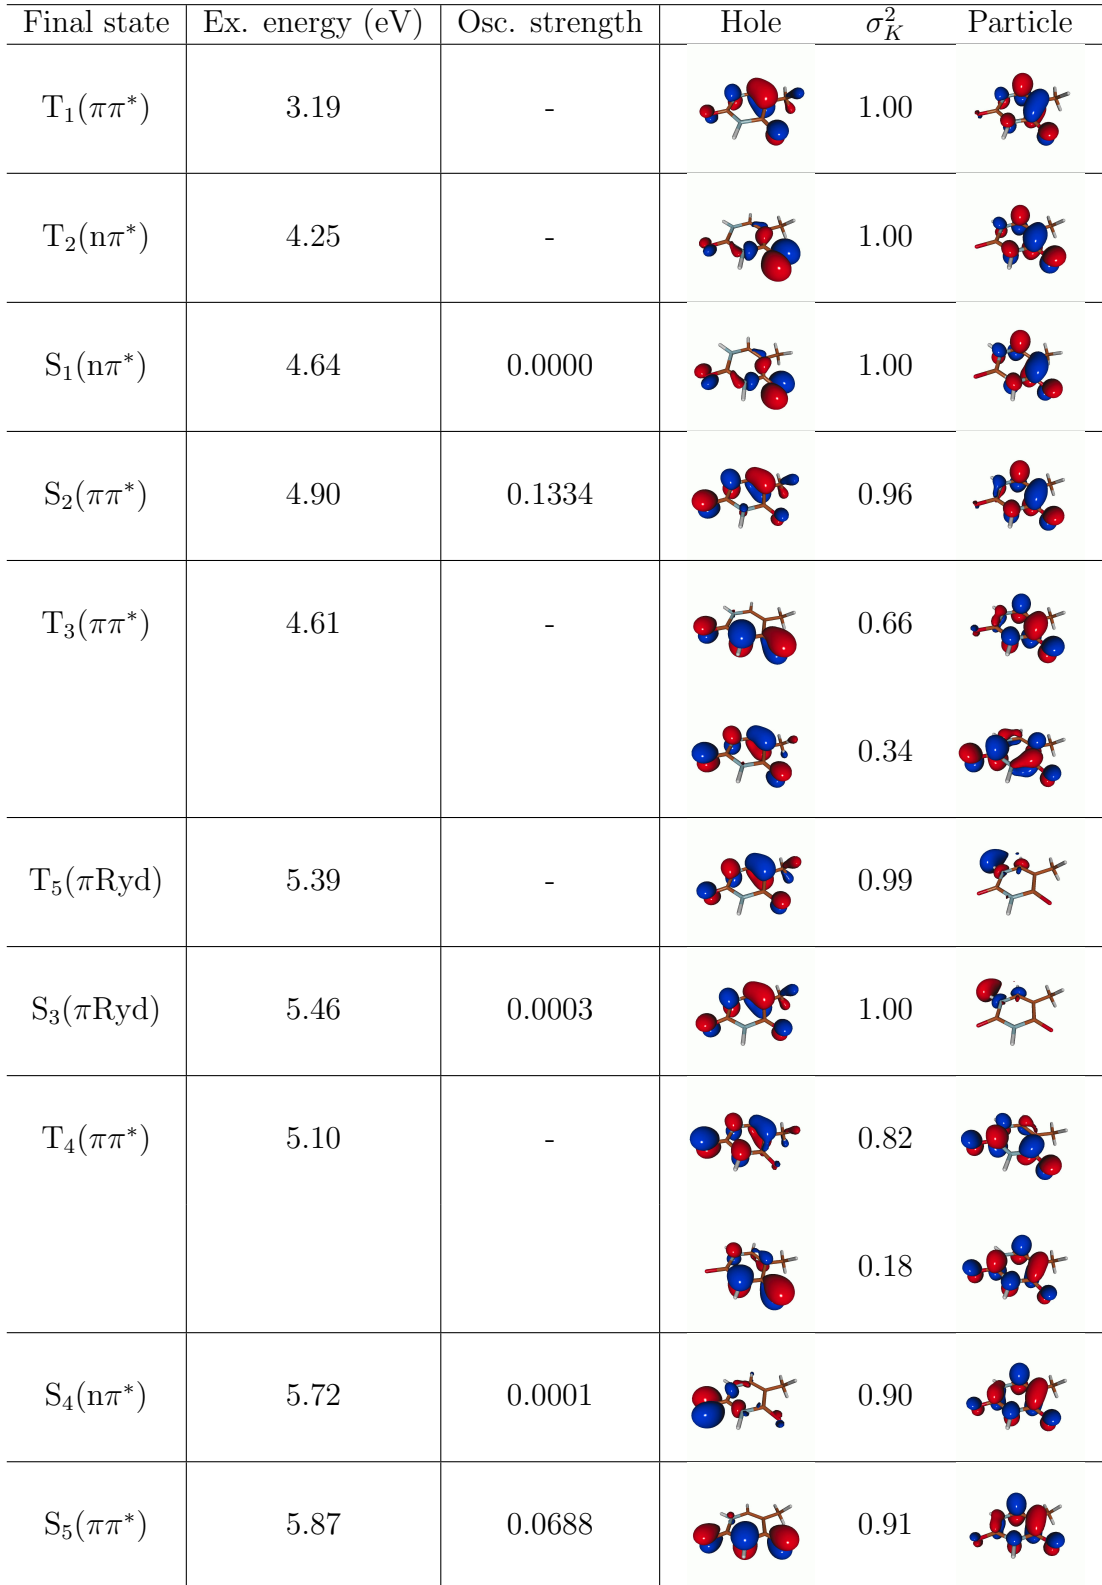   |
| $S_2(\pi\pi^*)$ | 4.90            | 0.1334        | 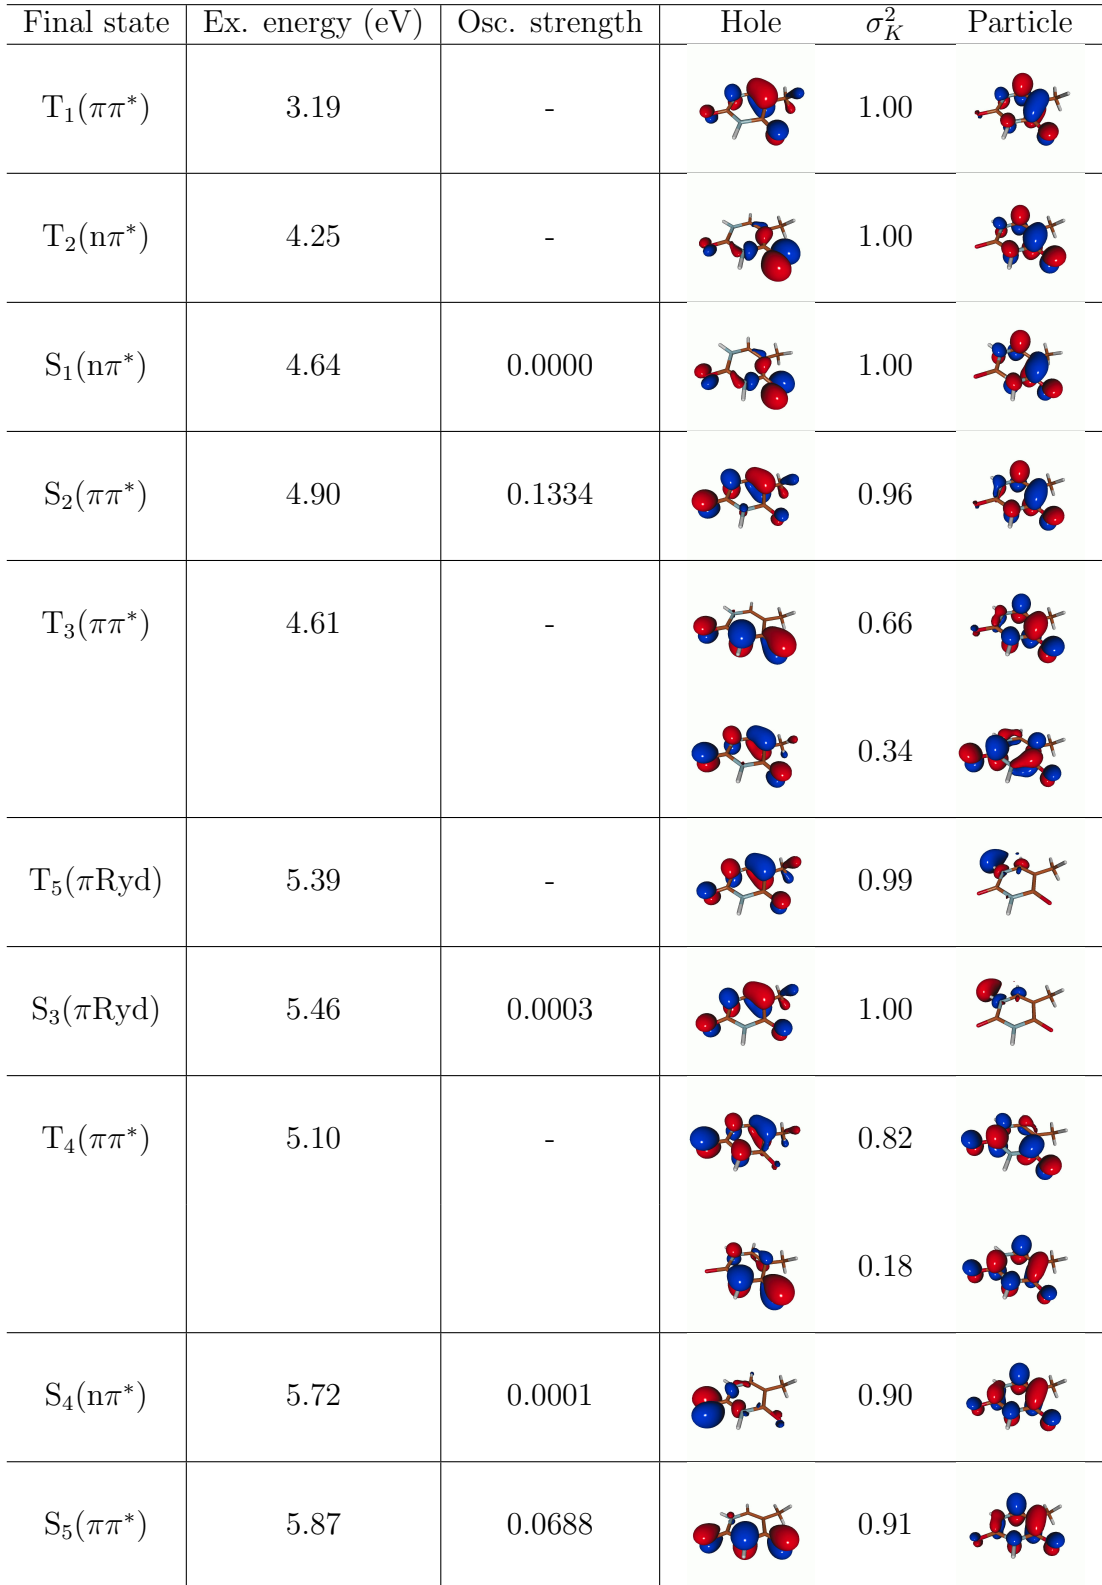   | 0.96         | 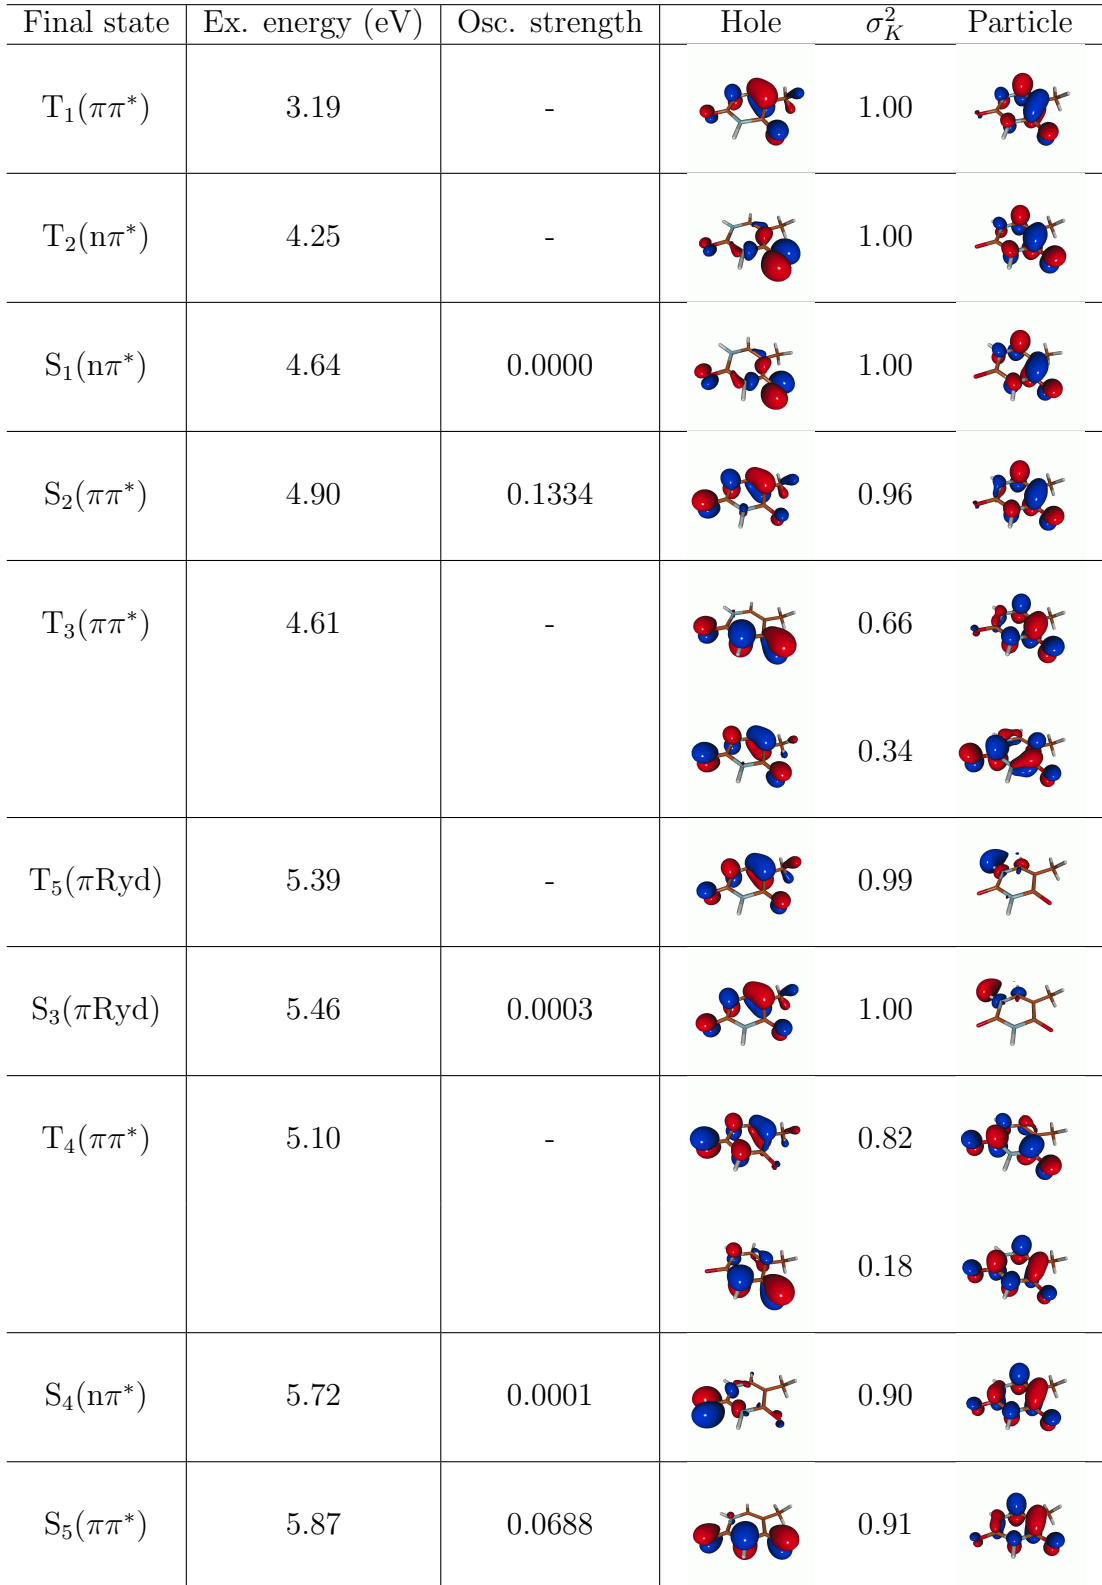   |
| $T_3(\pi\pi^*)$ | 4.61            | -             | 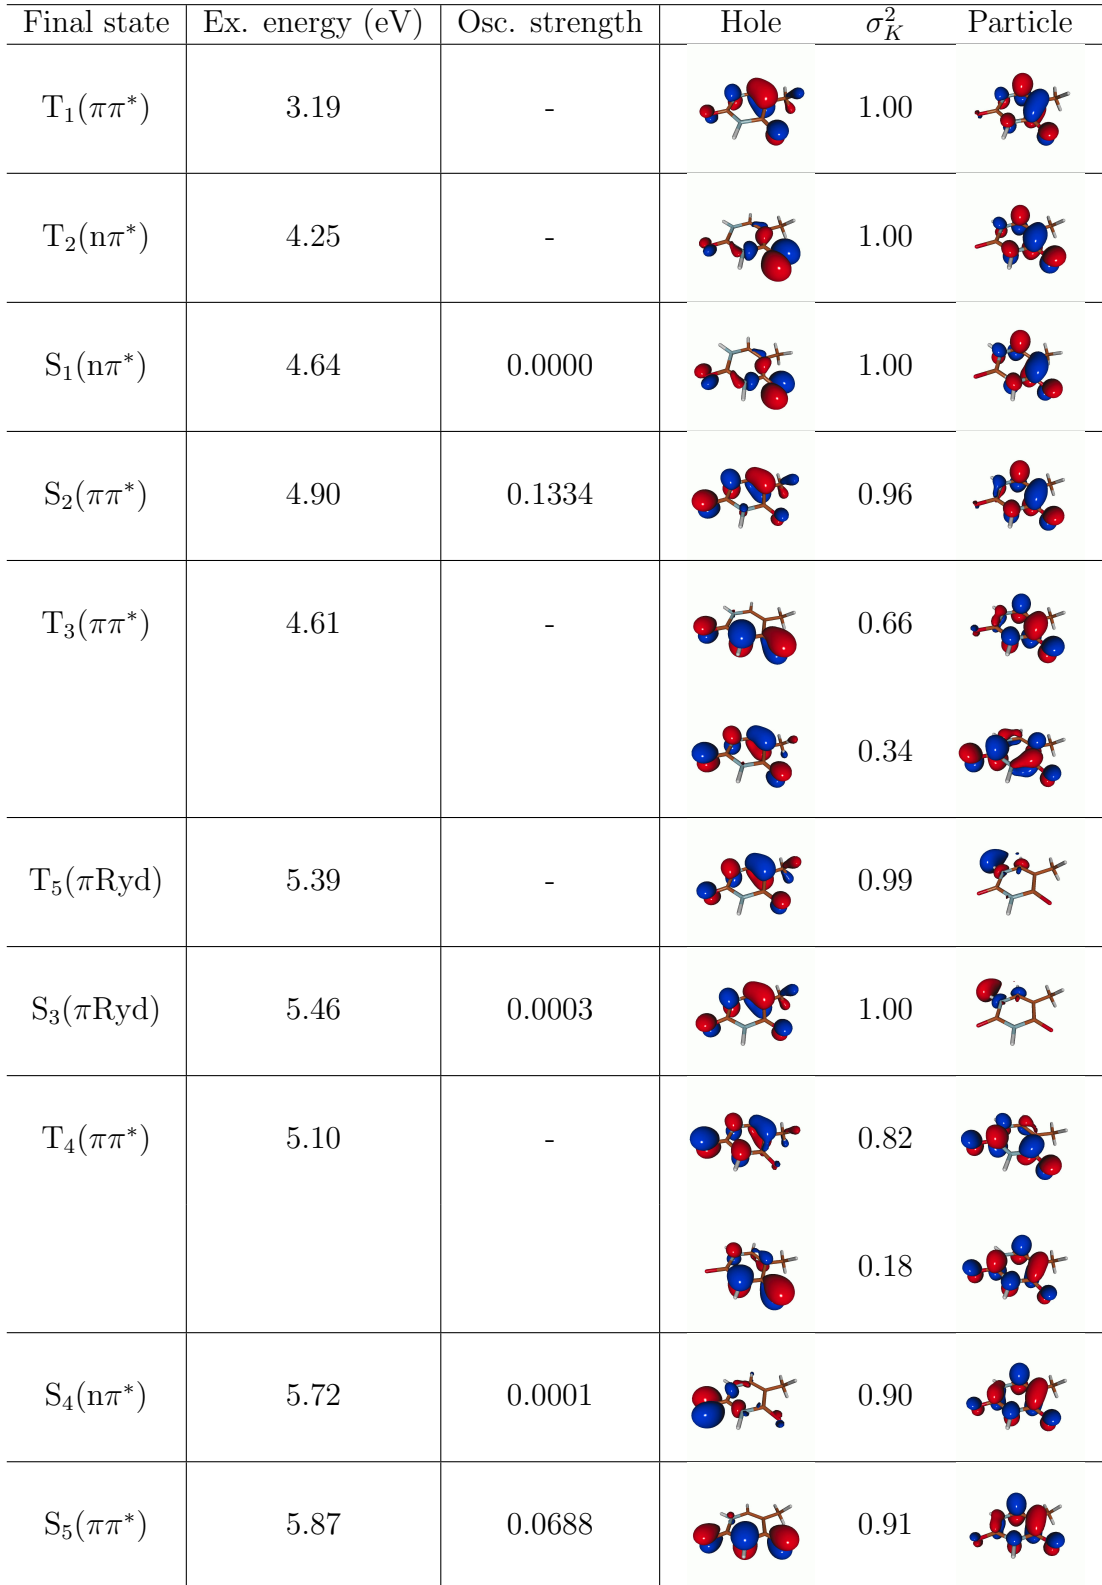  | 0.66         | 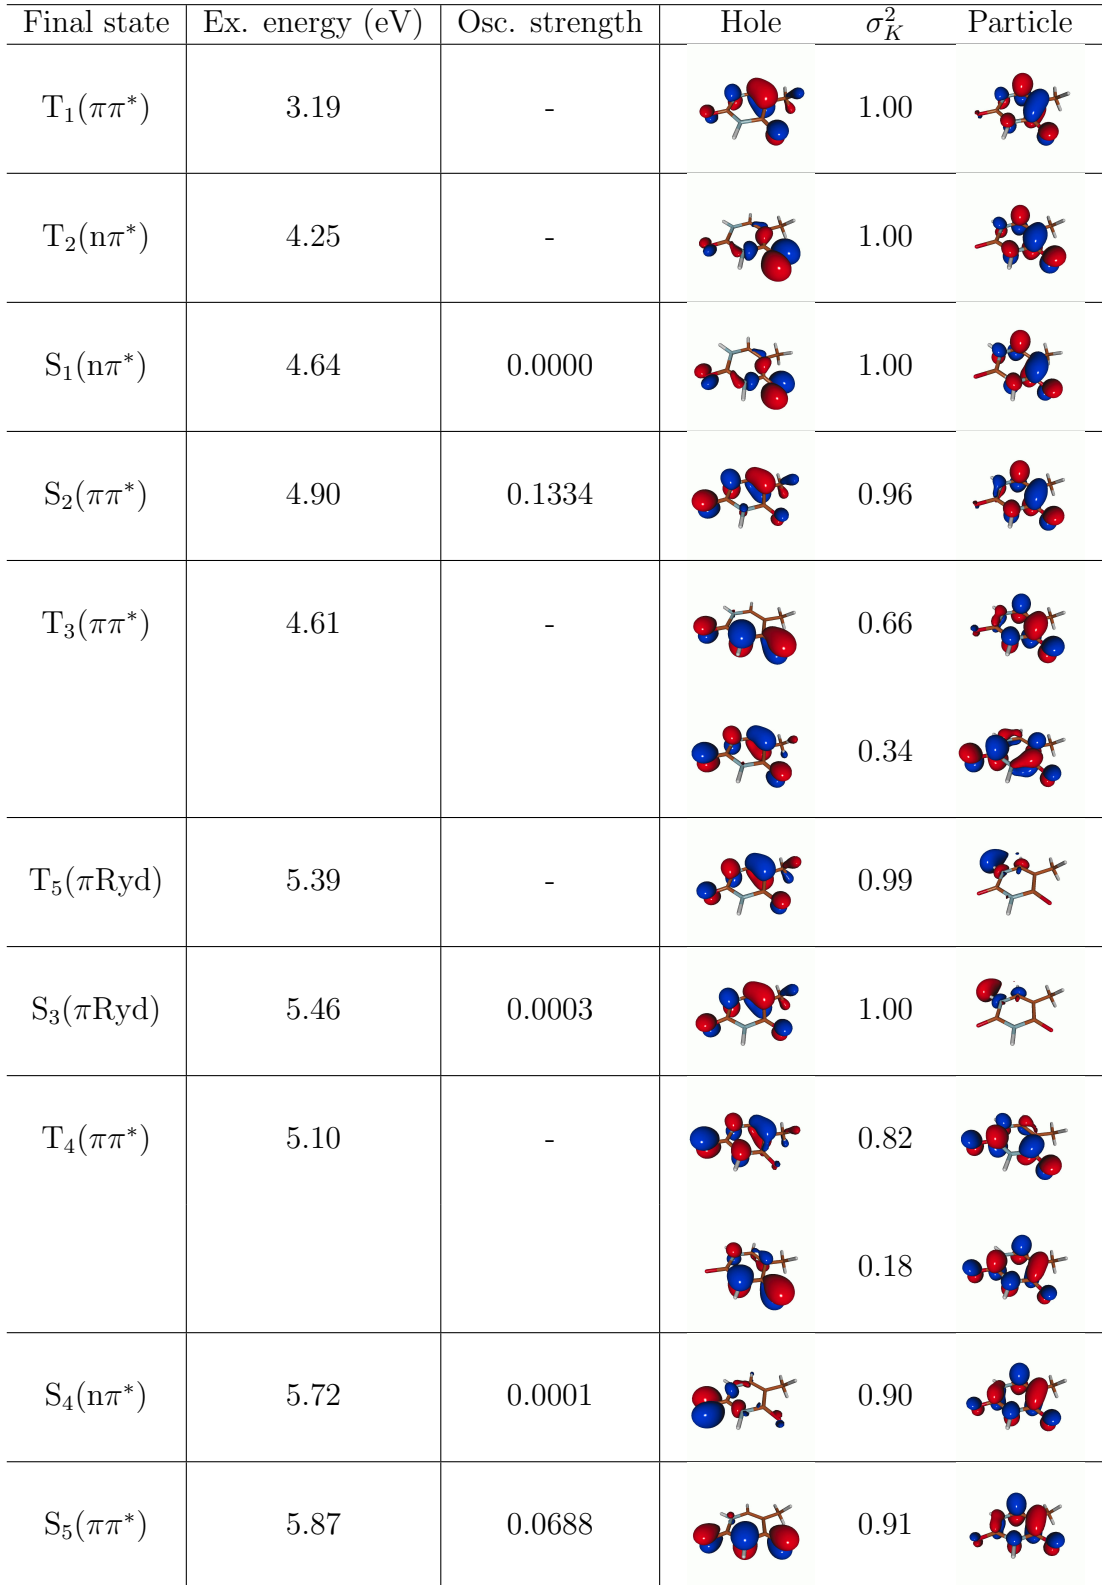  |
|                 |                 |               | 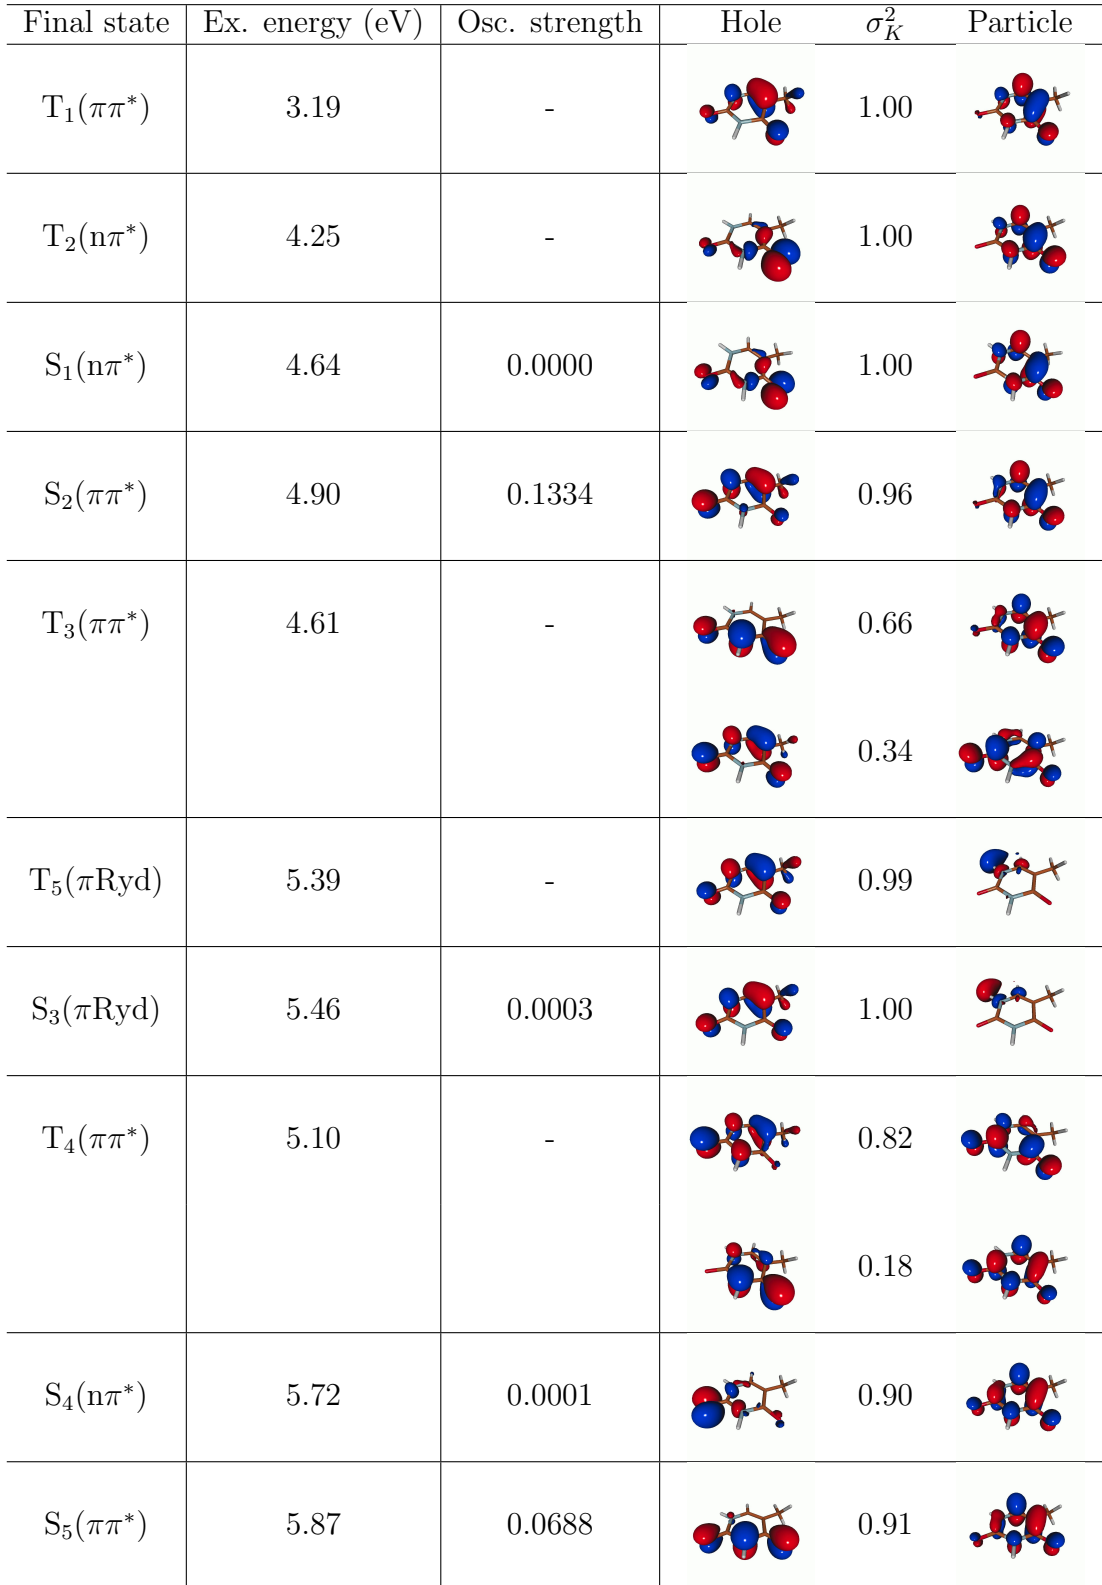 | 0.34         | 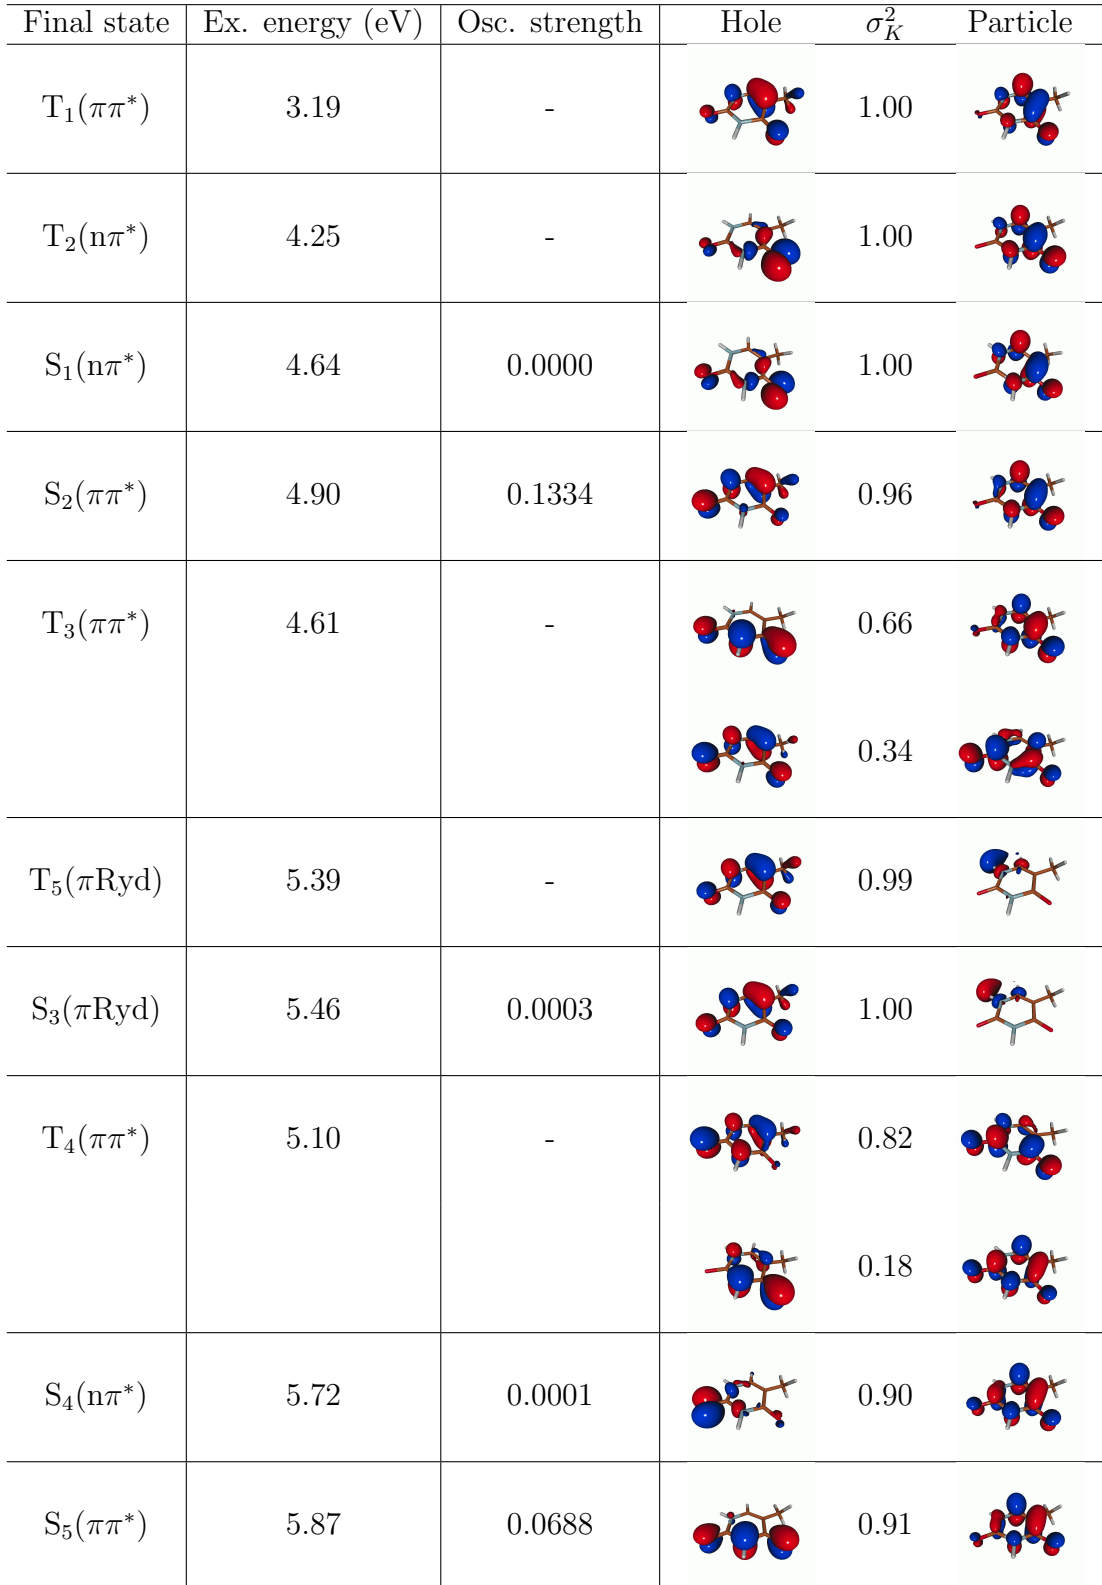 |
| $T_5(\pi Ryd)$  | 5.39            | -             | 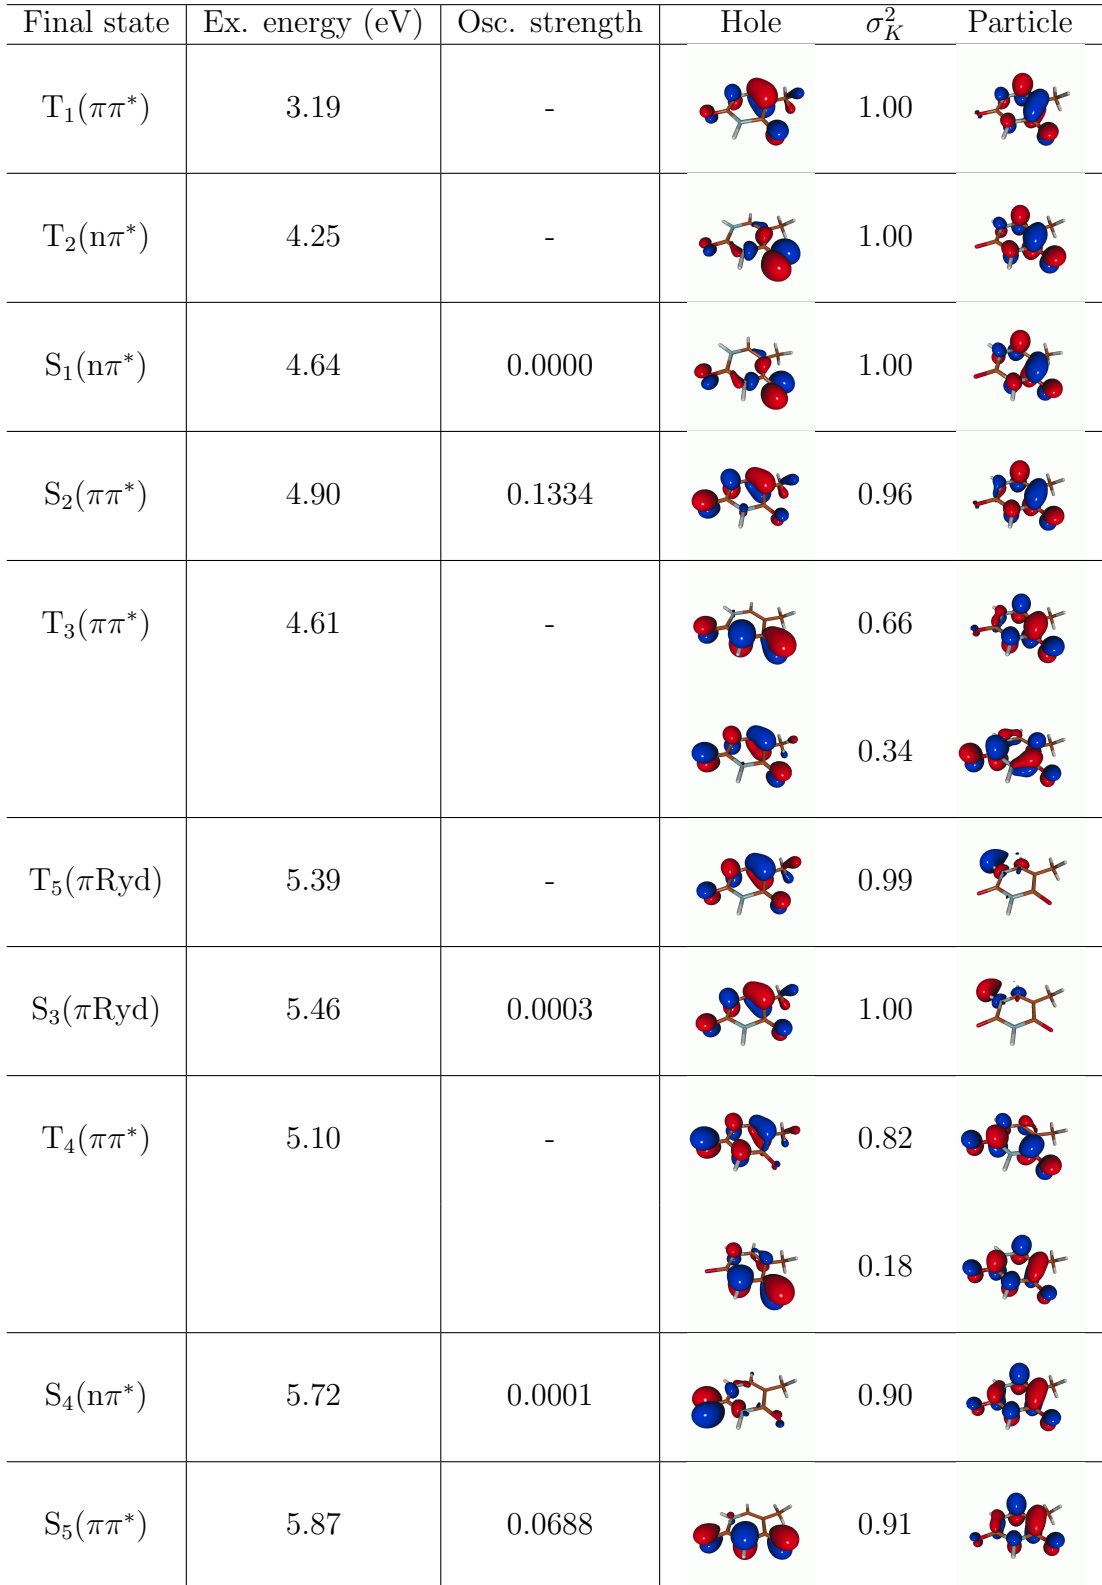 | 0.99         | 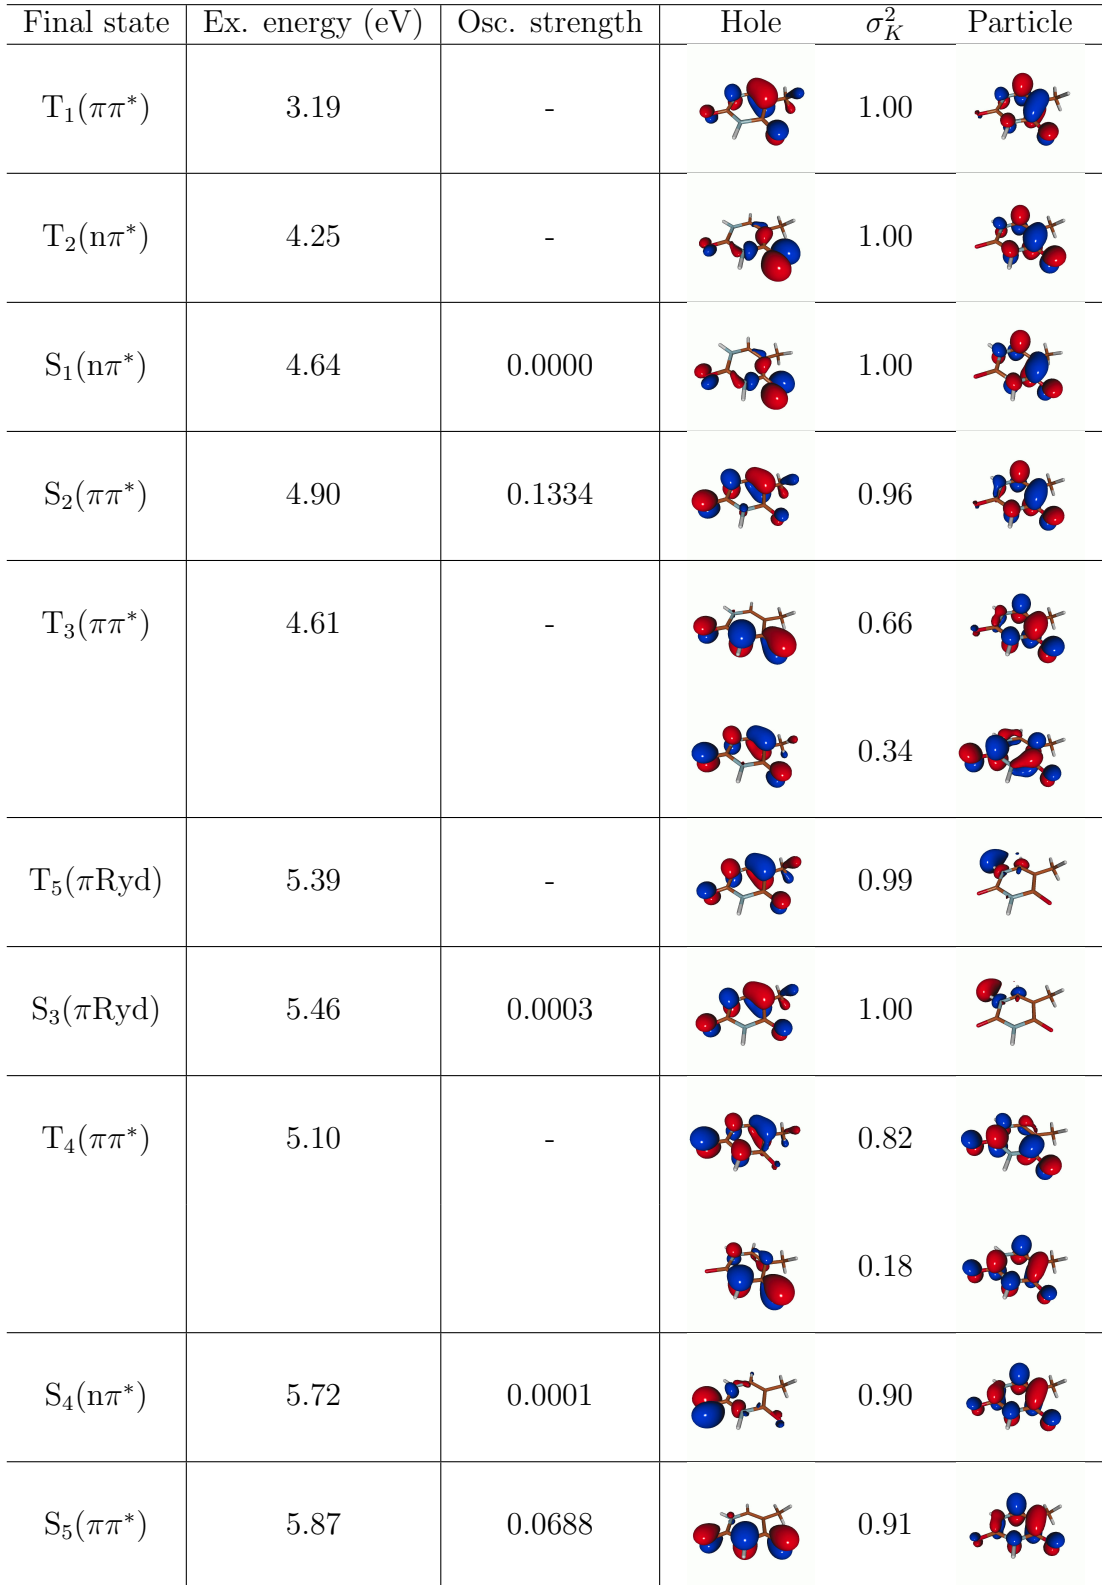 |
| $S_3(\pi Ryd)$  | 5.46            | 0.0003        | 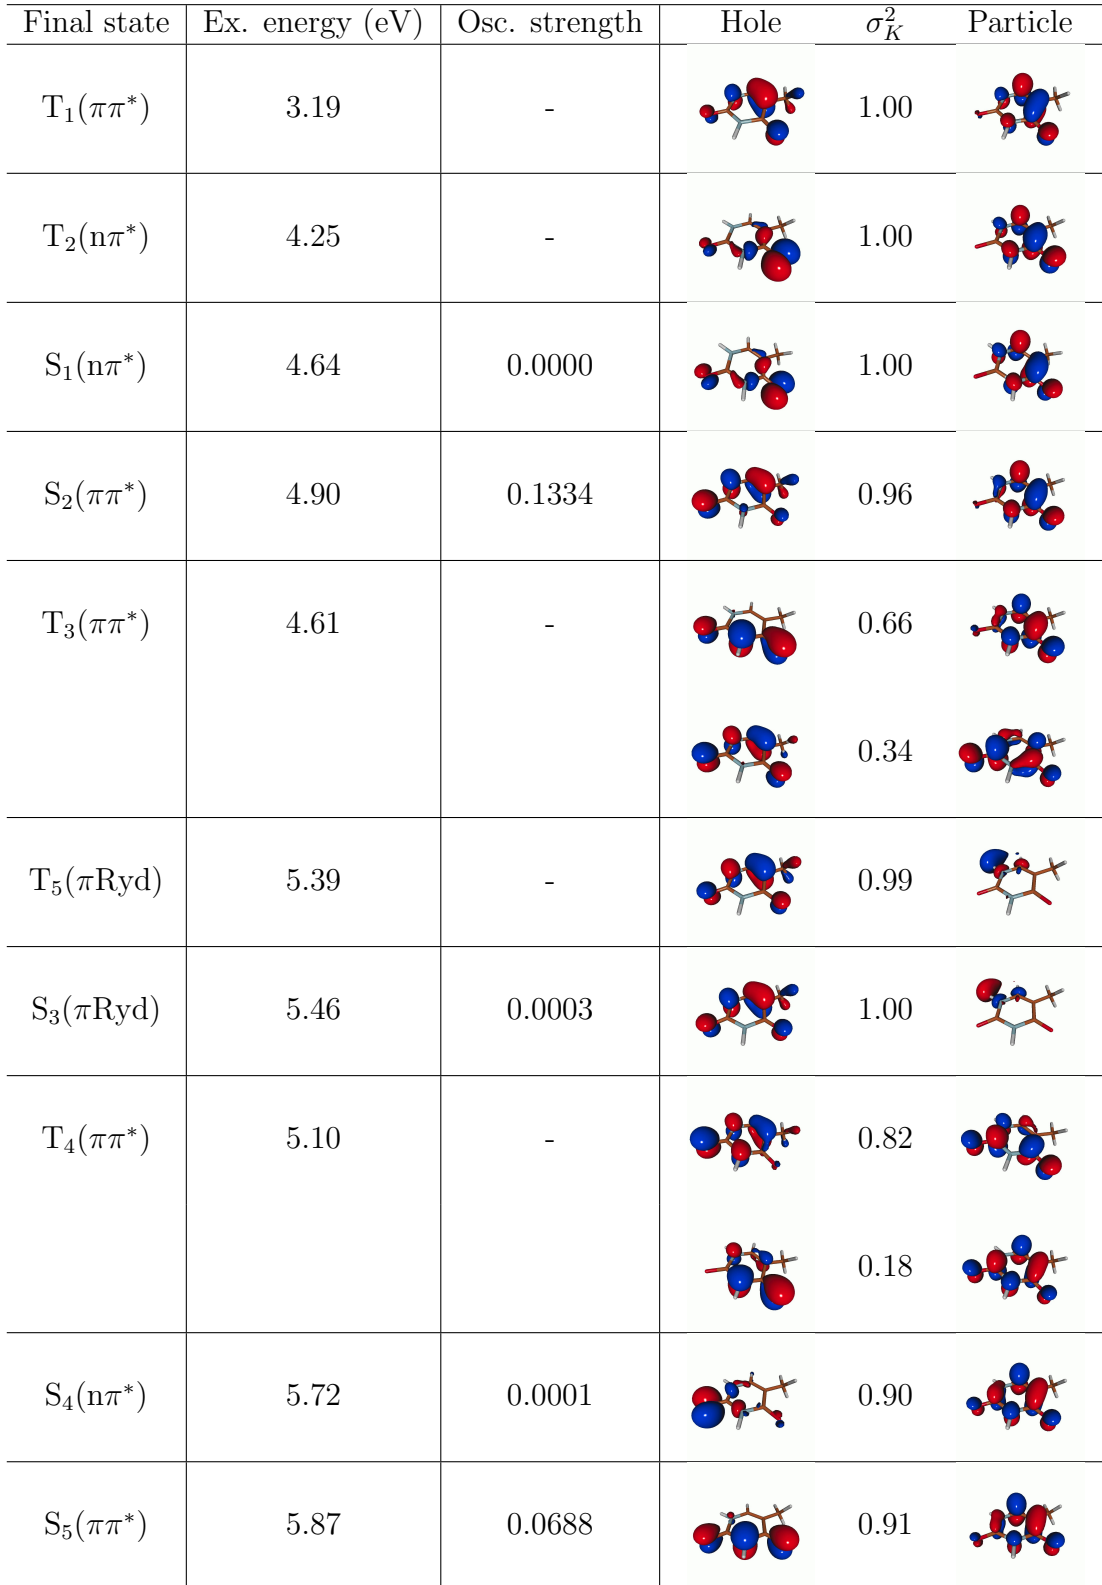 | 1.00         | 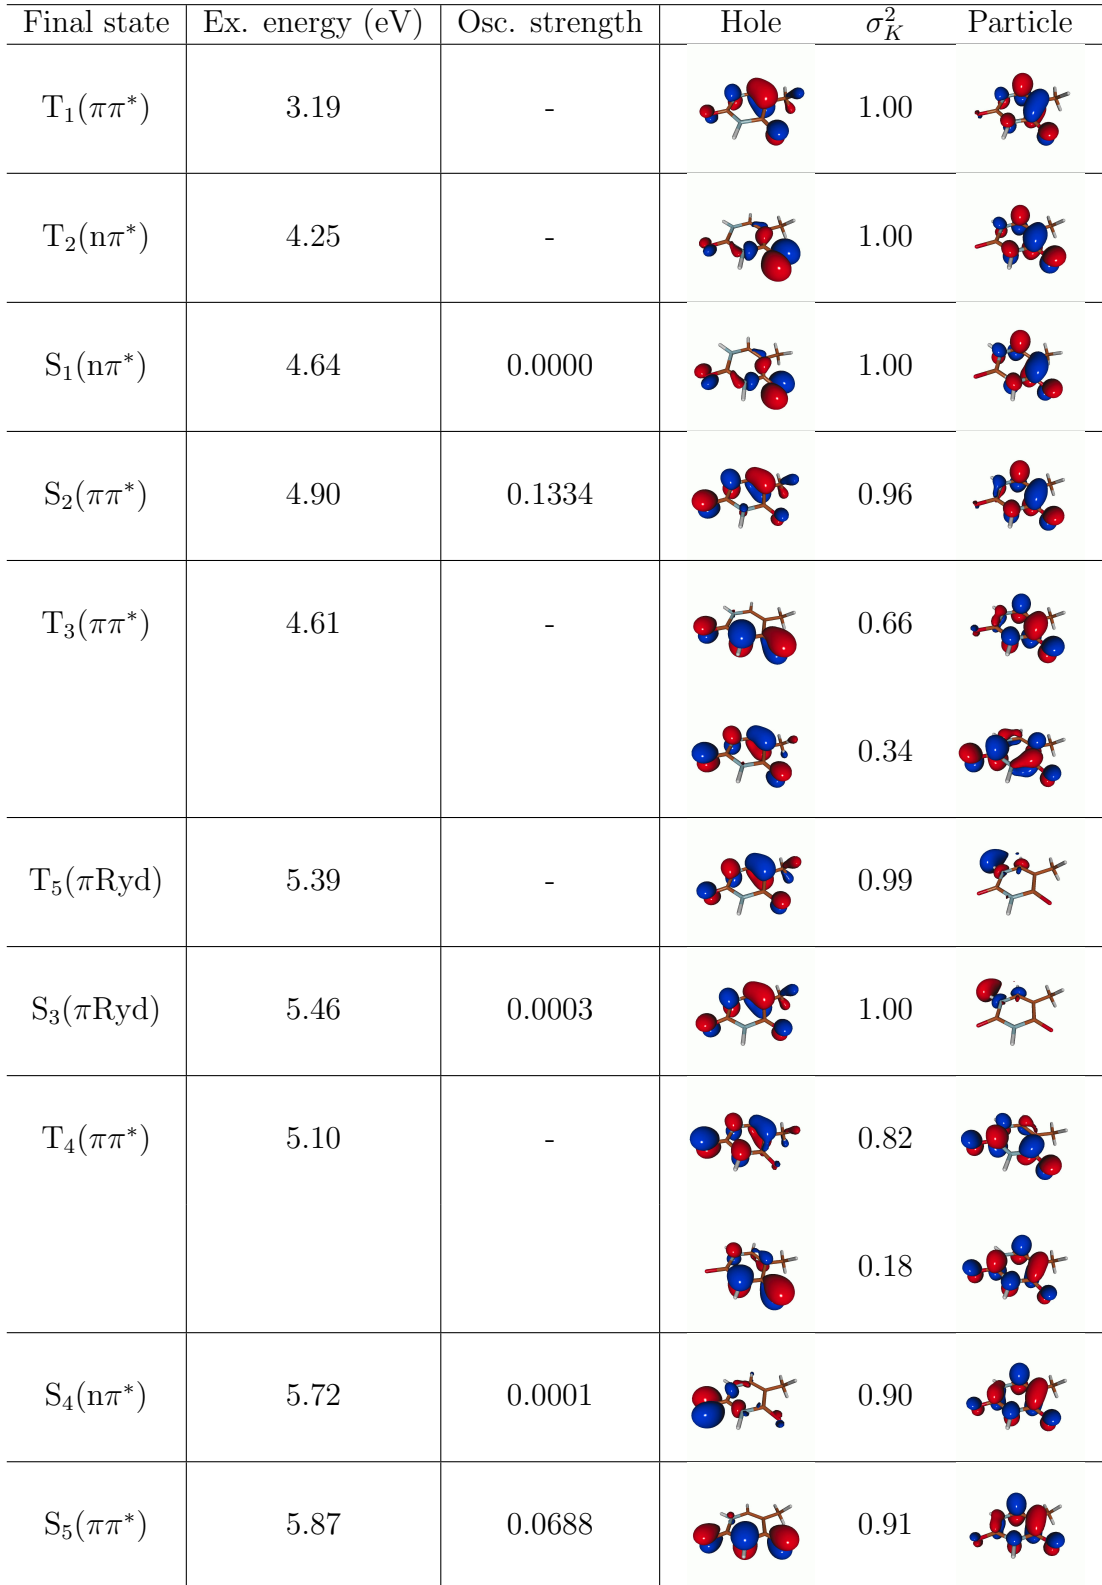 |
| $T_4(\pi\pi^*)$ | 5.10            | -             | 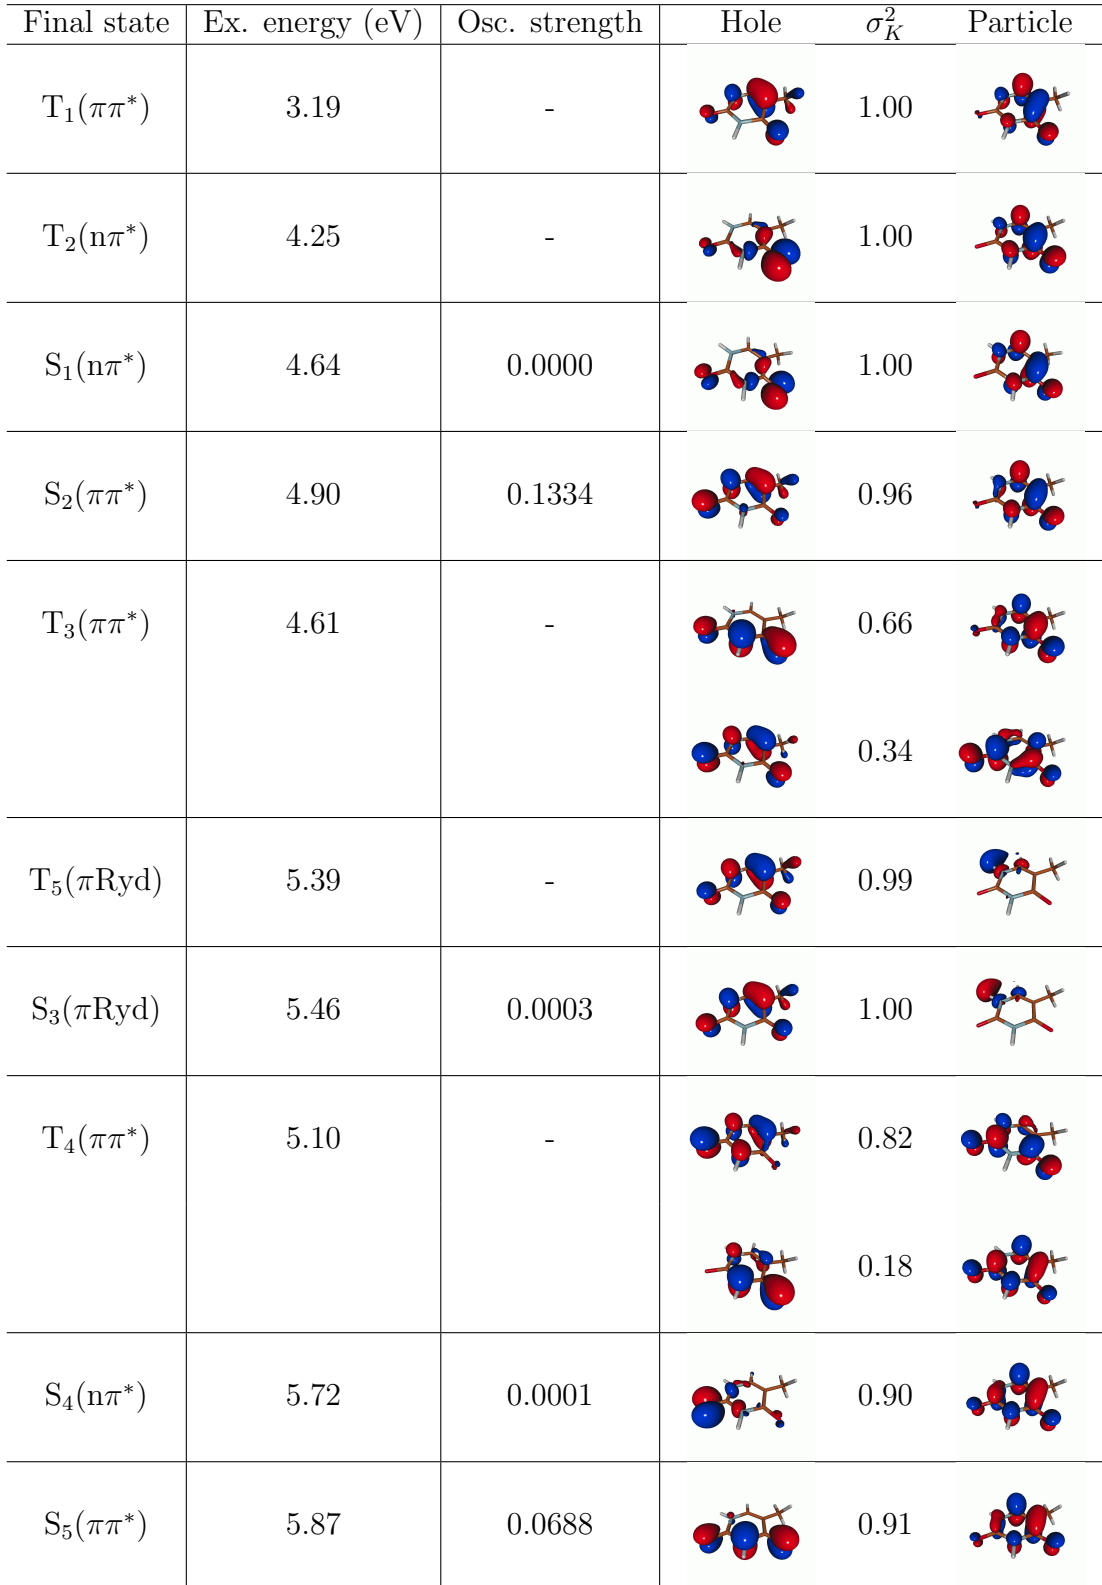 | 0.82         | 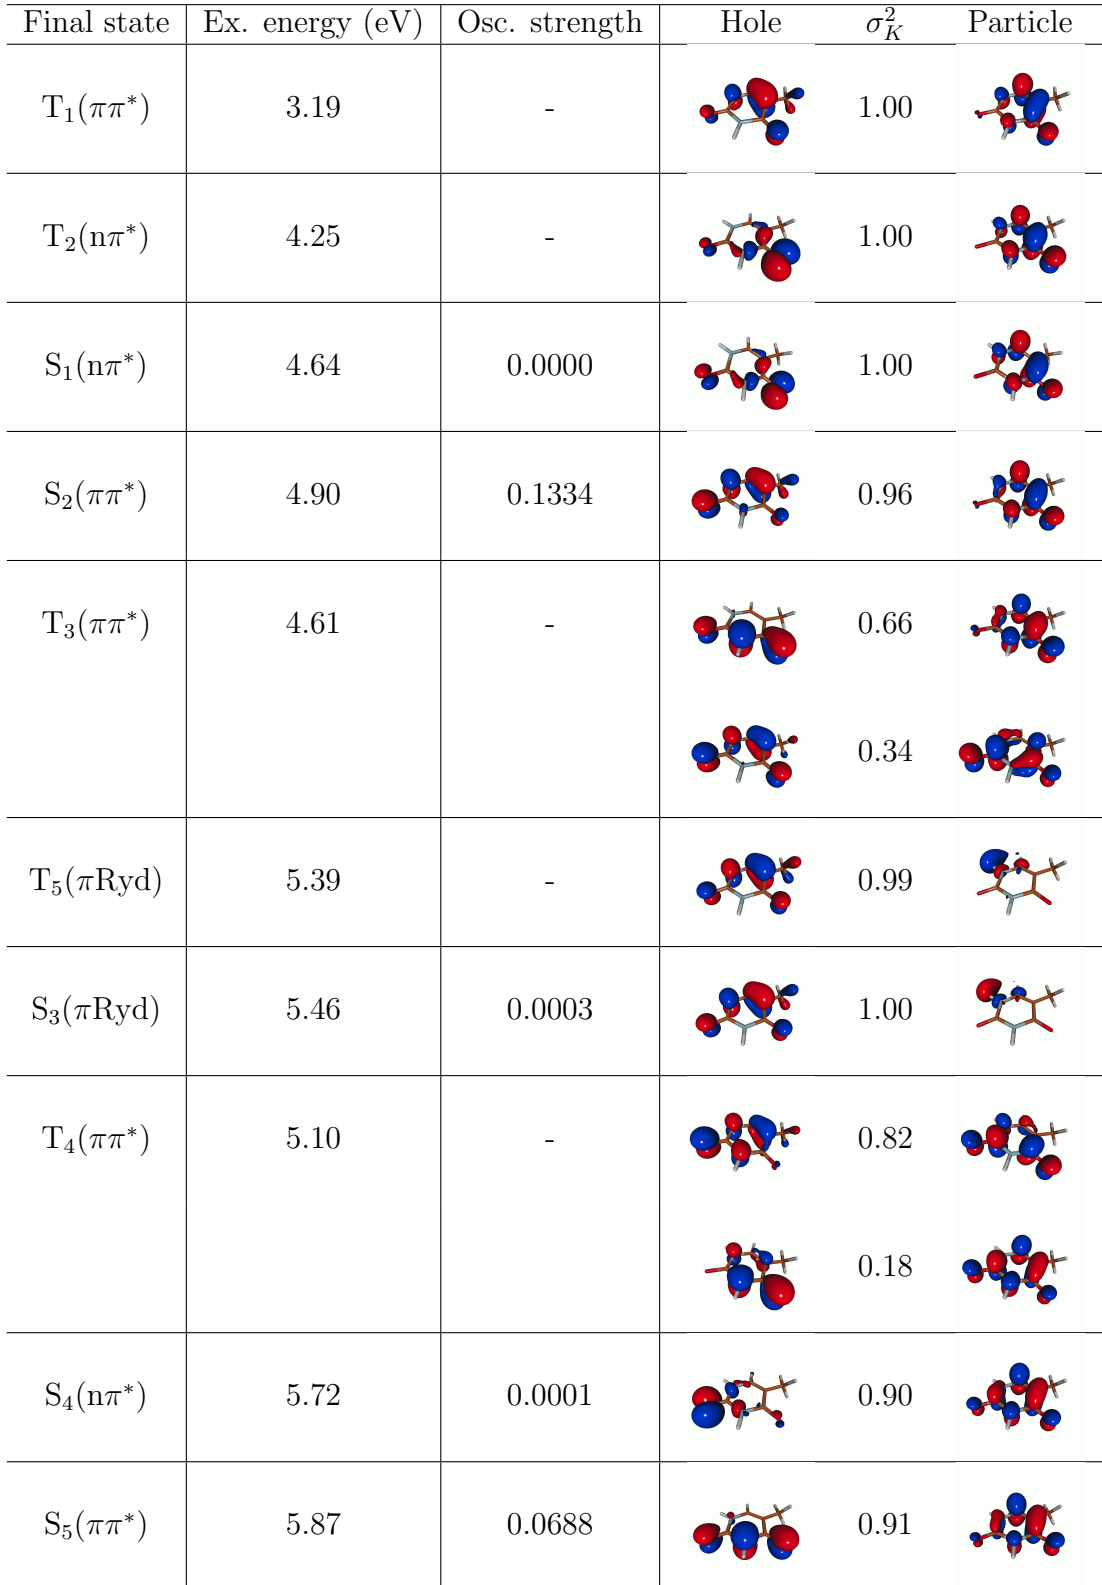 |
|                 |                 |               | 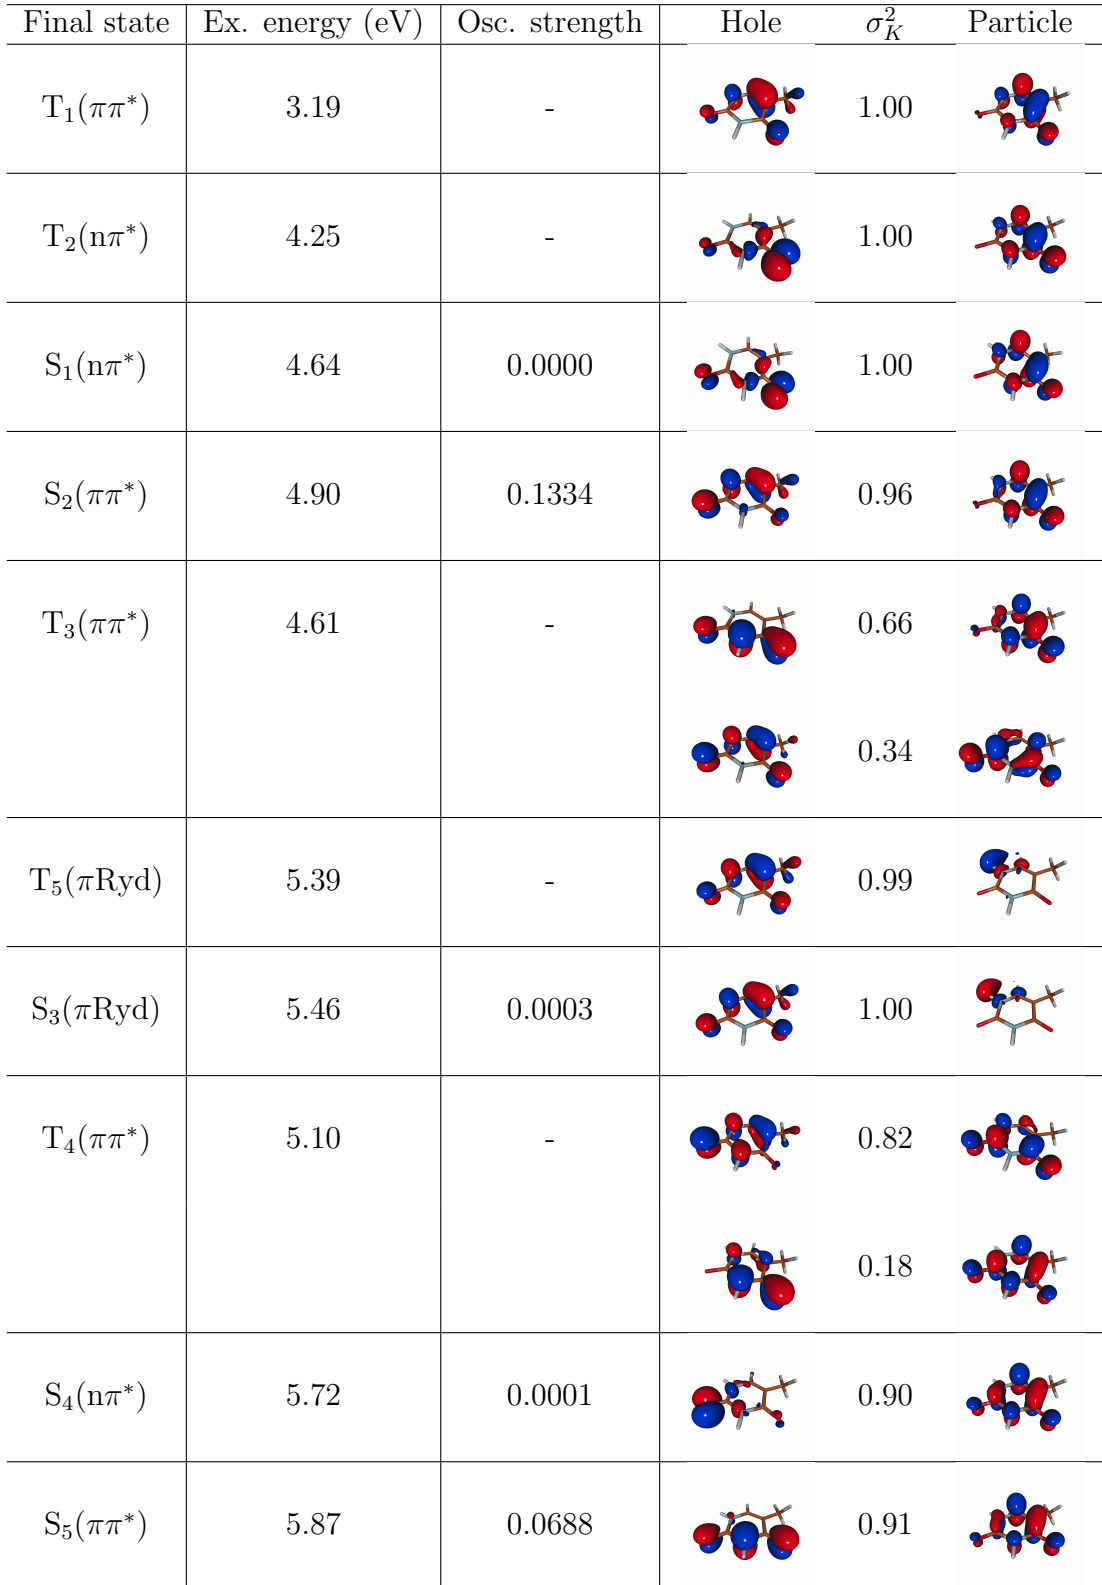 | 0.18         | 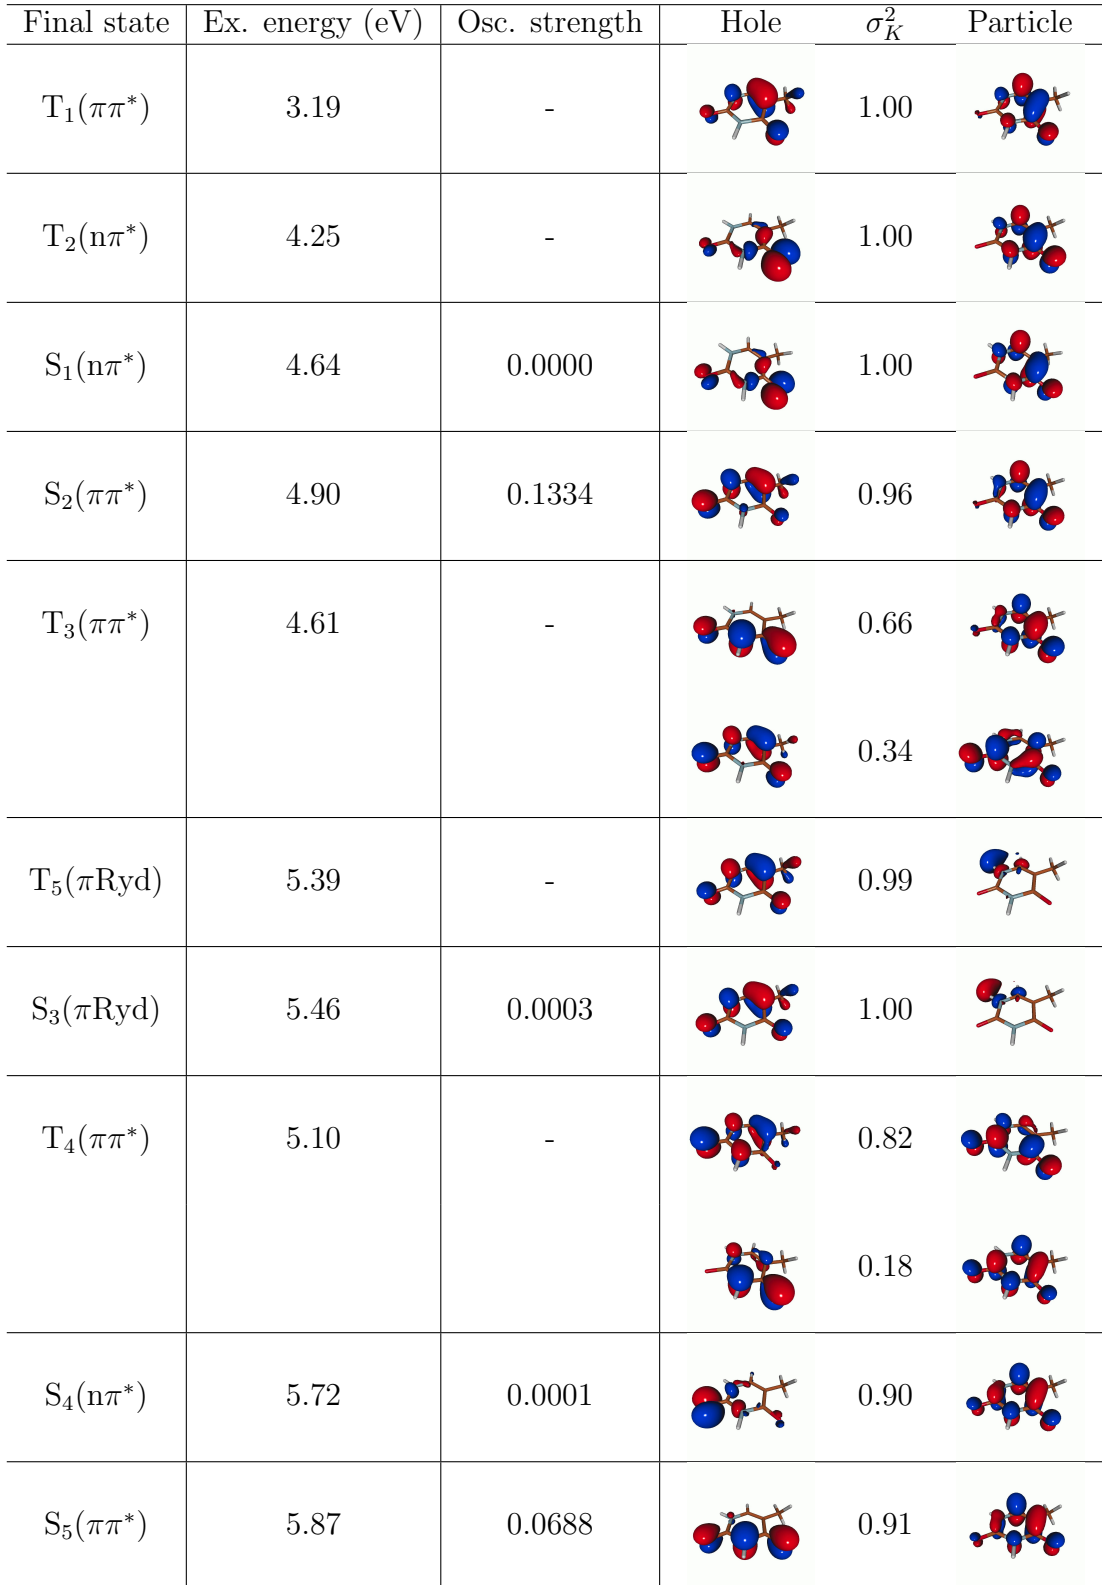 |
| $S_4(n\pi^*)$   | 5.72            | 0.0001        | 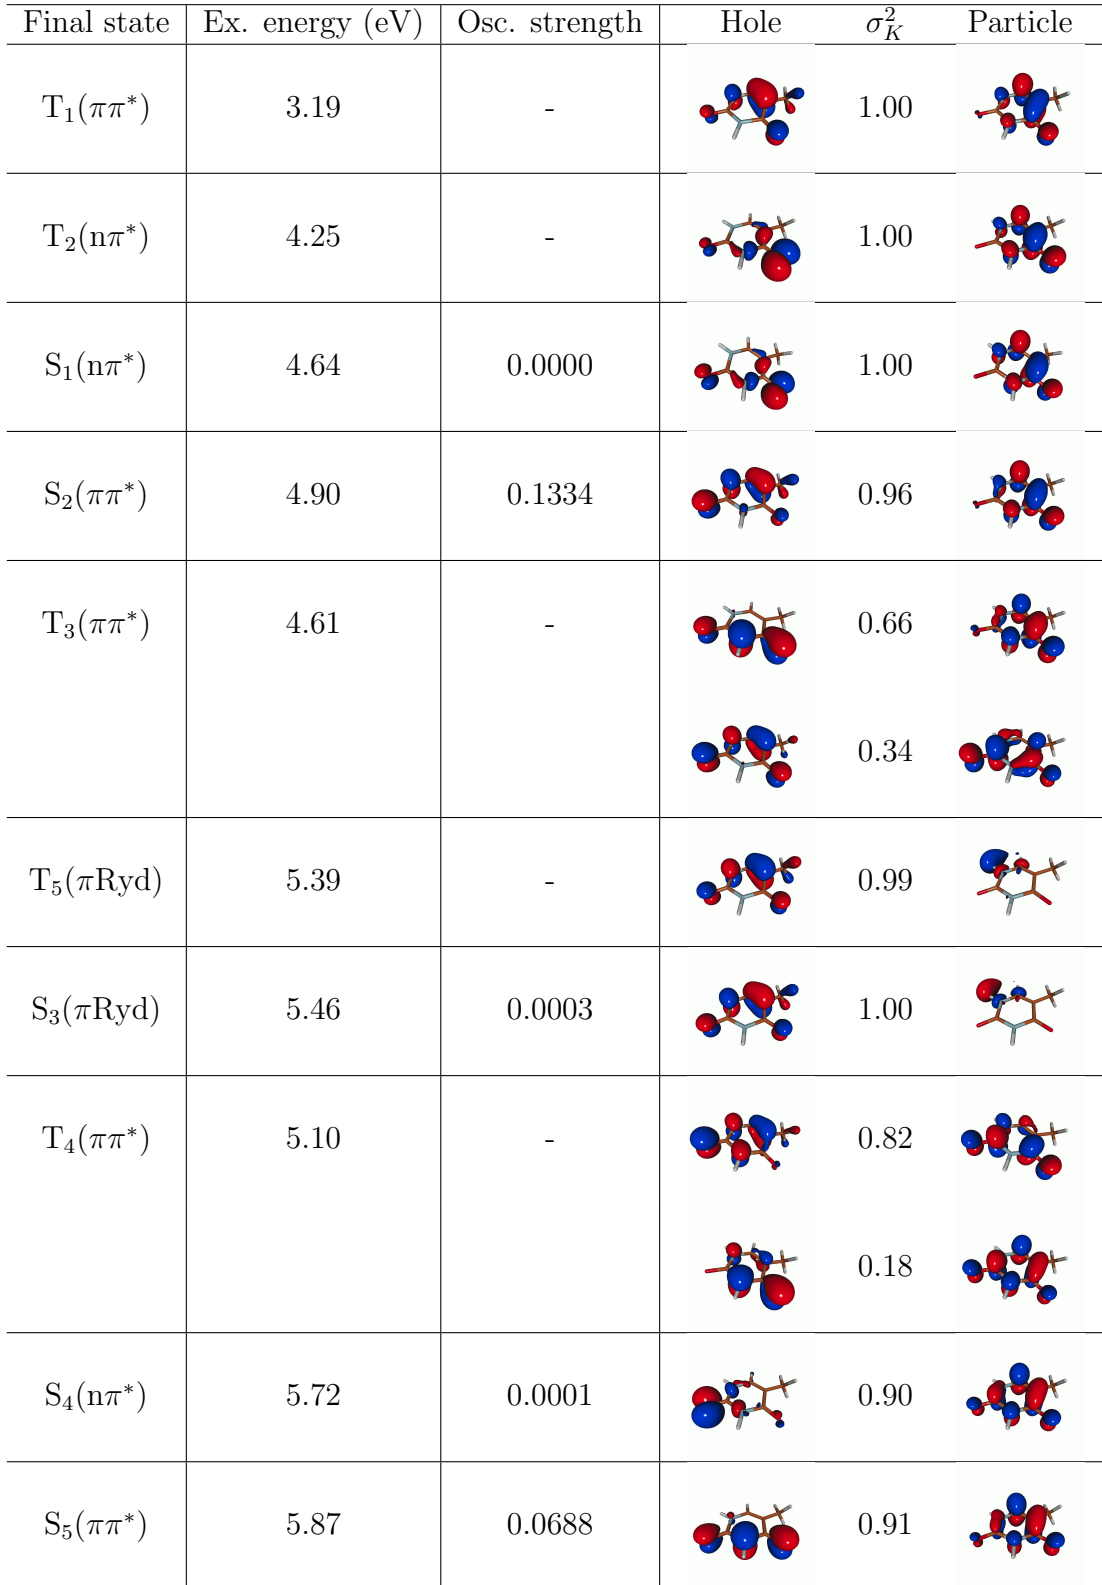 | 0.90         | 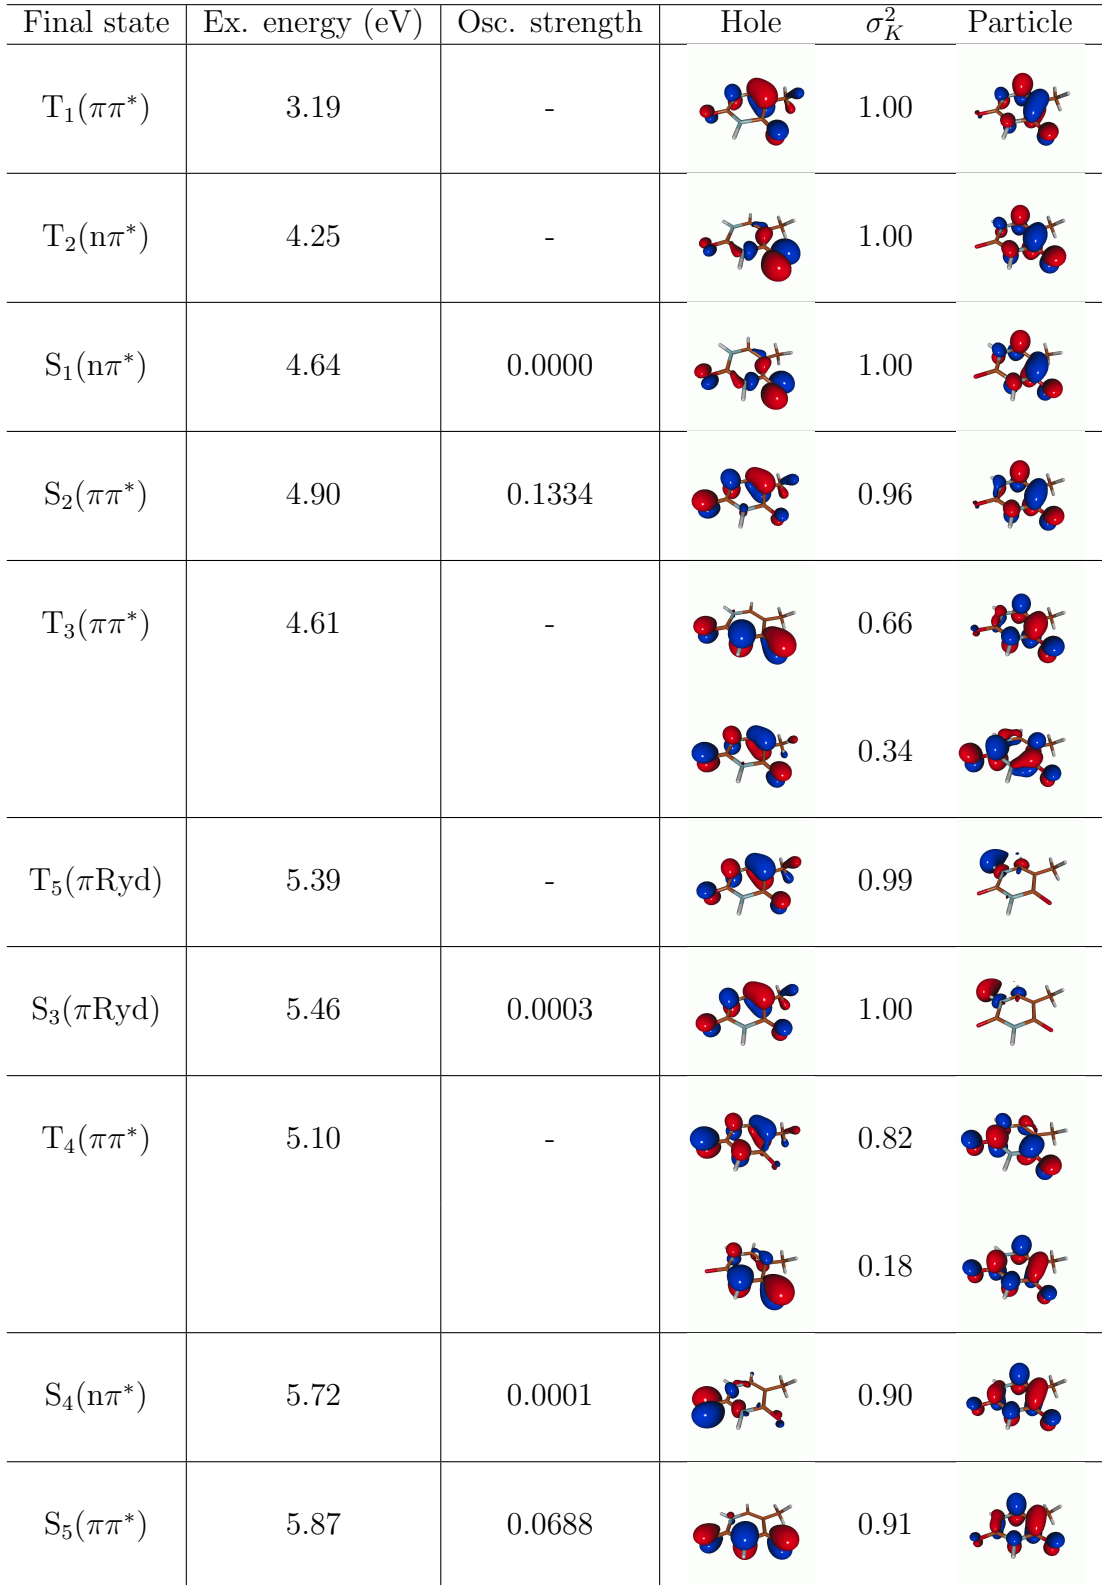 |
| $S_5(\pi\pi^*)$ | 5.87            | 0.0688        | 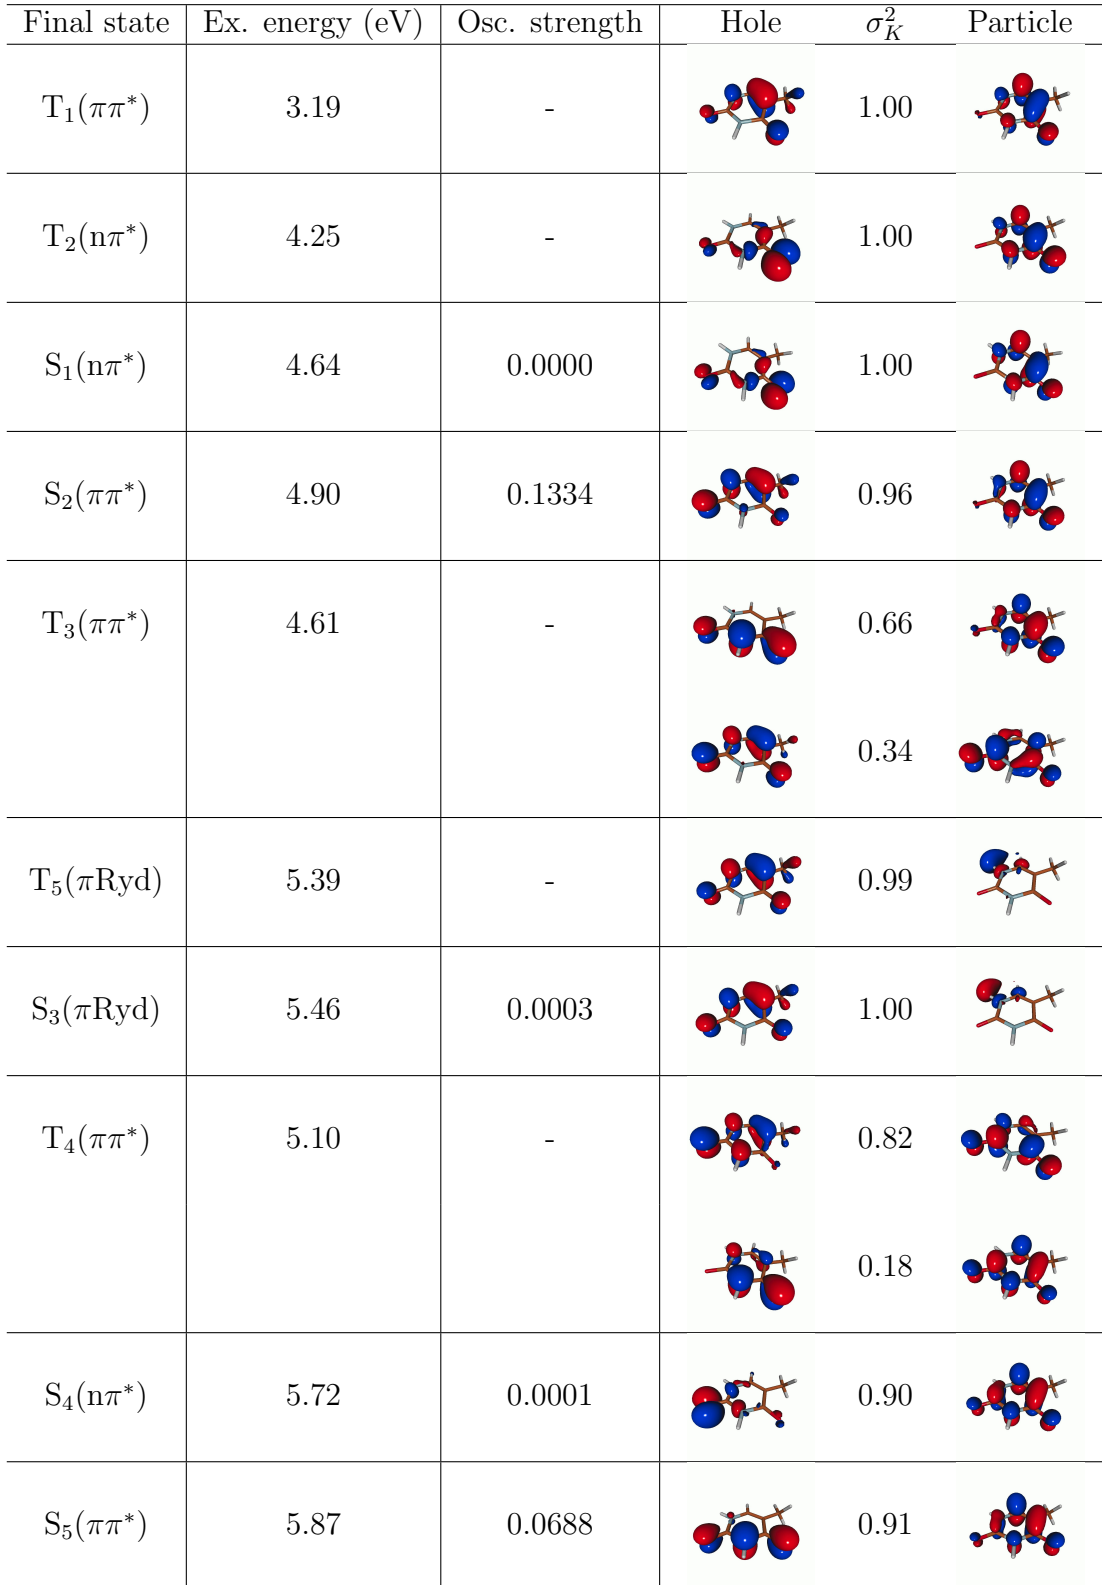 | 0.91         | 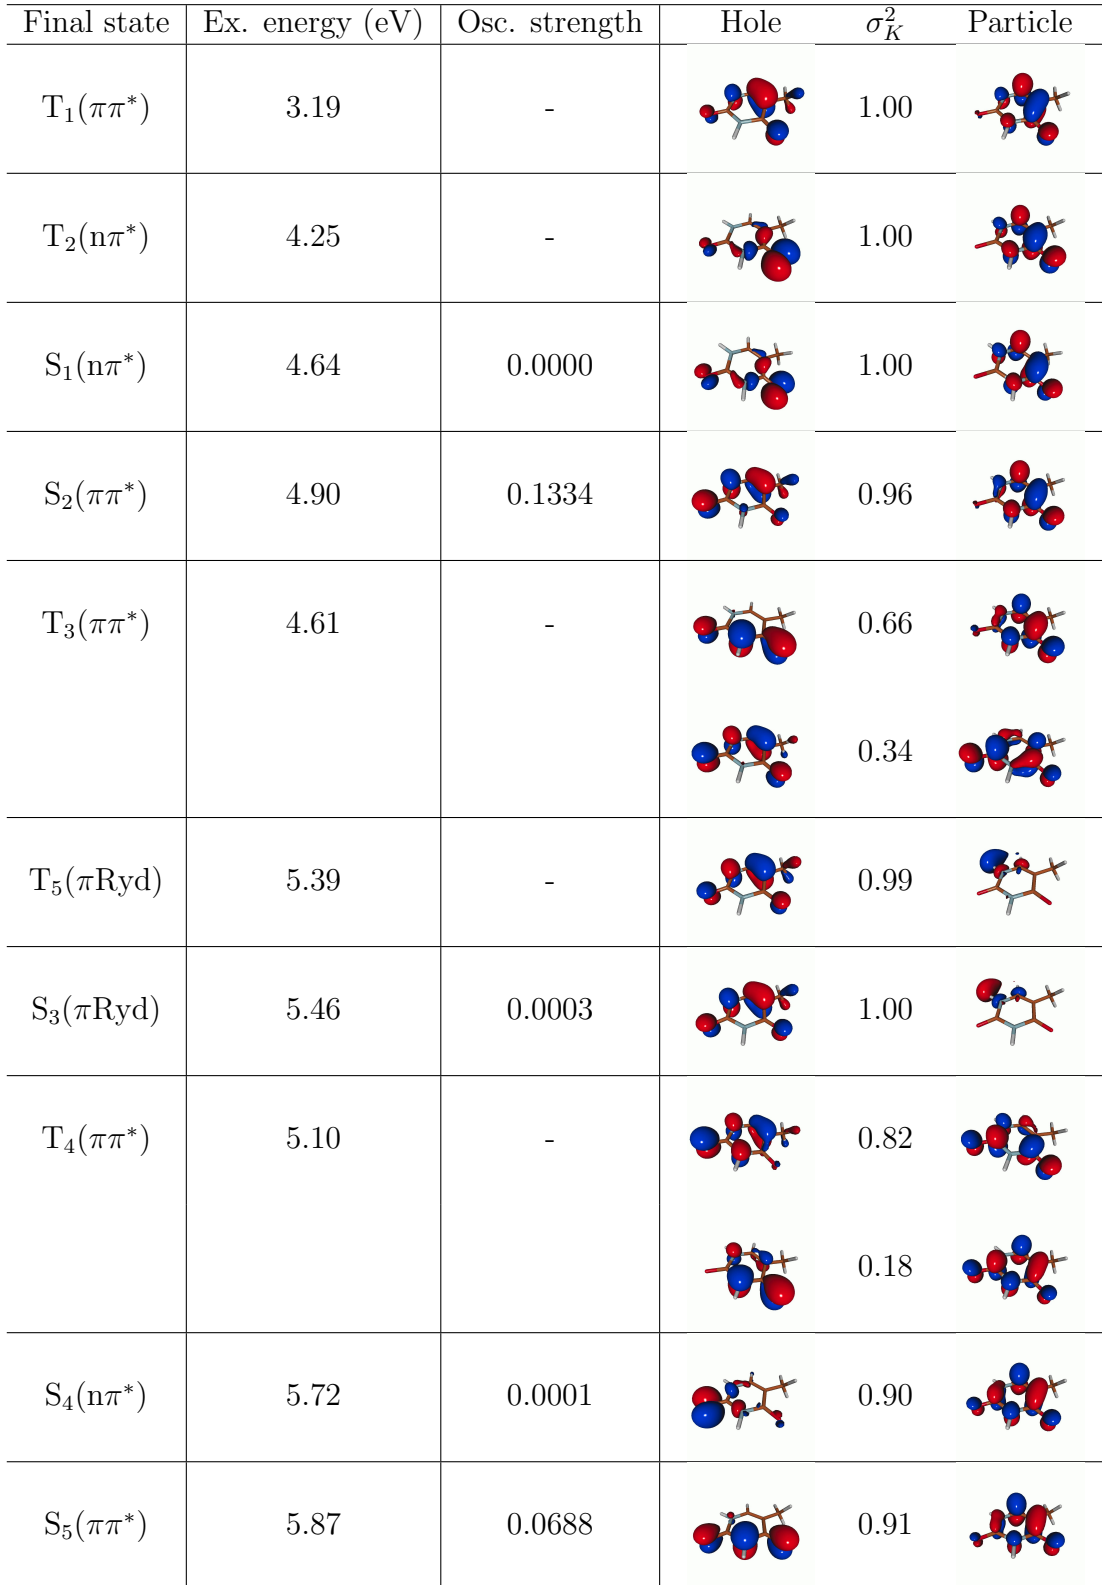 |



Table S16: Acetylacetone. EOM-EE-CCSD/6-311++G\*\* NTOs of the excitations from the ground state to the lowest-lying valence-excited states at the FC geometry (NTO isosurface is 0.03 for the Rydberg transitions and 0.05 for the others).

| Final state            | Ex. energy (eV) | Osc. strength | Hole                                                                                 | $\sigma_K^2$ | Particle                                                                              |
|------------------------|-----------------|---------------|--------------------------------------------------------------------------------------|--------------|---------------------------------------------------------------------------------------|
| $T_1(A', \pi\pi^*)$    | 3.69            | -             | 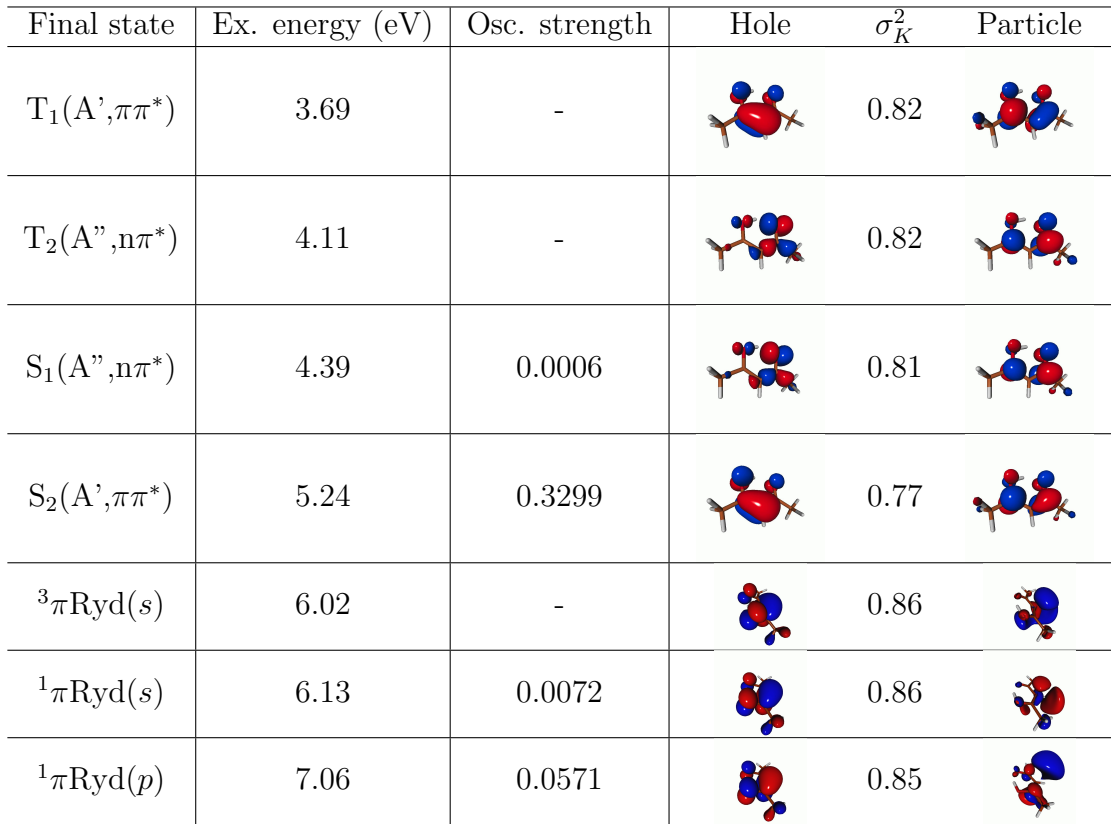   | 0.82         | 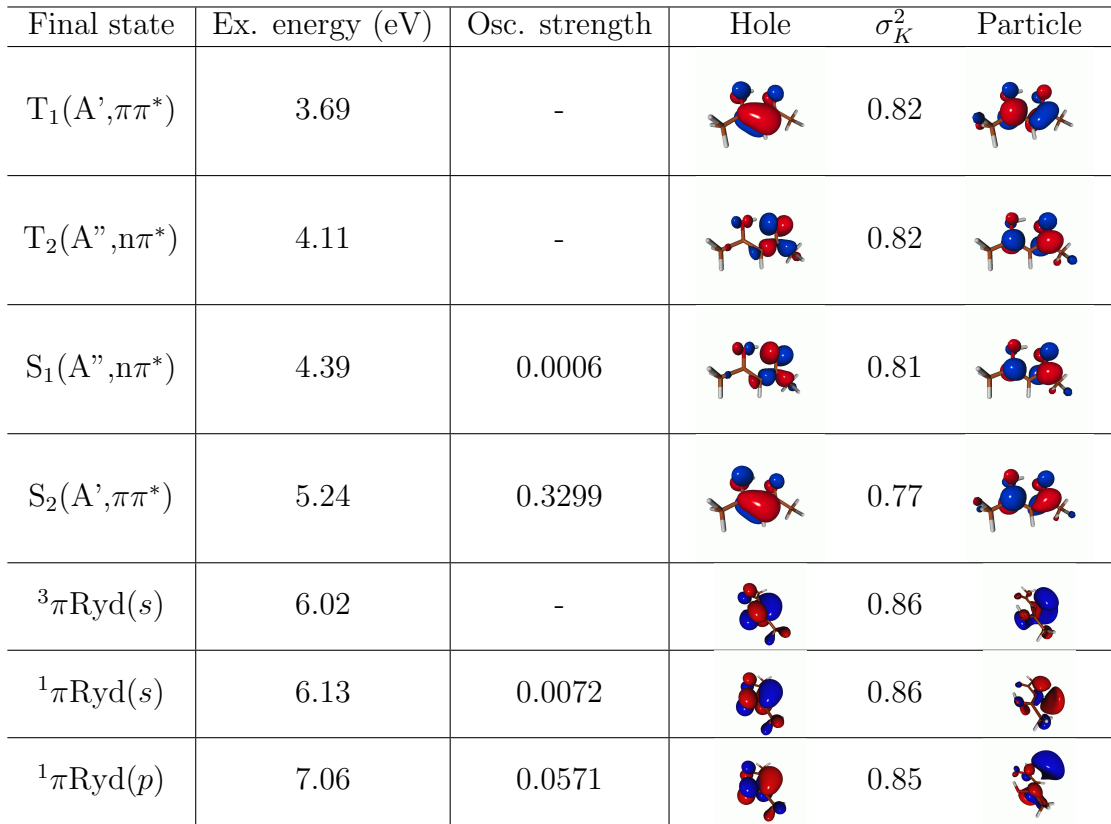   |
| $T_2(A'', n\pi^*)$     | 4.11            | -             | 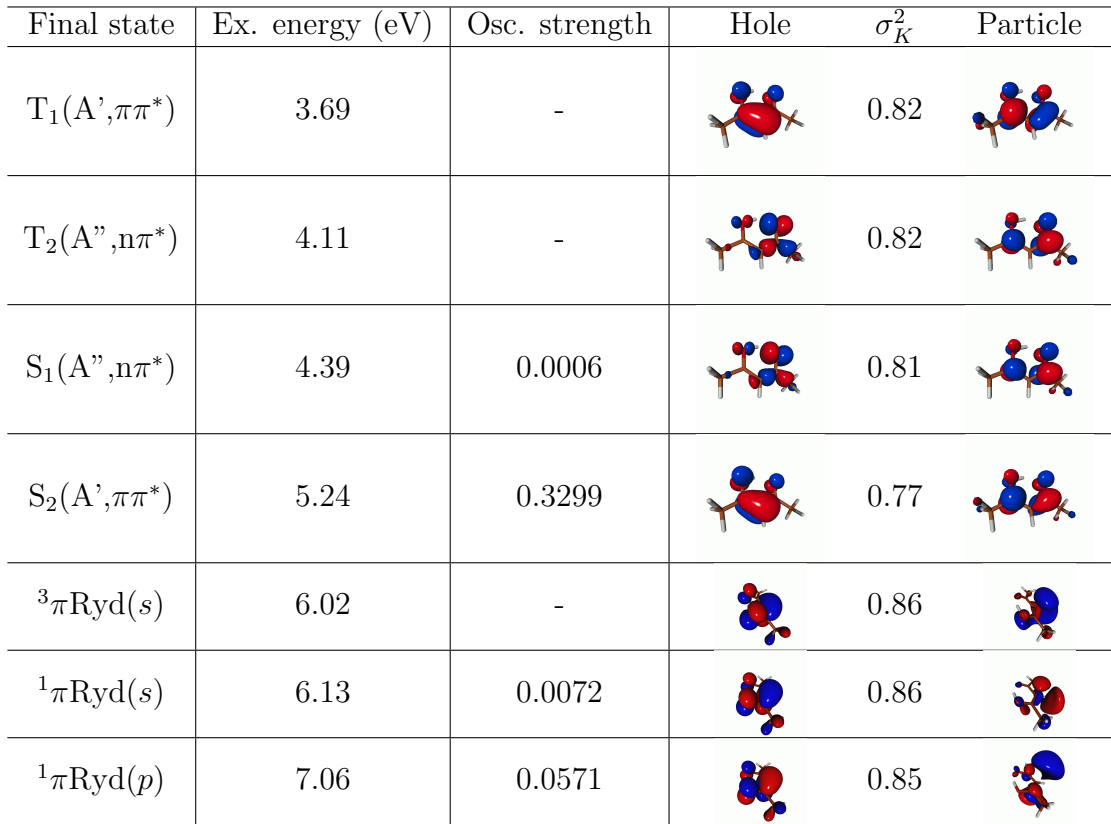   | 0.82         | 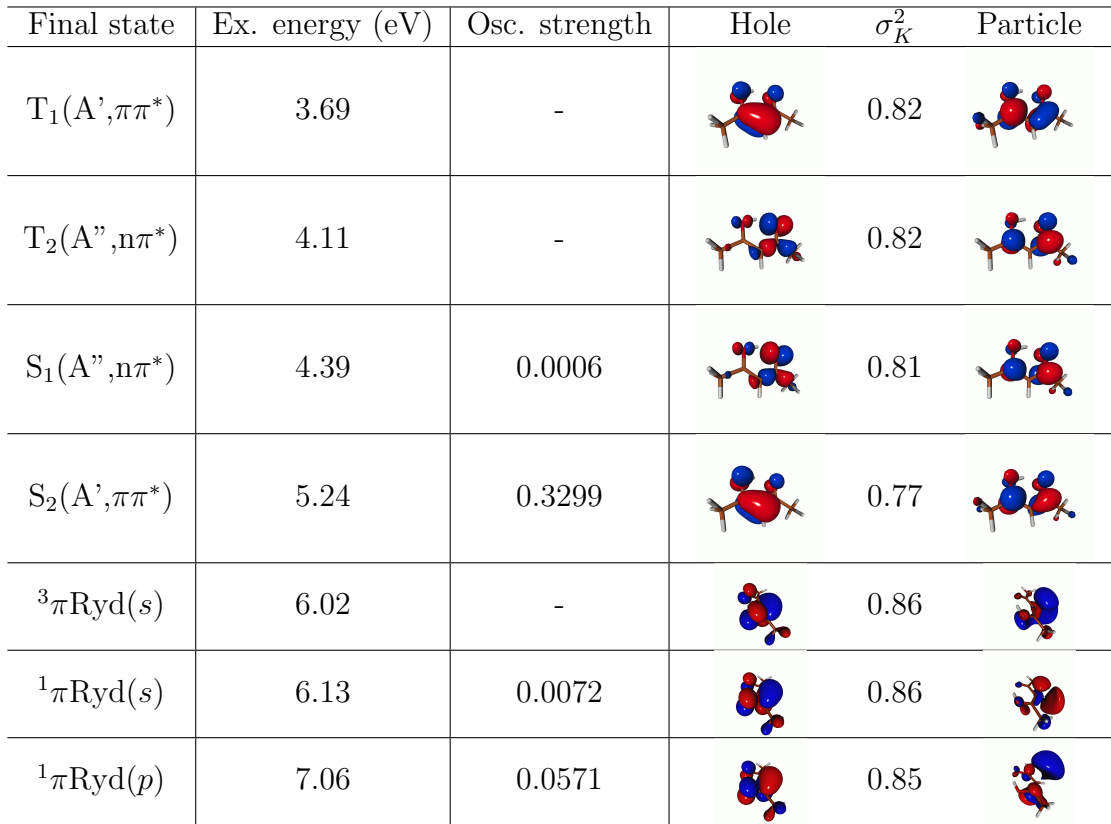   |
| $S_1(A'', n\pi^*)$     | 4.39            | 0.0006        | 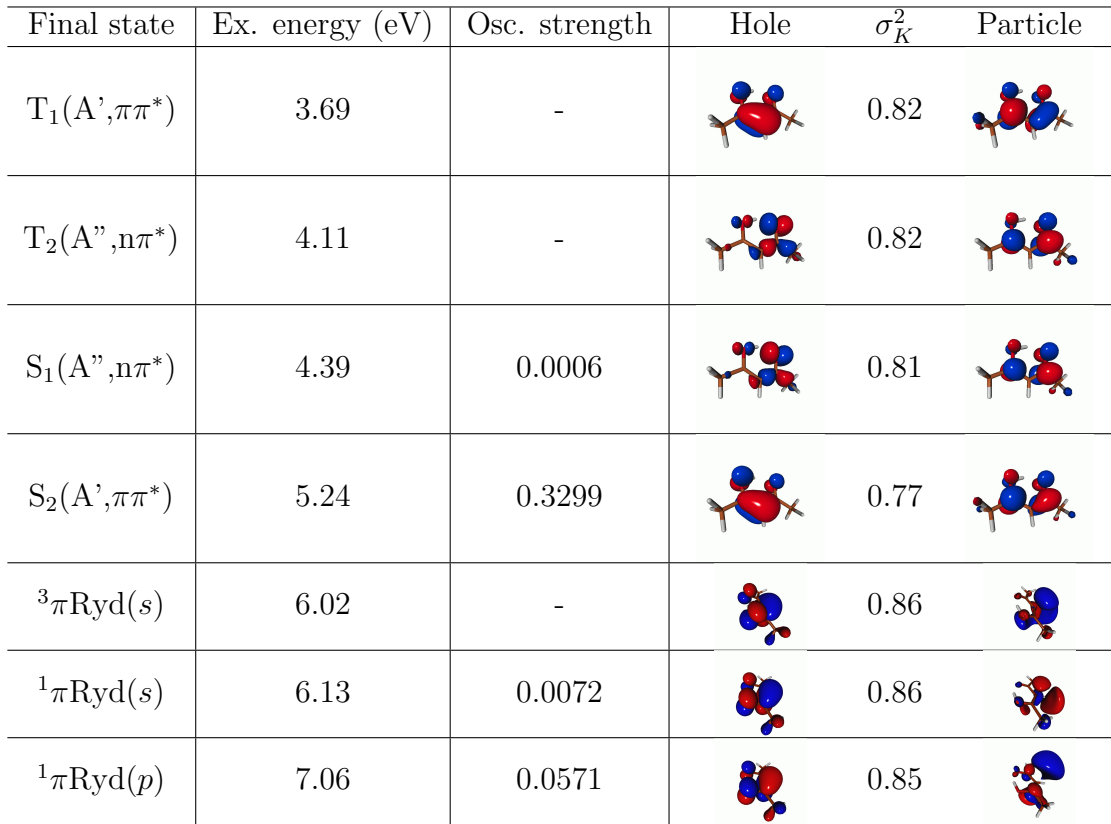 | 0.81         | 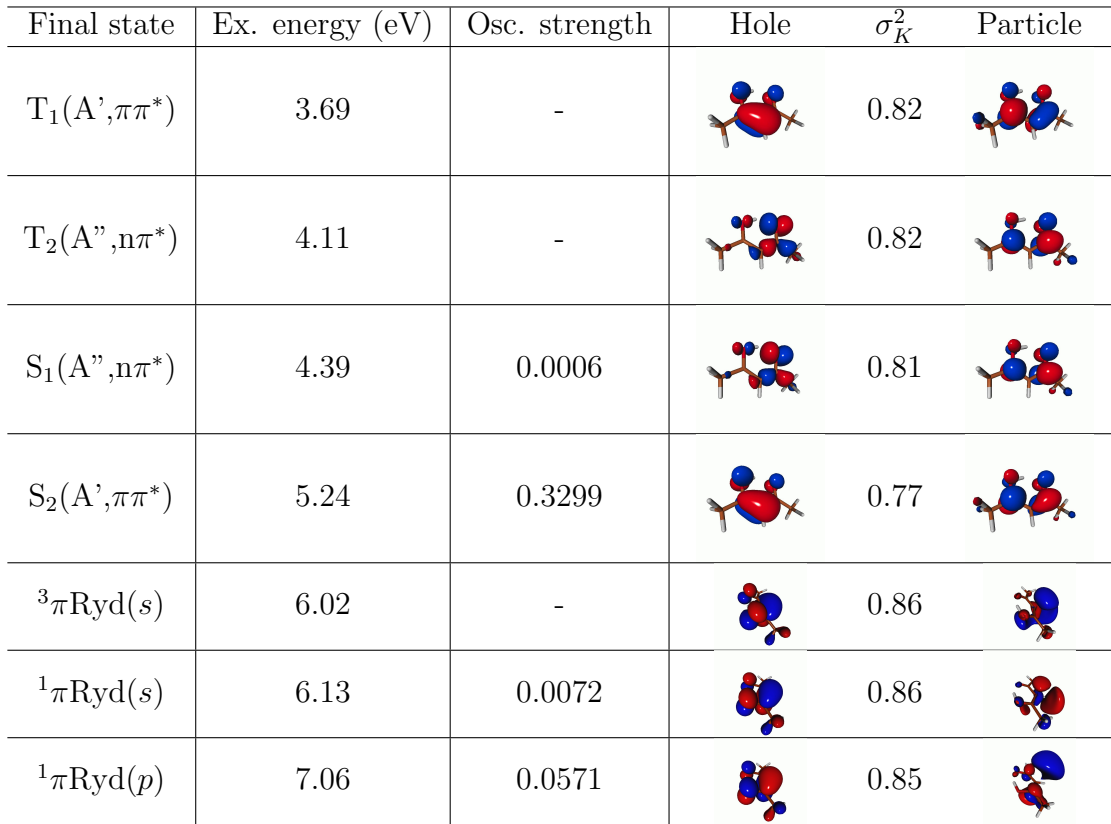 |
| $S_2(A', \pi\pi^*)$    | 5.24            | 0.3299        | 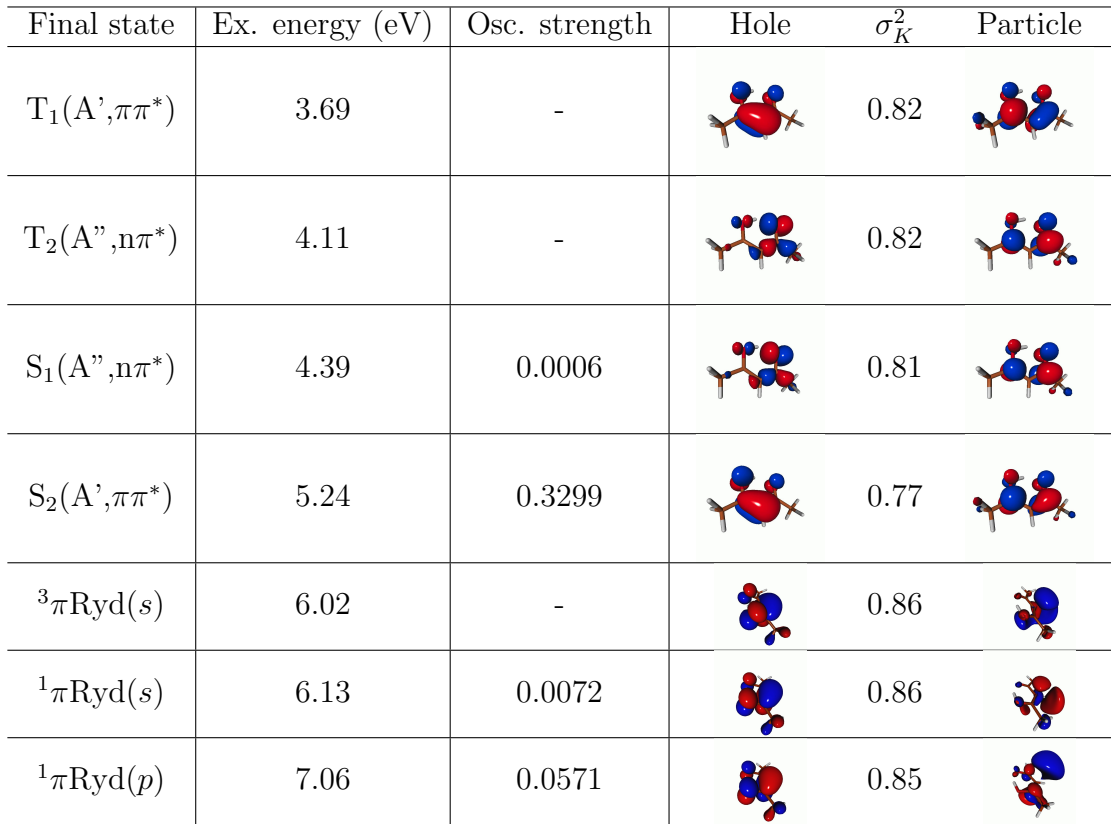 | 0.77         | 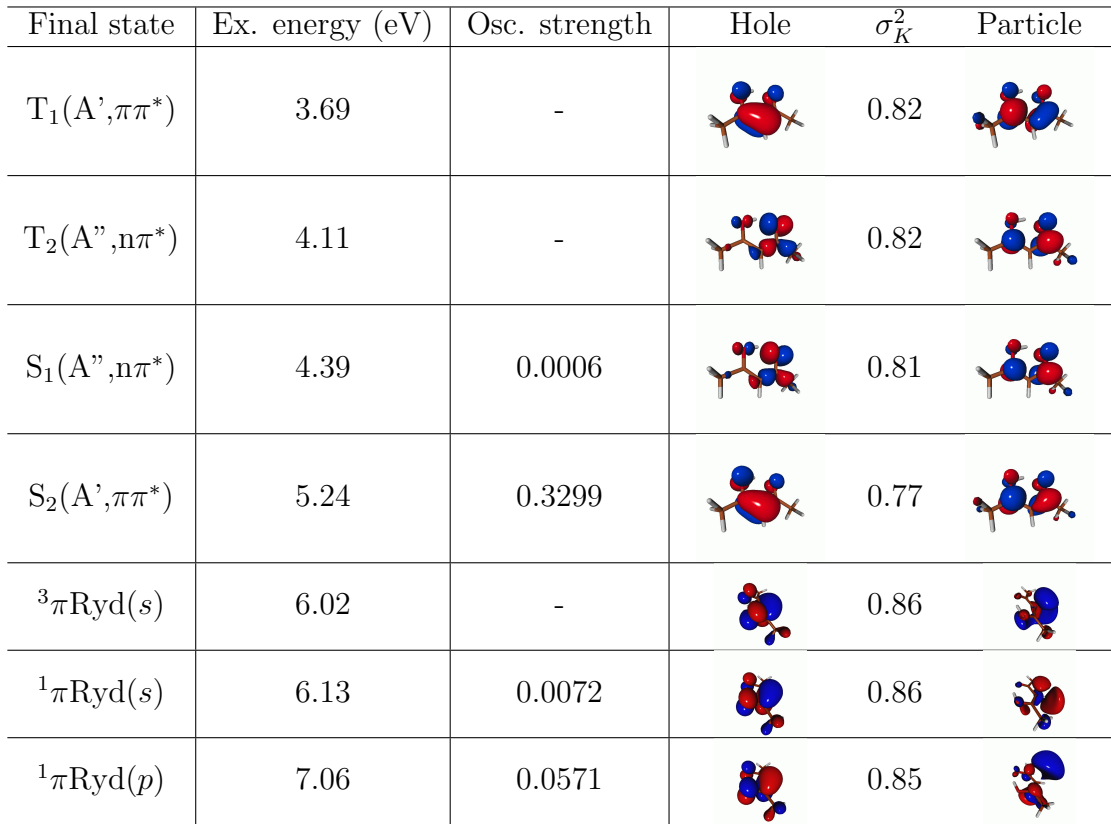 |
| ${}^3\pi\text{Ryd}(s)$ | 6.02            | -             | 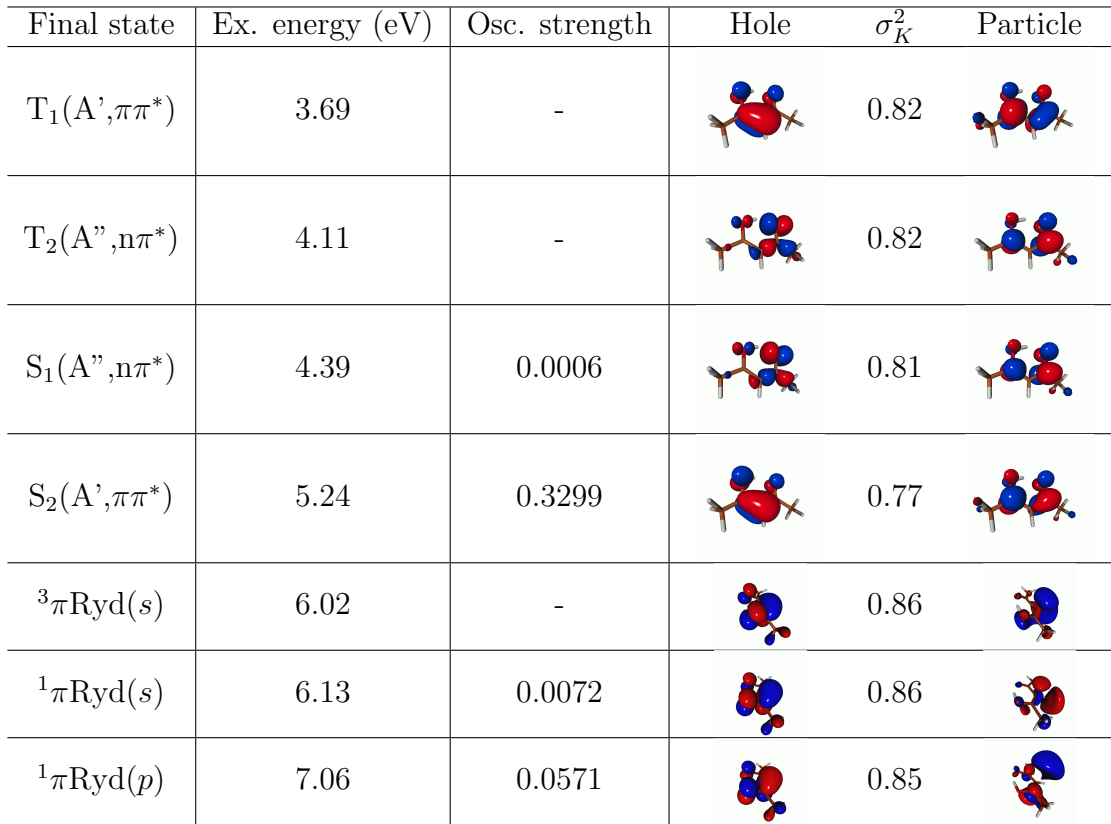 | 0.86         | 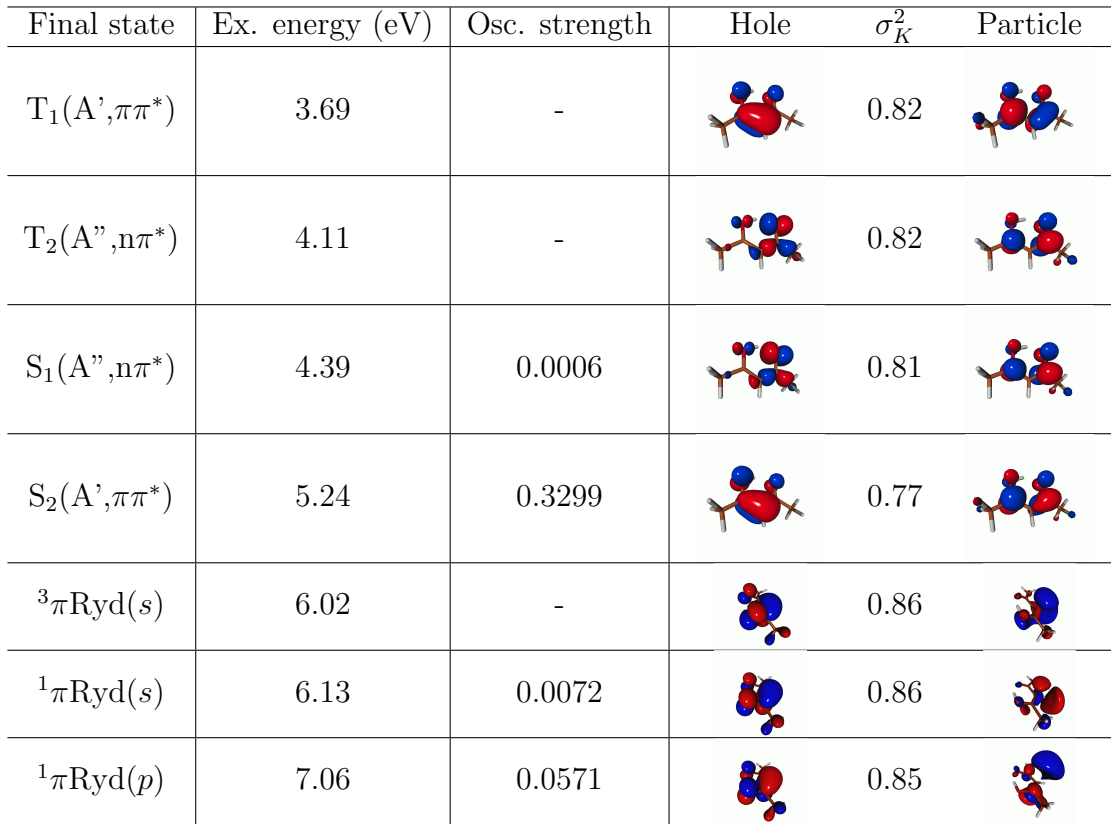 |
| ${}^1\pi\text{Ryd}(s)$ | 6.13            | 0.0072        | 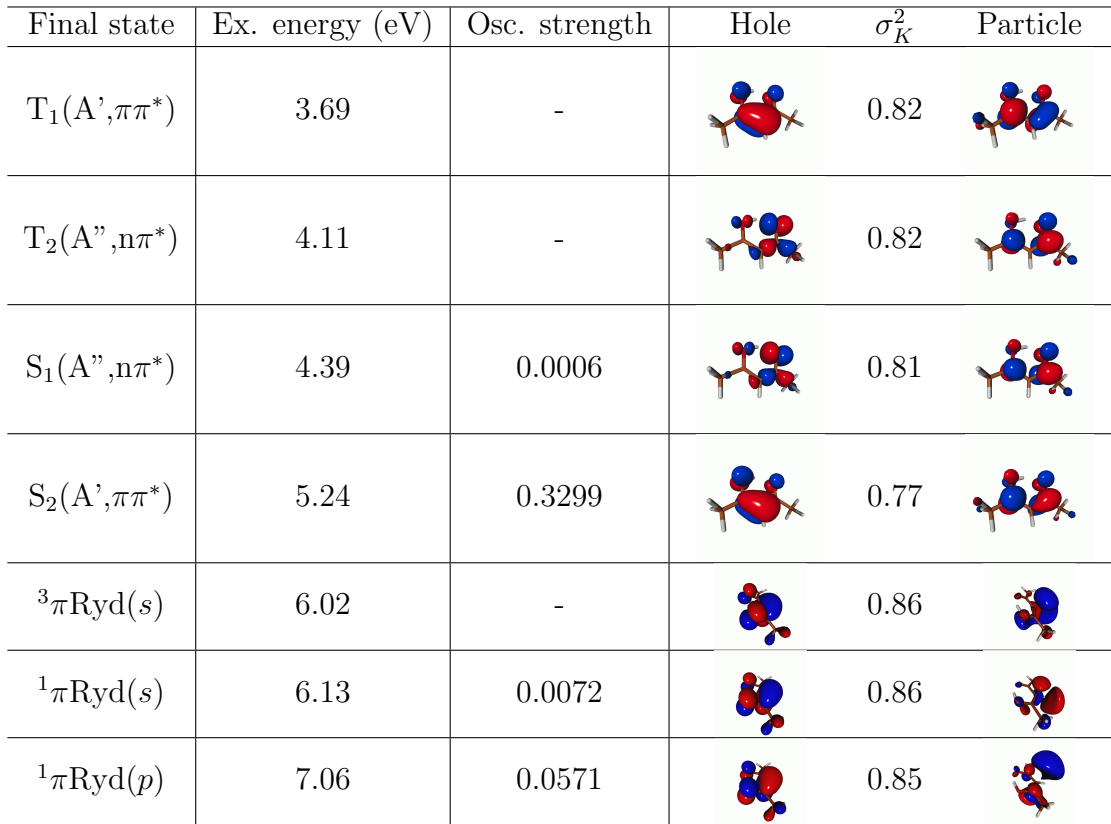 | 0.86         | 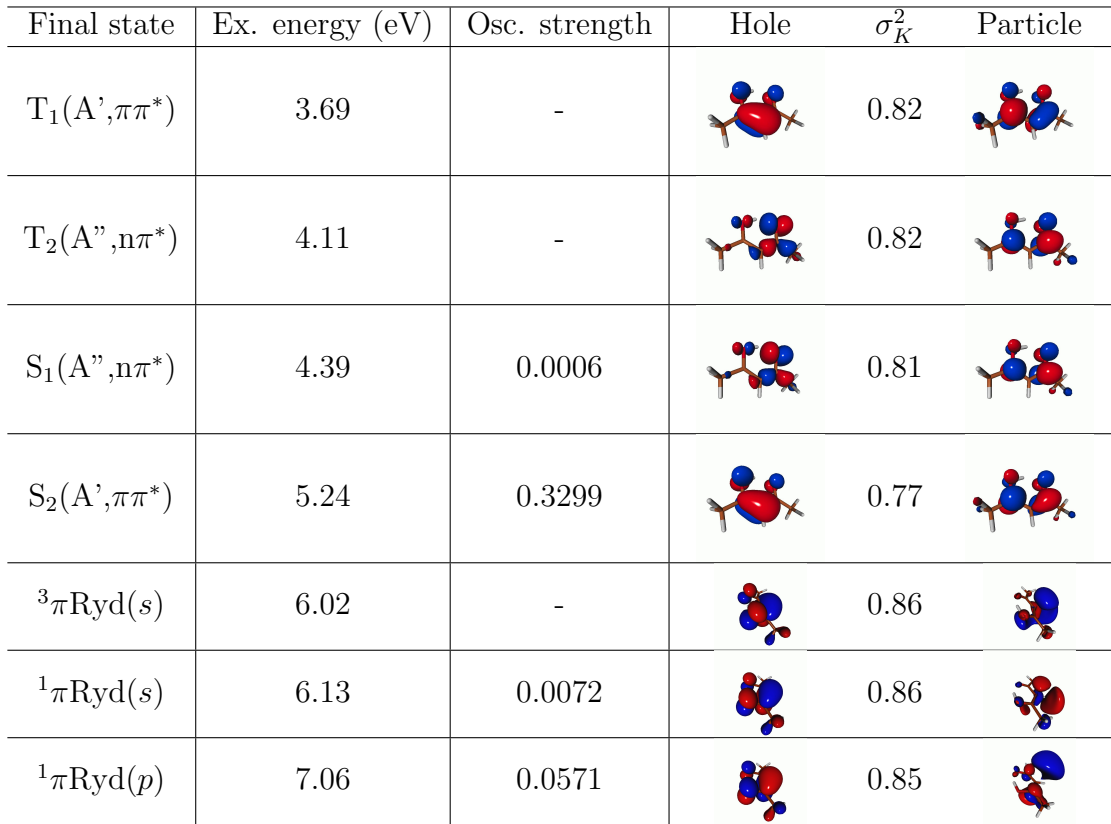 |
| ${}^1\pi\text{Ryd}(p)$ | 7.06            | 0.0571        | 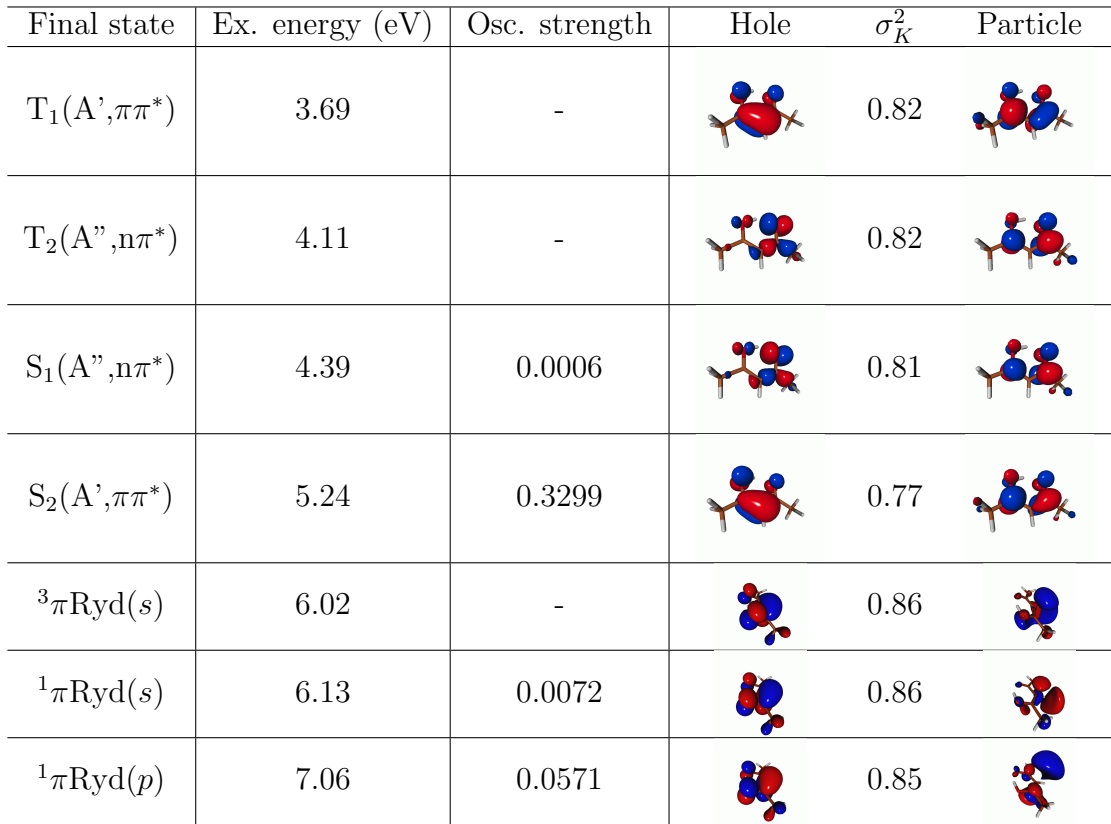 | 0.85         | 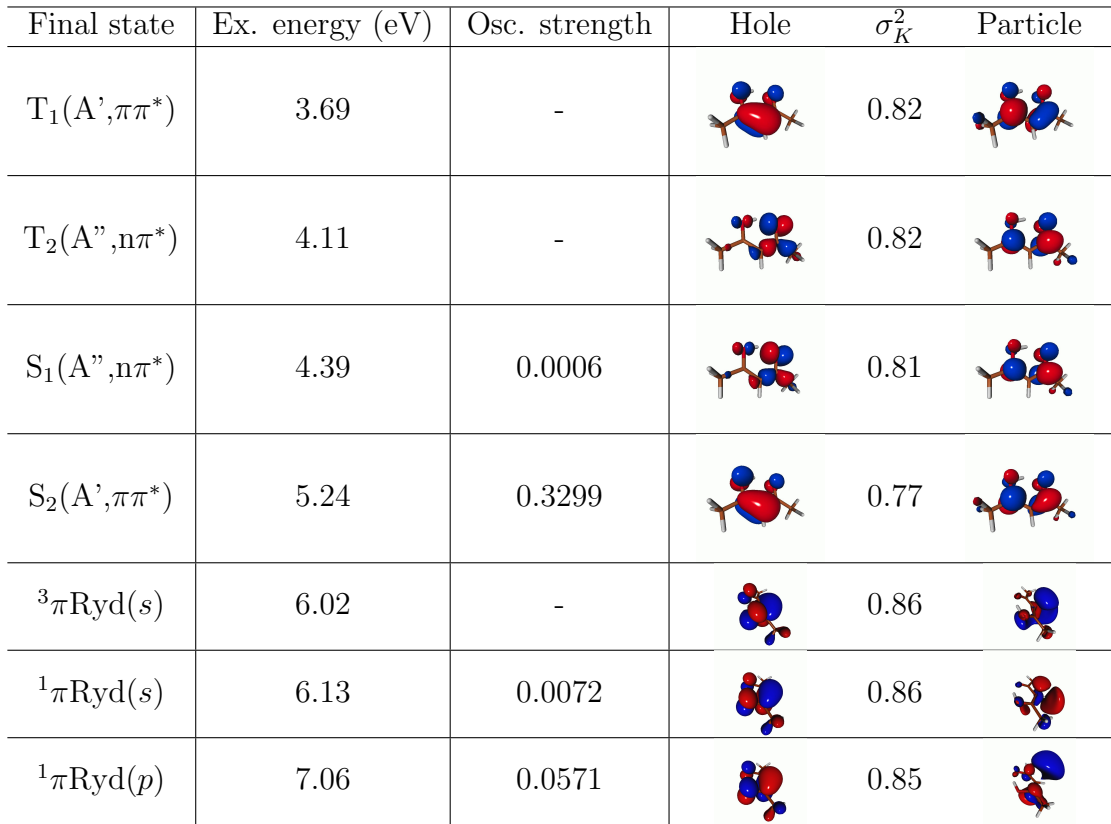 |

Table S17: Acetylacetone. ADC(2)/6-311++G\*\* NTOs of the excitations from the ground state to the lowest-lying valence-excited states at the FC geometry (NTO isosurface is 0.03 for the Rydberg transitions and 0.05 for the others).

| Final state            | Ex. energy (eV) | Osc. strength | Hole                                                                                 | $\sigma_K^2$ | Particle                                                                              |
|------------------------|-----------------|---------------|--------------------------------------------------------------------------------------|--------------|---------------------------------------------------------------------------------------|
| $T_1(A', \pi\pi^*)$    | 3.76            | -             | 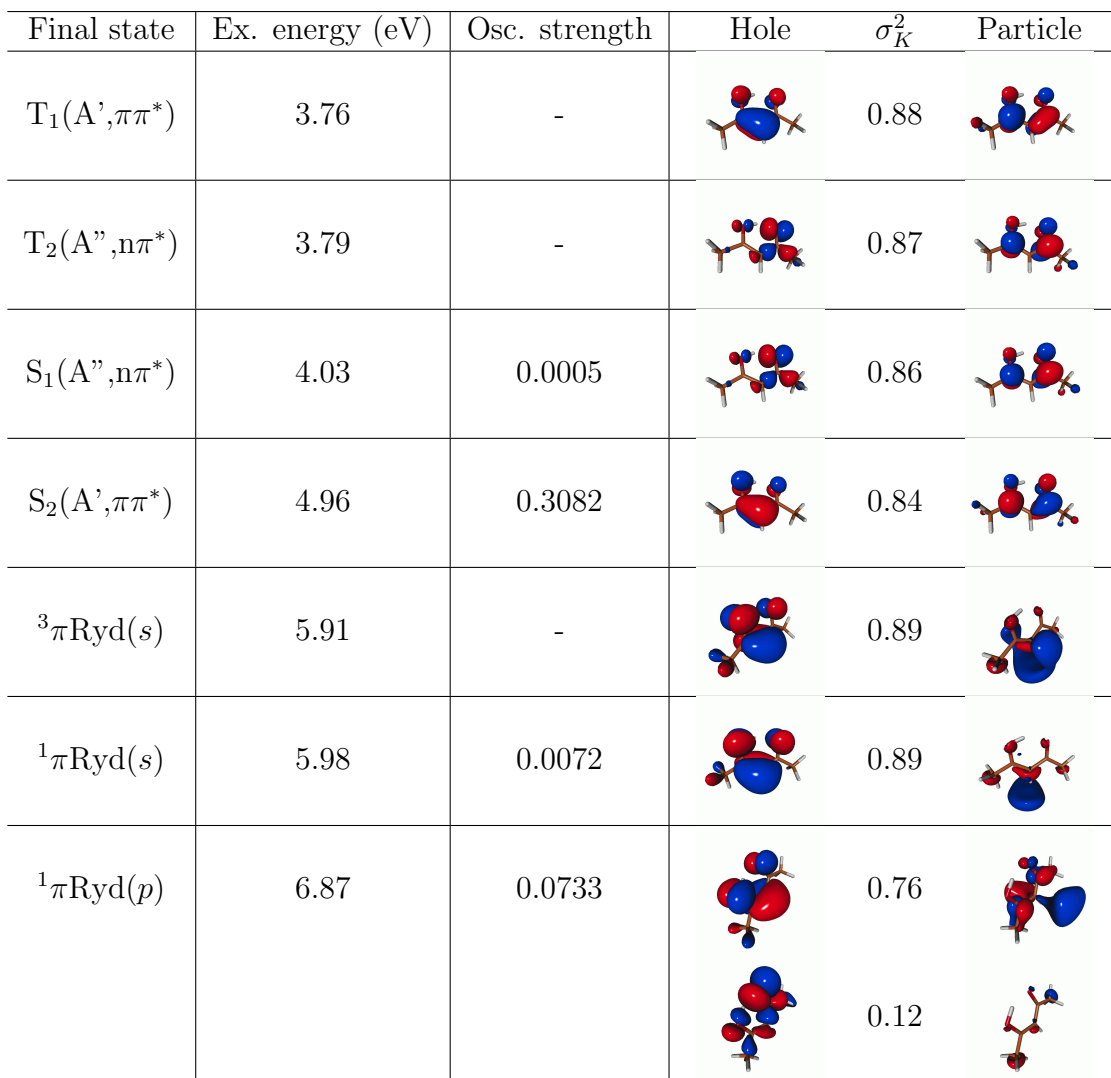   | 0.88         | 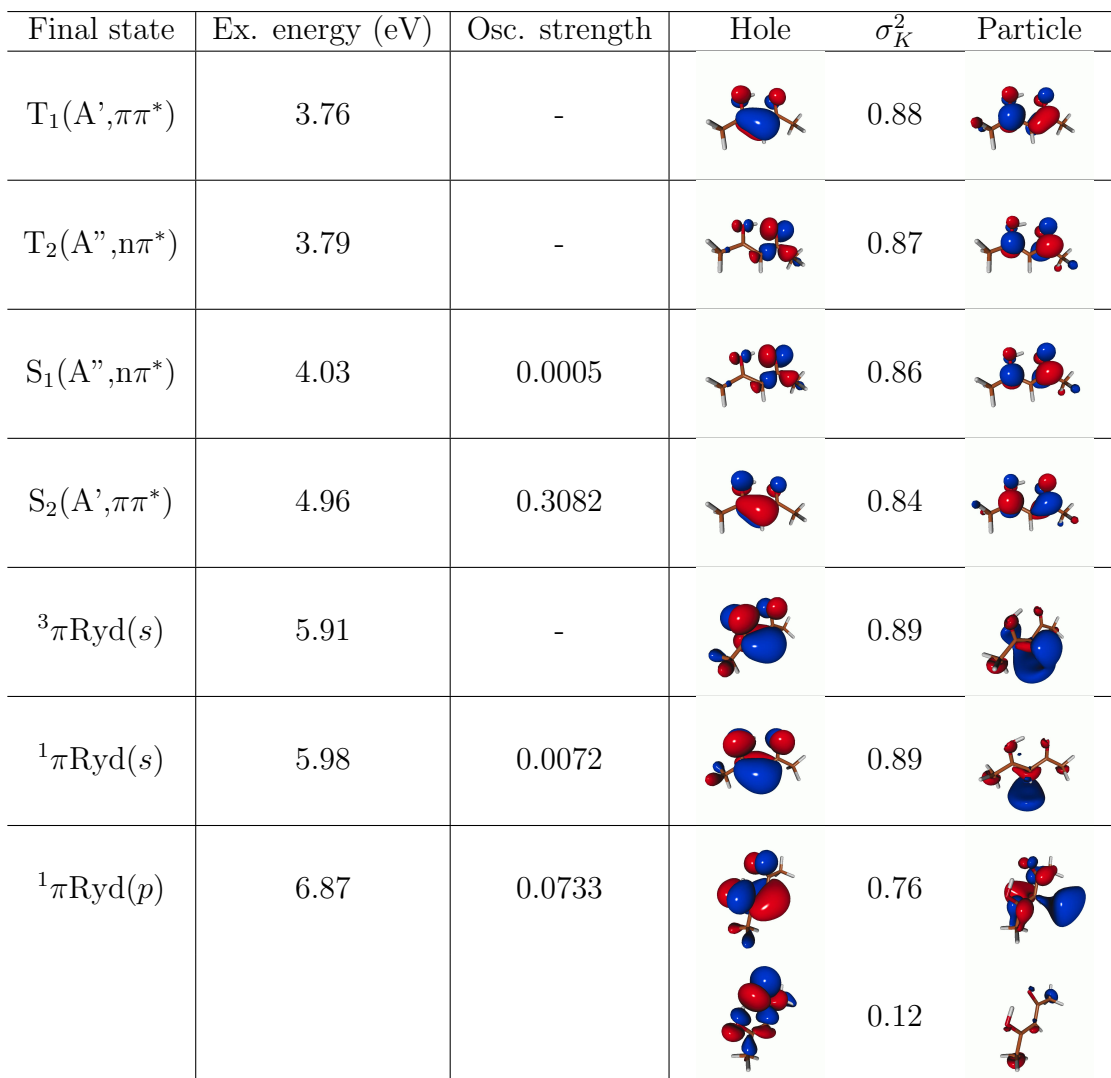   |
| $T_2(A'', n\pi^*)$     | 3.79            | -             | 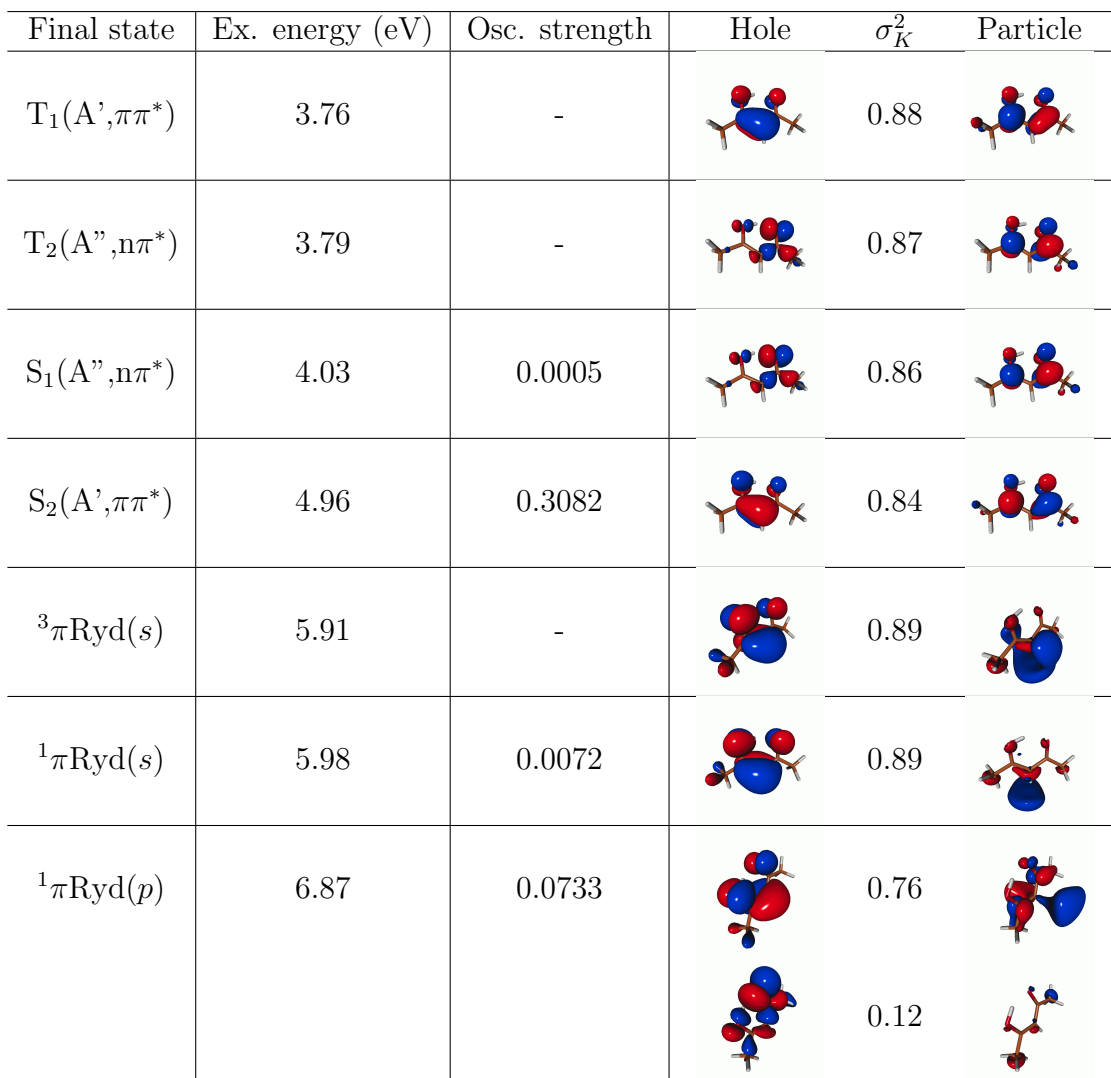   | 0.87         | 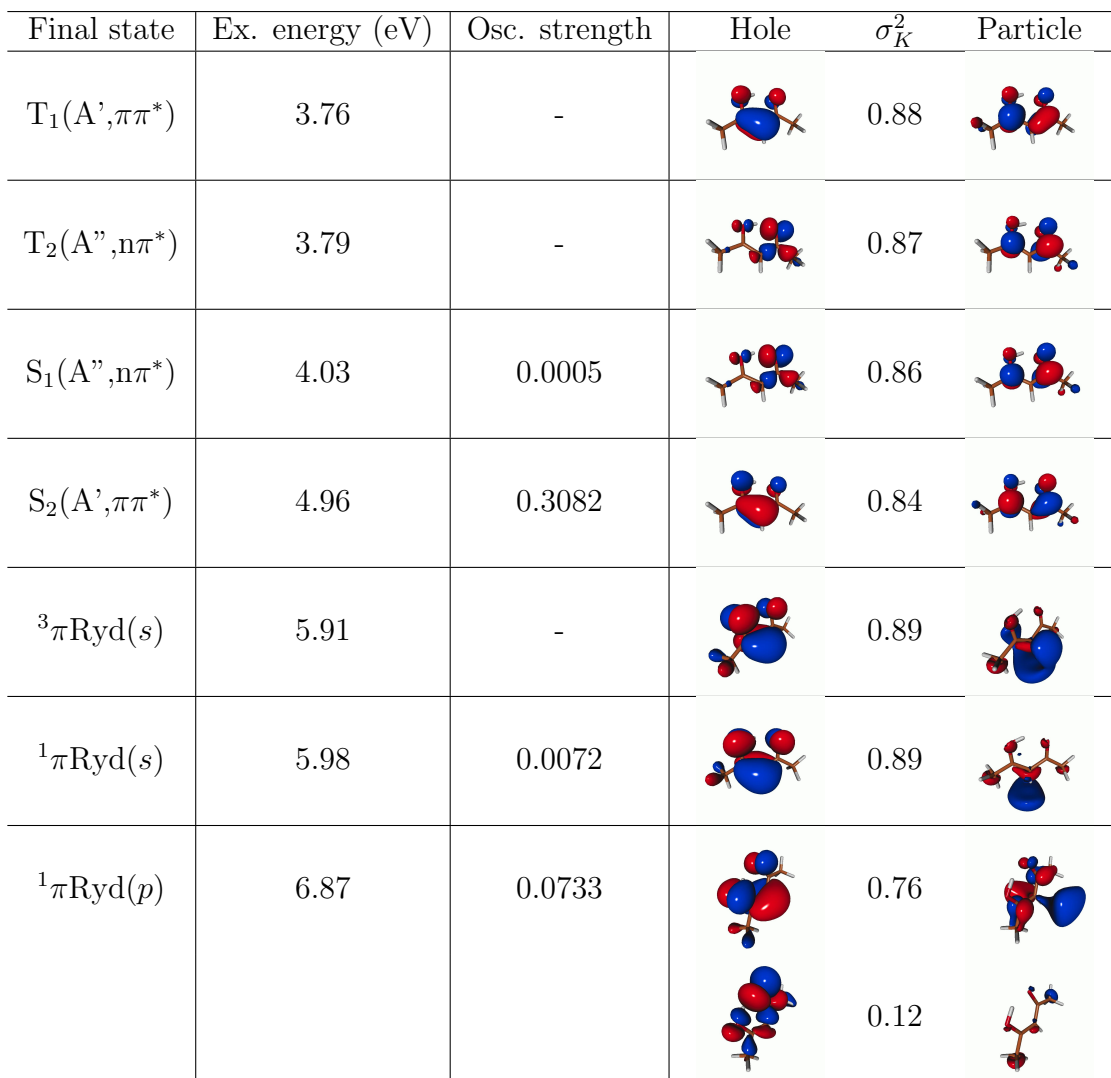   |
| $S_1(A'', n\pi^*)$     | 4.03            | 0.0005        | 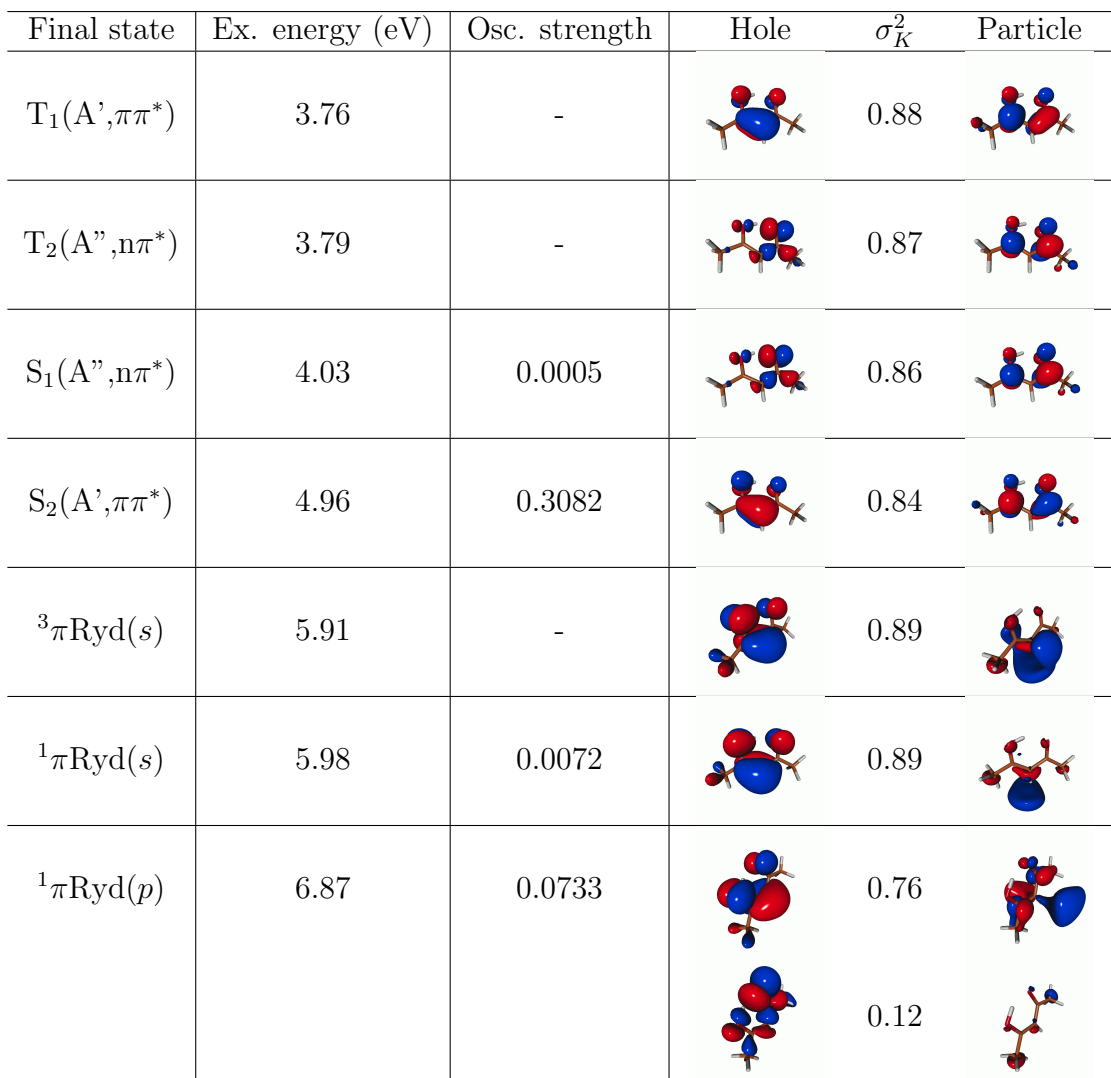   | 0.86         | 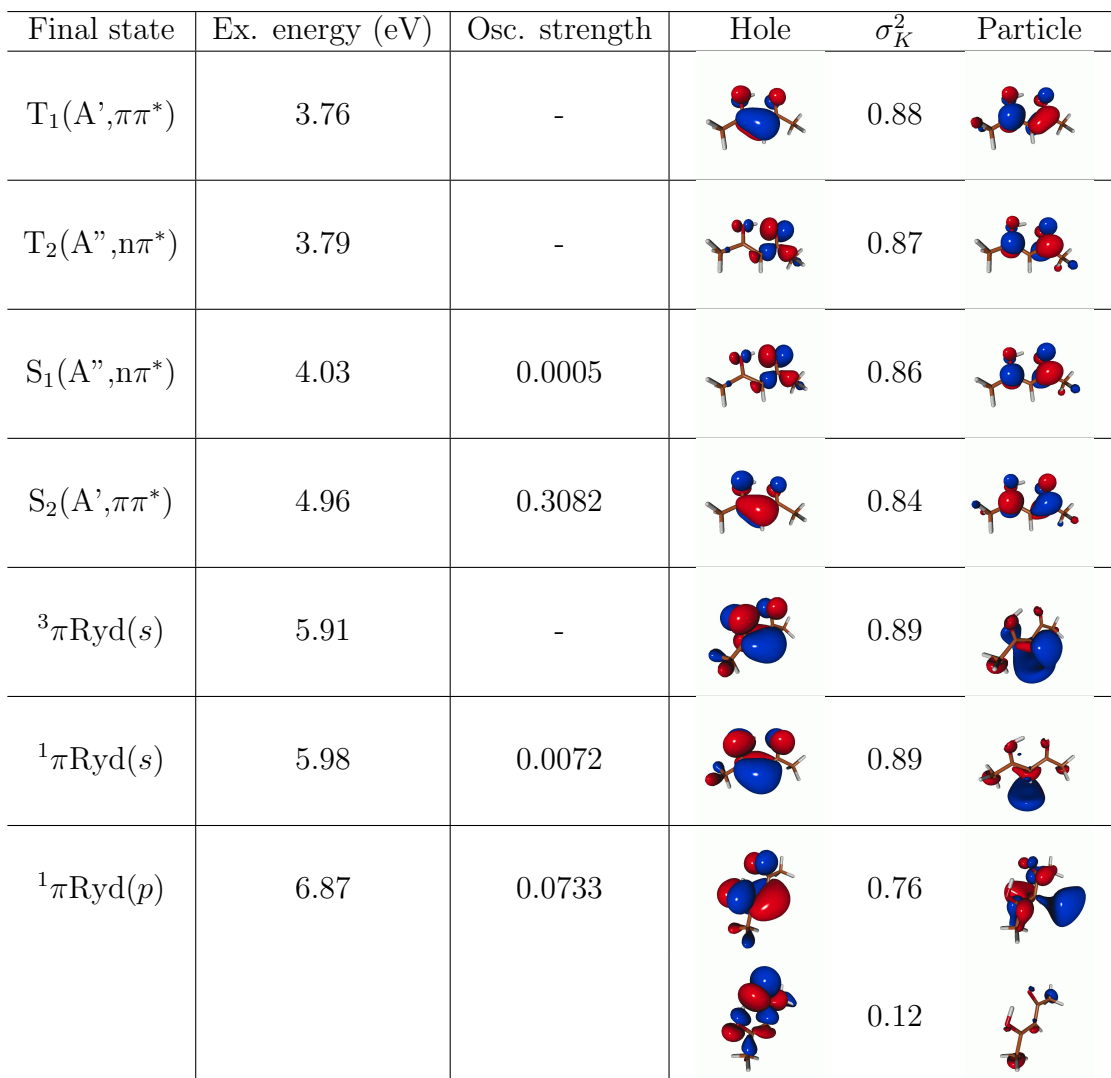   |
| $S_2(A', \pi\pi^*)$    | 4.96            | 0.3082        | 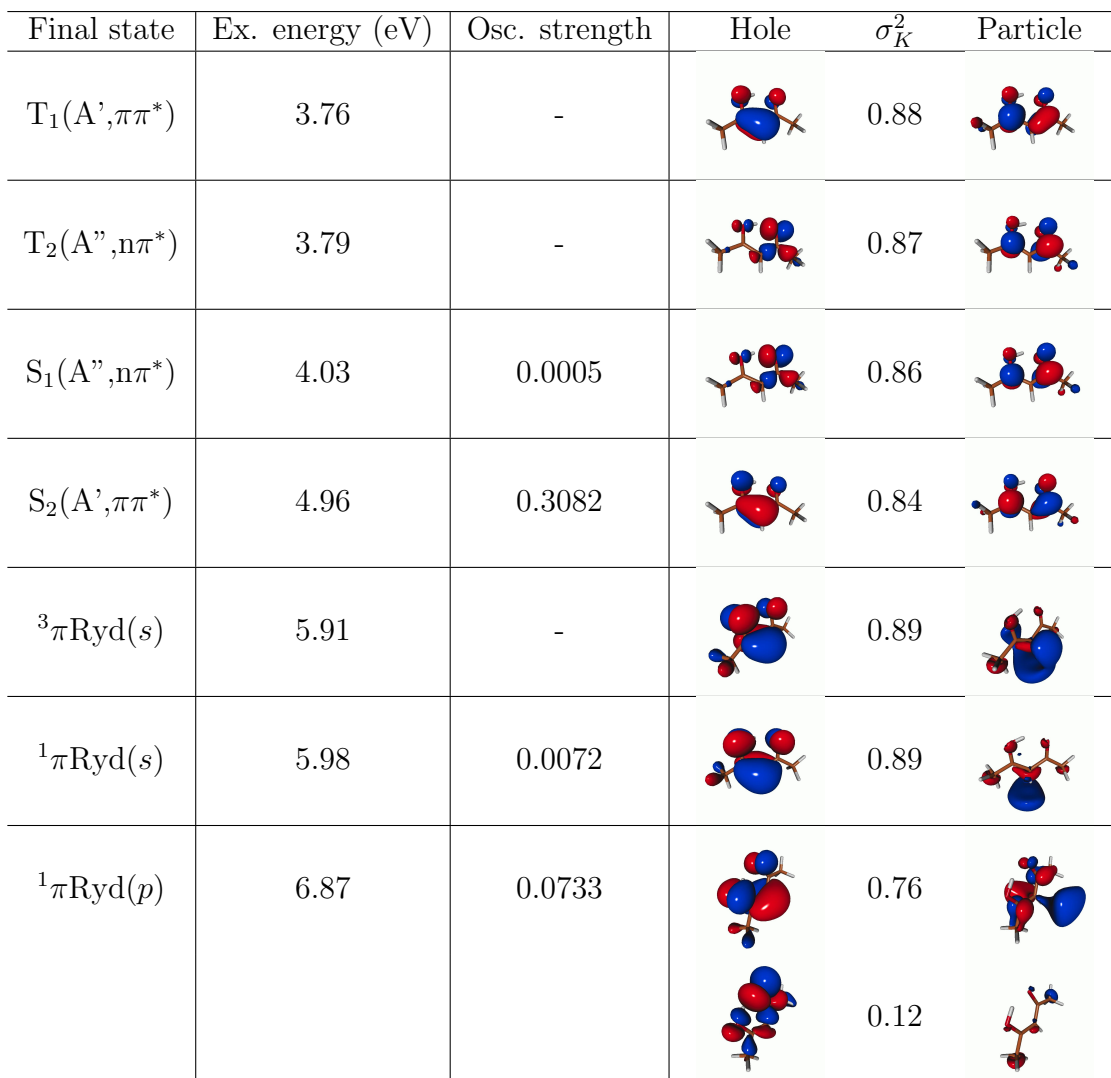 | 0.84         | 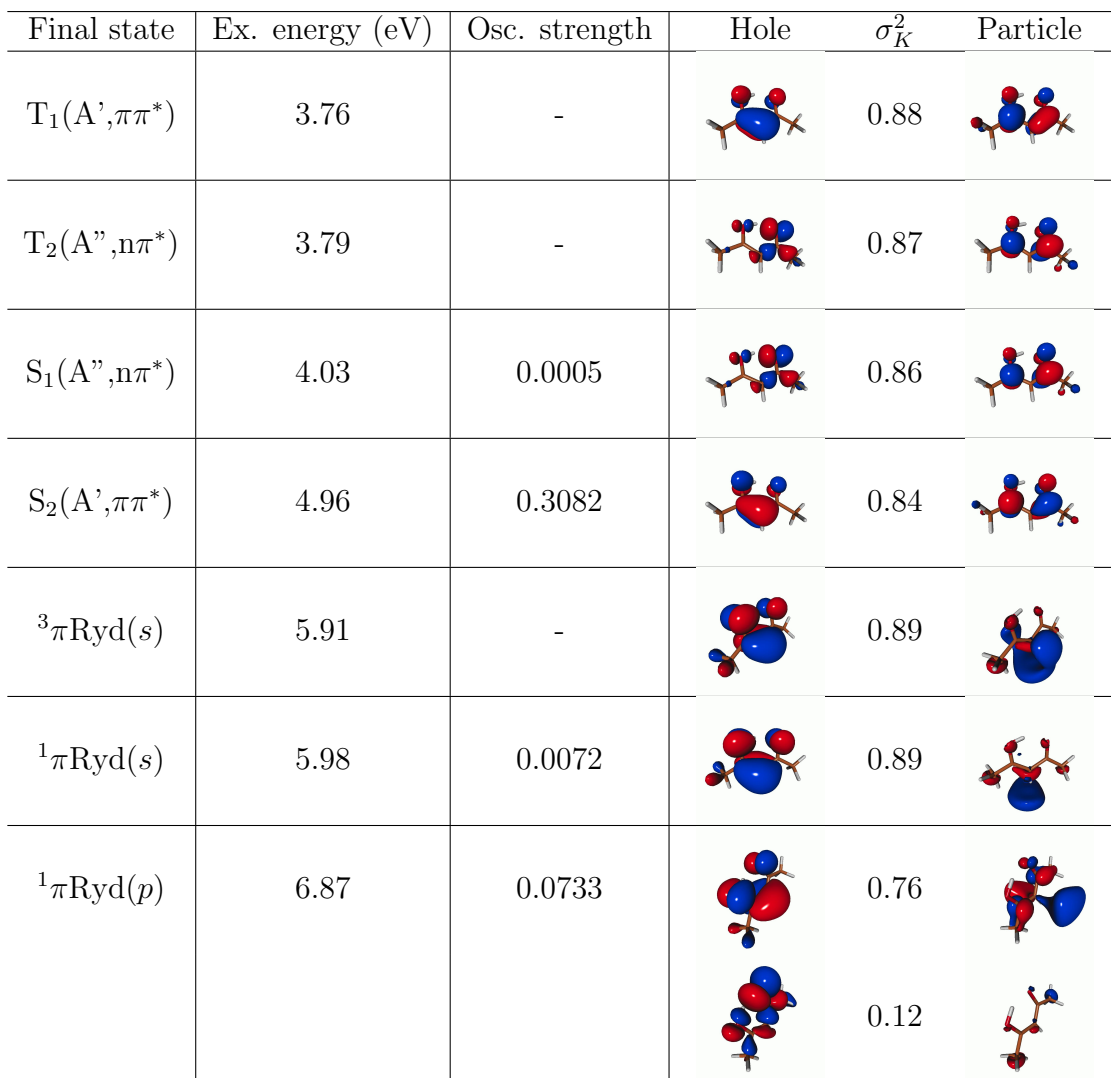 |
| ${}^3\pi\text{Ryd}(s)$ | 5.91            | -             | 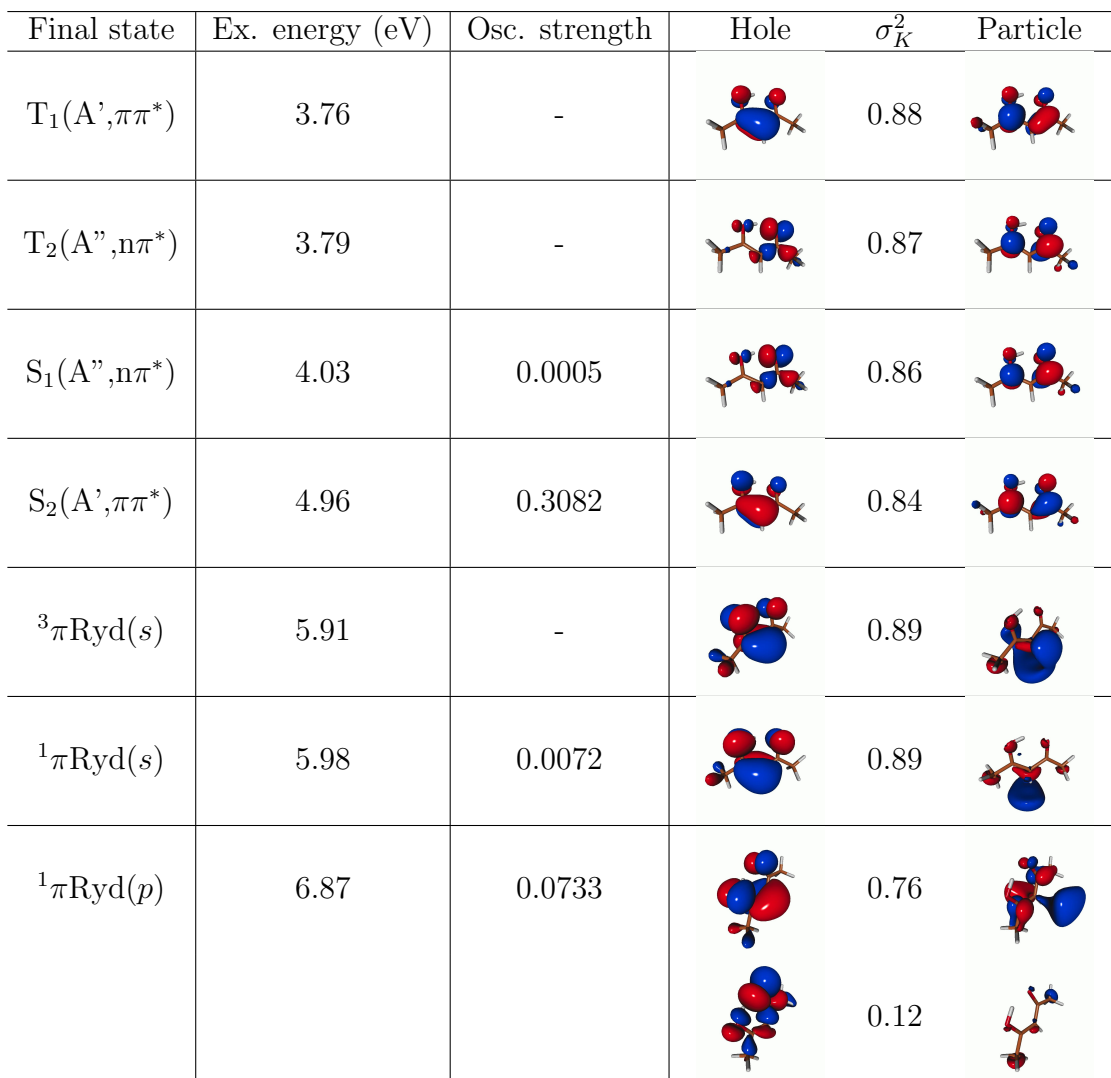 | 0.89         | 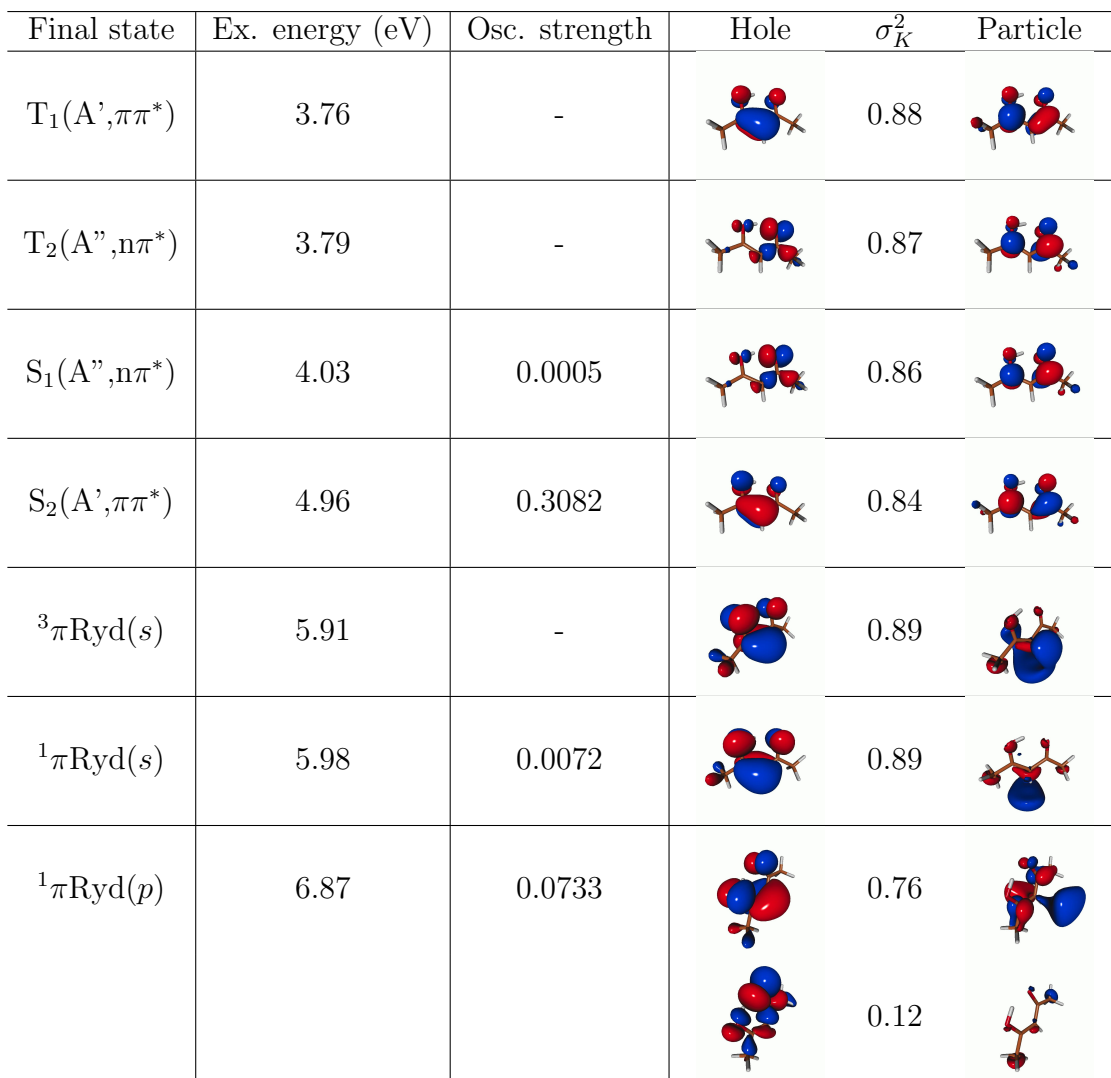 |
| ${}^1\pi\text{Ryd}(s)$ | 5.98            | 0.0072        | 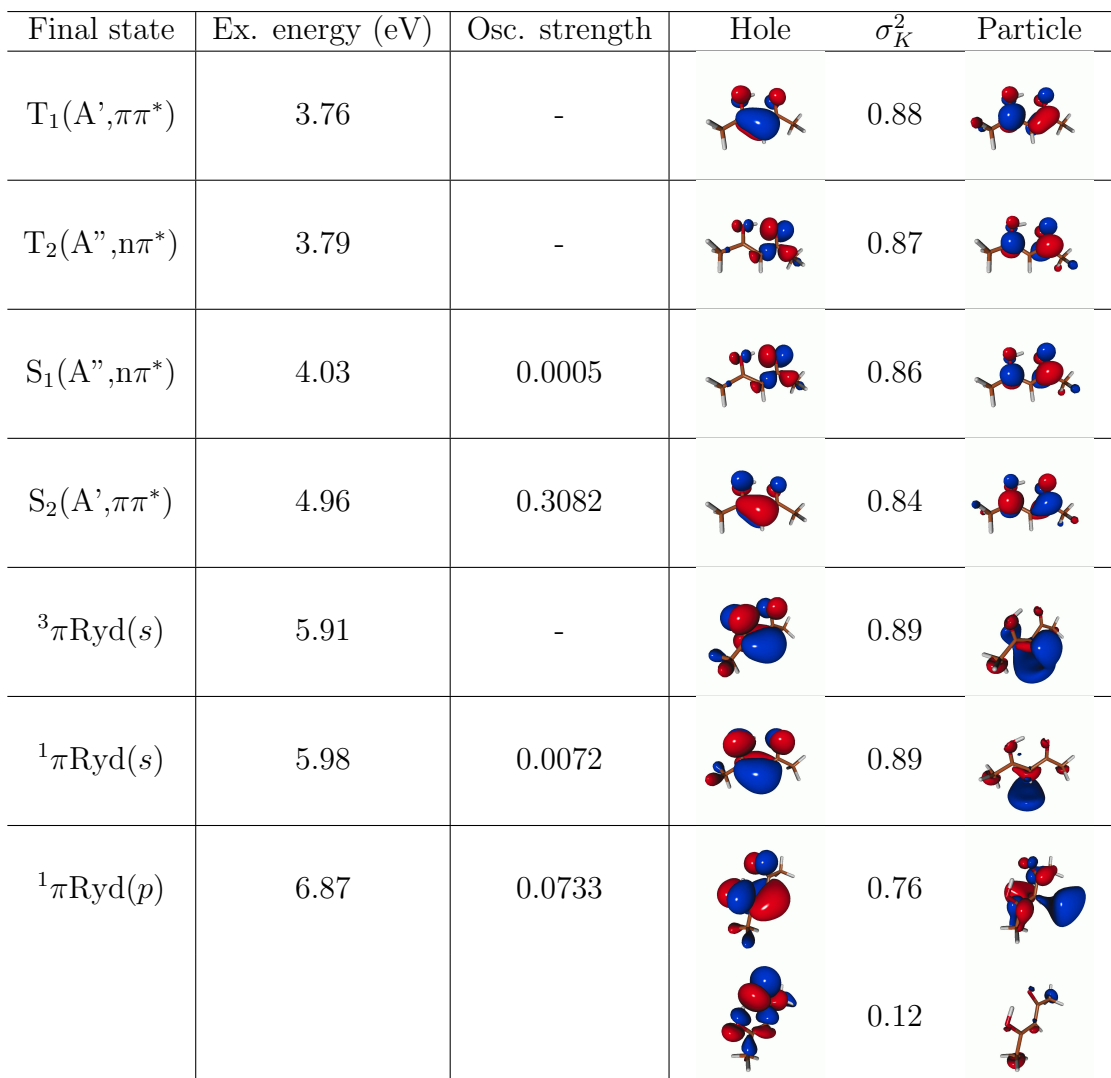 | 0.89         | 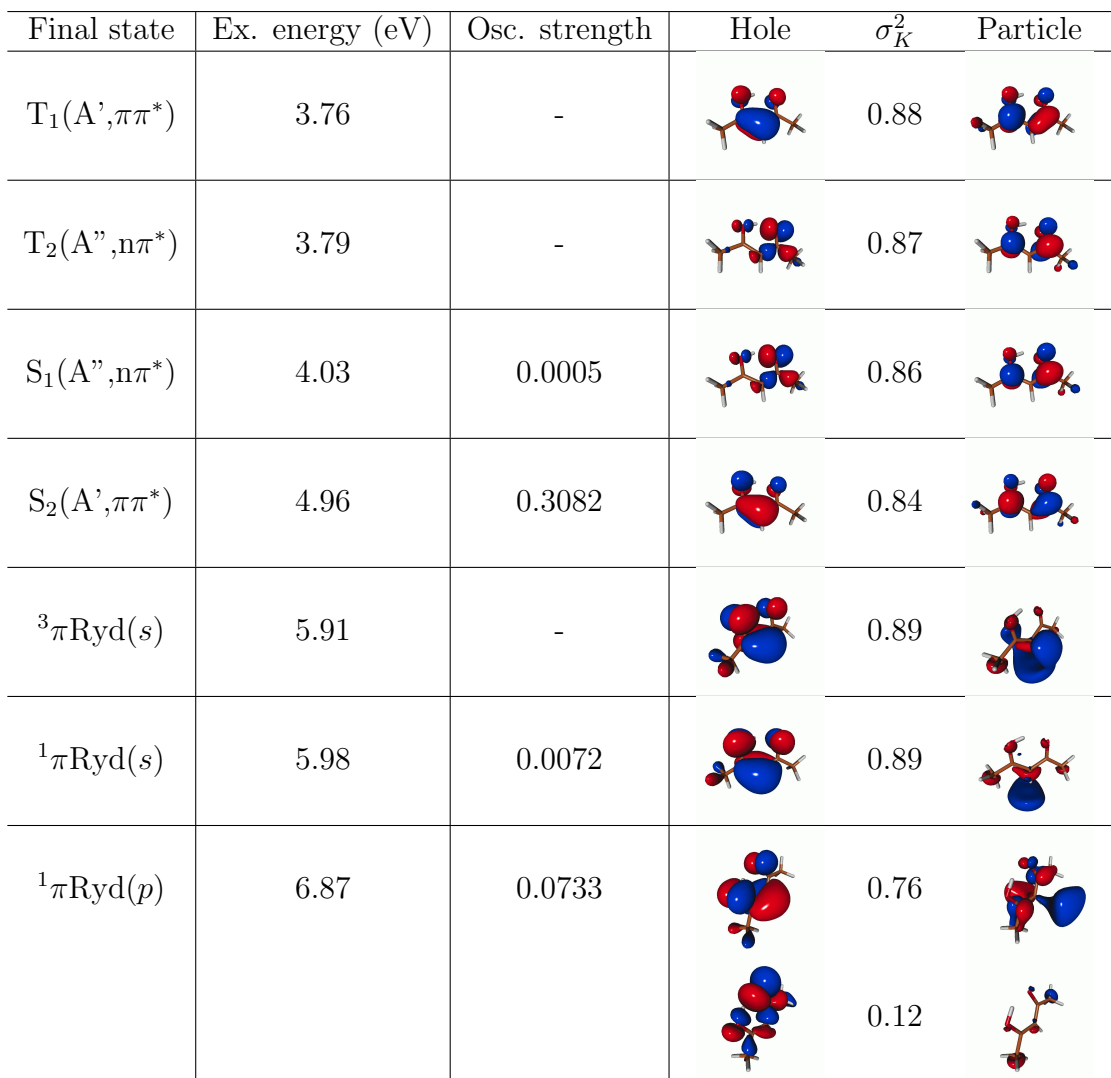 |
| ${}^1\pi\text{Ryd}(p)$ | 6.87            | 0.0733        | 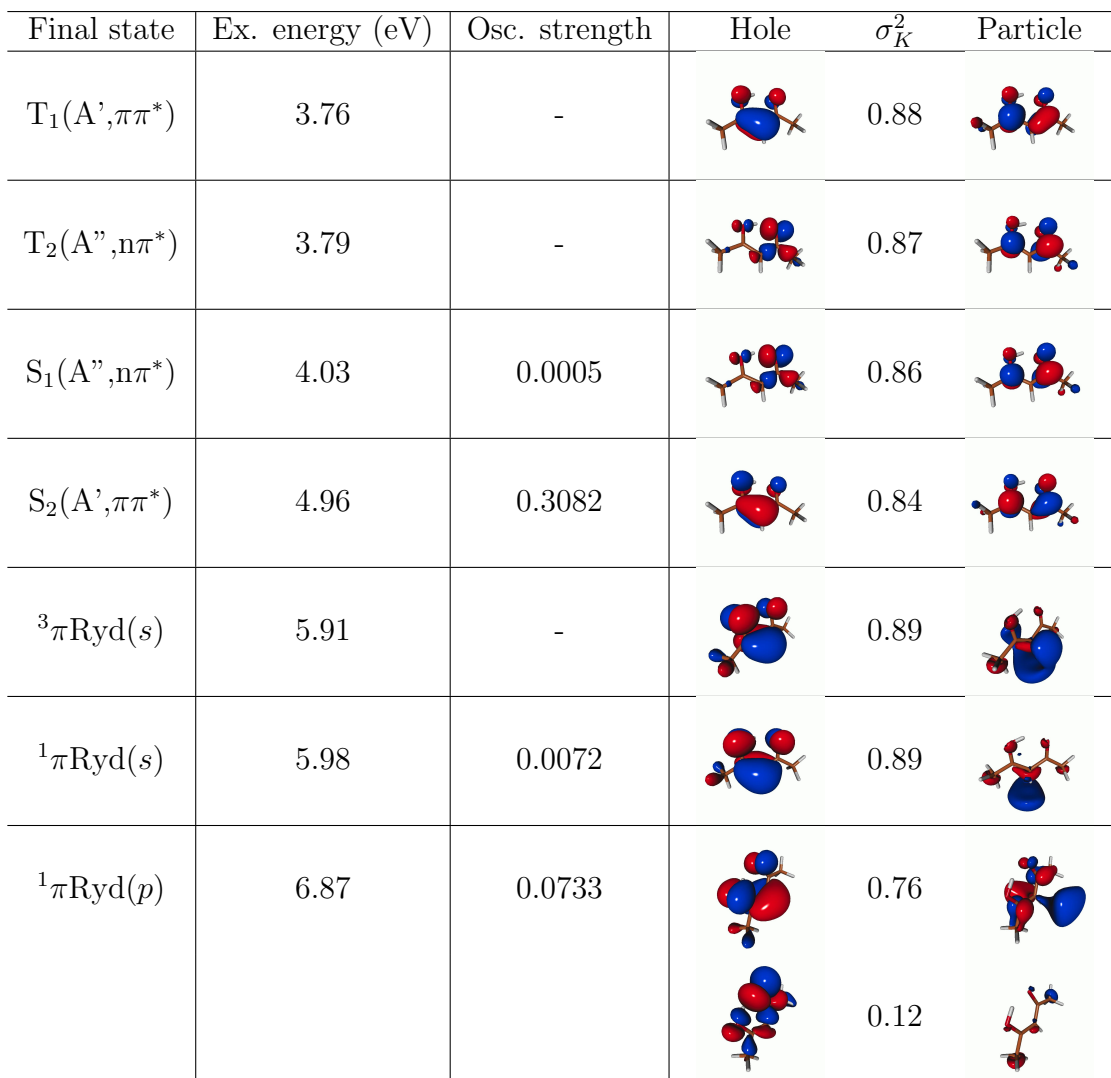 | 0.76         | 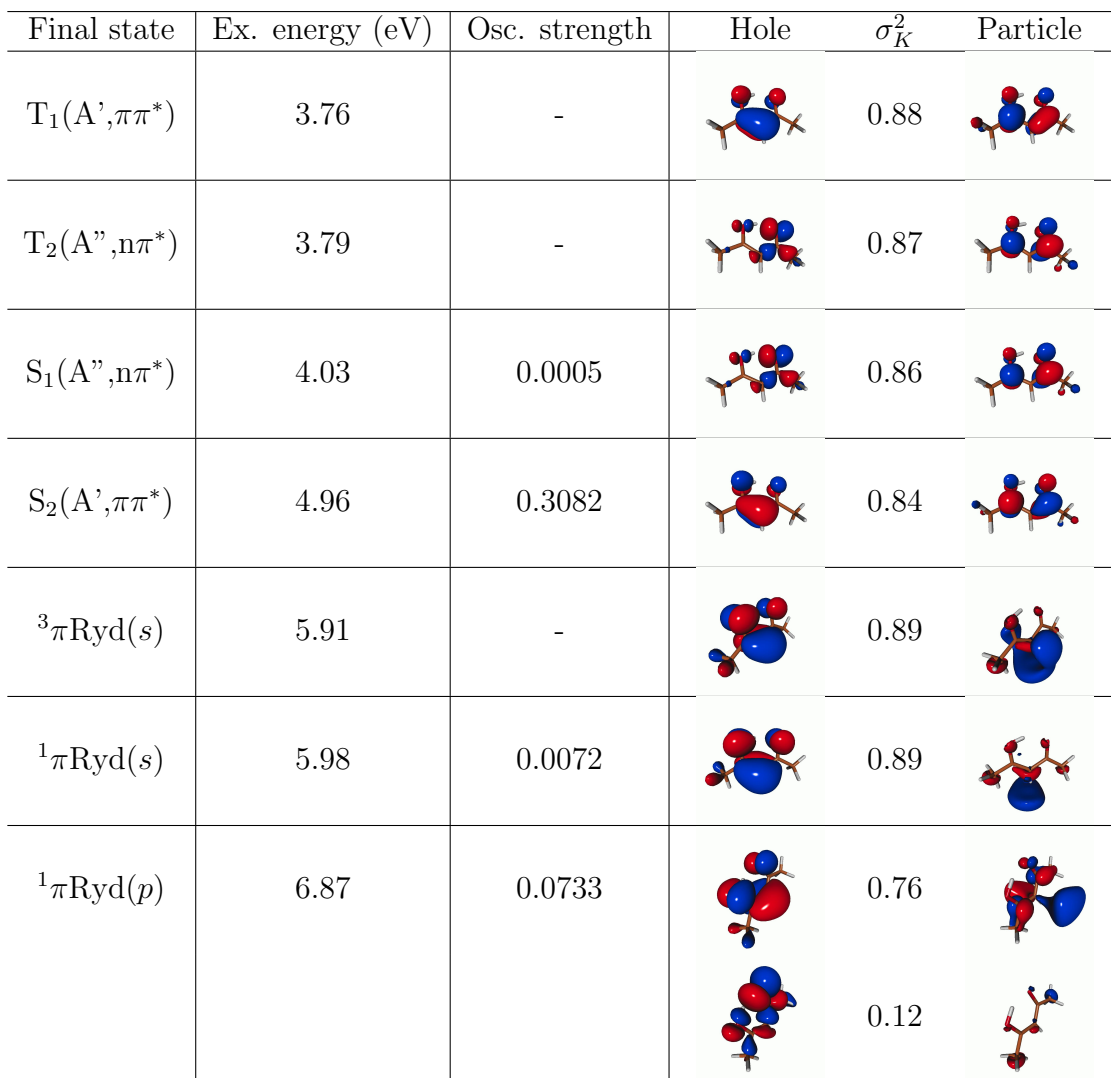 |
|                        |                 |               | 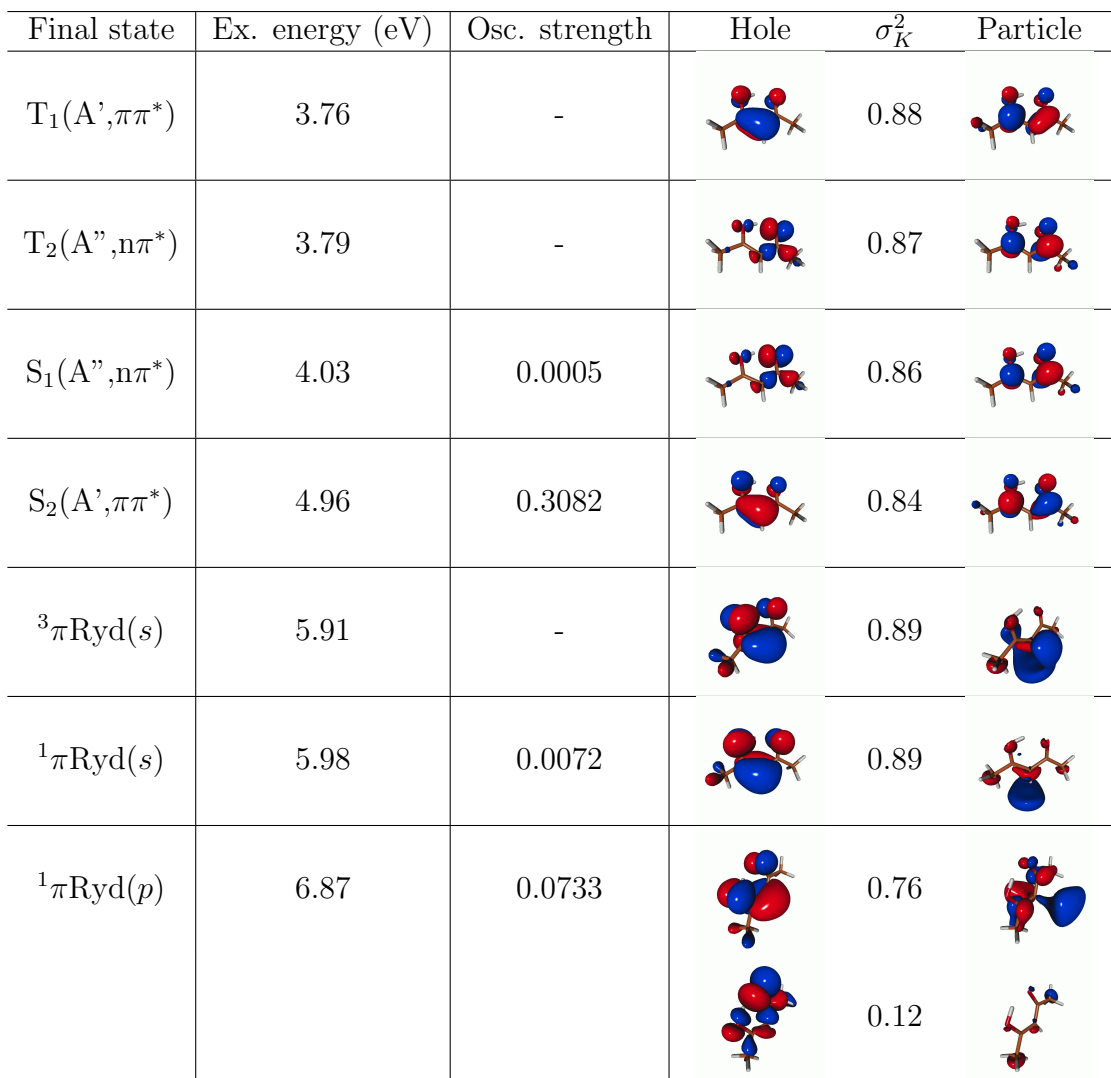 | 0.12         | 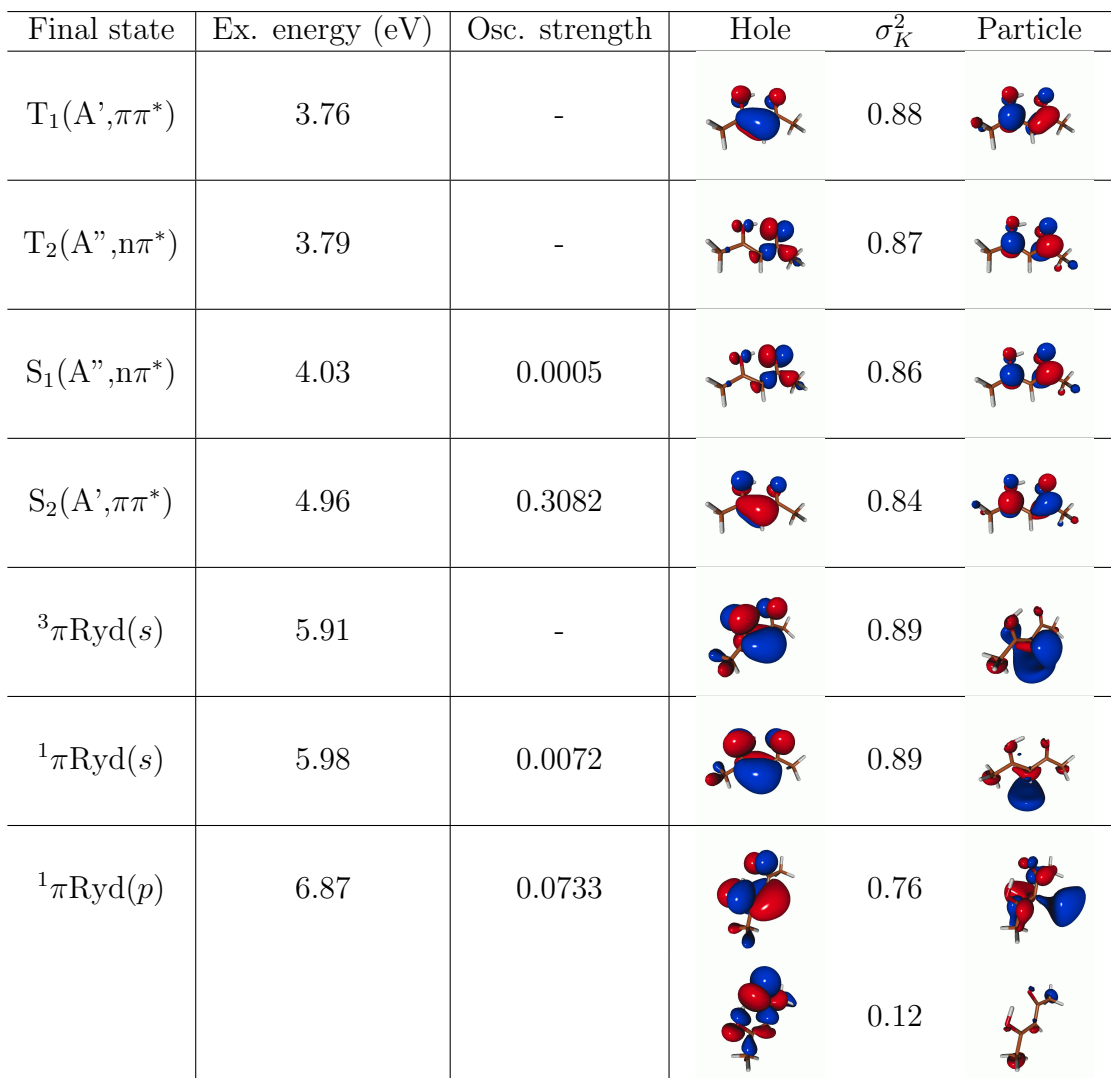 |

Table S18: Acetylacetone. TDDFT/B3LYP/6-311++G\*\* NTOs of the excitations from the ground state to the lowest-lying valence-excited states at the FC geometry (NTO isosurface is 0.03 for the Rydberg transitions and 0.05 for the others).

| Final state            | Ex. energy (eV) | Osc. strength | Hole                                                                                 | $\sigma_K^2$ | Particle                                                                              |
|------------------------|-----------------|---------------|--------------------------------------------------------------------------------------|--------------|---------------------------------------------------------------------------------------|
| $T_1(A', \pi\pi^*)$    | 3.23            | -             | 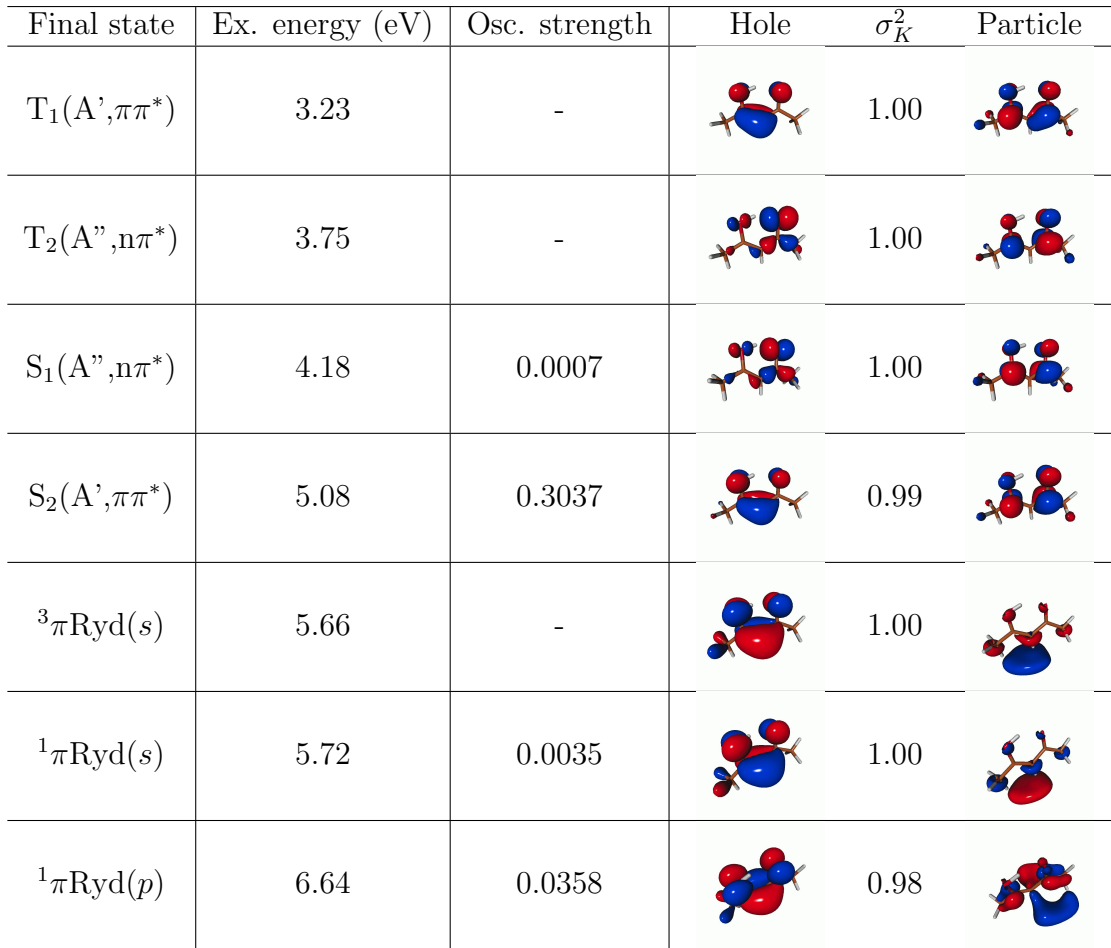   | 1.00         | 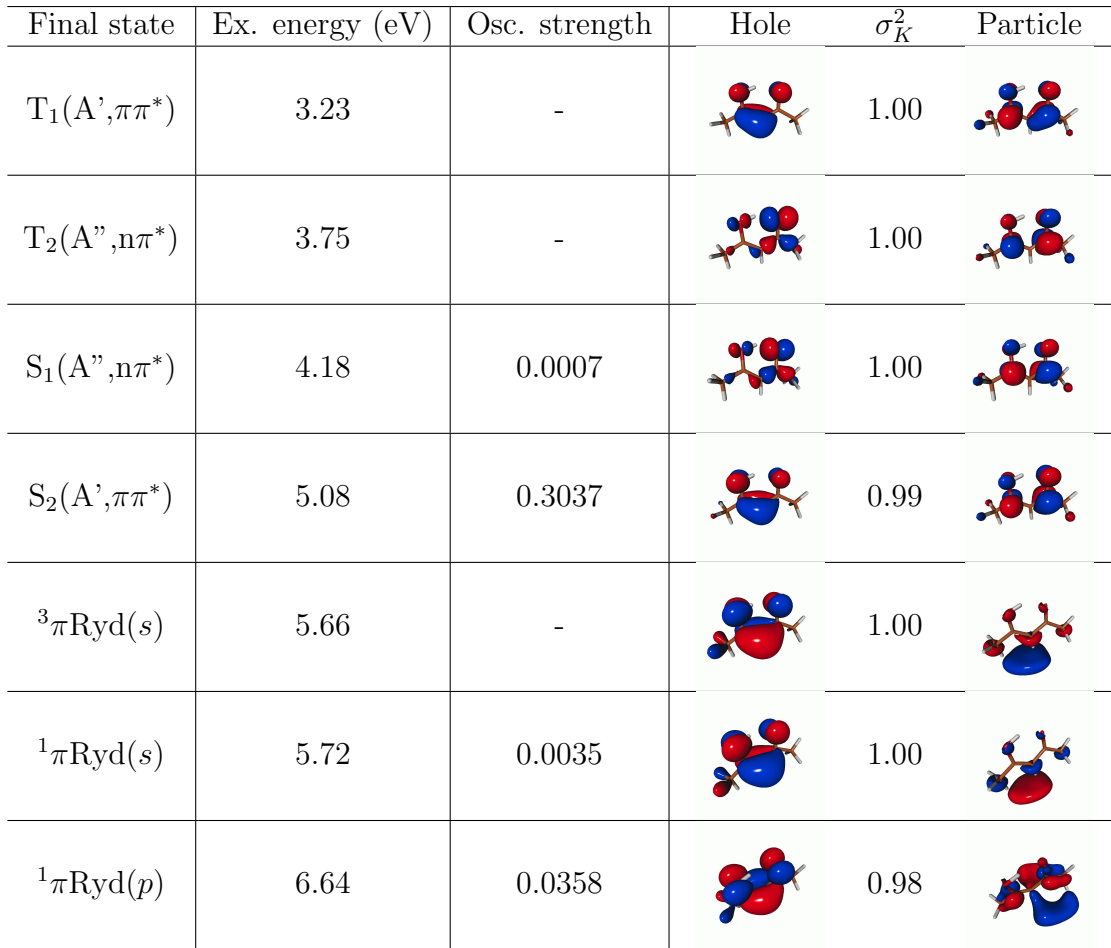   |
| $T_2(A'', n\pi^*)$     | 3.75            | -             | 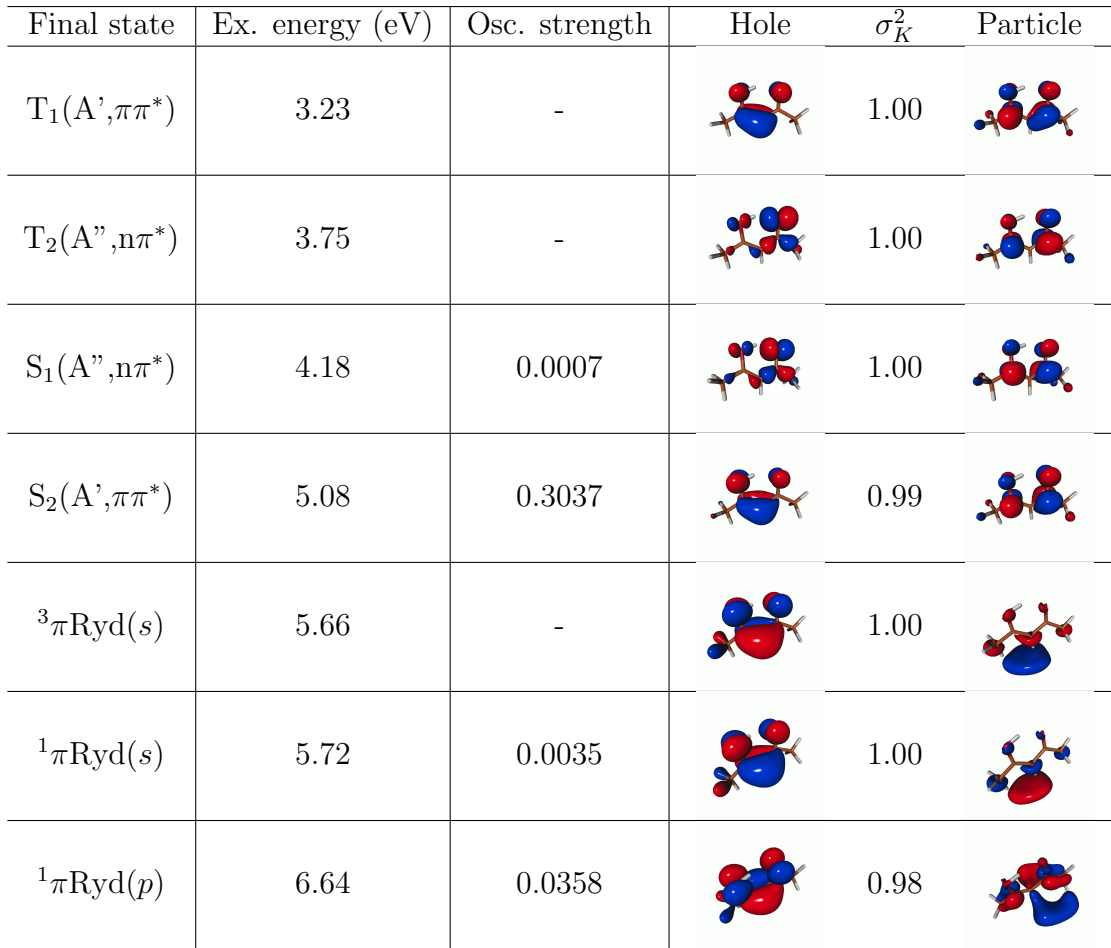   | 1.00         | 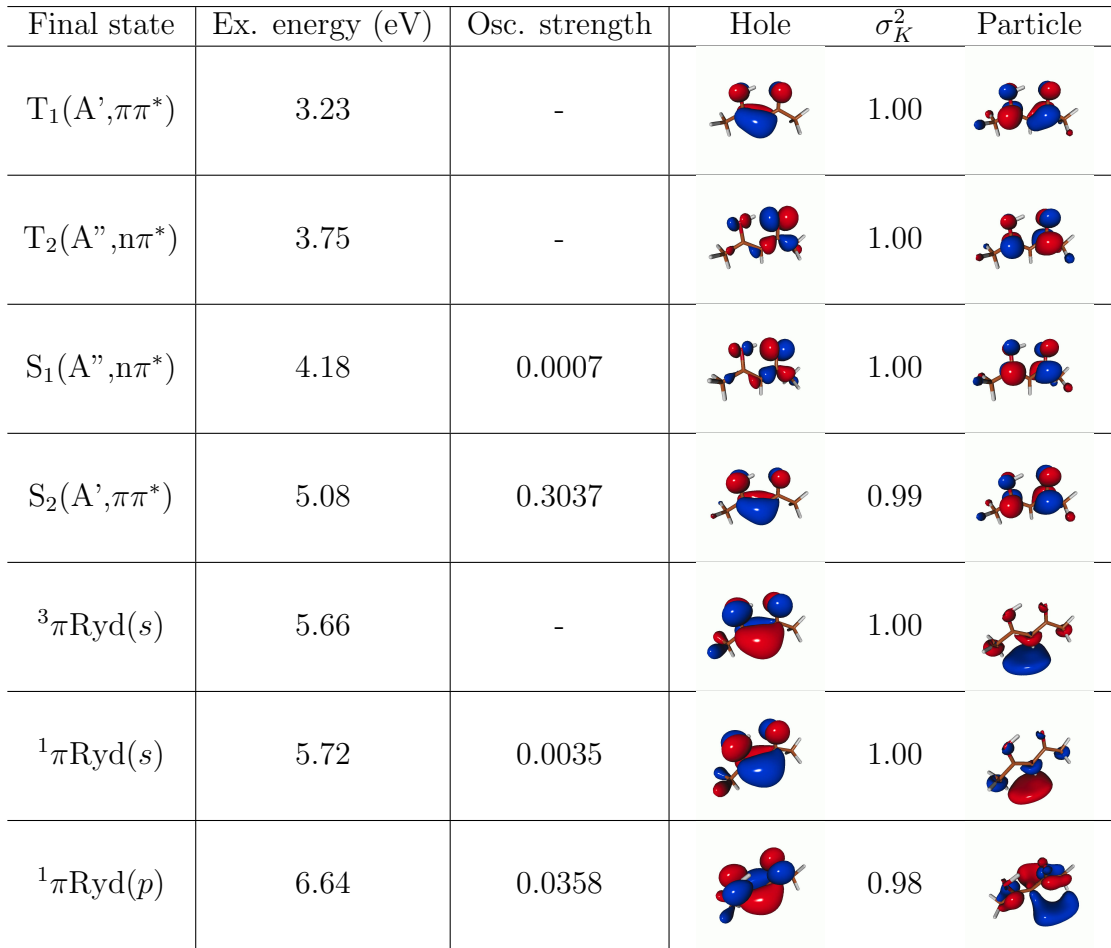   |
| $S_1(A'', n\pi^*)$     | 4.18            | 0.0007        | 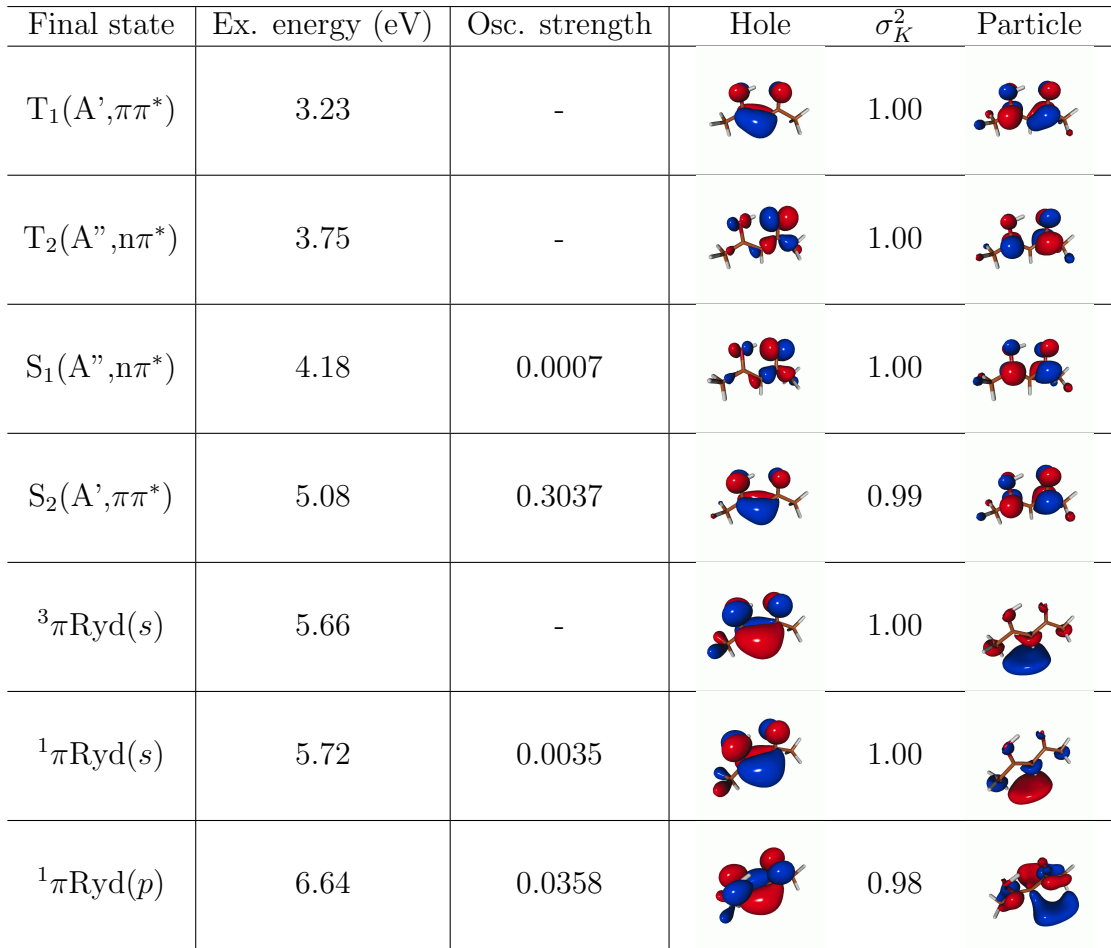  | 1.00         | 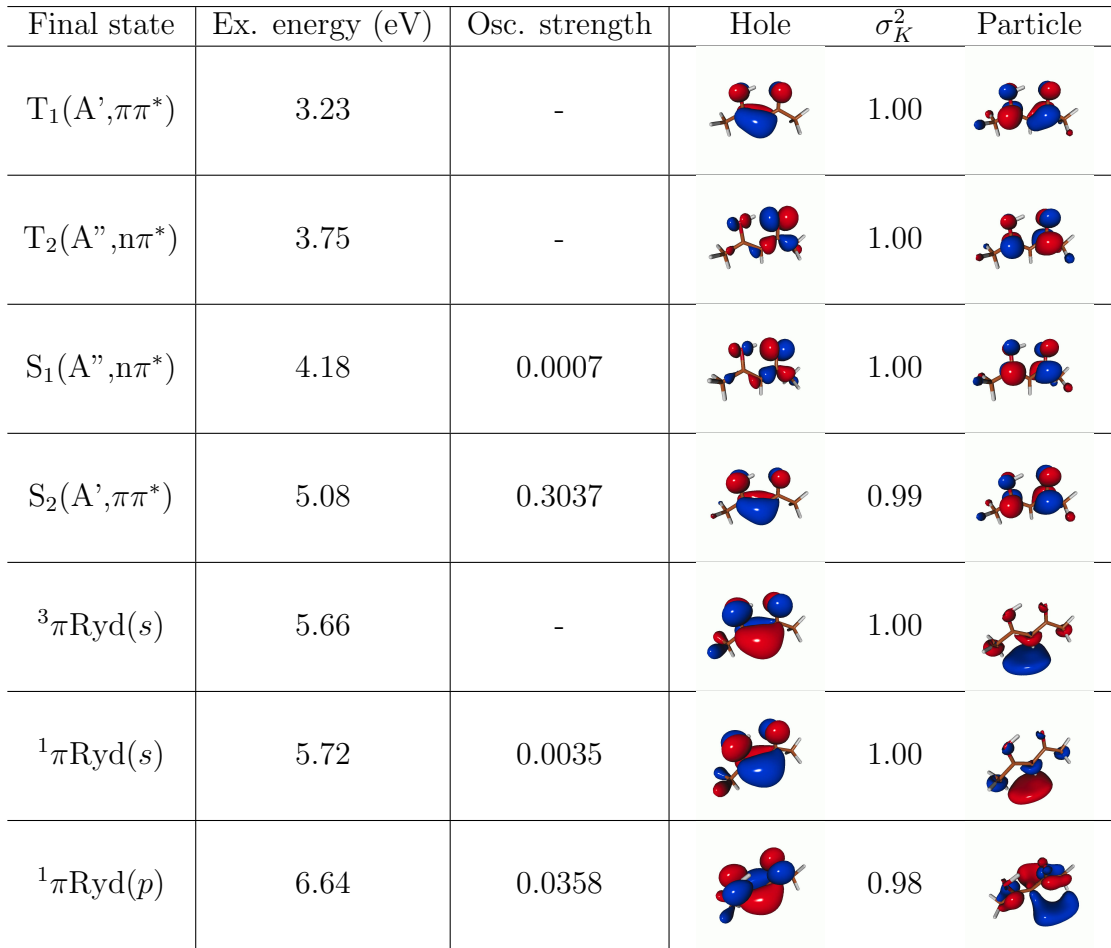  |
| $S_2(A', \pi\pi^*)$    | 5.08            | 0.3037        | 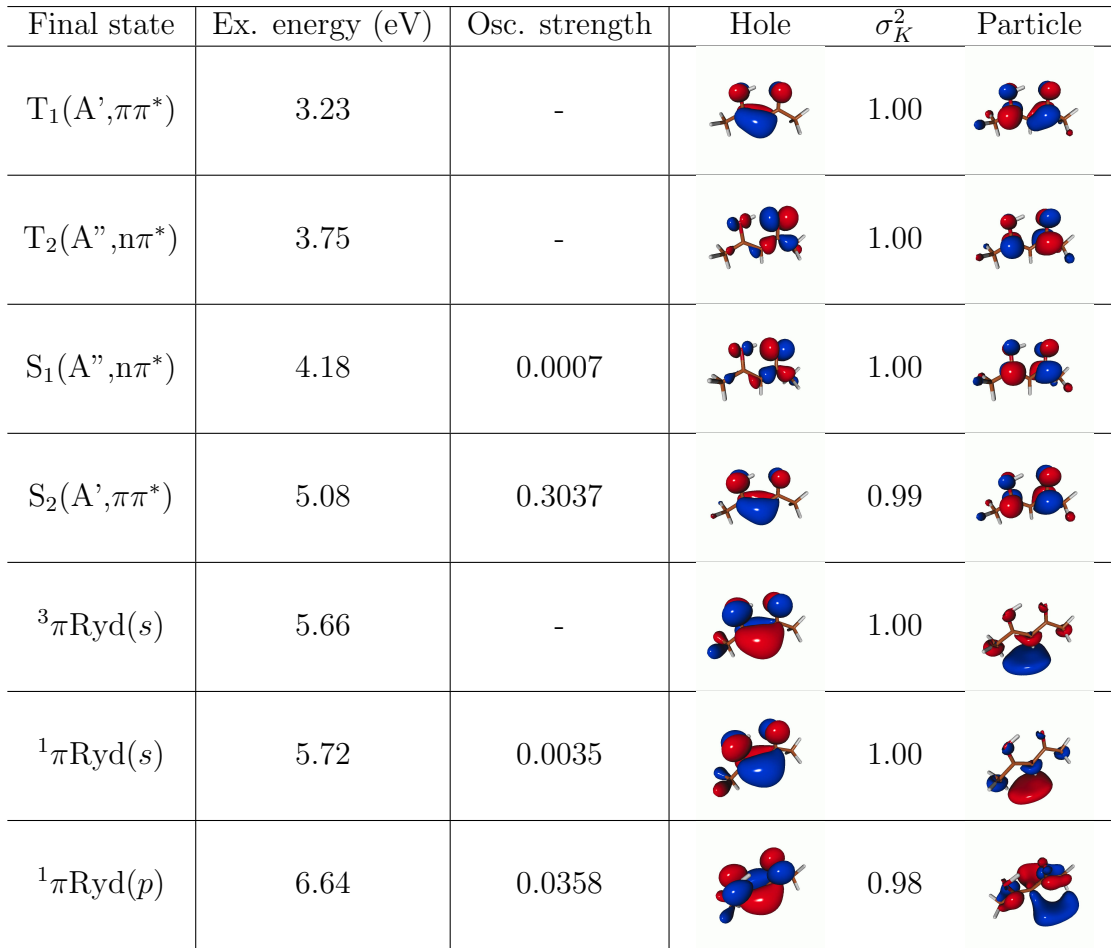 | 0.99         | 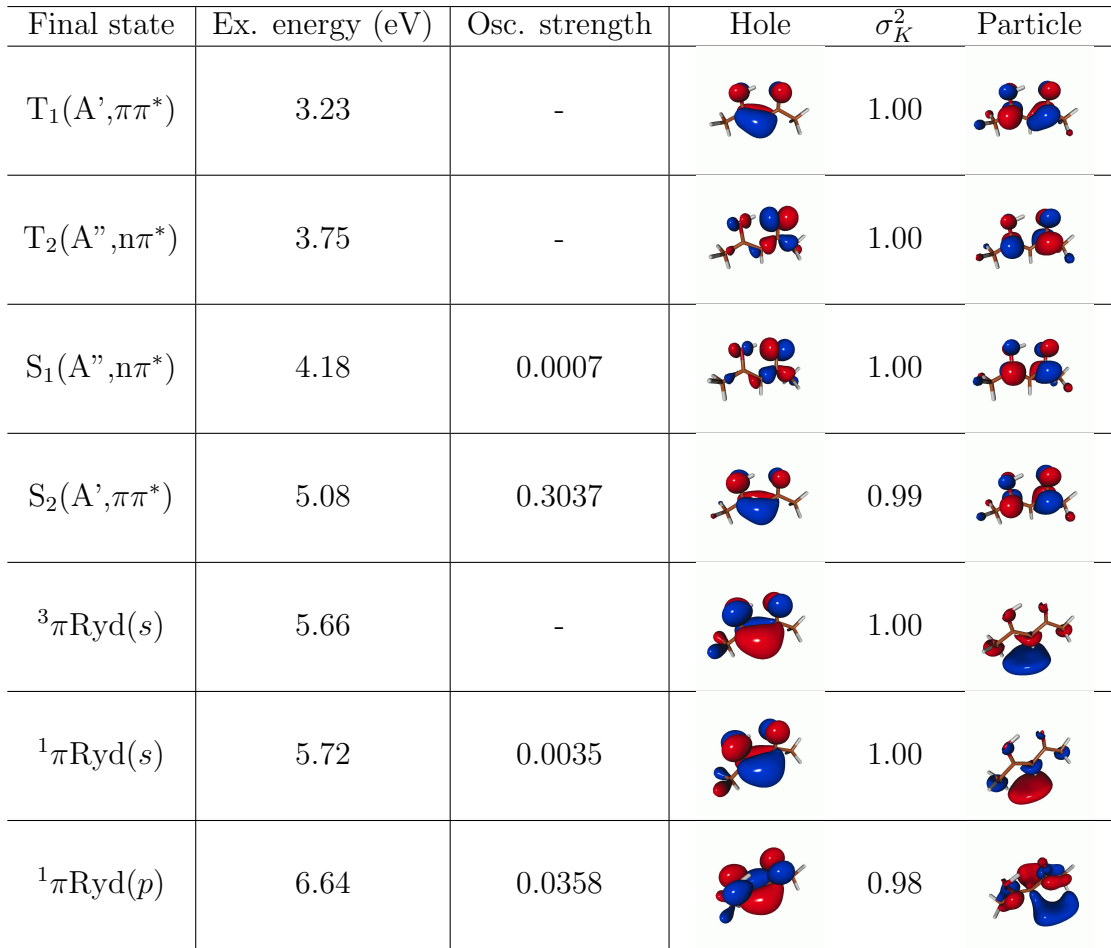 |
| ${}^3\pi\text{Ryd}(s)$ | 5.66            | -             | 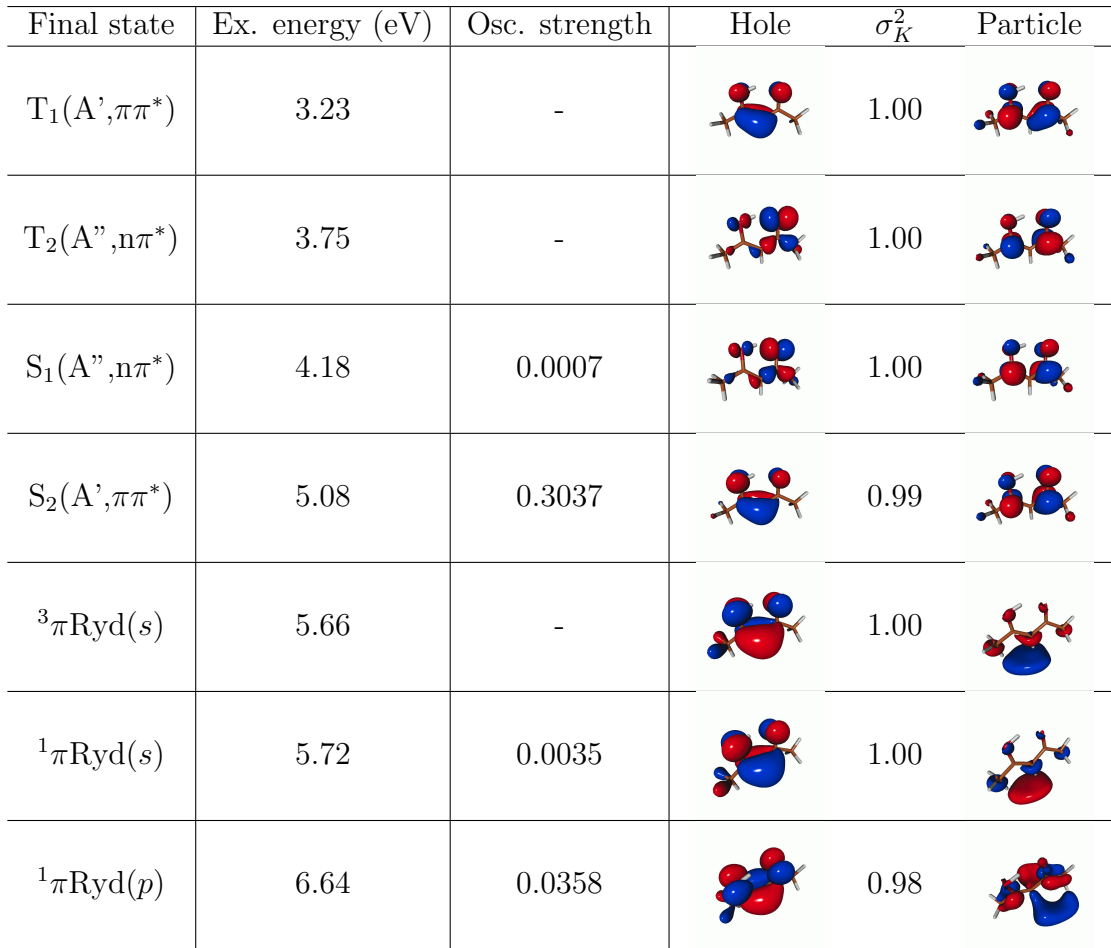 | 1.00         | 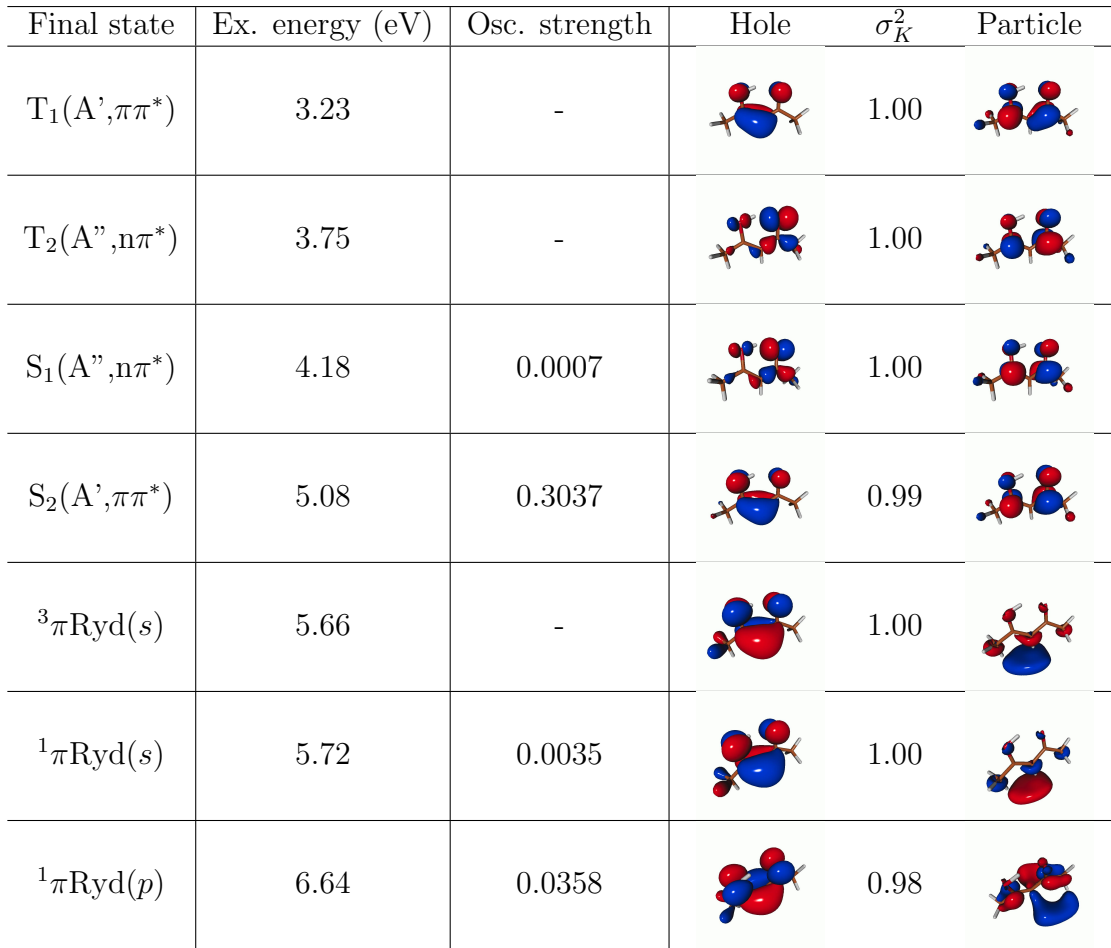 |
| ${}^1\pi\text{Ryd}(s)$ | 5.72            | 0.0035        | 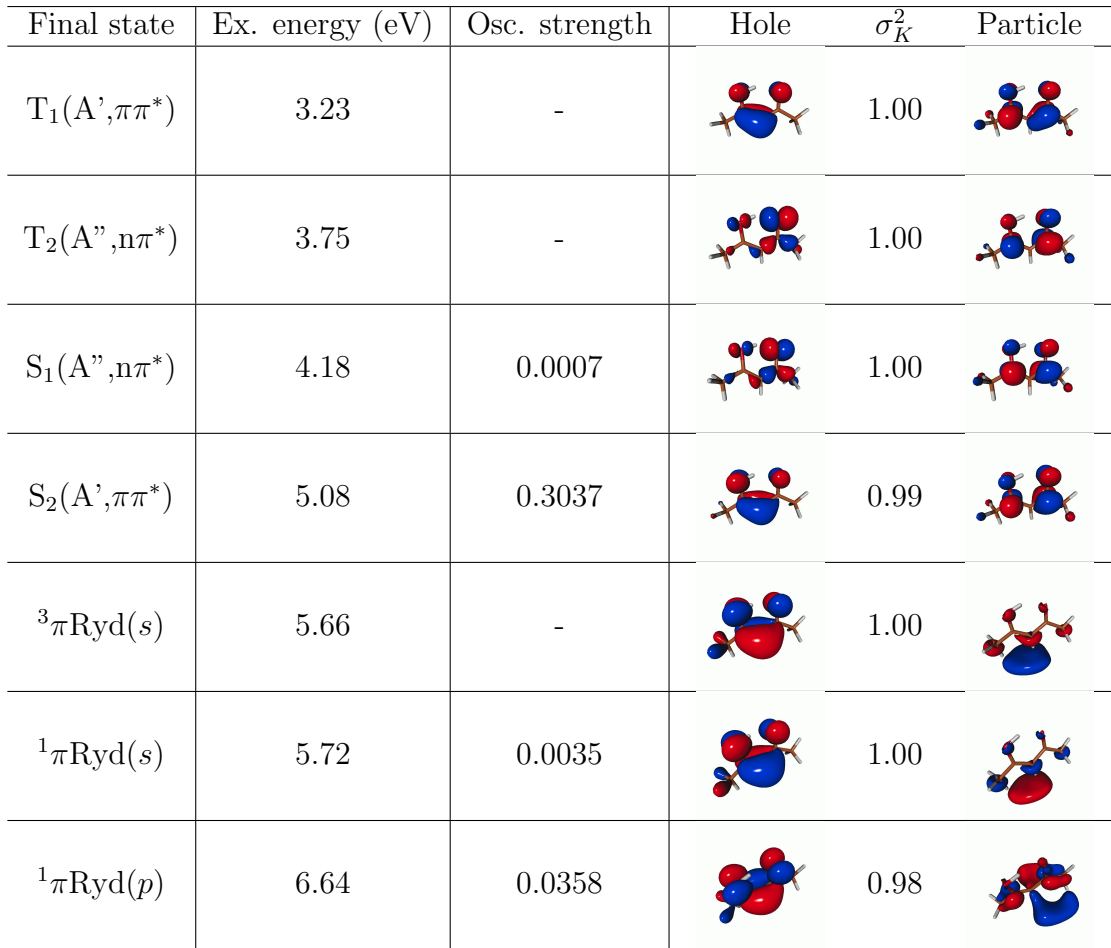 | 1.00         | 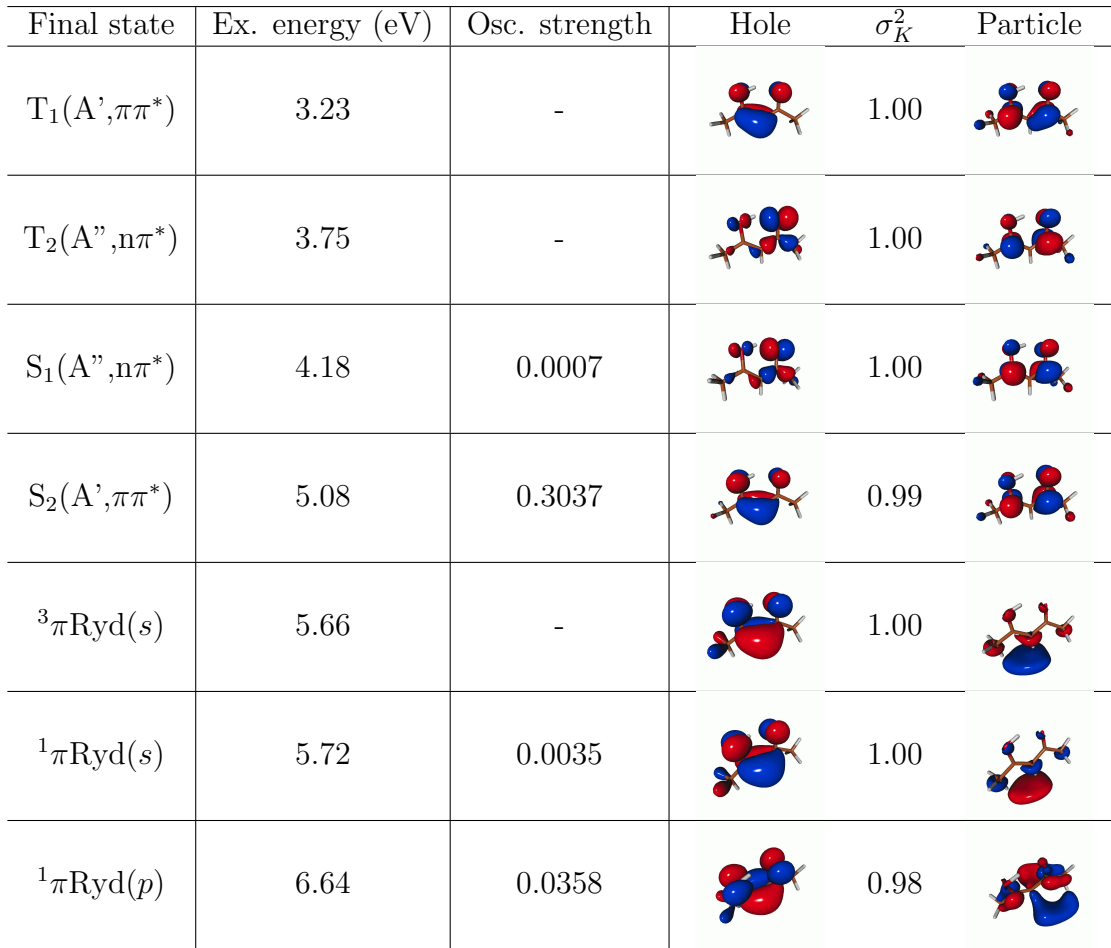 |
| ${}^1\pi\text{Ryd}(p)$ | 6.64            | 0.0358        | 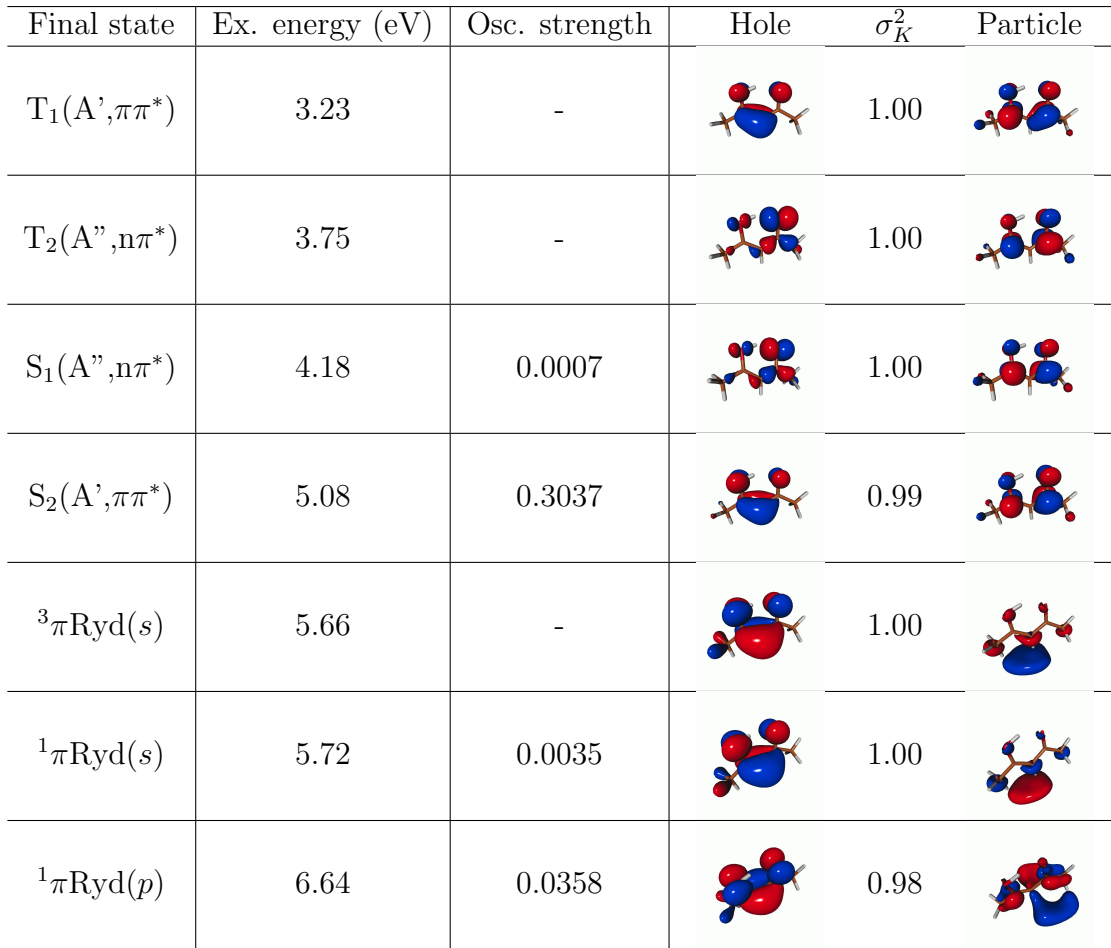 | 0.98         | 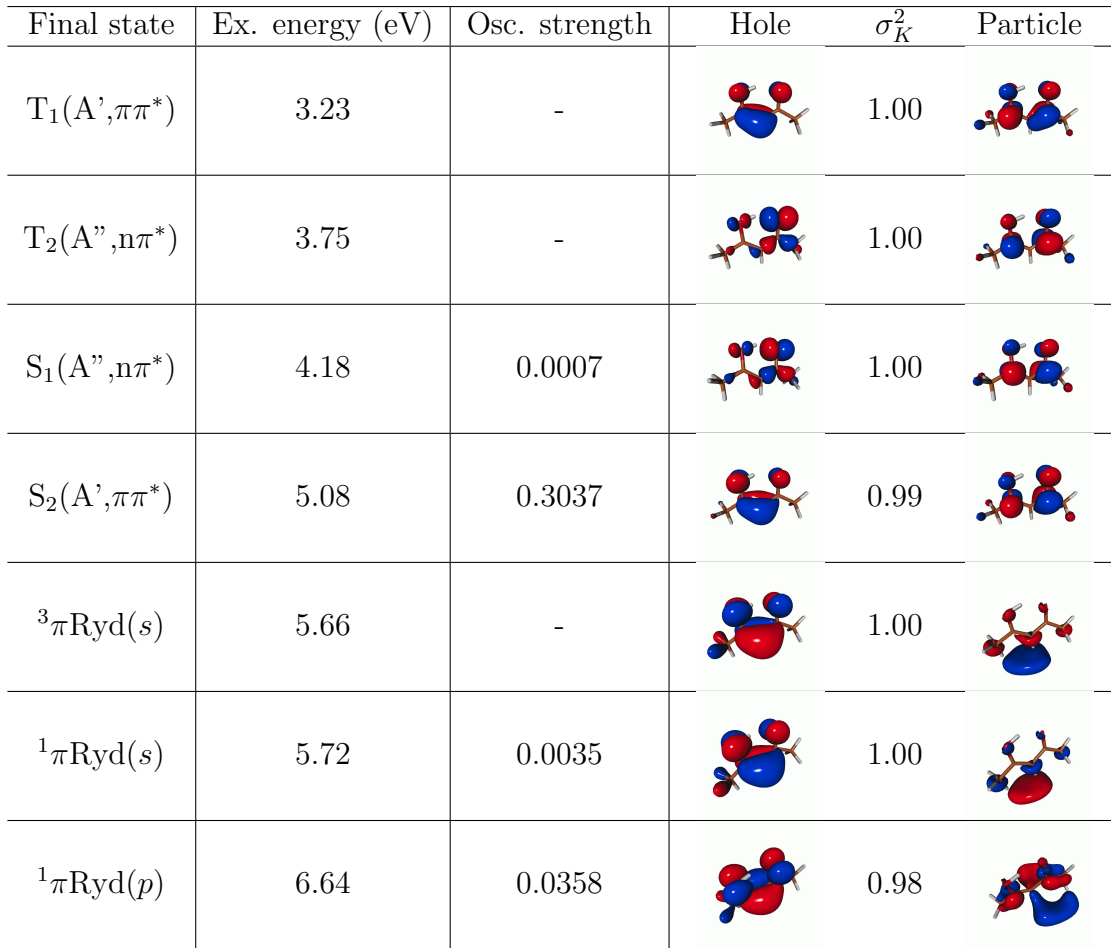 |

## S3 Natural transition orbitals of core excitations from the valence-excited states

Table S19: Uracil. LSOR-CCSD/6-311++G\*\* NTOs of the O<sub>1s</sub> core excitations from the S<sub>1</sub> state at the FC geometry (NTO isosurface value = 0.05).

| Ex. energy (eV) | Osc. strength | $\alpha$                                                                          |              |                                                                                    | $\beta$                                                                             |              |                                                                                     |
|-----------------|---------------|-----------------------------------------------------------------------------------|--------------|------------------------------------------------------------------------------------|-------------------------------------------------------------------------------------|--------------|-------------------------------------------------------------------------------------|
|                 |               | Hole                                                                              | $\sigma_K^2$ | Particle                                                                           | Hole                                                                                | $\sigma_K^2$ | Particle                                                                            |
| 526.39          | 0.0451        | 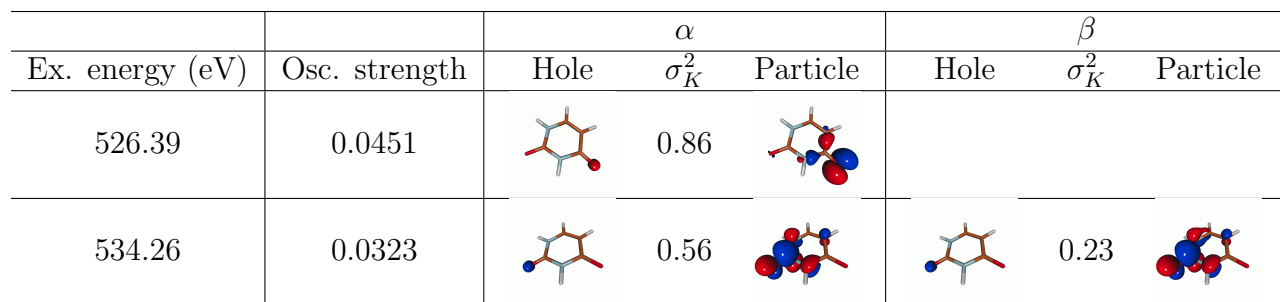 | 0.86         | 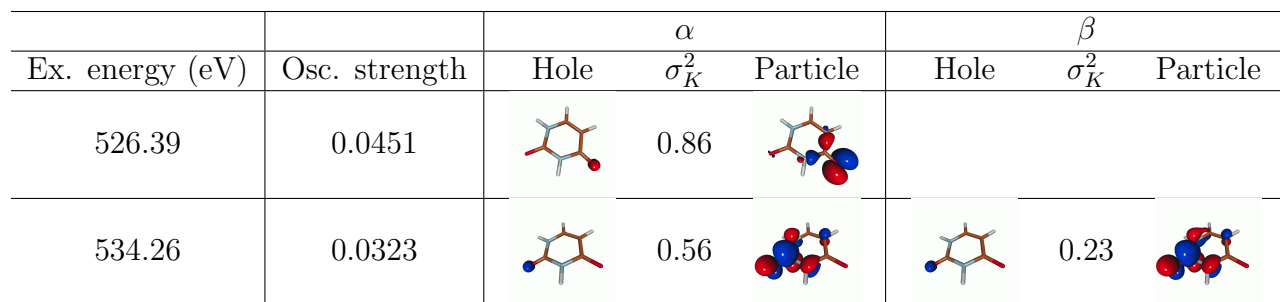 |                                                                                     |              |                                                                                     |
| 534.26          | 0.0323        | 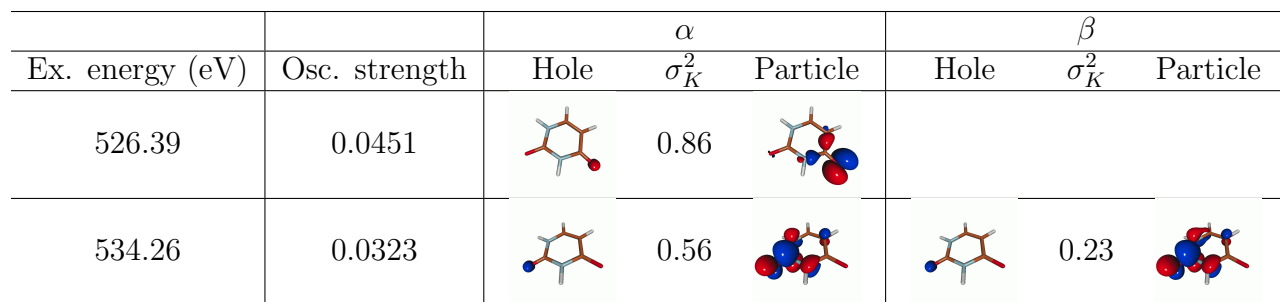 | 0.56         | 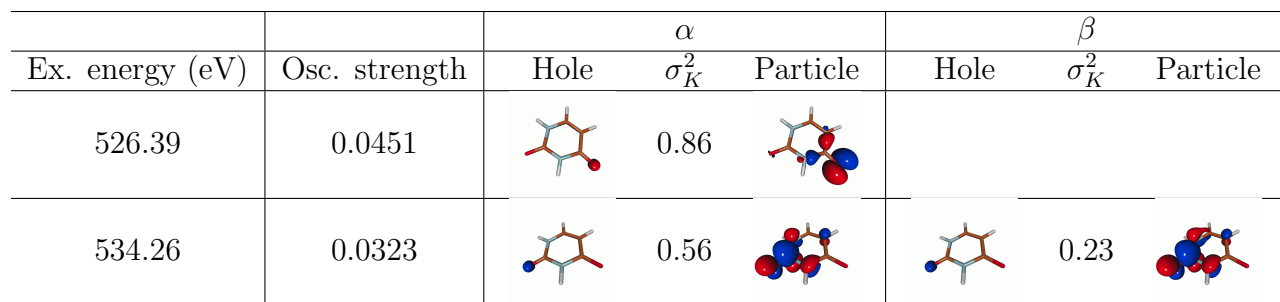 | 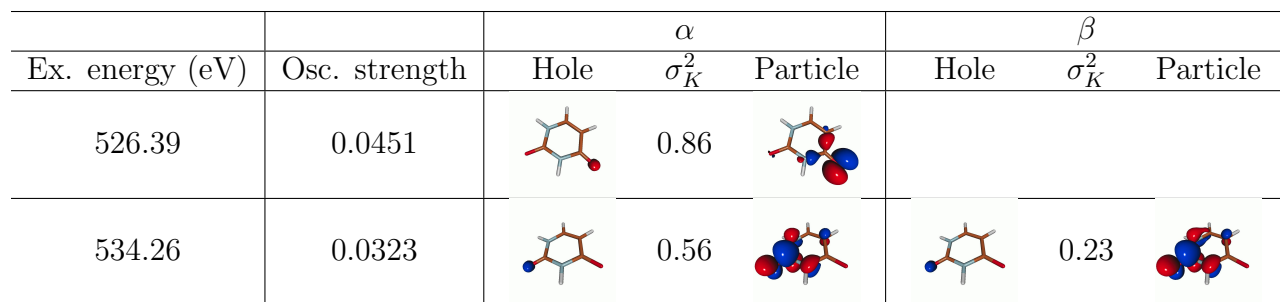 | 0.23         | 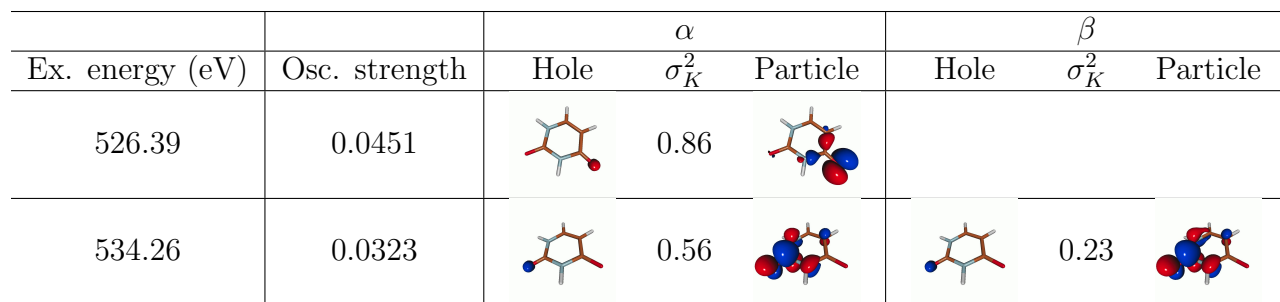 |

Table S20: Uracil. CVS-EOM-CCSD/6-311++G\*\* NTOs of the O<sub>1s</sub> core excitations from the S<sub>1</sub> state at the FC geometry (NTO isosurface is 0.05).

| Ex. energy (eV) | Osc. strength | Hole                                                                                | $\sigma_K^2$ | Particle                                                                              |
|-----------------|---------------|-------------------------------------------------------------------------------------|--------------|---------------------------------------------------------------------------------------|
| 528.02          | 0.0413        | 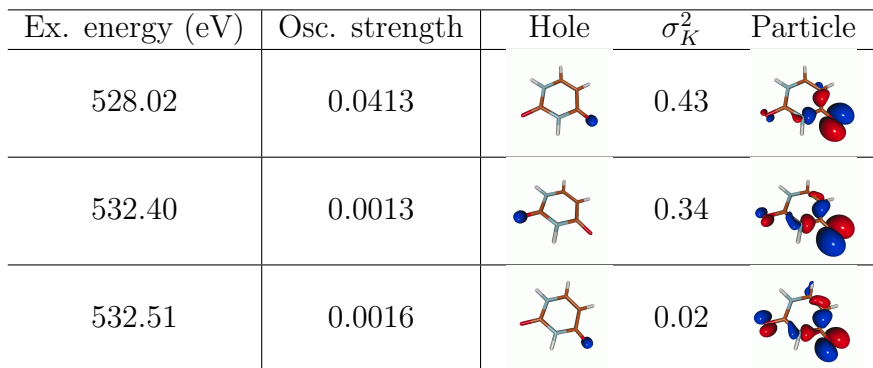 | 0.43         | 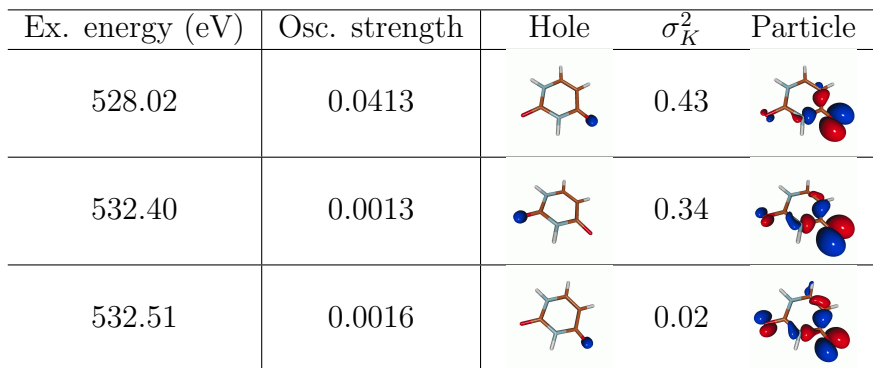 |
| 532.40          | 0.0013        | 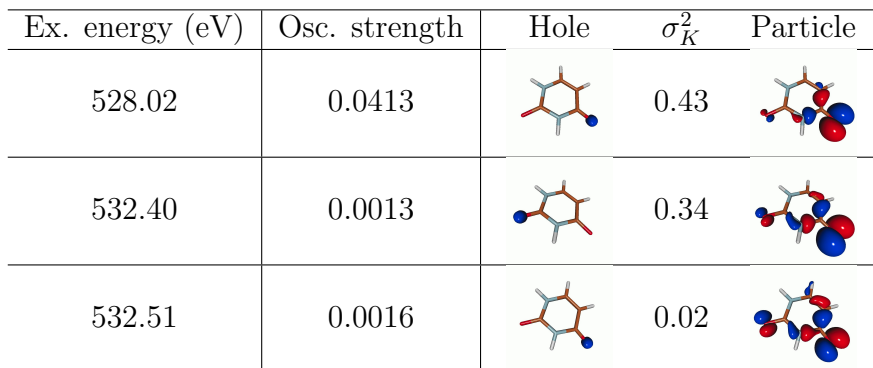 | 0.34         | 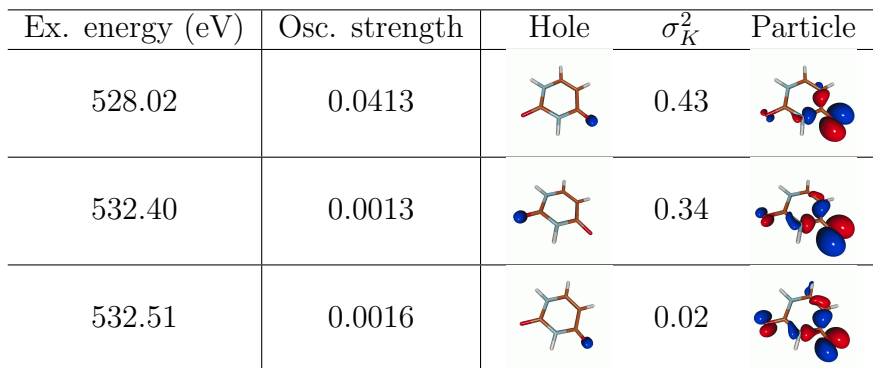 |
| 532.51          | 0.0016        | 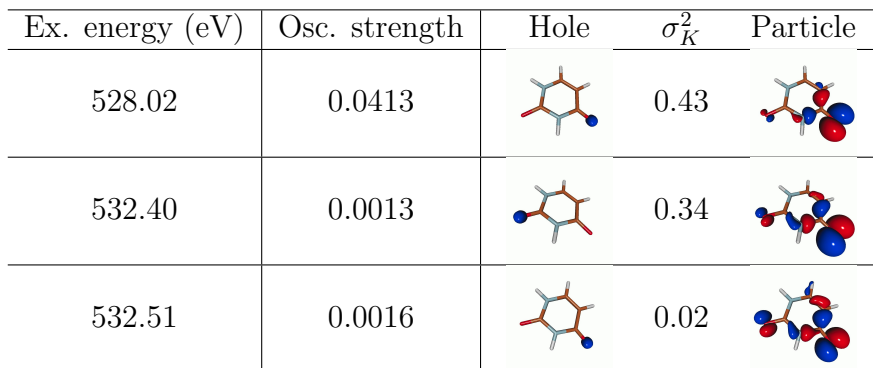 | 0.02         | 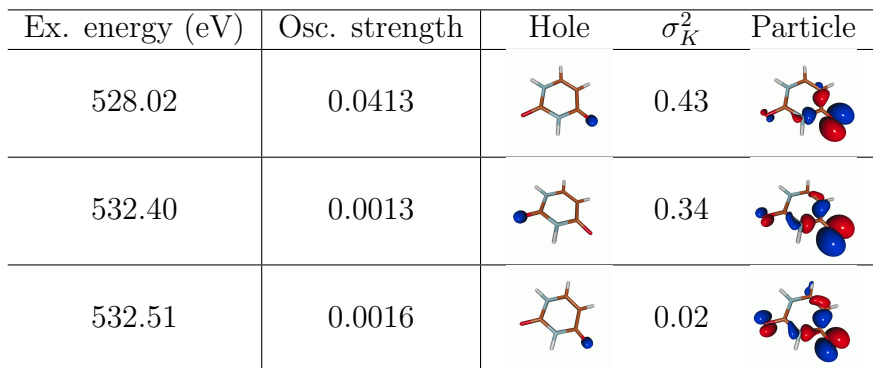 |

Table S21: Uracil. LSOR-CCSD/6-311++G\*\* NTOs of the  $O_{1s}$  core excitations from the  $T_2$  state at the FC geometry (NTO isosurface value = 0.05).

| Ex. energy (eV) | Osc. strength | $\alpha$                                                                          |              |                                                                                    | $\beta$                                                                             |              |                                                                                     |
|-----------------|---------------|-----------------------------------------------------------------------------------|--------------|------------------------------------------------------------------------------------|-------------------------------------------------------------------------------------|--------------|-------------------------------------------------------------------------------------|
|                 |               | Hole                                                                              | $\sigma_K^2$ | Particle                                                                           | Hole                                                                                | $\sigma_K^2$ | Particle                                                                            |
| 526.35          | 0.0448        |                                                                                   |              |                                                                                    | 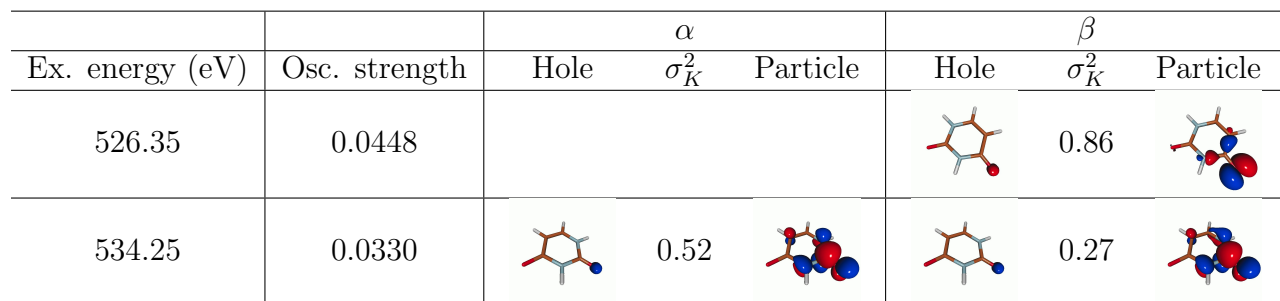 | 0.86         | 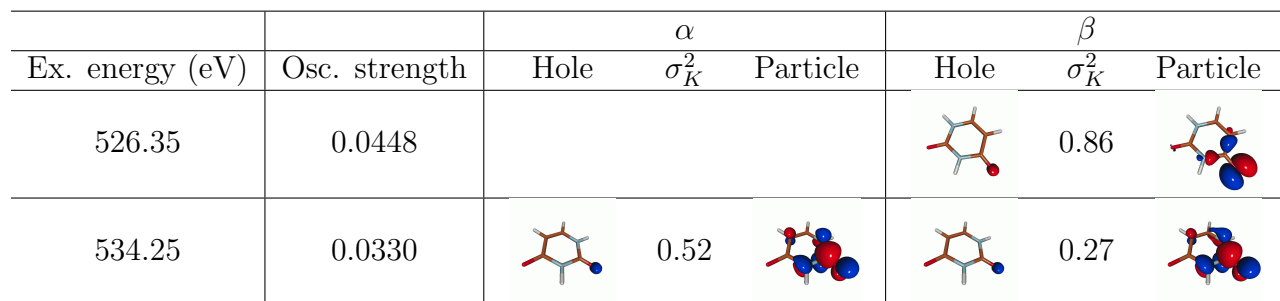 |
| 534.25          | 0.0330        | 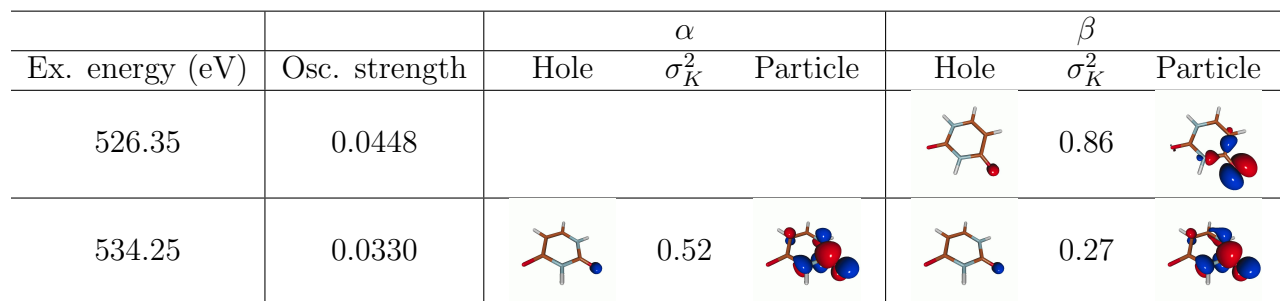 | 0.52         | 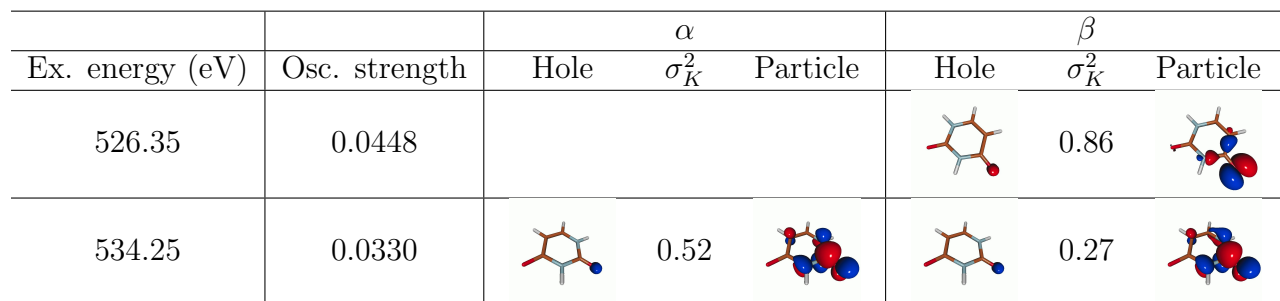 | 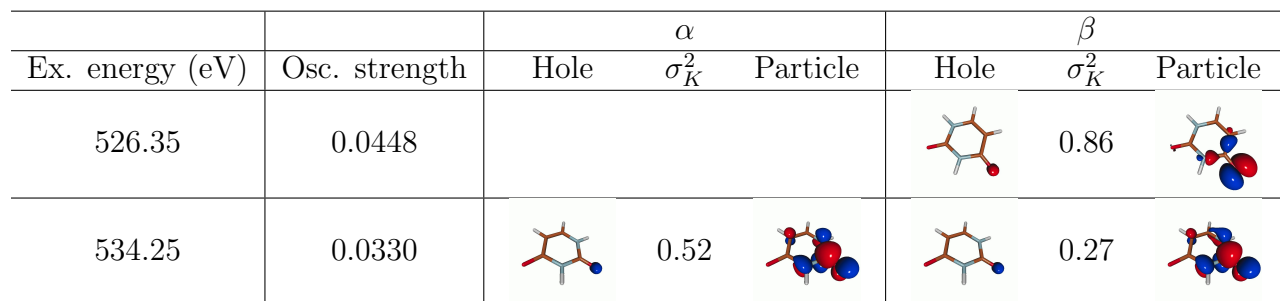 | 0.27         | 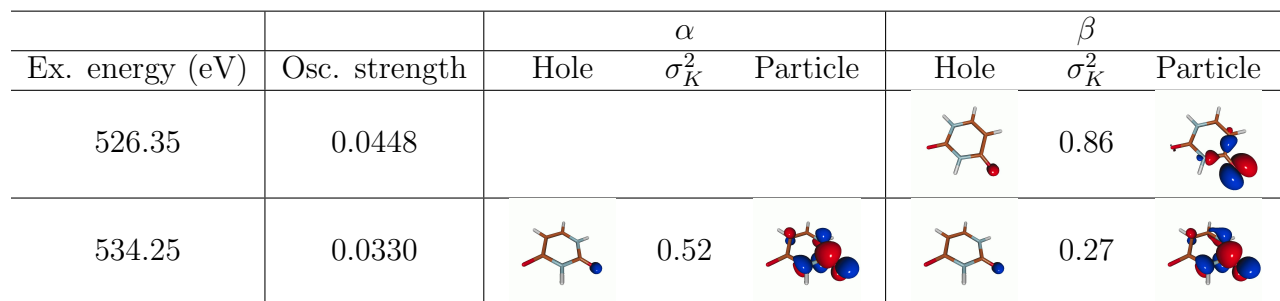 |

Table S22: Uracil. CVS-EOM-CCSD/6-311++G\*\* NTOs of the  $O_{1s}$  core excitations from the  $T_2$  state at the FC geometry (NTO isosurface is 0.05).

| Ex. energy (eV) | Osc. strength | Hole                                                                                | $\sigma_K^2$ | Particle                                                                              |
|-----------------|---------------|-------------------------------------------------------------------------------------|--------------|---------------------------------------------------------------------------------------|
| 527.74          | 0.0418        | 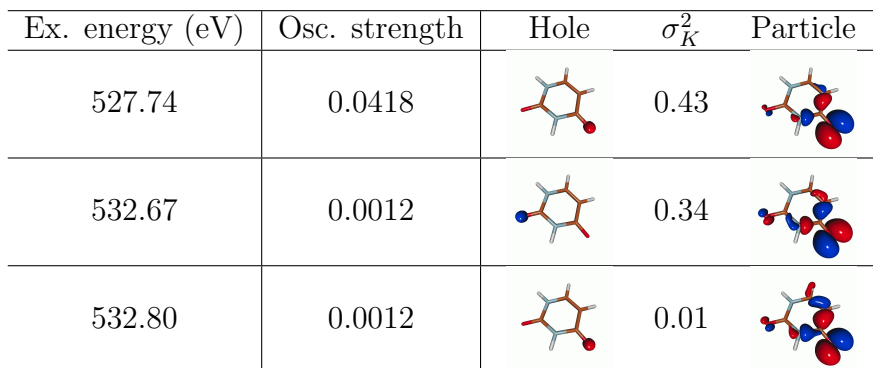 | 0.43         | 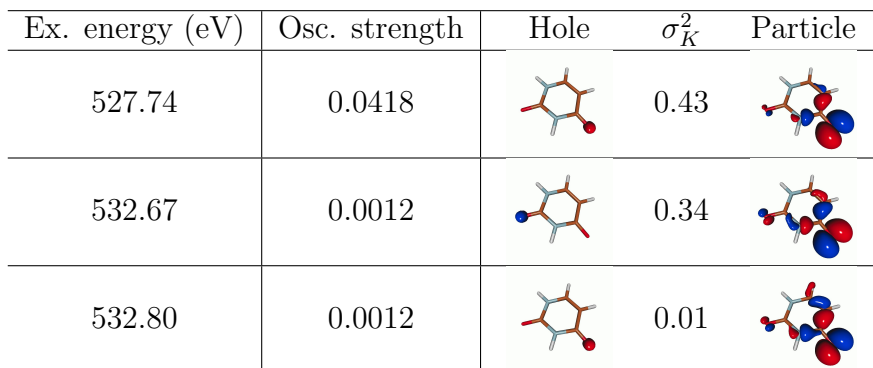 |
| 532.67          | 0.0012        | 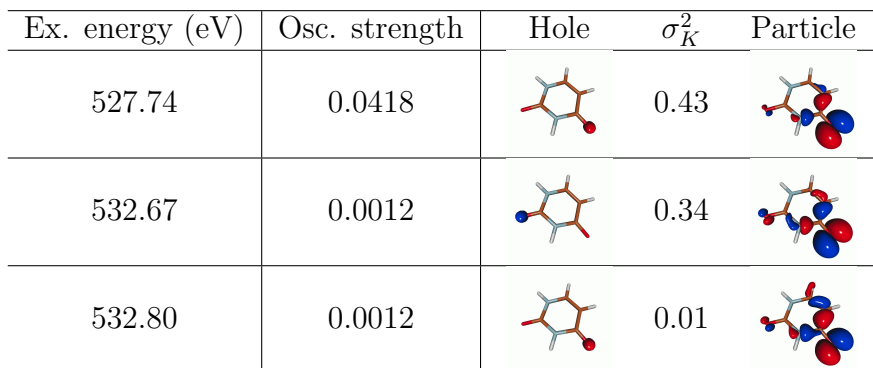 | 0.34         | 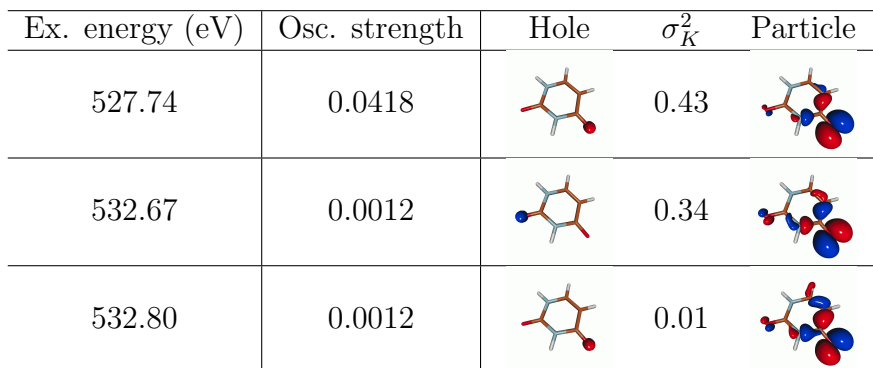 |
| 532.80          | 0.0012        | 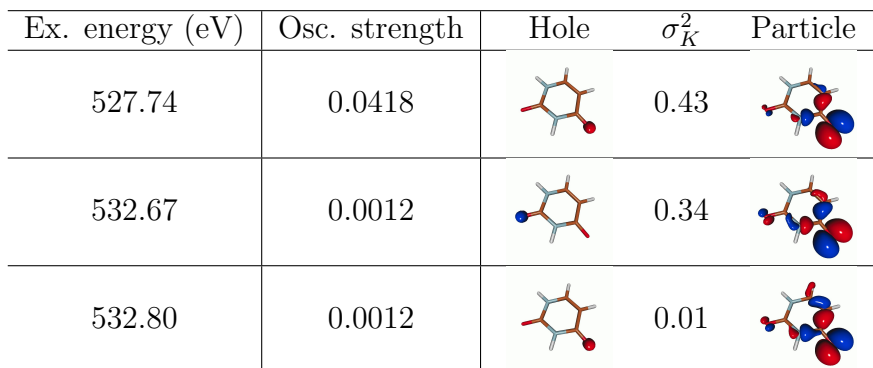 | 0.01         | 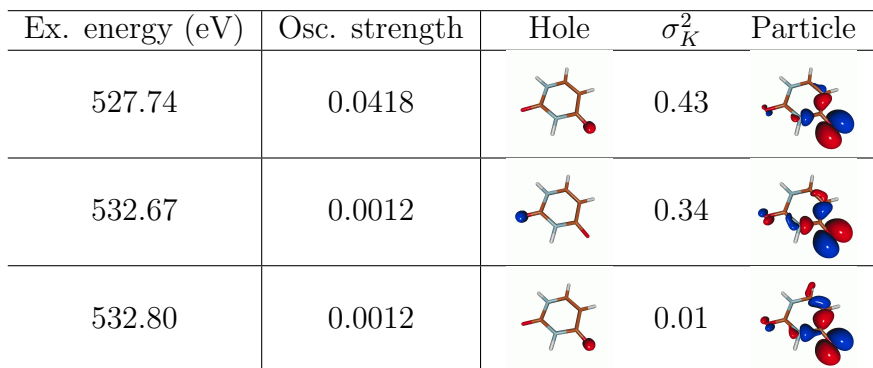 |

Table S23: Uracil. LSOR-CCSD/6-311++G\*\* NTOs of the O<sub>1s</sub> core excitations from the S<sub>2</sub> state at the FC geometry (NTO isosurface value = 0.05).

| Ex. energy (eV) | Osc. strength | $\alpha$                                                                           |              |                                                                                     | $\beta$                                                                             |              |                                                                                     |
|-----------------|---------------|------------------------------------------------------------------------------------|--------------|-------------------------------------------------------------------------------------|-------------------------------------------------------------------------------------|--------------|-------------------------------------------------------------------------------------|
|                 |               | Hole                                                                               | $\sigma_K^2$ | Particle                                                                            | Hole                                                                                | $\sigma_K^2$ | Particle                                                                            |
| 530.16          | 0.0102        | 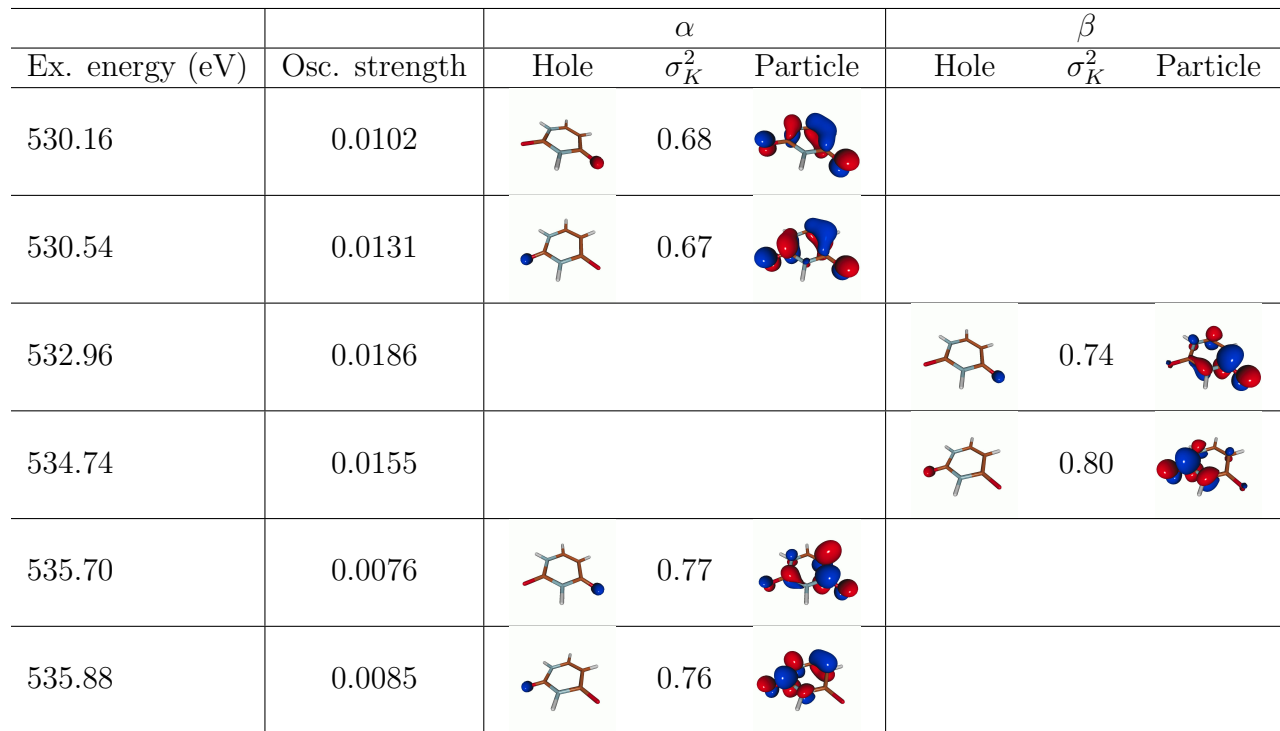  | 0.68         | 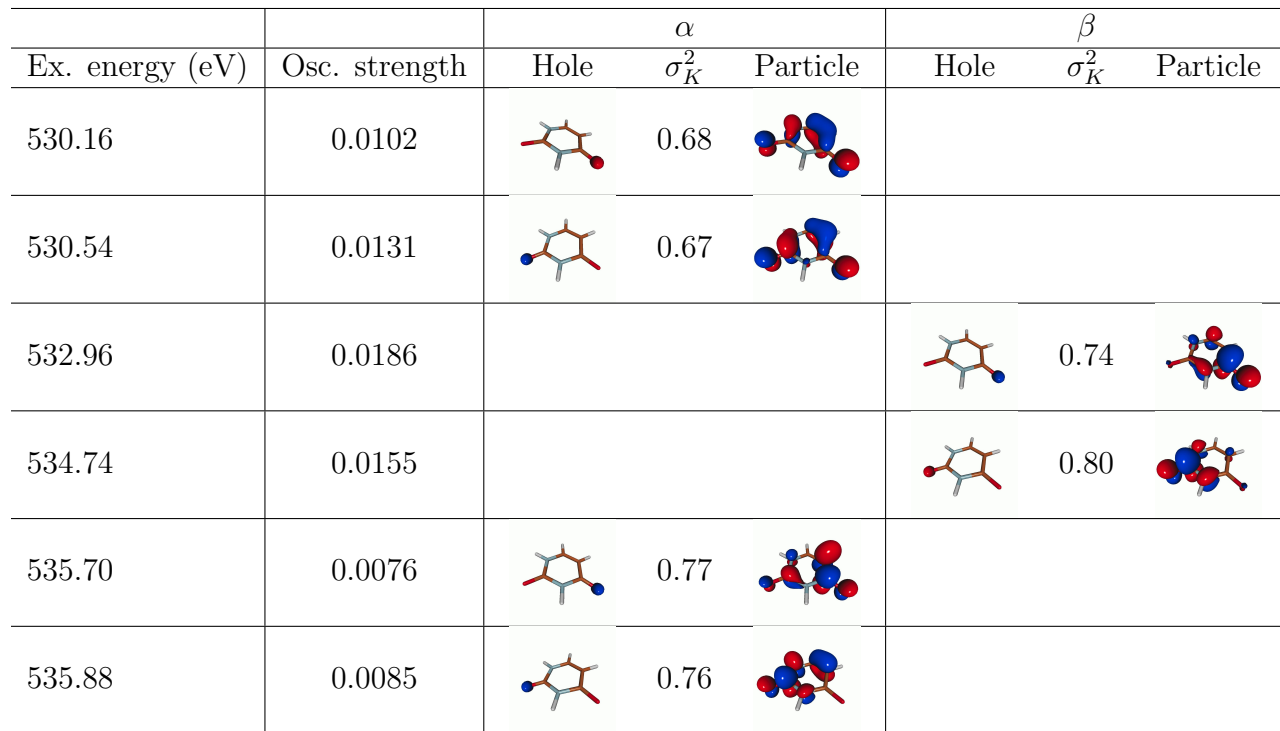  |                                                                                     |              |                                                                                     |
| 530.54          | 0.0131        | 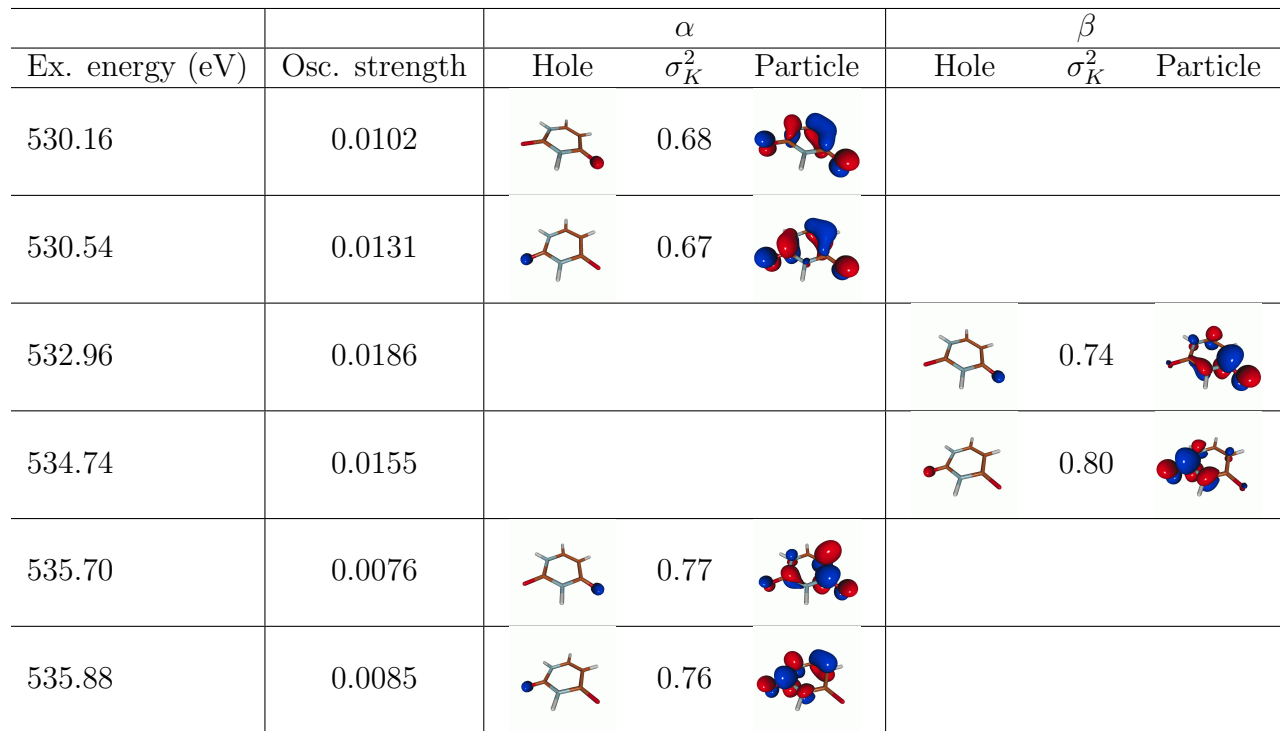  | 0.67         | 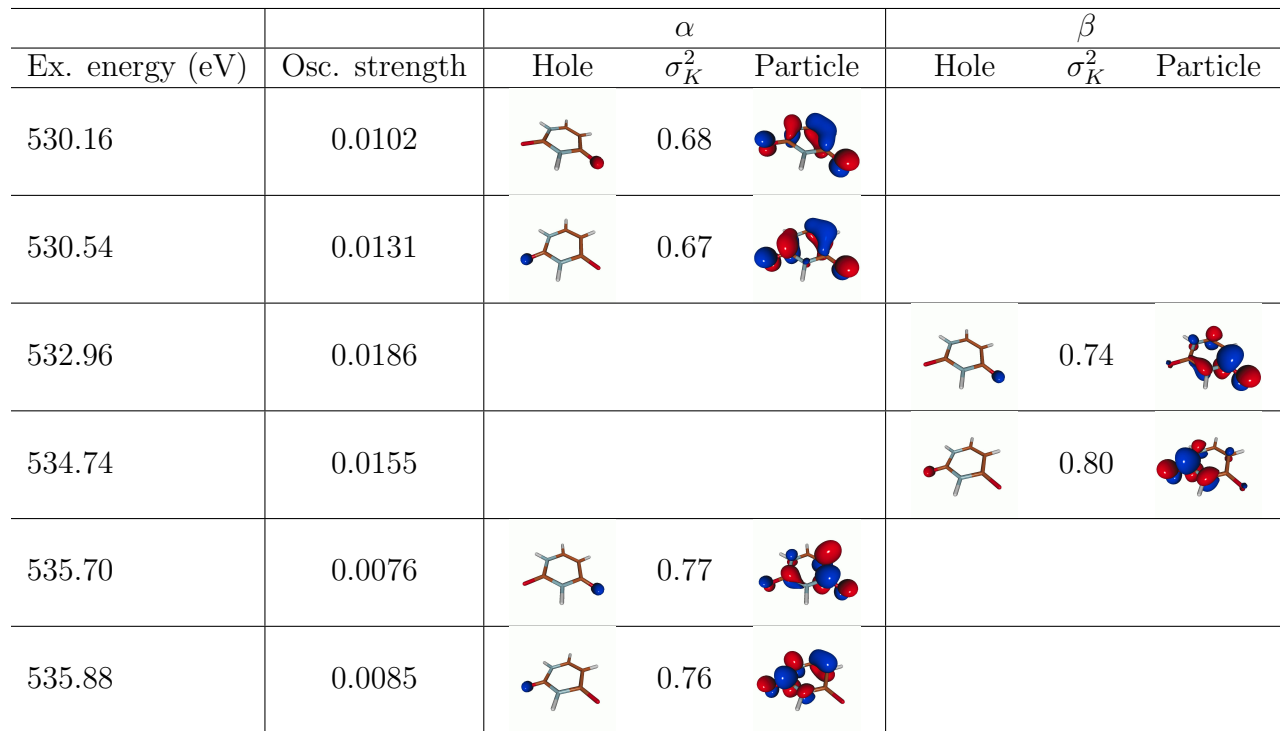  |                                                                                     |              |                                                                                     |
| 532.96          | 0.0186        |                                                                                    |              |                                                                                     | 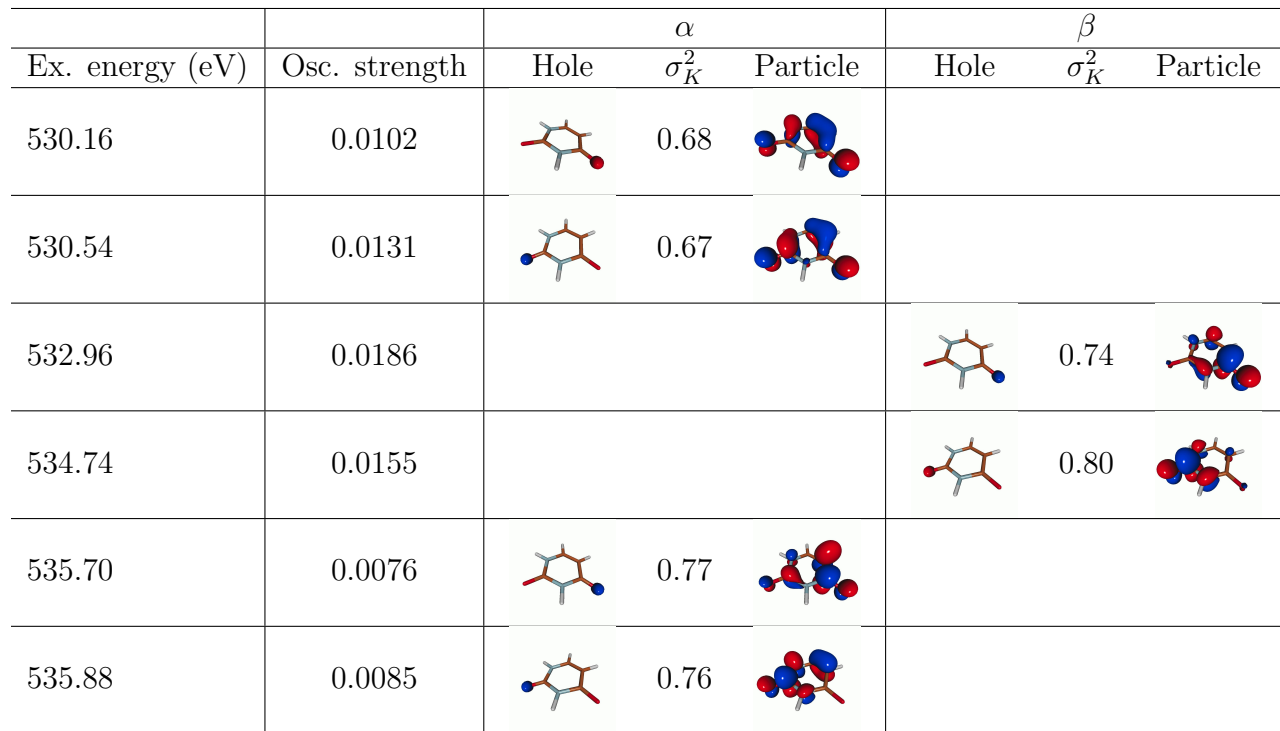 | 0.74         | 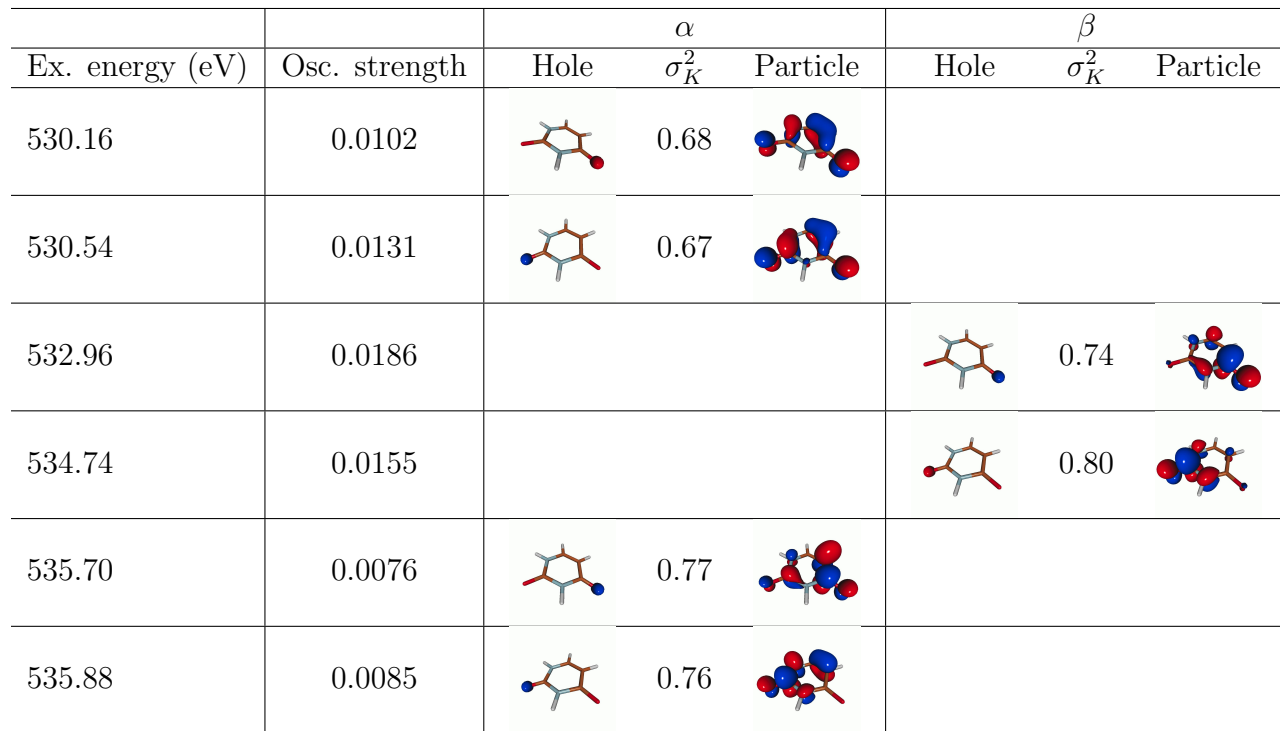 |
| 534.74          | 0.0155        |                                                                                    |              |                                                                                     | 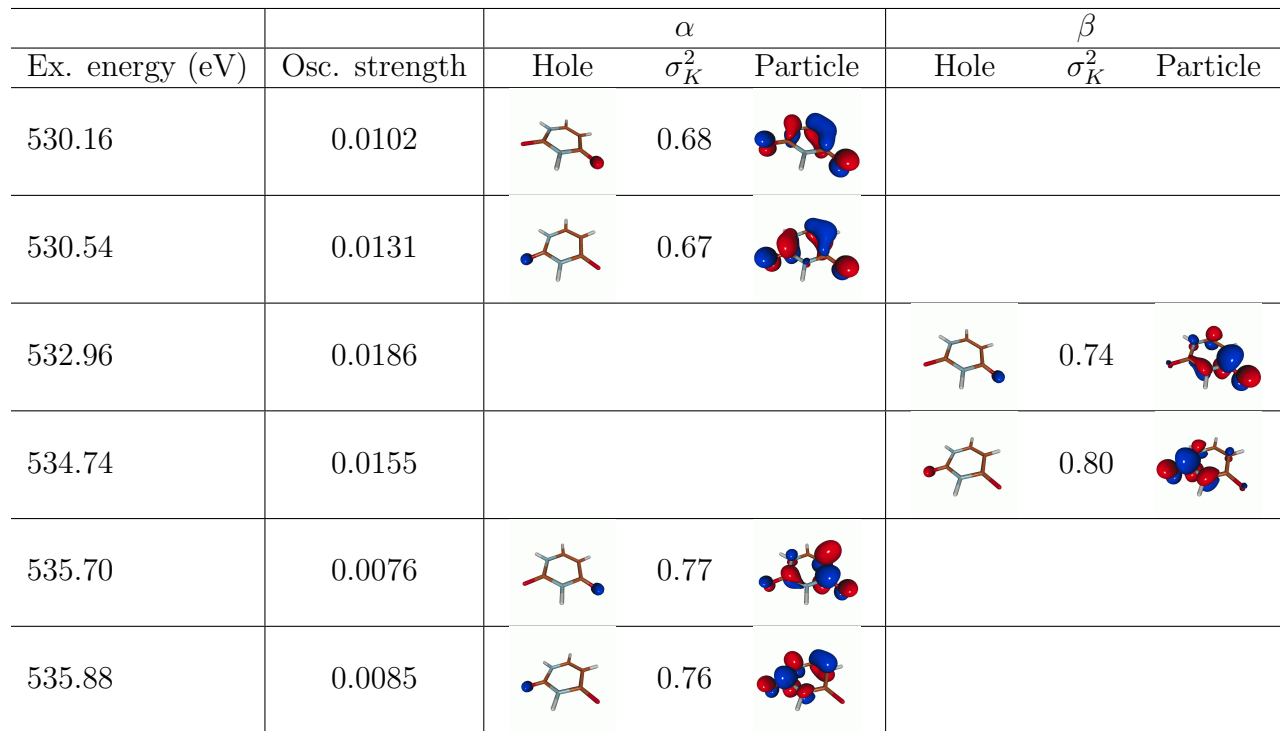 | 0.80         | 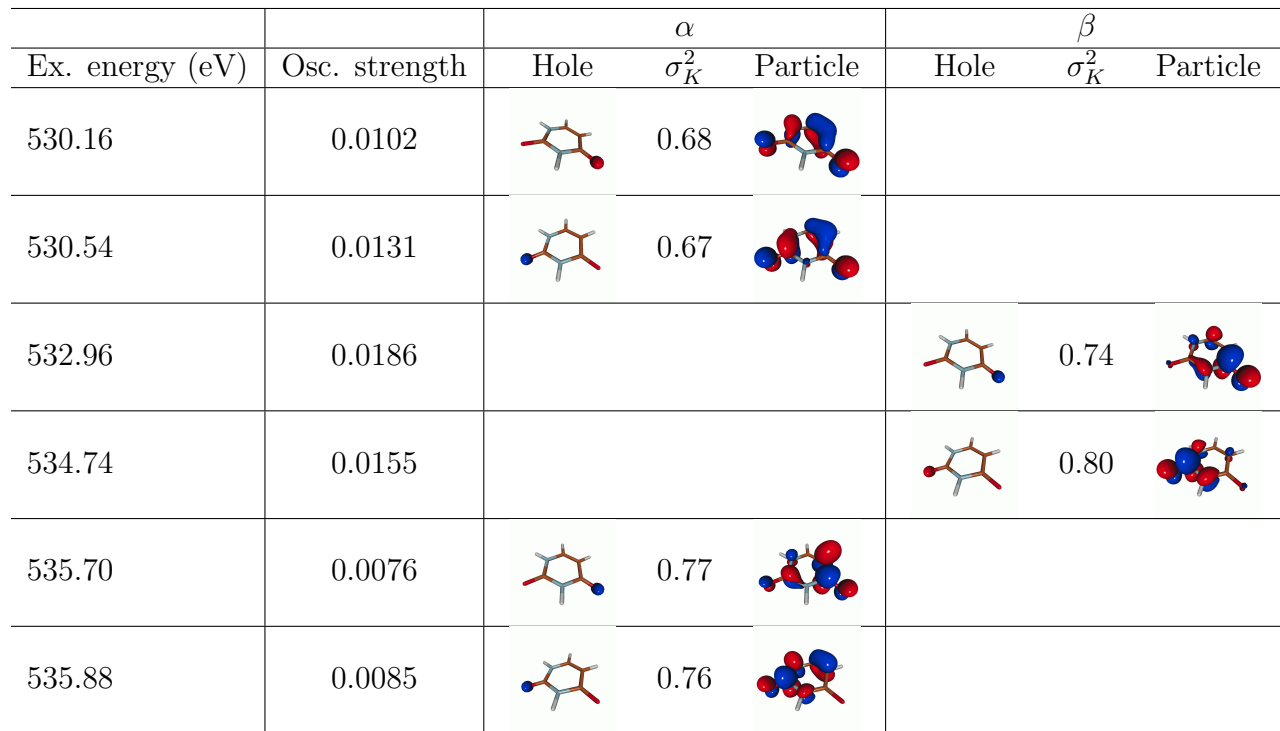 |
| 535.70          | 0.0076        | 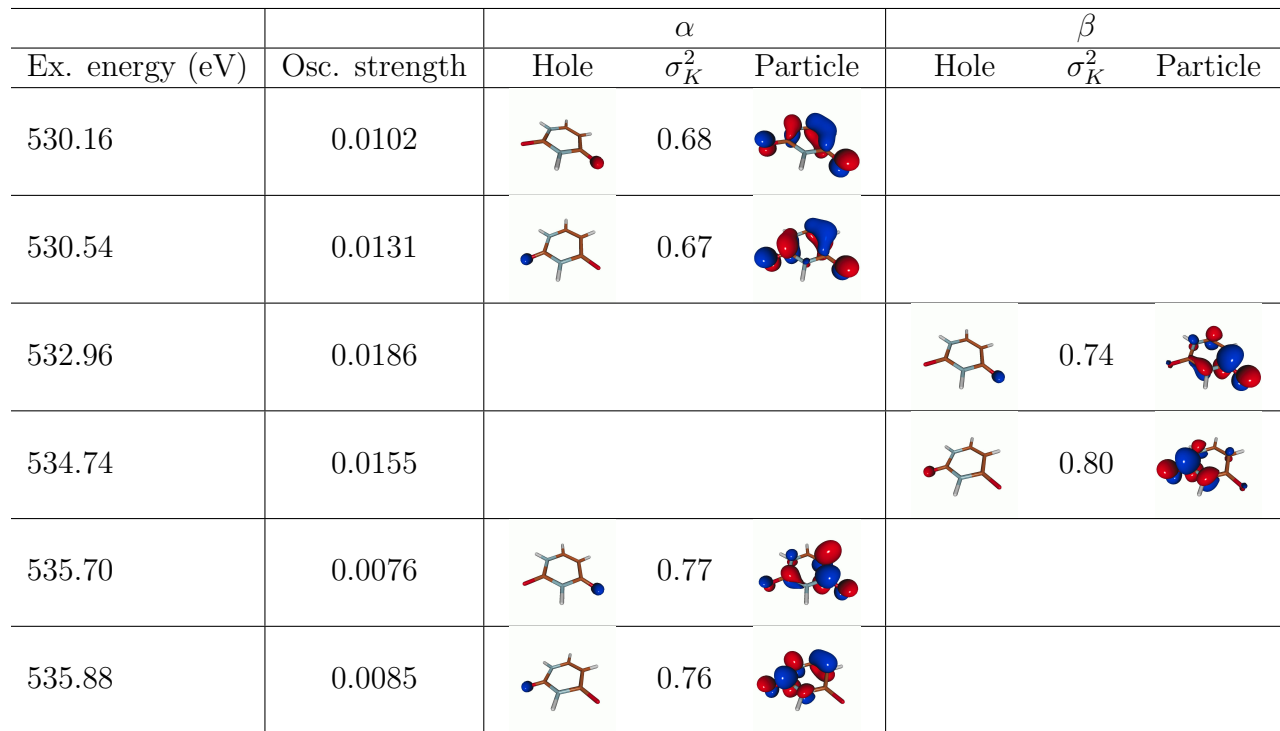  | 0.77         | 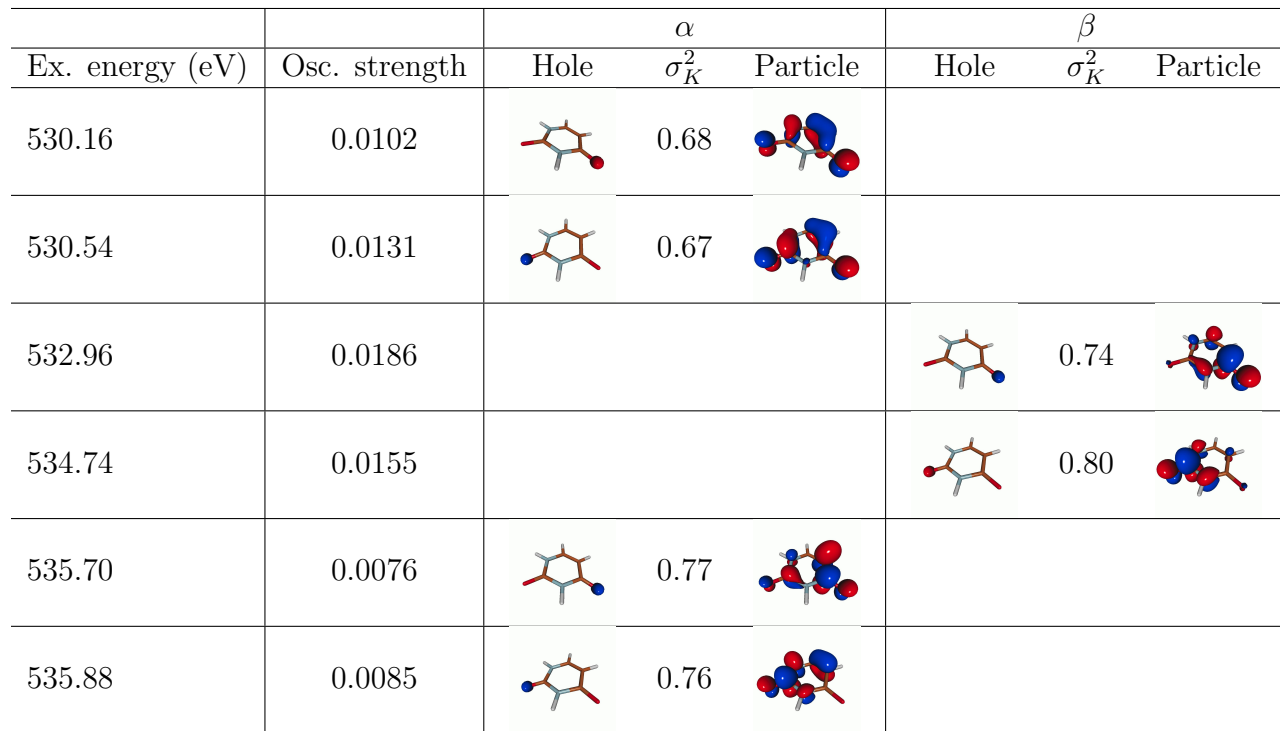  |                                                                                     |              |                                                                                     |
| 535.88          | 0.0085        | 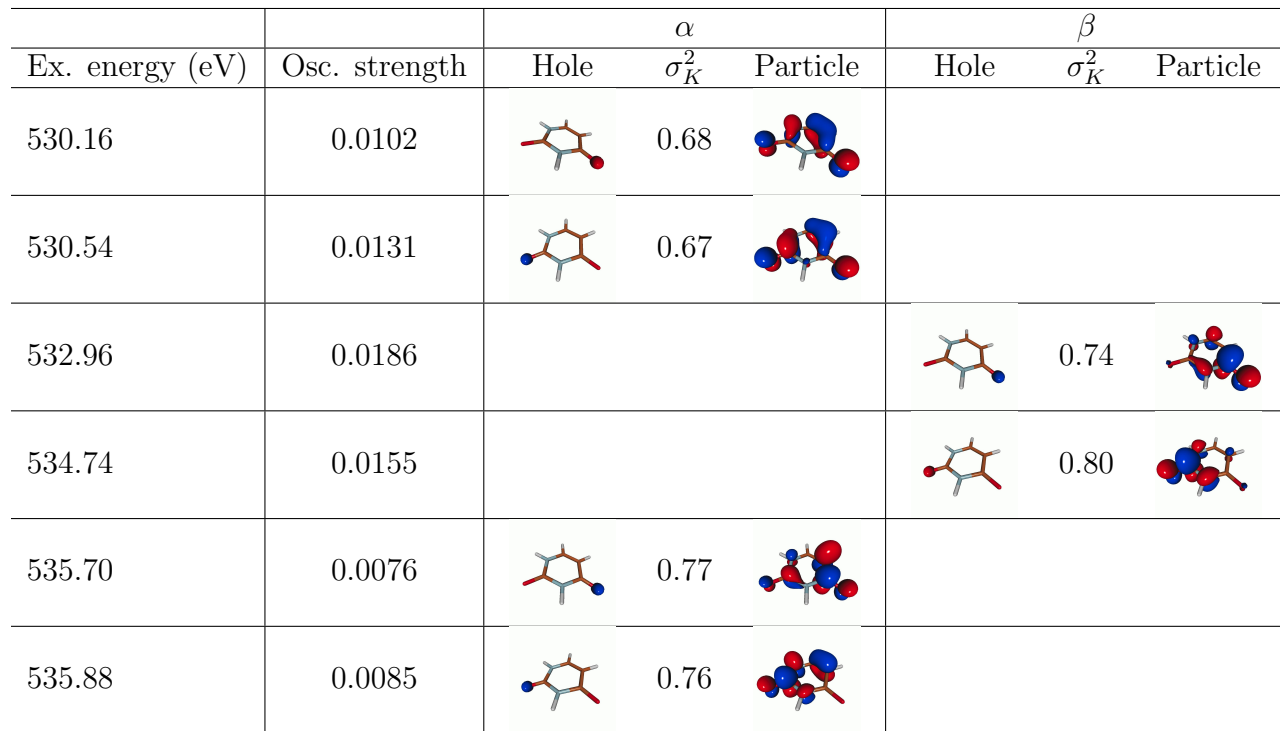 | 0.76         | 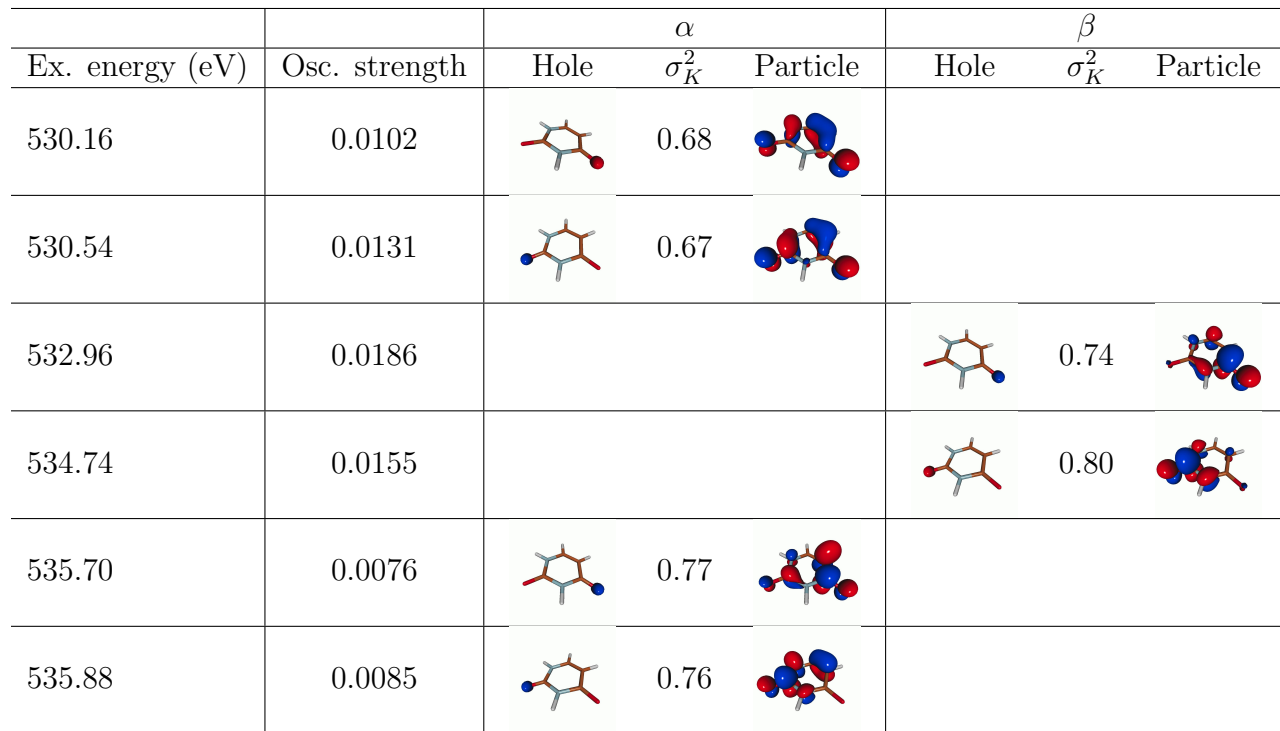 |                                                                                     |              |                                                                                     |

Table S24: Uracil. CVS-EOM-CCSD/6-311++G\*\* NTOs of the O<sub>1s</sub> core excitations from the S<sub>2</sub> state at the FC geometry (NTO isosurface is 0.05).

| Ex. energy (eV) | Osc. strength | Hole                                                                                | $\sigma_K^2$ | Particle                                                                              |
|-----------------|---------------|-------------------------------------------------------------------------------------|--------------|---------------------------------------------------------------------------------------|
| 527.50          | 0.0024        | 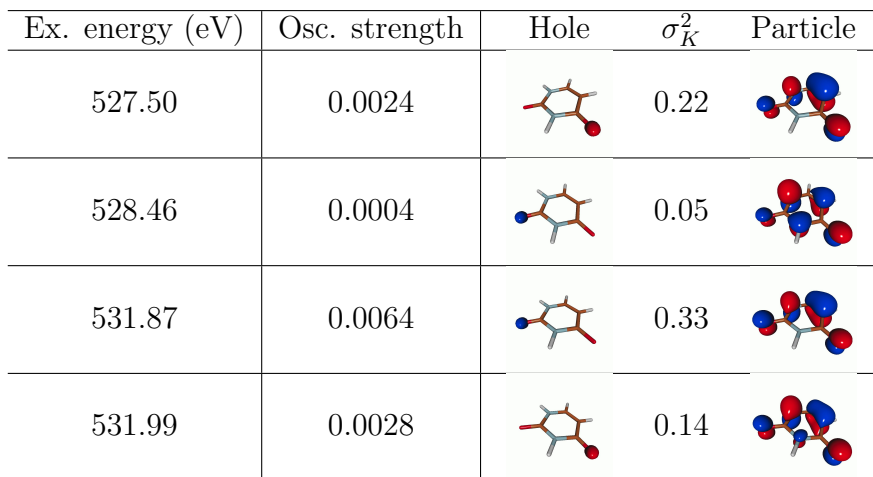 | 0.22         | 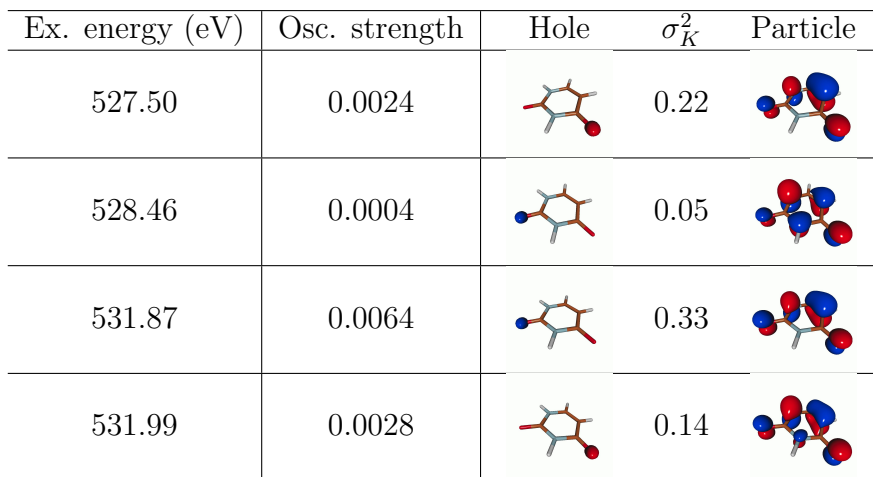 |
| 528.46          | 0.0004        | 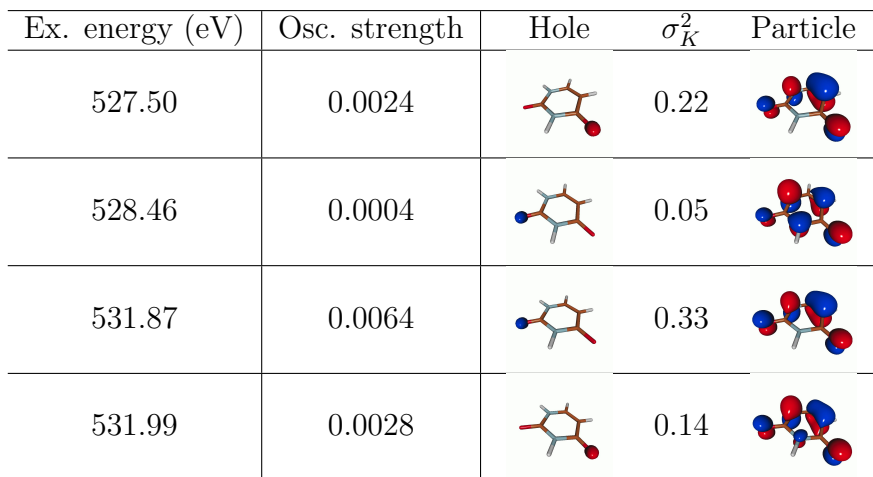 | 0.05         | 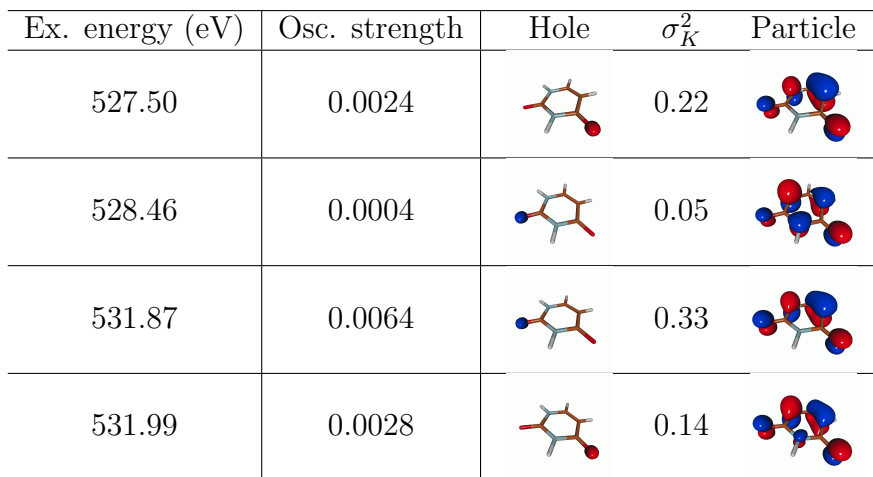 |
| 531.87          | 0.0064        | 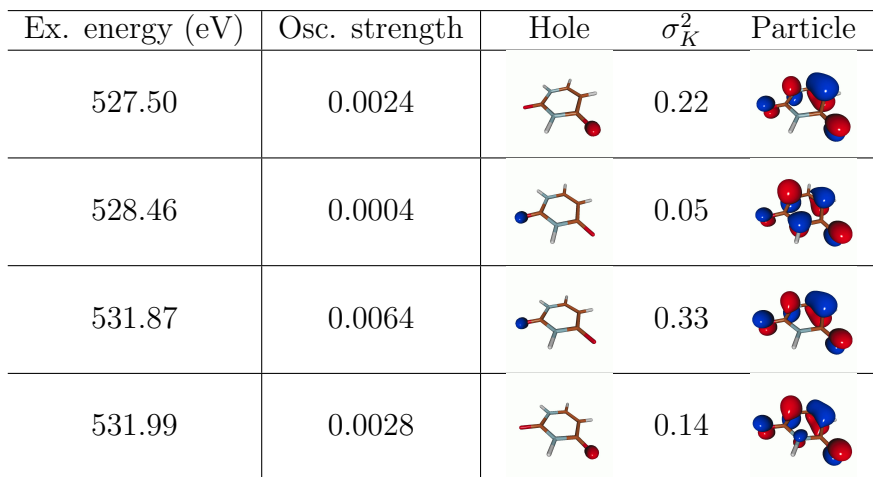 | 0.33         | 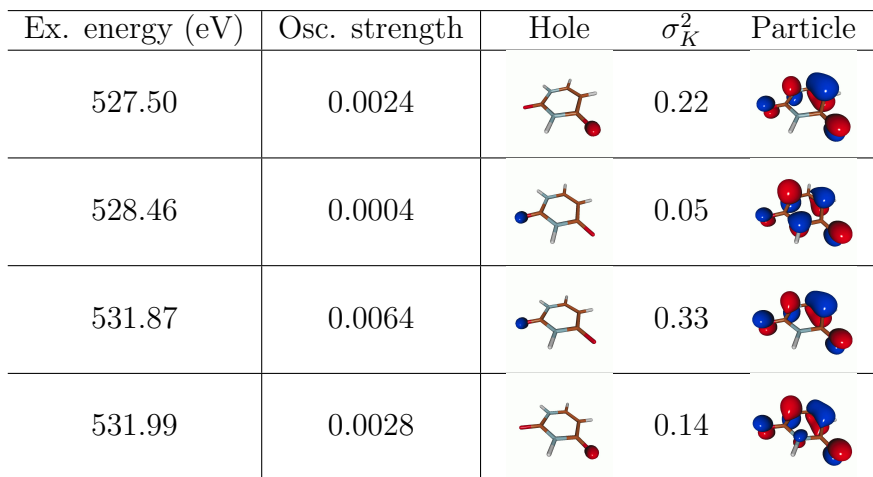 |
| 531.99          | 0.0028        | 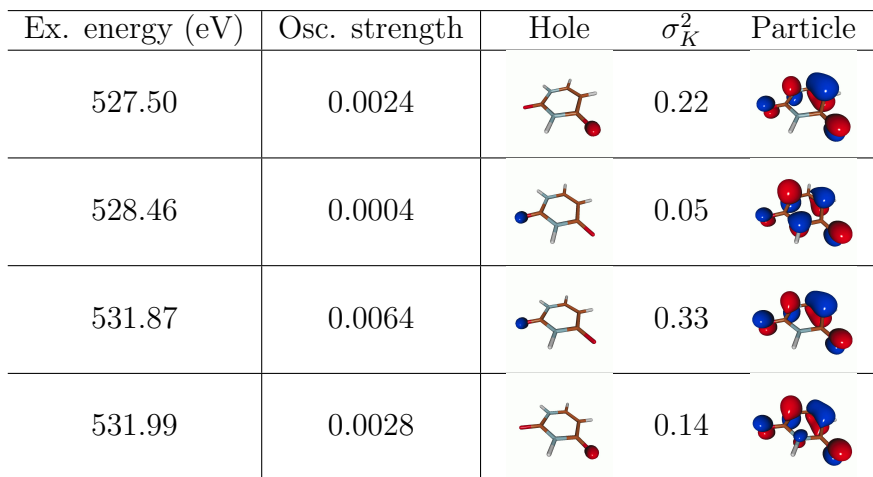 | 0.14         | 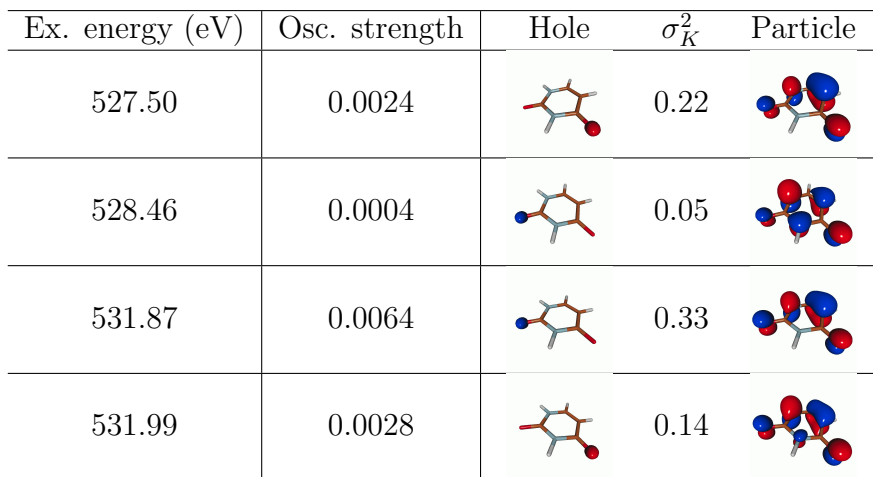 |

Table S25: Uracil. LSOR-CCSD/6-311++G\*\* NTOs of the O<sub>1s</sub> core excitations from the T<sub>1</sub> state at the FC geometry (NTO isosurface is 0.05).

| Ex. energy (eV) | Osc. strength | $\alpha$                                                                          |              |                                                                                    | $\beta$                                                                              |              |                                                                                      |
|-----------------|---------------|-----------------------------------------------------------------------------------|--------------|------------------------------------------------------------------------------------|--------------------------------------------------------------------------------------|--------------|--------------------------------------------------------------------------------------|
|                 |               | Hole                                                                              | $\sigma_K^2$ | Particle                                                                           | Hole                                                                                 | $\sigma_K^2$ | Particle                                                                             |
| 529.81          | 0.0212        |                                                                                   |              |                                                                                    | 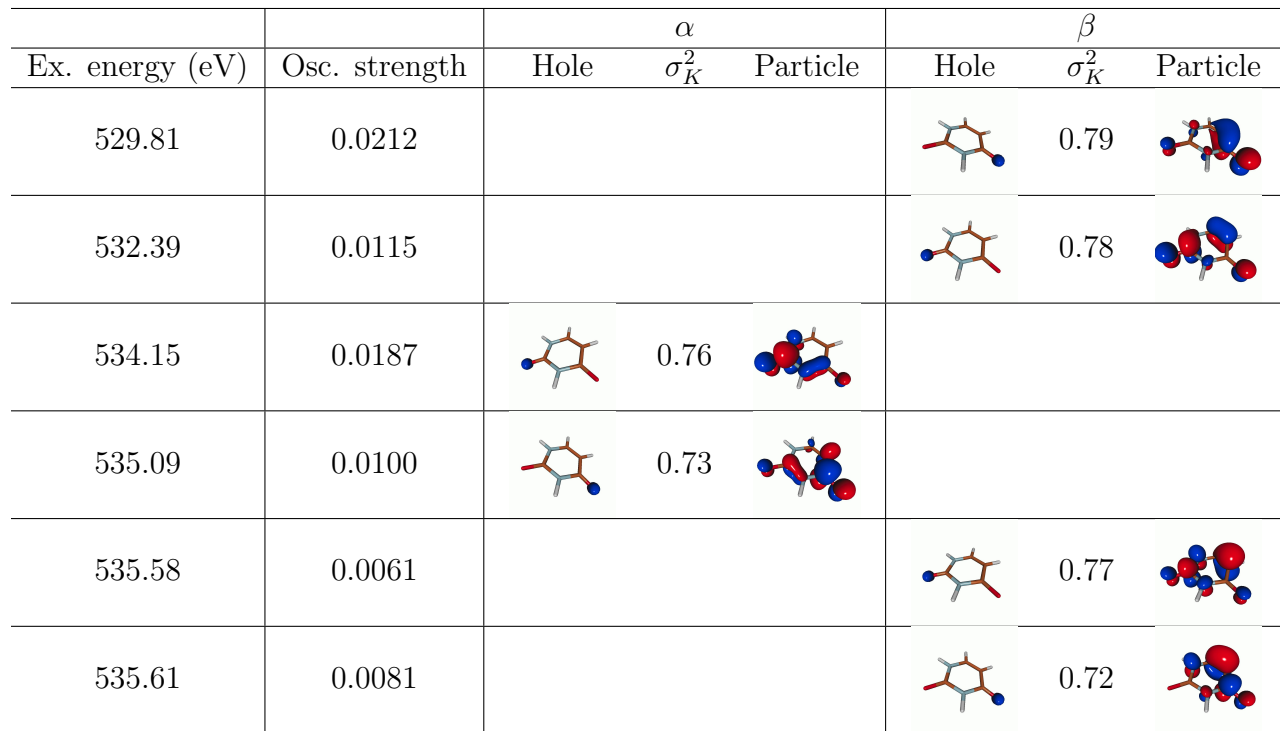  | 0.79         | 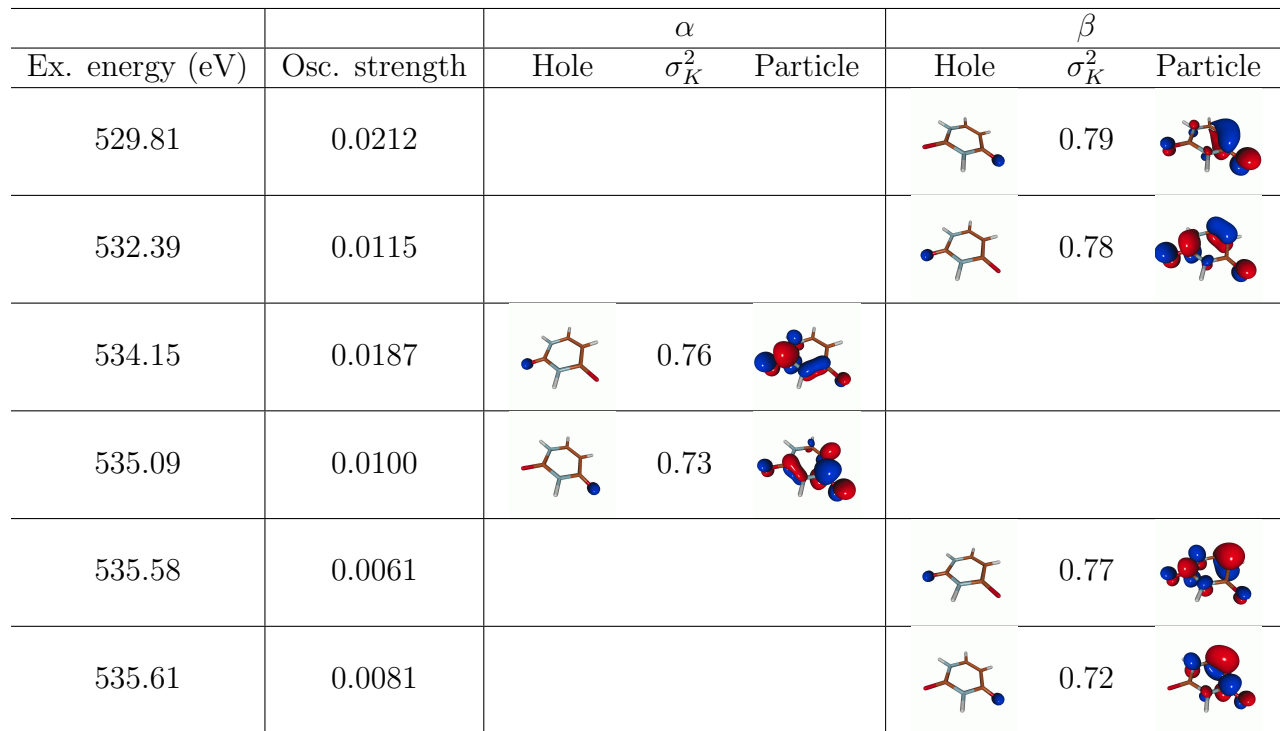  |
| 532.39          | 0.0115        |                                                                                   |              |                                                                                    | 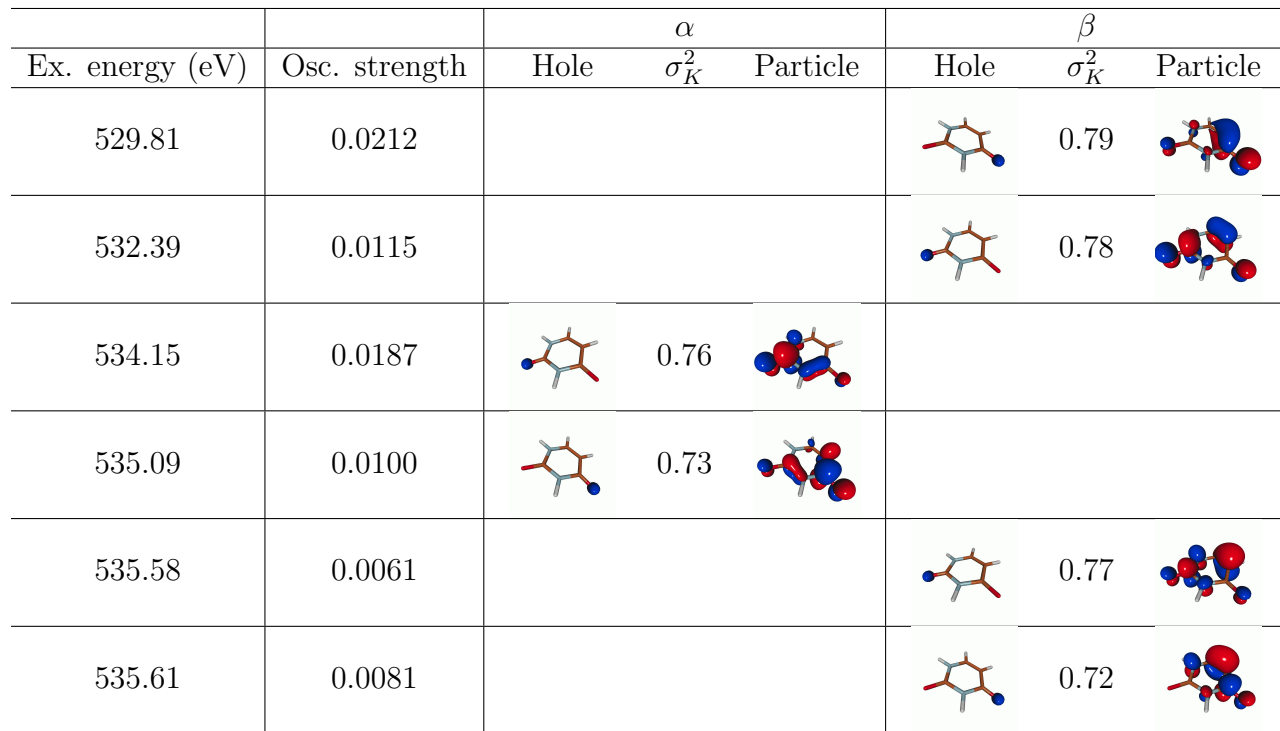  | 0.78         | 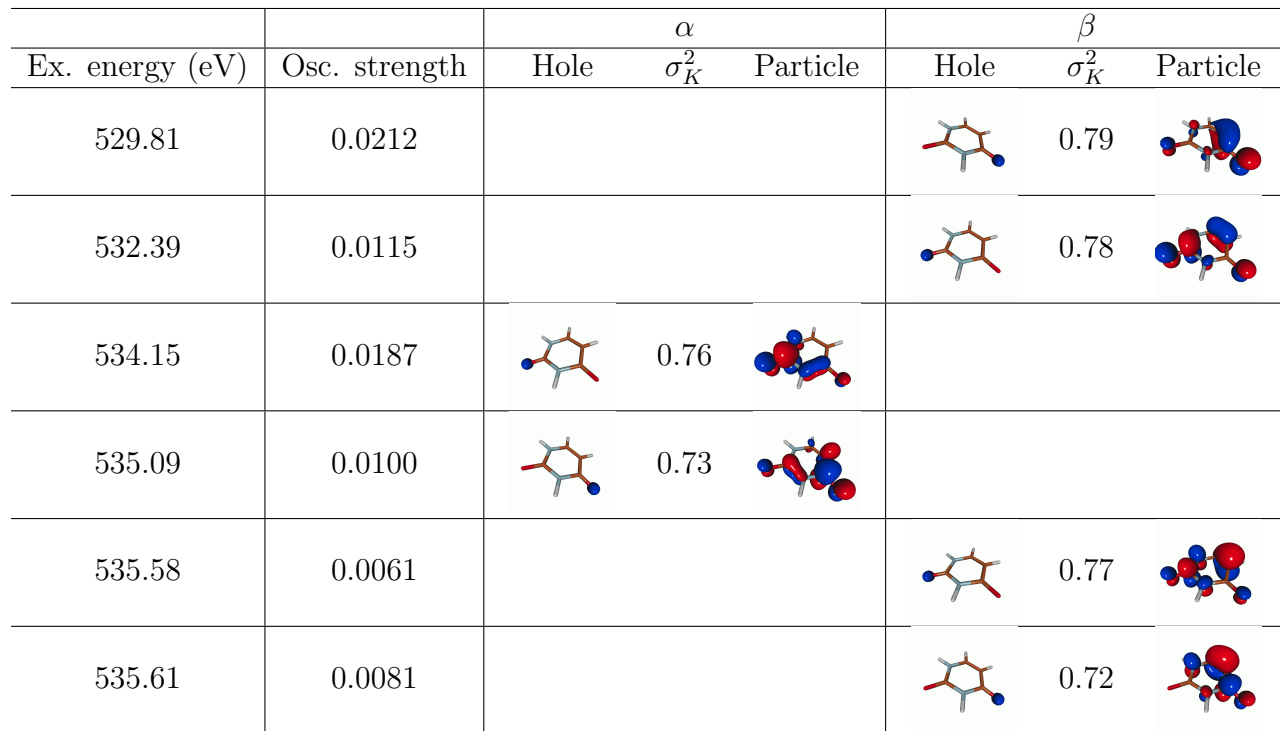  |
| 534.15          | 0.0187        | 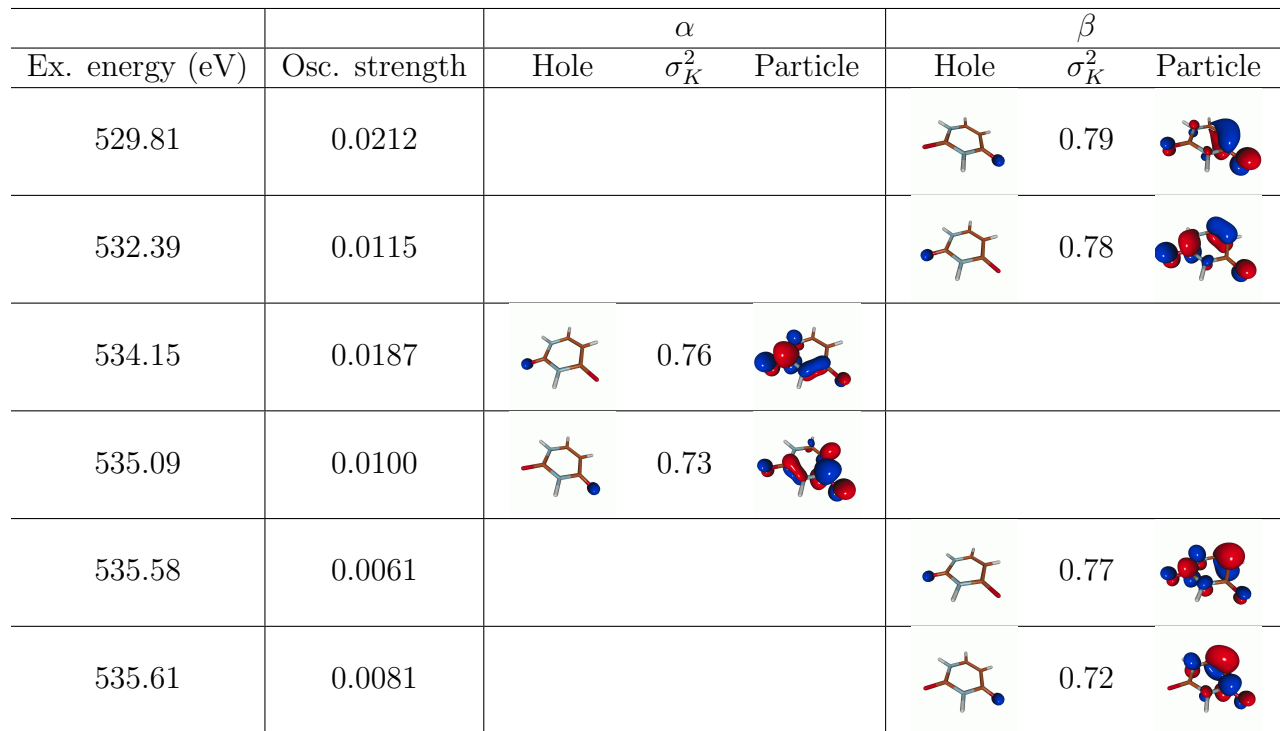 | 0.76         | 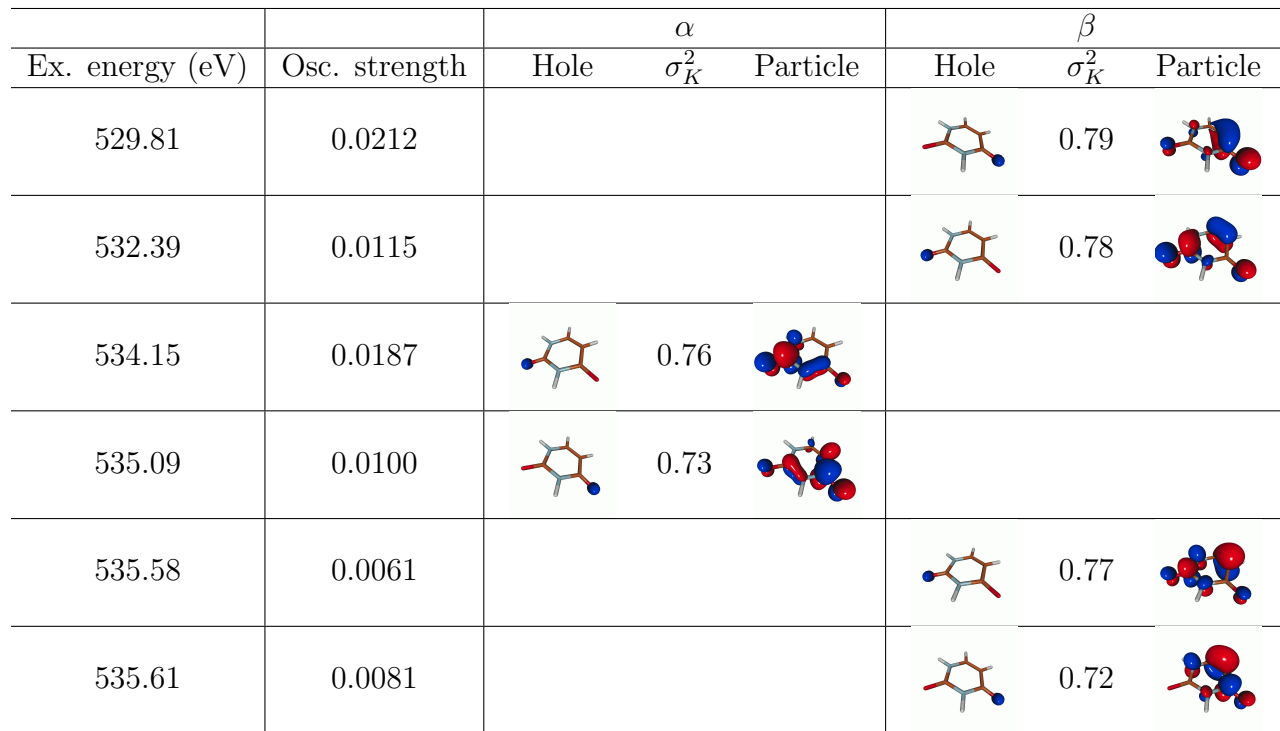 |                                                                                      |              |                                                                                      |
| 535.09          | 0.0100        | 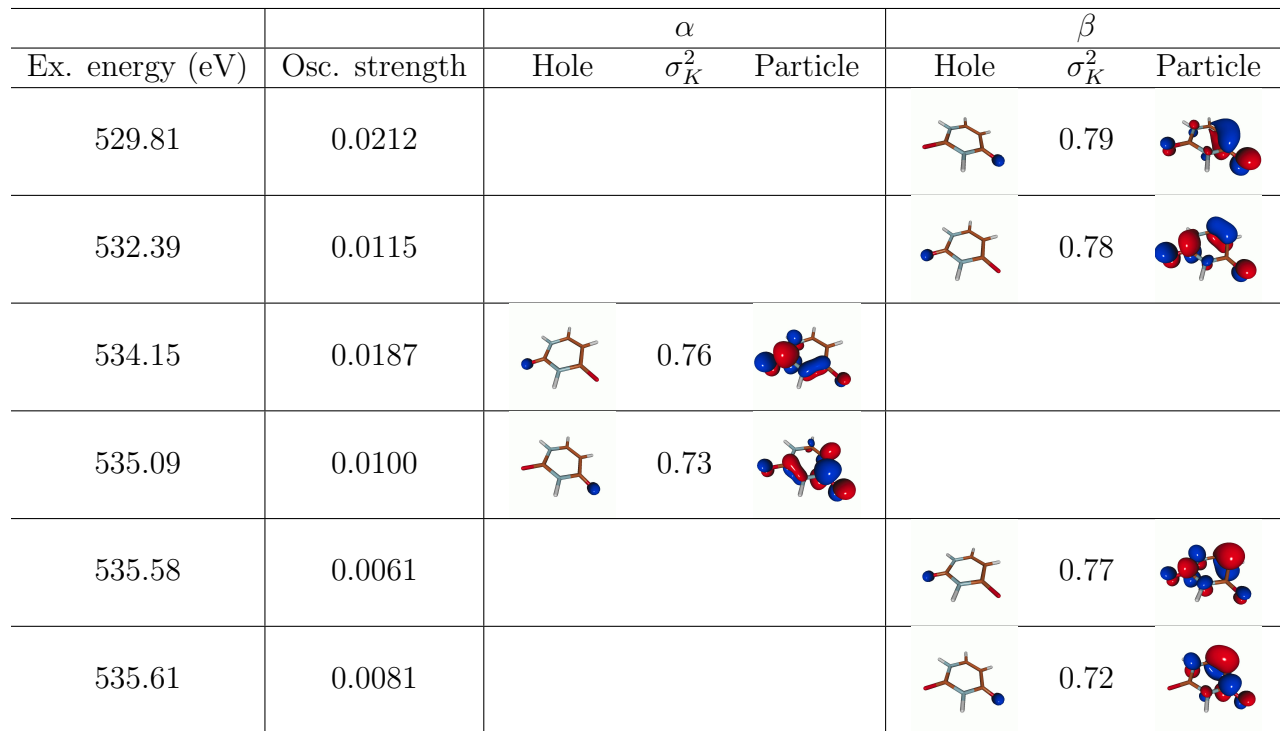 | 0.73         | 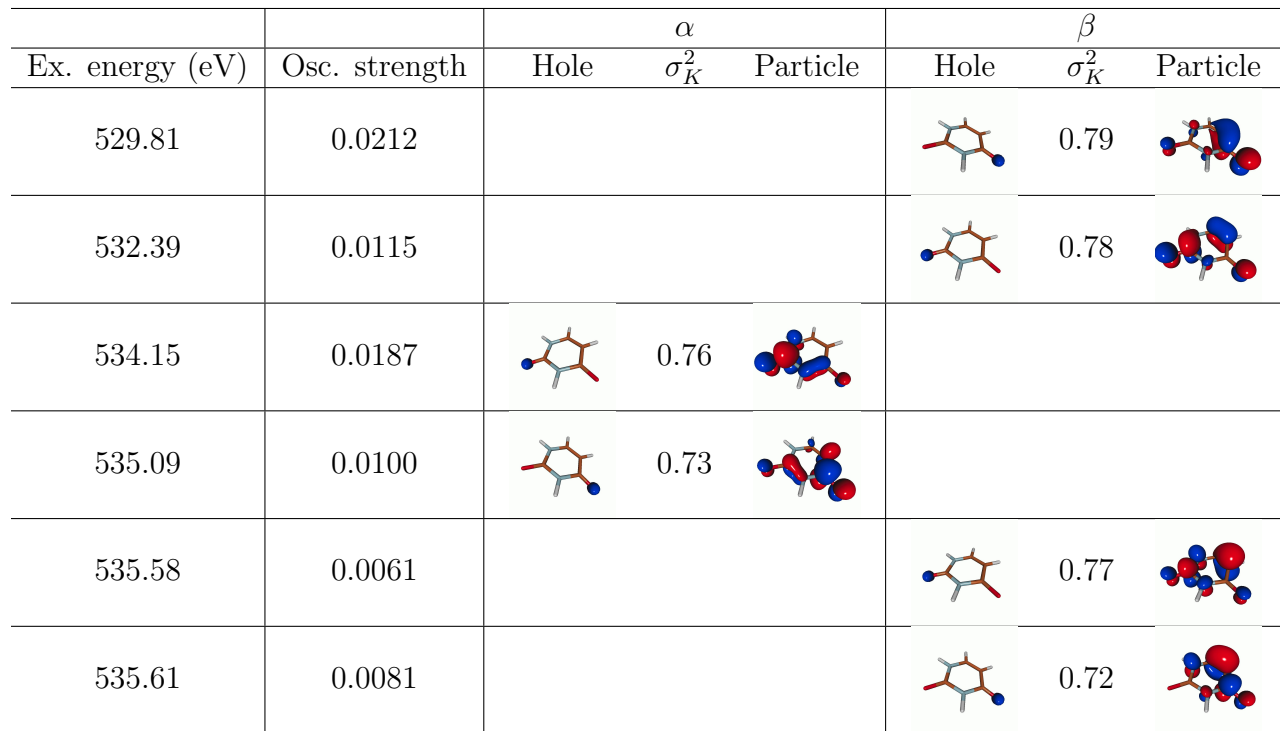 |                                                                                      |              |                                                                                      |
| 535.58          | 0.0061        |                                                                                   |              |                                                                                    | 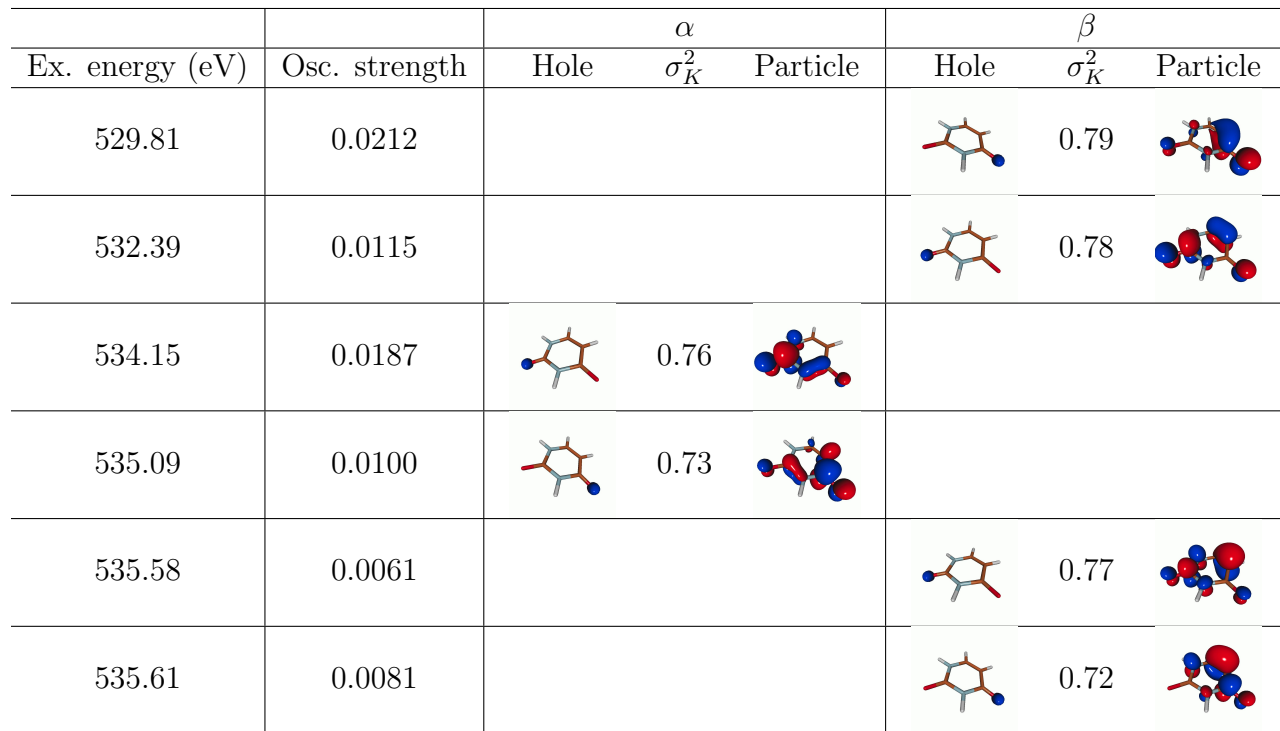  | 0.77         | 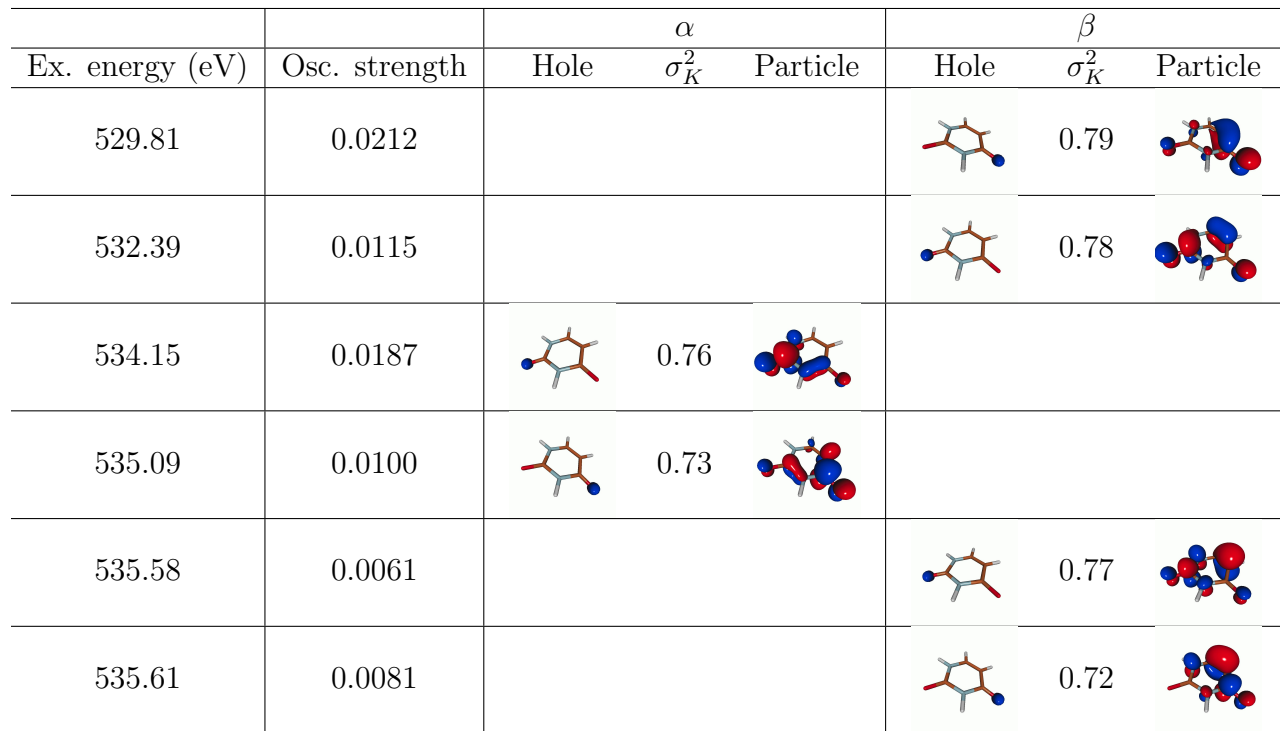  |
| 535.61          | 0.0081        |                                                                                   |              |                                                                                    | 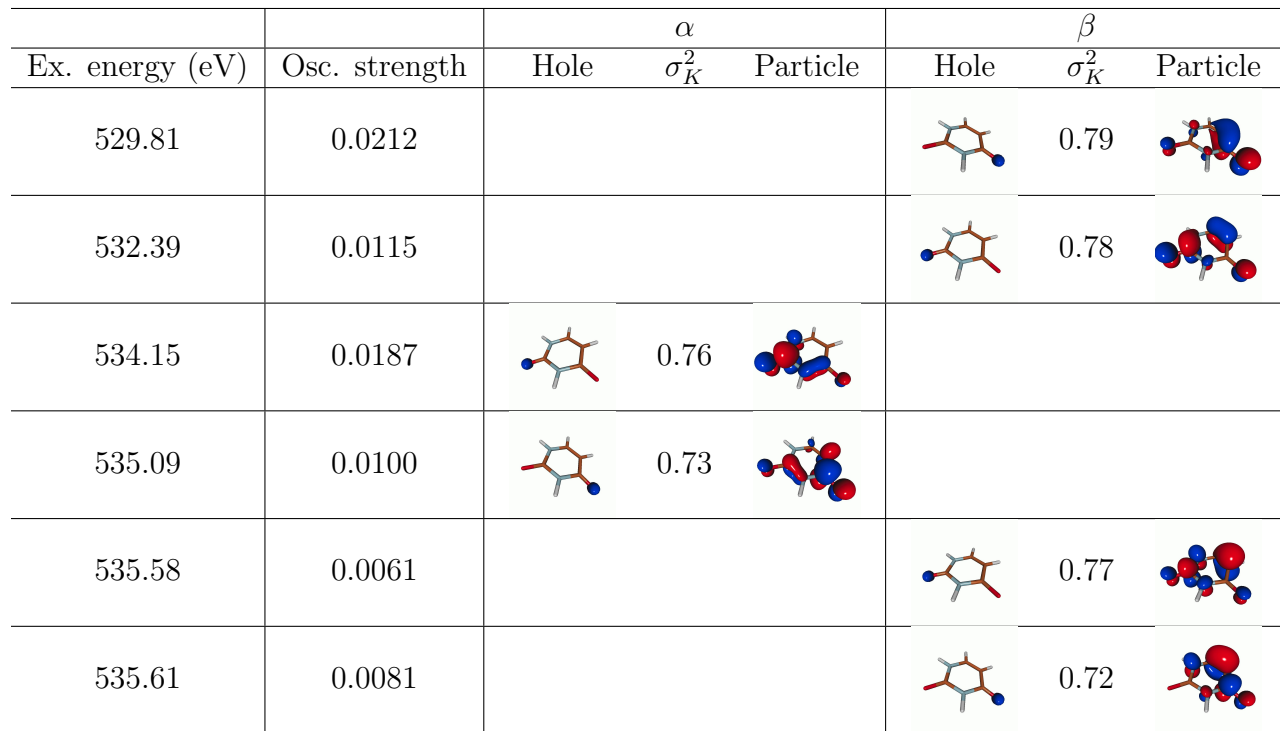 | 0.72         | 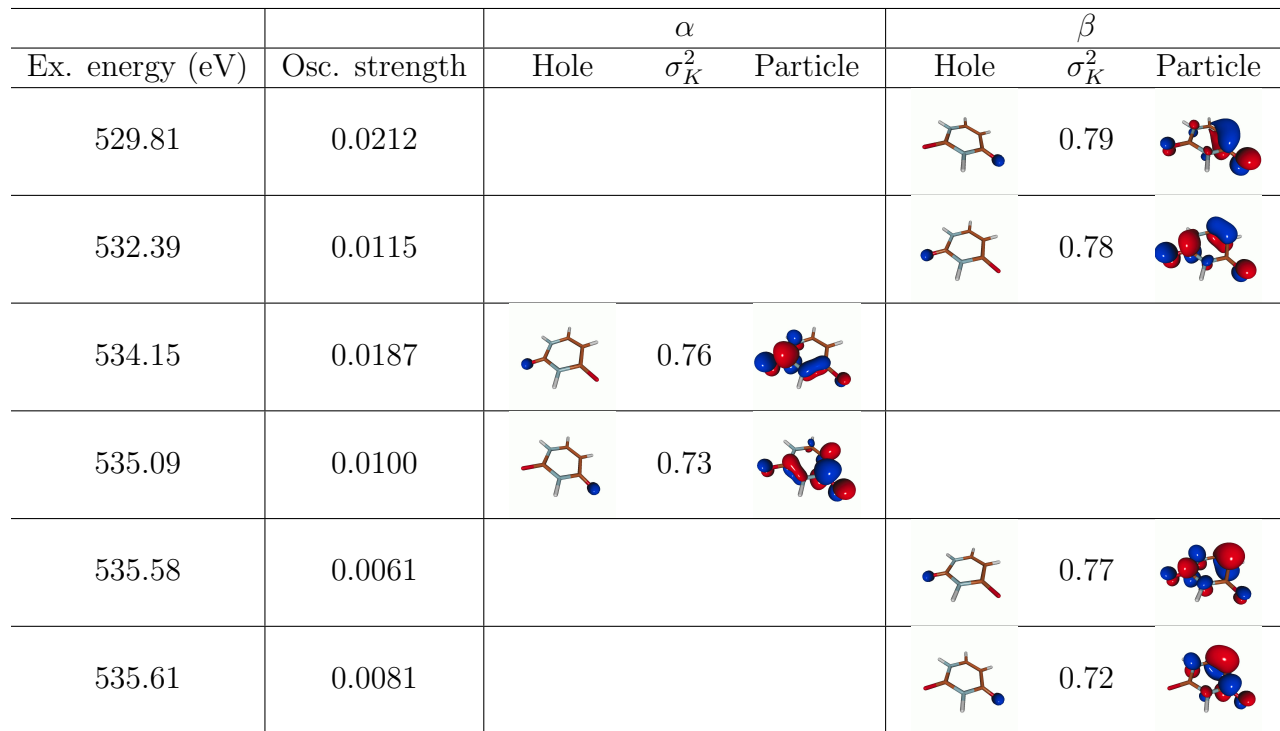 |

Table S26: Uracil. CVS-EOM-CCSD/6-311++G\*\* NTOs of the O<sub>1s</sub> core excitations from the T<sub>1</sub> state at the FC geometry (NTO isosurface is 0.05).

| Ex. energy (eV) | Osc. strength | Hole                                                                                | $\sigma_K^2$ | Particle                                                                              |
|-----------------|---------------|-------------------------------------------------------------------------------------|--------------|---------------------------------------------------------------------------------------|
| 528.78          | 0.0066        | 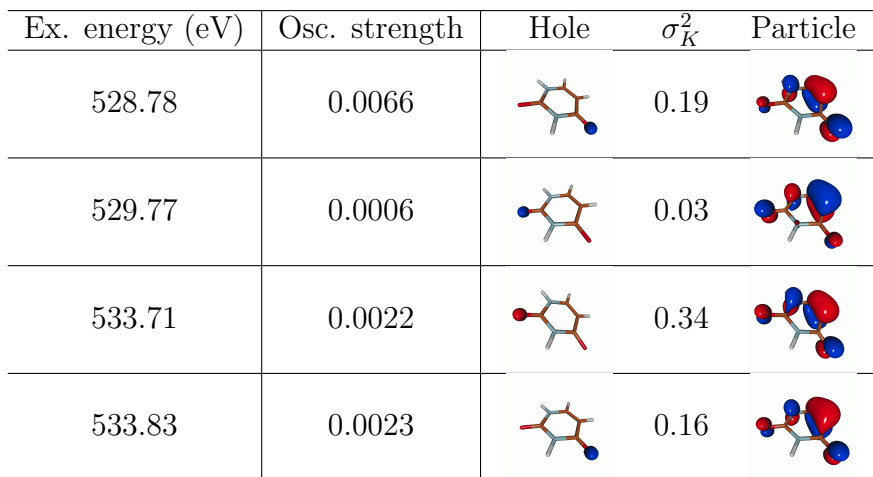 | 0.19         | 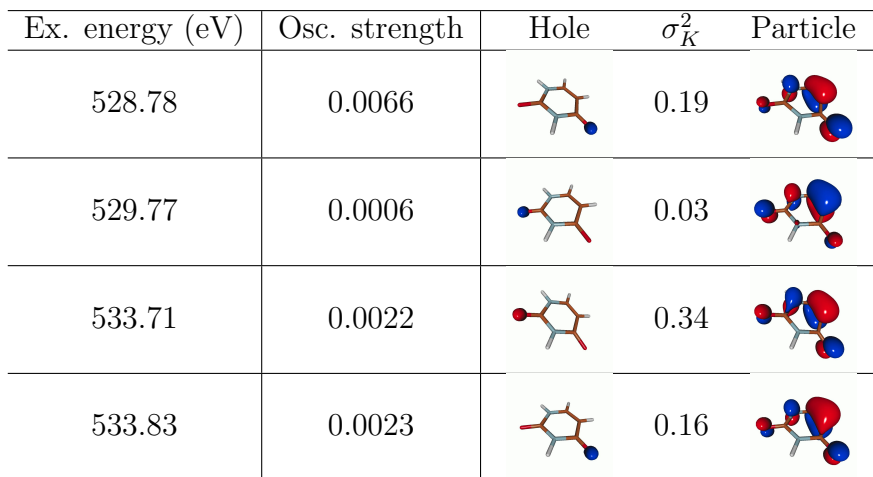 |
| 529.77          | 0.0006        | 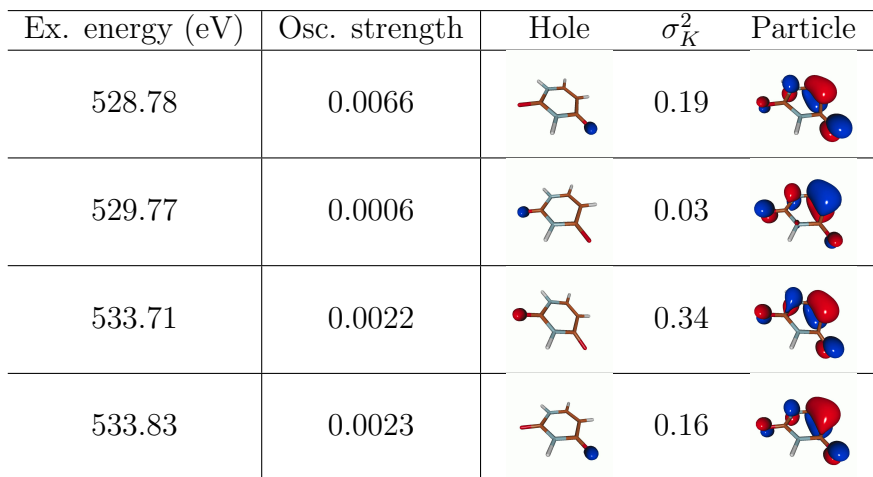 | 0.03         | 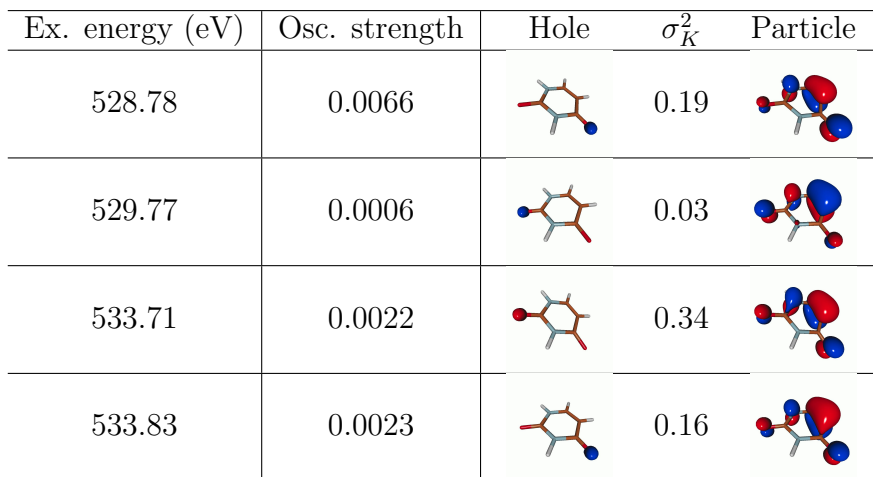 |
| 533.71          | 0.0022        | 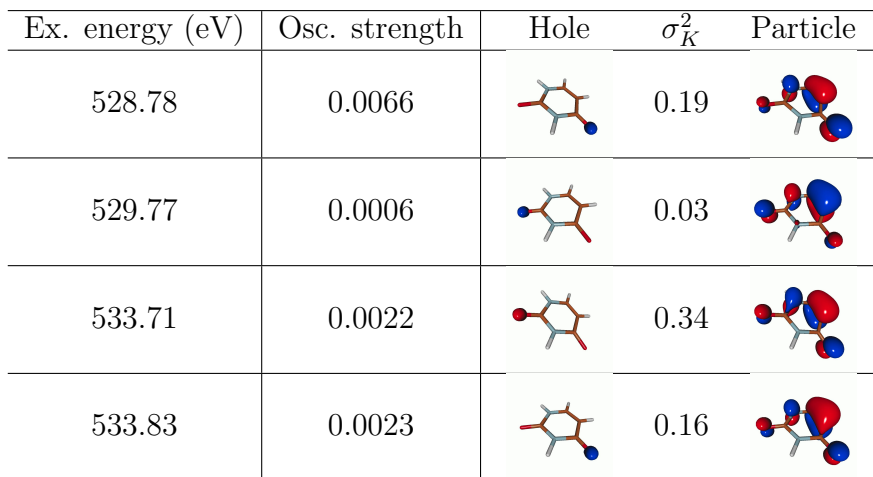 | 0.34         | 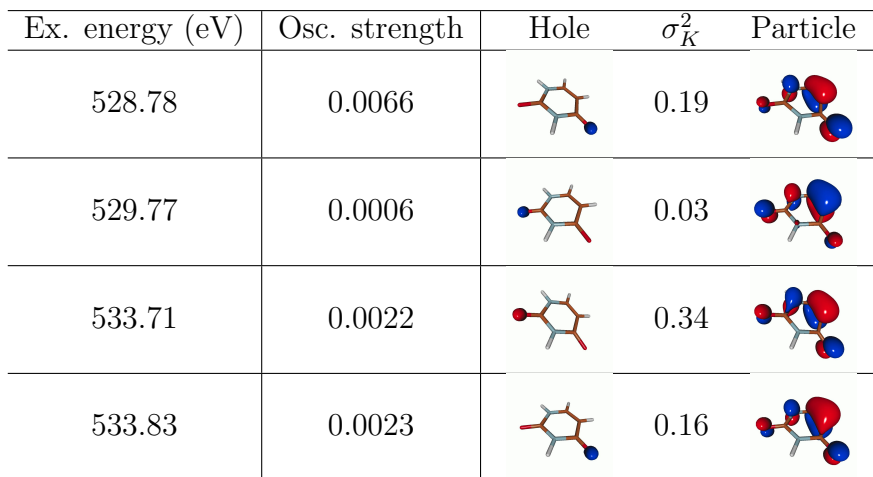 |
| 533.83          | 0.0023        | 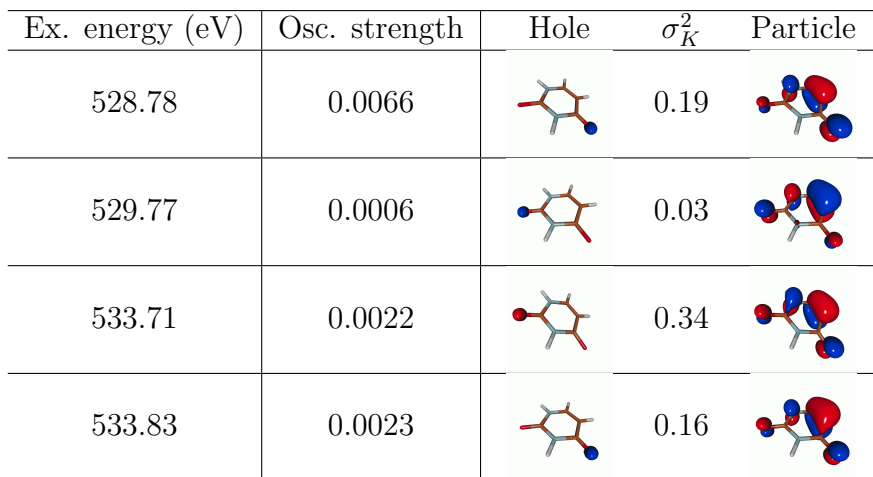 | 0.16         | 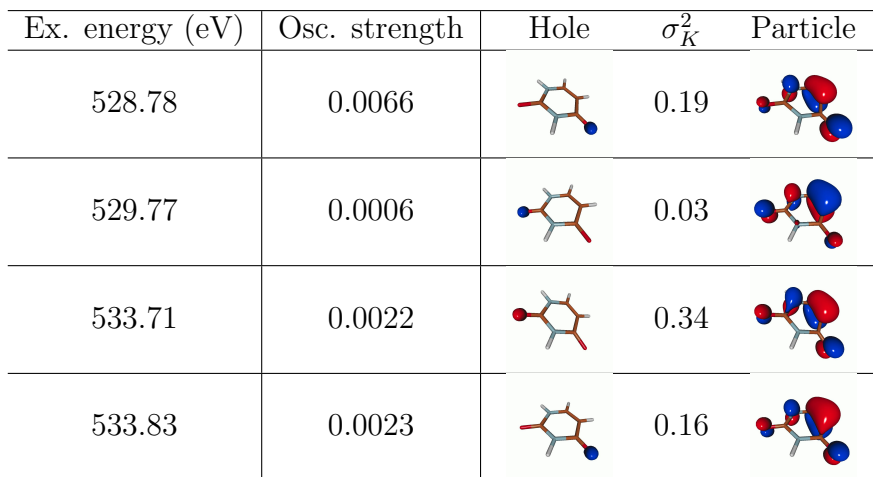 |

Table S27: Thymine. LSOR-CCSD/6-311++G\*\* NTOs of the  $O_{1s}$  core excitations from the  $S_1$  state at the minimum geometry (NTO isosurface is 0.05).

| Ex. energy (eV) | Osc. strength | $\alpha$                                                                          |              |                                                                                    | $\beta$                                                                             |              |                                                                                     |
|-----------------|---------------|-----------------------------------------------------------------------------------|--------------|------------------------------------------------------------------------------------|-------------------------------------------------------------------------------------|--------------|-------------------------------------------------------------------------------------|
|                 |               | Hole                                                                              | $\sigma_K^2$ | Particle                                                                           | Hole                                                                                | $\sigma_K^2$ | Particle                                                                            |
| 526.40          | 0.0472        | 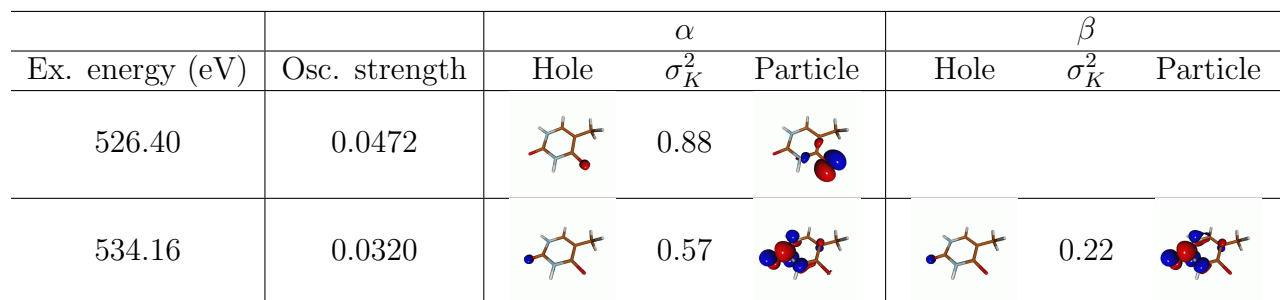 | 0.88         | 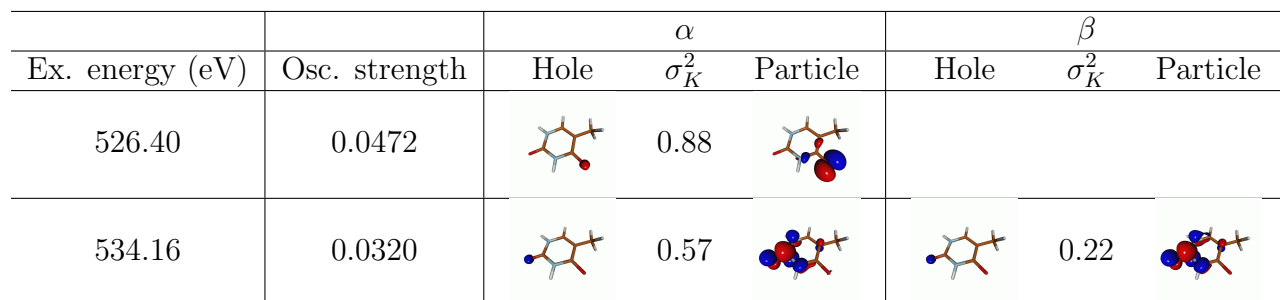 |                                                                                     |              |                                                                                     |
| 534.16          | 0.0320        | 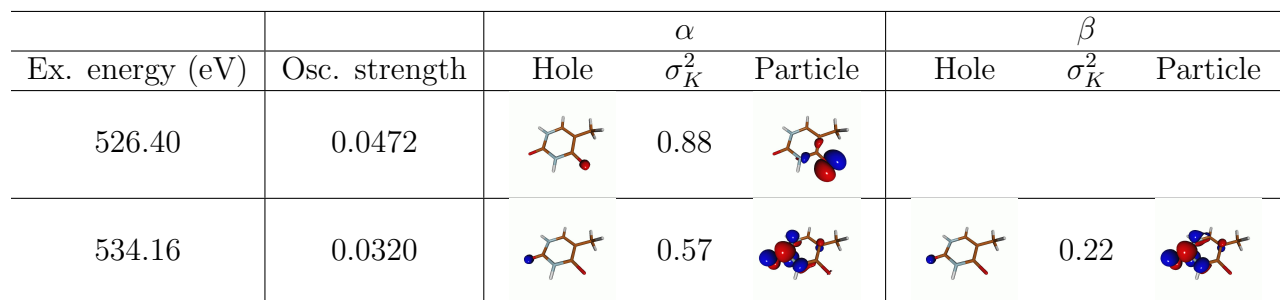 | 0.57         | 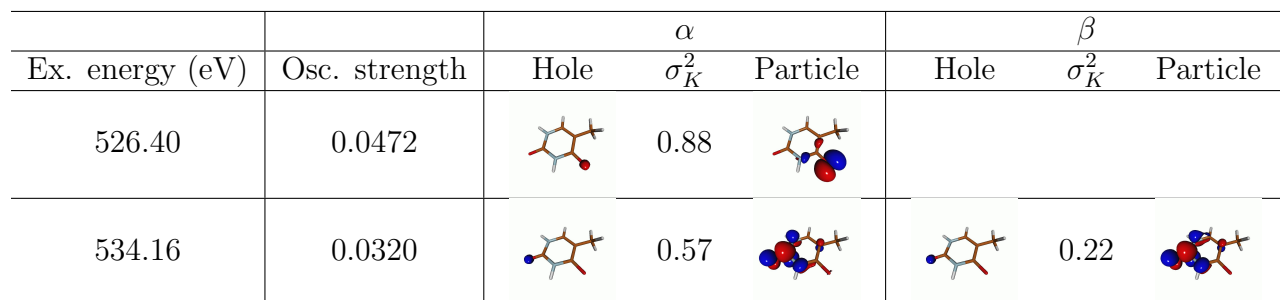 | 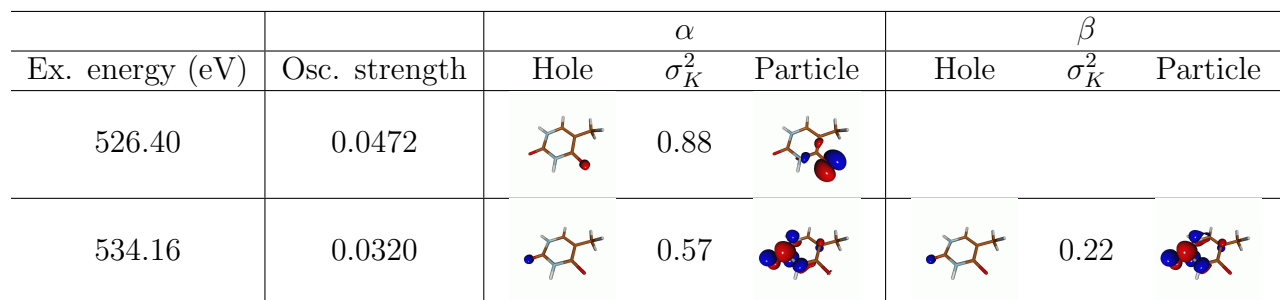 | 0.22         | 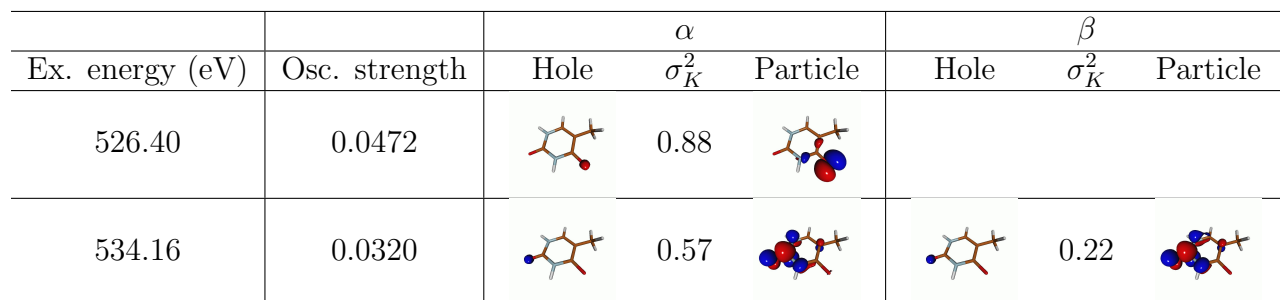 |

Table S28: Thymine. CVS-EOM-CCSD/6-311++G\*\* NTOs of the  $O_{1s}$  core excitations from the  $S_1$  state at the potential energy minimum (NTO isosurface is 0.05).

| Ex. energy (eV) | Osc. strength | Hole                                                                                | $\sigma_K^2$ | Particle                                                                              |
|-----------------|---------------|-------------------------------------------------------------------------------------|--------------|---------------------------------------------------------------------------------------|
| 528.32          | 0.0458        | 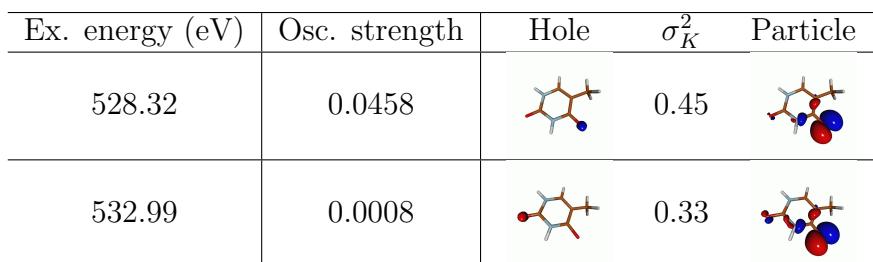   | 0.45         | 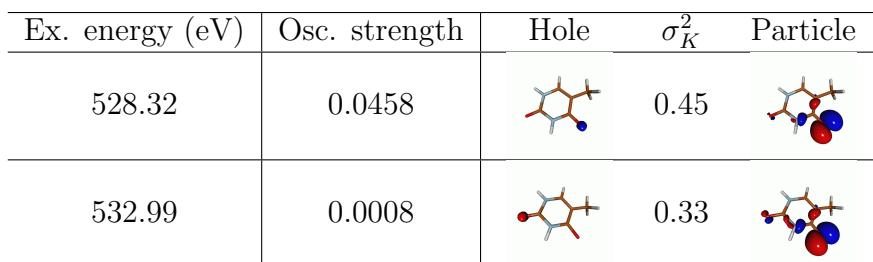   |
| 532.99          | 0.0008        | 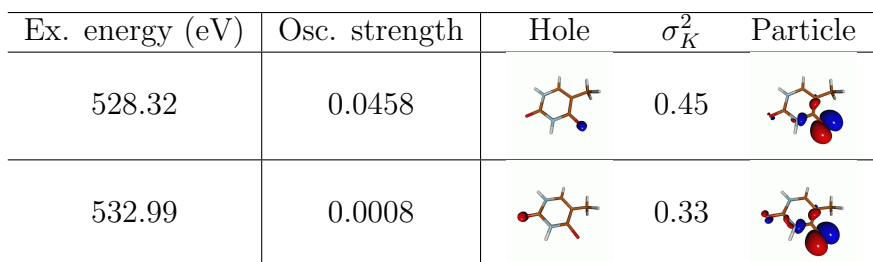 | 0.33         | 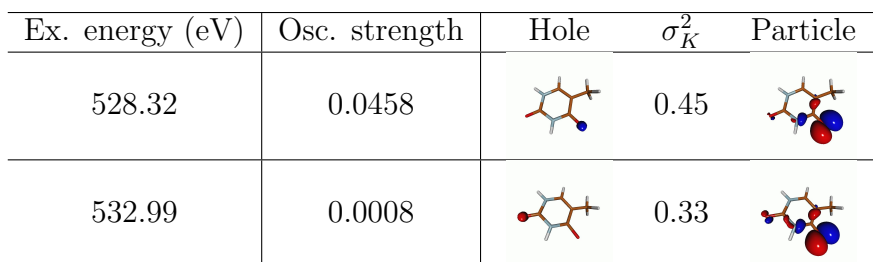 |

Table S29: Acetylacetone. LSOR-CCSD/6-311++G\*\* NTOs of the  $C_{1s}$  core excitations from the  $T_1$  state at the potential energy minimum (NTO isosurface is 0.05).

| Ex. energy (eV) | Osc. strength | $\alpha$                                                                            |              |                                                                                      | $\beta$                                                                               |              |                                                                                       |
|-----------------|---------------|-------------------------------------------------------------------------------------|--------------|--------------------------------------------------------------------------------------|---------------------------------------------------------------------------------------|--------------|---------------------------------------------------------------------------------------|
|                 |               | Hole                                                                                | $\sigma_K^2$ | Particle                                                                             | Hole                                                                                  | $\sigma_K^2$ | Particle                                                                              |
| 281.76          | 0.0347        |                                                                                     |              |                                                                                      | 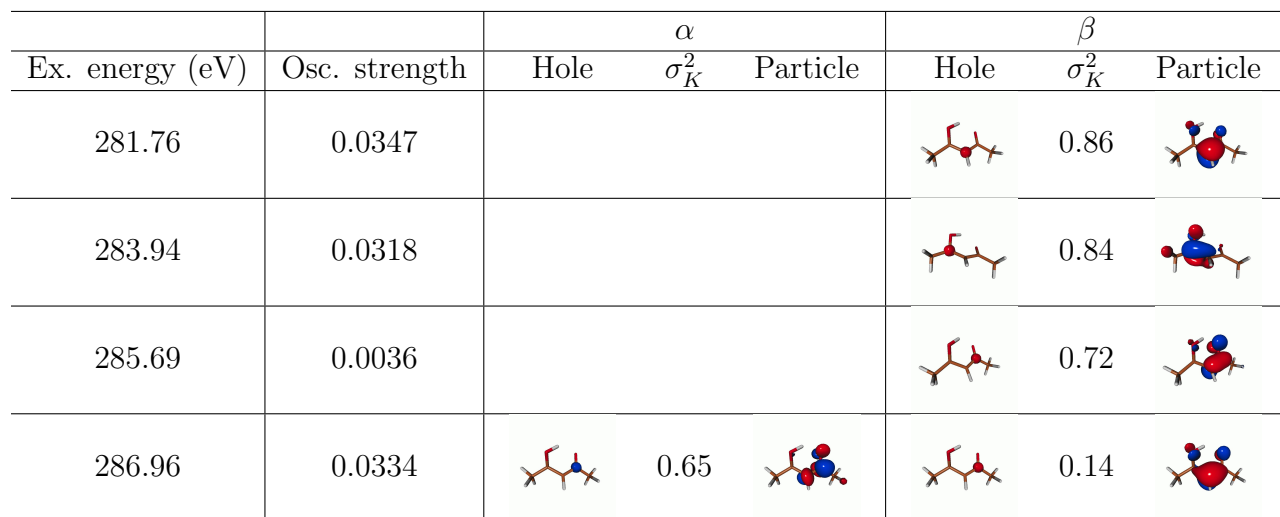 | 0.86         | 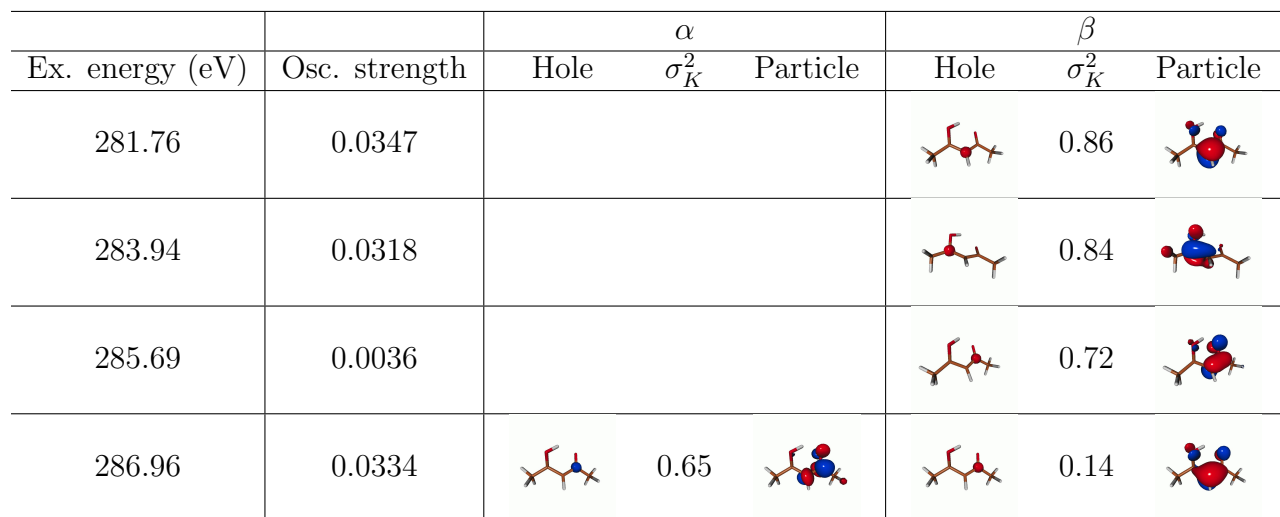 |
| 283.94          | 0.0318        |                                                                                     |              |                                                                                      | 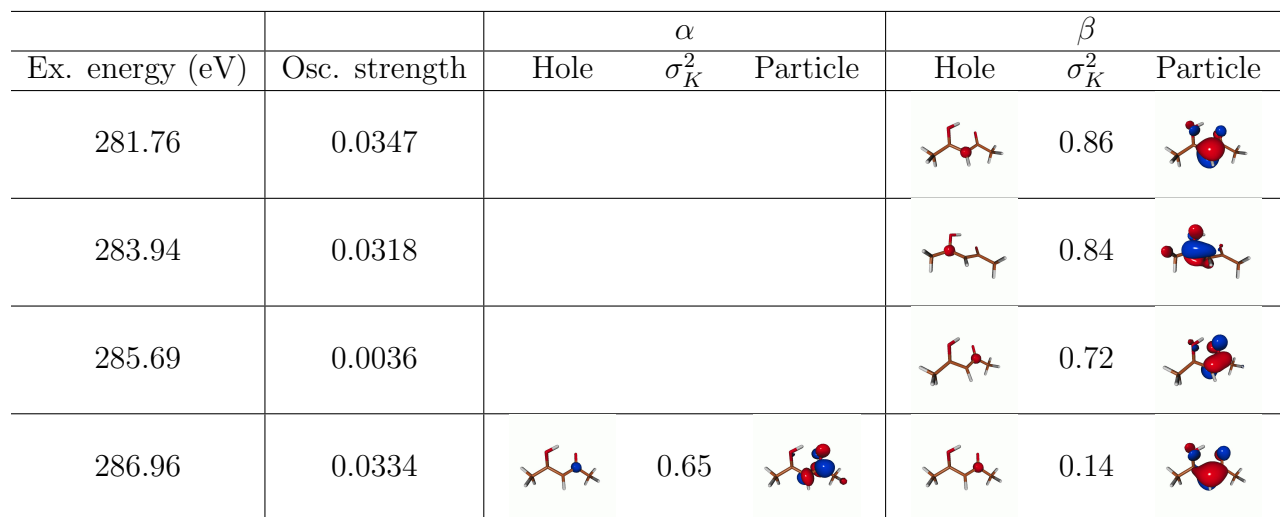 | 0.84         | 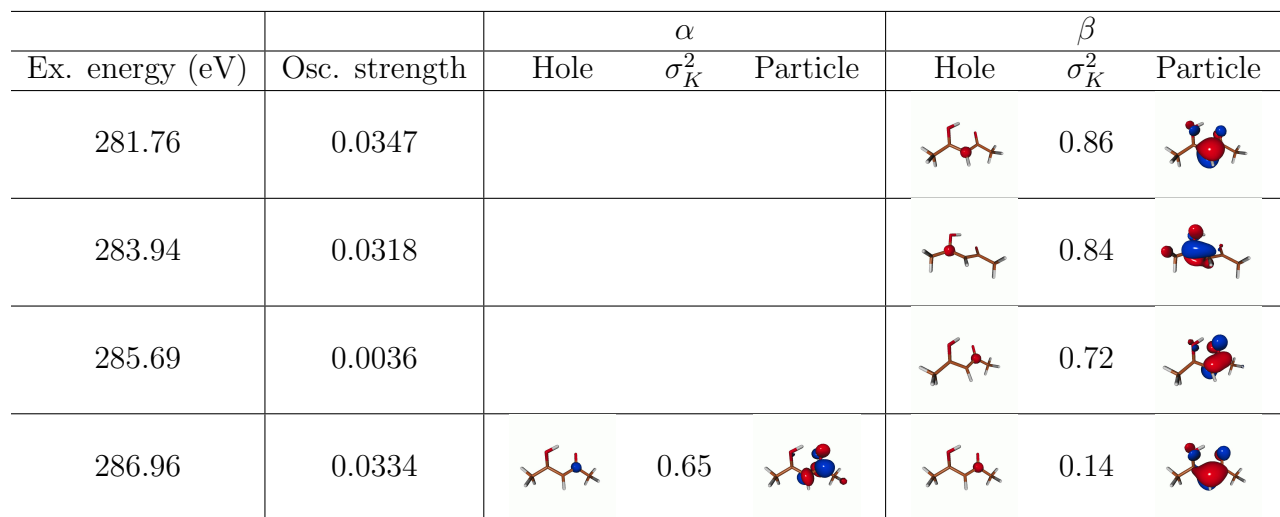 |
| 285.69          | 0.0036        |                                                                                     |              |                                                                                      | 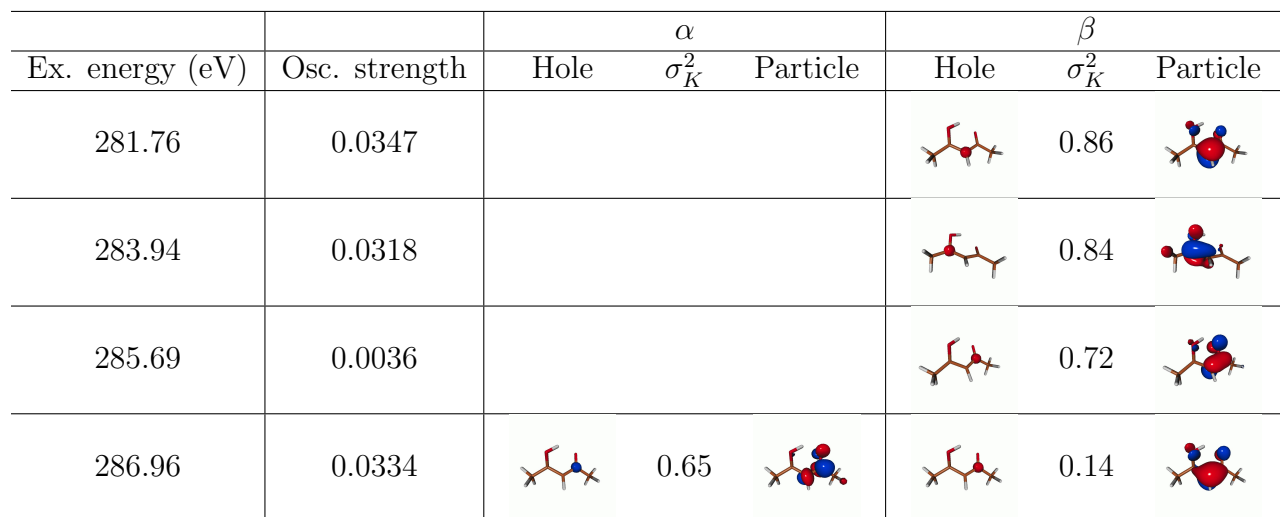 | 0.72         | 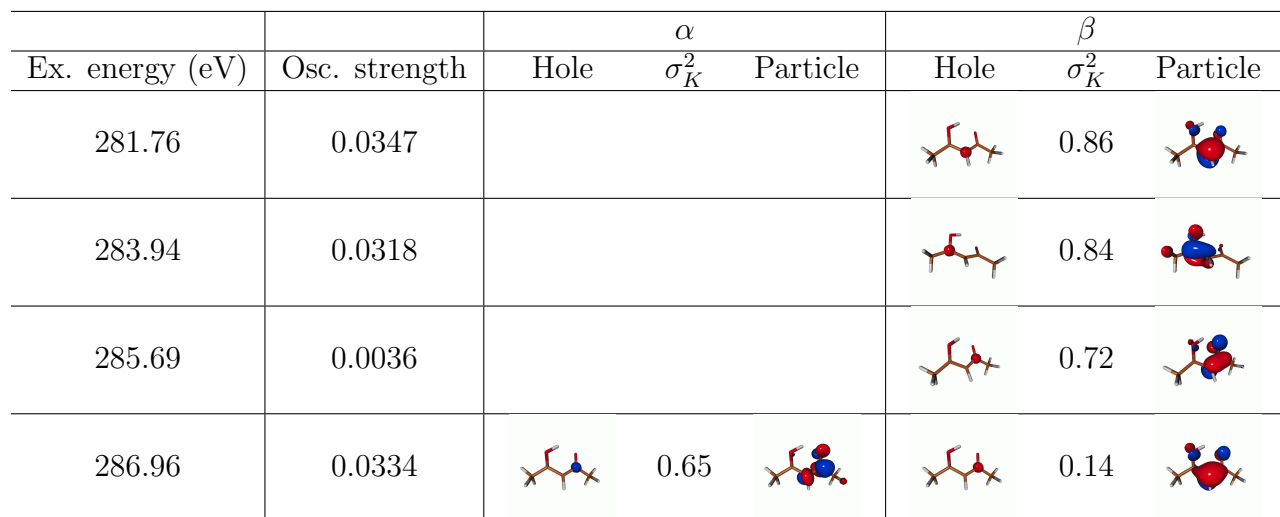 |
| 286.96          | 0.0334        | 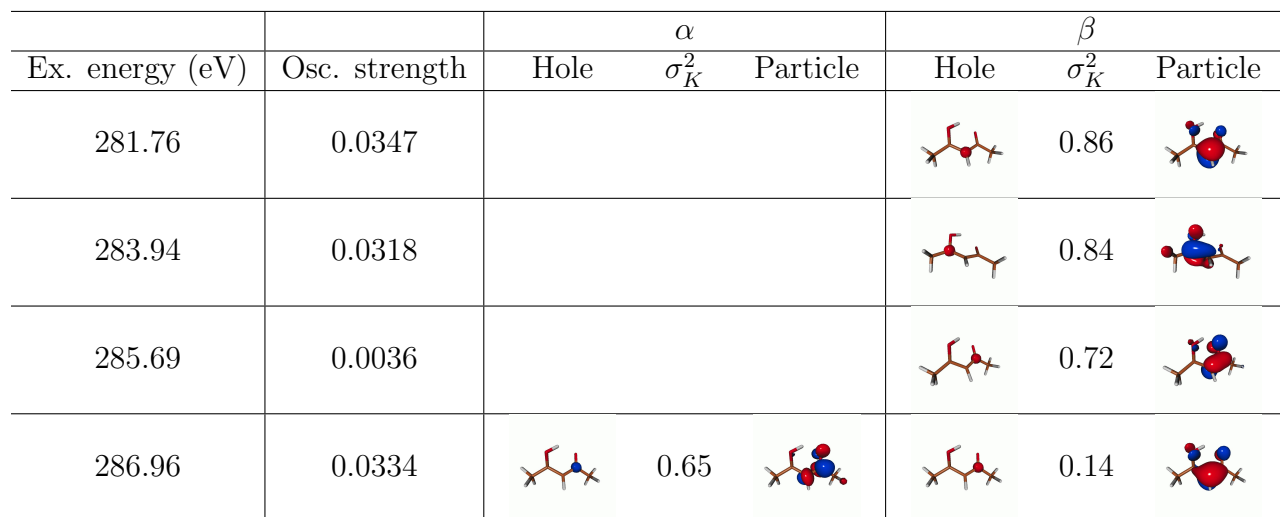 | 0.65         | 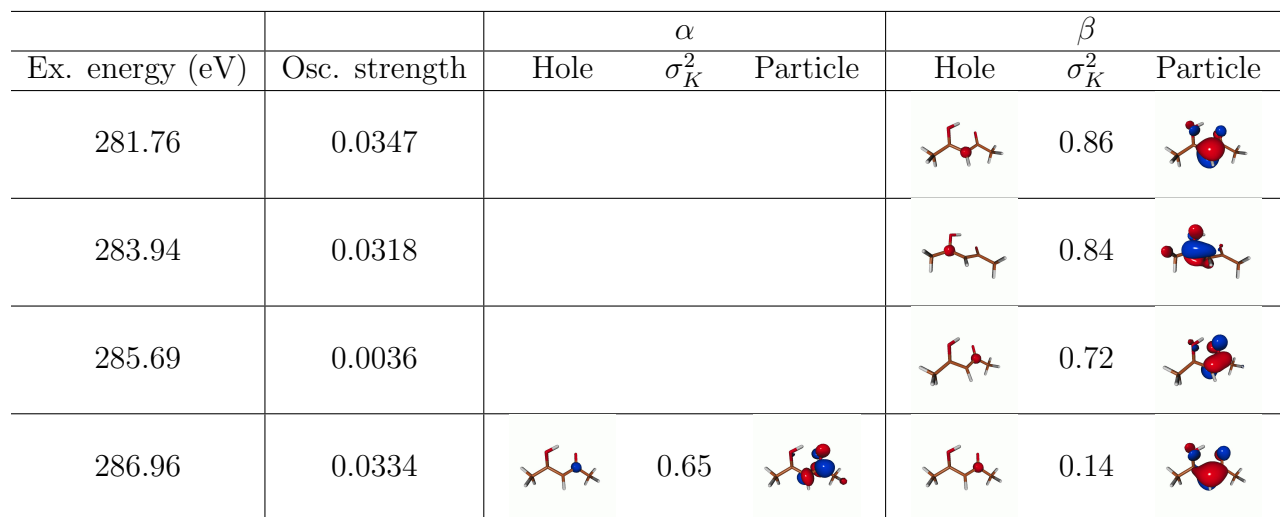 | 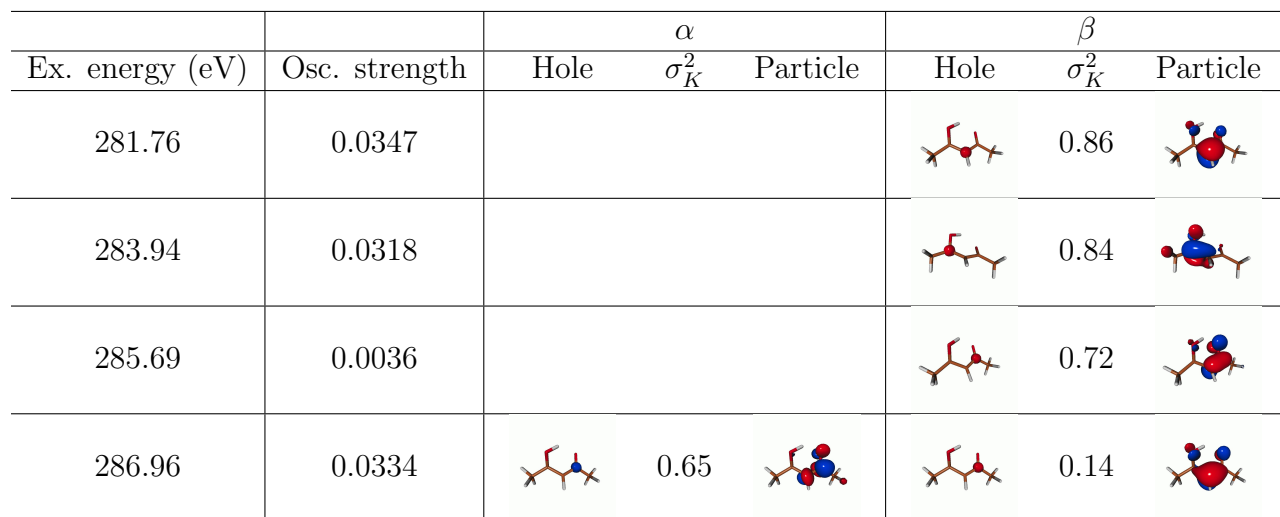 | 0.14         | 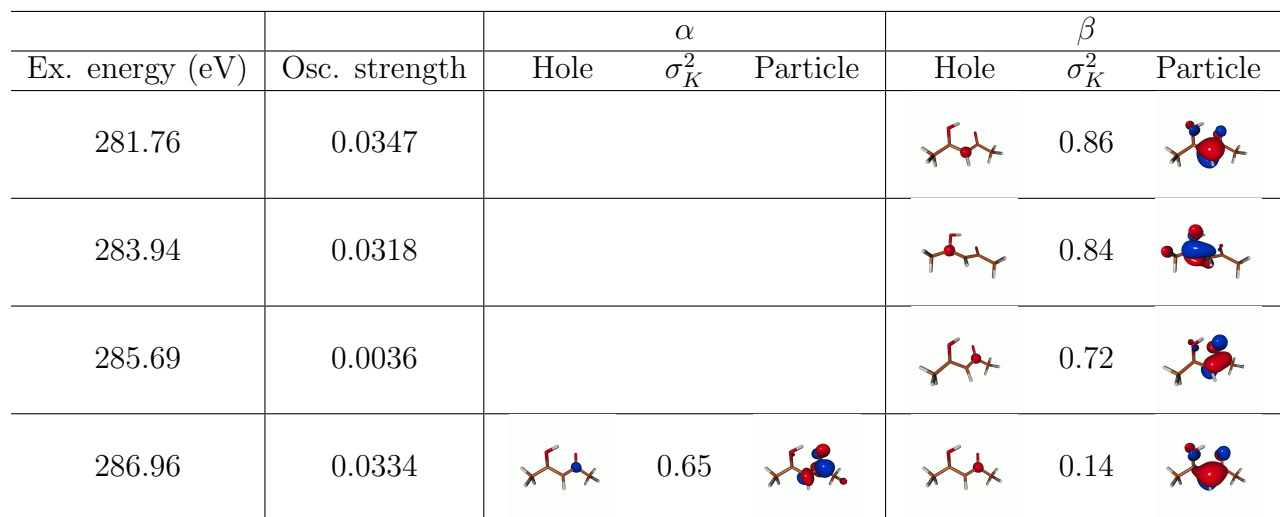 |



Table S30: Acetylacetone. CVS-EOM-CCSD/6-311++G\*\* NTOs of the  $C_{1s}$  core excitations from the  $T_1$  state at the potential energy minimum (NTO isosurface is 0.05).

| Ex. energy (eV) | Osc. strength | Hole                                                                              | $\sigma_K^2$ | Particle                                                                            |
|-----------------|---------------|-----------------------------------------------------------------------------------|--------------|-------------------------------------------------------------------------------------|
| 282.69          | 0.0292        | 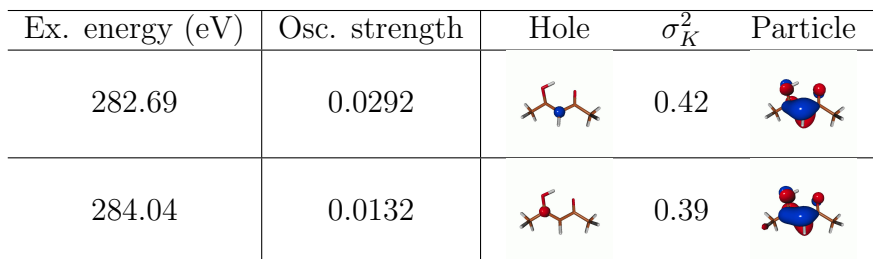 | 0.42         | 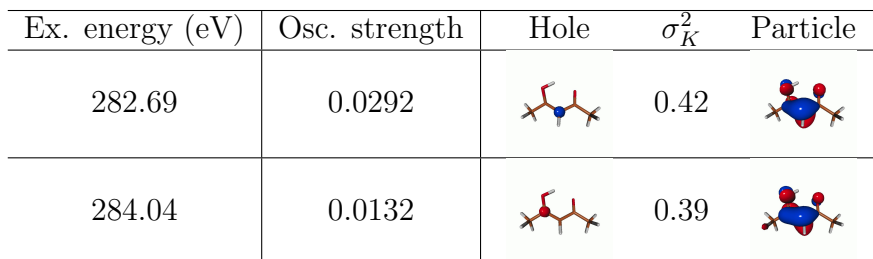 |
| 284.04          | 0.0132        | 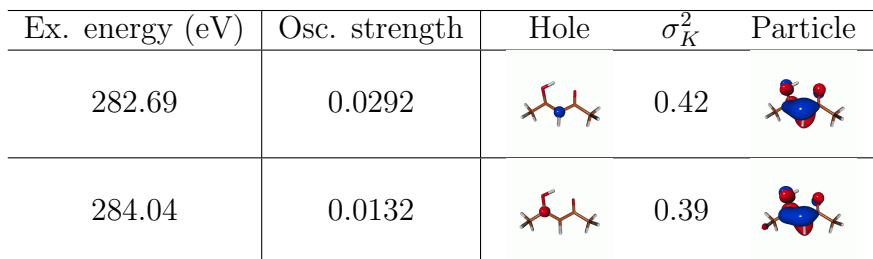 | 0.39         | 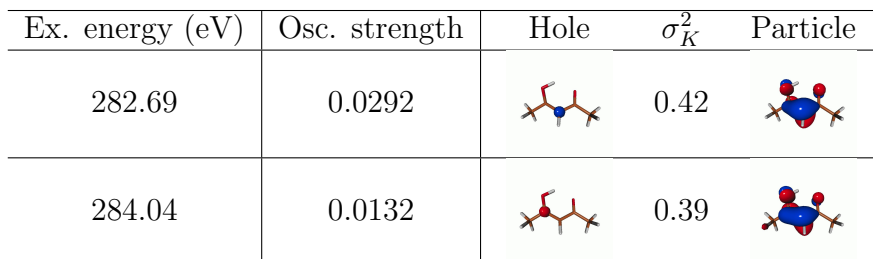 |

Table S31: Acetylacetone. LSOR-CCSD/6-311++G\*\* NTOs of the  $C_{1s}$  core excitations from the  $S_2$  state at the potential energy minimum of  $S_1$  (NTO isosurface is 0.05).

| Ex. energy (eV) | Osc. strength | $\alpha$                                                                            |              |                                                                                      | $\beta$                                                                               |              |                                                                                       |
|-----------------|---------------|-------------------------------------------------------------------------------------|--------------|--------------------------------------------------------------------------------------|---------------------------------------------------------------------------------------|--------------|---------------------------------------------------------------------------------------|
|                 |               | Hole                                                                                | $\sigma_K^2$ | Particle                                                                             | Hole                                                                                  | $\sigma_K^2$ | Particle                                                                              |
| 281.30          | 0.0228        | 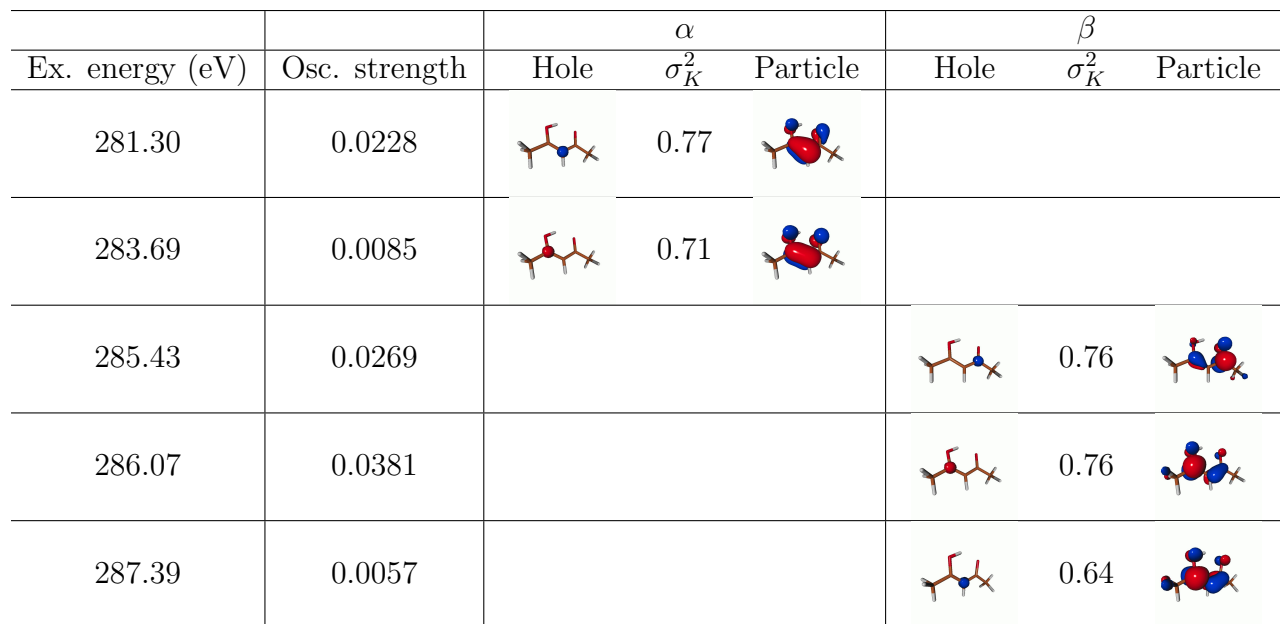   | 0.77         | 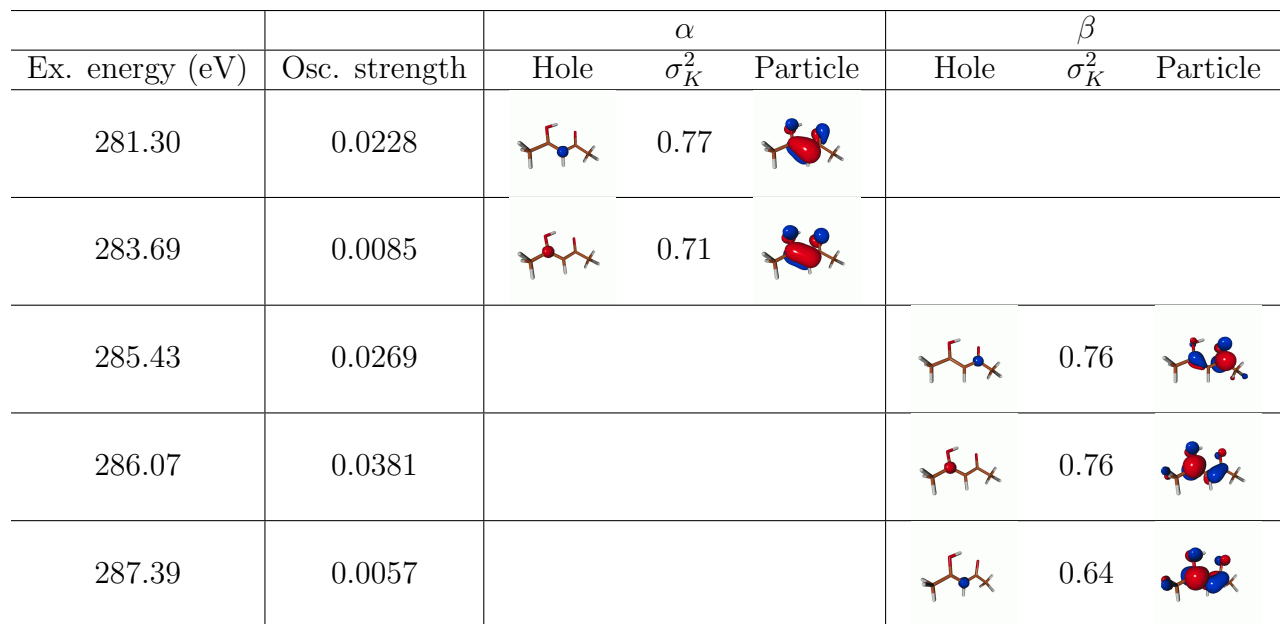   |                                                                                       |              |                                                                                       |
| 283.69          | 0.0085        | 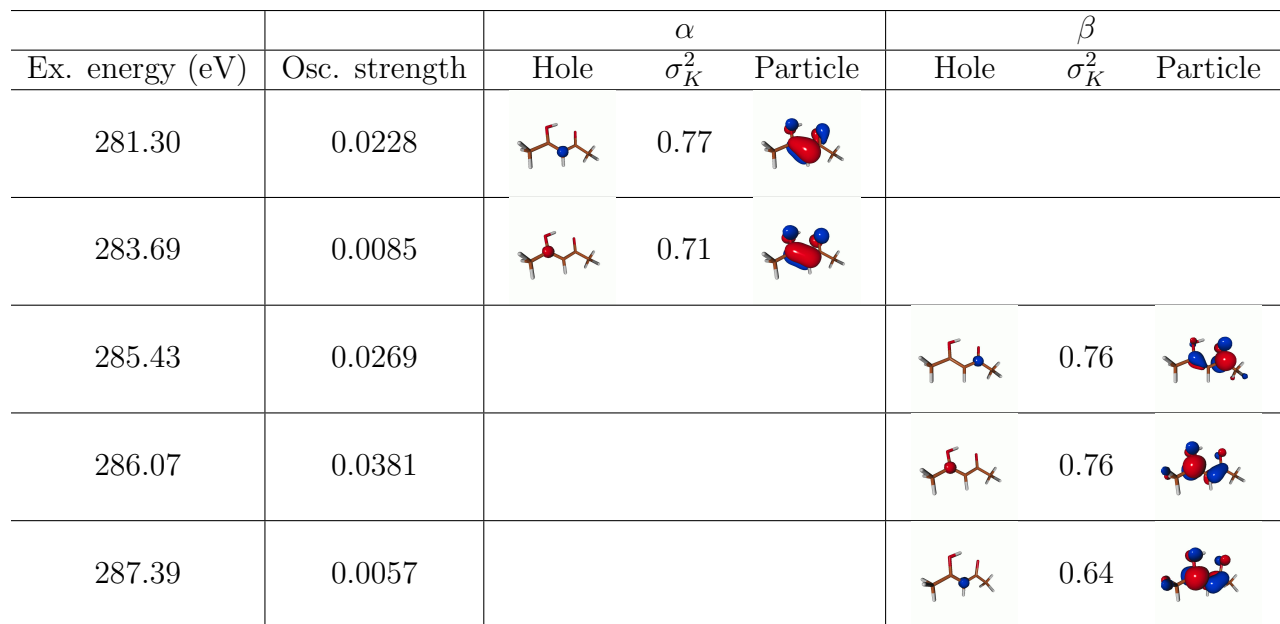 | 0.71         | 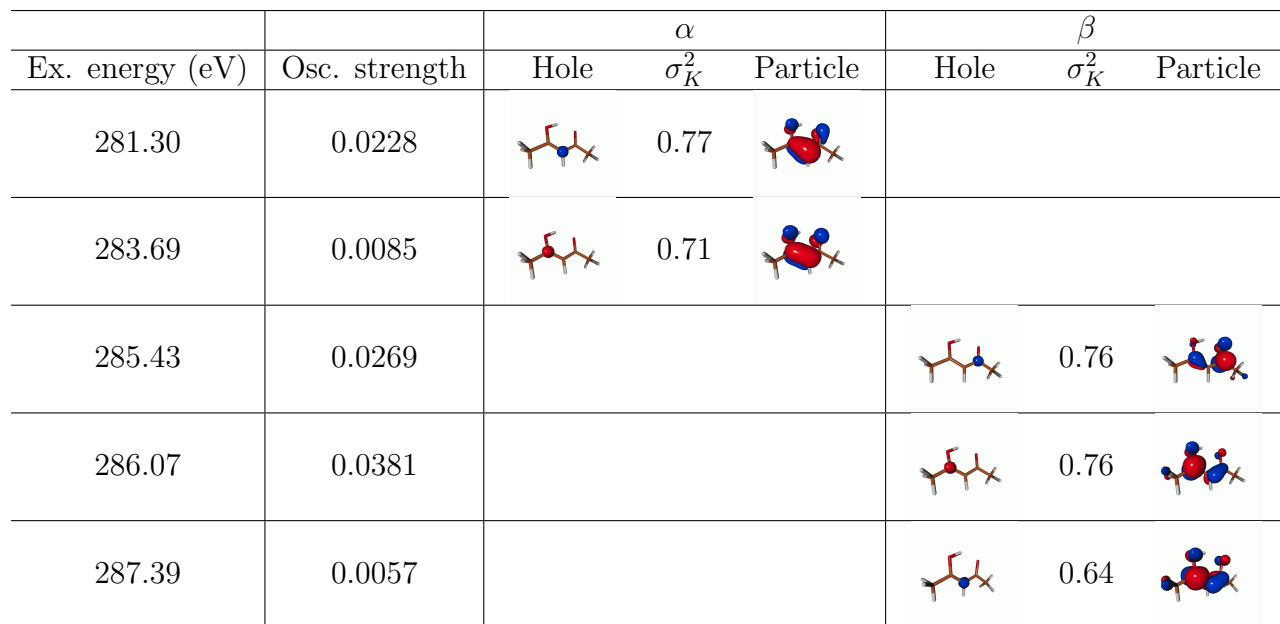 |                                                                                       |              |                                                                                       |
| 285.43          | 0.0269        |                                                                                     |              |                                                                                      | 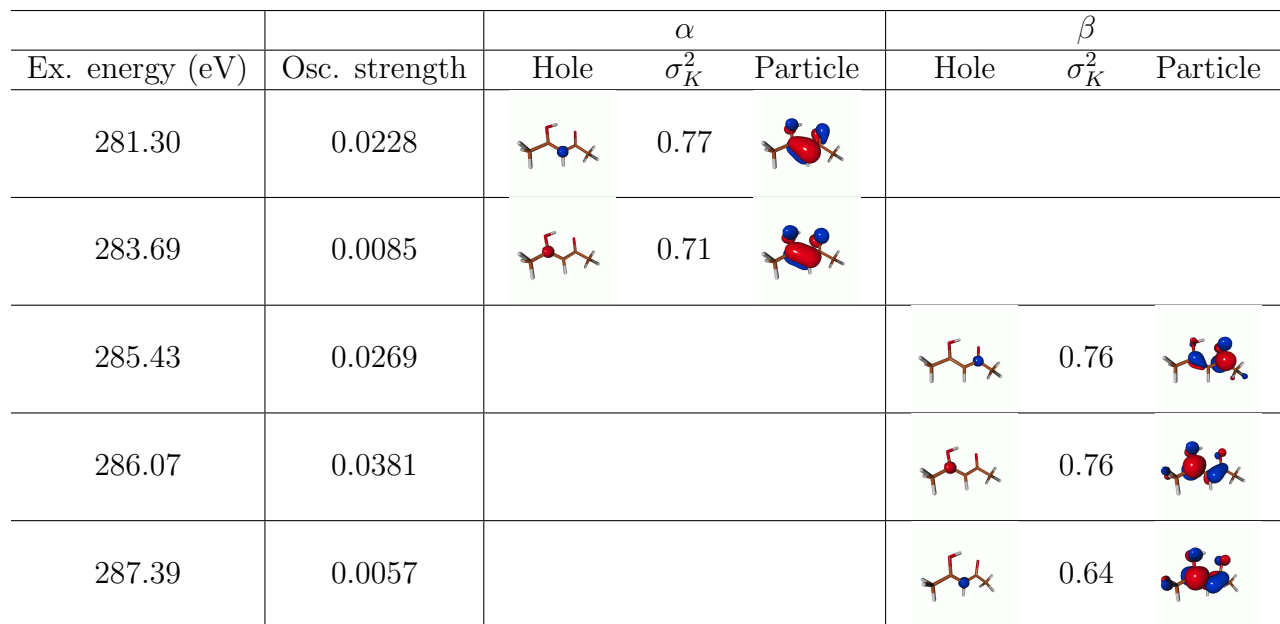 | 0.76         | 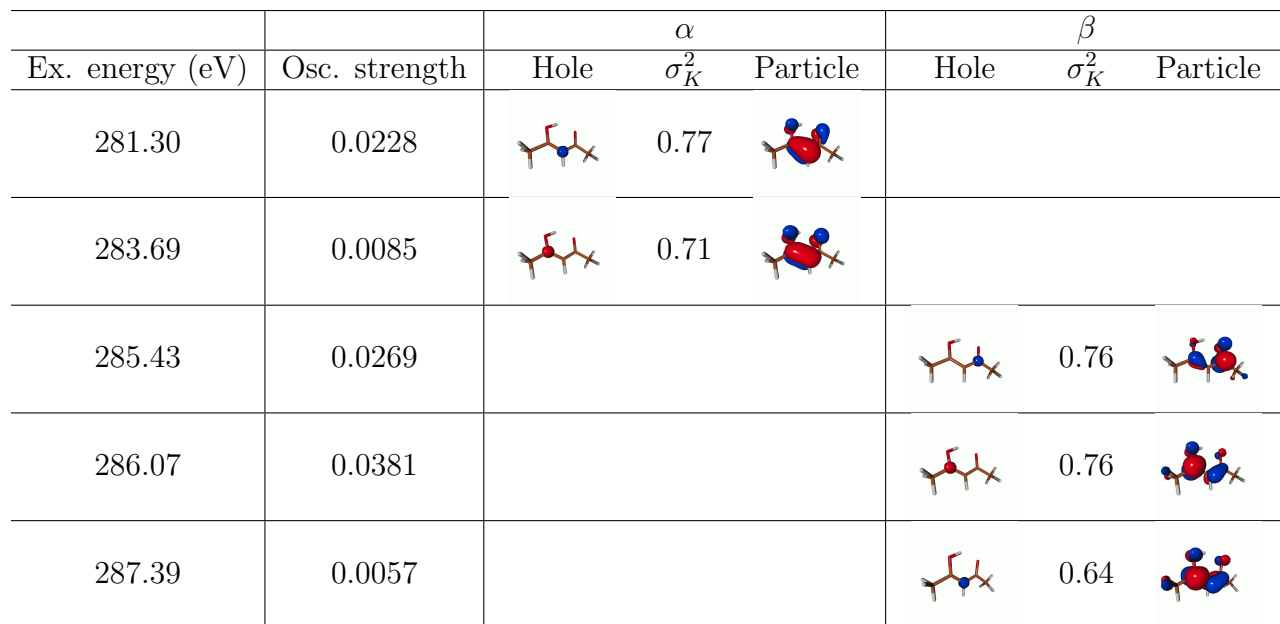 |
| 286.07          | 0.0381        |                                                                                     |              |                                                                                      | 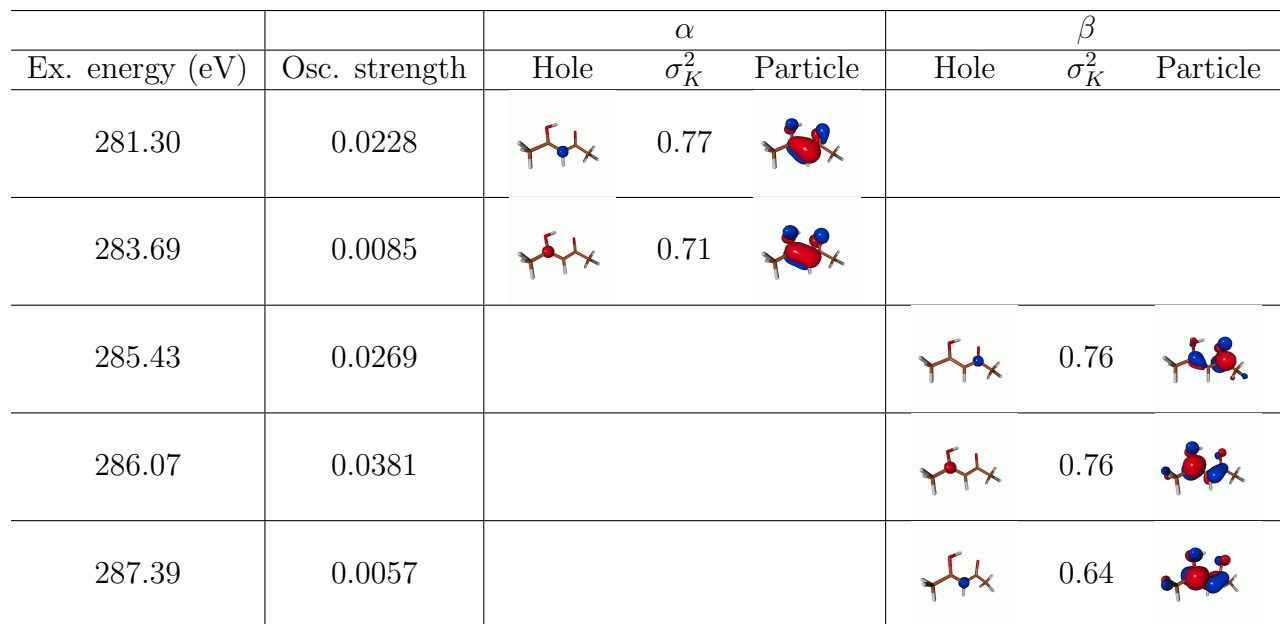 | 0.76         | 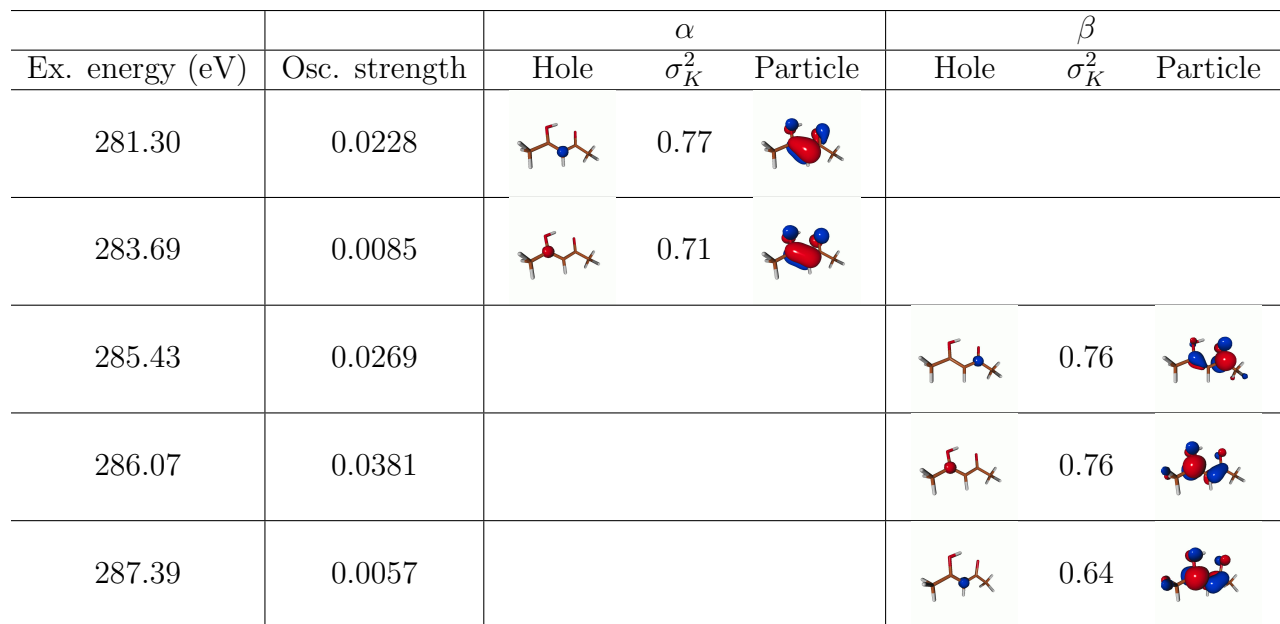 |
| 287.39          | 0.0057        |                                                                                     |              |                                                                                      | 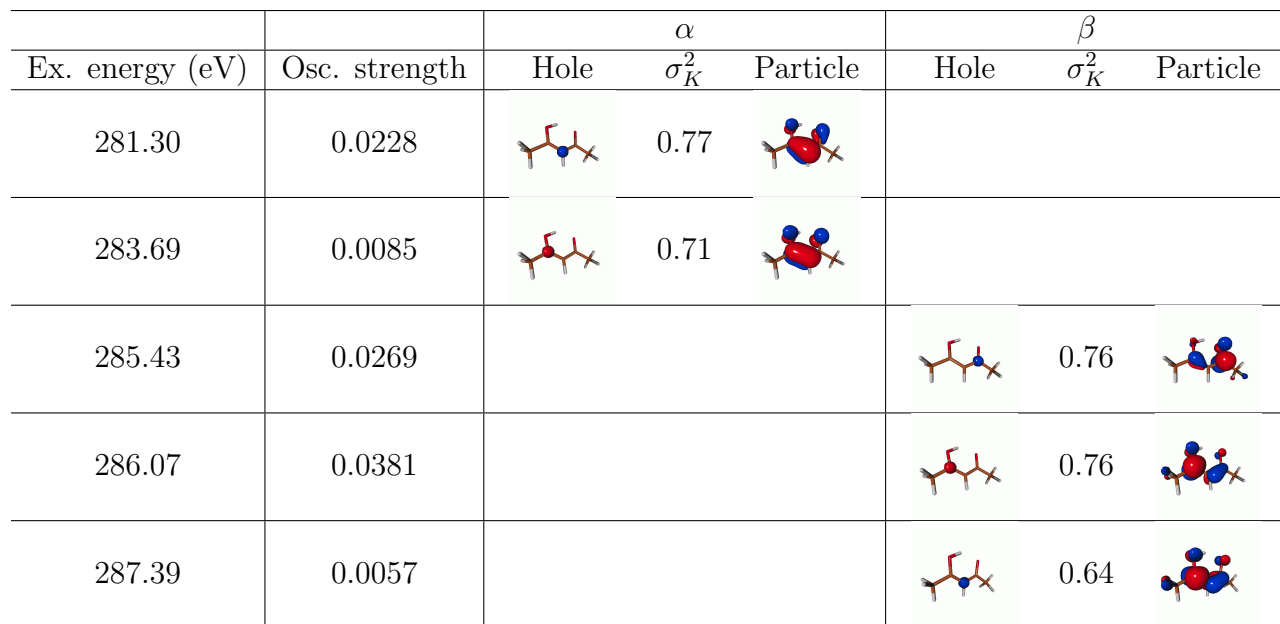 | 0.64         | 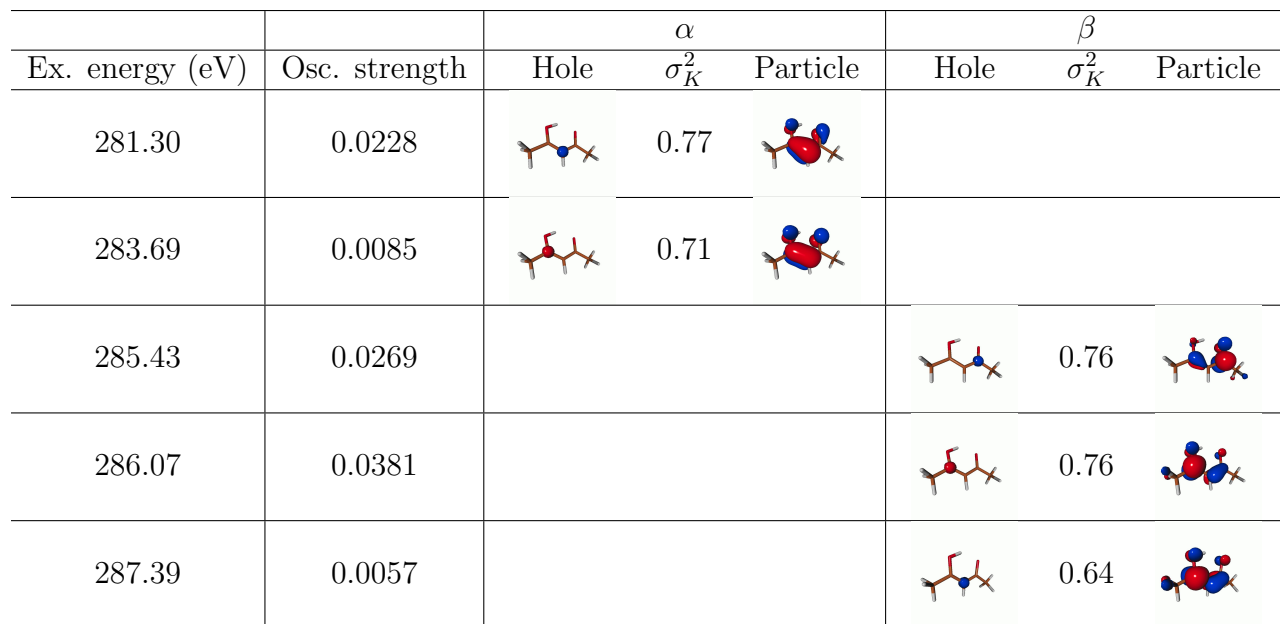 |

Table S32: Acetylacetone. CVS-EOM-CCSD/6-311++G\*\* NTOs of the  $C_{1s}$  core excitations from the  $S_2$  state at the potential energy minimum of  $S_1$  (NTO isosurface is 0.05).

| Ex. energy (eV) | Osc. strength | Hole                                                                                | $\sigma_K^2$ | Particle                                                                              |
|-----------------|---------------|-------------------------------------------------------------------------------------|--------------|---------------------------------------------------------------------------------------|
| 280.77          | 0.0157        | 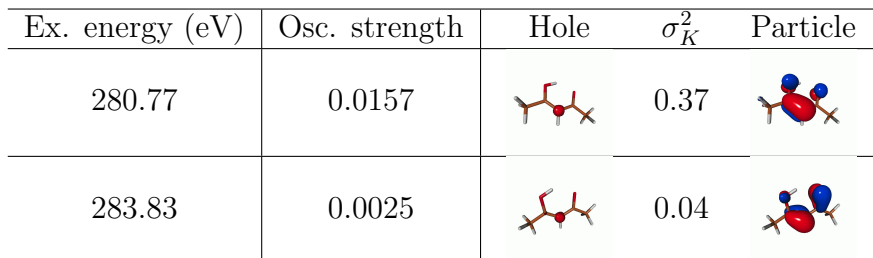 | 0.37         | 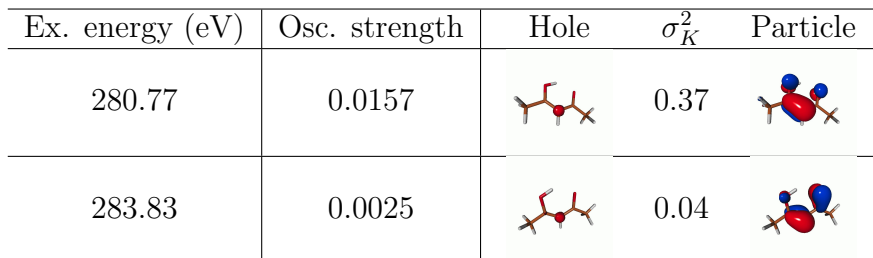 |
| 283.83          | 0.0025        | 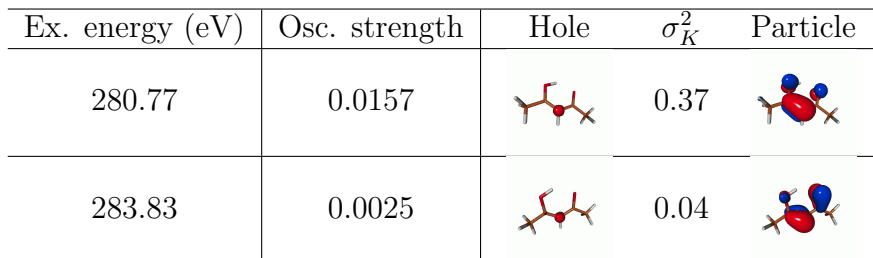 | 0.04         | 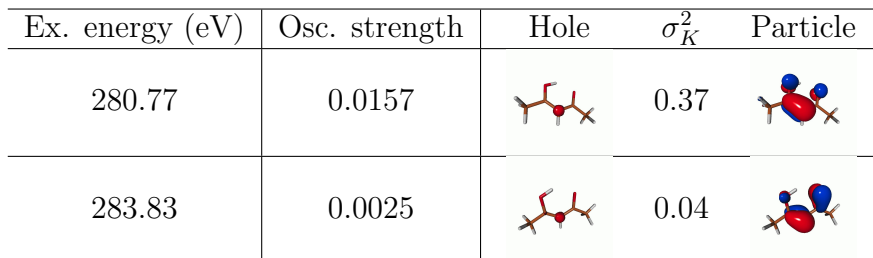 |

Table S33: Thymine. MOM-TDDFT/B3LYP/6-311++G\*\* NTOs of the O<sub>1s</sub> core excitations from the S<sub>1</sub> state at the minimum geometry (NTO isosurface is 0.05).

| Ex. energy (eV) | Osc. strength | $\alpha$                                                                          |              |                                                                                    | $\beta$                                                                             |              |                                                                                     |
|-----------------|---------------|-----------------------------------------------------------------------------------|--------------|------------------------------------------------------------------------------------|-------------------------------------------------------------------------------------|--------------|-------------------------------------------------------------------------------------|
|                 |               | Hole                                                                              | $\sigma_K^2$ | Particle                                                                           | Hole                                                                                | $\sigma_K^2$ | Particle                                                                            |
| 511.82          | 0.0389        | 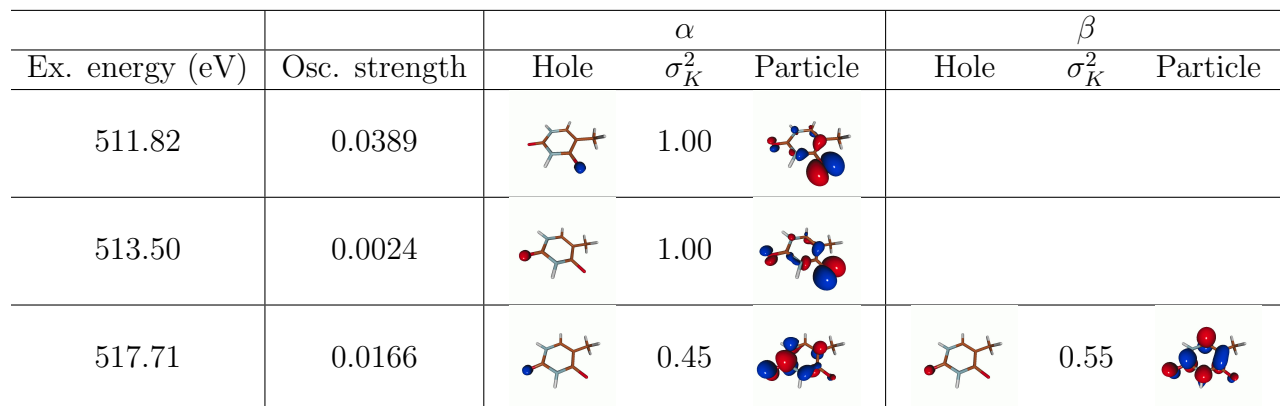 | 1.00         | 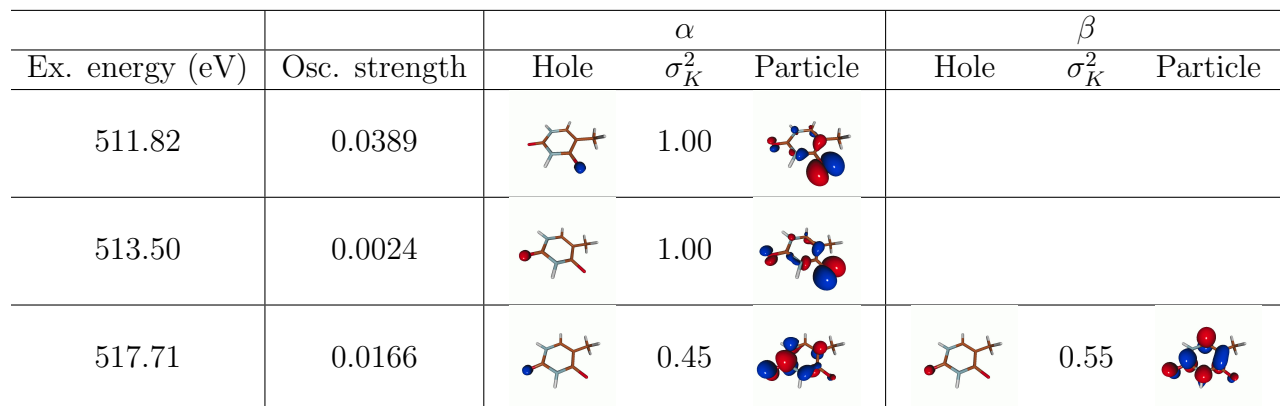 |                                                                                     |              |                                                                                     |
| 513.50          | 0.0024        | 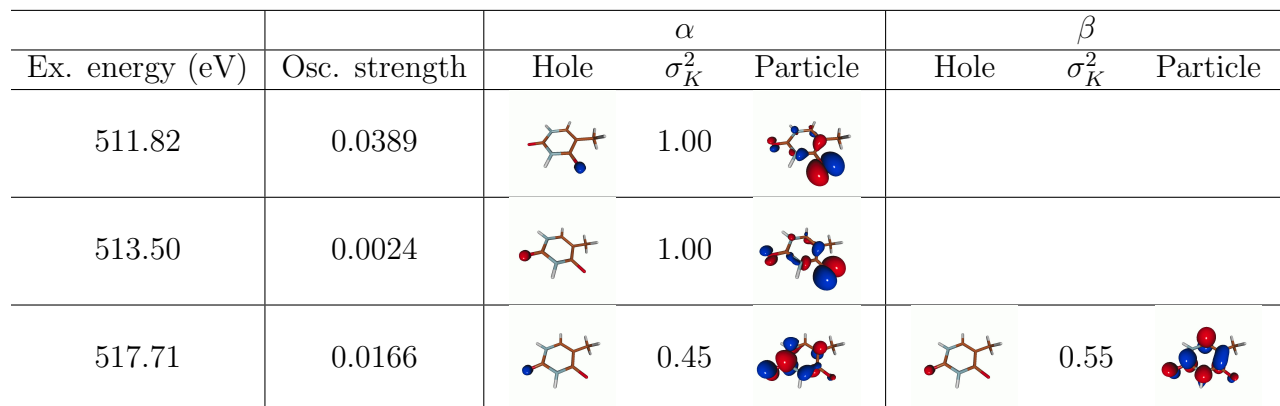 | 1.00         | 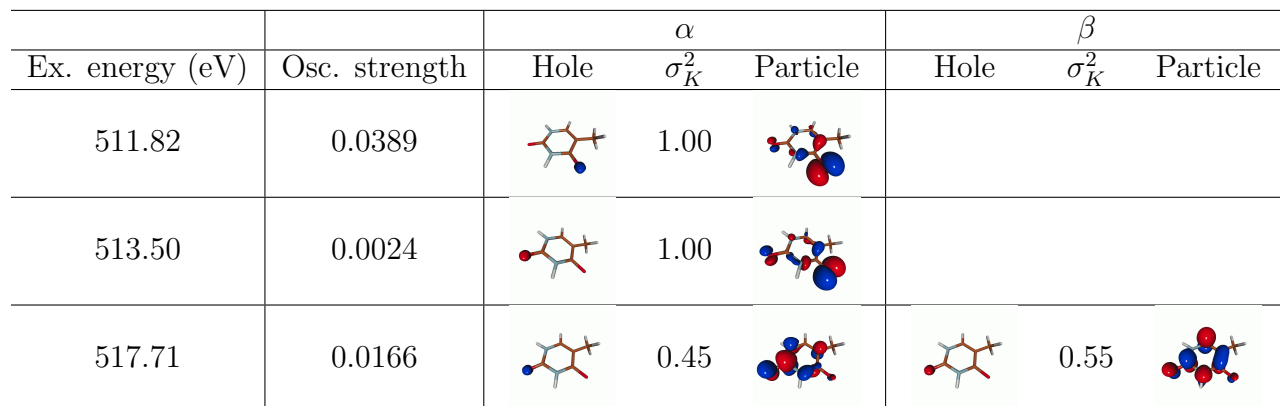 |                                                                                     |              |                                                                                     |
| 517.71          | 0.0166        | 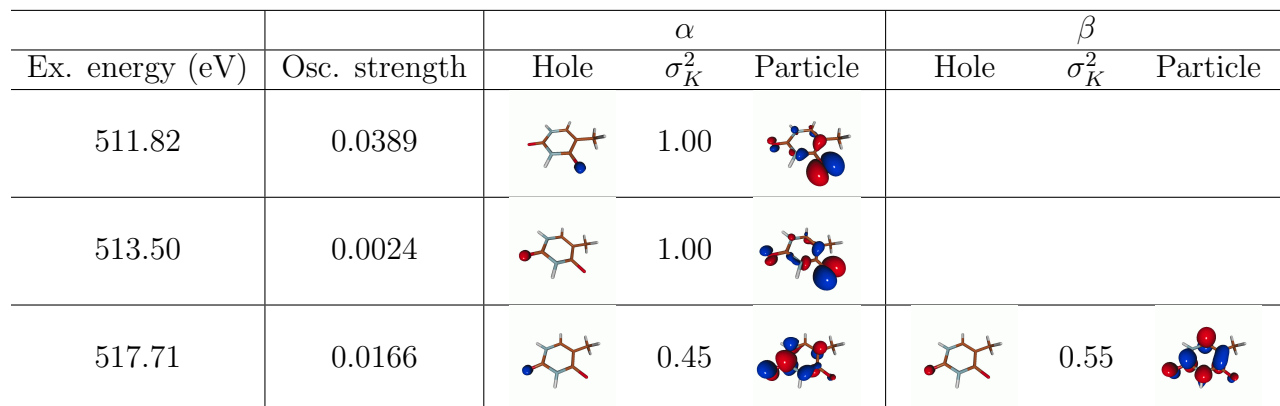 | 0.45         | 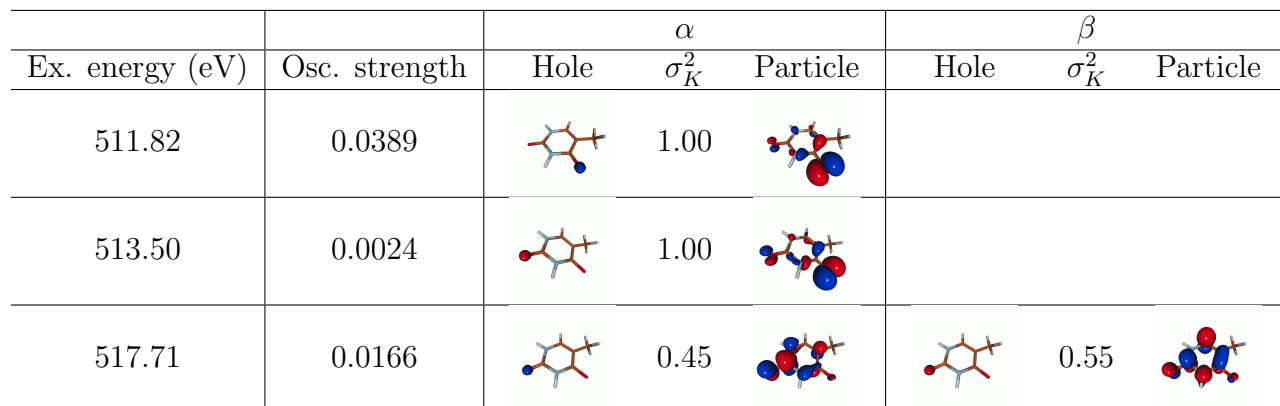 | 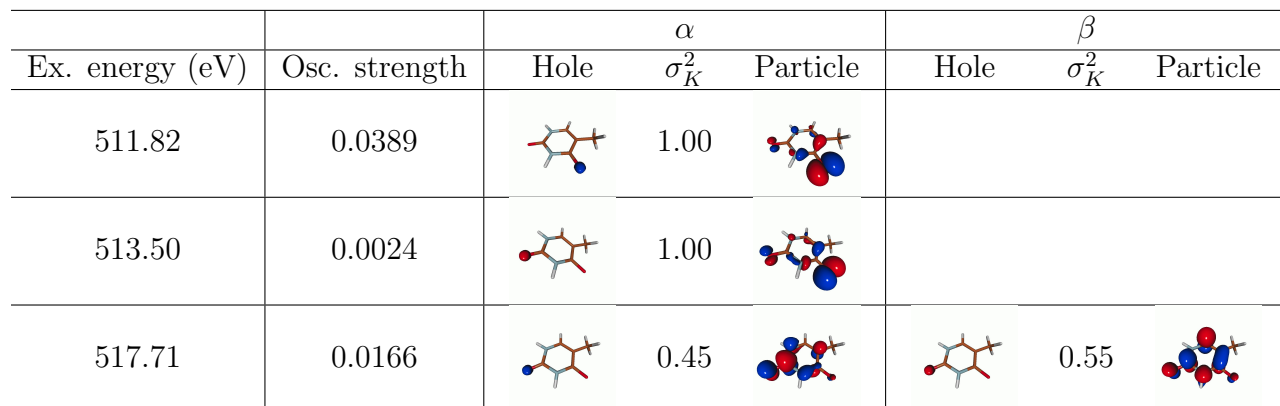 | 0.55         | 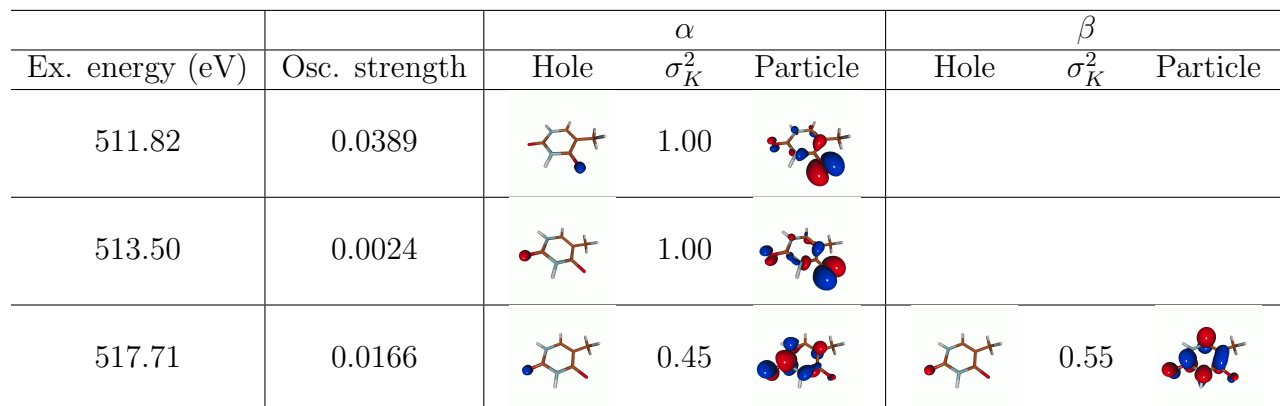 |

Table S34: Acetylacetone. MOM-TDDFT/B3LYP/6-311++G\*\* NTOs of the C<sub>1s</sub> core excitations from the T<sub>1</sub> state at the potential energy minimum (NTO isosurface is 0.05).

| Ex. energy (eV) | Osc. strength | $\alpha$ |              |          | $\beta$                                                                               |              |                                                                                       |
|-----------------|---------------|----------|--------------|----------|---------------------------------------------------------------------------------------|--------------|---------------------------------------------------------------------------------------|
|                 |               | Hole     | $\sigma_K^2$ | Particle | Hole                                                                                  | $\sigma_K^2$ | Particle                                                                              |
| 270.88          | 0.0267        |          |              |          | 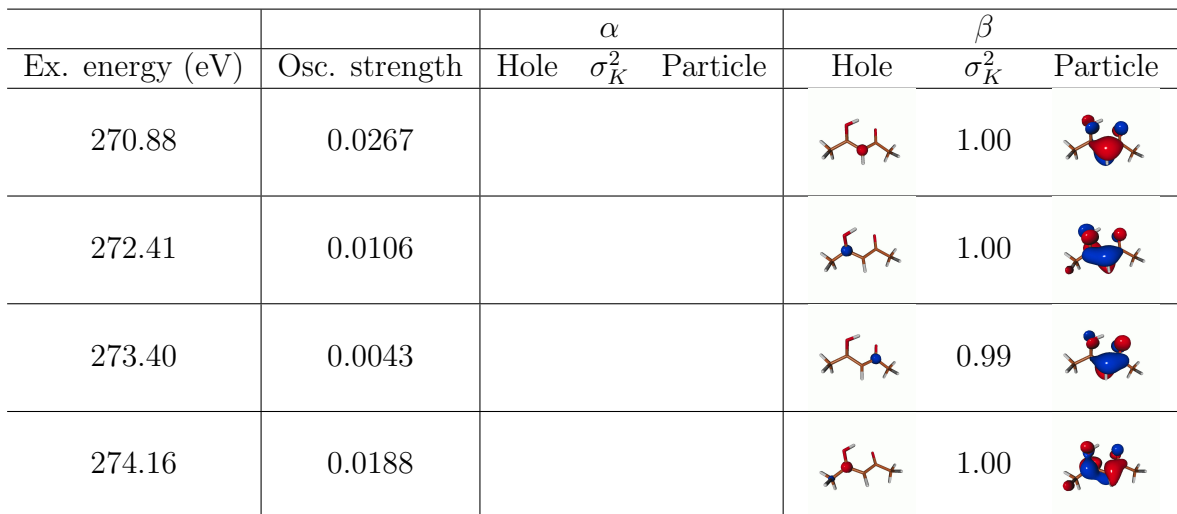 | 1.00         | 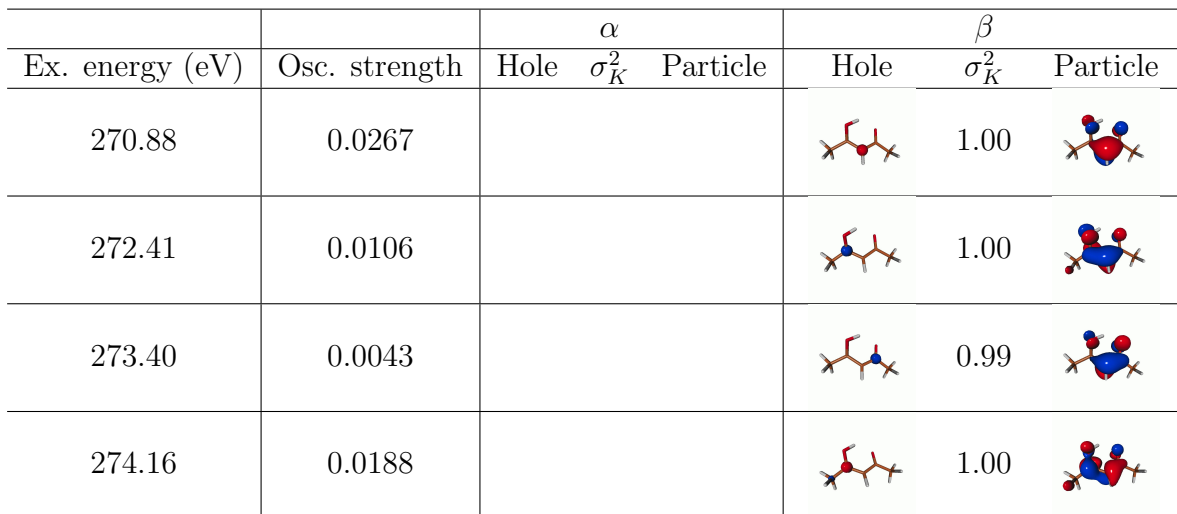 |
| 272.41          | 0.0106        |          |              |          | 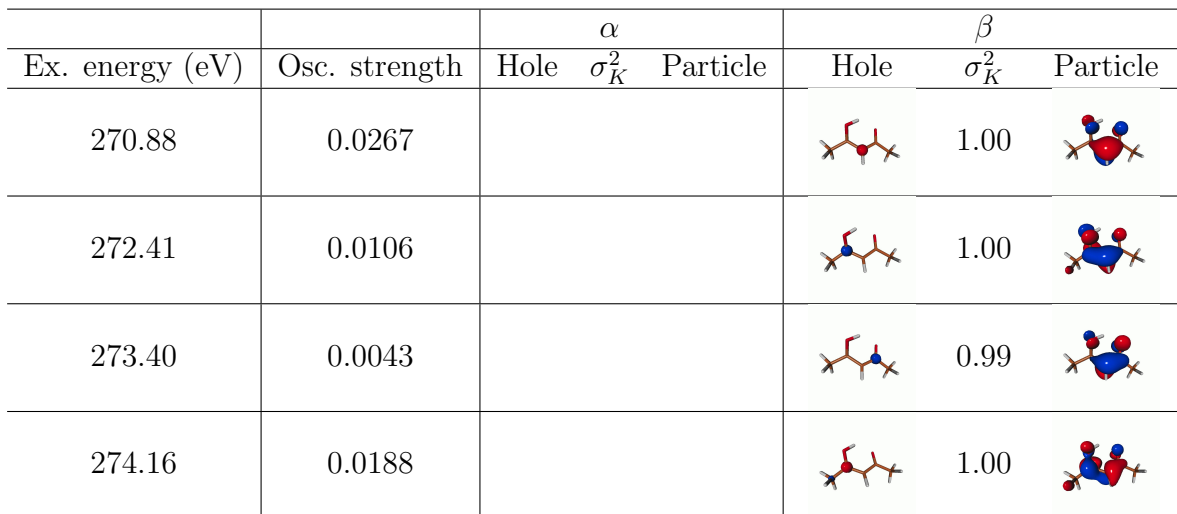 | 1.00         | 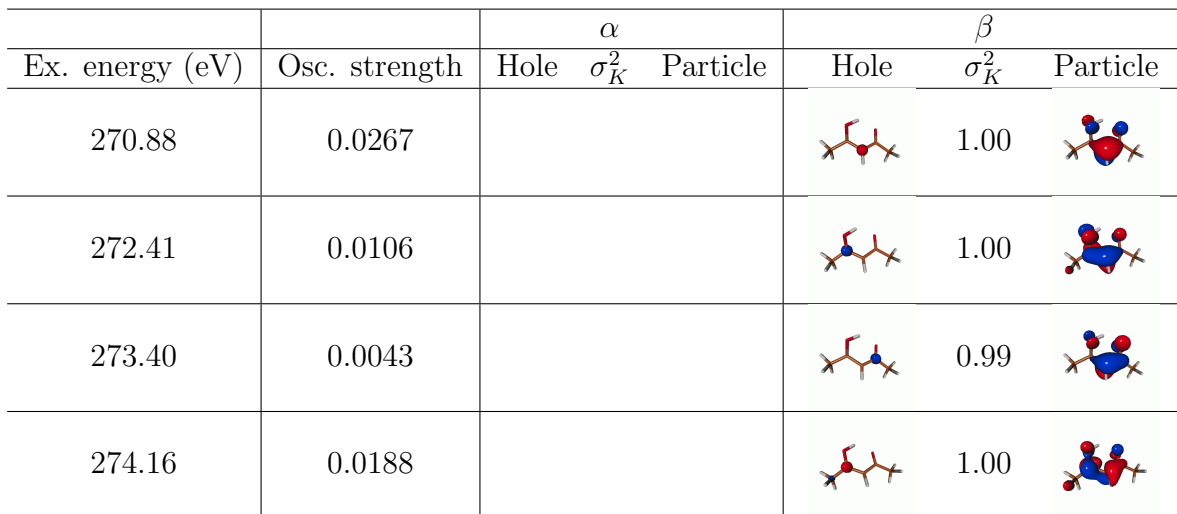 |
| 273.40          | 0.0043        |          |              |          | 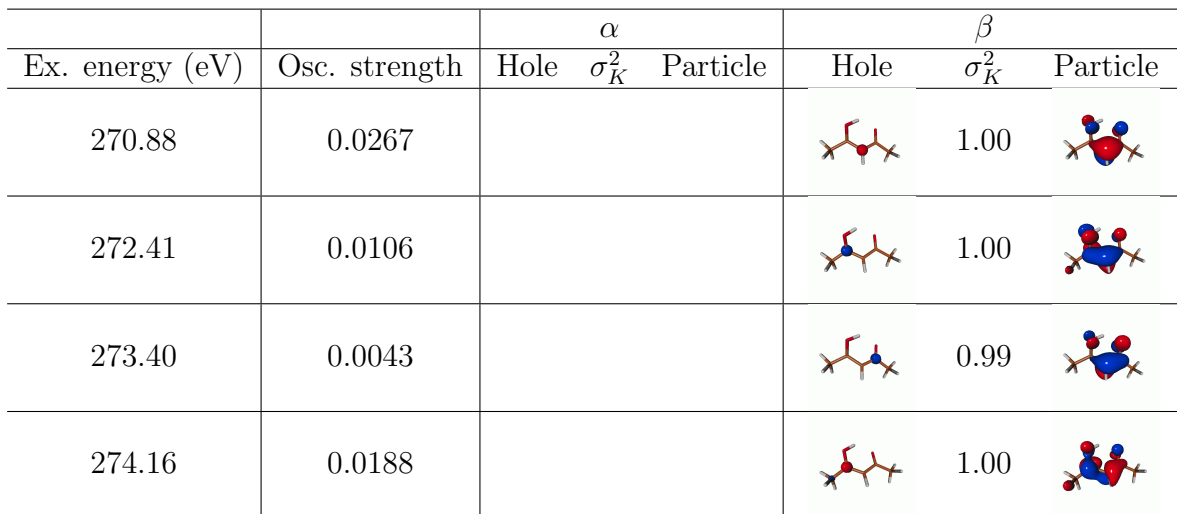 | 0.99         | 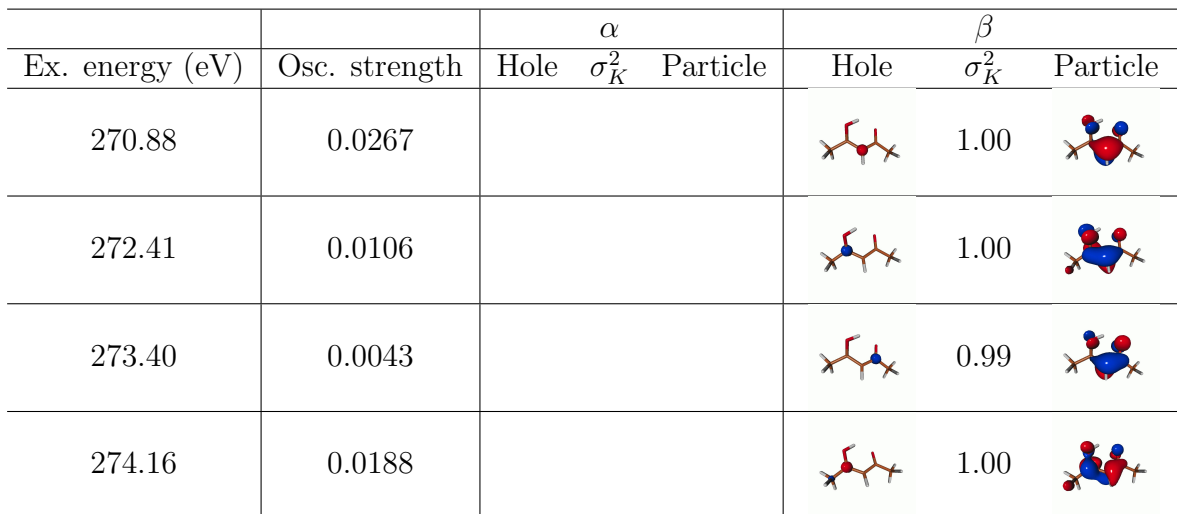 |
| 274.16          | 0.0188        |          |              |          | 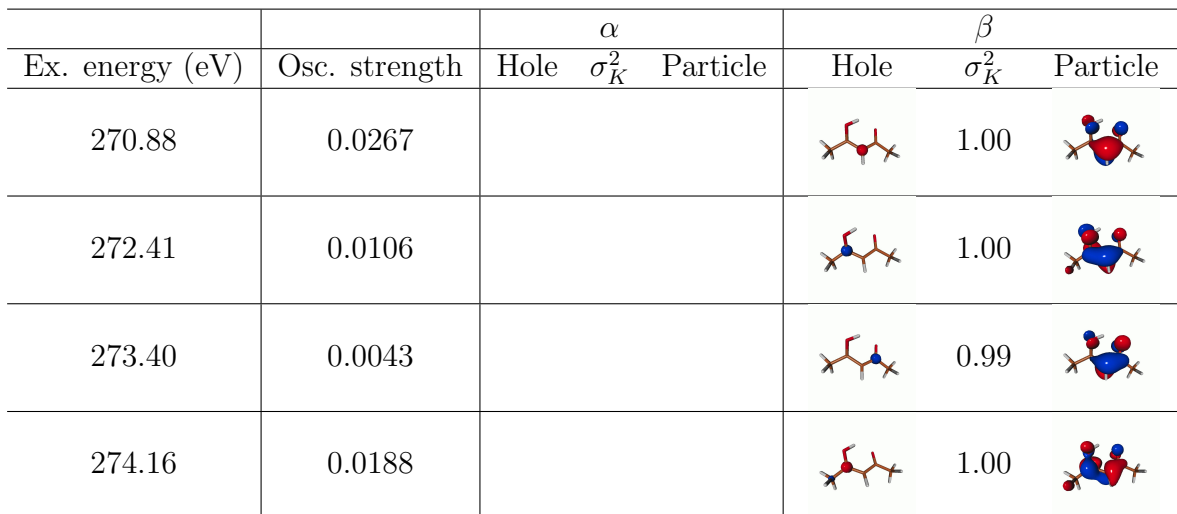 | 1.00         | 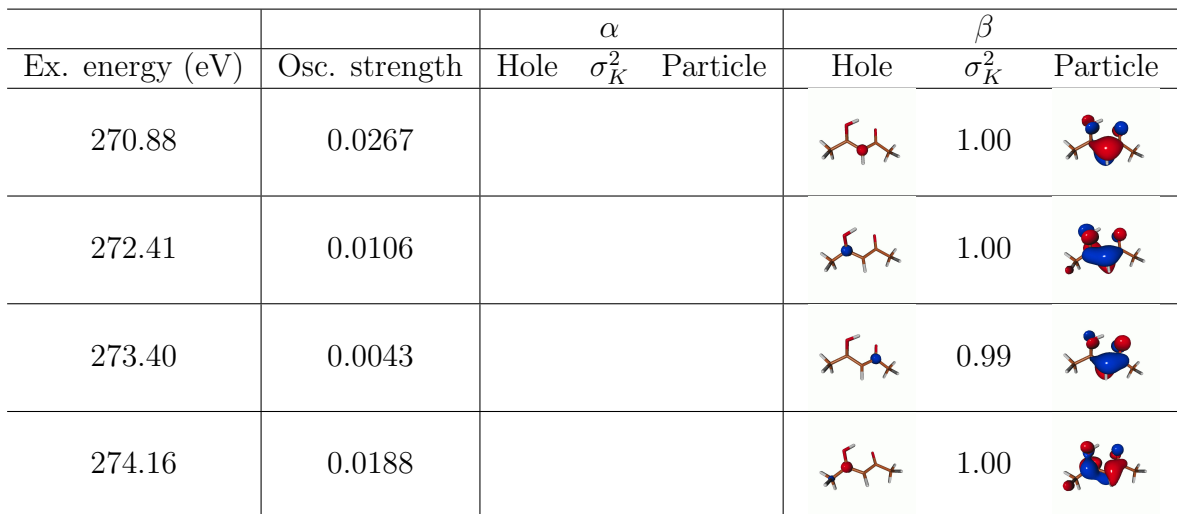 |

Table S35: Acetylacetone. MOM-TDDFT/B3LYP/6-311++G\*\* NTOs of the  $C_{1s}$  core excitations from the  $S_2$  state at the potential energy minimum of  $S_1$  (NTO isosurface is 0.05).

| Ex. energy (eV) | Osc. strength | $\alpha$                                                                            |              |                                                                                      | $\beta$                                                                               |              |                                                                                       |
|-----------------|---------------|-------------------------------------------------------------------------------------|--------------|--------------------------------------------------------------------------------------|---------------------------------------------------------------------------------------|--------------|---------------------------------------------------------------------------------------|
|                 |               | Hole                                                                                | $\sigma_K^2$ | Particle                                                                             | Hole                                                                                  | $\sigma_K^2$ | Particle                                                                              |
| 269.94          | 0.0169        | 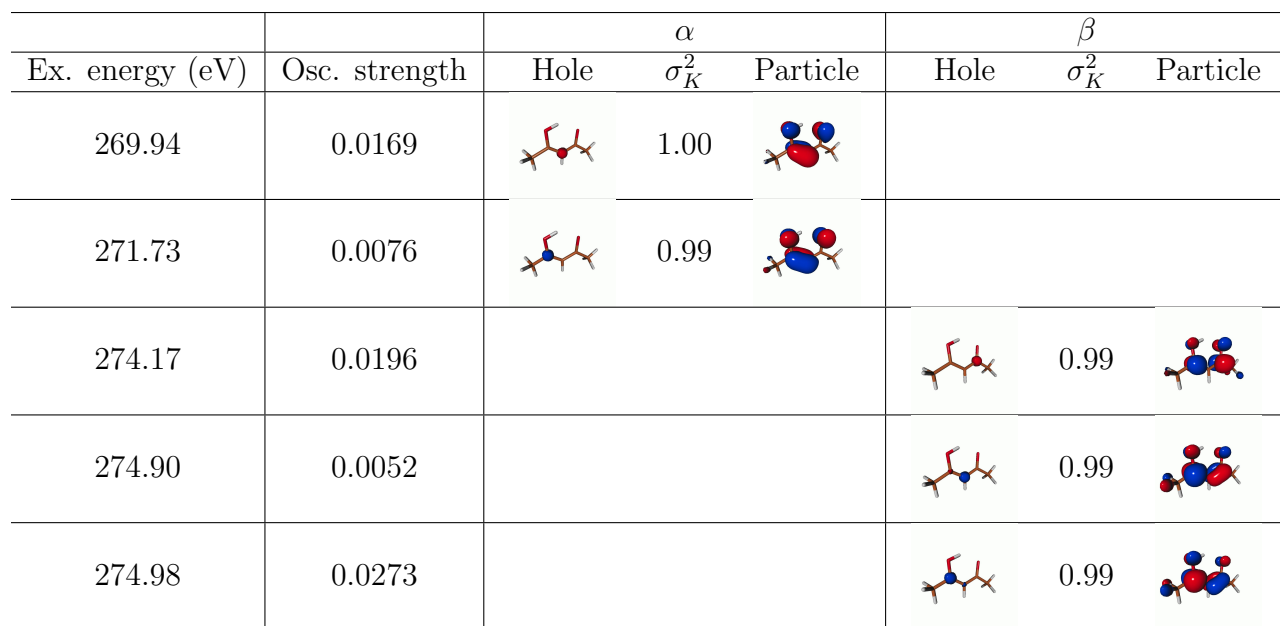   | 1.00         | 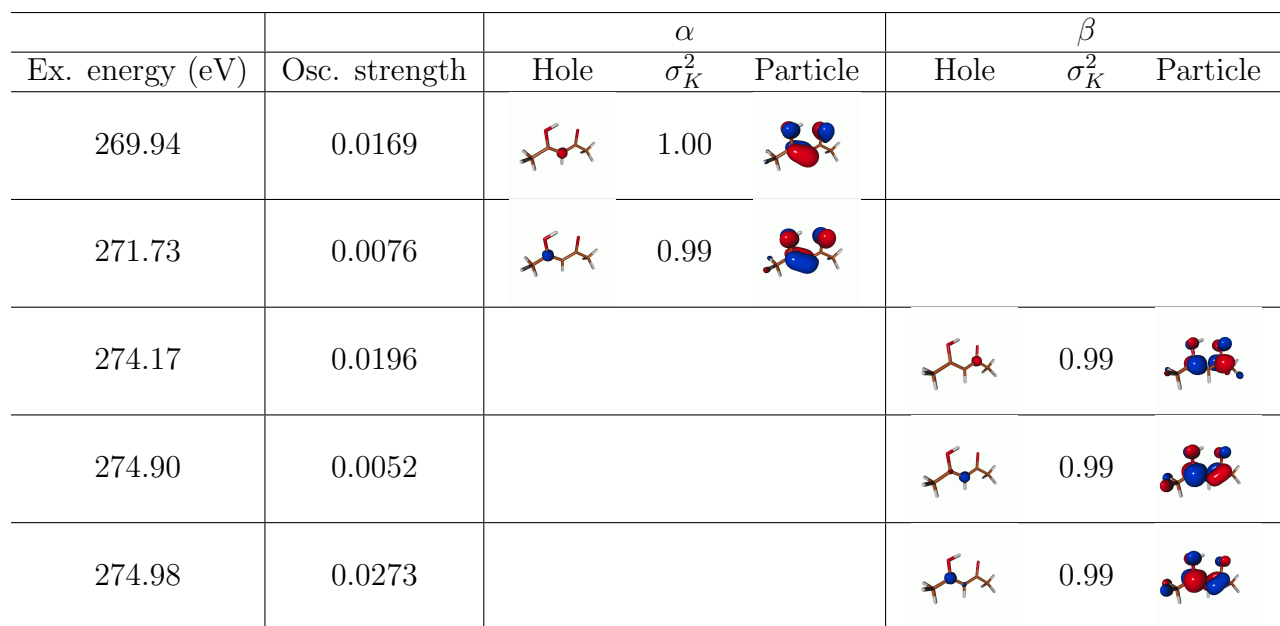   |                                                                                       |              |                                                                                       |
| 271.73          | 0.0076        | 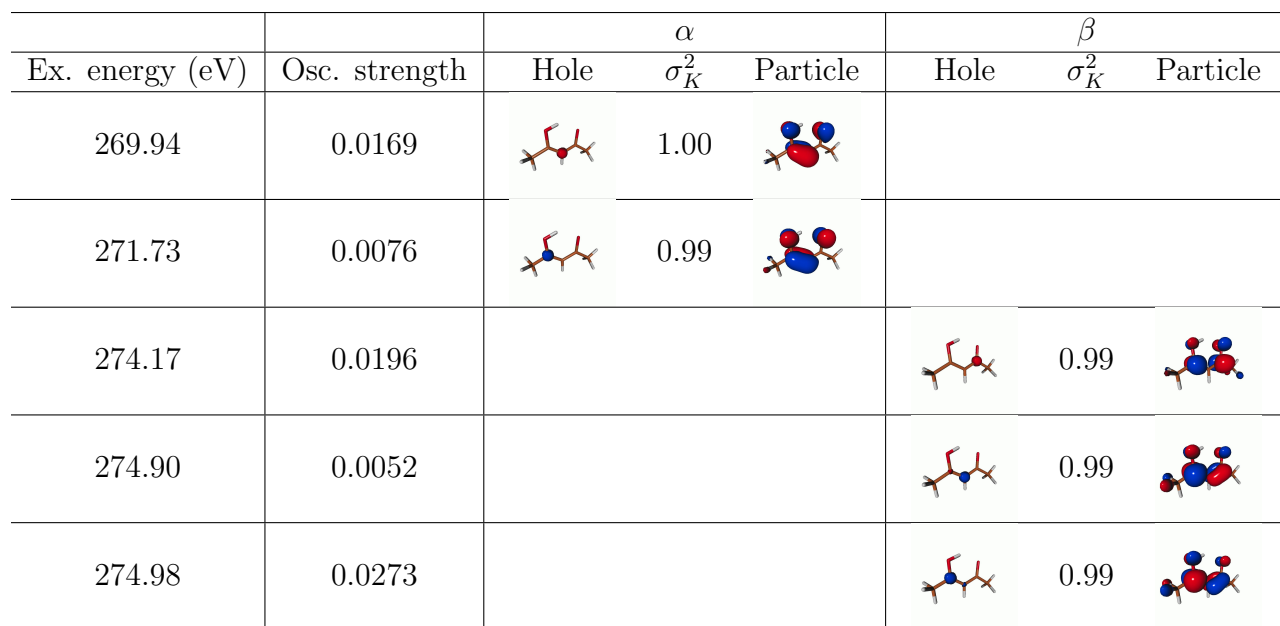 | 0.99         | 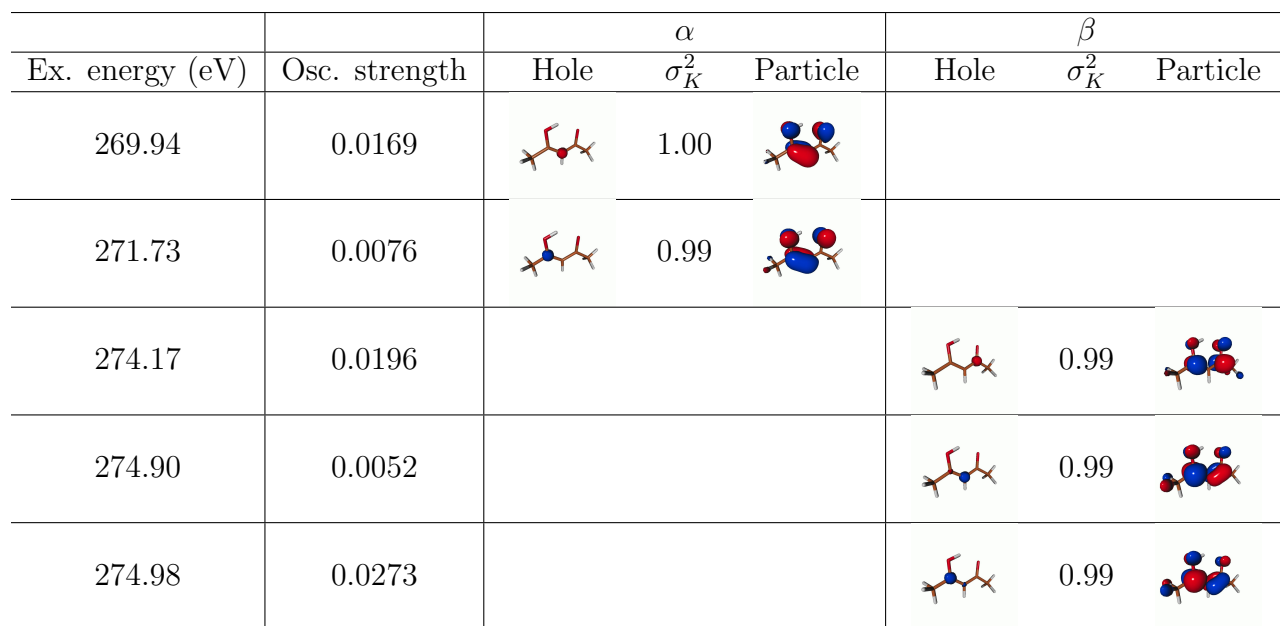 |                                                                                       |              |                                                                                       |
| 274.17          | 0.0196        |                                                                                     |              |                                                                                      | 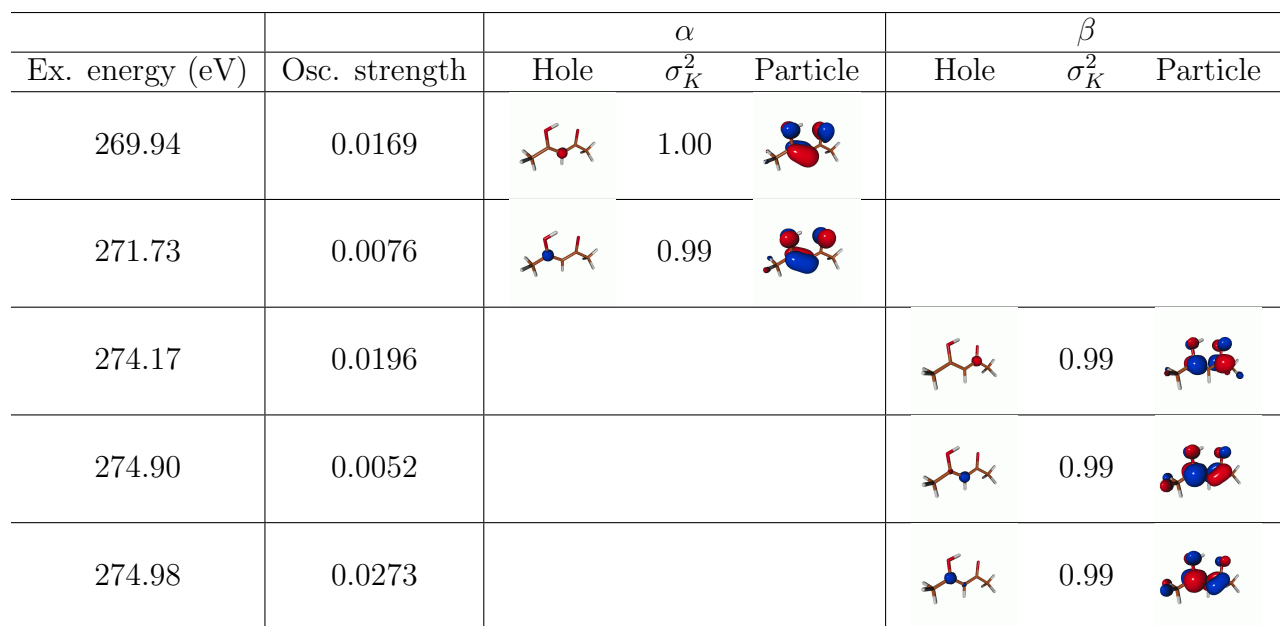 | 0.99         | 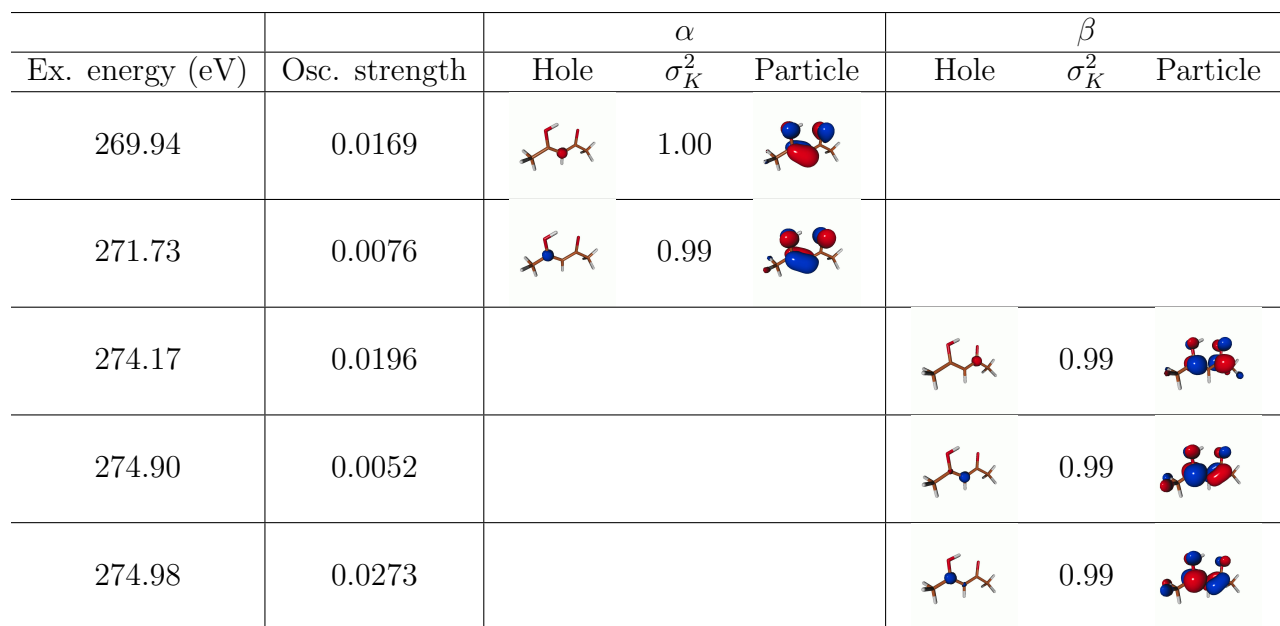 |
| 274.90          | 0.0052        |                                                                                     |              |                                                                                      | 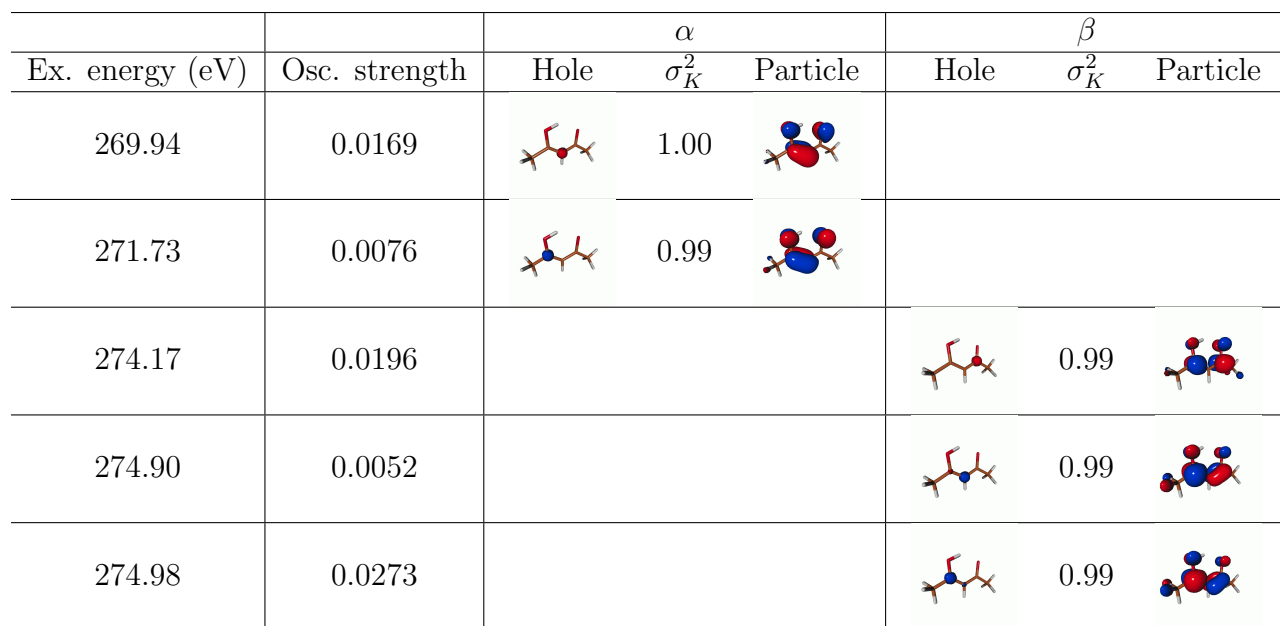 | 0.99         | 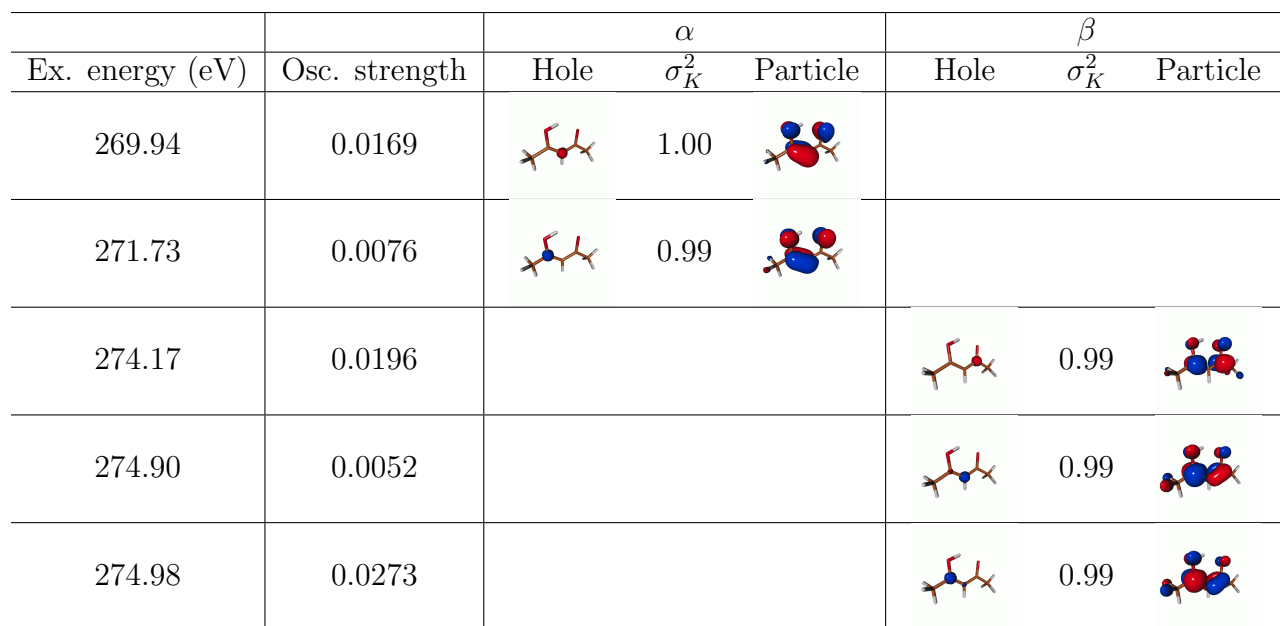 |
| 274.98          | 0.0273        |                                                                                     |              |                                                                                      | 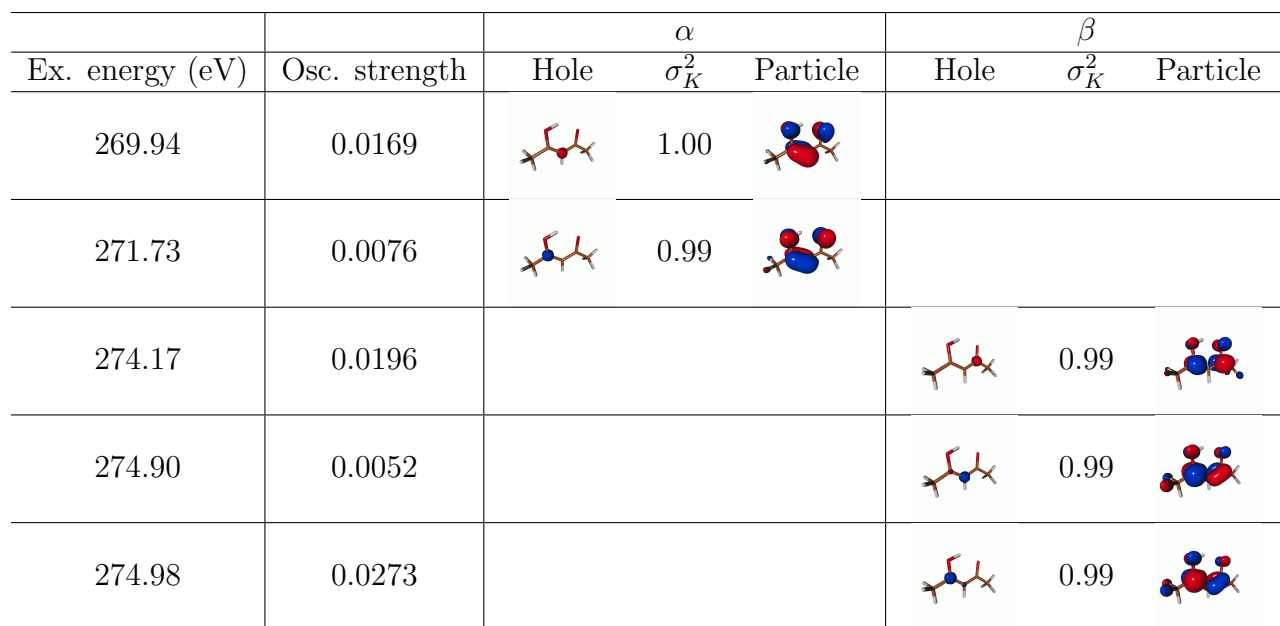 | 0.99         | 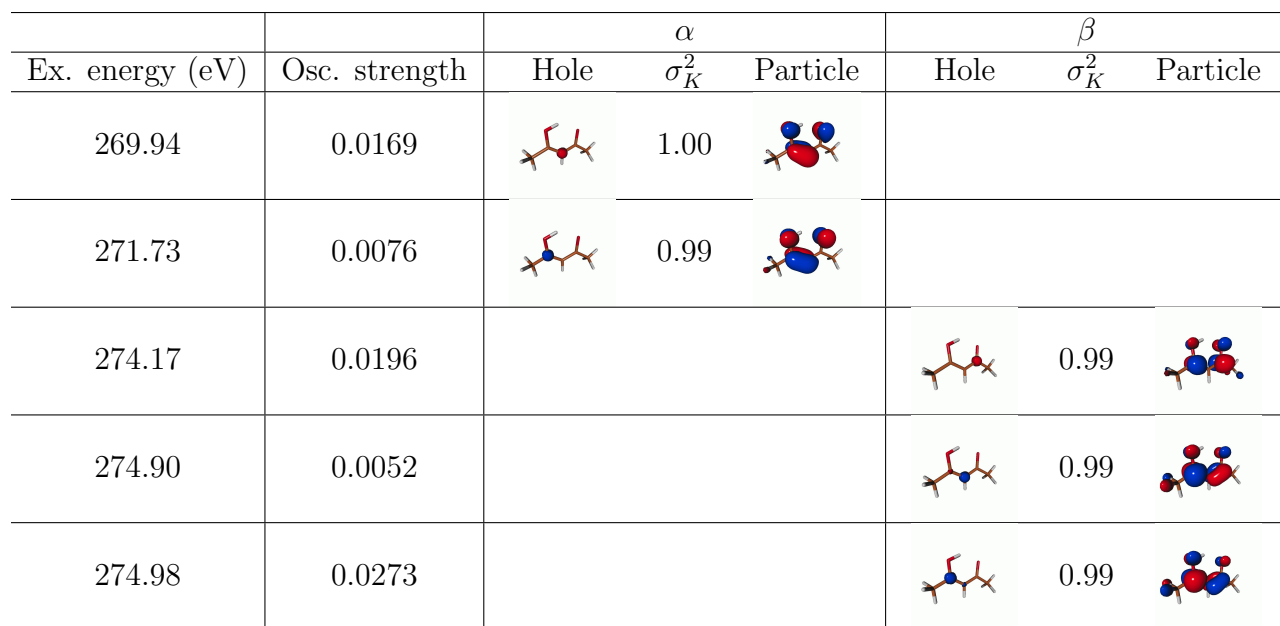 |
